# Supplementary material for: The QCD topological charge and its thermal dependence: the role of the $\eta'$
Source: arXiv:1907.11734 ancillary file (2019-11-02)
Supplement: Supplementary file 1 [file supmaterialv2.pdf]

We provide here the explicit expressions for the fourth-order cumulant  $c_4(T)$  at NLO and NNLO in the U(3) ChPT framework, including finite-temperature corrections, which arise in the NNLO contribution. We follow the same notation as in the main text,  $M_i$  being the tree-level meson masses.

$$\begin{aligned}
c_4^{\text{NLO}} = & \frac{1}{243 M_\eta^{10} M_{\eta'}^{10}} M_\theta^6 \left( 256 L_8^r M_\theta^2 M_K^6 \right. \\
& \left( M_\eta^{10} s_\theta^4 \left( 8 c_\theta^6 + 24 \sqrt{2} c_\theta^5 s_\theta + 60 c_\theta^4 s_\theta^2 + 40 \sqrt{2} c_\theta^3 s_\theta^3 + 30 c_\theta^2 s_\theta^4 + 6 \sqrt{2} c_\theta s_\theta^5 + s_\theta^6 \right) + \right. \\
& c_\theta^4 M_\eta^{10} \left( c_\theta^6 - 6 \sqrt{2} c_\theta^5 s_\theta + 30 c_\theta^4 s_\theta^2 - 40 \sqrt{2} c_\theta^3 s_\theta^3 + 60 c_\theta^2 s_\theta^4 - 24 \sqrt{2} c_\theta s_\theta^5 + 8 s_\theta^6 \right) + \\
& M_\eta^2 M_{\eta'}^8 s_\theta^3 \left( 16 \sqrt{2} c_\theta^7 + 52 c_\theta^6 s_\theta - 92 c_\theta^4 s_\theta^3 - 64 \sqrt{2} c_\theta^3 s_\theta^4 - 27 c_\theta^2 s_\theta^5 + 2 \sqrt{2} c_\theta s_\theta^6 + 2 s_\theta^7 \right) + \\
& 2 c_\theta^2 M_\eta^6 M_{\eta'}^4 s_\theta \left( 4 \sqrt{2} c_\theta^7 - 6 c_\theta^6 s_\theta - 24 \sqrt{2} c_\theta^5 s_\theta^2 + \right. \\
& \left. 49 c_\theta^4 s_\theta^3 + 18 \sqrt{2} c_\theta^3 s_\theta^4 - 48 c_\theta^2 s_\theta^5 - 4 \sqrt{2} c_\theta s_\theta^6 + 12 s_\theta^7 \right) + \\
& c_\theta^3 M_\eta^8 M_{\eta'}^2 \left( 2 c_\theta^7 - 2 \sqrt{2} c_\theta^6 s_\theta - 27 c_\theta^5 s_\theta^2 + 64 \sqrt{2} c_\theta^4 s_\theta^3 - 92 c_\theta^3 s_\theta^4 + 52 c_\theta s_\theta^6 - 16 \sqrt{2} s_\theta^7 \right) + \\
& \left. 2 c_\theta M_\eta^4 M_{\eta'}^6 s_\theta^2 \left( 12 c_\theta^7 + 4 \sqrt{2} c_\theta^6 s_\theta - 48 c_\theta^5 s_\theta^2 - 18 \sqrt{2} c_\theta^4 s_\theta^3 + \right. \right. \\
& \left. \left. 49 c_\theta^3 s_\theta^4 + 24 \sqrt{2} c_\theta^2 s_\theta^5 - 6 c_\theta s_\theta^6 - 4 \sqrt{2} s_\theta^7 \right) \right) + \\
& 8 M_K^4 \left( 2 M_\theta^2 M_\eta^{10} s_\theta^4 \left( -4 L_8^r M_\pi^2 \left( 46 c_\theta^6 + 150 \sqrt{2} c_\theta^5 s_\theta + 351 c_\theta^4 s_\theta^2 + 236 \sqrt{2} c_\theta^3 s_\theta^3 + \right. \right. \right. \\
& \left. \left. 192 c_\theta^2 s_\theta^4 + 36 \sqrt{2} c_\theta s_\theta^5 + 2 s_\theta^6 \right) + \right. \\
& F^2 s_\theta \left( 4 \sqrt{2} c_\theta^5 + 20 c_\theta^4 s_\theta + 20 \sqrt{2} c_\theta^3 s_\theta^2 + 20 c_\theta^2 s_\theta^3 + 5 \sqrt{2} c_\theta s_\theta^4 + s_\theta^5 \right) \Lambda_2 \Big) + \\
& c_\theta^3 M_\eta^{10} \left( 8 c_\theta L_8^r M_\theta^2 \left( -6 M_{\eta'}^2 \left( c_\theta^4 - 4 \sqrt{2} c_\theta^3 s_\theta + 12 c_\theta^2 s_\theta^2 - 8 \sqrt{2} c_\theta s_\theta^3 + 4 s_\theta^4 \right) + \right. \right. \\
& M_\pi^2 \left( -2 c_\theta^6 + 36 \sqrt{2} c_\theta^5 s_\theta - 192 c_\theta^4 s_\theta^2 + 236 \sqrt{2} c_\theta^3 s_\theta^3 - \right. \\
& \left. \left. 351 c_\theta^2 s_\theta^4 + 150 \sqrt{2} c_\theta s_\theta^5 - 46 s_\theta^6 \right) \right) + F^2 \left( 2 c_\theta^2 M_\theta^2 - M_{\eta'}^2 \right) \\
& \left( c_\theta^5 - 5 \sqrt{2} c_\theta^4 s_\theta + 20 c_\theta^3 s_\theta^2 - 20 \sqrt{2} c_\theta^2 s_\theta^3 + 20 c_\theta s_\theta^4 - 4 \sqrt{2} s_\theta^5 \right) \Lambda_2 \Big) + \\
& M_\eta^2 M_{\eta'}^8 s_\theta^3 \left( M_{\eta'}^2 \left( -48 L_8^r M_\theta^2 s_\theta \left( 4 c_\theta^4 + 8 \sqrt{2} c_\theta^3 s_\theta + 12 c_\theta^2 s_\theta^2 + 4 \sqrt{2} c_\theta s_\theta^3 + s_\theta^4 \right) - \right. \right. \\
& F^2 \left( 4 \sqrt{2} c_\theta^5 + 20 c_\theta^4 s_\theta + 20 \sqrt{2} c_\theta^3 s_\theta^2 + 20 c_\theta^2 s_\theta^3 + 5 \sqrt{2} c_\theta s_\theta^4 + s_\theta^5 \right) \Lambda_2 \Big) + \\
& 2 M_\theta^2 \left( -4 L_8^r M_\pi^2 \left( 101 \sqrt{2} c_\theta^7 + 305 c_\theta^6 s_\theta - 30 \sqrt{2} c_\theta^5 s_\theta^2 - 490 c_\theta^4 s_\theta^3 - \right. \right. \\
& 371 \sqrt{2} c_\theta^3 s_\theta^4 - 204 c_\theta^2 s_\theta^5 + 10 \sqrt{2} c_\theta s_\theta^6 + 16 s_\theta^7 \Big) + F^2 \left( 2 \sqrt{2} c_\theta^7 + 26 c_\theta^6 s_\theta + \right. \\
& 27 \sqrt{2} c_\theta^5 s_\theta^2 - 7 c_\theta^4 s_\theta^3 - 32 \sqrt{2} c_\theta^3 s_\theta^4 - 27 c_\theta^2 s_\theta^5 - 2 \sqrt{2} c_\theta s_\theta^6 + s_\theta^7 \Big) \Lambda_2 \Big) \Big) + \\
& c_\theta M_\eta^6 M_{\eta'}^4 s_\theta \left( -3 M_{\eta'}^2 \left( 96 c_\theta L_8^r M_\theta^2 s_\theta \left( 2 c_\theta^4 - 2 \sqrt{2} c_\theta^3 s_\theta - 3 c_\theta^2 s_\theta^2 + 2 \sqrt{2} c_\theta s_\theta^3 + 2 s_\theta^4 \right) + \right. \right. \\
& F^2 \left( 2 \sqrt{2} c_\theta^6 - 9 \sqrt{2} c_\theta^4 s_\theta^2 + 2 c_\theta^3 s_\theta^3 + 9 \sqrt{2} c_\theta^2 s_\theta^4 - 2 \sqrt{2} s_\theta^6 \right) \Lambda_2 \Big) + \\
& 2 c_\theta M_\theta^2 \left( -4 L_8^r M_\pi^2 \left( 46 \sqrt{2} c_\theta^7 - 36 c_\theta^6 s_\theta - 261 \sqrt{2} c_\theta^5 s_\theta^2 + 472 c_\theta^4 s_\theta^3 + 168 \sqrt{2} c_\theta^3 s_\theta^4 - \right. \right. \\
& 504 c_\theta^2 s_\theta^5 - 25 \sqrt{2} c_\theta s_\theta^6 + 138 s_\theta^7 \Big) + F^2 \left( 3 \sqrt{2} c_\theta^7 + 11 c_\theta^6 s_\theta - 34 \sqrt{2} c_\theta^5 s_\theta^2 - \right. \\
& 2 c_\theta^4 s_\theta^3 + 53 \sqrt{2} c_\theta^3 s_\theta^4 - 17 c_\theta^2 s_\theta^5 - 20 \sqrt{2} c_\theta s_\theta^6 + 6 s_\theta^7 \Big) \Lambda_2 \Big) \Big) + M_\eta^4 M_{\eta'}^6 s_\theta^2 \\
& \left( M_{\eta'}^2 \left( -192 c_\theta L_8^r M_\theta^2 s_\theta \left( 2 \sqrt{2} c_\theta^4 + 2 c_\theta^3 s_\theta - 3 \sqrt{2} c_\theta^2 s_\theta^2 - 5 c_\theta s_\theta^3 - \sqrt{2} s_\theta^4 \right) - F^2 \left( 12 c_\theta^6 + \right. \right. \right. \\
& 14 \sqrt{2} c_\theta^5 s_\theta - 14 c_\theta^4 s_\theta^2 - 29 \sqrt{2} c_\theta^3 s_\theta^3 - 20 c_\theta^2 s_\theta^4 + \sqrt{2} c_\theta s_\theta^5 + 2 s_\theta^6 \Big) \Lambda_2 \Big) + \\
& 2 c_\theta M_\theta^2 \left( -4 L_8^r M_\pi^2 \left( 138 c_\theta^7 + 25 \sqrt{2} c_\theta^6 s_\theta - 504 c_\theta^5 s_\theta^2 - 168 \sqrt{2} c_\theta^4 s_\theta^3 + \right. \right. \\
& 472 c_\theta^3 s_\theta^4 + 261 \sqrt{2} c_\theta^2 s_\theta^5 - 36 c_\theta s_\theta^6 - 46 \sqrt{2} s_\theta^7 \Big) + F^2 \left( 6 c_\theta^7 + 20 \sqrt{2} c_\theta^6 s_\theta - \right. \\
& \left. \left. 17 c_\theta^5 s_\theta^2 - 53 \sqrt{2} c_\theta^4 s_\theta^3 - 2 c_\theta^3 s_\theta^4 + 34 \sqrt{2} c_\theta^2 s_\theta^5 + 11 c_\theta s_\theta^6 - 3 \sqrt{2} s_\theta^7 \right) \Lambda_2 \Big) \right) +
\end{aligned}$$

$$\begin{aligned}
& c_\theta^2 M_\eta^8 M_{\eta'}^2 \left( M_{\eta'}^2 \left( -192 c_\theta L_8^r M_0^2 s_\theta \left( \sqrt{2} c_\theta^4 - 5 c_\theta^3 s_\theta + 3 \sqrt{2} c_\theta^2 s_\theta^2 + 2 c_\theta s_\theta^3 - 2 \sqrt{2} s_\theta^4 \right) + \right. \right. \\
& \quad F^2 \left( -2 c_\theta^6 + \sqrt{2} c_\theta^5 s_\theta + 20 c_\theta^4 s_\theta^2 - 29 \sqrt{2} c_\theta^3 s_\theta^3 + 14 c_\theta^2 s_\theta^4 + 14 \sqrt{2} c_\theta s_\theta^5 - 12 s_\theta^6 \right) \\
& \quad \left. \Lambda_2 \right) + 2 c_\theta M_0^2 \left( -4 L_8^r M_\pi^2 \left( 16 c_\theta^7 - 10 \sqrt{2} c_\theta^6 s_\theta - 204 c_\theta^5 s_\theta^2 + 371 \sqrt{2} c_\theta^4 s_\theta^3 - \right. \right. \\
& \quad 490 c_\theta^3 s_\theta^4 + 30 \sqrt{2} c_\theta^2 s_\theta^5 + 305 c_\theta s_\theta^6 - 101 \sqrt{2} s_\theta^7 \Big) + F^2 \left( c_\theta^7 + 2 \sqrt{2} c_\theta^6 s_\theta - \right. \\
& \quad 27 c_\theta^5 s_\theta^2 + 32 \sqrt{2} c_\theta^4 s_\theta^3 - 7 c_\theta^3 s_\theta^4 - 27 \sqrt{2} c_\theta^2 s_\theta^5 + 26 c_\theta s_\theta^6 - 2 \sqrt{2} s_\theta^7 \Big) \Lambda_2 \Big) \Big) + \\
& 2 M_K^2 \left( 2 M_0^2 M_\pi^2 M_{\eta'}^{10} s_\theta^4 \left( 16 L_8^r M_\pi^2 \left( 26 c_\theta^6 + 78 \sqrt{2} c_\theta^5 s_\theta + 159 c_\theta^4 s_\theta^2 + 112 \sqrt{2} c_\theta^3 s_\theta^3 + \right. \right. \right. \\
& \quad 111 c_\theta^2 s_\theta^4 + 24 \sqrt{2} c_\theta s_\theta^5 + s_\theta^6 \Big) + \\
& \quad F^2 s_\theta \left( -23 \sqrt{2} c_\theta^5 - 103 c_\theta^4 s_\theta - 64 \sqrt{2} c_\theta^3 s_\theta^2 - 52 c_\theta^2 s_\theta^3 - 10 \sqrt{2} c_\theta s_\theta^4 + 4 s_\theta^5 \right) \Lambda_2 \Big) + \\
& c_\theta^3 M_\eta^{10} \left( 6 F^2 M_{\eta'}^4 \left( c_\theta^3 - 3 \sqrt{2} c_\theta^2 s_\theta + 6 c_\theta s_\theta^2 - 2 \sqrt{2} s_\theta^3 \right) \Lambda_2 + 2 c_\theta M_0^2 M_\pi^2 \left( 16 L_8^r M_\pi^2 \left( c_\theta^6 - \right. \right. \right. \\
& \quad 24 \sqrt{2} c_\theta^5 s_\theta + 111 c_\theta^4 s_\theta^2 - 112 \sqrt{2} c_\theta^3 s_\theta^3 + 159 c_\theta^2 s_\theta^4 - 78 \sqrt{2} c_\theta s_\theta^5 + 26 s_\theta^6 \Big) + \\
& \quad F^2 c_\theta \left( 4 c_\theta^5 + 10 \sqrt{2} c_\theta^4 s_\theta - 52 c_\theta^3 s_\theta^2 + 64 \sqrt{2} c_\theta^2 s_\theta^3 - 103 c_\theta s_\theta^4 + 23 \sqrt{2} s_\theta^5 \right) \Lambda_2 \Big) + \\
& M_{\eta'}^2 \left( 192 c_\theta L_8^r M_0^2 M_\pi^2 \left( c_\theta^4 - 4 \sqrt{2} c_\theta^3 s_\theta + 12 c_\theta^2 s_\theta^2 - 8 \sqrt{2} c_\theta s_\theta^3 + 4 s_\theta^4 \right) - \right. \\
& \quad F^2 \left( 6 c_\theta^2 M_0^2 \left( c_\theta^3 - 3 \sqrt{2} c_\theta^2 s_\theta + 6 c_\theta s_\theta^2 - 2 \sqrt{2} s_\theta^3 \right) + M_\pi^2 \left( 4 c_\theta^5 + 10 \sqrt{2} c_\theta^4 s_\theta - \right. \right. \\
& \quad \left. \left. 52 c_\theta^3 s_\theta^2 + 64 \sqrt{2} c_\theta^2 s_\theta^3 - 103 c_\theta s_\theta^4 + 23 \sqrt{2} s_\theta^5 \right) \right) \Lambda_2 \Big) + M_\eta^2 M_{\eta'}^8 s_\theta^3 \\
& \left( M_0^2 M_\pi^2 \left( 32 L_8^r M_\pi^2 \left( 55 \sqrt{2} c_\theta^7 + 115 c_\theta^6 s_\theta - 39 \sqrt{2} c_\theta^5 s_\theta^2 - 149 c_\theta^4 s_\theta^3 - 151 \sqrt{2} c_\theta^3 s_\theta^4 - \right. \right. \right. \\
& \quad 141 c_\theta^2 s_\theta^5 - 7 \sqrt{2} c_\theta s_\theta^6 + 8 s_\theta^7 \Big) - F^2 \left( 23 \sqrt{2} c_\theta^7 + 284 c_\theta^6 s_\theta + 102 \sqrt{2} c_\theta^5 s_\theta^2 - \right. \\
& \quad 340 c_\theta^4 s_\theta^3 - 221 \sqrt{2} c_\theta^3 s_\theta^4 - 138 c_\theta^2 s_\theta^5 + 10 \sqrt{2} c_\theta s_\theta^6 + 16 s_\theta^7 \Big) \Lambda_2 \Big) + \\
& M_{\eta'}^2 \left( -6 F^2 M_0^2 s_\theta^2 \left( 2 \sqrt{2} c_\theta^3 + 6 c_\theta^2 s_\theta + 3 \sqrt{2} c_\theta s_\theta^2 + s_\theta^3 \right) \Lambda_2 + \right. \\
& \quad M_\pi^2 \left( 192 L_8^r M_0^2 s_\theta \left( 4 c_\theta^4 + 8 \sqrt{2} c_\theta^3 s_\theta + 12 c_\theta^2 s_\theta^2 + 4 \sqrt{2} c_\theta s_\theta^3 + s_\theta^4 \right) + F^2 \left( 23 \sqrt{2} \right. \right. \\
& \quad \left. \left. c_\theta^5 + 103 c_\theta^4 s_\theta + 64 \sqrt{2} c_\theta^3 s_\theta^2 + 52 c_\theta^2 s_\theta^3 + 10 \sqrt{2} c_\theta s_\theta^4 - 4 s_\theta^5 \right) \Lambda_2 \right) \Big) \Big) + \\
& M_\eta^4 M_{\eta'}^6 s_\theta^2 \left( 32 c_\theta L_8^r M_0^2 M_\pi^4 \left( 60 c_\theta^7 - 19 \sqrt{2} c_\theta^6 s_\theta - 123 c_\theta^5 s_\theta^2 - 27 \sqrt{2} c_\theta^4 s_\theta^3 + \right. \right. \\
& \quad 62 c_\theta^3 s_\theta^4 + 75 \sqrt{2} c_\theta^2 s_\theta^5 + 15 c_\theta s_\theta^6 - 17 \sqrt{2} s_\theta^7 \Big) + \\
& \quad 6 F^2 M_{\eta'}^2 s_\theta \left( M_{\eta'}^2 \left( 2 \sqrt{2} c_\theta^3 + 6 c_\theta^2 s_\theta + 3 \sqrt{2} c_\theta s_\theta^2 + s_\theta^3 \right) + \right. \\
& \quad \left. c_\theta M_0^2 \left( -2 \sqrt{2} c_\theta^4 - 12 c_\theta^3 s_\theta - 3 \sqrt{2} c_\theta^2 s_\theta^2 + 8 c_\theta s_\theta^3 + 3 \sqrt{2} s_\theta^4 \right) \right) \Lambda_2 + \\
& M_\pi^2 \left( F^2 c_\theta M_0^2 \left( -78 c_\theta^7 - 119 \sqrt{2} c_\theta^6 s_\theta + 464 c_\theta^5 s_\theta^2 + 236 \sqrt{2} c_\theta^4 s_\theta^3 - 394 c_\theta^3 s_\theta^4 - \right. \right. \\
& \quad 235 \sqrt{2} c_\theta^2 s_\theta^5 + 4 c_\theta s_\theta^6 + 30 \sqrt{2} s_\theta^7 \Big) \Lambda_2 + M_{\eta'}^2 \left( 768 c_\theta L_8^r M_0^2 s_\theta \right. \\
& \quad \left( 2 \sqrt{2} c_\theta^4 + 2 c_\theta^3 s_\theta - 3 \sqrt{2} c_\theta^2 s_\theta^2 - 5 c_\theta s_\theta^3 - \sqrt{2} s_\theta^4 \right) + F^2 \left( 78 c_\theta^6 + 25 \sqrt{2} c_\theta^5 \right. \\
& \quad \left. s_\theta - 136 c_\theta^4 s_\theta^2 - 79 \sqrt{2} c_\theta^3 s_\theta^3 - 10 c_\theta^2 s_\theta^4 + 20 \sqrt{2} c_\theta s_\theta^5 + 16 s_\theta^6 \right) \Lambda_2 \Big) \Big) \Big) + \\
& c_\theta^2 M_\eta^8 M_{\eta'}^2 \left( c_\theta M_0^2 M_\pi^2 \left( 32 L_8^r M_\pi^2 \left( 8 c_\theta^7 + 7 \sqrt{2} c_\theta^6 s_\theta - 141 c_\theta^5 s_\theta^2 + 151 \sqrt{2} c_\theta^4 s_\theta^3 - \right. \right. \right. \\
& \quad 149 c_\theta^3 s_\theta^4 + 39 \sqrt{2} c_\theta^2 s_\theta^5 + 115 c_\theta s_\theta^6 - 55 \sqrt{2} s_\theta^7 \Big) + \\
& \quad F^2 \left( -16 c_\theta^7 + 10 \sqrt{2} c_\theta^6 s_\theta + 138 c_\theta^5 s_\theta^2 - 221 \sqrt{2} c_\theta^4 s_\theta^3 + 340 c_\theta^3 s_\theta^4 + \right. \\
& \quad \left. 102 \sqrt{2} c_\theta^2 s_\theta^5 - 284 c_\theta s_\theta^6 + 23 \sqrt{2} s_\theta^7 \right) \Lambda_2 \Big) + \\
& M_{\eta'}^2 \left( 6 F^2 c_\theta M_0^2 s_\theta \left( -3 \sqrt{2} c_\theta^4 + 8 c_\theta^3 s_\theta + 3 \sqrt{2} c_\theta^2 s_\theta^2 - 12 c_\theta s_\theta^3 + 2 \sqrt{2} s_\theta^4 \right) \Lambda_2 + \right. \\
& \quad M_\pi^2 \left( 768 c_\theta L_8^r M_0^2 s_\theta \left( \sqrt{2} c_\theta^4 - 5 c_\theta^3 s_\theta + 3 \sqrt{2} c_\theta^2 s_\theta^2 + 2 c_\theta s_\theta^3 - 2 \sqrt{2} s_\theta^4 \right) + \right.
\end{aligned}$$

$$\begin{aligned}
& F^2 \left( 16 c_\theta^6 - 20 \sqrt{2} c_\theta^5 s_\theta - 10 c_\theta^4 s_\theta^2 + 79 \sqrt{2} c_\theta^3 s_\theta^3 - \right. \\
& \quad \left. 136 c_\theta^2 s_\theta^4 - 25 \sqrt{2} c_\theta s_\theta^5 + 78 s_\theta^6 \right) \Lambda_2 \Big) + c_\theta M_\eta^6 M_\eta^4 s_\theta \\
& \left( c_\theta M_\theta^2 M_\pi^2 \left( 32 L_8^r M_\pi^2 \left( 17 \sqrt{2} c_\theta^7 + 15 c_\theta^6 s_\theta - 75 \sqrt{2} c_\theta^5 s_\theta^2 + 62 c_\theta^4 s_\theta^3 + 27 \sqrt{2} c_\theta^3 s_\theta^4 - \right. \right. \right. \\
& \quad \left. \left. 123 c_\theta^2 s_\theta^5 + 19 \sqrt{2} c_\theta s_\theta^6 + 60 s_\theta^7 \right) + F^2 \left( -30 \sqrt{2} c_\theta^7 + 4 c_\theta^6 s_\theta + 235 \sqrt{2} c_\theta^5 s_\theta^2 - \right. \right. \\
& \quad \left. \left. 394 c_\theta^4 s_\theta^3 - 236 \sqrt{2} c_\theta^3 s_\theta^4 + 464 c_\theta^2 s_\theta^5 + 119 \sqrt{2} c_\theta s_\theta^6 - 78 s_\theta^7 \right) \Lambda_2 \right) + \\
& \quad 3 M_\eta^2 \left( -6 F^2 c_\theta M_\theta^2 s_\theta \left( 2 c_\theta^4 + \sqrt{2} c_\theta^3 s_\theta - 6 c_\theta^2 s_\theta^2 - \sqrt{2} c_\theta s_\theta^3 + 2 s_\theta^4 \right) \Lambda_2 + \right. \\
& \quad \left. M_\pi^2 \left( 384 c_\theta L_8^r M_\theta^2 s_\theta \left( 2 c_\theta^4 - 2 \sqrt{2} c_\theta^3 s_\theta - 3 c_\theta^2 s_\theta^2 + 2 \sqrt{2} c_\theta s_\theta^3 + 2 s_\theta^4 \right) + \right. \right. \\
& \quad \left. \left. F^2 \left( 10 \sqrt{2} c_\theta^6 - 24 c_\theta^5 s_\theta - 21 \sqrt{2} c_\theta^4 s_\theta^2 + 46 c_\theta^3 s_\theta^3 + \right. \right. \right. \\
& \quad \left. \left. \left. 21 \sqrt{2} c_\theta^2 s_\theta^4 - 24 c_\theta s_\theta^5 - 10 \sqrt{2} s_\theta^6 \right) \Lambda_2 \right) \right) \Big) + \\
& M_\pi^2 \left( 2 M_\theta^2 M_\pi^2 M_\eta^{10} s_\theta^4 \left( -24 L_8^r M_\pi^2 \left( c_\theta^2 + s_\theta^2 \right) \left( 7 c_\theta^4 + 20 \sqrt{2} c_\theta^3 s_\theta + 12 c_\theta^2 s_\theta^2 + 16 \sqrt{2} c_\theta s_\theta^3 - 2 s_\theta^4 \right) + \right. \right. \\
& \quad \left. \left. F^2 s_\theta \left( 14 \sqrt{2} c_\theta^5 + 73 c_\theta^4 s_\theta + 4 \sqrt{2} c_\theta^3 s_\theta^2 + 52 c_\theta^2 s_\theta^3 - 20 \sqrt{2} c_\theta s_\theta^4 + 2 s_\theta^5 \right) \Lambda_2 \right) + \right. \\
& \quad \left. c_\theta^3 M_\eta^{10} \left( 48 c_\theta L_8^r M_\theta^2 M_\pi^4 \left( c_\theta^2 + s_\theta^2 \right) \left( 2 c_\theta^4 + 16 \sqrt{2} c_\theta^3 s_\theta - 12 c_\theta^2 s_\theta^2 + 20 \sqrt{2} c_\theta s_\theta^3 - 7 s_\theta^4 \right) - \right. \right. \\
& \quad \left. \left. 3 F^2 M_\eta^2 \left( c_\theta^2 M_\theta^2 - M_\eta^2 \right) \left( 2 c_\theta^3 + 12 \sqrt{2} c_\theta^2 s_\theta - 6 c_\theta s_\theta^2 + 5 \sqrt{2} s_\theta^3 \right) \Lambda_2 + \right. \right. \\
& \quad \left. \left. M_\pi^2 \left( -144 c_\theta L_8^r M_\theta^2 M_\eta^2 \left( 2 c_\theta^4 + 12 c_\theta^2 s_\theta^2 - 4 \sqrt{2} c_\theta s_\theta^3 + 3 s_\theta^4 \right) + F^2 \left( 2 c_\theta^2 M_\theta^2 - M_\eta^2 \right) \right. \right. \right. \\
& \quad \left. \left. \left. \left( 2 c_\theta^5 + 20 \sqrt{2} c_\theta^4 s_\theta + 52 c_\theta^3 s_\theta^2 - 4 \sqrt{2} c_\theta^2 s_\theta^3 + 73 c_\theta s_\theta^4 - 14 \sqrt{2} s_\theta^5 \right) \Lambda_2 \right) \right) \right) + \\
& M_\eta^2 M_\eta^8 s_\theta^3 \left( 2 M_\theta^2 M_\pi^2 \left( 72 c_\theta L_8^r M_\pi^2 \left( c_\theta^2 + s_\theta^2 \right) \left( -5 \sqrt{2} c_\theta^4 + c_\theta^3 s_\theta + 3 \sqrt{2} c_\theta^2 s_\theta^2 + \right. \right. \right. \\
& \quad \left. \left. 8 c_\theta s_\theta^3 + 4 \sqrt{2} s_\theta^4 \right) + F^2 \left( 7 \sqrt{2} c_\theta^7 + 103 c_\theta^6 s_\theta - 42 \sqrt{2} c_\theta^5 s_\theta^2 - \right. \right. \\
& \quad \left. \left. 68 c_\theta^4 s_\theta^3 - 73 \sqrt{2} c_\theta^3 s_\theta^4 - 48 c_\theta^2 s_\theta^5 + 26 \sqrt{2} c_\theta s_\theta^6 + 8 s_\theta^7 \right) \Lambda_2 \right) - \\
& M_\eta^2 \left( -3 F^2 M_\theta^2 s_\theta^2 \left( 5 \sqrt{2} c_\theta^3 + 6 c_\theta^2 s_\theta + 12 \sqrt{2} c_\theta s_\theta^2 - 2 s_\theta^3 \right) \Lambda_2 + \right. \\
& \quad \left. M_\pi^2 \left( 144 L_8^r M_\theta^2 s_\theta \left( 3 c_\theta^4 + 4 \sqrt{2} c_\theta^3 s_\theta + 12 c_\theta^2 s_\theta^2 + 2 s_\theta^4 \right) + F^2 \right. \right. \\
& \quad \left. \left. \left( 14 \sqrt{2} c_\theta^5 + 73 c_\theta^4 s_\theta + 4 \sqrt{2} c_\theta^3 s_\theta^2 + 52 c_\theta^2 s_\theta^3 - 20 \sqrt{2} c_\theta s_\theta^4 + 2 s_\theta^5 \right) \Lambda_2 \right) \right) \Big) + \\
& c_\theta^2 M_\eta^8 M_\eta^2 \left( 2 M_\theta^2 M_\pi^2 \left( 72 c_\theta L_8^r M_\pi^2 s_\theta \left( c_\theta^2 + s_\theta^2 \right) \left( -4 \sqrt{2} c_\theta^4 + 8 c_\theta^3 s_\theta - 3 \sqrt{2} c_\theta^2 s_\theta^2 + \right. \right. \right. \\
& \quad \left. \left. c_\theta s_\theta^3 + 5 \sqrt{2} s_\theta^4 \right) + F^2 c_\theta \left( 8 c_\theta^7 - 26 \sqrt{2} c_\theta^6 s_\theta - 48 c_\theta^5 s_\theta^2 + \right. \right. \\
& \quad \left. \left. 73 \sqrt{2} c_\theta^4 s_\theta^3 - 68 c_\theta^3 s_\theta^4 + 42 \sqrt{2} c_\theta^2 s_\theta^5 + 103 c_\theta s_\theta^6 - 7 \sqrt{2} s_\theta^7 \right) \Lambda_2 \right) + \\
& M_\eta^2 \left( 3 F^2 c_\theta M_\theta^2 s_\theta \left( 12 \sqrt{2} c_\theta^4 - 20 c_\theta^3 s_\theta - 21 \sqrt{2} c_\theta^2 s_\theta^2 + 12 c_\theta s_\theta^3 - 5 \sqrt{2} s_\theta^4 \right) \Lambda_2 + \right. \\
& \quad \left. 2 M_\pi^2 \left( 288 c_\theta L_8^r M_\theta^2 s_\theta^2 \left( 4 c_\theta^3 - 3 \sqrt{2} c_\theta^2 s_\theta - 3 c_\theta s_\theta^2 + \sqrt{2} s_\theta^3 \right) + F^2 \left( -8 c_\theta^6 + 16 \sqrt{2} \right. \right. \right. \\
& \quad \left. \left. \left. c_\theta^5 s_\theta + 2 c_\theta^4 s_\theta^2 - 17 \sqrt{2} c_\theta^3 s_\theta^3 + 26 c_\theta^2 s_\theta^4 - 13 \sqrt{2} c_\theta s_\theta^5 - 30 s_\theta^6 \right) \Lambda_2 \right) \right) \Big) + \\
& M_\eta^4 M_\eta^6 s_\theta^2 \left( 48 c_\theta L_8^r M_\theta^2 M_\pi^4 \left( c_\theta^2 + s_\theta^2 \right) \left( -6 c_\theta^5 + \sqrt{2} c_\theta^4 s_\theta + 10 c_\theta^3 s_\theta^2 - 3 \sqrt{2} c_\theta^2 s_\theta^3 + \right. \right. \\
& \quad \left. \left. 2 c_\theta s_\theta^4 + 4 \sqrt{2} s_\theta^5 \right) + 3 F^2 M_\eta^2 s_\theta \left( -M_\eta^2 \left( 5 \sqrt{2} c_\theta^3 + 6 c_\theta^2 s_\theta + 12 \sqrt{2} c_\theta s_\theta^2 - 2 s_\theta^3 \right) + \right. \right. \\
& \quad \left. \left. c_\theta M_\theta^2 \left( 5 \sqrt{2} c_\theta^4 + 12 c_\theta^3 s_\theta + 21 \sqrt{2} c_\theta^2 s_\theta^2 - 20 c_\theta s_\theta^3 - 12 \sqrt{2} s_\theta^4 \right) \right) \Lambda_2 + \right. \\
& \quad \left. 2 M_\pi^2 \left( F^2 c_\theta M_\theta^2 \left( 30 c_\theta^7 - 5 \sqrt{2} c_\theta^6 s_\theta - 112 c_\theta^5 s_\theta^2 - 28 \sqrt{2} c_\theta^4 s_\theta^3 + 104 c_\theta^3 s_\theta^4 + \right. \right. \right. \\
& \quad \left. \left. 71 \sqrt{2} c_\theta^2 s_\theta^5 + 16 c_\theta s_\theta^6 - 6 \sqrt{2} s_\theta^7 \right) \Lambda_2 + M_\eta^2 \left( -288 c_\theta^2 L_8^r M_\theta^2 s_\theta \right. \right. \\
& \quad \left. \left. \left( \sqrt{2} c_\theta^3 + 3 c_\theta^2 s_\theta - 3 \sqrt{2} c_\theta s_\theta^2 - 4 s_\theta^3 \right) + F^2 \left( -30 c_\theta^6 + 13 \sqrt{2} c_\theta^5 s_\theta + \right. \right. \right. \\
& \quad \left. \left. \left. 26 c_\theta^4 s_\theta^2 + 17 \sqrt{2} c_\theta^3 s_\theta^3 + 2 c_\theta^2 s_\theta^4 - 16 \sqrt{2} c_\theta s_\theta^5 - 8 s_\theta^6 \right) \Lambda_2 \right) \right) \Big) +
\end{aligned}$$

$$\begin{aligned}
& c_\theta M_\eta^6 M_\eta^4 s_\theta \left( 2 c_\theta M_\theta^2 M_\pi^2 \left( -24 L_8^r M_\pi^2 (c_\theta^2 + s_\theta^2) \left( 4 \sqrt{2} c_\theta^5 - 2 c_\theta^4 s_\theta - 3 \sqrt{2} c_\theta^3 s_\theta^2 - \right. \right. \right. \\
& \quad \left. \left. \left. 10 c_\theta^2 s_\theta^3 + \sqrt{2} c_\theta s_\theta^4 + 6 s_\theta^5 \right) + F^2 \left( 6 \sqrt{2} c_\theta^7 + 16 c_\theta^6 s_\theta - 71 \sqrt{2} c_\theta^5 s_\theta^2 + \right. \right. \right. \\
& \quad \left. \left. \left. 104 c_\theta^4 s_\theta^3 + 28 \sqrt{2} c_\theta^3 s_\theta^4 - 112 c_\theta^2 s_\theta^5 + 5 \sqrt{2} c_\theta s_\theta^6 + 30 s_\theta^7 \right) \Lambda_2 \right) - \right. \\
& \quad \left. 3 M_\eta^2 \left( -3 F^2 c_\theta M_\theta^2 s_\theta \left( 2 c_\theta^4 + 7 \sqrt{2} c_\theta^3 s_\theta - 12 c_\theta^2 s_\theta^2 - 7 \sqrt{2} c_\theta s_\theta^3 + 2 s_\theta^4 \right) \Lambda_2 + \right. \right. \\
& \quad \left. \left. 2 M_\pi^2 \left( 144 c_\theta L_8^r M_\theta^2 s_\theta \left( 2 c_\theta^4 - 2 \sqrt{2} c_\theta^3 s_\theta - 3 c_\theta^2 s_\theta^2 + 2 \sqrt{2} c_\theta s_\theta^3 + 2 s_\theta^4 \right) + \right. \right. \right. \\
& \quad \left. \left. \left. F^2 \left( 2 \sqrt{2} c_\theta^6 - 6 c_\theta^5 s_\theta - 3 \sqrt{2} c_\theta^4 s_\theta^2 + 11 c_\theta^3 s_\theta^3 + \right. \right. \right. \right. \\
& \quad \left. \left. \left. 3 \sqrt{2} c_\theta^2 s_\theta^4 - 6 c_\theta s_\theta^5 - 2 \sqrt{2} s_\theta^6 \right) \Lambda_2 \right) \right) \right) \Big) \Big) \Big) \Big) \\
c_4^{\text{NNLO}}[T] = & -6 F^2 v_4^{(0)} - \frac{40\,960\, c_\theta^{12} L_8^2 r M_\theta^8 M_K^{10}}{729 F^2 M_\eta^{12}} + \frac{20\,480\, c_\theta^{12} L_8^2 r M_\theta^8 M_K^8 M_\pi^2}{243 F^2 M_\eta^{12}} - \frac{20\,480\, c_\theta^{12} L_8^2 r M_\theta^8 M_K^6 M_\pi^4}{243 F^2 M_\eta^{12}} + \\
& \frac{10\,240\, c_\theta^{12} L_8^2 r M_\theta^8 M_K^4 M_\pi^6}{729 F^2 M_\eta^{12}} + \frac{2560\, c_\theta^{12} L_8^2 r M_\theta^8 M_K^2 M_\pi^8}{243 F^2 M_\eta^{12}} - \frac{1280\, c_\theta^{12} L_8^2 r M_\theta^8 M_\pi^{10}}{81 F^2 M_\eta^{12}} + \frac{16 F^2 v_2^{(2)} c_\theta^{10} M_\theta^8 M_K^4}{27 M_\eta^{10}} - \\
& \frac{\text{Log}\left[\frac{M_K^2}{\mu^2}\right] c_\theta^{10} M_\theta^8 M_K^6}{243 \pi^2 M_\eta^{10}} + \frac{256\, c_\theta^{10} L_6^r M_\theta^8 M_K^6}{243 M_\eta^{10}} + \frac{256\, c_\theta^{10} L_7^r M_\theta^8 M_K^6}{243 M_\eta^{10}} - \frac{256\, c_\theta^{10} L_{25}^r M_\theta^8 M_K^6}{81 M_\eta^{10}} + \\
& \frac{512\, c_\theta^{10} C_{19} M_\theta^8 M_K^8}{81 M_\eta^{10}} + \frac{1024\, c_\theta^{10} C_{31} M_\theta^8 M_K^8}{243 M_\eta^{10}} + \frac{16 F^2 v_2^{(2)} c_\theta^{10} M_\theta^8 M_K^2 M_\pi^2}{27 M_\eta^{10}} - \frac{\text{Log}\left[\frac{M_K^2}{\mu^2}\right] c_\theta^{10} M_\theta^8 M_K^4 M_\pi^2}{486 \pi^2 M_\eta^{10}} + \\
& \frac{128\, c_\theta^{10} L_6^r M_\theta^8 M_K^4 M_\pi^2}{81 M_\eta^{10}} + \frac{128\, c_\theta^{10} L_7^r M_\theta^8 M_K^4 M_\pi^2}{81 M_\eta^{10}} + \frac{128\, c_\theta^{10} L_{25}^r M_\theta^8 M_K^4 M_\pi^2}{81 M_\eta^{10}} - \frac{512\, c_\theta^{10} C_{19} M_\theta^8 M_K^6 M_\pi^2}{81 M_\eta^{10}} - \\
& \frac{1024\, c_\theta^{10} C_{31} M_\theta^8 M_K^6 M_\pi^2}{243 M_\eta^{10}} + \frac{4 F^2 v_2^{(2)} c_\theta^{10} M_\theta^8 M_K^4}{27 M_\eta^{10}} - \frac{\text{Log}\left[\frac{M_\pi^2}{\mu^2}\right] c_\theta^{10} M_\theta^8 M_K^2 M_\pi^4}{324 \pi^2 M_\eta^{10}} + \frac{64\, c_\theta^{10} L_6^r M_\theta^8 M_K^2 M_\pi^4}{81 M_\eta^{10}} + \\
& \frac{64\, c_\theta^{10} L_7^r M_\theta^8 M_K^2 M_\pi^4}{81 M_\eta^{10}} - \frac{64\, c_\theta^{10} L_{25}^r M_\theta^8 M_K^2 M_\pi^4}{81 M_\eta^{10}} - \frac{\text{Log}\left[\frac{M_\pi^2}{\mu^2}\right] c_\theta^{10} M_\theta^8 M_K^6}{648 \pi^2 M_\eta^{10}} + \frac{32\, c_\theta^{10} L_6^r M_\theta^8 M_K^6}{243 M_\eta^{10}} + \\
& \frac{32\, c_\theta^{10} L_7^r M_\theta^8 M_K^6}{243 M_\eta^{10}} - \frac{32\, c_\theta^{10} L_{25}^r M_\theta^8 M_K^6}{27 M_\eta^{10}} + \frac{256\, c_\theta^{10} C_{19} M_\theta^8 M_K^2 M_\pi^6}{81 M_\eta^{10}} + \frac{512\, c_\theta^{10} C_{31} M_\theta^8 M_K^2 M_\pi^6}{243 M_\eta^{10}} + \\
& \frac{32\, c_\theta^{10} C_{19} M_\theta^8 M_\pi^8}{81 M_\eta^{10}} + \frac{64\, c_\theta^{10} C_{31} M_\theta^8 M_\pi^8}{243 M_\eta^{10}} - \frac{163\,840\, c_\theta^{12} L_8^2 r M_\theta^8 M_K^{10}}{729 F^2 M_\eta^2 M_\eta^{10}} + \frac{16\,384\, c_\theta^{12} L_8^2 r M_\theta^8 M_K^8 M_\pi^2}{27 F^2 M_\eta^2 M_\eta^{10}} - \\
& \frac{163\,840\, c_\theta^{12} L_8^2 r M_\theta^8 M_K^6 M_\pi^4}{243 F^2 M_\eta^2 M_\eta^{10}} + \frac{311\,296\, c_\theta^{12} L_8^2 r M_\theta^8 M_K^4 M_\pi^6}{729 F^2 M_\eta^2 M_\eta^{10}} - \frac{32\,768\, c_\theta^{12} L_8^2 r M_\theta^8 M_K^2 M_\pi^8}{243 F^2 M_\eta^2 M_\eta^{10}} - \\
& \frac{\text{Log}\left[\frac{M_\eta^2}{\mu^2}\right] c_\theta^{12} M_\theta^8 M_K^4 M_\pi^2}{729 \pi^2 M_\eta^{10}} - \frac{\text{Log}\left[\frac{M_\eta^2}{\mu^2}\right] c_\theta^{12} M_\theta^8 M_K^2 M_\pi^2 M_\pi^2}{2916 \pi^2 M_\eta^{10}} + \frac{\text{Log}\left[\frac{M_\eta^2}{\mu^2}\right] c_\theta^{12} M_\theta^8 M_K^4 M_\pi^2}{5832 \pi^2 M_\eta^{10}} - \frac{4 F^2 v_2^{(2)} c_\theta^8 M_\theta^8 M_K^2}{3 M_\eta^8} - \\
& \frac{16 F^2 v_2^{(2)} c_\theta^8 M_\theta^6 M_K^4}{27 M_\eta^8} + \frac{c_\theta^8 M_\theta^8 M_K^4}{216 \pi^2 M_\eta^8} + \frac{\text{Log}\left[\frac{M_K^2}{\mu^2}\right] c_\theta^8 M_\theta^8 M_K^4}{162 \pi^2 M_\eta^8} + \frac{5 c_\theta^{12} M_\theta^8 M_K^4}{1944 \pi^2 M_\eta^8} - \frac{\text{Log}\left[\frac{M_\eta^2}{\mu^2}\right] c_\theta^{12} M_\theta^8 M_K^4}{1458 \pi^2 M_\eta^8} -
\end{aligned}$$

$$\begin{aligned}
& \frac{\text{Log}\left[\frac{M_{\eta'}^2}{\mu^2}\right] c_{\theta}^{12} M_0^8 M_K^4}{5832 \pi^2 M_{\eta'}^8} - \frac{128 c_{\theta}^8 L_6^r M_0^8 M_K^4}{81 M_{\eta'}^8} - \frac{128 c_{\theta}^8 L_7^r M_0^8 M_K^4}{81 M_{\eta'}^8} - \frac{448 c_{\theta}^8 C_{19} M_0^8 M_K^6}{27 M_{\eta'}^8} - \frac{1280 c_{\theta}^8 C_{31} M_0^8 M_K^6}{81 M_{\eta'}^8} \\
& \frac{2 F^2 v_2^{(2)} c_{\theta}^8 M_0^8 M_{\pi}^2}{3 M_{\eta'}^8} - \frac{16 F^2 v_2^{(2)} c_{\theta}^8 M_0^6 M_K^2 M_{\pi}^2}{27 M_{\eta'}^8} - \frac{c_{\theta}^{12} M_0^8 M_K^2 M_{\pi}^2}{1944 \pi^2 M_{\eta'}^8} + \frac{5 \text{Log}\left[\frac{M_{\eta'}^2}{\mu^2}\right] c_{\theta}^{12} M_0^8 M_K^2 M_{\pi}^2}{1458 \pi^2 M_{\eta'}^8} - \\
& \frac{\text{Log}\left[\frac{M_{\eta'}^2}{\mu^2}\right] c_{\theta}^{12} M_0^8 M_K^2 M_{\pi}^2}{5832 \pi^2 M_{\eta'}^8} - \frac{128 c_{\theta}^8 L_6^r M_0^8 M_K^2 M_{\pi}^2}{81 M_{\eta'}^8} - \frac{128 c_{\theta}^8 L_7^r M_0^8 M_K^2 M_{\pi}^2}{81 M_{\eta'}^8} + \frac{224 c_{\theta}^8 C_{19} M_0^8 M_K^4 M_{\pi}^2}{9 M_{\eta'}^8} + \\
& \frac{640 c_{\theta}^8 C_{31} M_0^8 M_K^4 M_{\pi}^2}{27 M_{\eta'}^8} - \frac{4 F^2 v_2^{(2)} c_{\theta}^8 M_0^6 M_{\pi}^4}{27 M_{\eta'}^8} + \frac{c_{\theta}^8 M_0^8 M_{\pi}^4}{288 \pi^2 M_{\eta'}^8} + \frac{\text{Log}\left[\frac{M_{\eta'}^2}{\mu^2}\right] c_{\theta}^8 M_0^8 M_{\pi}^4}{216 \pi^2 M_{\eta'}^8} + \frac{c_{\theta}^{12} M_0^8 M_{\pi}^4}{3888 \pi^2 M_{\eta'}^8} - \\
& \frac{37 \text{Log}\left[\frac{M_{\eta'}^2}{\mu^2}\right] c_{\theta}^{12} M_0^8 M_{\pi}^4}{23 \ 328 \pi^2 M_{\eta'}^8} - \frac{\text{Log}\left[\frac{M_{\eta'}^2}{\mu^2}\right] c_{\theta}^{12} M_0^8 M_{\pi}^4}{23 \ 328 \pi^2 M_{\eta'}^8} - \frac{32 c_{\theta}^8 L_6^r M_0^8 M_{\pi}^4}{81 M_{\eta'}^8} - \frac{32 c_{\theta}^8 L_7^r M_0^8 M_{\pi}^4}{81 M_{\eta'}^8} - \\
& \frac{112 c_{\theta}^8 C_{19} M_0^8 M_K^2 M_{\pi}^4}{9 M_{\eta'}^8} - \frac{320 c_{\theta}^8 C_{31} M_0^8 M_K^2 M_{\pi}^4}{27 M_{\eta'}^8} - \frac{56 c_{\theta}^8 C_{19} M_0^8 M_{\pi}^6}{27 M_{\eta'}^8} - \frac{160 c_{\theta}^8 C_{31} M_0^8 M_{\pi}^6}{81 M_{\eta'}^8} - \\
& \frac{163 \ 840 c_{\theta}^{12} L_8^{2r} M_0^8 M_K^{10}}{729 F^2 M_{\eta'}^4 M_{\eta'}^8} + \frac{139 \ 264 c_{\theta}^{12} L_8^{2r} M_0^8 M_K^8 M_{\pi}^2}{243 F^2 M_{\eta'}^4 M_{\eta'}^8} - \frac{40 \ 960 c_{\theta}^{12} L_8^{2r} M_0^8 M_K^6 M_{\pi}^4}{81 F^2 M_{\eta'}^4 M_{\eta'}^8} + \\
& \frac{139 \ 264 c_{\theta}^{12} L_8^{2r} M_0^8 M_K^4 M_{\pi}^6}{729 F^2 M_{\eta'}^4 M_{\eta'}^8} - \frac{8192 c_{\theta}^{12} L_8^{2r} M_0^8 M_K^2 M_{\pi}^8}{243 F^2 M_{\eta'}^4 M_{\eta'}^8} - \frac{\text{Log}\left[\frac{M_K^2}{\mu^2}\right] c_{\theta}^{10} M_0^8 M_K^6}{243 \pi^2 M_{\eta'}^2 M_{\eta'}^8} + \frac{512 c_{\theta}^{10} L_6^r M_0^8 M_K^6}{243 M_{\eta'}^2 M_{\eta'}^8} + \\
& \frac{512 c_{\theta}^{10} L_7^r M_0^8 M_K^6}{243 M_{\eta'}^2 M_{\eta'}^8} - \frac{256 c_{\theta}^{10} L_{25}^r M_0^8 M_K^6}{81 M_{\eta'}^2 M_{\eta'}^8} + \frac{1024 c_{\theta}^{10} C_{19} M_0^8 M_K^8}{81 M_{\eta'}^2 M_{\eta'}^8} + \frac{2048 c_{\theta}^{10} C_{31} M_0^8 M_K^8}{243 M_{\eta'}^2 M_{\eta'}^8} + \\
& \frac{\text{Log}\left[\frac{M_K^2}{\mu^2}\right] c_{\theta}^{10} M_0^8 M_K^4 M_{\pi}^2}{162 \pi^2 M_{\eta'}^2 M_{\eta'}^8} - \frac{256 c_{\theta}^{10} L_6^r M_0^8 M_K^4 M_{\pi}^2}{81 M_{\eta'}^2 M_{\eta'}^8} - \frac{256 c_{\theta}^{10} L_7^r M_0^8 M_K^4 M_{\pi}^2}{81 M_{\eta'}^2 M_{\eta'}^8} + \frac{512 c_{\theta}^{10} L_{25}^r M_0^8 M_K^4 M_{\pi}^2}{81 M_{\eta'}^2 M_{\eta'}^8} - \\
& \frac{2560 c_{\theta}^{10} C_{19} M_0^8 M_K^6 M_{\pi}^2}{81 M_{\eta'}^2 M_{\eta'}^8} - \frac{5120 c_{\theta}^{10} C_{31} M_0^8 M_K^6 M_{\pi}^2}{243 M_{\eta'}^2 M_{\eta'}^8} - \frac{\text{Log}\left[\frac{M_K^2}{\mu^2}\right] c_{\theta}^{10} M_0^8 M_K^2 M_{\pi}^4}{486 \pi^2 M_{\eta'}^2 M_{\eta'}^8} + \frac{\text{Log}\left[\frac{M_{\pi}^2}{\mu^2}\right] c_{\theta}^{10} M_0^8 M_K^2 M_{\pi}^4}{324 \pi^2 M_{\eta'}^2 M_{\eta'}^8} - \\
& \frac{256 c_{\theta}^{10} L_{25}^r M_0^8 M_K^2 M_{\pi}^4}{81 M_{\eta'}^2 M_{\eta'}^8} + \frac{256 c_{\theta}^{10} C_{19} M_0^8 M_K^4 M_{\pi}^4}{9 M_{\eta'}^2 M_{\eta'}^8} + \frac{512 c_{\theta}^{10} C_{31} M_0^8 M_K^4 M_{\pi}^4}{27 M_{\eta'}^2 M_{\eta'}^8} - \frac{\text{Log}\left[\frac{M_{\pi}^2}{\mu^2}\right] c_{\theta}^{10} M_0^8 M_{\pi}^6}{324 \pi^2 M_{\eta'}^2 M_{\eta'}^8} + \\
& \frac{256 c_{\theta}^{10} L_6^r M_0^8 M_{\pi}^6}{243 M_{\eta'}^2 M_{\eta'}^8} + \frac{256 c_{\theta}^{10} L_7^r M_0^8 M_{\pi}^6}{243 M_{\eta'}^2 M_{\eta'}^8} - \frac{1024 c_{\theta}^{10} C_{19} M_0^8 M_K^2 M_{\pi}^6}{81 M_{\eta'}^2 M_{\eta'}^8} - \frac{2048 c_{\theta}^{10} C_{31} M_0^8 M_K^2 M_{\pi}^6}{243 M_{\eta'}^2 M_{\eta'}^8} + \\
& \frac{256 c_{\theta}^{10} C_{19} M_0^8 M_{\pi}^8}{81 M_{\eta'}^2 M_{\eta'}^8} + \frac{512 c_{\theta}^{10} C_{31} M_0^8 M_{\pi}^8}{243 M_{\eta'}^2 M_{\eta'}^8} + \frac{\text{Log}\left[\frac{M_{\eta'}^2}{\mu^2}\right] c_{\theta}^{10} M_0^8 M_K^2 M_{\eta'}^2}{1944 \pi^2 M_{\eta'}^8} - \frac{\text{Log}\left[\frac{M_{\eta'}^2}{\mu^2}\right] c_{\theta}^{10} M_0^8 M_{\pi}^2 M_{\eta'}^2}{7776 \pi^2 M_{\eta'}^8} + \\
& \frac{24 F^2 v_4^{(0)} c_{\theta}^6 M_0^6}{M_{\eta'}^6} + \frac{8 F^2 v_2^{(2)} c_{\theta}^6 M_0^6 M_K^2}{3 M_{\eta'}^6} + \frac{\text{Log}\left[\frac{M_{\eta'}^2}{\mu^2}\right] c_{\theta}^{10} M_0^8 M_K^2}{3888 \pi^2 M_{\eta'}^6} + \frac{4 F^2 v_2^{(2)} c_{\theta}^6 M_0^6 M_{\pi}^2}{3 M_{\eta'}^6} +
\end{aligned}$$

$$\begin{aligned}
& \frac{\text{Log}\left[\frac{M_{\eta'}^2}{\mu^2}\right] c_{\theta}^{10} M_{\theta}^8 M_{\pi}^2}{7776 \pi^2 M_{\eta'}^6} - \frac{\text{Log}\left[\frac{M_{\eta'}^2}{\mu^2}\right] c_{\theta}^{12} M_{\theta}^8 M_K^4}{729 \pi^2 M_{\eta'}^6} + \frac{2 \text{Log}\left[\frac{M_{\eta'}^2}{\mu^2}\right] c_{\theta}^{12} M_{\theta}^8 M_K^2 M_{\pi}^2}{729 \pi^2 M_{\eta'}^6} - \frac{\text{Log}\left[\frac{M_{\eta'}^2}{\mu^2}\right] c_{\theta}^{12} M_{\theta}^8 M_{\pi}^4}{729 \pi^2 M_{\eta'}^6} - \\
& \frac{4 F^2 v_2^{(2)} c_{\theta}^4 M_{\theta}^4 M_K^2}{3 M_{\eta'}^4} - \frac{2 F^2 v_2^{(2)} c_{\theta}^4 M_{\theta}^4 M_{\pi}^2}{3 M_{\eta'}^4} + \frac{24 F^2 v_4^{(0)} c_{\theta}^2 M_{\theta}^2}{M_{\eta'}^2} + \frac{\text{Log}\left[\frac{M_{\eta'}^2}{\mu^2}\right] c_{\theta}^{12} M_{\theta}^8 M_K^4 M_{\pi}^2}{486 \pi^2 M_{\eta'}^8 (M_{\eta'}^2 - M_{\pi}^2)} - \\
& \frac{\text{Log}\left[\frac{M_{\eta'}^2}{\mu^2}\right] c_{\theta}^{12} M_{\theta}^8 M_K^2 M_{\pi}^2 M_{\eta'}^2}{243 \pi^2 M_{\eta'}^8 (M_{\eta'}^2 - M_{\pi}^2)} + \frac{\text{Log}\left[\frac{M_{\eta'}^2}{\mu^2}\right] c_{\theta}^{12} M_{\theta}^8 M_{\pi}^4 M_{\eta'}^2}{486 \pi^2 M_{\eta'}^8 (M_{\eta'}^2 - M_{\pi}^2)} - \frac{\text{Log}\left[\frac{M_{\eta'}^2}{\mu^2}\right] c_{\theta}^{12} M_{\theta}^8 M_K^4}{486 \pi^2 M_{\eta'}^6 (M_{\eta'}^2 - M_{\pi}^2)} + \\
& \frac{\text{Log}\left[\frac{M_{\eta'}^2}{\mu^2}\right] c_{\theta}^{12} M_{\theta}^8 M_K^2 M_{\pi}^2}{243 \pi^2 M_{\eta'}^6 (M_{\eta'}^2 - M_{\pi}^2)} - \frac{\text{Log}\left[\frac{M_{\eta'}^2}{\mu^2}\right] c_{\theta}^{12} M_{\theta}^8 M_{\pi}^4}{486 \pi^2 M_{\eta'}^6 (M_{\eta'}^2 - M_{\pi}^2)} + \frac{327 680 \sqrt{2} c_{\theta}^{11} L_8^2 r M_{\theta}^8 M_K^{10} s_{\theta}}{729 F^2 M_{\eta'}^{12}} - \\
& \frac{81 920 \sqrt{2} c_{\theta}^{11} L_8^2 r M_{\theta}^8 M_K^8 M_{\pi}^2 s_{\theta}}{81 F^2 M_{\eta'}^{12}} + \frac{286 720 \sqrt{2} c_{\theta}^{11} L_8^2 r M_{\theta}^8 M_K^6 M_{\pi}^4 s_{\theta}}{243 F^2 M_{\eta'}^{12}} - \\
& \frac{634 880 \sqrt{2} c_{\theta}^{11} L_8^2 r M_{\theta}^8 M_K^4 M_{\pi}^6 s_{\theta}}{729 F^2 M_{\eta'}^{12}} + \frac{10 240 \sqrt{2} c_{\theta}^{11} L_8^2 r M_{\theta}^8 M_K^2 M_{\pi}^8 s_{\theta}}{27 F^2 M_{\eta'}^{12}} - \\
& \frac{10 240 \sqrt{2} c_{\theta}^{11} L_8^2 r M_{\theta}^8 M_{\pi}^{10} s_{\theta}}{81 F^2 M_{\eta'}^{12}} - \frac{64 \sqrt{2} F^2 v_2^{(2)} c_{\theta}^9 M_{\theta}^8 M_K^4 s_{\theta}}{27 M_{\eta'}^{10}} + \frac{5 \sqrt{2} \text{Log}\left[\frac{M_K^2}{\mu^2}\right] c_{\theta}^9 M_{\theta}^8 M_K^6 s_{\theta}}{243 \pi^2 M_{\eta'}^{10}} - \\
& \frac{512 \sqrt{2} c_{\theta}^9 L_6^r M_{\theta}^8 M_K^6 s_{\theta}}{81 M_{\eta'}^{10}} - \frac{512 \sqrt{2} c_{\theta}^9 L_7^r M_{\theta}^8 M_K^6 s_{\theta}}{81 M_{\eta'}^{10}} + \frac{1280 \sqrt{2} c_{\theta}^9 L_{25}^r M_{\theta}^8 M_K^6 s_{\theta}}{81 M_{\eta'}^{10}} - \\
& \frac{1024 \sqrt{2} c_{\theta}^9 C_{19} M_{\theta}^8 M_K^8 s_{\theta}}{27 M_{\eta'}^{10}} - \frac{2048 \sqrt{2} c_{\theta}^9 C_{31} M_{\theta}^8 M_K^8 s_{\theta}}{81 M_{\eta'}^{10}} + \frac{32 \sqrt{2} F^2 v_2^{(2)} c_{\theta}^9 M_{\theta}^8 M_K^2 M_{\pi}^2 s_{\theta}}{27 M_{\eta'}^{10}} - \\
& \frac{4 \sqrt{2} \text{Log}\left[\frac{M_K^2}{\mu^2}\right] c_{\theta}^9 M_{\theta}^8 M_K^4 M_{\pi}^2 s_{\theta}}{243 \pi^2 M_{\eta'}^{10}} - \frac{2176 \sqrt{2} c_{\theta}^9 L_{25}^r M_{\theta}^8 M_K^4 M_{\pi}^2 s_{\theta}}{81 M_{\eta'}^{10}} + \frac{2048 \sqrt{2} c_{\theta}^9 C_{19} M_{\theta}^8 M_K^6 M_{\pi}^2 s_{\theta}}{27 M_{\eta'}^{10}} + \\
& \frac{4096 \sqrt{2} c_{\theta}^9 C_{31} M_{\theta}^8 M_K^6 M_{\pi}^2 s_{\theta}}{81 M_{\eta'}^{10}} + \frac{32 \sqrt{2} F^2 v_2^{(2)} c_{\theta}^9 M_{\theta}^8 M_{\pi}^4 s_{\theta}}{27 M_{\eta'}^{10}} - \frac{\text{Log}\left[\frac{M_K^2}{\mu^2}\right] c_{\theta}^9 M_{\theta}^8 M_K^2 M_{\pi}^4 s_{\theta}}{486 \sqrt{2} \pi^2 M_{\eta'}^{10}} - \\
& \frac{\text{Log}\left[\frac{M_{\pi}^2}{\mu^2}\right] c_{\theta}^9 M_{\theta}^8 M_K^2 M_{\pi}^4 s_{\theta}}{162 \sqrt{2} \pi^2 M_{\eta'}^{10}} + \frac{\sqrt{2} \text{Log}\left[\frac{M_{\pi}^2}{\mu^2}\right] c_{\theta}^9 M_{\theta}^8 M_K^2 M_{\pi}^4 s_{\theta}}{81 \pi^2 M_{\eta'}^{10}} + \frac{128 \sqrt{2} c_{\theta}^9 L_6^r M_{\theta}^8 M_K^2 M_{\pi}^4 s_{\theta}}{27 M_{\eta'}^{10}} + \\
& \frac{128 \sqrt{2} c_{\theta}^9 L_7^r M_{\theta}^8 M_K^2 M_{\pi}^4 s_{\theta}}{27 M_{\eta'}^{10}} + \frac{1664 \sqrt{2} c_{\theta}^9 L_{25}^r M_{\theta}^8 M_K^2 M_{\pi}^4 s_{\theta}}{81 M_{\eta'}^{10}} - \frac{512 \sqrt{2} c_{\theta}^9 C_{19} M_{\theta}^8 M_K^4 M_{\pi}^4 s_{\theta}}{9 M_{\eta'}^{10}} - \\
& \frac{1024 \sqrt{2} c_{\theta}^9 C_{31} M_{\theta}^8 M_K^4 M_{\pi}^4 s_{\theta}}{27 M_{\eta'}^{10}} - \frac{\text{Log}\left[\frac{M_{\pi}^2}{\mu^2}\right] c_{\theta}^9 M_{\theta}^8 M_{\pi}^6 s_{\theta}}{324 \sqrt{2} \pi^2 M_{\eta'}^{10}} - \frac{\sqrt{2} \text{Log}\left[\frac{M_{\pi}^2}{\mu^2}\right] c_{\theta}^9 M_{\theta}^8 M_{\pi}^6 s_{\theta}}{81 \pi^2 M_{\eta'}^{10}} + \\
& \frac{128 \sqrt{2} c_{\theta}^9 L_6^r M_{\theta}^8 M_{\pi}^6 s_{\theta}}{81 M_{\eta'}^{10}} + \frac{128 \sqrt{2} c_{\theta}^9 L_7^r M_{\theta}^8 M_{\pi}^6 s_{\theta}}{81 M_{\eta'}^{10}} - \frac{256 \sqrt{2} c_{\theta}^9 L_{25}^r M_{\theta}^8 M_{\pi}^6 s_{\theta}}{27 M_{\eta'}^{10}} +
\end{aligned}$$

$$\begin{aligned}
& \frac{128 \sqrt{2} c_{\theta}^9 C_{19} M_0^8 M_K^2 M_{\pi}^6 s_{\theta}}{9 M_{\eta'}^{10}} + \frac{256 \sqrt{2} c_{\theta}^9 C_{31} M_0^8 M_K^2 M_{\pi}^6 s_{\theta}}{27 M_{\eta'}^{10}} + \frac{128 \sqrt{2} c_{\theta}^9 C_{19} M_0^8 M_{\pi}^8 s_{\theta}}{27 M_{\eta'}^{10}} + \\
& \frac{256 \sqrt{2} c_{\theta}^9 C_{31} M_0^8 M_{\pi}^8 s_{\theta}}{81 M_{\eta'}^{10}} + \frac{655360 \sqrt{2} c_{\theta}^{11} L_8^2 r M_0^8 M_K^{10} s_{\theta}}{729 F^2 M_{\eta'}^2 M_{\eta'}^{10}} - \frac{606208 \sqrt{2} c_{\theta}^{11} L_8^2 r M_0^8 M_K^8 M_{\pi}^2 s_{\theta}}{243 F^2 M_{\eta'}^2 M_{\eta'}^{10}} + \\
& \frac{65536 \sqrt{2} c_{\theta}^{11} L_8^2 r M_0^8 M_K^6 M_{\pi}^4 s_{\theta}}{27 F^2 M_{\eta'}^2 M_{\eta'}^{10}} - \frac{630784 \sqrt{2} c_{\theta}^{11} L_8^2 r M_0^8 M_K^4 M_{\pi}^6 s_{\theta}}{729 F^2 M_{\eta'}^2 M_{\eta'}^{10}} - \\
& \frac{10240 \sqrt{2} c_{\theta}^{11} L_8^2 r M_0^8 M_K^2 M_{\pi}^8 s_{\theta}}{243 F^2 M_{\eta'}^2 M_{\eta'}^{10}} + \frac{2048 \sqrt{2} c_{\theta}^{11} L_8^2 r M_0^8 M_{\pi}^{10} s_{\theta}}{27 F^2 M_{\eta'}^2 M_{\eta'}^{10}} + \frac{5 \sqrt{2} \text{Log} \left[ \frac{M_{\eta'}^2}{\mu^2} \right] c_{\theta}^{11} M_0^8 M_K^4 M_{\eta'}^2 s_{\theta}}{729 \pi^2 M_{\eta'}^{10}} + \\
& \frac{\text{Log} \left[ \frac{M_{\eta'}^2}{\mu^2} \right] c_{\theta}^{11} M_0^8 M_K^2 M_{\pi}^2 M_{\eta'}^2 s_{\theta}}{1458 \sqrt{2} \pi^2 M_{\eta'}^{10}} - \frac{5 \sqrt{2} \text{Log} \left[ \frac{M_{\eta'}^2}{\mu^2} \right] c_{\theta}^{11} M_0^8 M_K^2 M_{\pi}^2 M_{\eta'}^2 s_{\theta}}{729 \pi^2 M_{\eta'}^{10}} - \frac{\text{Log} \left[ \frac{M_{\eta'}^2}{\mu^2} \right] c_{\theta}^{11} M_0^8 M_{\pi}^4 M_{\eta'}^2 s_{\theta}}{2916 \sqrt{2} \pi^2 M_{\eta'}^{10}} + \\
& \frac{\sqrt{2} \text{Log} \left[ \frac{M_{\eta'}^2}{\mu^2} \right] c_{\theta}^{11} M_0^8 M_{\pi}^4 M_{\eta'}^2 s_{\theta}}{729 \pi^2 M_{\eta'}^{10}} + \frac{8 \sqrt{2} F^2 v_2^{(2)} c_{\theta}^7 M_0^8 M_K^2 s_{\theta}}{3 M_{\eta'}^8} + \frac{64 \sqrt{2} F^2 v_2^{(2)} c_{\theta}^7 M_0^6 M_K^4 s_{\theta}}{27 M_{\eta'}^8} + \\
& \frac{c_{\theta}^7 M_0^8 M_K^4 s_{\theta}}{162 \sqrt{2} \pi^2 M_{\eta'}^8} - \frac{\sqrt{2} c_{\theta}^7 M_0^8 M_K^4 s_{\theta}}{81 \pi^2 M_{\eta'}^8} - \frac{\sqrt{2} \text{Log} \left[ \frac{M_K^2}{\mu^2} \right] c_{\theta}^7 M_0^8 M_K^4 s_{\theta}}{81 \pi^2 M_{\eta'}^8} - \frac{2 \sqrt{2} c_{\theta}^{11} M_0^8 M_K^4 s_{\theta}}{243 \pi^2 M_{\eta'}^8} - \\
& \frac{\sqrt{2} \text{Log} \left[ \frac{M_{\eta'}^2}{\mu^2} \right] c_{\theta}^{11} M_0^8 M_K^4 s_{\theta}}{243 \pi^2 M_{\eta'}^8} + \frac{\sqrt{2} \text{Log} \left[ \frac{M_{\eta'}^2}{\mu^2} \right] c_{\theta}^{11} M_0^8 M_K^4 s_{\theta}}{729 \pi^2 M_{\eta'}^8} + \frac{512 \sqrt{2} c_{\theta}^7 L_6^r M_0^8 M_K^4 s_{\theta}}{81 M_{\eta'}^8} + \\
& \frac{512 \sqrt{2} c_{\theta}^7 L_7^r M_0^8 M_K^4 s_{\theta}}{81 M_{\eta'}^8} + \frac{1792 \sqrt{2} c_{\theta}^7 C_{19} M_0^8 M_K^6 s_{\theta}}{27 M_{\eta'}^8} + \frac{5120 \sqrt{2} c_{\theta}^7 C_{31} M_0^8 M_K^6 s_{\theta}}{81 M_{\eta'}^8} - \\
& \frac{8 \sqrt{2} F^2 v_2^{(2)} c_{\theta}^7 M_0^8 M_{\pi}^2 s_{\theta}}{3 M_{\eta'}^8} - \frac{32 \sqrt{2} F^2 v_2^{(2)} c_{\theta}^7 M_0^6 M_K^2 M_{\pi}^2 s_{\theta}}{27 M_{\eta'}^8} + \frac{c_{\theta}^7 M_0^8 M_K^2 M_{\pi}^2 s_{\theta}}{108 \sqrt{2} \pi^2 M_{\eta'}^8} + \\
& \frac{\text{Log} \left[ \frac{M_K^2}{\mu^2} \right] c_{\theta}^7 M_0^8 M_K^2 M_{\pi}^2 s_{\theta}}{81 \sqrt{2} \pi^2 M_{\eta'}^8} + \frac{\sqrt{2} c_{\theta}^{11} M_0^8 M_K^2 M_{\pi}^2 s_{\theta}}{243 \pi^2 M_{\eta'}^8} - \frac{23 \text{Log} \left[ \frac{M_{\eta'}^2}{\mu^2} \right] c_{\theta}^{11} M_0^8 M_K^2 M_{\pi}^2 s_{\theta}}{2916 \sqrt{2} \pi^2 M_{\eta'}^8} + \\
& \frac{4 \sqrt{2} \text{Log} \left[ \frac{M_{\eta'}^2}{\mu^2} \right] c_{\theta}^{11} M_0^8 M_K^2 M_{\pi}^2 s_{\theta}}{729 \pi^2 M_{\eta'}^8} + \frac{\text{Log} \left[ \frac{M_{\eta'}^2}{\mu^2} \right] c_{\theta}^{11} M_0^8 M_K^2 M_{\pi}^2 s_{\theta}}{243 \sqrt{2} \pi^2 M_{\eta'}^8} - \frac{2 \sqrt{2} \text{Log} \left[ \frac{M_{\eta'}^2}{\mu^2} \right] c_{\theta}^{11} M_0^8 M_K^2 M_{\pi}^2 s_{\theta}}{729 \pi^2 M_{\eta'}^8} - \\
& \frac{256 \sqrt{2} c_{\theta}^7 L_6^r M_0^8 M_K^2 M_{\pi}^2 s_{\theta}}{81 M_{\eta'}^8} - \frac{256 \sqrt{2} c_{\theta}^7 L_7^r M_0^8 M_K^2 M_{\pi}^2 s_{\theta}}{81 M_{\eta'}^8} - \frac{896 \sqrt{2} c_{\theta}^7 C_{19} M_0^8 M_K^4 M_{\pi}^2 s_{\theta}}{9 M_{\eta'}^8} - \\
& \frac{2560 \sqrt{2} c_{\theta}^7 C_{31} M_0^8 M_K^4 M_{\pi}^2 s_{\theta}}{27 M_{\eta'}^8} - \frac{32 \sqrt{2} F^2 v_2^{(2)} c_{\theta}^7 M_0^6 M_{\pi}^4 s_{\theta}}{27 M_{\eta'}^8} + \frac{c_{\theta}^7 M_0^8 M_{\pi}^4 s_{\theta}}{72 \sqrt{2} \pi^2 M_{\eta'}^8} + \\
& \frac{\text{Log} \left[ \frac{M_{\pi}^2}{\mu^2} \right] c_{\theta}^7 M_0^8 M_{\pi}^4 s_{\theta}}{54 \sqrt{2} \pi^2 M_{\eta'}^8} + \frac{7 c_{\theta}^{11} M_0^8 M_{\pi}^4 s_{\theta}}{1944 \sqrt{2} \pi^2 M_{\eta'}^8} + \frac{\text{Log} \left[ \frac{M_{\eta'}^2}{\mu^2} \right] c_{\theta}^{11} M_0^8 M_{\pi}^4 s_{\theta}}{486 \sqrt{2} \pi^2 M_{\eta'}^8} + \frac{\text{Log} \left[ \frac{M_{\eta'}^2}{\mu^2} \right] c_{\theta}^{11} M_0^8 M_{\pi}^4 s_{\theta}}{243 \sqrt{2} \pi^2 M_{\eta'}^8} -
\end{aligned}$$

$$\begin{aligned}
& \frac{2 \sqrt{2} \operatorname{Log} \left[ \frac{M_{\eta'}^2}{\mu^2} \right] c_{\theta}^{11} M_0^8 M_{\pi}^4 s_{\theta}}{729 \pi^2 M_{\eta'}^8} - \frac{256 \sqrt{2} c_{\theta}^7 L_6^r M_0^8 M_{\pi}^4 s_{\theta}}{81 M_{\eta'}^8} - \frac{256 \sqrt{2} c_{\theta}^7 L_7^r M_0^8 M_{\pi}^4 s_{\theta}}{81 M_{\eta'}^8} + \\
& \frac{448 \sqrt{2} c_{\theta}^7 C_{19} M_0^8 M_K^2 M_{\pi}^4 s_{\theta}}{9 M_{\eta'}^8} + \frac{1280 \sqrt{2} c_{\theta}^7 C_{31} M_0^8 M_K^2 M_{\pi}^4 s_{\theta}}{27 M_{\eta'}^8} - \frac{448 \sqrt{2} c_{\theta}^7 C_{19} M_0^8 M_{\pi}^6 s_{\theta}}{27 M_{\eta'}^8} - \\
& \frac{1280 \sqrt{2} c_{\theta}^7 C_{31} M_0^8 M_{\pi}^6 s_{\theta}}{81 M_{\eta'}^8} - \frac{327 680 \sqrt{2} c_{\theta}^{11} L_8^2 r M_0^8 M_K^{10} s_{\theta}}{729 F^2 M_{\eta'}^4 M_{\eta'}^8} + \frac{106 496 \sqrt{2} c_{\theta}^{11} L_8^2 r M_0^8 M_K^8 M_{\pi}^2 s_{\theta}}{81 F^2 M_{\eta'}^4 M_{\eta'}^8} - \\
& \frac{401 408 \sqrt{2} c_{\theta}^{11} L_8^2 r M_0^8 M_K^6 M_{\pi}^4 s_{\theta}}{243 F^2 M_{\eta'}^4 M_{\eta'}^8} + \frac{696 320 \sqrt{2} c_{\theta}^{11} L_8^2 r M_0^8 M_K^4 M_{\pi}^6 s_{\theta}}{729 F^2 M_{\eta'}^4 M_{\eta'}^8} - \\
& \frac{50 176 \sqrt{2} c_{\theta}^{11} L_8^2 r M_0^8 M_K^2 M_{\pi}^8 s_{\theta}}{243 F^2 M_{\eta'}^4 M_{\eta'}^8} + \frac{1024 \sqrt{2} c_{\theta}^{11} L_8^2 r M_0^8 M_{\pi}^{10} s_{\theta}}{27 F^2 M_{\eta'}^4 M_{\eta'}^8} + \frac{64 \sqrt{2} F^2 v_2^{(2)} c_{\theta}^9 M_0^8 M_K^4 s_{\theta}}{27 M_{\eta'}^2 M_{\eta'}^8} - \\
& \frac{2 \sqrt{2} \operatorname{Log} \left[ \frac{M_K^2}{\mu^2} \right] c_{\theta}^9 M_0^8 M_K^6 s_{\theta}}{243 \pi^2 M_{\eta'}^2 M_{\eta'}^8} - \frac{512 \sqrt{2} c_{\theta}^9 L_6^r M_0^8 M_K^6 s_{\theta}}{243 M_{\eta'}^2 M_{\eta'}^8} - \frac{512 \sqrt{2} c_{\theta}^9 L_7^r M_0^8 M_K^6 s_{\theta}}{243 M_{\eta'}^2 M_{\eta'}^8} - \\
& \frac{512 \sqrt{2} c_{\theta}^9 L_{25}^r M_0^8 M_K^6 s_{\theta}}{81 M_{\eta'}^2 M_{\eta'}^8} - \frac{1024 \sqrt{2} c_{\theta}^9 C_{19} M_0^8 M_K^8 s_{\theta}}{81 M_{\eta'}^2 M_{\eta'}^8} - \frac{2048 \sqrt{2} c_{\theta}^9 C_{31} M_0^8 M_K^8 s_{\theta}}{243 M_{\eta'}^2 M_{\eta'}^8} - \\
& \frac{32 \sqrt{2} F^2 v_2^{(2)} c_{\theta}^9 M_0^8 M_K^2 M_{\pi}^2 s_{\theta}}{27 M_{\eta'}^2 M_{\eta'}^8} - \frac{\operatorname{Log} \left[ \frac{M_K^2}{\mu^2} \right] c_{\theta}^9 M_0^8 M_K^4 M_{\pi}^2 s_{\theta}}{81 \sqrt{2} \pi^2 M_{\eta'}^2 M_{\eta'}^8} + \frac{\sqrt{2} \operatorname{Log} \left[ \frac{M_K^2}{\mu^2} \right] c_{\theta}^9 M_0^8 M_K^4 M_{\pi}^2 s_{\theta}}{81 \pi^2 M_{\eta'}^2 M_{\eta'}^8} + \\
& \frac{512 \sqrt{2} c_{\theta}^9 L_6^r M_0^8 M_K^4 M_{\pi}^2 s_{\theta}}{81 M_{\eta'}^2 M_{\eta'}^8} + \frac{896 \sqrt{2} c_{\theta}^9 L_7^r M_0^8 M_K^4 M_{\pi}^2 s_{\theta}}{81 M_{\eta'}^2 M_{\eta'}^8} + \frac{1216 \sqrt{2} c_{\theta}^9 L_{25}^r M_0^8 M_K^4 M_{\pi}^2 s_{\theta}}{81 M_{\eta'}^2 M_{\eta'}^8} + \\
& \frac{1792 \sqrt{2} c_{\theta}^9 C_{19} M_0^8 M_K^6 M_{\pi}^2 s_{\theta}}{81 M_{\eta'}^2 M_{\eta'}^8} + \frac{3584 \sqrt{2} c_{\theta}^9 C_{31} M_0^8 M_K^6 M_{\pi}^2 s_{\theta}}{243 M_{\eta'}^2 M_{\eta'}^8} - \frac{32 \sqrt{2} F^2 v_2^{(2)} c_{\theta}^9 M_0^8 M_{\pi}^4 s_{\theta}}{27 M_{\eta'}^2 M_{\eta'}^8} + \\
& \frac{7 \operatorname{Log} \left[ \frac{M_K^2}{\mu^2} \right] c_{\theta}^9 M_0^8 M_K^2 M_{\pi}^4 s_{\theta}}{972 \sqrt{2} \pi^2 M_{\eta'}^2 M_{\eta'}^8} - \frac{11 \operatorname{Log} \left[ \frac{M_K^2}{\mu^2} \right] c_{\theta}^9 M_0^8 M_K^2 M_{\pi}^4 s_{\theta}}{324 \sqrt{2} \pi^2 M_{\eta'}^2 M_{\eta'}^8} - \frac{128 \sqrt{2} c_{\theta}^9 L_6^r M_0^8 M_K^2 M_{\pi}^4 s_{\theta}}{81 M_{\eta'}^2 M_{\eta'}^8} - \\
& \frac{704 \sqrt{2} c_{\theta}^9 L_7^r M_0^8 M_K^2 M_{\pi}^4 s_{\theta}}{81 M_{\eta'}^2 M_{\eta'}^8} - \frac{1472 \sqrt{2} c_{\theta}^9 L_{25}^r M_0^8 M_K^2 M_{\pi}^4 s_{\theta}}{81 M_{\eta'}^2 M_{\eta'}^8} - \frac{128 \sqrt{2} c_{\theta}^9 C_{19} M_0^8 M_K^4 M_{\pi}^4 s_{\theta}}{9 M_{\eta'}^2 M_{\eta'}^8} - \\
& \frac{256 \sqrt{2} c_{\theta}^9 C_{31} M_0^8 M_K^4 M_{\pi}^4 s_{\theta}}{27 M_{\eta'}^2 M_{\eta'}^8} + \frac{19 \operatorname{Log} \left[ \frac{M_{\pi}^2}{\mu^2} \right] c_{\theta}^9 M_0^8 M_{\pi}^6 s_{\theta}}{648 \sqrt{2} \pi^2 M_{\eta'}^2 M_{\eta'}^8} - \frac{640 \sqrt{2} c_{\theta}^9 L_6^r M_0^8 M_{\pi}^6 s_{\theta}}{243 M_{\eta'}^2 M_{\eta'}^8} - \\
& \frac{64 \sqrt{2} c_{\theta}^9 L_7^r M_0^8 M_{\pi}^6 s_{\theta}}{243 M_{\eta'}^2 M_{\eta'}^8} + \frac{256 \sqrt{2} c_{\theta}^9 L_{25}^r M_0^8 M_{\pi}^6 s_{\theta}}{27 M_{\eta'}^2 M_{\eta'}^8} + \frac{1024 \sqrt{2} c_{\theta}^9 C_{19} M_0^8 M_K^2 M_{\pi}^6 s_{\theta}}{81 M_{\eta'}^2 M_{\eta'}^8} + \\
& \frac{2048 \sqrt{2} c_{\theta}^9 C_{31} M_0^8 M_K^2 M_{\pi}^6 s_{\theta}}{243 M_{\eta'}^2 M_{\eta'}^8} - \frac{640 \sqrt{2} c_{\theta}^9 C_{19} M_0^8 M_{\pi}^8 s_{\theta}}{81 M_{\eta'}^2 M_{\eta'}^8} - \frac{1280 \sqrt{2} c_{\theta}^9 C_{31} M_0^8 M_{\pi}^8 s_{\theta}}{243 M_{\eta'}^2 M_{\eta'}^8} -
\end{aligned}$$



$$\begin{aligned}
& \frac{\text{Log}\left[\frac{M_\eta^2}{\mu^2}\right] c_\theta^9 M_0^8 M_K^2 M_\eta^2 s_\theta}{324 \sqrt{2} \pi^2 M_{\eta'}^8} + \frac{\text{Log}\left[\frac{M_{\eta'}^2}{\mu^2}\right] c_\theta^9 M_0^8 M_\pi^2 M_\eta^2 s_\theta}{648 \sqrt{2} \pi^2 M_{\eta'}^8} - \frac{16 \sqrt{2} F^2 v_2^{(2)} c_\theta^5 M_0^6 M_K^2 s_\theta}{3 M_{\eta'}^6} + \\
& \frac{\text{Log}\left[\frac{M_\eta^2}{\mu^2}\right] c_\theta^9 M_0^8 M_K^2 s_\theta}{243 \sqrt{2} \pi^2 M_{\eta'}^6} - \frac{\text{Log}\left[\frac{M_{\eta'}^2}{\mu^2}\right] c_\theta^9 M_0^8 M_K^2 s_\theta}{324 \sqrt{2} \pi^2 M_{\eta'}^6} + \frac{16 \sqrt{2} F^2 v_2^{(2)} c_\theta^5 M_0^6 M_\pi^2 s_\theta}{3 M_{\eta'}^6} - \\
& \frac{5 \text{Log}\left[\frac{M_\eta^2}{\mu^2}\right] c_\theta^9 M_0^8 M_\pi^2 s_\theta}{1944 \sqrt{2} \pi^2 M_{\eta'}^6} + \frac{\text{Log}\left[\frac{M_{\eta'}^2}{\mu^2}\right] c_\theta^9 M_0^8 M_\pi^2 s_\theta}{324 \sqrt{2} \pi^2 M_{\eta'}^6} - \frac{655 360 \sqrt{2} c_\theta^{11} L_8^2 r M_0^8 M_K^{10} s_\theta}{729 F^2 M_{\eta'}^6 M_{\eta'}^6} + \\
& \frac{532 480 \sqrt{2} c_\theta^{11} L_8^2 r M_0^8 M_K^8 M_\pi^2 s_\theta}{243 F^2 M_{\eta'}^6 M_{\eta'}^6} - \frac{475 136 \sqrt{2} c_\theta^{11} L_8^2 r M_0^8 M_K^6 M_\pi^4 s_\theta}{243 F^2 M_{\eta'}^6 M_{\eta'}^6} + \\
& \frac{569 344 \sqrt{2} c_\theta^{11} L_8^2 r M_0^8 M_K^4 M_\pi^6 s_\theta}{729 F^2 M_{\eta'}^6 M_{\eta'}^6} - \frac{31 744 \sqrt{2} c_\theta^{11} L_8^2 r M_0^8 M_K^2 M_\pi^8 s_\theta}{243 F^2 M_{\eta'}^6 M_{\eta'}^6} + \frac{1024 \sqrt{2} c_\theta^{11} L_8^2 r M_0^8 M_\pi^{10} s_\theta}{81 F^2 M_{\eta'}^6 M_{\eta'}^6} - \\
& \frac{\sqrt{2} \text{Log}\left[\frac{M_K^2}{\mu^2}\right] c_\theta^9 M_0^8 M_K^6 s_\theta}{81 \pi^2 M_{\eta'}^4 M_{\eta'}^6} + \frac{2048 \sqrt{2} c_\theta^9 L_6^r M_0^8 M_K^6 s_\theta}{243 M_{\eta'}^4 M_{\eta'}^6} + \frac{2048 \sqrt{2} c_\theta^9 L_7^r M_0^8 M_K^6 s_\theta}{243 M_{\eta'}^4 M_{\eta'}^6} - \\
& \frac{256 \sqrt{2} c_\theta^9 L_{25}^r M_0^8 M_K^6 s_\theta}{27 M_{\eta'}^4 M_{\eta'}^6} + \frac{4096 \sqrt{2} c_\theta^9 C_{19} M_0^8 M_K^8 s_\theta}{81 M_{\eta'}^4 M_{\eta'}^6} + \frac{8192 \sqrt{2} c_\theta^9 C_{31} M_0^8 M_K^8 s_\theta}{243 M_{\eta'}^4 M_{\eta'}^6} + \\
& \frac{5 \text{Log}\left[\frac{M_K^2}{\mu^2}\right] c_\theta^9 M_0^8 M_K^4 M_\pi^2 s_\theta}{243 \sqrt{2} \pi^2 M_{\eta'}^4 M_{\eta'}^6} - \frac{512 \sqrt{2} c_\theta^9 L_6^r M_0^8 M_K^4 M_\pi^2 s_\theta}{81 M_{\eta'}^4 M_{\eta'}^6} - \frac{896 \sqrt{2} c_\theta^9 L_7^r M_0^8 M_K^4 M_\pi^2 s_\theta}{81 M_{\eta'}^4 M_{\eta'}^6} + \\
& \frac{320 \sqrt{2} c_\theta^9 L_{25}^r M_0^8 M_K^4 M_\pi^2 s_\theta}{27 M_{\eta'}^4 M_{\eta'}^6} - \frac{7936 \sqrt{2} c_\theta^9 C_{19} M_0^8 M_K^6 M_\pi^2 s_\theta}{81 M_{\eta'}^4 M_{\eta'}^6} - \frac{15 872 \sqrt{2} c_\theta^9 C_{31} M_0^8 M_K^6 M_\pi^2 s_\theta}{243 M_{\eta'}^4 M_{\eta'}^6} - \\
& \frac{5 \text{Log}\left[\frac{M_K^2}{\mu^2}\right] c_\theta^9 M_0^8 M_K^2 M_\pi^4 s_\theta}{972 \sqrt{2} \pi^2 M_{\eta'}^4 M_{\eta'}^6} + \frac{5 \text{Log}\left[\frac{M_\pi^2}{\mu^2}\right] c_\theta^9 M_0^8 M_K^2 M_\pi^4 s_\theta}{324 \sqrt{2} \pi^2 M_{\eta'}^4 M_{\eta'}^6} - \frac{256 \sqrt{2} c_\theta^9 L_6^r M_0^8 M_K^2 M_\pi^4 s_\theta}{81 M_{\eta'}^4 M_{\eta'}^6} + \\
& \frac{320 \sqrt{2} c_\theta^9 L_7^r M_0^8 M_K^2 M_\pi^4 s_\theta}{81 M_{\eta'}^4 M_{\eta'}^6} - \frac{64 \sqrt{2} c_\theta^9 L_{25}^r M_0^8 M_K^2 M_\pi^4 s_\theta}{27 M_{\eta'}^4 M_{\eta'}^6} + \frac{640 \sqrt{2} c_\theta^9 C_{19} M_0^8 M_K^4 M_\pi^4 s_\theta}{9 M_{\eta'}^4 M_{\eta'}^6} + \\
& \frac{1280 \sqrt{2} c_\theta^9 C_{31} M_0^8 M_K^4 M_\pi^4 s_\theta}{27 M_{\eta'}^4 M_{\eta'}^6} - \frac{\text{Log}\left[\frac{M_\pi^2}{\mu^2}\right] c_\theta^9 M_0^8 M_\pi^6 s_\theta}{648 \sqrt{2} \pi^2 M_{\eta'}^4 M_{\eta'}^6} + \frac{256 \sqrt{2} c_\theta^9 L_6^r M_0^8 M_\pi^6 s_\theta}{243 M_{\eta'}^4 M_{\eta'}^6} - \\
& \frac{320 \sqrt{2} c_\theta^9 L_7^r M_0^8 M_\pi^6 s_\theta}{243 M_{\eta'}^4 M_{\eta'}^6} - \frac{2176 \sqrt{2} c_\theta^9 C_{19} M_0^8 M_K^2 M_\pi^6 s_\theta}{81 M_{\eta'}^4 M_{\eta'}^6} - \frac{4352 \sqrt{2} c_\theta^9 C_{31} M_0^8 M_K^2 M_\pi^6 s_\theta}{243 M_{\eta'}^4 M_{\eta'}^6} + \\
& \frac{256 \sqrt{2} c_\theta^9 C_{19} M_0^8 M_\pi^8 s_\theta}{81 M_{\eta'}^4 M_{\eta'}^6} + \frac{512 \sqrt{2} c_\theta^9 C_{31} M_0^8 M_\pi^8 s_\theta}{243 M_{\eta'}^4 M_{\eta'}^6} - \frac{8 \sqrt{2} F^2 v_2^{(2)} c_\theta^7 M_0^8 M_K^2 s_\theta}{3 M_{\eta'}^2 M_{\eta'}^6} - \\
& \frac{64 \sqrt{2} F^2 v_2^{(2)} c_\theta^7 M_0^6 M_K^4 s_\theta}{27 M_{\eta'}^2 M_{\eta'}^6} - \frac{c_\theta^7 M_0^8 M_K^4 s_\theta}{162 \sqrt{2} \pi^2 M_{\eta'}^2 M_{\eta'}^6} + \frac{\sqrt{2} c_\theta^7 M_0^8 M_K^4 s_\theta}{81 \pi^2 M_{\eta'}^2 M_{\eta'}^6} + \frac{\sqrt{2} \text{Log}\left[\frac{M_K^2}{\mu^2}\right] c_\theta^7 M_0^8 M_K^4 s_\theta}{81 \pi^2 M_{\eta'}^2 M_{\eta'}^6} +
\end{aligned}$$

$$\begin{aligned}
& \frac{5 c_{\theta}^{11} M_{\theta}^8 M_K^4 s_{\theta}}{243 \sqrt{2} \pi^2 M_{\eta}^2 M_{\eta'}^6} - \frac{2 \sqrt{2} \operatorname{Log}\left[\frac{M_{\eta}^2}{\mu^2}\right] c_{\theta}^{11} M_{\theta}^8 M_K^4 s_{\theta}}{729 \pi^2 M_{\eta}^2 M_{\eta'}^6} + \frac{\operatorname{Log}\left[\frac{M_{\eta'}^2}{\mu^2}\right] c_{\theta}^{11} M_{\theta}^8 M_K^4 s_{\theta}}{243 \sqrt{2} \pi^2 M_{\eta}^2 M_{\eta'}^6} + \\
& \frac{\sqrt{2} \operatorname{Log}\left[\frac{M_{\eta'}^2}{\mu^2}\right] c_{\theta}^{11} M_{\theta}^8 M_K^4 s_{\theta}}{243 \pi^2 M_{\eta}^2 M_{\eta'}^6} - \frac{512 \sqrt{2} c_{\theta}^7 L_6^r M_{\theta}^8 M_K^4 s_{\theta}}{81 M_{\eta}^2 M_{\eta'}^6} - \frac{512 \sqrt{2} c_{\theta}^7 L_7^r M_{\theta}^8 M_K^4 s_{\theta}}{81 M_{\eta}^2 M_{\eta'}^6} - \\
& \frac{1792 \sqrt{2} c_{\theta}^7 C_{19} M_{\theta}^8 M_K^6 s_{\theta}}{27 M_{\eta}^2 M_{\eta'}^6} - \frac{5120 \sqrt{2} c_{\theta}^7 C_{31} M_{\theta}^8 M_K^6 s_{\theta}}{81 M_{\eta}^2 M_{\eta'}^6} + \frac{8 \sqrt{2} F^2 v_2^{(2)} c_{\theta}^7 M_{\theta}^8 M_{\pi}^2 s_{\theta}}{3 M_{\eta}^2 M_{\eta'}^6} + \\
& \frac{32 \sqrt{2} F^2 v_2^{(2)} c_{\theta}^7 M_{\theta}^8 M_K^2 M_{\pi}^2 s_{\theta}}{27 M_{\eta}^2 M_{\eta'}^6} - \frac{c_{\theta}^7 M_{\theta}^8 M_K^2 M_{\pi}^2 s_{\theta}}{108 \sqrt{2} \pi^2 M_{\eta}^2 M_{\eta'}^6} - \frac{\operatorname{Log}\left[\frac{M_K^2}{\mu^2}\right] c_{\theta}^7 M_{\theta}^8 M_K^2 M_{\pi}^2 s_{\theta}}{81 \sqrt{2} \pi^2 M_{\eta}^2 M_{\eta'}^6} - \\
& \frac{2 \sqrt{2} c_{\theta}^{11} M_{\theta}^8 M_K^2 M_{\pi}^2 s_{\theta}}{243 \pi^2 M_{\eta}^2 M_{\eta'}^6} + \frac{55 \operatorname{Log}\left[\frac{M_{\eta}^2}{\mu^2}\right] c_{\theta}^{11} M_{\theta}^8 M_K^2 M_{\pi}^2 s_{\theta}}{2916 \sqrt{2} \pi^2 M_{\eta}^2 M_{\eta'}^6} - \frac{4 \sqrt{2} \operatorname{Log}\left[\frac{M_{\eta'}^2}{\mu^2}\right] c_{\theta}^{11} M_{\theta}^8 M_K^2 M_{\pi}^2 s_{\theta}}{729 \pi^2 M_{\eta}^2 M_{\eta'}^6} - \\
& \frac{\operatorname{Log}\left[\frac{M_{\eta'}^2}{\mu^2}\right] c_{\theta}^{11} M_{\theta}^8 M_K^2 M_{\pi}^2 s_{\theta}}{486 \sqrt{2} \pi^2 M_{\eta}^2 M_{\eta'}^6} - \frac{2 \sqrt{2} \operatorname{Log}\left[\frac{M_{\eta'}^2}{\mu^2}\right] c_{\theta}^{11} M_{\theta}^8 M_K^2 M_{\pi}^2 s_{\theta}}{243 \pi^2 M_{\eta}^2 M_{\eta'}^6} + \frac{256 \sqrt{2} c_{\theta}^7 L_6^r M_{\theta}^8 M_K^2 M_{\pi}^2 s_{\theta}}{81 M_{\eta}^2 M_{\eta'}^6} + \\
& \frac{256 \sqrt{2} c_{\theta}^7 L_7^r M_{\theta}^8 M_K^2 M_{\pi}^2 s_{\theta}}{81 M_{\eta}^2 M_{\eta'}^6} + \frac{896 \sqrt{2} c_{\theta}^7 C_{19} M_{\theta}^8 M_K^4 M_{\pi}^2 s_{\theta}}{9 M_{\eta}^2 M_{\eta'}^6} + \frac{2560 \sqrt{2} c_{\theta}^7 C_{31} M_{\theta}^8 M_K^4 M_{\pi}^2 s_{\theta}}{27 M_{\eta}^2 M_{\eta'}^6} + \\
& \frac{32 \sqrt{2} F^2 v_2^{(2)} c_{\theta}^7 M_{\theta}^8 M_{\pi}^4 s_{\theta}}{27 M_{\eta}^2 M_{\eta'}^6} - \frac{c_{\theta}^7 M_{\theta}^8 M_{\pi}^4 s_{\theta}}{72 \sqrt{2} \pi^2 M_{\eta}^2 M_{\eta'}^6} - \frac{\operatorname{Log}\left[\frac{M_{\pi}^2}{\mu^2}\right] c_{\theta}^7 M_{\theta}^8 M_{\pi}^4 s_{\theta}}{54 \sqrt{2} \pi^2 M_{\eta}^2 M_{\eta'}^6} + \frac{c_{\theta}^{11} M_{\theta}^8 M_{\pi}^4 s_{\theta}}{1944 \sqrt{2} \pi^2 M_{\eta}^2 M_{\eta'}^6} - \\
& \frac{7 \operatorname{Log}\left[\frac{M_{\eta'}^2}{\mu^2}\right] c_{\theta}^{11} M_{\theta}^8 M_{\pi}^4 s_{\theta}}{2916 \sqrt{2} \pi^2 M_{\eta}^2 M_{\eta'}^6} - \frac{\operatorname{Log}\left[\frac{M_{\eta'}^2}{\mu^2}\right] c_{\theta}^{11} M_{\theta}^8 M_{\pi}^4 s_{\theta}}{486 \sqrt{2} \pi^2 M_{\eta}^2 M_{\eta'}^6} + \frac{\sqrt{2} \operatorname{Log}\left[\frac{M_{\eta'}^2}{\mu^2}\right] c_{\theta}^{11} M_{\theta}^8 M_{\pi}^4 s_{\theta}}{243 \pi^2 M_{\eta}^2 M_{\eta'}^6} + \\
& \frac{256 \sqrt{2} c_{\theta}^7 L_6^r M_{\theta}^8 M_{\pi}^4 s_{\theta}}{81 M_{\eta}^2 M_{\eta'}^6} + \frac{256 \sqrt{2} c_{\theta}^7 L_7^r M_{\theta}^8 M_{\pi}^4 s_{\theta}}{81 M_{\eta}^2 M_{\eta'}^6} - \frac{448 \sqrt{2} c_{\theta}^7 C_{19} M_{\theta}^8 M_K^2 M_{\pi}^4 s_{\theta}}{9 M_{\eta}^2 M_{\eta'}^6} - \\
& \frac{1280 \sqrt{2} c_{\theta}^7 C_{31} M_{\theta}^8 M_K^2 M_{\pi}^4 s_{\theta}}{27 M_{\eta}^2 M_{\eta'}^6} + \frac{448 \sqrt{2} c_{\theta}^7 C_{19} M_{\theta}^8 M_{\pi}^6 s_{\theta}}{27 M_{\eta}^2 M_{\eta'}^6} + \frac{1280 \sqrt{2} c_{\theta}^7 C_{31} M_{\theta}^8 M_{\pi}^6 s_{\theta}}{81 M_{\eta}^2 M_{\eta'}^6} + \\
& \frac{8 \sqrt{2} F^2 v_2^{(2)} c_{\theta}^3 M_{\theta}^4 M_K^2 s_{\theta}}{3 M_{\eta'}^4} - \frac{8 \sqrt{2} F^2 v_2^{(2)} c_{\theta}^3 M_{\theta}^4 M_{\pi}^2 s_{\theta}}{3 M_{\eta'}^4} - \frac{4 \sqrt{2} \operatorname{Log}\left[\frac{M_{\eta'}^2}{\mu^2}\right] c_{\theta}^{11} M_{\theta}^8 M_K^4 s_{\theta}}{729 \pi^2 M_{\eta}^4 M_{\eta'}^4} + \\
& \frac{5 \sqrt{2} \operatorname{Log}\left[\frac{M_{\eta'}^2}{\mu^2}\right] c_{\theta}^{11} M_{\theta}^8 M_K^2 M_{\pi}^2 s_{\theta}}{729 \pi^2 M_{\eta}^4 M_{\eta'}^4} - \frac{\sqrt{2} \operatorname{Log}\left[\frac{M_{\eta'}^2}{\mu^2}\right] c_{\theta}^{11} M_{\theta}^8 M_{\pi}^4 s_{\theta}}{729 \pi^2 M_{\eta}^4 M_{\eta'}^4} + \frac{\operatorname{Log}\left[\frac{M_{\eta'}^2}{\mu^2}\right] c_{\theta}^9 M_{\theta}^8 M_K^2 s_{\theta}}{486 \sqrt{2} \pi^2 M_{\eta}^2 M_{\eta'}^4} - \\
& \frac{\operatorname{Log}\left[\frac{M_{\eta'}^2}{\mu^2}\right] c_{\theta}^9 M_{\theta}^8 M_{\pi}^2 s_{\theta}}{486 \sqrt{2} \pi^2 M_{\eta}^2 M_{\eta'}^4} - \frac{8 \sqrt{2} F^2 v_2^{(2)} c_{\theta}^3 M_{\theta}^4 M_K^2 s_{\theta}}{3 M_{\eta}^2 M_{\eta'}^2} + \frac{8 \sqrt{2} F^2 v_2^{(2)} c_{\theta}^3 M_{\theta}^4 M_{\pi}^2 s_{\theta}}{3 M_{\eta}^2 M_{\eta'}^2} -
\end{aligned}$$

$$\begin{aligned}
& \frac{5 \operatorname{Log}\left[\frac{M_\eta^2}{\mu^2}\right] c_\theta^{11} M_\theta^8 M_K^4 M_\eta^2 s_\theta}{243 \sqrt{2} \pi^2 M_{\eta'}^8 (M_\eta^2 - M_{\eta'}^2)} + \frac{7 \operatorname{Log}\left[\frac{M_\eta^2}{\mu^2}\right] c_\theta^{11} M_\theta^8 M_K^2 M_\pi^2 M_\eta^2 s_\theta}{243 \sqrt{2} \pi^2 M_{\eta'}^8 (M_\eta^2 - M_{\eta'}^2)} - \frac{\sqrt{2} \operatorname{Log}\left[\frac{M_\eta^2}{\mu^2}\right] c_\theta^{11} M_\theta^8 M_\pi^4 M_\eta^2 s_\theta}{243 \pi^2 M_{\eta'}^8 (M_\eta^2 - M_{\eta'}^2)} + \\
& \frac{2 \sqrt{2} \operatorname{Log}\left[\frac{M_\eta^2}{\mu^2}\right] c_\theta^{11} M_\theta^8 M_K^4 s_\theta}{243 \pi^2 M_{\eta'}^6 (M_\eta^2 - M_{\eta'}^2)} + \frac{5 \operatorname{Log}\left[\frac{M_\eta^2}{\mu^2}\right] c_\theta^{11} M_\theta^8 M_K^4 s_\theta}{243 \sqrt{2} \pi^2 M_{\eta'}^6 (M_\eta^2 - M_{\eta'}^2)} - \frac{5 \operatorname{Log}\left[\frac{M_\eta^2}{\mu^2}\right] c_\theta^{11} M_\theta^8 M_K^2 M_\pi^2 s_\theta}{243 \sqrt{2} \pi^2 M_{\eta'}^6 (M_\eta^2 - M_{\eta'}^2)} - \\
& \frac{7 \operatorname{Log}\left[\frac{M_\eta^2}{\mu^2}\right] c_\theta^{11} M_\theta^8 M_K^2 M_\pi^2 s_\theta}{243 \sqrt{2} \pi^2 M_{\eta'}^6 (M_\eta^2 - M_{\eta'}^2)} + \frac{\operatorname{Log}\left[\frac{M_\eta^2}{\mu^2}\right] c_\theta^{11} M_\theta^8 M_\pi^4 s_\theta}{243 \sqrt{2} \pi^2 M_{\eta'}^6 (M_\eta^2 - M_{\eta'}^2)} + \frac{\sqrt{2} \operatorname{Log}\left[\frac{M_\eta^2}{\mu^2}\right] c_\theta^{11} M_\theta^8 M_\pi^4 s_\theta}{243 \pi^2 M_{\eta'}^6 (M_\eta^2 - M_{\eta'}^2)} - \\
& \frac{2 \sqrt{2} \operatorname{Log}\left[\frac{M_\eta^2}{\mu^2}\right] c_\theta^{11} M_\theta^8 M_K^4 s_\theta}{243 \pi^2 M_\eta^2 M_{\eta'}^4 (M_\eta^2 - M_{\eta'}^2)} + \frac{5 \operatorname{Log}\left[\frac{M_\eta^2}{\mu^2}\right] c_\theta^{11} M_\theta^8 M_K^2 M_\pi^2 s_\theta}{243 \sqrt{2} \pi^2 M_\eta^2 M_{\eta'}^4 (M_\eta^2 - M_{\eta'}^2)} - \frac{\operatorname{Log}\left[\frac{M_\eta^2}{\mu^2}\right] c_\theta^{11} M_\theta^8 M_\pi^4 s_\theta}{243 \sqrt{2} \pi^2 M_\eta^2 M_{\eta'}^4 (M_\eta^2 - M_{\eta'}^2)} - \\
& \frac{8 F^2 v_2^{(2)} c_\theta^2 M_\theta^4 M_K^2 s_\theta^2}{3 M_\eta^4} + \frac{2 F^2 v_2^{(2)} c_\theta^2 M_\theta^4 M_\pi^2 s_\theta^2}{3 M_\eta^4} + \frac{24 F^2 v_4^{(0)} M_\theta^2 s_\theta^2}{M_\eta^2} - \frac{2 \, 293 \, 760 c_\theta^{10} L_8^2 r M_\theta^8 M_K^{10} s_\theta^2}{729 F^2 M_{\eta'}^{12}} + \\
& \frac{1 \, 925 \, 120 c_\theta^{10} L_8^2 r M_\theta^8 M_K^8 M_\pi^2 s_\theta^2}{243 F^2 M_{\eta'}^{12}} - \frac{2 \, 191 \, 360 c_\theta^{10} L_8^2 r M_\theta^8 M_K^6 M_\pi^4 s_\theta^2}{243 F^2 M_{\eta'}^{12}} + \frac{4 \, 167 \, 680 c_\theta^{10} L_8^2 r M_\theta^8 M_K^4 M_\pi^6 s_\theta^2}{729 F^2 M_{\eta'}^{12}} - \\
& \frac{465 \, 920 c_\theta^{10} L_8^2 r M_\theta^8 M_K^2 M_\pi^8 s_\theta^2}{243 F^2 M_{\eta'}^{12}} + \frac{5120 c_\theta^{10} L_8^2 r M_\theta^8 M_\pi^{10} s_\theta^2}{81 F^2 M_{\eta'}^{12}} + \frac{64 F^2 v_2^{(2)} c_\theta^8 M_\theta^8 M_K^4 s_\theta^2}{9 M_{\eta'}^{10}} - \\
& \frac{20 \operatorname{Log}\left[\frac{M_K^2}{\mu^2}\right] c_\theta^8 M_\theta^8 M_K^6 s_\theta^2}{243 \pi^2 M_{\eta'}^{10}} + \frac{2560 c_\theta^8 L_6^r M_\theta^8 M_K^6 s_\theta^2}{81 M_{\eta'}^{10}} + \frac{2560 c_\theta^8 L_7^r M_\theta^8 M_K^6 s_\theta^2}{81 M_{\eta'}^{10}} - \frac{5120 c_\theta^8 L_{25}^r M_\theta^8 M_K^6 s_\theta^2}{81 M_{\eta'}^{10}} + \\
& \frac{5120 c_\theta^8 C_{19} M_\theta^8 M_K^8 s_\theta^2}{27 M_{\eta'}^{10}} + \frac{10 \, 240 c_\theta^8 C_{31} M_\theta^8 M_K^8 s_\theta^2}{81 M_{\eta'}^{10}} + \frac{16 F^2 v_2^{(2)} c_\theta^8 M_\theta^8 M_K^2 M_\pi^2 s_\theta^2}{9 M_{\eta'}^{10}} + \\
& \frac{61 \operatorname{Log}\left[\frac{M_K^2}{\mu^2}\right] c_\theta^8 M_\theta^8 M_K^4 M_\pi^2 s_\theta^2}{972 \pi^2 M_{\eta'}^{10}} - \frac{128 c_\theta^8 L_6^r M_\theta^8 M_K^4 M_\pi^2 s_\theta^2}{9 M_{\eta'}^{10}} - \frac{512 c_\theta^8 L_7^r M_\theta^8 M_K^4 M_\pi^2 s_\theta^2}{27 M_{\eta'}^{10}} + \\
& \frac{7936 c_\theta^8 L_{25}^r M_\theta^8 M_K^4 M_\pi^2 s_\theta^2}{81 M_{\eta'}^{10}} - \frac{3584 c_\theta^8 C_{19} M_\theta^8 M_K^6 M_\pi^2 s_\theta^2}{9 M_{\eta'}^{10}} - \frac{7168 c_\theta^8 C_{31} M_\theta^8 M_K^6 M_\pi^2 s_\theta^2}{27 M_{\eta'}^{10}} - \\
& \frac{8 F^2 v_2^{(2)} c_\theta^8 M_\theta^8 M_\pi^4 s_\theta^2}{9 M_{\eta'}^{10}} - \frac{31 \operatorname{Log}\left[\frac{M_K^2}{\mu^2}\right] c_\theta^8 M_\theta^8 M_K^2 M_\pi^4 s_\theta^2}{1944 \pi^2 M_{\eta'}^{10}} - \frac{\operatorname{Log}\left[\frac{M_K^2}{\mu^2}\right] c_\theta^8 M_\theta^8 M_K^2 M_\pi^4 s_\theta^2}{72 \pi^2 M_{\eta'}^{10}} - \\
& \frac{5120 c_\theta^8 L_{25}^r M_\theta^8 M_K^2 M_\pi^4 s_\theta^2}{81 M_{\eta'}^{10}} + \frac{2816 c_\theta^8 C_{19} M_\theta^8 M_K^4 M_\pi^4 s_\theta^2}{9 M_{\eta'}^{10}} + \frac{5632 c_\theta^8 C_{31} M_\theta^8 M_K^4 M_\pi^4 s_\theta^2}{27 M_{\eta'}^{10}} - \\
& \frac{7 \operatorname{Log}\left[\frac{M_\pi^2}{\mu^2}\right] c_\theta^8 M_\theta^8 M_\pi^6 s_\theta^2}{432 \pi^2 M_{\eta'}^{10}} + \frac{608 c_\theta^8 L_6^r M_\theta^8 M_\pi^6 s_\theta^2}{81 M_{\eta'}^{10}} + \frac{704 c_\theta^8 L_7^r M_\theta^8 M_\pi^6 s_\theta^2}{81 M_{\eta'}^{10}} + \frac{64 c_\theta^8 L_{25}^r M_\theta^8 M_\pi^6 s_\theta^2}{9 M_{\eta'}^{10}} - \\
& \frac{2752 c_\theta^8 C_{19} M_\theta^8 M_K^2 M_\pi^6 s_\theta^2}{27 M_{\eta'}^{10}} - \frac{5504 c_\theta^8 C_{31} M_\theta^8 M_K^2 M_\pi^6 s_\theta^2}{81 M_{\eta'}^{10}} + \frac{608 c_\theta^8 C_{19} M_\theta^8 M_\pi^8 s_\theta^2}{27 M_{\eta'}^{10}} + \frac{1216 c_\theta^8 C_{31} M_\theta^8 M_\pi^8 s_\theta^2}{81 M_{\eta'}^{10}} -
\end{aligned}$$

$$\begin{aligned}
& \frac{901\,120\,c_{\theta}^{10}\,L_8^2\,r\,M_0^8\,M_K^{10}\,s_{\theta}^2}{729\,F^2\,M_{\eta'}^2\,M_{\eta'}^{10}} + \frac{8192\,c_{\theta}^{10}\,L_8^2\,r\,M_0^8\,M_K^8\,M_{\pi}^2\,s_{\theta}^2}{3\,F^2\,M_{\eta'}^2\,M_{\eta'}^{10}} - \frac{16\,384\,c_{\theta}^{10}\,L_8^2\,r\,M_0^8\,M_K^6\,M_{\pi}^4\,s_{\theta}^2}{243\,F^2\,M_{\eta'}^2\,M_{\eta'}^{10}} - \\
& \frac{2\,121\,728\,c_{\theta}^{10}\,L_8^2\,r\,M_0^8\,M_K^4\,M_{\pi}^6\,s_{\theta}^2}{729\,F^2\,M_{\eta'}^2\,M_{\eta'}^{10}} + \frac{452\,608\,c_{\theta}^{10}\,L_8^2\,r\,M_0^8\,M_K^2\,M_{\pi}^8\,s_{\theta}^2}{243\,F^2\,M_{\eta'}^2\,M_{\eta'}^{10}} - \frac{4096\,c_{\theta}^{10}\,L_8^2\,r\,M_0^8\,M_{\pi}^{10}\,s_{\theta}^2}{27\,F^2\,M_{\eta'}^2\,M_{\eta'}^{10}} - \\
& \frac{37\,\text{Log}\left[\frac{M_{\eta'}^2}{\mu^2}\right]\,c_{\theta}^{10}\,M_0^8\,M_K^4\,M_{\pi}^2\,s_{\theta}^2}{1458\,\pi^2\,M_{\eta'}^{10}} + \frac{131\,\text{Log}\left[\frac{M_{\eta'}^2}{\mu^2}\right]\,c_{\theta}^{10}\,M_0^8\,M_K^2\,M_{\pi}^2\,M_{\eta'}^2\,s_{\theta}^2}{5832\,\pi^2\,M_{\eta'}^{10}} - \frac{47\,\text{Log}\left[\frac{M_{\eta'}^2}{\mu^2}\right]\,c_{\theta}^{10}\,M_0^8\,M_{\pi}^4\,M_{\eta'}^2\,s_{\theta}^2}{11\,664\,\pi^2\,M_{\eta'}^{10}} - \\
& \frac{8\,F^2\,v_2^{(2)}\,c_{\theta}^6\,M_0^8\,M_K^2\,s_{\theta}^2}{3\,M_{\eta'}^8} - \frac{64\,F^2\,v_2^{(2)}\,c_{\theta}^6\,M_0^6\,M_K^4\,s_{\theta}^2}{9\,M_{\eta'}^8} + \frac{c_{\theta}^6\,M_0^8\,M_K^4\,s_{\theta}^2}{108\,\pi^2\,M_{\eta'}^8} + \frac{\text{Log}\left[\frac{M_K^2}{\mu^2}\right]\,c_{\theta}^6\,M_0^8\,M_K^4\,s_{\theta}^2}{108\,\pi^2\,M_{\eta'}^8} + \\
& \frac{13\,c_{\theta}^{10}\,M_0^8\,M_K^4\,s_{\theta}^2}{486\,\pi^2\,M_{\eta'}^8} + \frac{19\,\text{Log}\left[\frac{M_{\eta'}^2}{\mu^2}\right]\,c_{\theta}^{10}\,M_0^8\,M_K^4\,s_{\theta}^2}{486\,\pi^2\,M_{\eta'}^8} - \frac{7\,\text{Log}\left[\frac{M_{\eta'}^2}{\mu^2}\right]\,c_{\theta}^{10}\,M_0^8\,M_K^4\,s_{\theta}^2}{729\,\pi^2\,M_{\eta'}^8} - \frac{512\,c_{\theta}^6\,L_7^r\,M_0^8\,M_K^4\,s_{\theta}^2}{27\,M_{\eta'}^8} - \\
& \frac{512\,c_{\theta}^6\,L_7^r\,M_0^8\,M_K^4\,s_{\theta}^2}{27\,M_{\eta'}^8} - \frac{1792\,c_{\theta}^6\,C_{19}\,M_0^8\,M_K^6\,s_{\theta}^2}{9\,M_{\eta'}^8} - \frac{5120\,c_{\theta}^6\,C_{31}\,M_0^8\,M_K^6\,s_{\theta}^2}{27\,M_{\eta'}^8} + \frac{2\,F^2\,v_2^{(2)}\,c_{\theta}^6\,M_0^8\,M_{\pi}^2\,s_{\theta}^2}{3\,M_{\eta'}^8} - \\
& \frac{16\,F^2\,v_2^{(2)}\,c_{\theta}^6\,M_0^6\,M_K^2\,M_{\pi}^2\,s_{\theta}^2}{9\,M_{\eta'}^8} - \frac{5\,c_{\theta}^6\,M_0^8\,M_K^2\,M_{\pi}^2\,s_{\theta}^2}{432\,\pi^2\,M_{\eta'}^8} - \frac{\text{Log}\left[\frac{M_K^2}{\mu^2}\right]\,c_{\theta}^6\,M_0^8\,M_K^2\,M_{\pi}^2\,s_{\theta}^2}{72\,\pi^2\,M_{\eta'}^8} - \frac{7\,c_{\theta}^{10}\,M_0^8\,M_K^2\,M_{\pi}^2\,s_{\theta}^2}{243\,\pi^2\,M_{\eta'}^8} - \\
& \frac{10\,\text{Log}\left[\frac{M_{\eta'}^2}{\mu^2}\right]\,c_{\theta}^{10}\,M_0^8\,M_K^2\,M_{\pi}^2\,s_{\theta}^2}{243\,\pi^2\,M_{\eta'}^8} + \frac{29\,\text{Log}\left[\frac{M_{\eta'}^2}{\mu^2}\right]\,c_{\theta}^{10}\,M_0^8\,M_K^2\,M_{\pi}^2\,s_{\theta}^2}{2916\,\pi^2\,M_{\eta'}^8} + \frac{448\,c_{\theta}^6\,L_6^r\,M_0^8\,M_K^2\,M_{\pi}^2\,s_{\theta}^2}{27\,M_{\eta'}^8} + \\
& \frac{448\,c_{\theta}^6\,L_7^r\,M_0^8\,M_K^2\,M_{\pi}^2\,s_{\theta}^2}{27\,M_{\eta'}^8} + \frac{896\,c_{\theta}^6\,C_{19}\,M_0^8\,M_K^4\,M_{\pi}^2\,s_{\theta}^2}{3\,M_{\eta'}^8} + \frac{2560\,c_{\theta}^6\,C_{31}\,M_0^8\,M_K^4\,M_{\pi}^2\,s_{\theta}^2}{9\,M_{\eta'}^8} + \frac{8\,F^2\,v_2^{(2)}\,c_{\theta}^6\,M_0^6\,M_{\pi}^4\,s_{\theta}^2}{9\,M_{\eta'}^8} + \\
& \frac{11\,c_{\theta}^6\,M_0^8\,M_{\pi}^4\,s_{\theta}^2}{864\,\pi^2\,M_{\eta'}^8} + \frac{\text{Log}\left[\frac{M_K^2}{\mu^2}\right]\,c_{\theta}^6\,M_0^8\,M_{\pi}^4\,s_{\theta}^2}{432\,\pi^2\,M_{\eta'}^8} + \frac{\text{Log}\left[\frac{M_{\pi}^2}{\mu^2}\right]\,c_{\theta}^6\,M_0^8\,M_{\pi}^4\,s_{\theta}^2}{72\,\pi^2\,M_{\eta'}^8} + \frac{115\,c_{\theta}^{10}\,M_0^8\,M_{\pi}^4\,s_{\theta}^2}{7776\,\pi^2\,M_{\eta'}^8} + \\
& \frac{79\,\text{Log}\left[\frac{M_{\eta'}^2}{\mu^2}\right]\,c_{\theta}^{10}\,M_0^8\,M_{\pi}^4\,s_{\theta}^2}{7776\,\pi^2\,M_{\eta'}^8} - \frac{29\,\text{Log}\left[\frac{M_{\eta'}^2}{\mu^2}\right]\,c_{\theta}^{10}\,M_0^8\,M_{\pi}^4\,s_{\theta}^2}{5832\,\pi^2\,M_{\eta'}^8} - \frac{224\,c_{\theta}^6\,L_6^r\,M_0^8\,M_{\pi}^4\,s_{\theta}^2}{27\,M_{\eta'}^8} - \frac{224\,c_{\theta}^6\,L_7^r\,M_0^8\,M_{\pi}^4\,s_{\theta}^2}{27\,M_{\eta'}^8} - \\
& \frac{448\,c_{\theta}^6\,C_{19}\,M_0^8\,M_K^2\,M_{\pi}^4\,s_{\theta}^2}{3\,M_{\eta'}^8} - \frac{1280\,c_{\theta}^6\,C_{31}\,M_0^8\,M_K^2\,M_{\pi}^4\,s_{\theta}^2}{9\,M_{\eta'}^8} + \frac{112\,c_{\theta}^6\,C_{19}\,M_0^8\,M_{\pi}^6\,s_{\theta}^2}{9\,M_{\eta'}^8} + \frac{320\,c_{\theta}^6\,C_{31}\,M_0^8\,M_{\pi}^6\,s_{\theta}^2}{27\,M_{\eta'}^8} + \\
& \frac{4\,259\,840\,c_{\theta}^{10}\,L_8^2\,r\,M_0^8\,M_K^{10}\,s_{\theta}^2}{729\,F^2\,M_{\eta'}^4\,M_{\eta'}^8} - \frac{3\,485\,696\,c_{\theta}^{10}\,L_8^2\,r\,M_0^8\,M_K^8\,M_{\pi}^2\,s_{\theta}^2}{243\,F^2\,M_{\eta'}^4\,M_{\eta'}^8} + \frac{987\,136\,c_{\theta}^{10}\,L_8^2\,r\,M_0^8\,M_K^6\,M_{\pi}^4\,s_{\theta}^2}{81\,F^2\,M_{\eta'}^4\,M_{\eta'}^8} - \\
& \frac{2\,846\,720\,c_{\theta}^{10}\,L_8^2\,r\,M_0^8\,M_K^4\,M_{\pi}^6\,s_{\theta}^2}{729\,F^2\,M_{\eta'}^4\,M_{\eta'}^8} + \frac{71\,680\,c_{\theta}^{10}\,L_8^2\,r\,M_0^8\,M_K^2\,M_{\pi}^8\,s_{\theta}^2}{243\,F^2\,M_{\eta'}^4\,M_{\eta'}^8} - \frac{1280\,c_{\theta}^{10}\,L_8^2\,r\,M_0^8\,M_{\pi}^{10}\,s_{\theta}^2}{27\,F^2\,M_{\eta'}^4\,M_{\eta'}^8} - \\
& \frac{304\,F^2\,v_2^{(2)}\,c_{\theta}^8\,M_0^8\,M_K^4\,s_{\theta}^2}{27\,M_{\eta'}^2\,M_{\eta'}^8} + \frac{\text{Log}\left[\frac{M_K^2}{\mu^2}\right]\,c_{\theta}^8\,M_0^8\,M_K^6\,s_{\theta}^2}{9\,\pi^2\,M_{\eta'}^2\,M_{\eta'}^8} - \frac{256\,c_{\theta}^8\,L_6^r\,M_0^8\,M_K^6\,s_{\theta}^2}{9\,M_{\eta'}^2\,M_{\eta'}^8} - \frac{256\,c_{\theta}^8\,L_7^r\,M_0^8\,M_K^6\,s_{\theta}^2}{9\,M_{\eta'}^2\,M_{\eta'}^8} + \\
& \frac{256\,c_{\theta}^8\,L_{25}^r\,M_0^8\,M_K^6\,s_{\theta}^2}{3\,M_{\eta'}^2\,M_{\eta'}^8} - \frac{512\,c_{\theta}^8\,C_{19}\,M_0^8\,M_K^8\,s_{\theta}^2}{3\,M_{\eta'}^2\,M_{\eta'}^8} - \frac{1024\,c_{\theta}^8\,C_{31}\,M_0^8\,M_K^8\,s_{\theta}^2}{9\,M_{\eta'}^2\,M_{\eta'}^8} - \frac{16\,F^2\,v_2^{(2)}\,c_{\theta}^8\,M_0^8\,M_K^2\,M_{\pi}^2\,s_{\theta}^2}{27\,M_{\eta'}^2\,M_{\eta'}^8} -
\end{aligned}$$

$$\begin{aligned}
& \frac{29 \operatorname{Log}\left[\frac{M_K^2}{\mu^2}\right] c_\theta^8 M_\theta^8 M_K^4 M_\pi^2 s_\theta^2}{324 \pi^2 M_\eta^2 M_{\eta'}^8} + \frac{1280 c_\theta^8 L_6^r M_\theta^8 M_K^4 M_\pi^2 s_\theta^2}{81 M_\eta^2 M_{\eta'}^8} - \frac{256 c_\theta^8 L_7^r M_\theta^8 M_K^4 M_\pi^2 s_\theta^2}{81 M_\eta^2 M_{\eta'}^8} - \\
& \frac{3904 c_\theta^8 L_{25}^r M_\theta^8 M_K^4 M_\pi^2 s_\theta^2}{27 M_\eta^2 M_{\eta'}^8} + \frac{11008 c_\theta^8 C_{19} M_\theta^8 M_K^6 M_\pi^2 s_\theta^2}{27 M_\eta^2 M_{\eta'}^8} + \frac{22016 c_\theta^8 C_{31} M_\theta^8 M_K^6 M_\pi^2 s_\theta^2}{81 M_\eta^2 M_{\eta'}^8} + \\
& \frac{68 F^2 v_2^{(2)} c_\theta^8 M_\theta^8 M_\pi^4 s_\theta^2}{27 M_\eta^2 M_{\eta'}^8} + \frac{\operatorname{Log}\left[\frac{M_K^2}{\mu^2}\right] c_\theta^8 M_\theta^8 M_K^2 M_\pi^4 s_\theta^2}{54 \pi^2 M_\eta^2 M_{\eta'}^8} + \frac{\operatorname{Log}\left[\frac{M_\pi^2}{\mu^2}\right] c_\theta^8 M_\theta^8 M_K^2 M_\pi^4 s_\theta^2}{36 \pi^2 M_\eta^2 M_{\eta'}^8} - \frac{64 c_\theta^8 L_6^r M_\theta^8 M_K^4 M_\pi^4 s_\theta^2}{81 M_\eta^2 M_{\eta'}^8} + \\
& \frac{1664 c_\theta^8 L_7^r M_\theta^8 M_K^4 M_\pi^4 s_\theta^2}{81 M_\eta^2 M_{\eta'}^8} + \frac{2816 c_\theta^8 L_{25}^r M_\theta^8 M_K^4 M_\pi^4 s_\theta^2}{27 M_\eta^2 M_{\eta'}^8} - \frac{3200 c_\theta^8 C_{19} M_\theta^8 M_K^4 M_\pi^4 s_\theta^2}{9 M_\eta^2 M_{\eta'}^8} - \\
& \frac{6400 c_\theta^8 C_{31} M_\theta^8 M_K^4 M_\pi^4 s_\theta^2}{27 M_\eta^2 M_{\eta'}^8} + \frac{\operatorname{Log}\left[\frac{M_\pi^2}{\mu^2}\right] c_\theta^8 M_\theta^8 M_\pi^6 s_\theta^2}{108 \pi^2 M_\eta^2 M_{\eta'}^8} - \frac{640 c_\theta^8 L_6^r M_\theta^8 M_\pi^6 s_\theta^2}{81 M_\eta^2 M_{\eta'}^8} - \frac{1120 c_\theta^8 L_7^r M_\theta^8 M_\pi^6 s_\theta^2}{81 M_\eta^2 M_{\eta'}^8} - \\
& \frac{544 c_\theta^8 L_{25}^r M_\theta^8 M_\pi^6 s_\theta^2}{27 M_\eta^2 M_{\eta'}^8} + \frac{1088 c_\theta^8 C_{19} M_\theta^8 M_K^2 M_\pi^6 s_\theta^2}{9 M_\eta^2 M_{\eta'}^8} + \frac{2176 c_\theta^8 C_{31} M_\theta^8 M_K^2 M_\pi^6 s_\theta^2}{27 M_\eta^2 M_{\eta'}^8} - \frac{640 c_\theta^8 C_{19} M_\theta^8 M_\pi^8 s_\theta^2}{27 M_\eta^2 M_{\eta'}^8} - \\
& \frac{1280 c_\theta^8 C_{31} M_\theta^8 M_\pi^8 s_\theta^2}{81 M_\eta^2 M_{\eta'}^8} + \frac{\operatorname{Log}\left[\frac{M_\eta^2}{\mu^2}\right] c_\theta^8 M_\theta^8 M_K^2 M_\eta^2 s_\theta^2}{432 \pi^2 M_{\eta'}^8} - \frac{\operatorname{Log}\left[\frac{M_\eta^2}{\mu^2}\right] c_\theta^8 M_\theta^8 M_\pi^2 M_\eta^2 s_\theta^2}{648 \pi^2 M_{\eta'}^8} + \\
& \frac{16 F^2 v_2^{(2)} c_\theta^4 M_\theta^6 M_K^2 s_\theta^2}{3 M_{\eta'}^6} - \frac{\operatorname{Log}\left[\frac{M_\eta^2}{\mu^2}\right] c_\theta^8 M_\theta^8 M_K^2 s_\theta^2}{162 \pi^2 M_{\eta'}^6} + \frac{5 \operatorname{Log}\left[\frac{M_{\eta'}^2}{\mu^2}\right] c_\theta^8 M_\theta^8 M_K^2 s_\theta^2}{648 \pi^2 M_{\eta'}^6} - \frac{4 F^2 v_2^{(2)} c_\theta^4 M_\theta^6 M_\pi^2 s_\theta^2}{3 M_{\eta'}^6} + \\
& \frac{5 \operatorname{Log}\left[\frac{M_\eta^2}{\mu^2}\right] c_\theta^8 M_\theta^8 M_\pi^2 s_\theta^2}{1296 \pi^2 M_{\eta'}^6} - \frac{5 \operatorname{Log}\left[\frac{M_{\eta'}^2}{\mu^2}\right] c_\theta^8 M_\theta^8 M_\pi^2 s_\theta^2}{2592 \pi^2 M_{\eta'}^6} - \frac{1310720 c_\theta^{10} L_8^2 r M_\theta^8 M_K^{10} s_\theta^2}{729 F^2 M_\eta^6 M_{\eta'}^6} + \\
& \frac{40960 c_\theta^{10} L_8^2 r M_\theta^8 M_K^8 M_\pi^2 s_\theta^2}{9 F^2 M_\eta^6 M_{\eta'}^6} - \frac{999424 c_\theta^{10} L_8^2 r M_\theta^8 M_K^6 M_\pi^4 s_\theta^2}{243 F^2 M_\eta^6 M_{\eta'}^6} + \frac{1323008 c_\theta^{10} L_8^2 r M_\theta^8 M_K^4 M_\pi^6 s_\theta^2}{729 F^2 M_\eta^6 M_{\eta'}^6} - \\
& \frac{44032 c_\theta^{10} L_8^2 r M_\theta^8 M_K^8 M_\pi^2 s_\theta^2}{81 F^2 M_\eta^6 M_{\eta'}^6} + \frac{1024 c_\theta^{10} L_8^2 r M_\theta^8 M_\pi^{10} s_\theta^2}{81 F^2 M_\eta^6 M_{\eta'}^6} + \frac{64 F^2 v_2^{(2)} c_\theta^8 M_\theta^8 M_K^4 s_\theta^2}{9 M_\eta^4 M_{\eta'}^6} - \\
& \frac{11 \operatorname{Log}\left[\frac{M_K^2}{\mu^2}\right] c_\theta^8 M_\theta^8 M_K^6 s_\theta^2}{243 \pi^2 M_\eta^4 M_{\eta'}^6} - \frac{1024 c_\theta^8 L_6^r M_\theta^8 M_K^6 s_\theta^2}{81 M_\eta^4 M_{\eta'}^6} - \frac{1024 c_\theta^8 L_7^r M_\theta^8 M_K^6 s_\theta^2}{81 M_\eta^4 M_{\eta'}^6} - \frac{2816 c_\theta^8 L_{25}^r M_\theta^8 M_K^6 s_\theta^2}{81 M_\eta^4 M_{\eta'}^6} - \\
& \frac{2048 c_\theta^8 C_{19} M_\theta^8 M_K^8 s_\theta^2}{27 M_\eta^4 M_{\eta'}^6} - \frac{4096 c_\theta^8 C_{31} M_\theta^8 M_K^8 s_\theta^2}{81 M_\eta^4 M_{\eta'}^6} + \frac{16 F^2 v_2^{(2)} c_\theta^8 M_\theta^8 M_K^2 M_\pi^2 s_\theta^2}{9 M_\eta^4 M_{\eta'}^6} + \\
& \frac{13 \operatorname{Log}\left[\frac{M_K^2}{\mu^2}\right] c_\theta^8 M_\theta^8 M_K^4 M_\pi^2 s_\theta^2}{972 \pi^2 M_\eta^4 M_{\eta'}^6} + \frac{128 c_\theta^8 L_6^r M_\theta^8 M_K^4 M_\pi^2 s_\theta^2}{27 M_\eta^4 M_{\eta'}^6} + \frac{512 c_\theta^8 L_7^r M_\theta^8 M_K^4 M_\pi^2 s_\theta^2}{9 M_\eta^4 M_{\eta'}^6} + \\
& \frac{4480 c_\theta^8 L_{25}^r M_\theta^8 M_K^4 M_\pi^2 s_\theta^2}{81 M_\eta^4 M_{\eta'}^6} + \frac{2560 c_\theta^8 C_{19} M_\theta^8 M_K^6 M_\pi^2 s_\theta^2}{27 M_\eta^4 M_{\eta'}^6} + \frac{5120 c_\theta^8 C_{31} M_\theta^8 M_K^6 M_\pi^2 s_\theta^2}{81 M_\eta^4 M_{\eta'}^6} -
\end{aligned}$$

$$\begin{aligned}
& \frac{8 F^2 v_2^{(2)} c_\theta^8 M_0^8 M_\pi^4 s_\theta^2}{9 M_\eta^4 M_{\eta'}^6} - \frac{7 \text{Log}\left[\frac{M_K^2}{\mu^2}\right] c_\theta^8 M_0^8 M_K^2 M_\pi^4 s_\theta^2}{1944 \pi^2 M_\eta^4 M_{\eta'}^6} - \frac{5 \text{Log}\left[\frac{M_\pi^2}{\mu^2}\right] c_\theta^8 M_0^8 M_K^2 M_\pi^4 s_\theta^2}{216 \pi^2 M_\eta^4 M_{\eta'}^6} + \\
& \frac{256 c_\theta^8 L_6^r M_0^8 M_K^2 M_\pi^4 s_\theta^2}{27 M_\eta^4 M_{\eta'}^6} - \frac{896 c_\theta^8 L_7^r M_0^8 M_K^2 M_\pi^4 s_\theta^2}{27 M_\eta^4 M_{\eta'}^6} - \frac{3968 c_\theta^8 L_{25}^r M_0^8 M_K^2 M_\pi^4 s_\theta^2}{81 M_\eta^4 M_{\eta'}^6} - \frac{256 c_\theta^8 C_{19} M_0^8 M_K^4 M_\pi^4 s_\theta^2}{9 M_\eta^4 M_{\eta'}^6} - \\
& \frac{512 c_\theta^8 C_{31} M_0^8 M_K^4 M_\pi^4 s_\theta^2}{27 M_\eta^4 M_{\eta'}^6} - \frac{\text{Log}\left[\frac{M_\pi^2}{\mu^2}\right] c_\theta^8 M_0^8 M_\pi^6 s_\theta^2}{144 \pi^2 M_\eta^4 M_{\eta'}^6} + \frac{160 c_\theta^8 L_6^r M_0^8 M_\pi^6 s_\theta^2}{81 M_\eta^4 M_{\eta'}^6} + \frac{832 c_\theta^8 L_7^r M_0^8 M_\pi^6 s_\theta^2}{81 M_\eta^4 M_{\eta'}^6} + \\
& \frac{64 c_\theta^8 L_{25}^r M_0^8 M_\pi^6 s_\theta^2}{9 M_\eta^4 M_{\eta'}^6} + \frac{64 c_\theta^8 C_{19} M_0^8 M_K^2 M_\pi^6 s_\theta^2}{9 M_\eta^4 M_{\eta'}^6} + \frac{128 c_\theta^8 C_{31} M_0^8 M_K^2 M_\pi^6 s_\theta^2}{27 M_\eta^4 M_{\eta'}^6} + \frac{160 c_\theta^8 C_{19} M_0^8 M_\pi^8 s_\theta^2}{27 M_\eta^4 M_{\eta'}^6} + \\
& \frac{320 c_\theta^8 C_{31} M_0^8 M_\pi^8 s_\theta^2}{81 M_\eta^4 M_{\eta'}^6} + \frac{320 F^2 v_2^{(2)} c_\theta^6 M_0^6 M_K^4 s_\theta^2}{27 M_\eta^2 M_{\eta'}^6} + \frac{\text{Log}\left[\frac{M_K^2}{\mu^2}\right] c_\theta^6 M_0^8 M_K^4 s_\theta^2}{162 \pi^2 M_\eta^2 M_{\eta'}^6} - \frac{17 c_\theta^{10} M_0^8 M_K^4 s_\theta^2}{486 \pi^2 M_\eta^2 M_{\eta'}^6} - \\
& \frac{10 \text{Log}\left[\frac{M_\eta^2}{\mu^2}\right] c_\theta^{10} M_0^8 M_K^4 s_\theta^2}{729 \pi^2 M_\eta^2 M_{\eta'}^6} - \frac{4 \text{Log}\left[\frac{M_\eta^2}{\mu^2}\right] c_\theta^{10} M_0^8 M_K^4 s_\theta^2}{243 \pi^2 M_\eta^2 M_{\eta'}^6} + \frac{2560 c_\theta^6 L_6^r M_0^8 M_K^4 s_\theta^2}{81 M_\eta^2 M_{\eta'}^6} + \frac{2560 c_\theta^6 L_7^r M_0^8 M_K^4 s_\theta^2}{81 M_\eta^2 M_{\eta'}^6} + \\
& \frac{8960 c_\theta^6 C_{19} M_0^8 M_K^6 s_\theta^2}{27 M_\eta^2 M_{\eta'}^6} + \frac{25600 c_\theta^6 C_{31} M_0^8 M_K^6 s_\theta^2}{81 M_\eta^2 M_{\eta'}^6} - \frac{4 F^2 v_2^{(2)} c_\theta^6 M_0^8 M_\pi^2 s_\theta^2}{M_\eta^2 M_{\eta'}^6} + \frac{32 F^2 v_2^{(2)} c_\theta^6 M_0^6 M_K^2 M_\pi^2 s_\theta^2}{27 M_\eta^2 M_{\eta'}^6} + \\
& \frac{5 c_\theta^6 M_0^8 M_K^2 M_\pi^2 s_\theta^2}{216 \pi^2 M_\eta^2 M_{\eta'}^6} + \frac{\text{Log}\left[\frac{M_K^2}{\mu^2}\right] c_\theta^6 M_0^8 M_K^2 M_\pi^2 s_\theta^2}{36 \pi^2 M_\eta^2 M_{\eta'}^6} + \frac{11 c_\theta^{10} M_0^8 M_K^2 M_\pi^2 s_\theta^2}{243 \pi^2 M_\eta^2 M_{\eta'}^6} + \frac{139 \text{Log}\left[\frac{M_\eta^2}{\mu^2}\right] c_\theta^{10} M_0^8 M_K^2 M_\pi^2 s_\theta^2}{5832 \pi^2 M_\eta^2 M_{\eta'}^6} + \\
& \frac{13 \text{Log}\left[\frac{M_\eta^2}{\mu^2}\right] c_\theta^{10} M_0^8 M_K^2 M_\pi^2 s_\theta^2}{972 \pi^2 M_\eta^2 M_{\eta'}^6} - \frac{3200 c_\theta^6 L_6^r M_0^8 M_K^2 M_\pi^2 s_\theta^2}{81 M_\eta^2 M_{\eta'}^6} - \frac{3200 c_\theta^6 L_7^r M_0^8 M_K^2 M_\pi^2 s_\theta^2}{81 M_\eta^2 M_{\eta'}^6} - \\
& \frac{4480 c_\theta^6 C_{19} M_0^8 M_K^4 M_\pi^2 s_\theta^2}{9 M_\eta^2 M_{\eta'}^6} - \frac{12800 c_\theta^6 C_{31} M_0^8 M_K^4 M_\pi^2 s_\theta^2}{27 M_\eta^2 M_{\eta'}^6} - \frac{64 F^2 v_2^{(2)} c_\theta^6 M_0^6 M_\pi^4 s_\theta^2}{27 M_\eta^2 M_{\eta'}^6} - \frac{5 c_\theta^6 M_0^8 M_\pi^4 s_\theta^2}{432 \pi^2 M_\eta^2 M_{\eta'}^6} - \\
& \frac{\text{Log}\left[\frac{M_K^2}{\mu^2}\right] c_\theta^6 M_0^8 M_\pi^4 s_\theta^2}{216 \pi^2 M_\eta^2 M_{\eta'}^6} - \frac{\text{Log}\left[\frac{M_\pi^2}{\mu^2}\right] c_\theta^6 M_0^8 M_\pi^4 s_\theta^2}{108 \pi^2 M_\eta^2 M_{\eta'}^6} - \frac{67 c_\theta^{10} M_0^8 M_\pi^4 s_\theta^2}{3888 \pi^2 M_\eta^2 M_{\eta'}^6} - \frac{59 \text{Log}\left[\frac{M_\eta^2}{\mu^2}\right] c_\theta^{10} M_0^8 M_\pi^4 s_\theta^2}{5832 \pi^2 M_\eta^2 M_{\eta'}^6} + \\
& \frac{1216 c_\theta^6 L_6^r M_0^8 M_\pi^4 s_\theta^2}{81 M_\eta^2 M_{\eta'}^6} + \frac{1216 c_\theta^6 L_7^r M_0^8 M_\pi^4 s_\theta^2}{81 M_\eta^2 M_{\eta'}^6} + \frac{2240 c_\theta^6 C_{19} M_0^8 M_K^2 M_\pi^4 s_\theta^2}{9 M_\eta^2 M_{\eta'}^6} + \frac{6400 c_\theta^6 C_{31} M_0^8 M_K^2 M_\pi^4 s_\theta^2}{27 M_\eta^2 M_{\eta'}^6} - \\
& \frac{896 c_\theta^6 C_{19} M_0^8 M_\pi^6 s_\theta^2}{27 M_\eta^2 M_{\eta'}^6} - \frac{2560 c_\theta^6 C_{31} M_0^8 M_\pi^6 s_\theta^2}{81 M_\eta^2 M_{\eta'}^6} - \frac{8 F^2 v_2^{(2)} c_\theta^2 M_0^4 M_K^2 s_\theta^2}{3 M_{\eta'}^4} + \frac{2 F^2 v_2^{(2)} c_\theta^2 M_0^4 M_\pi^2 s_\theta^2}{3 M_{\eta'}^4} - \\
& \frac{655360 c_\theta^{10} L_8^r M_0^8 M_K^{10} s_\theta^2}{243 F^2 M_\eta^8 M_{\eta'}^4} + \frac{544768 c_\theta^{10} L_8^r M_0^8 M_K^8 M_\pi^2 s_\theta^2}{81 F^2 M_\eta^8 M_{\eta'}^4} - \frac{532480 c_\theta^{10} L_8^r M_0^8 M_K^6 M_\pi^4 s_\theta^2}{81 F^2 M_\eta^8 M_{\eta'}^4} + \\
& \frac{747520 c_\theta^{10} L_8^r M_0^8 M_K^4 M_\pi^6 s_\theta^2}{243 F^2 M_\eta^8 M_{\eta'}^4} - \frac{17408 c_\theta^{10} L_8^r M_0^8 M_K^2 M_\pi^8 s_\theta^2}{27 F^2 M_\eta^8 M_{\eta'}^4} + \frac{256 c_\theta^{10} L_8^r M_0^8 M_\pi^{10} s_\theta^2}{9 F^2 M_\eta^8 M_{\eta'}^4} - \\
& \frac{2 \text{Log}\left[\frac{M_K^2}{\mu^2}\right] c_\theta^8 M_0^8 M_K^6 s_\theta^2}{81 \pi^2 M_\eta^6 M_{\eta'}^4} + \frac{2048 c_\theta^8 L_6^r M_0^8 M_K^6 s_\theta^2}{81 M_\eta^6 M_{\eta'}^4} + \frac{2048 c_\theta^8 L_7^r M_0^8 M_K^6 s_\theta^2}{81 M_\eta^6 M_{\eta'}^4} - \frac{512 c_\theta^8 L_{25}^r M_0^8 M_K^6 s_\theta^2}{27 M_\eta^6 M_{\eta'}^4} +
\end{aligned}$$

$$\begin{aligned}
& \frac{4096 c_{\theta}^8 C_{19} M_0^8 M_K^8 s_{\theta}^2}{27 M_{\eta}^6 M_{\eta'}^4} + \frac{8192 c_{\theta}^8 C_{31} M_0^8 M_K^8 s_{\theta}^2}{81 M_{\eta}^6 M_{\eta'}^4} + \frac{11 \operatorname{Log}\left[\frac{M_K^2}{\mu^2}\right] c_{\theta}^8 M_0^8 M_K^4 M_{\pi}^2 s_{\theta}^2}{324 \pi^2 M_{\eta}^6 M_{\eta'}^4} - \\
& \frac{128 c_{\theta}^8 L_6^r M_0^8 M_K^4 M_{\pi}^2 s_{\theta}^2}{9 M_{\eta}^6 M_{\eta'}^4} - \frac{128 c_{\theta}^8 L_7^r M_0^8 M_K^4 M_{\pi}^2 s_{\theta}^2}{3 M_{\eta}^6 M_{\eta'}^4} + \frac{832 c_{\theta}^8 L_{25}^r M_0^8 M_K^4 M_{\pi}^2 s_{\theta}^2}{27 M_{\eta}^6 M_{\eta'}^4} - \frac{7936 c_{\theta}^8 C_{19} M_0^8 M_K^6 M_{\pi}^2 s_{\theta}^2}{27 M_{\eta}^6 M_{\eta'}^4} - \\
& \frac{15872 c_{\theta}^8 C_{31} M_0^8 M_K^6 M_{\pi}^2 s_{\theta}^2}{81 M_{\eta}^6 M_{\eta'}^4} - \frac{\operatorname{Log}\left[\frac{M_K^2}{\mu^2}\right] c_{\theta}^8 M_0^8 M_K^2 M_{\pi}^4 s_{\theta}^2}{108 \pi^2 M_{\eta}^6 M_{\eta'}^4} + \frac{\operatorname{Log}\left[\frac{M_{\pi}^2}{\mu^2}\right] c_{\theta}^8 M_0^8 M_K^2 M_{\pi}^4 s_{\theta}^2}{108 \pi^2 M_{\eta}^6 M_{\eta'}^4} - \\
& \frac{128 c_{\theta}^8 L_6^r M_0^8 M_K^2 M_{\pi}^4 s_{\theta}^2}{27 M_{\eta}^6 M_{\eta'}^4} + \frac{448 c_{\theta}^8 L_7^r M_0^8 M_K^2 M_{\pi}^4 s_{\theta}^2}{27 M_{\eta}^6 M_{\eta'}^4} - \frac{320 c_{\theta}^8 L_{25}^r M_0^8 M_K^2 M_{\pi}^4 s_{\theta}^2}{27 M_{\eta}^6 M_{\eta'}^4} + \frac{640 c_{\theta}^8 C_{19} M_0^8 M_K^4 M_{\pi}^4 s_{\theta}^2}{3 M_{\eta}^6 M_{\eta'}^4} + \\
& \frac{1280 c_{\theta}^8 C_{31} M_0^8 M_K^4 M_{\pi}^4 s_{\theta}^2}{9 M_{\eta}^6 M_{\eta'}^4} - \frac{\operatorname{Log}\left[\frac{M_{\pi}^2}{\mu^2}\right] c_{\theta}^8 M_0^8 M_{\pi}^6 s_{\theta}^2}{108 \pi^2 M_{\eta}^6 M_{\eta'}^4} + \frac{352 c_{\theta}^8 L_6^r M_0^8 M_{\pi}^6 s_{\theta}^2}{81 M_{\eta}^6 M_{\eta'}^4} + \frac{64 c_{\theta}^8 L_7^r M_0^8 M_{\pi}^6 s_{\theta}^2}{81 M_{\eta}^6 M_{\eta'}^4} - \\
& \frac{1984 c_{\theta}^8 C_{19} M_0^8 M_K^2 M_{\pi}^6 s_{\theta}^2}{27 M_{\eta}^6 M_{\eta'}^4} - \frac{3968 c_{\theta}^8 C_{31} M_0^8 M_K^2 M_{\pi}^6 s_{\theta}^2}{81 M_{\eta}^6 M_{\eta'}^4} + \frac{352 c_{\theta}^8 C_{19} M_0^8 M_{\pi}^8 s_{\theta}^2}{27 M_{\eta}^6 M_{\eta'}^4} + \frac{704 c_{\theta}^8 C_{31} M_0^8 M_{\pi}^8 s_{\theta}^2}{81 M_{\eta}^6 M_{\eta'}^4} - \\
& \frac{8 F^2 v_2^{(2)} c_{\theta}^6 M_0^8 M_K^2 s_{\theta}^2}{3 M_{\eta}^4 M_{\eta'}^4} - \frac{64 F^2 v_2^{(2)} c_{\theta}^6 M_0^6 M_K^4 s_{\theta}^2}{9 M_{\eta}^4 M_{\eta'}^4} + \frac{c_{\theta}^6 M_0^8 M_K^4 s_{\theta}^2}{108 \pi^2 M_{\eta}^4 M_{\eta'}^4} + \frac{\operatorname{Log}\left[\frac{M_K^2}{\mu^2}\right] c_{\theta}^6 M_0^8 M_K^4 s_{\theta}^2}{108 \pi^2 M_{\eta}^4 M_{\eta'}^4} + \\
& \frac{5 c_{\theta}^{10} M_0^8 M_K^4 s_{\theta}^2}{162 \pi^2 M_{\eta}^4 M_{\eta'}^4} - \frac{2 \operatorname{Log}\left[\frac{M_{\eta'}^2}{\mu^2}\right] c_{\theta}^{10} M_0^8 M_K^4 s_{\theta}^2}{243 \pi^2 M_{\eta}^4 M_{\eta'}^4} + \frac{53 \operatorname{Log}\left[\frac{M_{\eta'}^2}{\mu^2}\right] c_{\theta}^{10} M_0^8 M_K^4 s_{\theta}^2}{1458 \pi^2 M_{\eta}^4 M_{\eta'}^4} - \frac{512 c_{\theta}^6 L_6^r M_0^8 M_K^4 s_{\theta}^2}{27 M_{\eta}^4 M_{\eta'}^4} - \\
& \frac{512 c_{\theta}^6 L_7^r M_0^8 M_K^4 s_{\theta}^2}{27 M_{\eta}^4 M_{\eta'}^4} - \frac{1792 c_{\theta}^6 C_{19} M_0^8 M_K^6 s_{\theta}^2}{9 M_{\eta}^4 M_{\eta'}^4} - \frac{5120 c_{\theta}^6 C_{31} M_0^8 M_K^6 s_{\theta}^2}{27 M_{\eta}^4 M_{\eta'}^4} + \frac{2 F^2 v_2^{(2)} c_{\theta}^6 M_0^8 M_{\pi}^2 s_{\theta}^2}{3 M_{\eta}^4 M_{\eta'}^4} - \\
& \frac{16 F^2 v_2^{(2)} c_{\theta}^6 M_0^6 M_K^2 M_{\pi}^2 s_{\theta}^2}{9 M_{\eta}^4 M_{\eta'}^4} - \frac{5 c_{\theta}^6 M_0^8 M_K^2 M_{\pi}^2 s_{\theta}^2}{432 \pi^2 M_{\eta}^4 M_{\eta'}^4} - \frac{\operatorname{Log}\left[\frac{M_K^2}{\mu^2}\right] c_{\theta}^6 M_0^8 M_K^2 M_{\pi}^2 s_{\theta}^2}{72 \pi^2 M_{\eta}^4 M_{\eta'}^4} - \frac{11 c_{\theta}^{10} M_0^8 M_K^2 M_{\pi}^2 s_{\theta}^2}{324 \pi^2 M_{\eta}^4 M_{\eta'}^4} + \\
& \frac{11 \operatorname{Log}\left[\frac{M_{\eta'}^2}{\mu^2}\right] c_{\theta}^{10} M_0^8 M_K^2 M_{\pi}^2 s_{\theta}^2}{1944 \pi^2 M_{\eta}^4 M_{\eta'}^4} - \frac{187 \operatorname{Log}\left[\frac{M_{\eta'}^2}{\mu^2}\right] c_{\theta}^{10} M_0^8 M_K^2 M_{\pi}^2 s_{\theta}^2}{5832 \pi^2 M_{\eta}^4 M_{\eta'}^4} + \frac{448 c_{\theta}^6 L_6^r M_0^8 M_K^2 M_{\pi}^2 s_{\theta}^2}{27 M_{\eta}^4 M_{\eta'}^4} + \\
& \frac{448 c_{\theta}^6 L_7^r M_0^8 M_K^2 M_{\pi}^2 s_{\theta}^2}{27 M_{\eta}^4 M_{\eta'}^4} + \frac{896 c_{\theta}^6 C_{19} M_0^8 M_K^4 M_{\pi}^2 s_{\theta}^2}{3 M_{\eta}^4 M_{\eta'}^4} + \frac{2560 c_{\theta}^6 C_{31} M_0^8 M_K^4 M_{\pi}^2 s_{\theta}^2}{9 M_{\eta}^4 M_{\eta'}^4} + \\
& \frac{8 F^2 v_2^{(2)} c_{\theta}^6 M_0^6 M_{\pi}^4 s_{\theta}^2}{9 M_{\eta}^4 M_{\eta'}^4} + \frac{11 c_{\theta}^6 M_0^8 M_{\pi}^4 s_{\theta}^2}{864 \pi^2 M_{\eta}^4 M_{\eta'}^4} + \frac{\operatorname{Log}\left[\frac{M_K^2}{\mu^2}\right] c_{\theta}^6 M_0^8 M_{\pi}^4 s_{\theta}^2}{432 \pi^2 M_{\eta}^4 M_{\eta'}^4} + \frac{\operatorname{Log}\left[\frac{M_{\pi}^2}{\mu^2}\right] c_{\theta}^6 M_0^8 M_{\pi}^4 s_{\theta}^2}{72 \pi^2 M_{\eta}^4 M_{\eta'}^4} + \\
& \frac{29 c_{\theta}^{10} M_0^8 M_{\pi}^4 s_{\theta}^2}{2592 \pi^2 M_{\eta}^4 M_{\eta'}^4} - \frac{7 \operatorname{Log}\left[\frac{M_{\eta'}^2}{\mu^2}\right] c_{\theta}^{10} M_0^8 M_{\pi}^4 s_{\theta}^2}{7776 \pi^2 M_{\eta}^4 M_{\eta'}^4} + \frac{67 \operatorname{Log}\left[\frac{M_{\eta'}^2}{\mu^2}\right] c_{\theta}^{10} M_0^8 M_{\pi}^4 s_{\theta}^2}{11664 \pi^2 M_{\eta}^4 M_{\eta'}^4} - \frac{224 c_{\theta}^6 L_6^r M_0^8 M_{\pi}^4 s_{\theta}^2}{27 M_{\eta}^4 M_{\eta'}^4} - \\
& \frac{224 c_{\theta}^6 L_7^r M_0^8 M_{\pi}^4 s_{\theta}^2}{27 M_{\eta}^4 M_{\eta'}^4} - \frac{448 c_{\theta}^6 C_{19} M_0^8 M_K^2 M_{\pi}^4 s_{\theta}^2}{3 M_{\eta}^4 M_{\eta'}^4} - \frac{1280 c_{\theta}^6 C_{31} M_0^8 M_K^2 M_{\pi}^4 s_{\theta}^2}{9 M_{\eta}^4 M_{\eta'}^4} + \frac{112 c_{\theta}^6 C_{19} M_0^8 M_{\pi}^6 s_{\theta}^2}{9 M_{\eta}^4 M_{\eta'}^4} +
\end{aligned}$$

$$\begin{aligned}
& \frac{320 c_\theta^6 C_{31} M_\theta^8 M_\pi^6 s_\theta^2}{27 M_\eta^4 M_{\eta'}^4} + \frac{\text{Log}\left[\frac{M_\eta^2}{\mu^2}\right] c_\theta^8 M_\theta^8 M_K^2 s_\theta^2}{162 \pi^2 M_\eta^2 M_{\eta'}^4} - \frac{\text{Log}\left[\frac{M_{\eta'}^2}{\mu^2}\right] c_\theta^8 M_\theta^8 M_K^2 s_\theta^2}{108 \pi^2 M_\eta^2 M_{\eta'}^4} - \frac{7 \text{Log}\left[\frac{M_\eta^2}{\mu^2}\right] c_\theta^8 M_\theta^8 M_\pi^2 s_\theta^2}{2592 \pi^2 M_\eta^2 M_{\eta'}^4} + \\
& \frac{\text{Log}\left[\frac{M_{\eta'}^2}{\mu^2}\right] c_\theta^8 M_\theta^8 M_\pi^2 s_\theta^2}{324 \pi^2 M_\eta^2 M_{\eta'}^4} - \frac{4 \text{Log}\left[\frac{M_\eta^2}{\mu^2}\right] c_\theta^{10} M_\theta^8 M_K^4 s_\theta^2}{243 \pi^2 M_\eta^6 M_{\eta'}^2} + \frac{17 \text{Log}\left[\frac{M_{\eta'}^2}{\mu^2}\right] c_\theta^{10} M_\theta^8 M_K^2 M_\pi^2 s_\theta^2}{972 \pi^2 M_\eta^6 M_{\eta'}^2} - \\
& \frac{11 \text{Log}\left[\frac{M_\eta^2}{\mu^2}\right] c_\theta^{10} M_\theta^8 M_\pi^4 s_\theta^2}{1944 \pi^2 M_\eta^6 M_{\eta'}^2} + \frac{\text{Log}\left[\frac{M_\eta^2}{\mu^2}\right] c_\theta^8 M_\theta^8 M_K^2 s_\theta^2}{324 \pi^2 M_\eta^4 M_{\eta'}^2} - \frac{\text{Log}\left[\frac{M_{\eta'}^2}{\mu^2}\right] c_\theta^8 M_\theta^8 M_\pi^2 s_\theta^2}{1296 \pi^2 M_\eta^4 M_{\eta'}^2} + \frac{8 F^2 v_2^{(2)} c_\theta^2 M_\theta^4 M_K^2 s_\theta^2}{3 M_\eta^2 M_{\eta'}^2} - \\
& \frac{8 F^2 v_2^{(2)} c_\theta^2 M_\theta^4 M_\pi^2 s_\theta^2}{3 M_\eta^2 M_{\eta'}^2} + \frac{37 \text{Log}\left[\frac{M_\eta^2}{\mu^2}\right] c_\theta^{10} M_\theta^8 M_K^4 M_\eta^2 s_\theta^2}{972 \pi^2 M_{\eta'}^8 (M_\eta^2 - M_{\eta'}^2)} - \frac{35 \text{Log}\left[\frac{M_{\eta'}^2}{\mu^2}\right] c_\theta^{10} M_\theta^8 M_K^2 M_\pi^2 M_{\eta'}^2 s_\theta^2}{972 \pi^2 M_{\eta'}^8 (M_\eta^2 - M_{\eta'}^2)} + \\
& \frac{7 \text{Log}\left[\frac{M_\eta^2}{\mu^2}\right] c_\theta^{10} M_\theta^8 M_\pi^4 M_{\eta'}^2 s_\theta^2}{972 \pi^2 M_{\eta'}^8 (M_\eta^2 - M_{\eta'}^2)} - \frac{14 \text{Log}\left[\frac{M_\eta^2}{\mu^2}\right] c_\theta^{10} M_\theta^8 M_K^4 s_\theta^2}{243 \pi^2 M_{\eta'}^6 (M_\eta^2 - M_{\eta'}^2)} - \frac{37 \text{Log}\left[\frac{M_{\eta'}^2}{\mu^2}\right] c_\theta^{10} M_\theta^8 M_K^4 s_\theta^2}{972 \pi^2 M_{\eta'}^6 (M_\eta^2 - M_{\eta'}^2)} + \\
& \frac{23 \text{Log}\left[\frac{M_\eta^2}{\mu^2}\right] c_\theta^{10} M_\theta^8 M_K^2 M_\pi^2 s_\theta^2}{486 \pi^2 M_{\eta'}^6 (M_\eta^2 - M_{\eta'}^2)} + \frac{35 \text{Log}\left[\frac{M_{\eta'}^2}{\mu^2}\right] c_\theta^{10} M_\theta^8 M_K^2 M_\pi^2 s_\theta^2}{972 \pi^2 M_{\eta'}^6 (M_\eta^2 - M_{\eta'}^2)} - \frac{2 \text{Log}\left[\frac{M_\eta^2}{\mu^2}\right] c_\theta^{10} M_\theta^8 M_\pi^4 s_\theta^2}{243 \pi^2 M_{\eta'}^6 (M_\eta^2 - M_{\eta'}^2)} - \\
& \frac{7 \text{Log}\left[\frac{M_\eta^2}{\mu^2}\right] c_\theta^{10} M_\theta^8 M_\pi^4 s_\theta^2}{972 \pi^2 M_{\eta'}^6 (M_\eta^2 - M_{\eta'}^2)} + \frac{2 \text{Log}\left[\frac{M_\eta^2}{\mu^2}\right] c_\theta^{10} M_\theta^8 M_K^4 s_\theta^2}{81 \pi^2 M_\eta^2 M_{\eta'}^4 (M_\eta^2 - M_{\eta'}^2)} + \frac{14 \text{Log}\left[\frac{M_{\eta'}^2}{\mu^2}\right] c_\theta^{10} M_\theta^8 M_K^4 s_\theta^2}{243 \pi^2 M_\eta^2 M_{\eta'}^4 (M_\eta^2 - M_{\eta'}^2)} - \\
& \frac{7 \text{Log}\left[\frac{M_\eta^2}{\mu^2}\right] c_\theta^{10} M_\theta^8 M_K^2 M_\pi^2 s_\theta^2}{324 \pi^2 M_\eta^2 M_{\eta'}^4 (M_\eta^2 - M_{\eta'}^2)} - \frac{23 \text{Log}\left[\frac{M_{\eta'}^2}{\mu^2}\right] c_\theta^{10} M_\theta^8 M_K^2 M_\pi^2 s_\theta^2}{486 \pi^2 M_\eta^2 M_{\eta'}^4 (M_\eta^2 - M_{\eta'}^2)} + \frac{\text{Log}\left[\frac{M_\eta^2}{\mu^2}\right] c_\theta^{10} M_\theta^8 M_\pi^4 s_\theta^2}{162 \pi^2 M_\eta^2 M_{\eta'}^4 (M_\eta^2 - M_{\eta'}^2)} + \\
& \frac{2 \text{Log}\left[\frac{M_\eta^2}{\mu^2}\right] c_\theta^{10} M_\theta^8 M_\pi^4 s_\theta^2}{243 \pi^2 M_\eta^2 M_{\eta'}^4 (M_\eta^2 - M_{\eta'}^2)} - \frac{2 \text{Log}\left[\frac{M_\eta^2}{\mu^2}\right] c_\theta^{10} M_\theta^8 M_K^4 s_\theta^2}{81 \pi^2 M_\eta^4 M_{\eta'}^2 (M_\eta^2 - M_{\eta'}^2)} + \frac{7 \text{Log}\left[\frac{M_{\eta'}^2}{\mu^2}\right] c_\theta^{10} M_\theta^8 M_K^2 M_\pi^2 s_\theta^2}{324 \pi^2 M_\eta^4 M_{\eta'}^2 (M_\eta^2 - M_{\eta'}^2)} - \\
& \frac{\text{Log}\left[\frac{M_\eta^2}{\mu^2}\right] c_\theta^{10} M_\theta^8 M_\pi^4 s_\theta^2}{162 \pi^2 M_\eta^4 M_{\eta'}^2 (M_\eta^2 - M_{\eta'}^2)} - \frac{8 \sqrt{2} \text{Log}\left[\frac{M_\eta^2}{\mu^2}\right] c_\theta^9 M_\theta^8 M_K^4 s_\theta^3}{729 \pi^2 M_\eta^8} + \frac{49 \text{Log}\left[\frac{M_{\eta'}^2}{\mu^2}\right] c_\theta^9 M_\theta^8 M_K^2 M_\pi^2 s_\theta^3}{2916 \sqrt{2} \pi^2 M_\eta^8} + \\
& \frac{2 \sqrt{2} \text{Log}\left[\frac{M_\eta^2}{\mu^2}\right] c_\theta^9 M_\theta^8 M_K^2 M_\pi^2 s_\theta^3}{729 \pi^2 M_\eta^8} - \frac{29 \text{Log}\left[\frac{M_{\eta'}^2}{\mu^2}\right] c_\theta^9 M_\theta^8 M_\pi^4 s_\theta^3}{5832 \sqrt{2} \pi^2 M_\eta^8} + \frac{\text{Log}\left[\frac{M_\eta^2}{\mu^2}\right] c_\theta^7 M_\theta^8 M_K^2 s_\theta^3}{243 \sqrt{2} \pi^2 M_\eta^6} - \\
& \frac{5 \text{Log}\left[\frac{M_\eta^2}{\mu^2}\right] c_\theta^7 M_\theta^8 M_\pi^2 s_\theta^3}{1944 \sqrt{2} \pi^2 M_\eta^6} - \frac{8 \sqrt{2} F^2 v_2^{(2)} c_\theta M_\theta^4 M_K^2 s_\theta^3}{3 M_\eta^4} + \frac{8 \sqrt{2} F^2 v_2^{(2)} c_\theta M_\theta^4 M_\pi^2 s_\theta^3}{3 M_\eta^4} + \\
& \frac{4 587 520 \sqrt{2} c_\theta^9 L_8^2 r M_\theta^8 M_K^{10} s_\theta^3}{729 F^2 M_\eta^{12}} - \frac{3 891 200 \sqrt{2} c_\theta^9 L_8^2 r M_\theta^8 M_K^8 M_\pi^2 s_\theta^3}{243 F^2 M_\eta^{12}} + \\
& \frac{4 136 960 \sqrt{2} c_\theta^9 L_8^2 r M_\theta^8 M_K^6 M_\pi^4 s_\theta^3}{243 F^2 M_\eta^{12}} - \frac{6 676 480 \sqrt{2} c_\theta^9 L_8^2 r M_\theta^8 M_K^4 M_\pi^6 s_\theta^3}{729 F^2 M_\eta^{12}} +
\end{aligned}$$



$$\begin{aligned}
& \frac{573\,440\sqrt{2}\,c_\theta^9 L_8^{2r} M_0^8 M_K^2 M_\pi^8 s_\theta^3}{243 F^2 M_{\eta'}^{12}} - \frac{33\,280\sqrt{2}\,c_\theta^9 L_8^{2r} M_0^8 M_\pi^{10} s_\theta^3}{81 F^2 M_{\eta'}^{12}} - \frac{128\sqrt{2}\,F^2 v_2^{(2)} c_\theta^7 M_0^8 M_K^4 s_\theta^3}{27 M_{\eta'}^{10}} + \\
& \frac{20\sqrt{2}\,\text{Log}\left[\frac{M_K^2}{\mu^2}\right] c_\theta^7 M_0^8 M_K^6 s_\theta^3}{243 \pi^2 M_{\eta'}^{10}} - \frac{10\,240\sqrt{2}\,c_\theta^7 L_6^r M_0^8 M_K^6 s_\theta^3}{243 M_{\eta'}^{10}} - \frac{10\,240\sqrt{2}\,c_\theta^7 L_7^r M_0^8 M_K^6 s_\theta^3}{243 M_{\eta'}^{10}} + \\
& \frac{5120\sqrt{2}\,c_\theta^7 L_{25}^r M_0^8 M_K^6 s_\theta^3}{81 M_{\eta'}^{10}} - \frac{20\,480\sqrt{2}\,c_\theta^7 C_{19} M_0^8 M_K^8 s_\theta^3}{81 M_{\eta'}^{10}} - \frac{40\,960\sqrt{2}\,c_\theta^7 C_{31} M_0^8 M_K^8 s_\theta^3}{243 M_{\eta'}^{10}} + \\
& \frac{16\sqrt{2}\,F^2 v_2^{(2)} c_\theta^7 M_0^8 M_K^2 M_\pi^2 s_\theta^3}{27 M_{\eta'}^{10}} - \frac{5\sqrt{2}\,\text{Log}\left[\frac{M_K^2}{\mu^2}\right] c_\theta^7 M_0^8 M_K^4 M_\pi^2 s_\theta^3}{81 \pi^2 M_{\eta'}^{10}} + \frac{1792\sqrt{2}\,c_\theta^7 L_6^r M_0^8 M_K^4 M_\pi^2 s_\theta^3}{81 M_{\eta'}^{10}} + \\
& \frac{3328\sqrt{2}\,c_\theta^7 L_7^r M_0^8 M_K^4 M_\pi^2 s_\theta^3}{81 M_{\eta'}^{10}} - \frac{7168\sqrt{2}\,c_\theta^7 L_{25}^r M_0^8 M_K^4 M_\pi^2 s_\theta^3}{81 M_{\eta'}^{10}} + \frac{40\,448\sqrt{2}\,c_\theta^7 C_{19} M_0^8 M_K^6 M_\pi^2 s_\theta^3}{81 M_{\eta'}^{10}} + \\
& \frac{80\,896\sqrt{2}\,c_\theta^7 C_{31} M_0^8 M_K^6 M_\pi^2 s_\theta^3}{243 M_{\eta'}^{10}} + \frac{40\sqrt{2}\,F^2 v_2^{(2)} c_\theta^7 M_0^8 M_\pi^4 s_\theta^3}{27 M_{\eta'}^{10}} + \frac{\text{Log}\left[\frac{M_K^2}{\mu^2}\right] c_\theta^7 M_0^8 M_K^2 M_\pi^4 s_\theta^3}{81 \sqrt{2}\,\pi^2 M_{\eta'}^{10}} + \\
& \frac{\sqrt{2}\,\text{Log}\left[\frac{M_K^2}{\mu^2}\right] c_\theta^7 M_0^8 M_K^2 M_\pi^4 s_\theta^3}{243 \pi^2 M_{\eta'}^{10}} + \frac{\text{Log}\left[\frac{M_\pi^2}{\mu^2}\right] c_\theta^7 M_0^8 M_K^2 M_\pi^4 s_\theta^3}{81 \sqrt{2}\,\pi^2 M_{\eta'}^{10}} - \frac{\sqrt{2}\,\text{Log}\left[\frac{M_\pi^2}{\mu^2}\right] c_\theta^7 M_0^8 M_K^2 M_\pi^4 s_\theta^3}{81 \pi^2 M_{\eta'}^{10}} + \\
& \frac{1280\sqrt{2}\,c_\theta^7 L_6^r M_0^8 M_K^2 M_\pi^4 s_\theta^3}{81 M_{\eta'}^{10}} - \frac{1024\sqrt{2}\,c_\theta^7 L_7^r M_0^8 M_K^2 M_\pi^4 s_\theta^3}{81 M_{\eta'}^{10}} + \frac{3584\sqrt{2}\,c_\theta^7 L_{25}^r M_0^8 M_K^2 M_\pi^4 s_\theta^3}{81 M_{\eta'}^{10}} - \\
& \frac{3328\sqrt{2}\,c_\theta^7 C_{19} M_0^8 M_K^4 M_\pi^4 s_\theta^3}{9 M_{\eta'}^{10}} - \frac{6656\sqrt{2}\,c_\theta^7 C_{31} M_0^8 M_K^4 M_\pi^4 s_\theta^3}{27 M_{\eta'}^{10}} - \frac{\sqrt{2}\,\text{Log}\left[\frac{M_\pi^2}{\mu^2}\right] c_\theta^7 M_0^8 M_\pi^6 s_\theta^3}{81 \pi^2 M_{\eta'}^{10}} - \\
& \frac{704\sqrt{2}\,c_\theta^7 L_6^r M_0^8 M_\pi^6 s_\theta^3}{243 M_{\eta'}^{10}} + \frac{1600\sqrt{2}\,c_\theta^7 L_7^r M_0^8 M_\pi^6 s_\theta^3}{243 M_{\eta'}^{10}} - \frac{320\sqrt{2}\,c_\theta^7 L_{25}^r M_0^8 M_\pi^6 s_\theta^3}{27 M_{\eta'}^{10}} + \\
& \frac{10\,112\sqrt{2}\,c_\theta^7 C_{19} M_0^8 M_K^2 M_\pi^6 s_\theta^3}{81 M_{\eta'}^{10}} + \frac{20\,224\sqrt{2}\,c_\theta^7 C_{31} M_0^8 M_K^2 M_\pi^6 s_\theta^3}{243 M_{\eta'}^{10}} - \frac{704\sqrt{2}\,c_\theta^7 C_{19} M_0^8 M_\pi^8 s_\theta^3}{81 M_{\eta'}^{10}} - \\
& \frac{1408\sqrt{2}\,c_\theta^7 C_{31} M_0^8 M_\pi^8 s_\theta^3}{243 M_{\eta'}^{10}} - \frac{3\,604\,480\sqrt{2}\,c_\theta^9 L_8^{2r} M_0^8 M_K^{10} s_\theta^3}{729 F^2 M_{\eta'}^2 M_{\eta'}^{10}} + \frac{3\,350\,528\sqrt{2}\,c_\theta^9 L_8^{2r} M_0^8 M_K^8 M_\pi^2 s_\theta^3}{243 F^2 M_{\eta'}^2 M_{\eta'}^{10}} - \\
& \frac{4\,112\,384\sqrt{2}\,c_\theta^9 L_8^{2r} M_0^8 M_K^6 M_\pi^4 s_\theta^3}{243 F^2 M_{\eta'}^2 M_{\eta'}^{10}} + \frac{7\,278\,592\sqrt{2}\,c_\theta^9 L_8^{2r} M_0^8 M_K^4 M_\pi^6 s_\theta^3}{729 F^2 M_{\eta'}^2 M_{\eta'}^{10}} - \\
& \frac{555\,008\sqrt{2}\,c_\theta^9 L_8^{2r} M_0^8 M_K^2 M_\pi^8 s_\theta^3}{243 F^2 M_{\eta'}^2 M_{\eta'}^{10}} + \frac{5632\sqrt{2}\,c_\theta^9 L_8^{2r} M_0^8 M_\pi^{10} s_\theta^3}{27 F^2 M_{\eta'}^2 M_{\eta'}^{10}} + \frac{13\sqrt{2}\,\text{Log}\left[\frac{M_\pi^2}{\mu^2}\right] c_\theta^9 M_0^8 M_K^4 M_\pi^2 s_\theta^3}{729 \pi^2 M_{\eta'}^{10}} + \\
& \frac{\text{Log}\left[\frac{M_\pi^2}{\mu^2}\right] c_\theta^9 M_0^8 M_K^2 M_\pi^2 M_\eta^2 s_\theta^3}{1458 \sqrt{2}\,\pi^2 M_{\eta'}^{10}} - \frac{2\sqrt{2}\,\text{Log}\left[\frac{M_\eta^2}{\mu^2}\right] c_\theta^9 M_0^8 M_K^2 M_\pi^2 M_\eta^2 s_\theta^3}{243 \pi^2 M_{\eta'}^{10}} + \frac{5\,\text{Log}\left[\frac{M_\eta^2}{\mu^2}\right] c_\theta^9 M_0^8 M_\pi^4 M_\eta^2 s_\theta^3}{2916 \sqrt{2}\,\pi^2 M_{\eta'}^{10}} +
\end{aligned}$$

$$\begin{aligned}
& \frac{128 \sqrt{2} F^2 v_2^{(2)} c_\theta^5 M_0^6 M_K^4 s_\theta^3}{27 M_{\eta'}^8} + \frac{11 \text{Log}\left[\frac{M_\eta^2}{\mu^2}\right] c_\theta^5 M_0^8 M_K^4 s_\theta^3}{1620 \sqrt{2} \pi^2 M_{\eta'}^8} - \frac{23 c_\theta^9 M_0^8 M_K^4 s_\theta^3}{243 \sqrt{2} \pi^2 M_{\eta'}^8} + \\
& \frac{5 \text{Log}\left[\frac{M_\eta^2}{\mu^2}\right] c_\theta^9 M_0^8 M_K^4 s_\theta^3}{243 \sqrt{2} \pi^2 M_{\eta'}^8} - \frac{4 \sqrt{2} \text{Log}\left[\frac{M_\eta^2}{\mu^2}\right] c_\theta^9 M_0^8 M_K^4 s_\theta^3}{81 \pi^2 M_{\eta'}^8} + \frac{14 \sqrt{2} \text{Log}\left[\frac{M_\eta^2}{\mu^2}\right] c_\theta^9 M_0^8 M_K^4 s_\theta^3}{729 \pi^2 M_{\eta'}^8} + \\
& \frac{1024 \sqrt{2} c_\theta^5 L_6^r M_0^8 M_K^4 s_\theta^3}{81 M_{\eta'}^8} + \frac{1024 \sqrt{2} c_\theta^5 L_7^r M_0^8 M_K^4 s_\theta^3}{81 M_{\eta'}^8} + \frac{3584 \sqrt{2} c_\theta^5 C_{19} M_0^8 M_K^6 s_\theta^3}{27 M_{\eta'}^8} + \\
& \frac{10240 \sqrt{2} c_\theta^5 C_{31} M_0^8 M_K^6 s_\theta^3}{81 M_{\eta'}^8} - \frac{16 \sqrt{2} F^2 v_2^{(2)} c_\theta^5 M_0^6 M_K^2 M_\pi^2 s_\theta^3}{27 M_{\eta'}^8} + \frac{c_\theta^5 M_0^8 M_K^2 M_\pi^2 s_\theta^3}{216 \sqrt{2} \pi^2 M_{\eta'}^8} + \\
& \frac{\text{Log}\left[\frac{M_K^2}{\mu^2}\right] c_\theta^5 M_0^8 M_K^2 M_\pi^2 s_\theta^3}{1080 \sqrt{2} \pi^2 M_{\eta'}^8} + \frac{14 \sqrt{2} c_\theta^9 M_0^8 M_K^2 M_\pi^2 s_\theta^3}{243 \pi^2 M_{\eta'}^8} + \frac{5 \sqrt{2} \text{Log}\left[\frac{M_\eta^2}{\mu^2}\right] c_\theta^9 M_0^8 M_K^2 M_\pi^2 s_\theta^3}{243 \pi^2 M_{\eta'}^8} + \\
& \frac{5 \text{Log}\left[\frac{M_\eta^2}{\mu^2}\right] c_\theta^9 M_0^8 M_K^2 M_\pi^2 s_\theta^3}{486 \sqrt{2} \pi^2 M_{\eta'}^8} - \frac{19 \sqrt{2} \text{Log}\left[\frac{M_\eta^2}{\mu^2}\right] c_\theta^9 M_0^8 M_K^2 M_\pi^2 s_\theta^3}{729 \pi^2 M_{\eta'}^8} - \frac{992 \sqrt{2} c_\theta^5 L_6^r M_0^8 M_K^2 M_\pi^2 s_\theta^3}{81 M_{\eta'}^8} - \\
& \frac{992 \sqrt{2} c_\theta^5 L_7^r M_0^8 M_K^2 M_\pi^2 s_\theta^3}{81 M_{\eta'}^8} - \frac{1792 \sqrt{2} c_\theta^5 C_{19} M_0^8 M_K^4 M_\pi^2 s_\theta^3}{9 M_{\eta'}^8} - \frac{5120 \sqrt{2} c_\theta^5 C_{31} M_0^8 M_K^4 M_\pi^2 s_\theta^3}{27 M_{\eta'}^8} - \\
& \frac{40 \sqrt{2} F^2 v_2^{(2)} c_\theta^5 M_0^6 M_\pi^4 s_\theta^3}{27 M_{\eta'}^8} + \frac{c_\theta^5 M_0^8 M_\pi^4 s_\theta^3}{216 \sqrt{2} \pi^2 M_{\eta'}^8} - \frac{\text{Log}\left[\frac{M_K^2}{\mu^2}\right] c_\theta^5 M_0^8 M_\pi^4 s_\theta^3}{432 \sqrt{2} \pi^2 M_{\eta'}^8} + \frac{\text{Log}\left[\frac{M_\eta^2}{\mu^2}\right] c_\theta^5 M_0^8 M_\pi^4 s_\theta^3}{108 \sqrt{2} \pi^2 M_{\eta'}^8} - \\
& \frac{71 c_\theta^9 M_0^8 M_\pi^4 s_\theta^3}{3888 \sqrt{2} \pi^2 M_{\eta'}^8} + \frac{5 \text{Log}\left[\frac{M_\eta^2}{\mu^2}\right] c_\theta^9 M_0^8 M_\pi^4 s_\theta^3}{3888 \sqrt{2} \pi^2 M_{\eta'}^8} - \frac{\sqrt{2} \text{Log}\left[\frac{M_\eta^2}{\mu^2}\right] c_\theta^9 M_0^8 M_\pi^4 s_\theta^3}{243 \pi^2 M_{\eta'}^8} - \frac{77 \text{Log}\left[\frac{M_\eta^2}{\mu^2}\right] c_\theta^9 M_0^8 M_\pi^4 s_\theta^3}{2916 \sqrt{2} \pi^2 M_{\eta'}^8} + \\
& \frac{4 \sqrt{2} \text{Log}\left[\frac{M_\eta^2}{\mu^2}\right] c_\theta^9 M_0^8 M_\pi^4 s_\theta^3}{243 \pi^2 M_{\eta'}^8} + \frac{112 \sqrt{2} c_\theta^5 L_6^r M_0^8 M_\pi^4 s_\theta^3}{81 M_{\eta'}^8} + \frac{112 \sqrt{2} c_\theta^5 L_7^r M_0^8 M_\pi^4 s_\theta^3}{81 M_{\eta'}^8} + \\
& \frac{896 \sqrt{2} c_\theta^5 C_{19} M_0^8 M_K^2 M_\pi^4 s_\theta^3}{9 M_{\eta'}^8} + \frac{2560 \sqrt{2} c_\theta^5 C_{31} M_0^8 M_K^2 M_\pi^4 s_\theta^3}{27 M_{\eta'}^8} - \frac{560 \sqrt{2} c_\theta^5 C_{19} M_0^8 M_\pi^6 s_\theta^3}{27 M_{\eta'}^8} - \\
& \frac{1600 \sqrt{2} c_\theta^5 C_{31} M_0^8 M_\pi^6 s_\theta^3}{81 M_{\eta'}^8} - \frac{2621440 \sqrt{2} c_\theta^9 L_8^{2r} M_0^8 M_K^{10} s_\theta^3}{729 F^2 M_{\eta'}^4 M_{\eta'}^8} + \frac{1630208 \sqrt{2} c_\theta^9 L_8^{2r} M_0^8 M_K^8 M_\pi^2 s_\theta^3}{243 F^2 M_{\eta'}^4 M_{\eta'}^8} - \\
& \frac{401408 \sqrt{2} c_\theta^9 L_8^{2r} M_0^8 M_K^6 M_\pi^4 s_\theta^3}{243 F^2 M_{\eta'}^4 M_{\eta'}^8} - \frac{1224704 \sqrt{2} c_\theta^9 L_8^{2r} M_0^8 M_K^4 M_\pi^6 s_\theta^3}{729 F^2 M_{\eta'}^4 M_{\eta'}^8} + \\
& \frac{34816 \sqrt{2} c_\theta^9 L_8^{2r} M_0^8 M_K^2 M_\pi^8 s_\theta^3}{243 F^2 M_{\eta'}^4 M_{\eta'}^8} + \frac{2048 \sqrt{2} c_\theta^9 L_8^{2r} M_0^8 M_\pi^{10} s_\theta^3}{27 F^2 M_{\eta'}^4 M_{\eta'}^8} + \frac{128 \sqrt{2} F^2 v_2^{(2)} c_\theta^7 M_0^8 M_K^4 s_\theta^3}{27 M_{\eta'}^2 M_{\eta'}^8} - \\
& \frac{32 \sqrt{2} \text{Log}\left[\frac{M_K^2}{\mu^2}\right] c_\theta^7 M_0^8 M_K^6 s_\theta^3}{243 \pi^2 M_{\eta'}^2 M_{\eta'}^8} + \frac{16384 \sqrt{2} c_\theta^7 L_6^r M_0^8 M_K^6 s_\theta^3}{243 M_{\eta'}^2 M_{\eta'}^8} + \frac{16384 \sqrt{2} c_\theta^7 L_7^r M_0^8 M_K^6 s_\theta^3}{243 M_{\eta'}^2 M_{\eta'}^8} -
\end{aligned}$$

$$\begin{aligned}
& \frac{8192 \sqrt{2} c_{\theta}^7 L_{25}^r M_0^8 M_K^6 s_{\theta}^3}{81 M_{\eta'}^2 M_{\eta'}^8} + \frac{32768 \sqrt{2} c_{\theta}^7 C_{19} M_0^8 M_K^8 s_{\theta}^3}{81 M_{\eta'}^2 M_{\eta'}^8} + \frac{65536 \sqrt{2} c_{\theta}^7 C_{31} M_0^8 M_K^8 s_{\theta}^3}{243 M_{\eta'}^2 M_{\eta'}^8} + \\
& \frac{80 \sqrt{2} F^2 v_2^{(2)} c_{\theta}^7 M_0^8 M_K^2 M_{\pi}^2 s_{\theta}^3}{27 M_{\eta'}^2 M_{\eta'}^8} + \frac{125 \text{Log}\left[\frac{M_K^2}{\mu^2}\right] c_{\theta}^7 M_0^8 M_K^4 M_{\pi}^2 s_{\theta}^3}{972 \sqrt{2} \pi^2 M_{\eta'}^2 M_{\eta'}^8} + \frac{5 \sqrt{2} \text{Log}\left[\frac{M_K^2}{\mu^2}\right] c_{\theta}^7 M_0^8 M_K^4 M_{\pi}^2 s_{\theta}^3}{243 \pi^2 M_{\eta'}^2 M_{\eta'}^8} - \\
& \frac{1216 \sqrt{2} c_{\theta}^7 L_6^r M_0^8 M_K^4 M_{\pi}^2 s_{\theta}^3}{27 M_{\eta'}^2 M_{\eta'}^8} - \frac{64 \sqrt{2} c_{\theta}^7 L_7^r M_0^8 M_K^4 M_{\pi}^2 s_{\theta}^3}{M_{\eta'}^2 M_{\eta'}^8} + \frac{10144 \sqrt{2} c_{\theta}^7 L_{25}^r M_0^8 M_K^4 M_{\pi}^2 s_{\theta}^3}{81 M_{\eta'}^2 M_{\eta'}^8} - \\
& \frac{63872 \sqrt{2} c_{\theta}^7 C_{19} M_0^8 M_K^6 M_{\pi}^2 s_{\theta}^3}{81 M_{\eta'}^2 M_{\eta'}^8} - \frac{127744 \sqrt{2} c_{\theta}^7 C_{31} M_0^8 M_K^6 M_{\pi}^2 s_{\theta}^3}{243 M_{\eta'}^2 M_{\eta'}^8} + \frac{8 \sqrt{2} F^2 v_2^{(2)} c_{\theta}^7 M_0^8 M_K^4 s_{\theta}^3}{27 M_{\eta'}^2 M_{\eta'}^8} - \\
& \frac{23 \text{Log}\left[\frac{M_K^2}{\mu^2}\right] c_{\theta}^7 M_0^8 M_K^2 M_{\pi}^4 s_{\theta}^3}{972 \sqrt{2} \pi^2 M_{\eta'}^2 M_{\eta'}^8} - \frac{\sqrt{2} \text{Log}\left[\frac{M_K^2}{\mu^2}\right] c_{\theta}^7 M_0^8 M_K^2 M_{\pi}^4 s_{\theta}^3}{81 \pi^2 M_{\eta'}^2 M_{\eta'}^8} + \frac{7 \text{Log}\left[\frac{M_K^2}{\mu^2}\right] c_{\theta}^7 M_0^8 M_K^2 M_{\pi}^4 s_{\theta}^3}{81 \sqrt{2} \pi^2 M_{\eta'}^2 M_{\eta'}^8} - \\
& \frac{1408 \sqrt{2} c_{\theta}^7 L_6^r M_0^8 M_K^2 M_{\pi}^4 s_{\theta}^3}{81 M_{\eta'}^2 M_{\eta'}^8} + \frac{1760 \sqrt{2} c_{\theta}^7 L_7^r M_0^8 M_K^2 M_{\pi}^4 s_{\theta}^3}{81 M_{\eta'}^2 M_{\eta'}^8} - \frac{3488 \sqrt{2} c_{\theta}^7 L_{25}^r M_0^8 M_K^2 M_{\pi}^4 s_{\theta}^3}{81 M_{\eta'}^2 M_{\eta'}^8} + \\
& \frac{576 \sqrt{2} c_{\theta}^7 C_{19} M_0^8 M_K^4 M_{\pi}^4 s_{\theta}^3}{M_{\eta'}^2 M_{\eta'}^8} + \frac{384 \sqrt{2} c_{\theta}^7 C_{31} M_0^8 M_K^4 M_{\pi}^4 s_{\theta}^3}{M_{\eta'}^2 M_{\eta'}^8} - \frac{13 \text{Log}\left[\frac{M_{\pi}^2}{\mu^2}\right] c_{\theta}^7 M_0^8 M_{\pi}^6 s_{\theta}^3}{324 \sqrt{2} \pi^2 M_{\eta'}^2 M_{\eta'}^8} + \\
& \frac{2672 \sqrt{2} c_{\theta}^7 L_6^r M_0^8 M_{\pi}^6 s_{\theta}^3}{243 M_{\eta'}^2 M_{\eta'}^8} - \frac{928 \sqrt{2} c_{\theta}^7 L_7^r M_0^8 M_{\pi}^6 s_{\theta}^3}{243 M_{\eta'}^2 M_{\eta'}^8} - \frac{64 \sqrt{2} c_{\theta}^7 L_{25}^r M_0^8 M_{\pi}^6 s_{\theta}^3}{27 M_{\eta'}^2 M_{\eta'}^8} - \\
& \frac{16928 \sqrt{2} c_{\theta}^7 C_{19} M_0^8 M_K^2 M_{\pi}^6 s_{\theta}^3}{81 M_{\eta'}^2 M_{\eta'}^8} - \frac{33856 \sqrt{2} c_{\theta}^7 C_{31} M_0^8 M_K^2 M_{\pi}^6 s_{\theta}^3}{243 M_{\eta'}^2 M_{\eta'}^8} + \frac{2672 \sqrt{2} c_{\theta}^7 C_{19} M_0^8 M_{\pi}^8 s_{\theta}^3}{81 M_{\eta'}^2 M_{\eta'}^8} + \\
& \frac{5344 \sqrt{2} c_{\theta}^7 C_{31} M_0^8 M_{\pi}^8 s_{\theta}^3}{243 M_{\eta'}^2 M_{\eta'}^8} + \frac{\text{Log}\left[\frac{M_{\eta'}^2}{\mu^2}\right] c_{\theta}^7 M_0^8 M_K^2 M_{\eta'}^2 s_{\theta}^3}{486 \sqrt{2} \pi^2 M_{\eta'}^8} - \frac{5 \text{Log}\left[\frac{M_{\eta'}^2}{\mu^2}\right] c_{\theta}^7 M_0^8 M_{\pi}^2 M_{\eta'}^2 s_{\theta}^3}{3888 \sqrt{2} \pi^2 M_{\eta'}^8} - \\
& \frac{\text{Log}\left[\frac{M_{\eta'}^2}{\mu^2}\right] c_{\theta}^7 M_0^8 M_K^2 s_{\theta}^3}{162 \sqrt{2} \pi^2 M_{\eta'}^6} - \frac{5 \text{Log}\left[\frac{M_{\eta'}^2}{\mu^2}\right] c_{\theta}^7 M_0^8 M_K^2 s_{\theta}^3}{243 \sqrt{2} \pi^2 M_{\eta'}^6} + \frac{5 \text{Log}\left[\frac{M_{\eta'}^2}{\mu^2}\right] c_{\theta}^7 M_0^8 M_{\pi}^2 s_{\theta}^3}{1296 \sqrt{2} \pi^2 M_{\eta'}^6} + \\
& \frac{25 \text{Log}\left[\frac{M_{\eta'}^2}{\mu^2}\right] c_{\theta}^7 M_0^8 M_{\pi}^2 s_{\theta}^3}{1944 \sqrt{2} \pi^2 M_{\eta'}^6} + \frac{6225920 \sqrt{2} c_{\theta}^9 L_8^2 r M_0^8 M_K^{10} s_{\theta}^3}{729 F^2 M_{\eta'}^6 M_{\eta'}^6} - \frac{4784128 \sqrt{2} c_{\theta}^9 L_8^2 r M_0^8 M_K^8 M_{\pi}^2 s_{\theta}^3}{243 F^2 M_{\eta'}^6 M_{\eta'}^6} + \\
& \frac{3604480 \sqrt{2} c_{\theta}^9 L_8^2 r M_0^8 M_K^6 M_{\pi}^4 s_{\theta}^3}{243 F^2 M_{\eta'}^6 M_{\eta'}^6} - \frac{3067904 \sqrt{2} c_{\theta}^9 L_8^2 r M_0^8 M_K^4 M_{\pi}^6 s_{\theta}^3}{729 F^2 M_{\eta'}^6 M_{\eta'}^6} + \\
& \frac{142336 \sqrt{2} c_{\theta}^9 L_8^2 r M_0^8 M_K^2 M_{\pi}^8 s_{\theta}^3}{243 F^2 M_{\eta'}^6 M_{\eta'}^6} + \frac{1024 \sqrt{2} c_{\theta}^9 L_8^2 r M_0^8 M_{\pi}^{10} s_{\theta}^3}{81 F^2 M_{\eta'}^6 M_{\eta'}^6} - \frac{128 \sqrt{2} F^2 v_2^{(2)} c_{\theta}^7 M_0^8 M_K^4 s_{\theta}^3}{27 M_{\eta'}^4 M_{\eta'}^6} + \\
& \frac{34 \sqrt{2} \text{Log}\left[\frac{M_K^2}{\mu^2}\right] c_{\theta}^7 M_0^8 M_K^6 s_{\theta}^3}{243 \pi^2 M_{\eta'}^4 M_{\eta'}^6} - \frac{4096 \sqrt{2} c_{\theta}^7 L_6^r M_0^8 M_K^6 s_{\theta}^3}{81 M_{\eta'}^4 M_{\eta'}^6} - \frac{4096 \sqrt{2} c_{\theta}^7 L_7^r M_0^8 M_K^6 s_{\theta}^3}{81 M_{\eta'}^4 M_{\eta'}^6} +
\end{aligned}$$

$$\begin{aligned}
& \frac{8704 \sqrt{2} c_{\theta}^7 L_{25}^r M_0^8 M_K^6 s_{\theta}^3}{81 M_{\eta}^4 M_{\eta'}^6} - \frac{8192 \sqrt{2} c_{\theta}^7 C_{19} M_0^8 M_K^8 s_{\theta}^3}{27 M_{\eta}^4 M_{\eta'}^6} - \frac{16384 \sqrt{2} c_{\theta}^7 C_{31} M_0^8 M_K^8 s_{\theta}^3}{81 M_{\eta}^4 M_{\eta'}^6} - \\
& \frac{80 \sqrt{2} F^2 v_2^{(2)} c_{\theta}^7 M_0^8 M_K^2 M_{\pi}^2 s_{\theta}^3}{27 M_{\eta}^4 M_{\eta'}^6} - \frac{71 \text{Log} \left[ \frac{M_K^2}{\mu^2} \right] c_{\theta}^7 M_0^8 M_K^4 M_{\pi}^2 s_{\theta}^3}{972 \sqrt{2} \pi^2 M_{\eta}^4 M_{\eta'}^6} - \frac{10 \sqrt{2} \text{Log} \left[ \frac{M_K^2}{\mu^2} \right] c_{\theta}^7 M_0^8 M_K^4 M_{\pi}^2 s_{\theta}^3}{243 \pi^2 M_{\eta}^4 M_{\eta'}^6} + \\
& \frac{1088 \sqrt{2} c_{\theta}^7 L_6^r M_0^8 M_K^4 M_{\pi}^2 s_{\theta}^3}{27 M_{\eta}^4 M_{\eta'}^6} + \frac{320 \sqrt{2} c_{\theta}^7 L_7^r M_0^8 M_K^4 M_{\pi}^2 s_{\theta}^3}{27 M_{\eta}^4 M_{\eta'}^6} - \frac{10592 \sqrt{2} c_{\theta}^7 L_{25}^r M_0^8 M_K^4 M_{\pi}^2 s_{\theta}^3}{81 M_{\eta}^4 M_{\eta'}^6} + \\
& \frac{15232 \sqrt{2} c_{\theta}^7 C_{19} M_0^8 M_K^6 M_{\pi}^2 s_{\theta}^3}{27 M_{\eta}^4 M_{\eta'}^6} + \frac{30464 \sqrt{2} c_{\theta}^7 C_{31} M_0^8 M_K^6 M_{\pi}^2 s_{\theta}^3}{81 M_{\eta}^4 M_{\eta'}^6} - \frac{8 \sqrt{2} F^2 v_2^{(2)} c_{\theta}^7 M_0^8 M_K^4 s_{\theta}^3}{27 M_{\eta}^4 M_{\eta'}^6} + \\
& \frac{\text{Log} \left[ \frac{M_K^2}{\mu^2} \right] c_{\theta}^7 M_0^8 M_K^2 M_{\pi}^4 s_{\theta}^3}{36 \sqrt{2} \pi^2 M_{\eta}^4 M_{\eta'}^6} + \frac{\sqrt{2} \text{Log} \left[ \frac{M_K^2}{\mu^2} \right] c_{\theta}^7 M_0^8 M_K^2 M_{\pi}^4 s_{\theta}^3}{243 \pi^2 M_{\eta}^4 M_{\eta'}^6} - \frac{\text{Log} \left[ \frac{M_{\pi}^2}{\mu^2} \right] c_{\theta}^7 M_0^8 M_K^2 M_{\pi}^4 s_{\theta}^3}{18 \sqrt{2} \pi^2 M_{\eta}^4 M_{\eta'}^6} - \\
& \frac{\sqrt{2} \text{Log} \left[ \frac{M_{\pi}^2}{\mu^2} \right] c_{\theta}^7 M_0^8 M_K^2 M_{\pi}^4 s_{\theta}^3}{27 \pi^2 M_{\eta}^4 M_{\eta'}^6} + \frac{128 \sqrt{2} c_{\theta}^7 L_6^r M_0^8 M_K^2 M_{\pi}^4 s_{\theta}^3}{9 M_{\eta}^4 M_{\eta'}^6} + \frac{224 \sqrt{2} c_{\theta}^7 L_7^r M_0^8 M_K^2 M_{\pi}^4 s_{\theta}^3}{9 M_{\eta}^4 M_{\eta'}^6} + \\
& \frac{3424 \sqrt{2} c_{\theta}^7 L_{25}^r M_0^8 M_K^2 M_{\pi}^4 s_{\theta}^3}{81 M_{\eta}^4 M_{\eta'}^6} - \frac{3520 \sqrt{2} c_{\theta}^7 C_{19} M_0^8 M_K^4 M_{\pi}^4 s_{\theta}^3}{9 M_{\eta}^4 M_{\eta'}^6} - \frac{7040 \sqrt{2} c_{\theta}^7 C_{31} M_0^8 M_K^4 M_{\pi}^4 s_{\theta}^3}{27 M_{\eta}^4 M_{\eta'}^6} + \\
& \frac{\text{Log} \left[ \frac{M_{\pi}^2}{\mu^2} \right] c_{\theta}^7 M_0^8 M_{\pi}^6 s_{\theta}^3}{18 \sqrt{2} \pi^2 M_{\eta}^4 M_{\eta'}^6} - \frac{752 \sqrt{2} c_{\theta}^7 L_6^r M_0^8 M_{\pi}^6 s_{\theta}^3}{81 M_{\eta}^4 M_{\eta'}^6} - \frac{608 \sqrt{2} c_{\theta}^7 L_7^r M_0^8 M_{\pi}^6 s_{\theta}^3}{81 M_{\eta}^4 M_{\eta'}^6} + \\
& \frac{64 \sqrt{2} c_{\theta}^7 L_{25}^r M_0^8 M_{\pi}^6 s_{\theta}^3}{27 M_{\eta}^4 M_{\eta'}^6} + \frac{1376 \sqrt{2} c_{\theta}^7 C_{19} M_0^8 M_K^2 M_{\pi}^6 s_{\theta}^3}{9 M_{\eta}^4 M_{\eta'}^6} + \frac{2752 \sqrt{2} c_{\theta}^7 C_{31} M_0^8 M_K^2 M_{\pi}^6 s_{\theta}^3}{27 M_{\eta}^4 M_{\eta'}^6} - \\
& \frac{752 \sqrt{2} c_{\theta}^7 C_{19} M_0^8 M_{\pi}^8 s_{\theta}^3}{27 M_{\eta}^4 M_{\eta'}^6} - \frac{1504 \sqrt{2} c_{\theta}^7 C_{31} M_0^8 M_{\pi}^8 s_{\theta}^3}{81 M_{\eta}^4 M_{\eta'}^6} + \frac{8 \sqrt{2} F^2 v_2^{(2)} c_{\theta}^5 M_0^8 M_K^2 s_{\theta}^3}{M_{\eta}^2 M_{\eta'}^6} - \\
& \frac{64 \sqrt{2} F^2 v_2^{(2)} c_{\theta}^5 M_0^8 M_K^4 s_{\theta}^3}{9 M_{\eta}^2 M_{\eta'}^6} - \frac{c_{\theta}^5 M_0^8 M_K^4 s_{\theta}^3}{18 \sqrt{2} \pi^2 M_{\eta}^2 M_{\eta'}^6} - \frac{17 \text{Log} \left[ \frac{M_K^2}{\mu^2} \right] c_{\theta}^5 M_0^8 M_K^4 s_{\theta}^3}{180 \sqrt{2} \pi^2 M_{\eta}^2 M_{\eta'}^6} + \\
& \frac{19 c_{\theta}^9 M_0^8 M_K^4 s_{\theta}^3}{243 \sqrt{2} \pi^2 M_{\eta}^2 M_{\eta'}^6} + \frac{32 \sqrt{2} \text{Log} \left[ \frac{M_{\eta}^2}{\mu^2} \right] c_{\theta}^9 M_0^8 M_K^4 s_{\theta}^3}{729 \pi^2 M_{\eta}^2 M_{\eta'}^6} + \frac{35 \text{Log} \left[ \frac{M_{\eta}^2}{\mu^2} \right] c_{\theta}^9 M_0^8 M_K^4 s_{\theta}^3}{243 \sqrt{2} \pi^2 M_{\eta}^2 M_{\eta'}^6} - \\
& \frac{19 \sqrt{2} \text{Log} \left[ \frac{M_{\eta}^2}{\mu^2} \right] c_{\theta}^9 M_0^8 M_K^4 s_{\theta}^3}{243 \pi^2 M_{\eta}^2 M_{\eta'}^6} - \frac{512 \sqrt{2} c_{\theta}^5 L_6^r M_0^8 M_K^4 s_{\theta}^3}{27 M_{\eta}^2 M_{\eta'}^6} - \frac{512 \sqrt{2} c_{\theta}^5 L_7^r M_0^8 M_K^4 s_{\theta}^3}{27 M_{\eta}^2 M_{\eta'}^6} - \\
& \frac{1792 \sqrt{2} c_{\theta}^5 C_{19} M_0^8 M_K^6 s_{\theta}^3}{9 M_{\eta}^2 M_{\eta'}^6} - \frac{5120 \sqrt{2} c_{\theta}^5 C_{31} M_0^8 M_K^6 s_{\theta}^3}{27 M_{\eta}^2 M_{\eta'}^6} - \frac{8 \sqrt{2} F^2 v_2^{(2)} c_{\theta}^5 M_0^8 M_{\pi}^2 s_{\theta}^3}{M_{\eta}^2 M_{\eta'}^6} - \\
& \frac{16 \sqrt{2} F^2 v_2^{(2)} c_{\theta}^5 M_0^8 M_K^2 M_{\pi}^2 s_{\theta}^3}{9 M_{\eta}^2 M_{\eta'}^6} + \frac{c_{\theta}^5 M_0^8 M_K^2 M_{\pi}^2 s_{\theta}^3}{72 \sqrt{2} \pi^2 M_{\eta}^2 M_{\eta'}^6} + \frac{37 \text{Log} \left[ \frac{M_K^2}{\mu^2} \right] c_{\theta}^5 M_0^8 M_K^2 M_{\pi}^2 s_{\theta}^3}{1080 \sqrt{2} \pi^2 M_{\eta}^2 M_{\eta'}^6} -
\end{aligned}$$

$$\begin{aligned}
& \frac{67 c_{\theta}^9 M_0^8 M_K^2 M_{\pi}^2 s_{\theta}^3}{486 \sqrt{2} \pi^2 M_{\eta}^2 M_{\eta'}^6} - \frac{31 \operatorname{Log}\left[\frac{M_{\eta}^2}{\mu^2}\right] c_{\theta}^9 M_0^8 M_K^2 M_{\pi}^2 s_{\theta}^3}{972 \sqrt{2} \pi^2 M_{\eta}^2 M_{\eta'}^6} - \frac{16 \sqrt{2} \operatorname{Log}\left[\frac{M_{\eta}^2}{\mu^2}\right] c_{\theta}^9 M_0^8 M_K^2 M_{\pi}^2 s_{\theta}^3}{729 \pi^2 M_{\eta}^2 M_{\eta'}^6} - \\
& \frac{149 \operatorname{Log}\left[\frac{M_{\eta}^2}{\mu^2}\right] c_{\theta}^9 M_0^8 M_K^2 M_{\pi}^2 s_{\theta}^3}{972 \sqrt{2} \pi^2 M_{\eta}^2 M_{\eta'}^6} + \frac{23 \sqrt{2} \operatorname{Log}\left[\frac{M_{\eta}^2}{\mu^2}\right] c_{\theta}^9 M_0^8 M_K^2 M_{\pi}^2 s_{\theta}^3}{243 \pi^2 M_{\eta}^2 M_{\eta'}^6} + \frac{736 \sqrt{2} c_{\theta}^5 L_6^r M_0^8 M_K^2 M_{\pi}^2 s_{\theta}^3}{27 M_{\eta}^2 M_{\eta'}^6} + \\
& \frac{736 \sqrt{2} c_{\theta}^5 L_7^r M_0^8 M_K^2 M_{\pi}^2 s_{\theta}^3}{27 M_{\eta}^2 M_{\eta'}^6} + \frac{896 \sqrt{2} c_{\theta}^5 C_{19} M_0^8 M_K^4 M_{\pi}^2 s_{\theta}^3}{3 M_{\eta}^2 M_{\eta'}^6} + \frac{2560 \sqrt{2} c_{\theta}^5 C_{31} M_0^8 M_K^4 M_{\pi}^2 s_{\theta}^3}{9 M_{\eta}^2 M_{\eta'}^6} + \\
& \frac{8 \sqrt{2} F^2 v_2^{(2)} c_{\theta}^5 M_0^8 M_{\pi}^4 s_{\theta}^3}{9 M_{\eta}^2 M_{\eta'}^6} + \frac{c_{\theta}^5 M_0^8 M_{\pi}^4 s_{\theta}^3}{36 \sqrt{2} \pi^2 M_{\eta}^2 M_{\eta'}^6} + \frac{\operatorname{Log}\left[\frac{M_K^2}{\mu^2}\right] c_{\theta}^5 M_0^8 M_{\pi}^4 s_{\theta}^3}{144 \sqrt{2} \pi^2 M_{\eta}^2 M_{\eta'}^6} + \frac{\operatorname{Log}\left[\frac{M_{\pi}^2}{\mu^2}\right] c_{\theta}^5 M_0^8 M_{\pi}^4 s_{\theta}^3}{36 \sqrt{2} \pi^2 M_{\eta}^2 M_{\eta'}^6} + \\
& \frac{215 c_{\theta}^9 M_0^8 M_{\pi}^4 s_{\theta}^3}{3888 \sqrt{2} \pi^2 M_{\eta}^2 M_{\eta'}^6} - \frac{2 \sqrt{2} c_{\theta}^9 M_0^8 M_{\pi}^4 s_{\theta}^3}{243 \pi^2 M_{\eta}^2 M_{\eta'}^6} + \frac{31 \operatorname{Log}\left[\frac{M_{\eta}^2}{\mu^2}\right] c_{\theta}^9 M_0^8 M_{\pi}^4 s_{\theta}^3}{1296 \sqrt{2} \pi^2 M_{\eta}^2 M_{\eta'}^6} - \frac{\sqrt{2} \operatorname{Log}\left[\frac{M_{\eta}^2}{\mu^2}\right] c_{\theta}^9 M_0^8 M_{\pi}^4 s_{\theta}^3}{729 \pi^2 M_{\eta}^2 M_{\eta'}^6} + \\
& \frac{5 \operatorname{Log}\left[\frac{M_{\eta}^2}{\mu^2}\right] c_{\theta}^9 M_0^8 M_{\pi}^4 s_{\theta}^3}{216 \sqrt{2} \pi^2 M_{\eta}^2 M_{\eta'}^6} - \frac{4 \sqrt{2} \operatorname{Log}\left[\frac{M_{\eta}^2}{\mu^2}\right] c_{\theta}^9 M_0^8 M_{\pi}^4 s_{\theta}^3}{243 \pi^2 M_{\eta}^2 M_{\eta'}^6} - \frac{368 \sqrt{2} c_{\theta}^5 L_6^r M_0^8 M_{\pi}^4 s_{\theta}^3}{27 M_{\eta}^2 M_{\eta'}^6} - \\
& \frac{368 \sqrt{2} c_{\theta}^5 L_7^r M_0^8 M_{\pi}^4 s_{\theta}^3}{27 M_{\eta}^2 M_{\eta'}^6} - \frac{448 \sqrt{2} c_{\theta}^5 C_{19} M_0^8 M_K^2 M_{\pi}^4 s_{\theta}^3}{3 M_{\eta}^2 M_{\eta'}^6} - \frac{1280 \sqrt{2} c_{\theta}^5 C_{31} M_0^8 M_K^2 M_{\pi}^4 s_{\theta}^3}{9 M_{\eta}^2 M_{\eta'}^6} + \\
& \frac{112 \sqrt{2} c_{\theta}^5 C_{19} M_0^8 M_{\pi}^6 s_{\theta}^3}{9 M_{\eta}^2 M_{\eta'}^6} + \frac{320 \sqrt{2} c_{\theta}^5 C_{31} M_0^8 M_{\pi}^6 s_{\theta}^3}{27 M_{\eta}^2 M_{\eta'}^6} - \frac{3276800 \sqrt{2} c_{\theta}^9 L_8^2 r M_0^8 M_K^{10} s_{\theta}^3}{729 F^2 M_{\eta}^8 M_{\eta'}^4} + \\
& \frac{286720 \sqrt{2} c_{\theta}^9 L_8^2 r M_0^8 M_K^8 M_{\pi}^2 s_{\theta}^3}{27 F^2 M_{\eta}^8 M_{\eta'}^4} - \frac{2048000 \sqrt{2} c_{\theta}^9 L_8^2 r M_0^8 M_K^6 M_{\pi}^4 s_{\theta}^3}{243 F^2 M_{\eta}^8 M_{\eta'}^4} + \\
& \frac{1728512 \sqrt{2} c_{\theta}^9 L_8^2 r M_0^8 M_K^4 M_{\pi}^6 s_{\theta}^3}{729 F^2 M_{\eta}^8 M_{\eta'}^4} - \frac{7168 \sqrt{2} c_{\theta}^9 L_8^2 r M_0^8 M_K^2 M_{\pi}^8 s_{\theta}^3}{243 F^2 M_{\eta}^8 M_{\eta'}^4} + \frac{512 \sqrt{2} c_{\theta}^9 L_8^2 r M_0^8 M_{\pi}^{10} s_{\theta}^3}{27 F^2 M_{\eta}^8 M_{\eta'}^4} + \\
& \frac{128 \sqrt{2} F^2 v_2^{(2)} c_{\theta}^7 M_0^8 M_K^4 s_{\theta}^3}{27 M_{\eta}^6 M_{\eta'}^4} - \frac{20 \sqrt{2} \operatorname{Log}\left[\frac{M_K^2}{\mu^2}\right] c_{\theta}^7 M_0^8 M_K^6 s_{\theta}^3}{243 \pi^2 M_{\eta}^6 M_{\eta'}^4} + \frac{2048 \sqrt{2} c_{\theta}^7 L_6^r M_0^8 M_K^6 s_{\theta}^3}{243 M_{\eta}^6 M_{\eta'}^4} + \\
& \frac{2048 \sqrt{2} c_{\theta}^7 L_7^r M_0^8 M_K^6 s_{\theta}^3}{243 M_{\eta}^6 M_{\eta'}^4} - \frac{5120 \sqrt{2} c_{\theta}^7 L_{25}^r M_0^8 M_K^6 s_{\theta}^3}{81 M_{\eta}^6 M_{\eta'}^4} + \frac{4096 \sqrt{2} c_{\theta}^7 C_{19} M_0^8 M_K^8 s_{\theta}^3}{81 M_{\eta}^6 M_{\eta'}^4} + \\
& \frac{8192 \sqrt{2} c_{\theta}^7 C_{31} M_0^8 M_K^8 s_{\theta}^3}{243 M_{\eta}^6 M_{\eta'}^4} - \frac{16 \sqrt{2} F^2 v_2^{(2)} c_{\theta}^7 M_0^8 M_K^2 M_{\pi}^2 s_{\theta}^3}{27 M_{\eta}^6 M_{\eta'}^4} + \frac{31 \operatorname{Log}\left[\frac{M_K^2}{\mu^2}\right] c_{\theta}^7 M_0^8 M_K^4 M_{\pi}^2 s_{\theta}^3}{972 \sqrt{2} \pi^2 M_{\eta}^6 M_{\eta'}^4} + \\
& \frac{2 \sqrt{2} \operatorname{Log}\left[\frac{M_K^2}{\mu^2}\right] c_{\theta}^7 M_0^8 M_K^4 M_{\pi}^2 s_{\theta}^3}{81 \pi^2 M_{\eta}^6 M_{\eta'}^4} - \frac{704 \sqrt{2} c_{\theta}^7 L_6^r M_0^8 M_K^4 M_{\pi}^2 s_{\theta}^3}{81 M_{\eta}^6 M_{\eta'}^4} + \frac{3904 \sqrt{2} c_{\theta}^7 L_7^r M_0^8 M_K^4 M_{\pi}^2 s_{\theta}^3}{81 M_{\eta}^6 M_{\eta'}^4} + \\
& \frac{6880 \sqrt{2} c_{\theta}^7 L_{25}^r M_0^8 M_K^4 M_{\pi}^2 s_{\theta}^3}{81 M_{\eta}^6 M_{\eta'}^4} - \frac{5248 \sqrt{2} c_{\theta}^7 C_{19} M_0^8 M_K^6 M_{\pi}^2 s_{\theta}^3}{81 M_{\eta}^6 M_{\eta'}^4} - \frac{10496 \sqrt{2} c_{\theta}^7 C_{31} M_0^8 M_K^6 M_{\pi}^2 s_{\theta}^3}{243 M_{\eta}^6 M_{\eta'}^4} -
\end{aligned}$$

$$\begin{aligned}
& \frac{40 \sqrt{2} F^2 v_2^{(2)} c_\theta^7 M_\theta^8 M_\pi^4 s_\theta^3}{27 M_\eta^6 M_{\eta'}^4} + \frac{\text{Log} \left[ \frac{M_K^2}{\mu^2} \right] c_\theta^7 M_\theta^8 M_K^2 M_\pi^4 s_\theta^3}{324 \sqrt{2} \pi^2 M_\eta^6 M_{\eta'}^4} + \frac{5 \text{Log} \left[ \frac{M_\pi^2}{\mu^2} \right] c_\theta^7 M_\theta^8 M_K^2 M_\pi^4 s_\theta^3}{81 \sqrt{2} \pi^2 M_\eta^6 M_{\eta'}^4} - \\
& \frac{640 \sqrt{2} c_\theta^7 L_6^r M_\theta^8 M_K^2 M_\pi^4 s_\theta^3}{81 M_\eta^6 M_{\eta'}^4} - \frac{4960 \sqrt{2} c_\theta^7 L_7^r M_\theta^8 M_K^2 M_\pi^4 s_\theta^3}{81 M_\eta^6 M_{\eta'}^4} - \frac{3296 \sqrt{2} c_\theta^7 L_{25}^r M_\theta^8 M_K^2 M_\pi^4 s_\theta^3}{81 M_\eta^6 M_{\eta'}^4} + \\
& \frac{64 \sqrt{2} c_\theta^7 C_{19} M_\theta^8 M_K^4 M_\pi^4 s_\theta^3}{3 M_\eta^6 M_{\eta'}^4} + \frac{128 \sqrt{2} c_\theta^7 C_{31} M_\theta^8 M_K^4 M_\pi^4 s_\theta^3}{9 M_\eta^6 M_{\eta'}^4} + \frac{\text{Log} \left[ \frac{M_\pi^2}{\mu^2} \right] c_\theta^7 M_\theta^8 M_\pi^6 s_\theta^3}{324 \sqrt{2} \pi^2 M_\eta^6 M_{\eta'}^4} - \\
& \frac{176 \sqrt{2} c_\theta^7 L_6^r M_\theta^8 M_\pi^6 s_\theta^3}{243 M_\eta^6 M_{\eta'}^4} + \frac{2848 \sqrt{2} c_\theta^7 L_7^r M_\theta^8 M_\pi^6 s_\theta^3}{243 M_\eta^6 M_{\eta'}^4} + \frac{320 \sqrt{2} c_\theta^7 L_{25}^r M_\theta^8 M_\pi^6 s_\theta^3}{27 M_\eta^6 M_{\eta'}^4} - \\
& \frac{1120 \sqrt{2} c_\theta^7 C_{19} M_\theta^8 M_K^2 M_\pi^6 s_\theta^3}{81 M_\eta^6 M_{\eta'}^4} - \frac{2240 \sqrt{2} c_\theta^7 C_{31} M_\theta^8 M_K^2 M_\pi^6 s_\theta^3}{243 M_\eta^6 M_{\eta'}^4} - \frac{176 \sqrt{2} c_\theta^7 C_{19} M_\theta^8 M_\pi^8 s_\theta^3}{81 M_\eta^6 M_{\eta'}^4} - \\
& \frac{352 \sqrt{2} c_\theta^7 C_{31} M_\theta^8 M_\pi^8 s_\theta^3}{243 M_\eta^6 M_{\eta'}^4} - \frac{8 \sqrt{2} F^2 v_2^{(2)} c_\theta^5 M_\theta^8 M_K^2 s_\theta^3}{M_\eta^4 M_{\eta'}^4} + \frac{64 \sqrt{2} F^2 v_2^{(2)} c_\theta^5 M_\theta^6 M_K^4 s_\theta^3}{9 M_\eta^4 M_{\eta'}^4} + \\
& \frac{c_\theta^5 M_\theta^8 M_K^4 s_\theta^3}{18 \sqrt{2} \pi^2 M_\eta^4 M_{\eta'}^4} + \frac{17 \text{Log} \left[ \frac{M_K^2}{\mu^2} \right] c_\theta^5 M_\theta^8 M_K^4 s_\theta^3}{180 \sqrt{2} \pi^2 M_\eta^4 M_{\eta'}^4} - \frac{c_\theta^9 M_\theta^8 M_K^4 s_\theta^3}{81 \sqrt{2} \pi^2 M_\eta^4 M_{\eta'}^4} - \frac{14 \sqrt{2} \text{Log} \left[ \frac{M_\eta^2}{\mu^2} \right] c_\theta^9 M_\theta^8 M_K^4 s_\theta^3}{729 \pi^2 M_\eta^4 M_{\eta'}^4} - \\
& \frac{5 \text{Log} \left[ \frac{M_\eta^2}{\mu^2} \right] c_\theta^9 M_\theta^8 M_K^4 s_\theta^3}{81 \sqrt{2} \pi^2 M_\eta^4 M_{\eta'}^4} + \frac{4 \sqrt{2} \text{Log} \left[ \frac{M_{\eta'}^2}{\mu^2} \right] c_\theta^9 M_\theta^8 M_K^4 s_\theta^3}{729 \pi^2 M_\eta^4 M_{\eta'}^4} + \frac{512 \sqrt{2} c_\theta^5 L_6^r M_\theta^8 M_K^4 s_\theta^3}{27 M_\eta^4 M_{\eta'}^4} + \\
& \frac{512 \sqrt{2} c_\theta^5 L_7^r M_\theta^8 M_K^4 s_\theta^3}{27 M_\eta^4 M_{\eta'}^4} + \frac{1792 \sqrt{2} c_\theta^5 C_{19} M_\theta^8 M_K^6 s_\theta^3}{9 M_\eta^4 M_{\eta'}^4} + \frac{5120 \sqrt{2} c_\theta^5 C_{31} M_\theta^8 M_K^6 s_\theta^3}{27 M_\eta^4 M_{\eta'}^4} + \\
& \frac{8 \sqrt{2} F^2 v_2^{(2)} c_\theta^5 M_\theta^8 M_\pi^2 s_\theta^3}{M_\eta^4 M_{\eta'}^4} + \frac{16 \sqrt{2} F^2 v_2^{(2)} c_\theta^5 M_\theta^6 M_K^2 M_\pi^2 s_\theta^3}{9 M_\eta^4 M_{\eta'}^4} - \frac{c_\theta^5 M_\theta^8 M_K^2 M_\pi^2 s_\theta^3}{72 \sqrt{2} \pi^2 M_\eta^4 M_{\eta'}^4} - \\
& \frac{37 \text{Log} \left[ \frac{M_K^2}{\mu^2} \right] c_\theta^5 M_\theta^8 M_K^2 M_\pi^2 s_\theta^3}{1080 \sqrt{2} \pi^2 M_\eta^4 M_{\eta'}^4} + \frac{7 c_\theta^9 M_\theta^8 M_K^2 M_\pi^2 s_\theta^3}{162 \sqrt{2} \pi^2 M_\eta^4 M_{\eta'}^4} + \frac{11 \text{Log} \left[ \frac{M_\eta^2}{\mu^2} \right] c_\theta^9 M_\theta^8 M_K^2 M_\pi^2 s_\theta^3}{324 \sqrt{2} \pi^2 M_\eta^4 M_{\eta'}^4} + \\
& \frac{\sqrt{2} \text{Log} \left[ \frac{M_\eta^2}{\mu^2} \right] c_\theta^9 M_\theta^8 M_K^2 M_\pi^2 s_\theta^3}{729 \pi^2 M_\eta^4 M_{\eta'}^4} + \frac{211 \text{Log} \left[ \frac{M_{\eta'}^2}{\mu^2} \right] c_\theta^9 M_\theta^8 M_K^2 M_\pi^2 s_\theta^3}{2916 \sqrt{2} \pi^2 M_\eta^4 M_{\eta'}^4} - \frac{22 \sqrt{2} \text{Log} \left[ \frac{M_{\eta'}^2}{\mu^2} \right] c_\theta^9 M_\theta^8 M_K^2 M_\pi^2 s_\theta^3}{729 \pi^2 M_\eta^4 M_{\eta'}^4} - \\
& \frac{736 \sqrt{2} c_\theta^5 L_6^r M_\theta^8 M_K^2 M_\pi^2 s_\theta^3}{27 M_\eta^4 M_{\eta'}^4} - \frac{736 \sqrt{2} c_\theta^5 L_7^r M_\theta^8 M_K^2 M_\pi^2 s_\theta^3}{27 M_\eta^4 M_{\eta'}^4} - \frac{896 \sqrt{2} c_\theta^5 C_{19} M_\theta^8 M_K^4 M_\pi^2 s_\theta^3}{3 M_\eta^4 M_{\eta'}^4} - \\
& \frac{2560 \sqrt{2} c_\theta^5 C_{31} M_\theta^8 M_K^4 M_\pi^2 s_\theta^3}{9 M_\eta^4 M_{\eta'}^4} - \frac{8 \sqrt{2} F^2 v_2^{(2)} c_\theta^5 M_\theta^6 M_\pi^4 s_\theta^3}{9 M_\eta^4 M_{\eta'}^4} - \frac{c_\theta^5 M_\theta^8 M_\pi^4 s_\theta^3}{36 \sqrt{2} \pi^2 M_\eta^4 M_{\eta'}^4} - \\
& \frac{\text{Log} \left[ \frac{M_K^2}{\mu^2} \right] c_\theta^5 M_\theta^8 M_\pi^4 s_\theta^3}{144 \sqrt{2} \pi^2 M_\eta^4 M_{\eta'}^4} - \frac{\text{Log} \left[ \frac{M_\pi^2}{\mu^2} \right] c_\theta^5 M_\theta^8 M_\pi^4 s_\theta^3}{36 \sqrt{2} \pi^2 M_\eta^4 M_{\eta'}^4} - \frac{25 c_\theta^9 M_\theta^8 M_\pi^4 s_\theta^3}{1296 \sqrt{2} \pi^2 M_\eta^4 M_{\eta'}^4} - \frac{79 \text{Log} \left[ \frac{M_\eta^2}{\mu^2} \right] c_\theta^9 M_\theta^8 M_\pi^4 s_\theta^3}{11664 \sqrt{2} \pi^2 M_\eta^4 M_{\eta'}^4} -
\end{aligned}$$

$$\begin{aligned}
& \frac{47 \operatorname{Log}\left[\frac{M_\eta^2}{\mu^2}\right] c_\theta^9 M_0^8 M_\pi^4 s_\theta^3}{5832 \sqrt{2} \pi^2 M_\eta^4 M_{\eta'}^4} + \frac{\sqrt{2} \operatorname{Log}\left[\frac{M_{\eta'}^2}{\mu^2}\right] c_\theta^9 M_0^8 M_\pi^4 s_\theta^3}{243 \pi^2 M_\eta^4 M_{\eta'}^4} + \frac{368 \sqrt{2} c_\theta^5 L_6^r M_0^8 M_\pi^4 s_\theta^3}{27 M_\eta^4 M_{\eta'}^4} + \\
& \frac{368 \sqrt{2} c_\theta^5 L_7^r M_0^8 M_\pi^4 s_\theta^3}{27 M_\eta^4 M_{\eta'}^4} + \frac{448 \sqrt{2} c_\theta^5 C_{19} M_0^8 M_K^2 M_\pi^4 s_\theta^3}{3 M_\eta^4 M_{\eta'}^4} + \frac{1280 \sqrt{2} c_\theta^5 C_{31} M_0^8 M_K^2 M_\pi^4 s_\theta^3}{9 M_\eta^4 M_{\eta'}^4} - \\
& \frac{112 \sqrt{2} c_\theta^5 C_{19} M_0^8 M_\pi^6 s_\theta^3}{9 M_\eta^4 M_{\eta'}^4} - \frac{320 \sqrt{2} c_\theta^5 C_{31} M_0^8 M_\pi^6 s_\theta^3}{27 M_\eta^4 M_{\eta'}^4} + \frac{5 \operatorname{Log}\left[\frac{M_{\eta'}^2}{\mu^2}\right] c_\theta^7 M_0^8 M_K^2 s_\theta^3}{162 \sqrt{2} \pi^2 M_\eta^2 M_{\eta'}^4} - \\
& \frac{\operatorname{Log}\left[\frac{M_\eta^2}{\mu^2}\right] c_\theta^7 M_0^8 M_\pi^2 s_\theta^3}{432 \sqrt{2} \pi^2 M_\eta^2 M_{\eta'}^4} - \frac{5 \operatorname{Log}\left[\frac{M_{\eta'}^2}{\mu^2}\right] c_\theta^7 M_0^8 M_\pi^2 s_\theta^3}{324 \sqrt{2} \pi^2 M_\eta^2 M_{\eta'}^4} - \frac{1310720 \sqrt{2} c_\theta^9 L_8^2 r M_0^8 M_K^{10} s_\theta^3}{729 F^2 M_\eta^{10} M_{\eta'}^2} + \\
& \frac{1114112 \sqrt{2} c_\theta^9 L_8^2 r M_0^8 M_K^2 M_\pi^2 s_\theta^3}{243 F^2 M_\eta^{10} M_{\eta'}^2} - \frac{131072 \sqrt{2} c_\theta^9 L_8^2 r M_0^8 M_K^6 M_\pi^4 s_\theta^3}{27 F^2 M_\eta^{10} M_{\eta'}^2} + \\
& \frac{1961984 \sqrt{2} c_\theta^9 L_8^2 r M_0^8 M_K^4 M_\pi^6 s_\theta^3}{729 F^2 M_\eta^{10} M_{\eta'}^2} - \frac{188416 \sqrt{2} c_\theta^9 L_8^2 r M_0^8 M_K^2 M_\pi^8 s_\theta^3}{243 F^2 M_\eta^{10} M_{\eta'}^2} + \\
& \frac{2560 \sqrt{2} c_\theta^9 L_8^2 r M_0^8 M_\pi^{10} s_\theta^3}{27 F^2 M_\eta^{10} M_{\eta'}^2} - \frac{2 \sqrt{2} \operatorname{Log}\left[\frac{M_K^2}{\mu^2}\right] c_\theta^7 M_0^8 M_K^6 s_\theta^3}{243 \pi^2 M_\eta^8 M_{\eta'}^2} + \frac{4096 \sqrt{2} c_\theta^7 L_6^r M_0^8 M_K^6 s_\theta^3}{243 M_\eta^8 M_{\eta'}^2} + \\
& \frac{4096 \sqrt{2} c_\theta^7 L_7^r M_0^8 M_K^6 s_\theta^3}{243 M_\eta^8 M_{\eta'}^2} - \frac{512 \sqrt{2} c_\theta^7 L_{25}^r M_0^8 M_K^6 s_\theta^3}{81 M_\eta^8 M_{\eta'}^2} + \frac{8192 \sqrt{2} c_\theta^7 C_{19} M_0^8 M_K^8 s_\theta^3}{81 M_\eta^8 M_{\eta'}^2} + \\
& \frac{16384 \sqrt{2} c_\theta^7 C_{31} M_0^8 M_K^8 s_\theta^3}{243 M_\eta^8 M_{\eta'}^2} + \frac{19 \operatorname{Log}\left[\frac{M_K^2}{\mu^2}\right] c_\theta^7 M_0^8 M_K^4 M_\pi^2 s_\theta^3}{972 \sqrt{2} \pi^2 M_\eta^8 M_{\eta'}^2} + \frac{\sqrt{2} \operatorname{Log}\left[\frac{M_K^2}{\mu^2}\right] c_\theta^7 M_0^8 M_K^4 M_\pi^2 s_\theta^3}{243 \pi^2 M_\eta^8 M_{\eta'}^2} - \\
& \frac{704 \sqrt{2} c_\theta^7 L_6^r M_0^8 M_K^4 M_\pi^2 s_\theta^3}{81 M_\eta^8 M_{\eta'}^2} - \frac{3008 \sqrt{2} c_\theta^7 L_7^r M_0^8 M_K^4 M_\pi^2 s_\theta^3}{81 M_\eta^8 M_{\eta'}^2} + \frac{736 \sqrt{2} c_\theta^7 L_{25}^r M_0^8 M_K^4 M_\pi^2 s_\theta^3}{81 M_\eta^8 M_{\eta'}^2} - \\
& \frac{17024 \sqrt{2} c_\theta^7 C_{19} M_0^8 M_K^6 M_\pi^2 s_\theta^3}{81 M_\eta^8 M_{\eta'}^2} - \frac{34048 \sqrt{2} c_\theta^7 C_{31} M_0^8 M_K^6 M_\pi^2 s_\theta^3}{243 M_\eta^8 M_{\eta'}^2} - \frac{11 \operatorname{Log}\left[\frac{M_K^2}{\mu^2}\right] c_\theta^7 M_0^8 M_K^2 M_\pi^4 s_\theta^3}{972 \sqrt{2} \pi^2 M_\eta^8 M_{\eta'}^2} - \\
& \frac{\operatorname{Log}\left[\frac{M_\pi^2}{\mu^2}\right] c_\theta^7 M_0^8 M_K^2 M_\pi^4 s_\theta^3}{162 \sqrt{2} \pi^2 M_\eta^8 M_{\eta'}^2} - \frac{128 \sqrt{2} c_\theta^7 L_6^r M_0^8 M_K^2 M_\pi^4 s_\theta^3}{27 M_\eta^8 M_{\eta'}^2} + \frac{736 \sqrt{2} c_\theta^7 L_7^r M_0^8 M_K^2 M_\pi^4 s_\theta^3}{27 M_\eta^8 M_{\eta'}^2} - \\
& \frac{224 \sqrt{2} c_\theta^7 L_{25}^r M_0^8 M_K^2 M_\pi^4 s_\theta^3}{81 M_\eta^8 M_{\eta'}^2} + \frac{1472 \sqrt{2} c_\theta^7 C_{19} M_0^8 M_K^4 M_\pi^4 s_\theta^3}{9 M_\eta^8 M_{\eta'}^2} + \frac{2944 \sqrt{2} c_\theta^7 C_{31} M_0^8 M_K^4 M_\pi^4 s_\theta^3}{27 M_\eta^8 M_{\eta'}^2} + \\
& \frac{\operatorname{Log}\left[\frac{M_\pi^2}{\mu^2}\right] c_\theta^7 M_0^8 M_\pi^6 s_\theta^3}{162 \sqrt{2} \pi^2 M_\eta^8 M_{\eta'}^2} + \frac{464 \sqrt{2} c_\theta^7 L_6^r M_0^8 M_\pi^6 s_\theta^3}{243 M_\eta^8 M_{\eta'}^2} - \frac{1696 \sqrt{2} c_\theta^7 L_7^r M_0^8 M_\pi^6 s_\theta^3}{243 M_\eta^8 M_{\eta'}^2} - \\
& \frac{4448 \sqrt{2} c_\theta^7 C_{19} M_0^8 M_K^2 M_\pi^6 s_\theta^3}{81 M_\eta^8 M_{\eta'}^2} - \frac{8896 \sqrt{2} c_\theta^7 C_{31} M_0^8 M_K^2 M_\pi^6 s_\theta^3}{243 M_\eta^8 M_{\eta'}^2} + \frac{464 \sqrt{2} c_\theta^7 C_{19} M_0^8 M_\pi^8 s_\theta^3}{81 M_\eta^8 M_{\eta'}^2} +
\end{aligned}$$

$$\begin{aligned}
& \frac{928 \sqrt{2} c_\theta^7 C_{31} M_\theta^8 M_\pi^8 s_\theta^3}{243 M_\eta^6 M_{\eta'}^2} - \frac{128 \sqrt{2} F^2 v_2^{(2)} c_\theta^5 M_\theta^6 M_K^4 s_\theta^3}{27 M_\eta^6 M_{\eta'}^2} - \frac{11 \text{Log} \left[ \frac{M_K^2}{\mu^2} \right] c_\theta^5 M_\theta^8 M_K^4 s_\theta^3}{1620 \sqrt{2} \pi^2 M_\eta^6 M_{\eta'}^2} + \\
& \frac{5 \sqrt{2} c_\theta^9 M_\theta^8 M_K^4 s_\theta^3}{243 \pi^2 M_\eta^6 M_{\eta'}^2} - \frac{4 \sqrt{2} \text{Log} \left[ \frac{M_\eta^2}{\mu^2} \right] c_\theta^9 M_\theta^8 M_K^4 s_\theta^3}{729 \pi^2 M_\eta^6 M_{\eta'}^2} + \frac{23 \sqrt{2} \text{Log} \left[ \frac{M_{\eta'}^2}{\mu^2} \right] c_\theta^9 M_\theta^8 M_K^4 s_\theta^3}{729 \pi^2 M_\eta^6 M_{\eta'}^2} - \\
& \frac{1024 \sqrt{2} c_\theta^5 L_6^r M_\theta^8 M_K^4 s_\theta^3}{81 M_\eta^6 M_{\eta'}^2} - \frac{1024 \sqrt{2} c_\theta^5 L_7^r M_\theta^8 M_K^4 s_\theta^3}{81 M_\eta^6 M_{\eta'}^2} - \frac{3584 \sqrt{2} c_\theta^5 C_{19} M_\theta^8 M_K^6 s_\theta^3}{27 M_\eta^6 M_{\eta'}^2} - \\
& \frac{10240 \sqrt{2} c_\theta^5 C_{31} M_\theta^8 M_K^6 s_\theta^3}{81 M_\eta^6 M_{\eta'}^2} + \frac{16 \sqrt{2} F^2 v_2^{(2)} c_\theta^5 M_\theta^6 M_K^2 M_\pi^2 s_\theta^3}{27 M_\eta^6 M_{\eta'}^2} - \frac{c_\theta^5 M_\theta^8 M_K^2 M_\pi^2 s_\theta^3}{216 \sqrt{2} \pi^2 M_\eta^6 M_{\eta'}^2} - \\
& \frac{\text{Log} \left[ \frac{M_K^2}{\mu^2} \right] c_\theta^5 M_\theta^8 M_K^2 M_\pi^2 s_\theta^3}{1080 \sqrt{2} \pi^2 M_\eta^6 M_{\eta'}^2} - \frac{11 c_\theta^9 M_\theta^8 M_K^2 M_\pi^2 s_\theta^3}{243 \sqrt{2} \pi^2 M_\eta^6 M_{\eta'}^2} - \frac{\text{Log} \left[ \frac{M_\eta^2}{\mu^2} \right] c_\theta^9 M_\theta^8 M_K^2 M_\pi^2 s_\theta^3}{486 \sqrt{2} \pi^2 M_\eta^6 M_{\eta'}^2} + \\
& \frac{5 \sqrt{2} \text{Log} \left[ \frac{M_\eta^2}{\mu^2} \right] c_\theta^9 M_\theta^8 M_K^2 M_\pi^2 s_\theta^3}{729 \pi^2 M_\eta^6 M_{\eta'}^2} - \frac{5 \text{Log} \left[ \frac{M_{\eta'}^2}{\mu^2} \right] c_\theta^9 M_\theta^8 M_K^2 M_\pi^2 s_\theta^3}{2916 \sqrt{2} \pi^2 M_\eta^6 M_{\eta'}^2} - \frac{2 \sqrt{2} \text{Log} \left[ \frac{M_{\eta'}^2}{\mu^2} \right] c_\theta^9 M_\theta^8 M_K^2 M_\pi^2 s_\theta^3}{81 \pi^2 M_\eta^6 M_{\eta'}^2} + \\
& \frac{992 \sqrt{2} c_\theta^5 L_6^r M_\theta^8 M_K^2 M_\pi^2 s_\theta^3}{81 M_\eta^6 M_{\eta'}^2} + \frac{992 \sqrt{2} c_\theta^5 L_7^r M_\theta^8 M_K^2 M_\pi^2 s_\theta^3}{81 M_\eta^6 M_{\eta'}^2} + \frac{1792 \sqrt{2} c_\theta^5 C_{19} M_\theta^8 M_K^4 M_\pi^2 s_\theta^3}{9 M_\eta^6 M_{\eta'}^2} + \\
& \frac{5120 \sqrt{2} c_\theta^5 C_{31} M_\theta^8 M_K^4 M_\pi^2 s_\theta^3}{27 M_\eta^6 M_{\eta'}^2} + \frac{40 \sqrt{2} F^2 v_2^{(2)} c_\theta^5 M_\theta^6 M_\pi^4 s_\theta^3}{27 M_\eta^6 M_{\eta'}^2} - \frac{c_\theta^5 M_\theta^8 M_\pi^4 s_\theta^3}{216 \sqrt{2} \pi^2 M_\eta^6 M_{\eta'}^2} + \\
& \frac{\text{Log} \left[ \frac{M_K^2}{\mu^2} \right] c_\theta^5 M_\theta^8 M_\pi^4 s_\theta^3}{432 \sqrt{2} \pi^2 M_\eta^6 M_{\eta'}^2} - \frac{\text{Log} \left[ \frac{M_\pi^2}{\mu^2} \right] c_\theta^5 M_\theta^8 M_\pi^4 s_\theta^3}{108 \sqrt{2} \pi^2 M_\eta^6 M_{\eta'}^2} + \frac{11 c_\theta^9 M_\theta^8 M_\pi^4 s_\theta^3}{3888 \sqrt{2} \pi^2 M_\eta^6 M_{\eta'}^2} + \frac{\sqrt{2} c_\theta^9 M_\theta^8 M_\pi^4 s_\theta^3}{243 \pi^2 M_\eta^6 M_{\eta'}^2} - \\
& \frac{131 \text{Log} \left[ \frac{M_\eta^2}{\mu^2} \right] c_\theta^9 M_\theta^8 M_\pi^4 s_\theta^3}{11664 \sqrt{2} \pi^2 M_\eta^6 M_{\eta'}^2} + \frac{\sqrt{2} \text{Log} \left[ \frac{M_\eta^2}{\mu^2} \right] c_\theta^9 M_\theta^8 M_\pi^4 s_\theta^3}{243 \pi^2 M_\eta^6 M_{\eta'}^2} + \frac{83 \text{Log} \left[ \frac{M_{\eta'}^2}{\mu^2} \right] c_\theta^9 M_\theta^8 M_\pi^4 s_\theta^3}{5832 \sqrt{2} \pi^2 M_\eta^6 M_{\eta'}^2} - \\
& \frac{112 \sqrt{2} c_\theta^5 L_6^r M_\theta^8 M_\pi^4 s_\theta^3}{81 M_\eta^6 M_{\eta'}^2} - \frac{112 \sqrt{2} c_\theta^5 L_7^r M_\theta^8 M_\pi^4 s_\theta^3}{81 M_\eta^6 M_{\eta'}^2} - \frac{896 \sqrt{2} c_\theta^5 C_{19} M_\theta^8 M_K^2 M_\pi^4 s_\theta^3}{9 M_\eta^6 M_{\eta'}^2} - \\
& \frac{2560 \sqrt{2} c_\theta^5 C_{31} M_\theta^8 M_K^2 M_\pi^4 s_\theta^3}{27 M_\eta^6 M_{\eta'}^2} + \frac{560 \sqrt{2} c_\theta^5 C_{19} M_\theta^8 M_\pi^6 s_\theta^3}{27 M_\eta^6 M_{\eta'}^2} + \frac{1600 \sqrt{2} c_\theta^5 C_{31} M_\theta^8 M_\pi^6 s_\theta^3}{81 M_\eta^6 M_{\eta'}^2} + \\
& \frac{\sqrt{2} \text{Log} \left[ \frac{M_\eta^2}{\mu^2} \right] c_\theta^7 M_\theta^8 M_K^2 s_\theta^3}{243 \pi^2 M_\eta^4 M_{\eta'}^2} - \frac{\text{Log} \left[ \frac{M_{\eta'}^2}{\mu^2} \right] c_\theta^7 M_\theta^8 M_K^2 s_\theta^3}{54 \sqrt{2} \pi^2 M_\eta^4 M_{\eta'}^2} - \frac{17 \text{Log} \left[ \frac{M_\eta^2}{\mu^2} \right] c_\theta^7 M_\theta^8 M_\pi^2 s_\theta^3}{3888 \sqrt{2} \pi^2 M_\eta^4 M_{\eta'}^2} + \\
& \frac{\text{Log} \left[ \frac{M_{\eta'}^2}{\mu^2} \right] c_\theta^7 M_\theta^8 M_\pi^2 s_\theta^3}{108 \sqrt{2} \pi^2 M_\eta^4 M_{\eta'}^2} + \frac{8 \sqrt{2} F^2 v_2^{(2)} c_\theta M_\theta^4 M_K^2 s_\theta^3}{3 M_\eta^2 M_{\eta'}^2} - \frac{8 \sqrt{2} F^2 v_2^{(2)} c_\theta M_\theta^4 M_\pi^2 s_\theta^3}{3 M_\eta^2 M_{\eta'}^2} - \\
& \frac{4 \sqrt{2} \text{Log} \left[ \frac{M_\eta^2}{\mu^2} \right] c_\theta^9 M_\theta^8 M_K^4 s_\theta^3}{243 \pi^2 M_\eta^6 (M_\eta^2 - M_{\eta'}^2)} + \frac{7 \text{Log} \left[ \frac{M_{\eta'}^2}{\mu^2} \right] c_\theta^9 M_\theta^8 M_K^2 M_\pi^2 s_\theta^3}{243 \sqrt{2} \pi^2 M_\eta^6 (M_\eta^2 - M_{\eta'}^2)} + \frac{\text{Log} \left[ \frac{M_{\eta'}^2}{\mu^2} \right] c_\theta^9 M_\theta^8 M_\pi^4 s_\theta^3}{324 \sqrt{2} \pi^2 M_\eta^6 (M_\eta^2 - M_{\eta'}^2)} -
\end{aligned}$$



$$\begin{aligned}
& \frac{\sqrt{2} \operatorname{Log}\left[\frac{M_{\eta'}^2}{\mu^2}\right] c_{\theta}^9 M_0^8 M_{\pi}^4 s_{\theta}^3}{243 \pi^2 M_{\eta'}^6 (M_{\eta}^2 - M_{\eta'}^2)} - \frac{13 \operatorname{Log}\left[\frac{M_{\eta}^2}{\mu^2}\right] c_{\theta}^9 M_0^8 M_K^4 M_{\eta}^2 s_{\theta}^3}{243 \sqrt{2} \pi^2 M_{\eta'}^8 (M_{\eta}^2 - M_{\eta'}^2)} + \frac{4 \sqrt{2} \operatorname{Log}\left[\frac{M_{\eta'}^2}{\mu^2}\right] c_{\theta}^9 M_0^8 M_K^2 M_{\pi}^2 M_{\eta}^2 s_{\theta}^3}{243 \pi^2 M_{\eta'}^8 (M_{\eta}^2 - M_{\eta'}^2)} - \\
& \frac{7 \operatorname{Log}\left[\frac{M_{\eta}^2}{\mu^2}\right] c_{\theta}^9 M_0^8 M_{\pi}^4 M_{\eta}^2 s_{\theta}^3}{972 \sqrt{2} \pi^2 M_{\eta'}^8 (M_{\eta}^2 - M_{\eta'}^2)} + \frac{13 \sqrt{2} \operatorname{Log}\left[\frac{M_{\eta}^2}{\mu^2}\right] c_{\theta}^9 M_0^8 M_K^4 s_{\theta}^3}{243 \pi^2 M_{\eta'}^6 (M_{\eta}^2 - M_{\eta'}^2)} + \frac{13 \operatorname{Log}\left[\frac{M_{\eta'}^2}{\mu^2}\right] c_{\theta}^9 M_0^8 M_K^4 s_{\theta}^3}{243 \sqrt{2} \pi^2 M_{\eta'}^6 (M_{\eta}^2 - M_{\eta'}^2)} + \\
& \frac{29 \operatorname{Log}\left[\frac{M_{\eta}^2}{\mu^2}\right] c_{\theta}^9 M_0^8 M_K^2 M_{\pi}^2 s_{\theta}^3}{486 \sqrt{2} \pi^2 M_{\eta'}^6 (M_{\eta}^2 - M_{\eta'}^2)} - \frac{13 \sqrt{2} \operatorname{Log}\left[\frac{M_{\eta}^2}{\mu^2}\right] c_{\theta}^9 M_0^8 M_K^2 M_{\pi}^2 s_{\theta}^3}{243 \pi^2 M_{\eta'}^6 (M_{\eta}^2 - M_{\eta'}^2)} - \frac{4 \sqrt{2} \operatorname{Log}\left[\frac{M_{\eta'}^2}{\mu^2}\right] c_{\theta}^9 M_0^8 M_K^2 M_{\pi}^2 s_{\theta}^3}{243 \pi^2 M_{\eta'}^6 (M_{\eta}^2 - M_{\eta'}^2)} - \\
& \frac{\operatorname{Log}\left[\frac{M_{\eta}^2}{\mu^2}\right] c_{\theta}^9 M_0^8 M_{\pi}^4 s_{\theta}^3}{324 \sqrt{2} \pi^2 M_{\eta'}^6 (M_{\eta}^2 - M_{\eta'}^2)} + \frac{\sqrt{2} \operatorname{Log}\left[\frac{M_{\eta}^2}{\mu^2}\right] c_{\theta}^9 M_0^8 M_{\pi}^4 s_{\theta}^3}{243 \pi^2 M_{\eta'}^6 (M_{\eta}^2 - M_{\eta'}^2)} + \frac{7 \operatorname{Log}\left[\frac{M_{\eta'}^2}{\mu^2}\right] c_{\theta}^9 M_0^8 M_{\pi}^4 s_{\theta}^3}{972 \sqrt{2} \pi^2 M_{\eta'}^6 (M_{\eta}^2 - M_{\eta'}^2)} - \\
& \frac{4 \sqrt{2} \operatorname{Log}\left[\frac{M_{\eta}^2}{\mu^2}\right] c_{\theta}^9 M_0^8 M_K^4 s_{\theta}^3}{81 \pi^2 M_{\eta}^2 M_{\eta'}^4 (M_{\eta}^2 - M_{\eta'}^2)} - \frac{13 \sqrt{2} \operatorname{Log}\left[\frac{M_{\eta}^2}{\mu^2}\right] c_{\theta}^9 M_0^8 M_K^4 s_{\theta}^3}{243 \pi^2 M_{\eta}^2 M_{\eta'}^4 (M_{\eta}^2 - M_{\eta'}^2)} - \frac{5 \operatorname{Log}\left[\frac{M_{\eta}^2}{\mu^2}\right] c_{\theta}^9 M_0^8 M_K^2 M_{\pi}^2 s_{\theta}^3}{162 \sqrt{2} \pi^2 M_{\eta}^2 M_{\eta'}^4 (M_{\eta}^2 - M_{\eta'}^2)} + \\
& \frac{4 \sqrt{2} \operatorname{Log}\left[\frac{M_{\eta}^2}{\mu^2}\right] c_{\theta}^9 M_0^8 M_K^2 M_{\pi}^2 s_{\theta}^3}{81 \pi^2 M_{\eta}^2 M_{\eta'}^4 (M_{\eta}^2 - M_{\eta'}^2)} - \frac{29 \operatorname{Log}\left[\frac{M_{\eta}^2}{\mu^2}\right] c_{\theta}^9 M_0^8 M_K^2 M_{\pi}^2 s_{\theta}^3}{486 \sqrt{2} \pi^2 M_{\eta}^2 M_{\eta'}^4 (M_{\eta}^2 - M_{\eta'}^2)} + \frac{13 \sqrt{2} \operatorname{Log}\left[\frac{M_{\eta'}^2}{\mu^2}\right] c_{\theta}^9 M_0^8 M_K^2 M_{\pi}^2 s_{\theta}^3}{243 \pi^2 M_{\eta}^2 M_{\eta'}^4 (M_{\eta}^2 - M_{\eta'}^2)} + \\
& \frac{\operatorname{Log}\left[\frac{M_{\eta}^2}{\mu^2}\right] c_{\theta}^9 M_0^8 M_{\pi}^4 s_{\theta}^3}{108 \sqrt{2} \pi^2 M_{\eta}^2 M_{\eta'}^4 (M_{\eta}^2 - M_{\eta'}^2)} - \frac{\sqrt{2} \operatorname{Log}\left[\frac{M_{\eta}^2}{\mu^2}\right] c_{\theta}^9 M_0^8 M_{\pi}^4 s_{\theta}^3}{81 \pi^2 M_{\eta}^2 M_{\eta'}^4 (M_{\eta}^2 - M_{\eta'}^2)} + \frac{\operatorname{Log}\left[\frac{M_{\eta'}^2}{\mu^2}\right] c_{\theta}^9 M_0^8 M_{\pi}^4 s_{\theta}^3}{324 \sqrt{2} \pi^2 M_{\eta}^2 M_{\eta'}^4 (M_{\eta}^2 - M_{\eta'}^2)} - \\
& \frac{\sqrt{2} \operatorname{Log}\left[\frac{M_{\eta'}^2}{\mu^2}\right] c_{\theta}^9 M_0^8 M_{\pi}^4 s_{\theta}^3}{243 \pi^2 M_{\eta}^2 M_{\eta'}^4 (M_{\eta}^2 - M_{\eta'}^2)} + \frac{4 \sqrt{2} \operatorname{Log}\left[\frac{M_{\eta}^2}{\mu^2}\right] c_{\theta}^9 M_0^8 M_K^4 s_{\theta}^3}{243 \pi^2 M_{\eta}^4 M_{\eta'}^2 (M_{\eta}^2 - M_{\eta'}^2)} + \frac{4 \sqrt{2} \operatorname{Log}\left[\frac{M_{\eta'}^2}{\mu^2}\right] c_{\theta}^9 M_0^8 M_K^4 s_{\theta}^3}{81 \pi^2 M_{\eta}^4 M_{\eta'}^2 (M_{\eta}^2 - M_{\eta'}^2)} - \\
& \frac{7 \operatorname{Log}\left[\frac{M_{\eta}^2}{\mu^2}\right] c_{\theta}^9 M_0^8 M_K^2 M_{\pi}^2 s_{\theta}^3}{243 \sqrt{2} \pi^2 M_{\eta}^4 M_{\eta'}^2 (M_{\eta}^2 - M_{\eta'}^2)} + \frac{5 \operatorname{Log}\left[\frac{M_{\eta'}^2}{\mu^2}\right] c_{\theta}^9 M_0^8 M_K^2 M_{\pi}^2 s_{\theta}^3}{162 \sqrt{2} \pi^2 M_{\eta}^4 M_{\eta'}^2 (M_{\eta}^2 - M_{\eta'}^2)} - \frac{4 \sqrt{2} \operatorname{Log}\left[\frac{M_{\eta'}^2}{\mu^2}\right] c_{\theta}^9 M_0^8 M_K^2 M_{\pi}^2 s_{\theta}^3}{81 \pi^2 M_{\eta}^4 M_{\eta'}^2 (M_{\eta}^2 - M_{\eta'}^2)} - \\
& \frac{\operatorname{Log}\left[\frac{M_{\eta}^2}{\mu^2}\right] c_{\theta}^9 M_0^8 M_{\pi}^4 s_{\theta}^3}{324 \sqrt{2} \pi^2 M_{\eta}^4 M_{\eta'}^2 (M_{\eta}^2 - M_{\eta'}^2)} + \frac{\sqrt{2} \operatorname{Log}\left[\frac{M_{\eta}^2}{\mu^2}\right] c_{\theta}^9 M_0^8 M_{\pi}^4 s_{\theta}^3}{243 \pi^2 M_{\eta}^4 M_{\eta'}^2 (M_{\eta}^2 - M_{\eta'}^2)} - \frac{\operatorname{Log}\left[\frac{M_{\eta'}^2}{\mu^2}\right] c_{\theta}^9 M_0^8 M_{\pi}^4 s_{\theta}^3}{108 \sqrt{2} \pi^2 M_{\eta}^4 M_{\eta'}^2 (M_{\eta}^2 - M_{\eta'}^2)} + \\
& \frac{\sqrt{2} \operatorname{Log}\left[\frac{M_{\eta'}^2}{\mu^2}\right] c_{\theta}^9 M_0^8 M_{\pi}^4 s_{\theta}^3}{81 \pi^2 M_{\eta}^4 M_{\eta'}^2 (M_{\eta}^2 - M_{\eta'}^2)} - \frac{655 360 c_{\theta}^8 L_8^2 r M_0^8 M_K^{10} s_{\theta}^4}{729 F^2 M_{\eta}^{12}} + \frac{532 480 c_{\theta}^8 L_8^2 r M_0^8 M_K^8 M_{\pi}^2 s_{\theta}^4}{243 F^2 M_{\eta}^{12}} - \\
& \frac{573 440 c_{\theta}^8 L_8^2 r M_0^8 M_K^6 M_{\pi}^4 s_{\theta}^4}{243 F^2 M_{\eta}^{12}} + \frac{993 280 c_{\theta}^8 L_8^2 r M_0^8 M_K^4 M_{\pi}^6 s_{\theta}^4}{729 F^2 M_{\eta}^{12}} - \frac{102 400 c_{\theta}^8 L_8^2 r M_0^8 M_K^2 M_{\pi}^8 s_{\theta}^4}{243 F^2 M_{\eta}^{12}} + \\
& \frac{4480 c_{\theta}^8 L_8^2 r M_0^8 M_{\pi}^{10} s_{\theta}^4}{81 F^2 M_{\eta}^{12}} + \frac{2048 c_{\theta}^6 L_6^r M_0^8 M_K^6 s_{\theta}^4}{243 M_{\eta}^{10}} + \frac{2048 c_{\theta}^6 L_7^r M_0^8 M_K^6 s_{\theta}^4}{243 M_{\eta}^{10}} + \frac{4096 c_{\theta}^6 C_{19} M_0^8 M_K^8 s_{\theta}^4}{81 M_{\eta}^{10}} + \\
& \frac{8192 c_{\theta}^6 C_{31} M_0^8 M_K^8 s_{\theta}^4}{243 M_{\eta}^{10}} + \frac{\operatorname{Log}\left[\frac{M_K^2}{\mu^2}\right] c_{\theta}^6 M_0^8 M_K^4 M_{\pi}^2 s_{\theta}^4}{243 \pi^2 M_{\eta}^{10}} - \frac{128 c_{\theta}^6 L_6^r M_0^8 M_K^4 M_{\pi}^2 s_{\theta}^4}{81 M_{\eta}^{10}} -
\end{aligned}$$

$$\begin{aligned}
& \frac{1664 c_\theta^6 L_7^r M_0^8 M_K^4 M_\pi^2 s_\theta^4}{81 M_\eta^{10}} - \frac{7936 c_\theta^6 C_{19} M_0^8 M_K^6 M_\pi^2 s_\theta^4}{81 M_\eta^{10}} - \frac{15872 c_\theta^6 C_{31} M_0^8 M_K^6 M_\pi^2 s_\theta^4}{243 M_\eta^{10}} - \\
& \frac{7 \operatorname{Log}\left[\frac{M_K^2}{\mu^2}\right] c_\theta^6 M_0^8 M_K^2 M_\pi^4 s_\theta^4}{3888 \pi^2 M_\eta^{10}} - \frac{\operatorname{Log}\left[\frac{M_\pi^2}{\mu^2}\right] c_\theta^6 M_0^8 M_K^2 M_\pi^4 s_\theta^4}{162 \pi^2 M_\eta^{10}} - \frac{160 c_\theta^6 L_6^r M_0^8 M_K^2 M_\pi^4 s_\theta^4}{81 M_\eta^{10}} + \\
& \frac{1280 c_\theta^6 L_7^r M_0^8 M_K^2 M_\pi^4 s_\theta^4}{81 M_\eta^{10}} + \frac{640 c_\theta^6 C_{19} M_0^8 M_K^4 M_\pi^4 s_\theta^4}{9 M_\eta^{10}} + \frac{1280 c_\theta^6 C_{31} M_0^8 M_K^4 M_\pi^4 s_\theta^4}{27 M_\eta^{10}} + \\
& \frac{7 \operatorname{Log}\left[\frac{M_\pi^2}{\mu^2}\right] c_\theta^6 M_0^8 M_\pi^6 s_\theta^4}{2592 \pi^2 M_\eta^{10}} + \frac{112 c_\theta^6 L_6^r M_0^8 M_\pi^6 s_\theta^4}{243 M_\eta^{10}} - \frac{896 c_\theta^6 L_7^r M_0^8 M_\pi^6 s_\theta^4}{243 M_\eta^{10}} - \frac{1600 c_\theta^6 C_{19} M_0^8 M_K^2 M_\pi^6 s_\theta^4}{81 M_\eta^{10}} - \\
& \frac{3200 c_\theta^6 C_{31} M_0^8 M_K^2 M_\pi^6 s_\theta^4}{243 M_\eta^{10}} + \frac{112 c_\theta^6 C_{19} M_0^8 M_\pi^8 s_\theta^4}{81 M_\eta^{10}} + \frac{224 c_\theta^6 C_{31} M_0^8 M_\pi^8 s_\theta^4}{243 M_\eta^{10}} - \frac{g1Dk c_\theta^4 M_0^8 s_\theta^4}{30 M_\eta^8} - \\
& \frac{64 F^2 v_2^{(2)} c_\theta^4 M_0^6 M_K^4 s_\theta^4}{27 M_\eta^8} - \frac{\operatorname{Log}\left[\frac{M_K^2}{\mu^2}\right] c_\theta^4 M_0^8 M_K^4 s_\theta^4}{1620 \pi^2 M_\eta^8} + \frac{5 c_\theta^8 M_0^8 M_K^4 s_\theta^4}{486 \pi^2 M_\eta^8} - \frac{2 \operatorname{Log}\left[\frac{M_\pi^2}{\mu^2}\right] c_\theta^8 M_0^8 M_K^4 s_\theta^4}{729 \pi^2 M_\eta^8} + \\
& \frac{5 \operatorname{Log}\left[\frac{M_\eta^2}{\mu^2}\right] c_\theta^8 M_0^8 M_K^4 s_\theta^4}{486 \pi^2 M_\eta^8} - \frac{512 c_\theta^4 L_6^r M_0^8 M_K^4 s_\theta^4}{81 M_\eta^8} - \frac{512 c_\theta^4 L_7^r M_0^8 M_K^4 s_\theta^4}{81 M_\eta^8} - \frac{1792 c_\theta^4 C_{19} M_0^8 M_K^6 s_\theta^4}{27 M_\eta^8} - \\
& \frac{5120 c_\theta^4 C_{31} M_0^8 M_K^6 s_\theta^4}{81 M_\eta^8} - \frac{4 F^2 v_2^{(2)} c_\theta^4 M_0^6 M_K^2 M_\pi^2 s_\theta^4}{27 M_\eta^8} + \frac{29 \operatorname{Log}\left[\frac{M_K^2}{\mu^2}\right] c_\theta^4 M_0^8 M_K^2 M_\pi^2 s_\theta^4}{25920 \pi^2 M_\eta^8} - \frac{2 c_\theta^8 M_0^8 M_K^2 M_\pi^2 s_\theta^4}{243 \pi^2 M_\eta^8} + \\
& \frac{7 \operatorname{Log}\left[\frac{M_\pi^2}{\mu^2}\right] c_\theta^8 M_0^8 M_K^2 M_\pi^2 s_\theta^4}{2916 \pi^2 M_\eta^8} - \frac{7 \operatorname{Log}\left[\frac{M_\eta^2}{\mu^2}\right] c_\theta^8 M_0^8 M_K^2 M_\pi^2 s_\theta^4}{1944 \pi^2 M_\eta^8} + \frac{184 c_\theta^4 L_6^r M_0^8 M_K^2 M_\pi^2 s_\theta^4}{81 M_\eta^8} + \\
& \frac{832 c_\theta^4 L_7^r M_0^8 M_K^2 M_\pi^2 s_\theta^4}{81 M_\eta^8} + \frac{896 c_\theta^4 C_{19} M_0^8 M_K^4 M_\pi^2 s_\theta^4}{9 M_\eta^8} + \frac{2560 c_\theta^4 C_{31} M_0^8 M_K^4 M_\pi^2 s_\theta^4}{27 M_\eta^8} + \\
& \frac{14 F^2 v_2^{(2)} c_\theta^4 M_0^6 M_\pi^4 s_\theta^4}{27 M_\eta^8} + \frac{c_\theta^4 M_0^8 M_\pi^4 s_\theta^4}{864 \pi^2 M_\eta^8} + \frac{\operatorname{Log}\left[\frac{M_K^2}{\mu^2}\right] c_\theta^4 M_0^8 M_\pi^4 s_\theta^4}{3456 \pi^2 M_\eta^8} + \frac{\operatorname{Log}\left[\frac{M_\pi^2}{\mu^2}\right] c_\theta^4 M_0^8 M_\pi^4 s_\theta^4}{864 \pi^2 M_\eta^8} + \\
& \frac{53 c_\theta^8 M_0^8 M_\pi^4 s_\theta^4}{31104 \pi^2 M_\eta^8} - \frac{49 \operatorname{Log}\left[\frac{M_\eta^2}{\mu^2}\right] c_\theta^8 M_0^8 M_\pi^4 s_\theta^4}{93312 \pi^2 M_\eta^8} - \frac{25 \operatorname{Log}\left[\frac{M_\eta^2}{\mu^2}\right] c_\theta^8 M_0^8 M_\pi^4 s_\theta^4}{7776 \pi^2 M_\eta^8} + \frac{4 c_\theta^4 L_6^r M_0^8 M_\pi^4 s_\theta^4}{81 M_\eta^8} - \\
& \frac{320 c_\theta^4 L_7^r M_0^8 M_\pi^4 s_\theta^4}{81 M_\eta^8} - \frac{448 c_\theta^4 C_{19} M_0^8 M_K^2 M_\pi^4 s_\theta^4}{9 M_\eta^8} - \frac{1280 c_\theta^4 C_{31} M_0^8 M_K^2 M_\pi^4 s_\theta^4}{27 M_\eta^8} + \frac{196 c_\theta^4 C_{19} M_0^8 M_\pi^6 s_\theta^4}{27 M_\eta^8} + \\
& \frac{560 c_\theta^4 C_{31} M_0^8 M_\pi^6 s_\theta^4}{81 M_\eta^8} + \frac{16 F^2 v_2^{(2)} c_\theta^2 M_0^6 M_K^2 s_\theta^4}{3 M_\eta^6} + \frac{\operatorname{Log}\left[\frac{M_\eta^2}{\mu^2}\right] c_\theta^6 M_0^8 M_K^2 s_\theta^4}{486 \pi^2 M_\eta^6} - \frac{\operatorname{Log}\left[\frac{M_\eta^2}{\mu^2}\right] c_\theta^6 M_0^8 M_K^2 s_\theta^4}{162 \pi^2 M_\eta^6} - \\
& \frac{4 F^2 v_2^{(2)} c_\theta^2 M_0^6 M_\pi^2 s_\theta^4}{3 M_\eta^6} - \frac{31 \operatorname{Log}\left[\frac{M_\eta^2}{\mu^2}\right] c_\theta^6 M_0^8 M_\pi^2 s_\theta^4}{31104 \pi^2 M_\eta^6} + \frac{5 \operatorname{Log}\left[\frac{M_\eta^2}{\mu^2}\right] c_\theta^6 M_0^8 M_\pi^2 s_\theta^4}{1296 \pi^2 M_\eta^6} - \frac{4 F^2 v_2^{(2)} M_0^4 M_K^2 s_\theta^4}{3 M_\eta^4} -
\end{aligned}$$

$$\begin{aligned}
& \frac{2 F^2 v_2^{(2)} M_0^4 M_\pi^2 S_\theta^4}{3 M_\eta^4} - \frac{11\,468\,800 c_\theta^8 L_8^2 r M_0^8 M_K^{10} S_\theta^4}{729 F^2 M_\eta^{12}} + \frac{3\,184\,640 c_\theta^8 L_8^2 r M_0^8 M_K^8 M_\pi^2 S_\theta^4}{81 F^2 M_\eta^{12}} - \\
& \frac{9\,482\,240 c_\theta^8 L_8^2 r M_0^8 M_K^6 M_\pi^4 S_\theta^4}{243 F^2 M_\eta^{12}} + \frac{14\,064\,640 c_\theta^8 L_8^2 r M_0^8 M_K^4 M_\pi^6 S_\theta^4}{729 F^2 M_\eta^{12}} - \frac{386\,560 c_\theta^8 L_8^2 r M_0^8 M_K^2 M_\pi^8 S_\theta^4}{81 F^2 M_\eta^{12}} + \\
& \frac{18\,560 c_\theta^8 L_8^2 r M_0^8 M_\pi^{10} S_\theta^4}{81 F^2 M_\eta^{12}} + \frac{64 F^2 v_2^{(2)} c_\theta^6 M_0^8 M_K^4 S_\theta^4}{27 M_\eta^{10}} - \frac{20 \text{Log} \left[ \frac{M_K^2}{\mu^2} \right] c_\theta^6 M_0^8 M_K^6 S_\theta^4}{243 \pi^2 M_\eta^{10}} + \\
& \frac{5120 c_\theta^6 L_6^r M_0^8 M_K^6 S_\theta^4}{81 M_\eta^{10}} + \frac{5120 c_\theta^6 L_7^r M_0^8 M_K^6 S_\theta^4}{81 M_\eta^{10}} - \frac{5120 c_\theta^6 L_{25}^r M_0^8 M_K^6 S_\theta^4}{81 M_\eta^{10}} + \frac{10\,240 c_\theta^6 C_{19} M_0^8 M_K^8 S_\theta^4}{27 M_\eta^{10}} + \\
& \frac{20\,480 c_\theta^6 C_{31} M_0^8 M_K^8 S_\theta^4}{81 M_\eta^{10}} + \frac{4 F^2 v_2^{(2)} c_\theta^6 M_0^8 M_K^2 M_\pi^2 S_\theta^4}{27 M_\eta^{10}} + \frac{91 \text{Log} \left[ \frac{M_K^2}{\mu^2} \right] c_\theta^6 M_0^8 M_K^4 M_\pi^2 S_\theta^4}{972 \pi^2 M_\eta^{10}} - \\
& \frac{320 c_\theta^6 L_6^r M_0^8 M_K^4 M_\pi^2 S_\theta^4}{9 M_\eta^{10}} - \frac{832 c_\theta^6 L_7^r M_0^8 M_K^4 M_\pi^2 S_\theta^4}{9 M_\eta^{10}} + \frac{8128 c_\theta^6 L_{25}^r M_0^8 M_K^4 M_\pi^2 S_\theta^4}{81 M_\eta^{10}} - \\
& \frac{20\,096 c_\theta^6 C_{19} M_0^8 M_K^6 M_\pi^2 S_\theta^4}{27 M_\eta^{10}} - \frac{40\,192 c_\theta^6 C_{31} M_0^8 M_K^6 M_\pi^2 S_\theta^4}{81 M_\eta^{10}} - \frac{14 F^2 v_2^{(2)} c_\theta^6 M_0^8 M_K^4 S_\theta^4}{27 M_\eta^{10}} - \\
& \frac{23 \text{Log} \left[ \frac{M_K^2}{\mu^2} \right] c_\theta^6 M_0^8 M_K^2 M_\pi^4 S_\theta^4}{972 \pi^2 M_\eta^{10}} + \frac{\text{Log} \left[ \frac{M_\pi^2}{\mu^2} \right] c_\theta^6 M_0^8 M_K^2 M_\pi^4 S_\theta^4}{54 \pi^2 M_\eta^{10}} - \frac{320 c_\theta^6 L_6^r M_0^8 M_K^2 M_\pi^4 S_\theta^4}{27 M_\eta^{10}} + \\
& \frac{832 c_\theta^6 L_7^r M_0^8 M_K^2 M_\pi^4 S_\theta^4}{27 M_\eta^{10}} - \frac{3776 c_\theta^6 L_{25}^r M_0^8 M_K^2 M_\pi^4 S_\theta^4}{81 M_\eta^{10}} + \frac{4928 c_\theta^6 C_{19} M_0^8 M_K^4 M_\pi^4 S_\theta^4}{9 M_\eta^{10}} + \\
& \frac{9856 c_\theta^6 C_{31} M_0^8 M_K^4 M_\pi^4 S_\theta^4}{27 M_\eta^{10}} - \frac{\text{Log} \left[ \frac{M_\pi^2}{\mu^2} \right] c_\theta^6 M_0^8 M_\pi^6 S_\theta^4}{48 \pi^2 M_\eta^{10}} + \frac{880 c_\theta^6 L_6^r M_0^8 M_\pi^6 S_\theta^4}{81 M_\eta^{10}} + \frac{304 c_\theta^6 L_7^r M_0^8 M_\pi^6 S_\theta^4}{81 M_\eta^{10}} + \\
& \frac{112 c_\theta^6 L_{25}^r M_0^8 M_\pi^6 S_\theta^4}{27 M_\eta^{10}} - \frac{1696 c_\theta^6 C_{19} M_0^8 M_K^2 M_\pi^6 S_\theta^4}{9 M_\eta^{10}} - \frac{3392 c_\theta^6 C_{31} M_0^8 M_K^2 M_\pi^6 S_\theta^4}{27 M_\eta^{10}} + \frac{880 c_\theta^6 C_{19} M_0^8 M_\pi^8 S_\theta^4}{27 M_\eta^{10}} + \\
& \frac{1760 c_\theta^6 C_{31} M_0^8 M_\pi^8 S_\theta^4}{81 M_\eta^{10}} + \frac{16\,875\,520 c_\theta^8 L_8^2 r M_0^8 M_K^{10} S_\theta^4}{729 F^2 M_\eta^2 M_\eta^{10}} - \frac{13\,975\,552 c_\theta^8 L_8^2 r M_0^8 M_K^8 M_\pi^2 S_\theta^4}{243 F^2 M_\eta^2 M_\eta^{10}} + \\
& \frac{4\,341\,760 c_\theta^8 L_8^2 r M_0^8 M_K^6 M_\pi^4 S_\theta^4}{81 F^2 M_\eta^2 M_\eta^{10}} - \frac{16\,703\,488 c_\theta^8 L_8^2 r M_0^8 M_K^4 M_\pi^6 S_\theta^4}{729 F^2 M_\eta^2 M_\eta^{10}} + \frac{1\,040\,384 c_\theta^8 L_8^2 r M_0^8 M_K^2 M_\pi^8 S_\theta^4}{243 F^2 M_\eta^2 M_\eta^{10}} - \\
& \frac{8704 c_\theta^8 L_8^2 r M_0^8 M_\pi^{10} S_\theta^4}{27 F^2 M_\eta^2 M_\eta^{10}} + \frac{5 \text{Log} \left[ \frac{M_\eta^2}{\mu^2} \right] c_\theta^8 M_0^8 M_K^4 M_\eta^2 S_\theta^4}{729 \pi^2 M_\eta^{10}} - \frac{5 \text{Log} \left[ \frac{M_\eta^2}{\mu^2} \right] c_\theta^8 M_0^8 M_K^2 M_\pi^2 M_\eta^2 S_\theta^4}{1458 \pi^2 M_\eta^{10}} + \\
& \frac{5 \text{Log} \left[ \frac{M_\eta^2}{\mu^2} \right] c_\theta^8 M_0^8 M_\pi^4 M_\eta^2 S_\theta^4}{11\,664 \pi^2 M_\eta^{10}} - \frac{g1Dk c_\theta^4 M_0^8 S_\theta^4}{30 M_\eta^8} - \frac{64 F^2 v_2^{(2)} c_\theta^4 M_0^6 M_K^4 S_\theta^4}{27 M_\eta^8} - \frac{\text{Log} \left[ \frac{M_K^2}{\mu^2} \right] c_\theta^4 M_0^8 M_K^4 S_\theta^4}{1620 \pi^2 M_\eta^8} + \\
& \frac{281 c_\theta^8 M_0^8 M_K^4 S_\theta^4}{1944 \pi^2 M_\eta^8} - \frac{59 \text{Log} \left[ \frac{M_\eta^2}{\mu^2} \right] c_\theta^8 M_0^8 M_K^4 S_\theta^4}{1944 \pi^2 M_\eta^8} - \frac{35 \text{Log} \left[ \frac{M_\eta^2}{\mu^2} \right] c_\theta^8 M_0^8 M_K^4 S_\theta^4}{729 \pi^2 M_\eta^8} - \frac{512 c_\theta^4 L_6^r M_0^8 M_K^4 S_\theta^4}{81 M_\eta^8} -
\end{aligned}$$

$$\begin{aligned}
& \frac{512 c_{\theta}^4 L_7^r M_0^8 M_K^4 s_{\theta}^4}{81 M_{\eta'}^8} - \frac{1792 c_{\theta}^4 C_{19} M_0^8 M_K^6 s_{\theta}^4}{27 M_{\eta'}^8} - \frac{5120 c_{\theta}^4 C_{31} M_0^8 M_K^6 s_{\theta}^4}{81 M_{\eta'}^8} - \frac{4 F^2 v_2^{(2)} c_{\theta}^4 M_0^6 M_K^2 M_{\pi}^2 s_{\theta}^4}{27 M_{\eta'}^8} + \\
& \frac{29 \text{Log}\left[\frac{M_K^2}{\mu^2}\right] c_{\theta}^4 M_0^8 M_K^2 M_{\pi}^2 s_{\theta}^4}{25920 \pi^2 M_{\eta'}^8} - \frac{35 c_{\theta}^8 M_0^8 M_K^2 M_{\pi}^2 s_{\theta}^4}{243 \pi^2 M_{\eta'}^8} + \frac{5 \text{Log}\left[\frac{M_{\eta'}^2}{\mu^2}\right] c_{\theta}^8 M_0^8 M_K^2 M_{\pi}^2 s_{\theta}^4}{432 \pi^2 M_{\eta'}^8} + \\
& \frac{559 \text{Log}\left[\frac{M_{\eta'}^2}{\mu^2}\right] c_{\theta}^8 M_0^8 M_K^2 M_{\pi}^2 s_{\theta}^4}{11664 \pi^2 M_{\eta'}^8} + \frac{184 c_{\theta}^4 L_6^r M_0^8 M_K^2 M_{\pi}^2 s_{\theta}^4}{81 M_{\eta'}^8} + \frac{832 c_{\theta}^4 L_7^r M_0^8 M_K^2 M_{\pi}^2 s_{\theta}^4}{81 M_{\eta'}^8} + \\
& \frac{896 c_{\theta}^4 C_{19} M_0^8 M_K^4 M_{\pi}^2 s_{\theta}^4}{9 M_{\eta'}^8} + \frac{2560 c_{\theta}^4 C_{31} M_0^8 M_K^4 M_{\pi}^2 s_{\theta}^4}{27 M_{\eta'}^8} + \frac{14 F^2 v_2^{(2)} c_{\theta}^4 M_0^6 M_{\pi}^4 s_{\theta}^4}{27 M_{\eta'}^8} + \\
& \frac{c_{\theta}^4 M_0^8 M_{\pi}^4 s_{\theta}^4}{864 \pi^2 M_{\eta'}^8} + \frac{\text{Log}\left[\frac{M_K^2}{\mu^2}\right] c_{\theta}^4 M_0^8 M_{\pi}^4 s_{\theta}^4}{3456 \pi^2 M_{\eta'}^8} + \frac{\text{Log}\left[\frac{M_{\pi}^2}{\mu^2}\right] c_{\theta}^4 M_0^8 M_{\pi}^4 s_{\theta}^4}{864 \pi^2 M_{\eta'}^8} + \frac{1397 c_{\theta}^8 M_0^8 M_{\pi}^4 s_{\theta}^4}{31104 \pi^2 M_{\eta'}^8} + \\
& \frac{77 \text{Log}\left[\frac{M_{\eta'}^2}{\mu^2}\right] c_{\theta}^8 M_0^8 M_{\pi}^4 s_{\theta}^4}{31104 \pi^2 M_{\eta'}^8} - \frac{349 \text{Log}\left[\frac{M_{\eta'}^2}{\mu^2}\right] c_{\theta}^8 M_0^8 M_{\pi}^4 s_{\theta}^4}{23328 \pi^2 M_{\eta'}^8} + \frac{4 c_{\theta}^4 L_6^r M_0^8 M_{\pi}^4 s_{\theta}^4}{81 M_{\eta'}^8} - \frac{320 c_{\theta}^4 L_7^r M_0^8 M_{\pi}^4 s_{\theta}^4}{81 M_{\eta'}^8} - \\
& \frac{448 c_{\theta}^4 C_{19} M_0^8 M_K^2 M_{\pi}^4 s_{\theta}^4}{9 M_{\eta'}^8} - \frac{1280 c_{\theta}^4 C_{31} M_0^8 M_K^2 M_{\pi}^4 s_{\theta}^4}{27 M_{\eta'}^8} + \frac{196 c_{\theta}^4 C_{19} M_0^8 M_{\pi}^6 s_{\theta}^4}{27 M_{\eta'}^8} + \frac{560 c_{\theta}^4 C_{31} M_0^8 M_{\pi}^6 s_{\theta}^4}{81 M_{\eta'}^8} - \\
& \frac{12738560 c_{\theta}^8 L_8^{2r} M_0^8 M_K^{10} s_{\theta}^4}{729 F^2 M_{\eta'}^4 M_{\eta'}^8} + \frac{1146880 c_{\theta}^8 L_8^{2r} M_0^8 M_K^8 M_{\pi}^2 s_{\theta}^4}{27 F^2 M_{\eta'}^4 M_{\eta'}^8} - \frac{8474624 c_{\theta}^8 L_8^{2r} M_0^8 M_K^6 M_{\pi}^4 s_{\theta}^4}{243 F^2 M_{\eta'}^4 M_{\eta'}^8} + \\
& \frac{7374848 c_{\theta}^8 L_8^{2r} M_0^8 M_K^4 M_{\pi}^6 s_{\theta}^4}{729 F^2 M_{\eta'}^4 M_{\eta'}^8} + \frac{512 c_{\theta}^8 L_8^{2r} M_0^8 M_K^2 M_{\pi}^8 s_{\theta}^4}{243 F^2 M_{\eta'}^4 M_{\eta'}^8} - \frac{3968 c_{\theta}^8 L_8^{2r} M_0^8 M_{\pi}^{10} s_{\theta}^4}{27 F^2 M_{\eta'}^4 M_{\eta'}^8} + \\
& \frac{320 F^2 v_2^{(2)} c_{\theta}^6 M_0^8 M_K^4 s_{\theta}^4}{27 M_{\eta'}^2 M_{\eta'}^8} + \frac{7 \text{Log}\left[\frac{M_K^2}{\mu^2}\right] c_{\theta}^6 M_0^8 M_K^6 s_{\theta}^4}{243 \pi^2 M_{\eta'}^2 M_{\eta'}^8} - \frac{23552 c_{\theta}^6 L_6^r M_0^8 M_K^6 s_{\theta}^4}{243 M_{\eta'}^2 M_{\eta'}^8} - \\
& \frac{23552 c_{\theta}^6 L_7^r M_0^8 M_K^6 s_{\theta}^4}{243 M_{\eta'}^2 M_{\eta'}^8} + \frac{1792 c_{\theta}^6 L_{25}^r M_0^8 M_K^6 s_{\theta}^4}{81 M_{\eta'}^2 M_{\eta'}^8} - \frac{47104 c_{\theta}^6 C_{19} M_0^8 M_K^8 s_{\theta}^4}{81 M_{\eta'}^2 M_{\eta'}^8} - \frac{94208 c_{\theta}^6 C_{31} M_0^8 M_K^8 s_{\theta}^4}{243 M_{\eta'}^2 M_{\eta'}^8} + \\
& \frac{128 F^2 v_2^{(2)} c_{\theta}^6 M_0^8 M_K^2 M_{\pi}^2 s_{\theta}^4}{27 M_{\eta'}^2 M_{\eta'}^8} - \frac{35 \text{Log}\left[\frac{M_K^2}{\mu^2}\right] c_{\theta}^6 M_0^8 M_K^4 M_{\pi}^2 s_{\theta}^4}{324 \pi^2 M_{\eta'}^2 M_{\eta'}^8} + \frac{1792 c_{\theta}^6 L_6^r M_0^8 M_K^4 M_{\pi}^2 s_{\theta}^4}{27 M_{\eta'}^2 M_{\eta'}^8} + \\
& \frac{5504 c_{\theta}^6 L_7^r M_0^8 M_K^4 M_{\pi}^2 s_{\theta}^4}{27 M_{\eta'}^2 M_{\eta'}^8} - \frac{3200 c_{\theta}^6 L_{25}^r M_0^8 M_K^4 M_{\pi}^2 s_{\theta}^4}{81 M_{\eta'}^2 M_{\eta'}^8} + \frac{86272 c_{\theta}^6 C_{19} M_0^8 M_K^6 M_{\pi}^2 s_{\theta}^4}{81 M_{\eta'}^2 M_{\eta'}^8} + \\
& \frac{172544 c_{\theta}^6 C_{31} M_0^8 M_K^6 M_{\pi}^2 s_{\theta}^4}{243 M_{\eta'}^2 M_{\eta'}^8} - \frac{16 F^2 v_2^{(2)} c_{\theta}^6 M_0^8 M_{\pi}^4 s_{\theta}^4}{27 M_{\eta'}^2 M_{\eta'}^8} + \frac{95 \text{Log}\left[\frac{M_K^2}{\mu^2}\right] c_{\theta}^6 M_0^8 M_K^2 M_{\pi}^4 s_{\theta}^4}{3888 \pi^2 M_{\eta'}^2 M_{\eta'}^8} - \\
& \frac{65 \text{Log}\left[\frac{M_{\pi}^2}{\mu^2}\right] c_{\theta}^6 M_0^8 M_K^2 M_{\pi}^4 s_{\theta}^4}{648 \pi^2 M_{\eta'}^2 M_{\eta'}^8} + \frac{2912 c_{\theta}^6 L_6^r M_0^8 M_K^2 M_{\pi}^4 s_{\theta}^4}{81 M_{\eta'}^2 M_{\eta'}^8} - \frac{6016 c_{\theta}^6 L_7^r M_0^8 M_K^2 M_{\pi}^4 s_{\theta}^4}{81 M_{\eta'}^2 M_{\eta'}^8} - \\
& \frac{2432 c_{\theta}^6 L_{25}^r M_0^8 M_K^2 M_{\pi}^4 s_{\theta}^4}{81 M_{\eta'}^2 M_{\eta'}^8} - \frac{2176 c_{\theta}^6 C_{19} M_0^8 M_K^4 M_{\pi}^4 s_{\theta}^4}{3 M_{\eta'}^2 M_{\eta'}^8} - \frac{4352 c_{\theta}^6 C_{31} M_0^8 M_K^4 M_{\pi}^4 s_{\theta}^4}{9 M_{\eta'}^2 M_{\eta'}^8} +
\end{aligned}$$

$$\begin{aligned}
& \frac{41 \operatorname{Log}\left[\frac{M_\pi^2}{\mu^2}\right] c_\theta^6 M_0^8 M_\pi^6 s_\theta^4}{2592 \pi^2 M_\eta^2 M_\eta^8} - \frac{2608 c_\theta^6 L_6^r M_0^8 M_\pi^6 s_\theta^4}{243 M_\eta^2 M_\eta^8} + \frac{2432 c_\theta^6 L_7^r M_0^8 M_\pi^6 s_\theta^4}{243 M_\eta^2 M_\eta^8} + \frac{128 c_\theta^6 L_{25}^r M_0^8 M_\pi^6 s_\theta^4}{27 M_\eta^2 M_\eta^8} + \\
& \frac{21760 c_\theta^6 C_{19} M_0^8 M_K^2 M_\pi^6 s_\theta^4}{81 M_\eta^2 M_\eta^8} + \frac{43520 c_\theta^6 C_{31} M_0^8 M_K^2 M_\pi^6 s_\theta^4}{243 M_\eta^2 M_\eta^8} - \frac{2608 c_\theta^6 C_{19} M_0^8 M_\pi^8 s_\theta^4}{81 M_\eta^2 M_\eta^8} - \\
& \frac{5216 c_\theta^6 C_{31} M_0^8 M_\pi^8 s_\theta^4}{243 M_\eta^2 M_\eta^8} - \frac{\operatorname{Log}\left[\frac{M_\eta^2}{\mu^2}\right] c_\theta^6 M_0^8 M_K^2 M_\eta^2 s_\theta^4}{324 \pi^2 M_\eta^8} + \frac{19 \operatorname{Log}\left[\frac{M_\eta^2}{\mu^2}\right] c_\theta^6 M_0^8 M_\pi^2 M_\eta^2 s_\theta^4}{10368 \pi^2 M_\eta^8} + \\
& \frac{11 \operatorname{Log}\left[\frac{M_\eta^2}{\mu^2}\right] c_\theta^6 M_0^8 M_K^2 s_\theta^4}{972 \pi^2 M_\eta^6} + \frac{5 \operatorname{Log}\left[\frac{M_\eta^2}{\mu^2}\right] c_\theta^6 M_0^8 M_K^2 s_\theta^4}{324 \pi^2 M_\eta^6} - \frac{55 \operatorname{Log}\left[\frac{M_\eta^2}{\mu^2}\right] c_\theta^6 M_0^8 M_\pi^2 s_\theta^4}{7776 \pi^2 M_\eta^6} - \\
& \frac{35 \operatorname{Log}\left[\frac{M_\eta^2}{\mu^2}\right] c_\theta^6 M_0^8 M_\pi^2 s_\theta^4}{5184 \pi^2 M_\eta^6} + \frac{3604480 c_\theta^8 L_8^2 r M_0^8 M_K^{10} s_\theta^4}{729 F^2 M_\eta^6 M_\eta^6} - \frac{2711552 c_\theta^8 L_8^2 r M_0^8 M_K^8 M_\pi^2 s_\theta^4}{243 F^2 M_\eta^6 M_\eta^6} + \\
& \frac{1703936 c_\theta^8 L_8^2 r M_0^8 M_K^6 M_\pi^4 s_\theta^4}{243 F^2 M_\eta^6 M_\eta^6} - \frac{495616 c_\theta^8 L_8^2 r M_0^8 M_K^4 M_\pi^6 s_\theta^4}{729 F^2 M_\eta^6 M_\eta^6} - \frac{28672 c_\theta^8 L_8^2 r M_0^8 M_K^2 M_\pi^8 s_\theta^4}{243 F^2 M_\eta^6 M_\eta^6} - \\
& \frac{1024 c_\theta^8 L_8^2 r M_0^8 M_\pi^{10} s_\theta^4}{27 F^2 M_\eta^6 M_\eta^6} - \frac{608 F^2 v_2^{(2)} c_\theta^6 M_0^8 M_K^4 s_\theta^4}{27 M_\eta^4 M_\eta^6} + \frac{2 \operatorname{Log}\left[\frac{M_K^2}{\mu^2}\right] c_\theta^6 M_0^8 M_K^6 s_\theta^4}{243 \pi^2 M_\eta^4 M_\eta^6} + \frac{25088 c_\theta^6 L_6^r M_0^8 M_K^6 s_\theta^4}{243 M_\eta^4 M_\eta^6} + \\
& \frac{25088 c_\theta^6 L_7^r M_0^8 M_K^6 s_\theta^4}{243 M_\eta^4 M_\eta^6} + \frac{512 c_\theta^6 L_{25}^r M_0^8 M_K^6 s_\theta^4}{81 M_\eta^4 M_\eta^6} + \frac{50176 c_\theta^6 C_{19} M_0^8 M_K^8 s_\theta^4}{81 M_\eta^4 M_\eta^6} + \frac{100352 c_\theta^6 C_{31} M_0^8 M_K^8 s_\theta^4}{243 M_\eta^4 M_\eta^6} - \\
& \frac{104 F^2 v_2^{(2)} c_\theta^6 M_0^8 M_K^2 M_\pi^2 s_\theta^4}{27 M_\eta^4 M_\eta^6} + \frac{\operatorname{Log}\left[\frac{M_K^2}{\mu^2}\right] c_\theta^6 M_0^8 M_K^4 M_\pi^2 s_\theta^4}{12 \pi^2 M_\eta^4 M_\eta^6} - \frac{6656 c_\theta^6 L_6^r M_0^8 M_K^2 M_\pi^2 s_\theta^4}{81 M_\eta^4 M_\eta^6} - \\
& \frac{18944 c_\theta^6 L_7^r M_0^8 M_K^4 M_\pi^2 s_\theta^4}{81 M_\eta^4 M_\eta^6} - \frac{1984 c_\theta^6 L_{25}^r M_0^8 M_K^4 M_\pi^2 s_\theta^4}{81 M_\eta^4 M_\eta^6} - \frac{85504 c_\theta^6 C_{19} M_0^8 M_K^6 M_\pi^2 s_\theta^4}{81 M_\eta^4 M_\eta^6} - \\
& \frac{171008 c_\theta^6 C_{31} M_0^8 M_K^6 M_\pi^2 s_\theta^4}{243 M_\eta^4 M_\eta^6} + \frac{100 F^2 v_2^{(2)} c_\theta^6 M_0^8 M_\pi^4 s_\theta^4}{27 M_\eta^4 M_\eta^6} - \frac{23 \operatorname{Log}\left[\frac{M_K^2}{\mu^2}\right] c_\theta^6 M_0^8 M_K^2 M_\pi^4 s_\theta^4}{972 \pi^2 M_\eta^4 M_\eta^6} + \\
& \frac{29 \operatorname{Log}\left[\frac{M_\pi^2}{\mu^2}\right] c_\theta^6 M_0^8 M_K^2 M_\pi^4 s_\theta^4}{162 \pi^2 M_\eta^4 M_\eta^6} - \frac{3328 c_\theta^6 L_6^r M_0^8 M_K^2 M_\pi^4 s_\theta^4}{81 M_\eta^4 M_\eta^6} + \frac{6464 c_\theta^6 L_7^r M_0^8 M_K^2 M_\pi^4 s_\theta^4}{81 M_\eta^4 M_\eta^6} + \\
& \frac{8768 c_\theta^6 L_{25}^r M_0^8 M_K^2 M_\pi^4 s_\theta^4}{81 M_\eta^4 M_\eta^6} + \frac{5888 c_\theta^6 C_{19} M_0^8 M_K^4 M_\pi^4 s_\theta^4}{9 M_\eta^4 M_\eta^6} + \frac{11776 c_\theta^6 C_{31} M_0^8 M_K^4 M_\pi^4 s_\theta^4}{27 M_\eta^4 M_\eta^6} - \\
& \frac{29 \operatorname{Log}\left[\frac{M_\pi^2}{\mu^2}\right] c_\theta^6 M_0^8 M_\pi^6 s_\theta^4}{648 \pi^2 M_\eta^4 M_\eta^6} + \frac{3136 c_\theta^6 L_6^r M_0^8 M_\pi^6 s_\theta^4}{243 M_\eta^4 M_\eta^6} - \frac{2336 c_\theta^6 L_7^r M_0^8 M_\pi^6 s_\theta^4}{243 M_\eta^4 M_\eta^6} - \frac{800 c_\theta^6 L_{25}^r M_0^8 M_\pi^6 s_\theta^4}{27 M_\eta^4 M_\eta^6} - \\
& \frac{21376 c_\theta^6 C_{19} M_0^8 M_K^2 M_\pi^6 s_\theta^4}{81 M_\eta^4 M_\eta^6} - \frac{42752 c_\theta^6 C_{31} M_0^8 M_K^2 M_\pi^6 s_\theta^4}{243 M_\eta^4 M_\eta^6} + \frac{3136 c_\theta^6 C_{19} M_0^8 M_\pi^8 s_\theta^4}{81 M_\eta^4 M_\eta^6} + \\
& \frac{6272 c_\theta^6 C_{31} M_0^8 M_\pi^8 s_\theta^4}{243 M_\eta^4 M_\eta^6} + \frac{2 \operatorname{g1Dk} c_\theta^4 M_0^8 s_\theta^4}{15 M_\eta^2 M_\eta^6} - \frac{16 F^2 v_2^{(2)} c_\theta^4 M_0^8 M_K^2 s_\theta^4}{3 M_\eta^2 M_\eta^6} - \frac{128 F^2 v_2^{(2)} c_\theta^4 M_0^6 M_K^4 s_\theta^4}{27 M_\eta^2 M_\eta^6} +
\end{aligned}$$

$$\begin{aligned}
& \frac{c_\theta^4 M_\theta^8 M_K^4 s_\theta^4}{54 \pi^2 M_\eta^2 M_{\eta'}^6} + \frac{17 \operatorname{Log}\left[\frac{M_K^2}{\mu^2}\right] c_\theta^4 M_\theta^8 M_K^4 s_\theta^4}{810 \pi^2 M_\eta^2 M_{\eta'}^6} - \frac{47 c_\theta^8 M_\theta^8 M_K^4 s_\theta^4}{243 \pi^2 M_\eta^2 M_{\eta'}^6} + \frac{10 \operatorname{Log}\left[\frac{M_\eta^2}{\mu^2}\right] c_\theta^8 M_\theta^8 M_K^4 s_\theta^4}{729 \pi^2 M_\eta^2 M_{\eta'}^6} + \\
& \frac{2 \operatorname{Log}\left[\frac{M_\eta^2}{\mu^2}\right] c_\theta^8 M_\theta^8 M_K^4 s_\theta^4}{27 \pi^2 M_\eta^2 M_{\eta'}^6} - \frac{1024 c_\theta^4 L_6^r M_\theta^8 M_K^4 s_\theta^4}{81 M_\eta^2 M_{\eta'}^6} - \frac{1024 c_\theta^4 L_7^r M_\theta^8 M_K^4 s_\theta^4}{81 M_\eta^2 M_{\eta'}^6} - \frac{3584 c_\theta^4 C_{19} M_\theta^8 M_K^6 s_\theta^4}{27 M_\eta^2 M_{\eta'}^6} - \\
& \frac{10240 c_\theta^4 C_{31} M_\theta^8 M_K^6 s_\theta^4}{81 M_\eta^2 M_{\eta'}^6} + \frac{4 F^2 v_2^{(2)} c_\theta^4 M_\theta^8 M_\pi^2 s_\theta^4}{3 M_\eta^2 M_{\eta'}^6} - \frac{80 F^2 v_2^{(2)} c_\theta^4 M_\theta^6 M_K^2 M_\pi^2 s_\theta^4}{27 M_\eta^2 M_{\eta'}^6} - \frac{5 c_\theta^4 M_\theta^8 M_K^2 M_\pi^2 s_\theta^4}{216 \pi^2 M_\eta^2 M_{\eta'}^6} - \\
& \frac{209 \operatorname{Log}\left[\frac{M_K^2}{\mu^2}\right] c_\theta^4 M_\theta^8 M_K^2 M_\pi^2 s_\theta^4}{6480 \pi^2 M_\eta^2 M_{\eta'}^6} + \frac{181 c_\theta^8 M_\theta^8 M_K^2 M_\pi^2 s_\theta^4}{972 \pi^2 M_\eta^2 M_{\eta'}^6} + \frac{65 \operatorname{Log}\left[\frac{M_\eta^2}{\mu^2}\right] c_\theta^8 M_\theta^8 M_K^2 M_\pi^2 s_\theta^4}{5832 \pi^2 M_\eta^2 M_{\eta'}^6} - \\
& \frac{47 \operatorname{Log}\left[\frac{M_\eta^2}{\mu^2}\right] c_\theta^8 M_\theta^8 M_K^2 M_\pi^2 s_\theta^4}{648 \pi^2 M_\eta^2 M_{\eta'}^6} + \frac{1952 c_\theta^4 L_6^r M_\theta^8 M_K^2 M_\pi^2 s_\theta^4}{81 M_\eta^2 M_{\eta'}^6} - \frac{640 c_\theta^4 L_7^r M_\theta^8 M_K^2 M_\pi^2 s_\theta^4}{81 M_\eta^2 M_{\eta'}^6} + \\
& \frac{1792 c_\theta^4 C_{19} M_\theta^8 M_K^4 M_\pi^2 s_\theta^4}{9 M_\eta^2 M_{\eta'}^6} + \frac{5120 c_\theta^4 C_{31} M_\theta^8 M_K^4 M_\pi^2 s_\theta^4}{27 M_\eta^2 M_{\eta'}^6} - \frac{8 F^2 v_2^{(2)} c_\theta^4 M_\theta^6 M_\pi^4 s_\theta^4}{27 M_\eta^2 M_{\eta'}^6} + \\
& \frac{c_\theta^4 M_\theta^8 M_\pi^4 s_\theta^4}{48 \pi^2 M_\eta^2 M_{\eta'}^6} + \frac{\operatorname{Log}\left[\frac{M_K^2}{\mu^2}\right] c_\theta^4 M_\theta^8 M_\pi^4 s_\theta^4}{288 \pi^2 M_\eta^2 M_{\eta'}^6} + \frac{5 \operatorname{Log}\left[\frac{M_\pi^2}{\mu^2}\right] c_\theta^4 M_\theta^8 M_\pi^4 s_\theta^4}{216 \pi^2 M_\eta^2 M_{\eta'}^6} - \frac{331 c_\theta^8 M_\theta^8 M_\pi^4 s_\theta^4}{7776 \pi^2 M_\eta^2 M_{\eta'}^6} - \\
& \frac{175 \operatorname{Log}\left[\frac{M_\eta^2}{\mu^2}\right] c_\theta^8 M_\theta^8 M_\pi^4 s_\theta^4}{23328 \pi^2 M_\eta^2 M_{\eta'}^6} + \frac{11 \operatorname{Log}\left[\frac{M_\eta^2}{\mu^2}\right] c_\theta^8 M_\theta^8 M_\pi^4 s_\theta^4}{648 \pi^2 M_\eta^2 M_{\eta'}^6} - \frac{1360 c_\theta^4 L_6^r M_\theta^8 M_\pi^4 s_\theta^4}{81 M_\eta^2 M_{\eta'}^6} - \\
& \frac{64 c_\theta^4 L_7^r M_\theta^8 M_\pi^4 s_\theta^4}{81 M_\eta^2 M_{\eta'}^6} - \frac{896 c_\theta^4 C_{19} M_\theta^8 M_K^2 M_\pi^4 s_\theta^4}{9 M_\eta^2 M_{\eta'}^6} - \frac{2560 c_\theta^4 C_{31} M_\theta^8 M_K^2 M_\pi^4 s_\theta^4}{27 M_\eta^2 M_{\eta'}^6} - \frac{112 c_\theta^4 C_{19} M_\theta^8 M_\pi^6 s_\theta^4}{27 M_\eta^2 M_{\eta'}^6} - \\
& \frac{320 c_\theta^4 C_{31} M_\theta^8 M_\pi^6 s_\theta^4}{81 M_\eta^2 M_{\eta'}^6} + \frac{6062080 c_\theta^8 L_8^{2r} M_\theta^8 M_K^{10} s_\theta^4}{729 F^2 M_\eta^8 M_{\eta'}^4} - \frac{5183488 c_\theta^8 L_8^{2r} M_\theta^8 M_K^8 M_\pi^2 s_\theta^4}{243 F^2 M_\eta^8 M_{\eta'}^4} + \\
& \frac{20480 c_\theta^8 L_8^{2r} M_\theta^8 M_K^6 M_\pi^4 s_\theta^4}{F^2 M_\eta^8 M_{\eta'}^4} - \frac{5862400 c_\theta^8 L_8^{2r} M_\theta^8 M_K^4 M_\pi^6 s_\theta^4}{729 F^2 M_\eta^8 M_{\eta'}^4} + \frac{108032 c_\theta^8 L_8^{2r} M_\theta^8 M_K^2 M_\pi^8 s_\theta^4}{243 F^2 M_\eta^8 M_{\eta'}^4} + \\
& \frac{128 c_\theta^8 L_8^{2r} M_\theta^8 M_\pi^{10} s_\theta^4}{27 F^2 M_\eta^8 M_{\eta'}^4} + \frac{320 F^2 v_2^{(2)} c_\theta^6 M_\theta^8 M_K^4 s_\theta^4}{27 M_\eta^6 M_{\eta'}^4} + \frac{17 \operatorname{Log}\left[\frac{M_K^2}{\mu^2}\right] c_\theta^6 M_\theta^8 M_K^6 s_\theta^4}{243 \pi^2 M_\eta^6 M_{\eta'}^4} - \frac{8192 c_\theta^6 L_6^r M_\theta^8 M_K^6 s_\theta^4}{81 M_\eta^6 M_{\eta'}^4} - \\
& \frac{8192 c_\theta^6 L_7^r M_\theta^8 M_K^6 s_\theta^4}{81 M_\eta^6 M_{\eta'}^4} + \frac{4352 c_\theta^6 L_{25}^r M_\theta^8 M_K^6 s_\theta^4}{81 M_\eta^6 M_{\eta'}^4} - \frac{16384 c_\theta^6 C_{19} M_\theta^8 M_K^8 s_\theta^4}{27 M_\eta^6 M_{\eta'}^4} - \frac{32768 c_\theta^6 C_{31} M_\theta^8 M_K^8 s_\theta^4}{81 M_\eta^6 M_{\eta'}^4} + \\
& \frac{128 F^2 v_2^{(2)} c_\theta^6 M_\theta^8 M_K^2 M_\pi^2 s_\theta^4}{27 M_\eta^6 M_{\eta'}^4} - \frac{139 \operatorname{Log}\left[\frac{M_K^2}{\mu^2}\right] c_\theta^6 M_\theta^8 M_K^4 M_\pi^2 s_\theta^4}{972 \pi^2 M_\eta^6 M_{\eta'}^4} + \frac{2176 c_\theta^6 L_6^r M_\theta^8 M_K^4 M_\pi^2 s_\theta^4}{27 M_\eta^6 M_{\eta'}^4} + \\
& \frac{4864 c_\theta^6 L_7^r M_\theta^8 M_K^4 M_\pi^2 s_\theta^4}{27 M_\eta^6 M_{\eta'}^4} - \frac{7168 c_\theta^6 L_{25}^r M_\theta^8 M_K^4 M_\pi^2 s_\theta^4}{81 M_\eta^6 M_{\eta'}^4} + \frac{29696 c_\theta^6 C_{19} M_\theta^8 M_K^6 M_\pi^2 s_\theta^4}{27 M_\eta^6 M_{\eta'}^4} +
\end{aligned}$$

$$\begin{aligned}
& \frac{59\,392\,c_\theta^6\,C_{31}\,M_\theta^8\,M_K^6\,M_\pi^2\,s_\theta^4}{81\,M_\eta^6\,M_{\eta'}^4} - \frac{16\,F^2\,v_2^{(2)}\,c_\theta^6\,M_\theta^8\,M_\pi^4\,s_\theta^4}{27\,M_\eta^6\,M_{\eta'}^4} + \frac{29\,\text{Log}\left[\frac{M_K^2}{\mu^2}\right]\,c_\theta^6\,M_\theta^8\,M_K^2\,M_\pi^4\,s_\theta^4}{972\,\pi^2\,M_\eta^6\,M_{\eta'}^4} - \\
& \frac{31\,\text{Log}\left[\frac{M_\pi^2}{\mu^2}\right]\,c_\theta^6\,M_\theta^8\,M_K^2\,M_\pi^4\,s_\theta^4}{216\,\pi^2\,M_\eta^6\,M_{\eta'}^4} + \frac{320\,c_\theta^6\,L_6^r\,M_\theta^8\,M_K^2\,M_\pi^4\,s_\theta^4}{9\,M_\eta^6\,M_{\eta'}^4} - \frac{256\,c_\theta^6\,L_7^r\,M_\theta^8\,M_K^2\,M_\pi^4\,s_\theta^4}{9\,M_\eta^6\,M_{\eta'}^4} - \\
& \frac{1024\,c_\theta^6\,L_{25}^r\,M_\theta^8\,M_K^2\,M_\pi^4\,s_\theta^4}{81\,M_\eta^6\,M_{\eta'}^4} - \frac{6656\,c_\theta^6\,C_{19}\,M_\theta^8\,M_K^4\,M_\pi^4\,s_\theta^4}{9\,M_\eta^6\,M_{\eta'}^4} - \frac{13\,312\,c_\theta^6\,C_{31}\,M_\theta^8\,M_K^4\,M_\pi^4\,s_\theta^4}{27\,M_\eta^6\,M_{\eta'}^4} + \\
& \frac{\text{Log}\left[\frac{M_\pi^2}{\mu^2}\right]\,c_\theta^6\,M_\theta^8\,M_\pi^6\,s_\theta^4}{24\,\pi^2\,M_\eta^6\,M_{\eta'}^4} - \frac{1216\,c_\theta^6\,L_6^r\,M_\theta^8\,M_\pi^6\,s_\theta^4}{81\,M_\eta^6\,M_{\eta'}^4} - \frac{640\,c_\theta^6\,L_7^r\,M_\theta^8\,M_\pi^6\,s_\theta^4}{81\,M_\eta^6\,M_{\eta'}^4} + \frac{128\,c_\theta^6\,L_{25}^r\,M_\theta^8\,M_\pi^6\,s_\theta^4}{27\,M_\eta^6\,M_{\eta'}^4} + \\
& \frac{2624\,c_\theta^6\,C_{19}\,M_\theta^8\,M_K^2\,M_\pi^6\,s_\theta^4}{9\,M_\eta^6\,M_{\eta'}^4} + \frac{5248\,c_\theta^6\,C_{31}\,M_\theta^8\,M_K^2\,M_\pi^6\,s_\theta^4}{27\,M_\eta^6\,M_{\eta'}^4} - \frac{1216\,c_\theta^6\,C_{19}\,M_\theta^8\,M_\pi^8\,s_\theta^4}{27\,M_\eta^6\,M_{\eta'}^4} - \\
& \frac{2432\,c_\theta^6\,C_{31}\,M_\theta^8\,M_\pi^8\,s_\theta^4}{81\,M_\eta^6\,M_{\eta'}^4} - \frac{g1Dk\,c_\theta^4\,M_\theta^8\,s_\theta^4}{5\,M_\eta^4\,M_{\eta'}^4} + \frac{8\,F^2\,v_2^{(2)}\,c_\theta^4\,M_\theta^8\,M_K^2\,s_\theta^4}{3\,M_\eta^4\,M_{\eta'}^4} + \frac{32\,F^2\,v_2^{(2)}\,c_\theta^4\,M_\theta^6\,M_K^4\,s_\theta^4}{3\,M_\eta^4\,M_{\eta'}^4} - \\
& \frac{c_\theta^4\,M_\theta^8\,M_K^4\,s_\theta^4}{108\,\pi^2\,M_\eta^4\,M_{\eta'}^4} - \frac{\text{Log}\left[\frac{M_\eta^2}{\mu^2}\right]\,c_\theta^4\,M_\theta^8\,M_K^4\,s_\theta^4}{270\,\pi^2\,M_\eta^4\,M_{\eta'}^4} + \frac{17\,c_\theta^8\,M_\theta^8\,M_K^4\,s_\theta^4}{324\,\pi^2\,M_\eta^4\,M_{\eta'}^4} + \frac{23\,\text{Log}\left[\frac{M_\eta^2}{\mu^2}\right]\,c_\theta^8\,M_\theta^8\,M_K^4\,s_\theta^4}{729\,\pi^2\,M_\eta^4\,M_{\eta'}^4} - \\
& \frac{199\,\text{Log}\left[\frac{M_\eta^2}{\mu^2}\right]\,c_\theta^8\,M_\theta^8\,M_K^4\,s_\theta^4}{2916\,\pi^2\,M_\eta^4\,M_{\eta'}^4} + \frac{256\,c_\theta^4\,L_6^r\,M_\theta^8\,M_K^4\,s_\theta^4}{9\,M_\eta^4\,M_{\eta'}^4} + \frac{256\,c_\theta^4\,L_7^r\,M_\theta^8\,M_K^4\,s_\theta^4}{9\,M_\eta^4\,M_{\eta'}^4} + \frac{896\,c_\theta^4\,C_{19}\,M_\theta^8\,M_K^6\,s_\theta^4}{3\,M_\eta^4\,M_{\eta'}^4} + \\
& \frac{2560\,c_\theta^4\,C_{31}\,M_\theta^8\,M_K^6\,s_\theta^4}{9\,M_\eta^4\,M_{\eta'}^4} - \frac{20\,F^2\,v_2^{(2)}\,c_\theta^4\,M_\theta^8\,M_\pi^2\,s_\theta^4}{3\,M_\eta^4\,M_{\eta'}^4} + \frac{8\,F^2\,v_2^{(2)}\,c_\theta^4\,M_\theta^6\,M_K^2\,M_\pi^2\,s_\theta^4}{3\,M_\eta^4\,M_{\eta'}^4} + \frac{5\,c_\theta^4\,M_\theta^8\,M_K^2\,M_\pi^2\,s_\theta^4}{108\,\pi^2\,M_\eta^4\,M_{\eta'}^4} + \\
& \frac{269\,\text{Log}\left[\frac{M_K^2}{\mu^2}\right]\,c_\theta^4\,M_\theta^8\,M_K^2\,M_\pi^2\,s_\theta^4}{4320\,\pi^2\,M_\eta^4\,M_{\eta'}^4} - \frac{23\,c_\theta^8\,M_\theta^8\,M_K^2\,M_\pi^2\,s_\theta^4}{648\,\pi^2\,M_\eta^4\,M_{\eta'}^4} - \frac{499\,\text{Log}\left[\frac{M_\eta^2}{\mu^2}\right]\,c_\theta^8\,M_\theta^8\,M_K^2\,M_\pi^2\,s_\theta^4}{11\,664\,\pi^2\,M_\eta^4\,M_{\eta'}^4} + \\
& \frac{689\,\text{Log}\left[\frac{M_\eta^2}{\mu^2}\right]\,c_\theta^8\,M_\theta^8\,M_K^2\,M_\pi^2\,s_\theta^4}{11\,664\,\pi^2\,M_\eta^4\,M_{\eta'}^4} - \frac{560\,c_\theta^4\,L_6^r\,M_\theta^8\,M_K^2\,M_\pi^2\,s_\theta^4}{9\,M_\eta^4\,M_{\eta'}^4} - \frac{128\,c_\theta^4\,L_7^r\,M_\theta^8\,M_K^2\,M_\pi^2\,s_\theta^4}{9\,M_\eta^4\,M_{\eta'}^4} - \\
& \frac{448\,c_\theta^4\,C_{19}\,M_\theta^8\,M_K^4\,M_\pi^2\,s_\theta^4}{M_\eta^4\,M_{\eta'}^4} - \frac{1280\,c_\theta^4\,C_{31}\,M_\theta^8\,M_K^4\,M_\pi^2\,s_\theta^4}{3\,M_\eta^4\,M_{\eta'}^4} - \frac{4\,F^2\,v_2^{(2)}\,c_\theta^4\,M_\theta^6\,M_\pi^4\,s_\theta^4}{3\,M_\eta^4\,M_{\eta'}^4} - \frac{5\,c_\theta^4\,M_\theta^8\,M_\pi^4\,s_\theta^4}{216\,\pi^2\,M_\eta^4\,M_{\eta'}^4} - \\
& \frac{13\,\text{Log}\left[\frac{M_K^2}{\mu^2}\right]\,c_\theta^4\,M_\theta^8\,M_\pi^4\,s_\theta^4}{1728\,\pi^2\,M_\eta^4\,M_{\eta'}^4} - \frac{\text{Log}\left[\frac{M_\pi^2}{\mu^2}\right]\,c_\theta^4\,M_\theta^8\,M_\pi^4\,s_\theta^4}{48\,\pi^2\,M_\eta^4\,M_{\eta'}^4} + \frac{41\,c_\theta^8\,M_\theta^8\,M_\pi^4\,s_\theta^4}{5184\,\pi^2\,M_\eta^4\,M_{\eta'}^4} + \frac{407\,\text{Log}\left[\frac{M_\eta^2}{\mu^2}\right]\,c_\theta^8\,M_\theta^8\,M_\pi^4\,s_\theta^4}{46\,656\,\pi^2\,M_\eta^4\,M_{\eta'}^4} - \\
& \frac{245\,\text{Log}\left[\frac{M_\eta^2}{\mu^2}\right]\,c_\theta^8\,M_\theta^8\,M_\pi^4\,s_\theta^4}{23\,328\,\pi^2\,M_\eta^4\,M_{\eta'}^4} + \frac{280\,c_\theta^4\,L_6^r\,M_\theta^8\,M_\pi^4\,s_\theta^4}{9\,M_\eta^4\,M_{\eta'}^4} + \frac{64\,c_\theta^4\,L_7^r\,M_\theta^8\,M_\pi^4\,s_\theta^4}{9\,M_\eta^4\,M_{\eta'}^4} + \frac{224\,c_\theta^4\,C_{19}\,M_\theta^8\,M_K^2\,M_\pi^4\,s_\theta^4}{M_\eta^4\,M_{\eta'}^4} + \\
& \frac{640\,c_\theta^4\,C_{31}\,M_\theta^8\,M_K^2\,M_\pi^4\,s_\theta^4}{3\,M_\eta^4\,M_{\eta'}^4} - \frac{56\,c_\theta^4\,C_{19}\,M_\theta^8\,M_\pi^6\,s_\theta^4}{3\,M_\eta^4\,M_{\eta'}^4} - \frac{160\,c_\theta^4\,C_{31}\,M_\theta^8\,M_\pi^6\,s_\theta^4}{9\,M_\eta^4\,M_{\eta'}^4} - \frac{\text{Log}\left[\frac{M_\eta^2}{\mu^2}\right]\,c_\theta^6\,M_\theta^8\,M_K^2\,s_\theta^4}{54\,\pi^2\,M_\eta^2\,M_{\eta'}^4} -
\end{aligned}$$

$$\begin{aligned}
& \frac{5 \operatorname{Log}\left[\frac{M_\eta^2}{\mu^2}\right] c_\theta^6 M_\theta^8 M_\pi^2 s_\theta^4}{243 \pi^2 M_\eta^2 M_{\eta'}^4} + \frac{19 \operatorname{Log}\left[\frac{M_\eta^2}{\mu^2}\right] c_\theta^6 M_\theta^8 M_\pi^2 s_\theta^4}{1728 \pi^2 M_\eta^2 M_{\eta'}^4} + \frac{25 \operatorname{Log}\left[\frac{M_\eta^2}{\mu^2}\right] c_\theta^6 M_\theta^8 M_\pi^2 s_\theta^4}{1944 \pi^2 M_\eta^2 M_{\eta'}^4} - \\
& \frac{7208960 c_\theta^8 L_8^2 r M_\theta^8 M_K^{10} s_\theta^4}{729 F^2 M_\eta^{10} M_{\eta'}^2} + \frac{2023424 c_\theta^8 L_8^2 r M_\theta^8 M_K^8 M_\pi^2 s_\theta^4}{81 F^2 M_\eta^{10} M_{\eta'}^2} - \frac{5783552 c_\theta^8 L_8^2 r M_\theta^8 M_K^6 M_\pi^4 s_\theta^4}{243 F^2 M_\eta^{10} M_{\eta'}^2} + \\
& \frac{7540736 c_\theta^8 L_8^2 r M_\theta^8 M_K^4 M_\pi^6 s_\theta^4}{729 F^2 M_\eta^{10} M_{\eta'}^2} - \frac{434176 c_\theta^8 L_8^2 r M_\theta^8 M_K^2 M_\pi^8 s_\theta^4}{243 F^2 M_\eta^{10} M_{\eta'}^2} - \frac{512 c_\theta^8 L_8^2 r M_\theta^8 M_\pi^{10} s_\theta^4}{27 F^2 M_\eta^{10} M_{\eta'}^2} + \\
& \frac{64 F^2 v_2^{(2)} c_\theta^6 M_\theta^8 M_K^4 s_\theta^4}{27 M_\eta^8 M_{\eta'}^2} - \frac{26 \operatorname{Log}\left[\frac{M_K^2}{\mu^2}\right] c_\theta^6 M_\theta^8 M_K^6 s_\theta^4}{243 \pi^2 M_\eta^8 M_{\eta'}^2} + \frac{13312 c_\theta^6 L_6^r M_\theta^8 M_K^6 s_\theta^4}{243 M_\eta^8 M_{\eta'}^2} + \\
& \frac{13312 c_\theta^6 L_7^r M_\theta^8 M_K^6 s_\theta^4}{243 M_\eta^8 M_{\eta'}^2} - \frac{6656 c_\theta^6 L_{25}^r M_\theta^8 M_K^6 s_\theta^4}{81 M_\eta^8 M_{\eta'}^2} + \frac{26624 c_\theta^6 C_{19} M_\theta^8 M_K^8 s_\theta^4}{81 M_\eta^8 M_{\eta'}^2} + \frac{53248 c_\theta^6 C_{31} M_\theta^8 M_K^8 s_\theta^4}{243 M_\eta^8 M_{\eta'}^2} + \\
& \frac{4 F^2 v_2^{(2)} c_\theta^6 M_\theta^8 M_K^2 M_\pi^2 s_\theta^4}{27 M_\eta^8 M_{\eta'}^2} + \frac{\operatorname{Log}\left[\frac{M_K^2}{\mu^2}\right] c_\theta^6 M_\theta^8 M_K^4 M_\pi^2 s_\theta^4}{9 \pi^2 M_\eta^8 M_{\eta'}^2} - \frac{3520 c_\theta^6 L_6^r M_\theta^8 M_K^4 M_\pi^2 s_\theta^4}{81 M_\eta^8 M_{\eta'}^2} - \\
& \frac{4288 c_\theta^6 L_7^r M_\theta^8 M_K^4 M_\pi^2 s_\theta^4}{81 M_\eta^8 M_{\eta'}^2} + \frac{10624 c_\theta^6 L_{25}^r M_\theta^8 M_K^4 M_\pi^2 s_\theta^4}{81 M_\eta^8 M_{\eta'}^2} - \frac{52352 c_\theta^6 C_{19} M_\theta^8 M_K^6 M_\pi^2 s_\theta^4}{81 M_\eta^8 M_{\eta'}^2} - \\
& \frac{104704 c_\theta^6 C_{31} M_\theta^8 M_K^6 M_\pi^2 s_\theta^4}{243 M_\eta^8 M_{\eta'}^2} - \frac{14 F^2 v_2^{(2)} c_\theta^6 M_\theta^8 M_\pi^4 s_\theta^4}{27 M_\eta^8 M_{\eta'}^2} - \frac{25 \operatorname{Log}\left[\frac{M_K^2}{\mu^2}\right] c_\theta^6 M_\theta^8 M_K^2 M_\pi^4 s_\theta^4}{972 \pi^2 M_\eta^8 M_{\eta'}^2} + \\
& \frac{17 \operatorname{Log}\left[\frac{M_\pi^2}{\mu^2}\right] c_\theta^6 M_\theta^8 M_K^2 M_\pi^4 s_\theta^4}{324 \pi^2 M_\eta^8 M_{\eta'}^2} - \frac{704 c_\theta^6 L_6^r M_\theta^8 M_K^2 M_\pi^4 s_\theta^4}{81 M_\eta^8 M_{\eta'}^2} - \frac{1280 c_\theta^6 L_7^r M_\theta^8 M_K^2 M_\pi^4 s_\theta^4}{81 M_\eta^8 M_{\eta'}^2} - \\
& \frac{4736 c_\theta^6 L_{25}^r M_\theta^8 M_K^2 M_\pi^4 s_\theta^4}{81 M_\eta^8 M_{\eta'}^2} + \frac{4288 c_\theta^6 C_{19} M_\theta^8 M_K^4 M_\pi^4 s_\theta^4}{9 M_\eta^8 M_{\eta'}^2} + \frac{8576 c_\theta^6 C_{31} M_\theta^8 M_K^4 M_\pi^4 s_\theta^4}{27 M_\eta^8 M_{\eta'}^2} - \\
& \frac{53 \operatorname{Log}\left[\frac{M_\pi^2}{\mu^2}\right] c_\theta^6 M_\theta^8 M_\pi^6 s_\theta^4}{1296 \pi^2 M_\eta^8 M_{\eta'}^2} + \frac{3248 c_\theta^6 L_6^r M_\theta^8 M_\pi^6 s_\theta^4}{243 M_\eta^8 M_{\eta'}^2} + \frac{4688 c_\theta^6 L_7^r M_\theta^8 M_\pi^6 s_\theta^4}{243 M_\eta^8 M_{\eta'}^2} + \frac{112 c_\theta^6 L_{25}^r M_\theta^8 M_\pi^6 s_\theta^4}{27 M_\eta^8 M_{\eta'}^2} - \\
& \frac{14816 c_\theta^6 C_{19} M_\theta^8 M_K^2 M_\pi^6 s_\theta^4}{81 M_\eta^8 M_{\eta'}^2} - \frac{29632 c_\theta^6 C_{31} M_\theta^8 M_K^2 M_\pi^6 s_\theta^4}{243 M_\eta^8 M_{\eta'}^2} + \frac{3248 c_\theta^6 C_{19} M_\theta^8 M_\pi^8 s_\theta^4}{81 M_\eta^8 M_{\eta'}^2} + \\
& \frac{6496 c_\theta^6 C_{31} M_\theta^8 M_\pi^8 s_\theta^4}{243 M_\eta^8 M_{\eta'}^2} + \frac{2 \text{g1Dk} c_\theta^4 M_\theta^8 s_\theta^4}{15 M_\eta^6 M_{\eta'}^2} - \frac{16 F^2 v_2^{(2)} c_\theta^4 M_\theta^8 M_K^2 s_\theta^4}{3 M_\eta^6 M_{\eta'}^2} - \frac{128 F^2 v_2^{(2)} c_\theta^4 M_\theta^6 M_K^4 s_\theta^4}{27 M_\eta^6 M_{\eta'}^2} + \\
& \frac{c_\theta^4 M_\theta^8 M_K^4 s_\theta^4}{54 \pi^2 M_\eta^6 M_{\eta'}^2} + \frac{17 \operatorname{Log}\left[\frac{M_K^2}{\mu^2}\right] c_\theta^4 M_\theta^8 M_K^4 s_\theta^4}{810 \pi^2 M_\eta^6 M_{\eta'}^2} + \frac{13 c_\theta^8 M_\theta^8 M_K^4 s_\theta^4}{243 \pi^2 M_\eta^6 M_{\eta'}^2} - \frac{8 \operatorname{Log}\left[\frac{M_\eta^2}{\mu^2}\right] c_\theta^8 M_\theta^8 M_K^4 s_\theta^4}{243 \pi^2 M_\eta^6 M_{\eta'}^2} + \\
& \frac{19 \operatorname{Log}\left[\frac{M_\eta^2}{\mu^2}\right] c_\theta^8 M_\theta^8 M_K^4 s_\theta^4}{729 \pi^2 M_\eta^6 M_{\eta'}^2} - \frac{1024 c_\theta^4 L_6^r M_\theta^8 M_K^4 s_\theta^4}{81 M_\eta^6 M_{\eta'}^2} - \frac{1024 c_\theta^4 L_7^r M_\theta^8 M_K^4 s_\theta^4}{81 M_\eta^6 M_{\eta'}^2} - \frac{3584 c_\theta^4 C_{19} M_\theta^8 M_K^6 s_\theta^4}{27 M_\eta^6 M_{\eta'}^2} - \\
& \frac{10240 c_\theta^4 C_{31} M_\theta^8 M_K^6 s_\theta^4}{81 M_\eta^6 M_{\eta'}^2} + \frac{4 F^2 v_2^{(2)} c_\theta^4 M_\theta^8 M_\pi^2 s_\theta^4}{3 M_\eta^6 M_{\eta'}^2} - \frac{80 F^2 v_2^{(2)} c_\theta^4 M_\theta^6 M_K^2 M_\pi^2 s_\theta^4}{27 M_\eta^6 M_{\eta'}^2} - \frac{5 c_\theta^4 M_\theta^8 M_K^2 M_\pi^2 s_\theta^4}{216 \pi^2 M_\eta^6 M_{\eta'}^2} -
\end{aligned}$$



$$\begin{aligned}
& \frac{209 \operatorname{Log}\left[\frac{M_K^2}{\mu^2}\right] c_\theta^4 M_\theta^8 M_K^2 M_\pi^2 s_\theta^4}{6480 \pi^2 M_\eta^6 M_{\eta'}^2} - \frac{31 c_\theta^8 M_\theta^8 M_K^2 M_\pi^2 s_\theta^4}{486 \pi^2 M_\eta^6 M_{\eta'}^2} + \frac{35 \operatorname{Log}\left[\frac{M_\eta^2}{\mu^2}\right] c_\theta^8 M_\theta^8 M_K^2 M_\pi^2 s_\theta^4}{972 \pi^2 M_\eta^6 M_{\eta'}^2} - \\
& \frac{65 \operatorname{Log}\left[\frac{M_\eta^2}{\mu^2}\right] c_\theta^8 M_\theta^8 M_K^2 M_\pi^2 s_\theta^4}{2916 \pi^2 M_\eta^6 M_{\eta'}^2} + \frac{1952 c_\theta^4 L_6^r M_\theta^8 M_K^2 M_\pi^2 s_\theta^4}{81 M_\eta^6 M_{\eta'}^2} - \frac{640 c_\theta^4 L_7^r M_\theta^8 M_K^2 M_\pi^2 s_\theta^4}{81 M_\eta^6 M_{\eta'}^2} + \\
& \frac{1792 c_\theta^4 C_{19} M_\theta^8 M_K^4 M_\pi^2 s_\theta^4}{9 M_\eta^6 M_{\eta'}^2} + \frac{5120 c_\theta^4 C_{31} M_\theta^8 M_K^4 M_\pi^2 s_\theta^4}{27 M_\eta^6 M_{\eta'}^2} - \frac{8 F^2 v_2^{(2)} c_\theta^4 M_\theta^8 M_\pi^4 s_\theta^4}{27 M_\eta^6 M_{\eta'}^2} + \frac{c_\theta^4 M_\theta^8 M_\pi^4 s_\theta^4}{48 \pi^2 M_\eta^6 M_{\eta'}^2} + \\
& \frac{\operatorname{Log}\left[\frac{M_K^2}{\mu^2}\right] c_\theta^4 M_\theta^8 M_\pi^4 s_\theta^4}{288 \pi^2 M_\eta^6 M_{\eta'}^2} + \frac{5 \operatorname{Log}\left[\frac{M_\pi^2}{\mu^2}\right] c_\theta^4 M_\theta^8 M_\pi^4 s_\theta^4}{216 \pi^2 M_\eta^6 M_{\eta'}^2} + \frac{161 c_\theta^8 M_\theta^8 M_\pi^4 s_\theta^4}{7776 \pi^2 M_\eta^6 M_{\eta'}^2} - \frac{\operatorname{Log}\left[\frac{M_\eta^2}{\mu^2}\right] c_\theta^8 M_\theta^8 M_\pi^4 s_\theta^4}{96 \pi^2 M_\eta^6 M_{\eta'}^2} + \\
& \frac{4 \operatorname{Log}\left[\frac{M_{\eta'}^2}{\mu^2}\right] c_\theta^8 M_\theta^8 M_\pi^4 s_\theta^4}{729 \pi^2 M_\eta^6 M_{\eta'}^2} - \frac{1360 c_\theta^4 L_6^r M_\theta^8 M_\pi^4 s_\theta^4}{81 M_\eta^6 M_{\eta'}^2} - \frac{64 c_\theta^4 L_7^r M_\theta^8 M_\pi^4 s_\theta^4}{81 M_\eta^6 M_{\eta'}^2} - \frac{896 c_\theta^4 C_{19} M_\theta^8 M_K^2 M_\pi^4 s_\theta^4}{9 M_\eta^6 M_{\eta'}^2} - \\
& \frac{2560 c_\theta^4 C_{31} M_\theta^8 M_K^2 M_\pi^4 s_\theta^4}{27 M_\eta^6 M_{\eta'}^2} - \frac{112 c_\theta^4 C_{19} M_\theta^8 M_\pi^4 s_\theta^4}{27 M_\eta^6 M_{\eta'}^2} - \frac{320 c_\theta^4 C_{31} M_\theta^8 M_\pi^4 s_\theta^4}{81 M_\eta^6 M_{\eta'}^2} + \frac{\operatorname{Log}\left[\frac{M_\eta^2}{\mu^2}\right] c_\theta^6 M_\theta^8 M_K^2 s_\theta^4}{81 \pi^2 M_\eta^4 M_{\eta'}^2} + \\
& \frac{\operatorname{Log}\left[\frac{M_\eta^2}{\mu^2}\right] c_\theta^6 M_\theta^8 M_K^2 s_\theta^4}{72 \pi^2 M_\eta^4 M_{\eta'}^2} - \frac{13 \operatorname{Log}\left[\frac{M_\eta^2}{\mu^2}\right] c_\theta^6 M_\theta^8 M_\pi^2 s_\theta^4}{2592 \pi^2 M_\eta^4 M_{\eta'}^2} - \frac{\operatorname{Log}\left[\frac{M_\eta^2}{\mu^2}\right] c_\theta^6 M_\theta^8 M_\pi^2 s_\theta^4}{108 \pi^2 M_\eta^4 M_{\eta'}^2} - \\
& \frac{4 \operatorname{Log}\left[\frac{M_\eta^2}{\mu^2}\right] c_\theta^8 M_\theta^8 M_K^2 M_{\eta'}^2 s_\theta^4}{729 \pi^2 M_\eta^{10}} + \frac{11 \operatorname{Log}\left[\frac{M_\eta^2}{\mu^2}\right] c_\theta^8 M_\theta^8 M_K^2 M_\pi^2 M_{\eta'}^2 s_\theta^4}{2916 \pi^2 M_\eta^{10}} - \frac{7 \operatorname{Log}\left[\frac{M_\eta^2}{\mu^2}\right] c_\theta^8 M_\theta^8 M_\pi^4 M_{\eta'}^2 s_\theta^4}{11664 \pi^2 M_\eta^{10}} + \\
& \frac{\operatorname{Log}\left[\frac{M_\eta^2}{\mu^2}\right] c_\theta^6 M_\theta^8 M_K^2 M_{\eta'}^2 s_\theta^4}{972 \pi^2 M_\eta^8} - \frac{7 \operatorname{Log}\left[\frac{M_\eta^2}{\mu^2}\right] c_\theta^6 M_\theta^8 M_\pi^2 M_{\eta'}^2 s_\theta^4}{15552 \pi^2 M_\eta^8} + \frac{2 \operatorname{Log}\left[\frac{M_\eta^2}{\mu^2}\right] c_\theta^8 M_\theta^8 M_\pi^4 s_\theta^4}{243 \pi^2 M_\eta^6 (M_\eta^2 - M_{\eta'}^2)} + \\
& \frac{4 \operatorname{Log}\left[\frac{M_\eta^2}{\mu^2}\right] c_\theta^8 M_\theta^8 M_K^4 s_\theta^4}{243 \pi^2 M_\eta^6 (M_\eta^2 - M_{\eta'}^2)} - \frac{5 \operatorname{Log}\left[\frac{M_\eta^2}{\mu^2}\right] c_\theta^8 M_\theta^8 M_K^2 M_\pi^2 s_\theta^4}{486 \pi^2 M_\eta^6 (M_\eta^2 - M_{\eta'}^2)} - \frac{13 \operatorname{Log}\left[\frac{M_\eta^2}{\mu^2}\right] c_\theta^8 M_\theta^8 M_K^2 M_\pi^2 s_\theta^4}{486 \pi^2 M_\eta^6 (M_\eta^2 - M_{\eta'}^2)} + \\
& \frac{25 \operatorname{Log}\left[\frac{M_\eta^2}{\mu^2}\right] c_\theta^8 M_\theta^8 M_\pi^4 s_\theta^4}{7776 \pi^2 M_\eta^6 (M_\eta^2 - M_{\eta'}^2)} + \frac{11 \operatorname{Log}\left[\frac{M_\eta^2}{\mu^2}\right] c_\theta^8 M_\theta^8 M_\pi^4 s_\theta^4}{1944 \pi^2 M_\eta^6 (M_\eta^2 - M_{\eta'}^2)} - \frac{5 \operatorname{Log}\left[\frac{M_\eta^2}{\mu^2}\right] c_\theta^8 M_\theta^8 M_K^4 M_{\eta'}^2 s_\theta^4}{486 \pi^2 M_{\eta'}^6 (M_\eta^2 - M_{\eta'}^2)} + \\
& \frac{19 \operatorname{Log}\left[\frac{M_\eta^2}{\mu^2}\right] c_\theta^8 M_\theta^8 M_K^2 M_\pi^2 M_{\eta'}^2 s_\theta^4}{1944 \pi^2 M_{\eta'}^8 (M_\eta^2 - M_{\eta'}^2)} - \frac{23 \operatorname{Log}\left[\frac{M_\eta^2}{\mu^2}\right] c_\theta^8 M_\theta^8 M_\pi^4 M_{\eta'}^2 s_\theta^4}{7776 \pi^2 M_{\eta'}^8 (M_\eta^2 - M_{\eta'}^2)} + \frac{11 \operatorname{Log}\left[\frac{M_\eta^2}{\mu^2}\right] c_\theta^8 M_\theta^8 M_K^4 s_\theta^4}{243 \pi^2 M_{\eta'}^6 (M_\eta^2 - M_{\eta'}^2)} + \\
& \frac{5 \operatorname{Log}\left[\frac{M_\eta^2}{\mu^2}\right] c_\theta^8 M_\theta^8 M_K^4 s_\theta^4}{486 \pi^2 M_{\eta'}^6 (M_\eta^2 - M_{\eta'}^2)} - \frac{37 \operatorname{Log}\left[\frac{M_\eta^2}{\mu^2}\right] c_\theta^8 M_\theta^8 M_K^2 M_\pi^2 s_\theta^4}{972 \pi^2 M_{\eta'}^6 (M_\eta^2 - M_{\eta'}^2)} - \frac{19 \operatorname{Log}\left[\frac{M_\eta^2}{\mu^2}\right] c_\theta^8 M_\theta^8 M_K^2 M_\pi^2 s_\theta^4}{1944 \pi^2 M_{\eta'}^6 (M_\eta^2 - M_{\eta'}^2)} + \\
& \frac{13 \operatorname{Log}\left[\frac{M_\eta^2}{\mu^2}\right] c_\theta^8 M_\theta^8 M_\pi^4 s_\theta^4}{1944 \pi^2 M_{\eta'}^6 (M_\eta^2 - M_{\eta'}^2)} + \frac{23 \operatorname{Log}\left[\frac{M_\eta^2}{\mu^2}\right] c_\theta^8 M_\theta^8 M_\pi^4 s_\theta^4}{7776 \pi^2 M_{\eta'}^6 (M_\eta^2 - M_{\eta'}^2)} - \frac{2 \operatorname{Log}\left[\frac{M_\eta^2}{\mu^2}\right] c_\theta^8 M_\theta^8 M_K^4 s_\theta^4}{81 \pi^2 M_\eta^2 M_{\eta'}^4 (M_\eta^2 - M_{\eta'}^2)} -
\end{aligned}$$

$$\begin{aligned}
& \frac{11 \operatorname{Log}\left[\frac{M_\eta^2}{\mu^2}\right] c_\theta^8 M_\theta^8 M_K^4 s_\theta^4}{243 \pi^2 M_\eta^2 M_{\eta'}^4 (M_\eta^2 - M_{\eta'}^2)} + \frac{5 \operatorname{Log}\left[\frac{M_\eta^2}{\mu^2}\right] c_\theta^8 M_\theta^8 M_K^2 M_\pi^2 s_\theta^4}{648 \pi^2 M_\eta^2 M_{\eta'}^4 (M_\eta^2 - M_{\eta'}^2)} + \frac{37 \operatorname{Log}\left[\frac{M_\eta^2}{\mu^2}\right] c_\theta^8 M_\theta^8 M_K^2 M_\pi^2 s_\theta^4}{972 \pi^2 M_\eta^2 M_{\eta'}^4 (M_\eta^2 - M_{\eta'}^2)} + \\
& \frac{\operatorname{Log}\left[\frac{M_\eta^2}{\mu^2}\right] c_\theta^8 M_\theta^8 M_\pi^4 s_\theta^4}{1296 \pi^2 M_\eta^2 M_{\eta'}^4 (M_\eta^2 - M_{\eta'}^2)} - \frac{13 \operatorname{Log}\left[\frac{M_\eta^2}{\mu^2}\right] c_\theta^8 M_\theta^8 M_\pi^4 s_\theta^4}{1944 \pi^2 M_\eta^2 M_{\eta'}^4 (M_\eta^2 - M_{\eta'}^2)} - \frac{4 \operatorname{Log}\left[\frac{M_\eta^2}{\mu^2}\right] c_\theta^8 M_\theta^8 M_K^4 s_\theta^4}{243 \pi^2 M_\eta^4 M_{\eta'}^2 (M_\eta^2 - M_{\eta'}^2)} + \\
& \frac{2 \operatorname{Log}\left[\frac{M_\eta^2}{\mu^2}\right] c_\theta^8 M_\theta^8 M_K^4 s_\theta^4}{81 \pi^2 M_\eta^4 M_{\eta'}^2 (M_\eta^2 - M_{\eta'}^2)} + \frac{13 \operatorname{Log}\left[\frac{M_\eta^2}{\mu^2}\right] c_\theta^8 M_\theta^8 M_K^2 M_\pi^2 s_\theta^4}{486 \pi^2 M_\eta^4 M_{\eta'}^2 (M_\eta^2 - M_{\eta'}^2)} - \frac{5 \operatorname{Log}\left[\frac{M_\eta^2}{\mu^2}\right] c_\theta^8 M_\theta^8 M_K^2 M_\pi^2 s_\theta^4}{648 \pi^2 M_\eta^4 M_{\eta'}^2 (M_\eta^2 - M_{\eta'}^2)} - \\
& \frac{11 \operatorname{Log}\left[\frac{M_\eta^2}{\mu^2}\right] c_\theta^8 M_\theta^8 M_\pi^4 s_\theta^4}{1944 \pi^2 M_\eta^4 M_{\eta'}^2 (M_\eta^2 - M_{\eta'}^2)} - \frac{\operatorname{Log}\left[\frac{M_\eta^2}{\mu^2}\right] c_\theta^8 M_\theta^8 M_\pi^4 s_\theta^4}{1296 \pi^2 M_\eta^4 M_{\eta'}^2 (M_\eta^2 - M_{\eta'}^2)} - \frac{2 \operatorname{Log}\left[\frac{M_\eta^2}{\mu^2}\right] c_\theta^8 M_\theta^8 M_K^4 M_{\eta'}^2 s_\theta^4}{243 \pi^2 M_\eta^8 (M_\eta^2 - M_{\eta'}^2)} + \\
& \frac{5 \operatorname{Log}\left[\frac{M_\eta^2}{\mu^2}\right] c_\theta^8 M_\theta^8 M_K^2 M_\pi^2 M_{\eta'}^2 s_\theta^4}{486 \pi^2 M_\eta^8 (M_\eta^2 - M_{\eta'}^2)} - \frac{25 \operatorname{Log}\left[\frac{M_\eta^2}{\mu^2}\right] c_\theta^8 M_\theta^8 M_\pi^4 M_{\eta'}^2 s_\theta^4}{7776 \pi^2 M_\eta^8 (M_\eta^2 - M_{\eta'}^2)} - \frac{2 \, 621 \, 440 \, \sqrt{2} \, c_\theta^7 L_8^2 r M_\theta^8 M_K^{10} s_\theta^5}{729 F^2 M_\eta^{12}} + \\
& \frac{81 \, 920 \, \sqrt{2} \, c_\theta^7 L_8^2 r M_\theta^8 M_K^8 M_\pi^2 s_\theta^5}{9 F^2 M_\eta^{12}} - \frac{2 \, 293 \, 760 \, \sqrt{2} \, c_\theta^7 L_8^2 r M_\theta^8 M_K^6 M_\pi^4 s_\theta^5}{243 F^2 M_\eta^{12}} + \\
& \frac{3 \, 696 \, 640 \, \sqrt{2} \, c_\theta^7 L_8^2 r M_\theta^8 M_K^4 M_\pi^6 s_\theta^5}{729 F^2 M_\eta^{12}} - \frac{112 \, 640 \, \sqrt{2} \, c_\theta^7 L_8^2 r M_\theta^8 M_K^2 M_\pi^8 s_\theta^5}{81 F^2 M_\eta^{12}} + \\
& \frac{12 \, 800 \, \sqrt{2} \, c_\theta^7 L_8^2 r M_\theta^8 M_\pi^{10} s_\theta^5}{81 F^2 M_\eta^{12}} - \frac{4 \, \sqrt{2} \operatorname{Log}\left[\frac{M_K^2}{\mu^2}\right] c_\theta^5 M_\theta^8 M_K^6 s_\theta^5}{243 \pi^2 M_\eta^{10}} + \frac{2048 \, \sqrt{2} \, c_\theta^5 L_6^r M_\theta^8 M_K^6 s_\theta^5}{81 M_\eta^{10}} + \\
& \frac{2048 \, \sqrt{2} \, c_\theta^5 L_7^r M_\theta^8 M_K^6 s_\theta^5}{81 M_\eta^{10}} - \frac{1024 \, \sqrt{2} \, c_\theta^5 L_{25}^r M_\theta^8 M_K^6 s_\theta^5}{81 M_\eta^{10}} + \frac{4096 \, \sqrt{2} \, c_\theta^5 C_{19} M_\theta^8 M_K^8 s_\theta^5}{27 M_\eta^{10}} + \\
& \frac{8192 \, \sqrt{2} \, c_\theta^5 C_{31} M_\theta^8 M_K^8 s_\theta^5}{81 M_\eta^{10}} + \frac{7 \operatorname{Log}\left[\frac{M_K^2}{\mu^2}\right] c_\theta^5 M_\theta^8 M_K^4 M_\pi^2 s_\theta^5}{486 \sqrt{2} \pi^2 M_\eta^{10}} + \frac{4 \, \sqrt{2} \operatorname{Log}\left[\frac{M_K^2}{\mu^2}\right] c_\theta^5 M_\theta^8 M_K^4 M_\pi^2 s_\theta^5}{243 \pi^2 M_\eta^{10}} - \\
& \frac{128 \, \sqrt{2} \, c_\theta^5 L_6^r M_\theta^8 M_K^4 M_\pi^2 s_\theta^5}{9 M_\eta^{10}} - \frac{1408 \, \sqrt{2} \, c_\theta^5 L_7^r M_\theta^8 M_K^4 M_\pi^2 s_\theta^5}{27 M_\eta^{10}} + \frac{1472 \, \sqrt{2} \, c_\theta^5 L_{25}^r M_\theta^8 M_K^4 M_\pi^2 s_\theta^5}{81 M_\eta^{10}} - \\
& \frac{2816 \, \sqrt{2} \, c_\theta^5 C_{19} M_\theta^8 M_K^6 M_\pi^2 s_\theta^5}{9 M_\eta^{10}} - \frac{5632 \, \sqrt{2} \, c_\theta^5 C_{31} M_\theta^8 M_K^6 M_\pi^2 s_\theta^5}{27 M_\eta^{10}} - \frac{17 \operatorname{Log}\left[\frac{M_K^2}{\mu^2}\right] c_\theta^5 M_\theta^8 M_K^2 M_\pi^4 s_\theta^5}{972 \sqrt{2} \pi^2 M_\eta^{10}} - \\
& \frac{64 \, \sqrt{2} \, c_\theta^5 L_6^r M_\theta^8 M_K^2 M_\pi^4 s_\theta^5}{9 M_\eta^{10}} + \frac{320 \, \sqrt{2} \, c_\theta^5 L_7^r M_\theta^8 M_K^2 M_\pi^4 s_\theta^5}{9 M_\eta^{10}} - \frac{448 \, \sqrt{2} \, c_\theta^5 L_{25}^r M_\theta^8 M_K^2 M_\pi^4 s_\theta^5}{81 M_\eta^{10}} + \\
& \frac{2176 \, \sqrt{2} \, c_\theta^5 C_{19} M_\theta^8 M_K^4 M_\pi^4 s_\theta^5}{9 M_\eta^{10}} + \frac{4352 \, \sqrt{2} \, c_\theta^5 C_{31} M_\theta^8 M_K^4 M_\pi^4 s_\theta^5}{27 M_\eta^{10}} + \frac{\operatorname{Log}\left[\frac{M_\pi^2}{\mu^2}\right] c_\theta^5 M_\theta^8 M_\pi^6 s_\theta^5}{216 \sqrt{2} \pi^2 M_\eta^{10}} + \\
& \frac{256 \, \sqrt{2} \, c_\theta^5 L_6^r M_\theta^8 M_\pi^6 s_\theta^5}{81 M_\eta^{10}} - \frac{704 \, \sqrt{2} \, c_\theta^5 L_7^r M_\theta^8 M_\pi^6 s_\theta^5}{81 M_\eta^{10}} - \frac{2240 \, \sqrt{2} \, c_\theta^5 C_{19} M_\theta^8 M_K^2 M_\pi^6 s_\theta^5}{27 M_\eta^{10}} -
\end{aligned}$$

$$\begin{aligned}
& \frac{4480 \sqrt{2} c_\theta^5 C_{31} M_\theta^8 M_K^2 M_\pi^6 s_\theta^5}{81 M_\eta^{10}} + \frac{256 \sqrt{2} c_\theta^5 C_{19} M_\theta^8 M_\pi^8 s_\theta^5}{27 M_\eta^{10}} + \frac{512 \sqrt{2} c_\theta^5 C_{31} M_\theta^8 M_\pi^8 s_\theta^5}{81 M_\eta^{10}} - \\
& \frac{128 \sqrt{2} F^2 v_2^{(2)} c_\theta^3 M_\theta^6 M_K^4 s_\theta^5}{27 M_\eta^8} - \frac{11 \text{Log}\left[\frac{M_K^2}{\mu^2}\right] c_\theta^3 M_\theta^8 M_K^4 s_\theta^5}{1620 \sqrt{2} \pi^2 M_\eta^8} + \frac{7 \sqrt{2} c_\theta^7 M_\theta^8 M_K^4 s_\theta^5}{243 \pi^2 M_\eta^8} - \\
& \frac{8 \sqrt{2} \text{Log}\left[\frac{M_\eta^2}{\mu^2}\right] c_\theta^7 M_\theta^8 M_K^4 s_\theta^5}{729 \pi^2 M_\eta^8} + \frac{11 \sqrt{2} \text{Log}\left[\frac{M_\eta^2}{\mu^2}\right] c_\theta^7 M_\theta^8 M_K^4 s_\theta^5}{243 \pi^2 M_\eta^8} - \frac{1024 \sqrt{2} c_\theta^3 L_6^r M_\theta^8 M_K^4 s_\theta^5}{81 M_\eta^8} - \\
& \frac{1024 \sqrt{2} c_\theta^3 L_7^r M_\theta^8 M_K^4 s_\theta^5}{81 M_\eta^8} - \frac{3584 \sqrt{2} c_\theta^3 C_{19} M_\theta^8 M_K^6 s_\theta^5}{27 M_\eta^8} - \frac{10240 \sqrt{2} c_\theta^3 C_{31} M_\theta^8 M_K^6 s_\theta^5}{81 M_\eta^8} + \\
& \frac{16 \sqrt{2} F^2 v_2^{(2)} c_\theta^3 M_\theta^6 M_K^2 M_\pi^2 s_\theta^5}{27 M_\eta^8} - \frac{c_\theta^3 M_\theta^8 M_K^2 M_\pi^2 s_\theta^5}{216 \sqrt{2} \pi^2 M_\eta^8} - \frac{\text{Log}\left[\frac{M_K^2}{\mu^2}\right] c_\theta^3 M_\theta^8 M_K^2 M_\pi^2 s_\theta^5}{1080 \sqrt{2} \pi^2 M_\eta^8} - \\
& \frac{8 \sqrt{2} c_\theta^7 M_\theta^8 M_K^2 M_\pi^2 s_\theta^5}{243 \pi^2 M_\eta^8} - \frac{17 \text{Log}\left[\frac{M_\eta^2}{\mu^2}\right] c_\theta^7 M_\theta^8 M_K^2 M_\pi^2 s_\theta^5}{243 \sqrt{2} \pi^2 M_\eta^8} + \frac{34 \sqrt{2} \text{Log}\left[\frac{M_\eta^2}{\mu^2}\right] c_\theta^7 M_\theta^8 M_K^2 M_\pi^2 s_\theta^5}{729 \pi^2 M_\eta^8} - \\
& \frac{11 \text{Log}\left[\frac{M_\eta^2}{\mu^2}\right] c_\theta^7 M_\theta^8 M_K^2 M_\pi^2 s_\theta^5}{1458 \sqrt{2} \pi^2 M_\eta^8} - \frac{22 \sqrt{2} \text{Log}\left[\frac{M_\eta^2}{\mu^2}\right] c_\theta^7 M_\theta^8 M_K^2 M_\pi^2 s_\theta^5}{729 \pi^2 M_\eta^8} + \frac{992 \sqrt{2} c_\theta^3 L_6^r M_\theta^8 M_K^2 M_\pi^2 s_\theta^5}{81 M_\eta^8} + \\
& \frac{992 \sqrt{2} c_\theta^3 L_7^r M_\theta^8 M_K^2 M_\pi^2 s_\theta^5}{81 M_\eta^8} + \frac{1792 \sqrt{2} c_\theta^3 C_{19} M_\theta^8 M_K^4 M_\pi^2 s_\theta^5}{9 M_\eta^8} + \frac{5120 \sqrt{2} c_\theta^3 C_{31} M_\theta^8 M_K^4 M_\pi^2 s_\theta^5}{27 M_\eta^8} + \\
& \frac{40 \sqrt{2} F^2 v_2^{(2)} c_\theta^3 M_\theta^6 M_K^4 s_\theta^5}{27 M_\eta^8} - \frac{c_\theta^3 M_\theta^8 M_K^4 s_\theta^5}{216 \sqrt{2} \pi^2 M_\eta^8} + \frac{\text{Log}\left[\frac{M_K^2}{\mu^2}\right] c_\theta^3 M_\theta^8 M_K^4 s_\theta^5}{432 \sqrt{2} \pi^2 M_\eta^8} - \frac{\text{Log}\left[\frac{M_\pi^2}{\mu^2}\right] c_\theta^3 M_\theta^8 M_K^4 s_\theta^5}{108 \sqrt{2} \pi^2 M_\eta^8} + \\
& \frac{c_\theta^7 M_\theta^8 M_K^4 s_\theta^5}{972 \sqrt{2} \pi^2 M_\eta^8} + \frac{2 \sqrt{2} c_\theta^7 M_\theta^8 M_K^4 s_\theta^5}{243 \pi^2 M_\eta^8} - \frac{131 \text{Log}\left[\frac{M_\eta^2}{\mu^2}\right] c_\theta^7 M_\theta^8 M_K^4 s_\theta^5}{5832 \sqrt{2} \pi^2 M_\eta^8} + \frac{2 \sqrt{2} \text{Log}\left[\frac{M_\eta^2}{\mu^2}\right] c_\theta^7 M_\theta^8 M_K^4 s_\theta^5}{243 \pi^2 M_\eta^8} - \\
& \frac{\text{Log}\left[\frac{M_\eta^2}{\mu^2}\right] c_\theta^7 M_\theta^8 M_K^4 s_\theta^5}{1944 \sqrt{2} \pi^2 M_\eta^8} + \frac{2 \sqrt{2} \text{Log}\left[\frac{M_\eta^2}{\mu^2}\right] c_\theta^7 M_\theta^8 M_K^4 s_\theta^5}{243 \pi^2 M_\eta^8} - \frac{112 \sqrt{2} c_\theta^3 L_6^r M_\theta^8 M_K^4 s_\theta^5}{81 M_\eta^8} - \\
& \frac{112 \sqrt{2} c_\theta^3 L_7^r M_\theta^8 M_K^4 s_\theta^5}{81 M_\eta^8} - \frac{896 \sqrt{2} c_\theta^3 C_{19} M_\theta^8 M_K^2 M_\pi^4 s_\theta^5}{9 M_\eta^8} - \frac{2560 \sqrt{2} c_\theta^3 C_{31} M_\theta^8 M_K^2 M_\pi^4 s_\theta^5}{27 M_\eta^8} + \\
& \frac{560 \sqrt{2} c_\theta^3 C_{19} M_\theta^8 M_\pi^6 s_\theta^5}{27 M_\eta^8} + \frac{1600 \sqrt{2} c_\theta^3 C_{31} M_\theta^8 M_\pi^6 s_\theta^5}{81 M_\eta^8} + \frac{16 \sqrt{2} F^2 v_2^{(2)} c_\theta M_\theta^6 M_K^2 s_\theta^5}{3 M_\eta^6} + \\
& \frac{\text{Log}\left[\frac{M_\eta^2}{\mu^2}\right] c_\theta^5 M_\theta^8 M_K^2 s_\theta^5}{81 \sqrt{2} \pi^2 M_\eta^6} - \frac{\text{Log}\left[\frac{M_\eta^2}{\mu^2}\right] c_\theta^5 M_\theta^8 M_K^2 s_\theta^5}{162 \sqrt{2} \pi^2 M_\eta^6} - \frac{16 \sqrt{2} F^2 v_2^{(2)} c_\theta M_\theta^6 M_\pi^2 s_\theta^5}{3 M_\eta^6} -
\end{aligned}$$

$$\begin{aligned}
& \frac{17 \operatorname{Log}\left[\frac{M_\eta^2}{\mu^2}\right] c_\theta^5 M_\theta^8 M_\pi^2 s_\theta^5}{2592 \sqrt{2} \pi^2 M_\eta^6} + \frac{5 \operatorname{Log}\left[\frac{M_\eta^2}{\mu^2}\right] c_\theta^5 M_\theta^8 M_\pi^2 s_\theta^5}{1296 \sqrt{2} \pi^2 M_\eta^6} + \frac{9175040 \sqrt{2} c_\theta^7 L_8^2 r M_\theta^8 M_K^{10} s_\theta^5}{729 F^2 M_\eta^{12}} - \\
& \frac{7577600 \sqrt{2} c_\theta^7 L_8^2 r M_\theta^8 M_K^8 M_\pi^2 s_\theta^5}{243 F^2 M_\eta^{12}} + \frac{7290880 \sqrt{2} c_\theta^7 L_8^2 r M_\theta^8 M_K^6 M_\pi^4 s_\theta^5}{243 F^2 M_\eta^{12}} - \\
& \frac{10311680 \sqrt{2} c_\theta^7 L_8^2 r M_\theta^8 M_K^4 M_\pi^6 s_\theta^5}{729 F^2 M_\eta^{12}} + \frac{819200 \sqrt{2} c_\theta^7 L_8^2 r M_\theta^8 M_K^2 M_\pi^8 s_\theta^5}{243 F^2 M_\eta^{12}} - \\
& \frac{35840 \sqrt{2} c_\theta^7 L_8^2 r M_\theta^8 M_\pi^{10} s_\theta^5}{81 F^2 M_\eta^{12}} + \frac{4 \sqrt{2} \operatorname{Log}\left[\frac{M_\eta^2}{\mu^2}\right] c_\theta^5 M_\theta^8 M_K^6 s_\theta^5}{243 \pi^2 M_\eta^{10}} - \frac{2048 \sqrt{2} c_\theta^5 L_6^r M_\theta^8 M_K^6 s_\theta^5}{81 M_\eta^{10}} - \\
& \frac{2048 \sqrt{2} c_\theta^5 L_7^r M_\theta^8 M_K^6 s_\theta^5}{81 M_\eta^{10}} + \frac{1024 \sqrt{2} c_\theta^5 L_{25}^r M_\theta^8 M_K^6 s_\theta^5}{81 M_\eta^{10}} - \frac{4096 \sqrt{2} c_\theta^5 C_{19} M_\theta^8 M_K^8 s_\theta^5}{27 M_\eta^{10}} - \\
& \frac{8192 \sqrt{2} c_\theta^5 C_{31} M_\theta^8 M_K^8 s_\theta^5}{81 M_\eta^{10}} - \frac{7 \operatorname{Log}\left[\frac{M_K^2}{\mu^2}\right] c_\theta^5 M_\theta^8 M_K^4 M_\pi^2 s_\theta^5}{486 \sqrt{2} \pi^2 M_\eta^{10}} - \frac{4 \sqrt{2} \operatorname{Log}\left[\frac{M_K^2}{\mu^2}\right] c_\theta^5 M_\theta^8 M_K^4 M_\pi^2 s_\theta^5}{243 \pi^2 M_\eta^{10}} + \\
& \frac{128 \sqrt{2} c_\theta^5 L_6^r M_\theta^8 M_K^4 M_\pi^2 s_\theta^5}{9 M_\eta^{10}} + \frac{1408 \sqrt{2} c_\theta^5 L_7^r M_\theta^8 M_K^4 M_\pi^2 s_\theta^5}{27 M_\eta^{10}} - \frac{1472 \sqrt{2} c_\theta^5 L_{25}^r M_\theta^8 M_K^4 M_\pi^2 s_\theta^5}{81 M_\eta^{10}} + \\
& \frac{2816 \sqrt{2} c_\theta^5 C_{19} M_\theta^8 M_K^6 M_\pi^2 s_\theta^5}{9 M_\eta^{10}} + \frac{5632 \sqrt{2} c_\theta^5 C_{31} M_\theta^8 M_K^6 M_\pi^2 s_\theta^5}{27 M_\eta^{10}} + \frac{17 \operatorname{Log}\left[\frac{M_\pi^2}{\mu^2}\right] c_\theta^5 M_\theta^8 M_K^2 M_\pi^4 s_\theta^5}{972 \sqrt{2} \pi^2 M_\eta^{10}} + \\
& \frac{64 \sqrt{2} c_\theta^5 L_6^r M_\theta^8 M_K^2 M_\pi^4 s_\theta^5}{9 M_\eta^{10}} - \frac{320 \sqrt{2} c_\theta^5 L_7^r M_\theta^8 M_K^2 M_\pi^4 s_\theta^5}{9 M_\eta^{10}} + \frac{448 \sqrt{2} c_\theta^5 L_{25}^r M_\theta^8 M_K^2 M_\pi^4 s_\theta^5}{81 M_\eta^{10}} - \\
& \frac{2176 \sqrt{2} c_\theta^5 C_{19} M_\theta^8 M_K^4 M_\pi^4 s_\theta^5}{9 M_\eta^{10}} - \frac{4352 \sqrt{2} c_\theta^5 C_{31} M_\theta^8 M_K^4 M_\pi^4 s_\theta^5}{27 M_\eta^{10}} - \frac{\operatorname{Log}\left[\frac{M_\pi^2}{\mu^2}\right] c_\theta^5 M_\theta^8 M_\pi^6 s_\theta^5}{216 \sqrt{2} \pi^2 M_\eta^{10}} - \\
& \frac{256 \sqrt{2} c_\theta^5 L_6^r M_\theta^8 M_\pi^6 s_\theta^5}{81 M_\eta^{10}} + \frac{704 \sqrt{2} c_\theta^5 L_7^r M_\theta^8 M_\pi^6 s_\theta^5}{81 M_\eta^{10}} + \frac{2240 \sqrt{2} c_\theta^5 C_{19} M_\theta^8 M_K^2 M_\pi^6 s_\theta^5}{27 M_\eta^{10}} + \\
& \frac{4480 \sqrt{2} c_\theta^5 C_{31} M_\theta^8 M_K^2 M_\pi^6 s_\theta^5}{81 M_\eta^{10}} - \frac{256 \sqrt{2} c_\theta^5 C_{19} M_\theta^8 M_\pi^8 s_\theta^5}{27 M_\eta^{10}} - \frac{512 \sqrt{2} c_\theta^5 C_{31} M_\theta^8 M_\pi^8 s_\theta^5}{81 M_\eta^{10}} - \\
& \frac{14090240 \sqrt{2} c_\theta^7 L_8^2 r M_\theta^8 M_K^{10} s_\theta^5}{729 F^2 M_\eta^2 M_\eta^{10}} + \frac{3751936 \sqrt{2} c_\theta^7 L_8^2 r M_\theta^8 M_K^8 M_\pi^2 s_\theta^5}{81 F^2 M_\eta^2 M_\eta^{10}} - \\
& \frac{9469952 \sqrt{2} c_\theta^7 L_8^2 r M_\theta^8 M_K^6 M_\pi^4 s_\theta^5}{243 F^2 M_\eta^2 M_\eta^{10}} + \frac{10514432 \sqrt{2} c_\theta^7 L_8^2 r M_\theta^8 M_K^4 M_\pi^6 s_\theta^5}{729 F^2 M_\eta^2 M_\eta^{10}} - \\
& \frac{686080 \sqrt{2} c_\theta^7 L_8^2 r M_\theta^8 M_K^8 M_\pi^8 s_\theta^5}{243 F^2 M_\eta^2 M_\eta^{10}} + \frac{2560 \sqrt{2} c_\theta^7 L_8^2 r M_\theta^8 M_\pi^{10} s_\theta^5}{27 F^2 M_\eta^2 M_\eta^{10}} - \frac{16 \sqrt{2} \operatorname{Log}\left[\frac{M_\eta^2}{\mu^2}\right] c_\theta^7 M_\theta^8 M_K^4 M_\pi^2 s_\theta^5}{729 \pi^2 M_\eta^{10}} +
\end{aligned}$$

$$\begin{aligned}
& \frac{23 \operatorname{Log}\left[\frac{M_\eta^2}{\mu^2}\right] c_\theta^7 M_\theta^8 M_K^2 M_\pi^2 M_\eta^2 s_\theta^5}{1458 \sqrt{2} \pi^2 M_\eta^{10}} + \frac{\sqrt{2} \operatorname{Log}\left[\frac{M_\eta^2}{\mu^2}\right] c_\theta^7 M_\theta^8 M_K^2 M_\pi^2 M_\eta^2 s_\theta^5}{243 \pi^2 M_\eta^{10}} - \frac{35 \operatorname{Log}\left[\frac{M_\eta^2}{\mu^2}\right] c_\theta^7 M_\theta^8 M_\pi^4 M_\eta^2 s_\theta^5}{5832 \sqrt{2} \pi^2 M_\eta^{10}} + \\
& \frac{\sqrt{2} \operatorname{Log}\left[\frac{M_\eta^2}{\mu^2}\right] c_\theta^7 M_\theta^8 M_\pi^4 M_\eta^2 s_\theta^5}{729 \pi^2 M_\eta^{10}} - \frac{61 c_\theta^7 M_\theta^8 M_K^4 s_\theta^5}{243 \sqrt{2} \pi^2 M_\eta^8} - \frac{5 \operatorname{Log}\left[\frac{M_\eta^2}{\mu^2}\right] c_\theta^7 M_\theta^8 M_K^4 s_\theta^5}{243 \sqrt{2} \pi^2 M_\eta^8} + \\
& \frac{20 \sqrt{2} \operatorname{Log}\left[\frac{M_\eta^2}{\mu^2}\right] c_\theta^7 M_\theta^8 M_K^4 s_\theta^5}{243 \pi^2 M_\eta^8} + \frac{28 \sqrt{2} \operatorname{Log}\left[\frac{M_\eta^2}{\mu^2}\right] c_\theta^7 M_\theta^8 M_K^4 s_\theta^5}{729 \pi^2 M_\eta^8} + \frac{28 \sqrt{2} c_\theta^7 M_\theta^8 M_K^2 M_\pi^2 s_\theta^5}{243 \pi^2 M_\eta^8} + \\
& \frac{\operatorname{Log}\left[\frac{M_\eta^2}{\mu^2}\right] c_\theta^7 M_\theta^8 M_K^2 M_\pi^2 s_\theta^5}{1458 \sqrt{2} \pi^2 M_\eta^8} - \frac{13 \sqrt{2} \operatorname{Log}\left[\frac{M_\eta^2}{\mu^2}\right] c_\theta^7 M_\theta^8 M_K^2 M_\pi^2 s_\theta^5}{729 \pi^2 M_\eta^8} - \frac{5 \operatorname{Log}\left[\frac{M_\eta^2}{\mu^2}\right] c_\theta^7 M_\theta^8 M_K^2 M_\pi^2 s_\theta^5}{486 \sqrt{2} \pi^2 M_\eta^8} - \\
& \frac{23 \sqrt{2} \operatorname{Log}\left[\frac{M_\eta^2}{\mu^2}\right] c_\theta^7 M_\theta^8 M_K^2 M_\pi^2 s_\theta^5}{729 \pi^2 M_\eta^8} - \frac{181 c_\theta^7 M_\theta^8 M_\pi^4 s_\theta^5}{3888 \sqrt{2} \pi^2 M_\eta^8} - \frac{5 \operatorname{Log}\left[\frac{M_\eta^2}{\mu^2}\right] c_\theta^7 M_\theta^8 M_\pi^4 s_\theta^5}{3888 \sqrt{2} \pi^2 M_\eta^8} - \\
& \frac{\sqrt{2} \operatorname{Log}\left[\frac{M_\eta^2}{\mu^2}\right] c_\theta^7 M_\theta^8 M_\pi^4 s_\theta^5}{243 \pi^2 M_\eta^8} - \frac{11 \operatorname{Log}\left[\frac{M_\eta^2}{\mu^2}\right] c_\theta^7 M_\theta^8 M_\pi^4 s_\theta^5}{243 \sqrt{2} \pi^2 M_\eta^8} + \frac{22 \sqrt{2} \operatorname{Log}\left[\frac{M_\eta^2}{\mu^2}\right] c_\theta^7 M_\theta^8 M_\pi^4 s_\theta^5}{729 \pi^2 M_\eta^8} + \\
& \frac{15400960 \sqrt{2} c_\theta^7 L_8^2 r M_\theta^8 M_K^{10} s_\theta^5}{729 F^2 M_\eta^4 M_\eta^8} - \frac{11542528 \sqrt{2} c_\theta^7 L_8^2 r M_\theta^8 M_K^8 M_\pi^2 s_\theta^5}{243 F^2 M_\eta^4 M_\eta^8} + \\
& \frac{2523136 \sqrt{2} c_\theta^7 L_8^2 r M_\theta^8 M_K^6 M_\pi^4 s_\theta^5}{81 F^2 M_\eta^4 M_\eta^8} - \frac{3450880 \sqrt{2} c_\theta^7 L_8^2 r M_\theta^8 M_K^4 M_\pi^6 s_\theta^5}{729 F^2 M_\eta^4 M_\eta^8} - \\
& \frac{28672 \sqrt{2} c_\theta^7 L_8^2 r M_\theta^8 M_K^2 M_\pi^8 s_\theta^5}{243 F^2 M_\eta^4 M_\eta^8} + \frac{512 \sqrt{2} c_\theta^7 L_8^2 r M_\theta^8 M_\pi^{10} s_\theta^5}{27 F^2 M_\eta^4 M_\eta^8} - \frac{256 \sqrt{2} F^2 v_2^{(2)} c_\theta^5 M_\theta^8 M_K^4 s_\theta^5}{27 M_\eta^2 M_\eta^8} + \\
& \frac{\sqrt{2} \operatorname{Log}\left[\frac{M_K^2}{\mu^2}\right] c_\theta^5 M_\theta^8 M_K^6 s_\theta^5}{9 \pi^2 M_\eta^2 M_\eta^8} + \frac{256 \sqrt{2} c_\theta^5 L_{25}^r M_\theta^8 M_K^6 s_\theta^5}{3 M_\eta^2 M_\eta^8} + \frac{32 \sqrt{2} F^2 v_2^{(2)} c_\theta^5 M_\theta^8 M_K^2 M_\pi^2 s_\theta^5}{27 M_\eta^2 M_\eta^8} - \\
& \frac{\operatorname{Log}\left[\frac{M_K^2}{\mu^2}\right] c_\theta^5 M_\theta^8 M_K^4 M_\pi^2 s_\theta^5}{27 \sqrt{2} \pi^2 M_\eta^2 M_\eta^8} - \frac{2 \sqrt{2} \operatorname{Log}\left[\frac{M_K^2}{\mu^2}\right] c_\theta^5 M_\theta^8 M_K^4 M_\pi^2 s_\theta^5}{81 \pi^2 M_\eta^2 M_\eta^8} - \frac{256 \sqrt{2} c_\theta^5 L_6^r M_\theta^8 M_K^4 M_\pi^2 s_\theta^5}{81 M_\eta^2 M_\eta^8} - \\
& \frac{7552 \sqrt{2} c_\theta^5 L_7^r M_\theta^8 M_K^4 M_\pi^2 s_\theta^5}{81 M_\eta^2 M_\eta^8} - \frac{3136 \sqrt{2} c_\theta^5 L_{25}^r M_\theta^8 M_K^4 M_\pi^2 s_\theta^5}{27 M_\eta^2 M_\eta^8} - \frac{1280 \sqrt{2} c_\theta^5 C_{19} M_\theta^8 M_K^6 M_\pi^2 s_\theta^5}{27 M_\eta^2 M_\eta^8} - \\
& \frac{2560 \sqrt{2} c_\theta^5 C_{31} M_\theta^8 M_K^6 M_\pi^2 s_\theta^5}{81 M_\eta^2 M_\eta^8} + \frac{80 \sqrt{2} F^2 v_2^{(2)} c_\theta^5 M_\theta^8 M_\pi^4 s_\theta^5}{27 M_\eta^2 M_\eta^8} - \frac{\operatorname{Log}\left[\frac{M_K^2}{\mu^2}\right] c_\theta^5 M_\theta^8 M_K^2 M_\pi^4 s_\theta^5}{54 \sqrt{2} \pi^2 M_\eta^2 M_\eta^8} - \\
& \frac{\operatorname{Log}\left[\frac{M_\pi^2}{\mu^2}\right] c_\theta^5 M_\theta^8 M_K^2 M_\pi^4 s_\theta^5}{36 \sqrt{2} \pi^2 M_\eta^2 M_\eta^8} + \frac{704 \sqrt{2} c_\theta^5 L_6^r M_\theta^8 M_K^2 M_\pi^4 s_\theta^5}{81 M_\eta^2 M_\eta^8} + \frac{7616 \sqrt{2} c_\theta^5 L_7^r M_\theta^8 M_K^2 M_\pi^4 s_\theta^5}{81 M_\eta^2 M_\eta^8} + \\
& \frac{1856 \sqrt{2} c_\theta^5 L_{25}^r M_\theta^8 M_K^2 M_\pi^4 s_\theta^5}{27 M_\eta^2 M_\eta^8} + \frac{640 \sqrt{2} c_\theta^5 C_{19} M_\theta^8 M_K^4 M_\pi^4 s_\theta^5}{9 M_\eta^2 M_\eta^8} + \frac{1280 \sqrt{2} c_\theta^5 C_{31} M_\theta^8 M_K^4 M_\pi^4 s_\theta^5}{27 M_\eta^2 M_\eta^8} -
\end{aligned}$$

$$\begin{aligned}
& \frac{\text{Log}\left[\frac{M_\pi^2}{\mu^2}\right] c_\theta^5 M_0^8 M_\pi^6 s_\theta^5}{27 \sqrt{2} \pi^2 M_\eta^2 M_{\eta'}^8} + \frac{416 \sqrt{2} c_\theta^5 L_6^r M_0^8 M_\pi^6 s_\theta^5}{81 M_\eta^2 M_{\eta'}^8} - \frac{1216 \sqrt{2} c_\theta^5 L_7^r M_0^8 M_\pi^6 s_\theta^5}{81 M_\eta^2 M_{\eta'}^8} - \\
& \frac{640 \sqrt{2} c_\theta^5 L_{25}^r M_0^8 M_\pi^6 s_\theta^5}{27 M_\eta^2 M_{\eta'}^8} - \frac{256 \sqrt{2} c_\theta^5 C_{19} M_0^8 M_K^2 M_\pi^6 s_\theta^5}{9 M_\eta^2 M_{\eta'}^8} - \frac{512 \sqrt{2} c_\theta^5 C_{31} M_0^8 M_K^2 M_\pi^6 s_\theta^5}{27 M_\eta^2 M_{\eta'}^8} + \\
& \frac{416 \sqrt{2} c_\theta^5 C_{19} M_0^8 M_\pi^8 s_\theta^5}{27 M_\eta^2 M_{\eta'}^8} + \frac{832 \sqrt{2} c_\theta^5 C_{31} M_0^8 M_\pi^8 s_\theta^5}{81 M_\eta^2 M_{\eta'}^8} + \frac{\text{Log}\left[\frac{M_\eta^2}{\mu^2}\right] c_\theta^5 M_0^8 M_\pi^2 M_\eta^2 s_\theta^5}{2592 \sqrt{2} \pi^2 M_{\eta'}^8} + \\
& \frac{\text{Log}\left[\frac{M_\eta^2}{\mu^2}\right] c_\theta^5 M_0^8 M_K^2 s_\theta^5}{162 \sqrt{2} \pi^2 M_{\eta'}^6} - \frac{\text{Log}\left[\frac{M_\eta^2}{\mu^2}\right] c_\theta^5 M_0^8 M_K^2 s_\theta^5}{81 \sqrt{2} \pi^2 M_{\eta'}^6} - \frac{5 \text{Log}\left[\frac{M_\eta^2}{\mu^2}\right] c_\theta^5 M_0^8 M_\pi^2 s_\theta^5}{1296 \sqrt{2} \pi^2 M_{\eta'}^6} + \frac{17 \text{Log}\left[\frac{M_\eta^2}{\mu^2}\right] c_\theta^5 M_0^8 M_\pi^2 s_\theta^5}{2592 \sqrt{2} \pi^2 M_{\eta'}^6} - \\
& \frac{16\,056\,320 \sqrt{2} c_\theta^7 L_8^2 r M_0^8 M_K^{10} s_\theta^5}{729 F^2 M_\eta^6 M_{\eta'}^6} + \frac{11\,886\,592 \sqrt{2} c_\theta^7 L_8^2 r M_0^8 M_K^8 M_\pi^2 s_\theta^5}{243 F^2 M_\eta^6 M_{\eta'}^6} - \\
& \frac{7\,389\,184 \sqrt{2} c_\theta^7 L_8^2 r M_0^8 M_K^6 M_\pi^4 s_\theta^5}{243 F^2 M_\eta^6 M_{\eta'}^6} + \frac{2\,097\,152 \sqrt{2} c_\theta^7 L_8^2 r M_0^8 M_K^4 M_\pi^6 s_\theta^5}{729 F^2 M_\eta^6 M_{\eta'}^6} + \\
& \frac{174\,080 \sqrt{2} c_\theta^7 L_8^2 r M_0^8 M_K^2 M_\pi^8 s_\theta^5}{243 F^2 M_\eta^6 M_{\eta'}^6} + \frac{128 \sqrt{2} F^2 v_2^{(2)} c_\theta^5 M_0^8 M_K^4 s_\theta^5}{9 M_\eta^4 M_{\eta'}^6} - \frac{53 \sqrt{2} \text{Log}\left[\frac{M_K^2}{\mu^2}\right] c_\theta^5 M_0^8 M_K^6 s_\theta^5}{243 \pi^2 M_\eta^4 M_{\eta'}^6} + \\
& \frac{1024 \sqrt{2} c_\theta^5 L_6^r M_0^8 M_K^6 s_\theta^5}{27 M_\eta^4 M_{\eta'}^6} + \frac{1024 \sqrt{2} c_\theta^5 L_7^r M_0^8 M_K^6 s_\theta^5}{27 M_\eta^4 M_{\eta'}^6} - \frac{13\,568 \sqrt{2} c_\theta^5 L_{25}^r M_0^8 M_K^6 s_\theta^5}{81 M_\eta^4 M_{\eta'}^6} + \\
& \frac{2048 \sqrt{2} c_\theta^5 C_{19} M_0^8 M_K^8 s_\theta^5}{9 M_\eta^4 M_{\eta'}^6} + \frac{4096 \sqrt{2} c_\theta^5 C_{31} M_0^8 M_K^8 s_\theta^5}{27 M_\eta^4 M_{\eta'}^6} + \frac{32 \sqrt{2} F^2 v_2^{(2)} c_\theta^5 M_0^8 M_K^2 M_\pi^2 s_\theta^5}{9 M_\eta^4 M_{\eta'}^6} + \\
& \frac{7 \text{Log}\left[\frac{M_K^2}{\mu^2}\right] c_\theta^5 M_0^8 M_K^4 M_\pi^2 s_\theta^5}{162 \sqrt{2} \pi^2 M_\eta^4 M_{\eta'}^6} + \frac{16 \sqrt{2} \text{Log}\left[\frac{M_K^2}{\mu^2}\right] c_\theta^5 M_0^8 M_K^4 M_\pi^2 s_\theta^5}{243 \pi^2 M_\eta^4 M_{\eta'}^6} - \frac{640 \sqrt{2} c_\theta^5 L_6^r M_0^8 M_K^4 M_\pi^2 s_\theta^5}{27 M_\eta^4 M_{\eta'}^6} + \\
& \frac{256 \sqrt{2} c_\theta^5 L_7^r M_0^8 M_K^4 M_\pi^2 s_\theta^5}{3 M_\eta^4 M_{\eta'}^6} + \frac{16\,768 \sqrt{2} c_\theta^5 L_{25}^r M_0^8 M_K^4 M_\pi^2 s_\theta^5}{81 M_\eta^4 M_{\eta'}^6} - \frac{10\,240 \sqrt{2} c_\theta^5 C_{19} M_0^8 M_K^6 M_\pi^2 s_\theta^5}{27 M_\eta^4 M_{\eta'}^6} - \\
& \frac{20\,480 \sqrt{2} c_\theta^5 C_{31} M_0^8 M_K^6 M_\pi^2 s_\theta^5}{81 M_\eta^4 M_{\eta'}^6} - \frac{16 \sqrt{2} F^2 v_2^{(2)} c_\theta^5 M_0^8 M_K^4 s_\theta^5}{9 M_\eta^4 M_{\eta'}^6} - \frac{13 \text{Log}\left[\frac{M_K^2}{\mu^2}\right] c_\theta^5 M_0^8 M_K^2 M_\pi^4 s_\theta^5}{972 \sqrt{2} \pi^2 M_\eta^4 M_{\eta'}^6} + \\
& \frac{\text{Log}\left[\frac{M_\pi^2}{\mu^2}\right] c_\theta^5 M_0^8 M_K^2 M_\pi^4 s_\theta^5}{36 \sqrt{2} \pi^2 M_\eta^4 M_{\eta'}^6} + \frac{\sqrt{2} \text{Log}\left[\frac{M_\pi^2}{\mu^2}\right] c_\theta^5 M_0^8 M_K^2 M_\pi^4 s_\theta^5}{27 \pi^2 M_\eta^4 M_{\eta'}^6} - \frac{128 \sqrt{2} c_\theta^5 L_6^r M_0^8 M_K^2 M_\pi^4 s_\theta^5}{9 M_\eta^4 M_{\eta'}^6} - \\
& \frac{896 \sqrt{2} c_\theta^5 L_7^r M_0^8 M_K^2 M_\pi^4 s_\theta^5}{9 M_\eta^4 M_{\eta'}^6} - \frac{7808 \sqrt{2} c_\theta^5 L_{25}^r M_0^8 M_K^2 M_\pi^4 s_\theta^5}{81 M_\eta^4 M_{\eta'}^6} + \frac{2048 \sqrt{2} c_\theta^5 C_{19} M_0^8 M_K^4 M_\pi^4 s_\theta^5}{9 M_\eta^4 M_{\eta'}^6} + \\
& \frac{4096 \sqrt{2} c_\theta^5 C_{31} M_0^8 M_K^4 M_\pi^4 s_\theta^5}{27 M_\eta^4 M_{\eta'}^6} - \frac{5 \text{Log}\left[\frac{M_\pi^2}{\mu^2}\right] c_\theta^5 M_0^8 M_\pi^6 s_\theta^5}{216 \sqrt{2} \pi^2 M_\eta^4 M_{\eta'}^6} + \frac{32 \sqrt{2} c_\theta^5 L_6^r M_0^8 M_\pi^6 s_\theta^5}{9 M_\eta^4 M_{\eta'}^6} +
\end{aligned}$$

$$\begin{aligned}
& \frac{512 \sqrt{2} c_{\theta}^5 L_7^r M_0^8 M_{\pi}^6 s_{\theta}^5}{27 M_{\eta}^4 M_{\eta'}^6} + \frac{128 \sqrt{2} c_{\theta}^5 L_{25}^r M_0^8 M_{\pi}^6 s_{\theta}^5}{9 M_{\eta}^4 M_{\eta'}^6} - \frac{2240 \sqrt{2} c_{\theta}^5 C_{19} M_0^8 M_K^2 M_{\pi}^6 s_{\theta}^5}{27 M_{\eta}^4 M_{\eta'}^6} - \\
& \frac{4480 \sqrt{2} c_{\theta}^5 C_{31} M_0^8 M_K^2 M_{\pi}^6 s_{\theta}^5}{81 M_{\eta}^4 M_{\eta'}^6} + \frac{32 \sqrt{2} c_{\theta}^5 C_{19} M_0^8 M_{\pi}^8 s_{\theta}^5}{3 M_{\eta}^4 M_{\eta'}^6} + \frac{64 \sqrt{2} c_{\theta}^5 C_{31} M_0^8 M_{\pi}^8 s_{\theta}^5}{9 M_{\eta}^4 M_{\eta'}^6} + \\
& \frac{128 \sqrt{2} F^2 v_2^{(2)} c_{\theta}^3 M_0^6 M_K^4 s_{\theta}^5}{27 M_{\eta}^2 M_{\eta'}^6} + \frac{11 \text{Log}\left[\frac{M_K^2}{\mu^2}\right] c_{\theta}^3 M_0^8 M_K^4 s_{\theta}^5}{1620 \sqrt{2} \pi^2 M_{\eta}^2 M_{\eta'}^6} + \frac{95 c_{\theta}^7 M_0^8 M_K^4 s_{\theta}^5}{243 \sqrt{2} \pi^2 M_{\eta}^2 M_{\eta'}^6} + \\
& \frac{25 \text{Log}\left[\frac{M_{\eta}^2}{\mu^2}\right] c_{\theta}^7 M_0^8 M_K^4 s_{\theta}^5}{243 \sqrt{2} \pi^2 M_{\eta}^2 M_{\eta'}^6} - \frac{110 \sqrt{2} \text{Log}\left[\frac{M_{\eta}^2}{\mu^2}\right] c_{\theta}^7 M_0^8 M_K^4 s_{\theta}^5}{729 \pi^2 M_{\eta}^2 M_{\eta'}^6} - \frac{17 \sqrt{2} \text{Log}\left[\frac{M_{\eta'}^2}{\mu^2}\right] c_{\theta}^7 M_0^8 M_K^4 s_{\theta}^5}{243 \pi^2 M_{\eta}^2 M_{\eta'}^6} + \\
& \frac{1024 \sqrt{2} c_{\theta}^3 L_6^r M_0^8 M_K^4 s_{\theta}^5}{81 M_{\eta}^2 M_{\eta'}^6} + \frac{1024 \sqrt{2} c_{\theta}^3 L_7^r M_0^8 M_K^4 s_{\theta}^5}{81 M_{\eta}^2 M_{\eta'}^6} + \frac{3584 \sqrt{2} c_{\theta}^3 C_{19} M_0^8 M_K^6 s_{\theta}^5}{27 M_{\eta}^2 M_{\eta'}^6} + \\
& \frac{10240 \sqrt{2} c_{\theta}^3 C_{31} M_0^8 M_K^6 s_{\theta}^5}{81 M_{\eta}^2 M_{\eta'}^6} - \frac{16 \sqrt{2} F^2 v_2^{(2)} c_{\theta}^3 M_0^6 M_K^2 M_{\pi}^2 s_{\theta}^5}{27 M_{\eta}^2 M_{\eta'}^6} + \frac{c_{\theta}^3 M_0^8 M_K^2 M_{\pi}^2 s_{\theta}^5}{216 \sqrt{2} \pi^2 M_{\eta}^2 M_{\eta'}^6} + \\
& \frac{\text{Log}\left[\frac{M_K^2}{\mu^2}\right] c_{\theta}^3 M_0^8 M_K^2 M_{\pi}^2 s_{\theta}^5}{1080 \sqrt{2} \pi^2 M_{\eta}^2 M_{\eta'}^6} - \frac{35 \sqrt{2} c_{\theta}^7 M_0^8 M_K^2 M_{\pi}^2 s_{\theta}^5}{243 \pi^2 M_{\eta}^2 M_{\eta'}^6} - \frac{25 \text{Log}\left[\frac{M_{\eta}^2}{\mu^2}\right] c_{\theta}^7 M_0^8 M_K^2 M_{\pi}^2 s_{\theta}^5}{486 \sqrt{2} \pi^2 M_{\eta}^2 M_{\eta'}^6} + \\
& \frac{37 \sqrt{2} \text{Log}\left[\frac{M_{\eta}^2}{\mu^2}\right] c_{\theta}^7 M_0^8 M_K^2 M_{\pi}^2 s_{\theta}^5}{729 \pi^2 M_{\eta}^2 M_{\eta'}^6} + \frac{25 \text{Log}\left[\frac{M_{\eta'}^2}{\mu^2}\right] c_{\theta}^7 M_0^8 M_K^2 M_{\pi}^2 s_{\theta}^5}{486 \sqrt{2} \pi^2 M_{\eta}^2 M_{\eta'}^6} + \frac{7 \sqrt{2} \text{Log}\left[\frac{M_{\eta'}^2}{\mu^2}\right] c_{\theta}^7 M_0^8 M_K^2 M_{\pi}^2 s_{\theta}^5}{243 \pi^2 M_{\eta}^2 M_{\eta'}^6} - \\
& \frac{992 \sqrt{2} c_{\theta}^3 L_6^r M_0^8 M_K^2 M_{\pi}^2 s_{\theta}^5}{81 M_{\eta}^2 M_{\eta'}^6} - \frac{992 \sqrt{2} c_{\theta}^3 L_7^r M_0^8 M_K^2 M_{\pi}^2 s_{\theta}^5}{81 M_{\eta}^2 M_{\eta'}^6} - \frac{1792 \sqrt{2} c_{\theta}^3 C_{19} M_0^8 M_K^4 M_{\pi}^2 s_{\theta}^5}{9 M_{\eta}^2 M_{\eta'}^6} - \\
& \frac{5120 \sqrt{2} c_{\theta}^3 C_{31} M_0^8 M_K^4 M_{\pi}^2 s_{\theta}^5}{27 M_{\eta}^2 M_{\eta'}^6} - \frac{40 \sqrt{2} F^2 v_2^{(2)} c_{\theta}^3 M_0^6 M_{\pi}^4 s_{\theta}^5}{27 M_{\eta}^2 M_{\eta'}^6} + \frac{c_{\theta}^3 M_0^8 M_{\pi}^4 s_{\theta}^5}{216 \sqrt{2} \pi^2 M_{\eta}^2 M_{\eta'}^6} - \\
& \frac{\text{Log}\left[\frac{M_K^2}{\mu^2}\right] c_{\theta}^3 M_0^8 M_{\pi}^4 s_{\theta}^5}{432 \sqrt{2} \pi^2 M_{\eta}^2 M_{\eta'}^6} + \frac{\text{Log}\left[\frac{M_{\pi}^2}{\mu^2}\right] c_{\theta}^3 M_0^8 M_{\pi}^4 s_{\theta}^5}{108 \sqrt{2} \pi^2 M_{\eta}^2 M_{\eta'}^6} + \frac{275 c_{\theta}^7 M_0^8 M_{\pi}^4 s_{\theta}^5}{3888 \sqrt{2} \pi^2 M_{\eta}^2 M_{\eta'}^6} + \frac{5 \text{Log}\left[\frac{M_{\eta}^2}{\mu^2}\right] c_{\theta}^7 M_0^8 M_{\pi}^4 s_{\theta}^5}{3888 \sqrt{2} \pi^2 M_{\eta}^2 M_{\eta'}^6} + \\
& \frac{4 \sqrt{2} \text{Log}\left[\frac{M_{\eta}^2}{\mu^2}\right] c_{\theta}^7 M_0^8 M_{\pi}^4 s_{\theta}^5}{729 \pi^2 M_{\eta}^2 M_{\eta'}^6} + \frac{13 \text{Log}\left[\frac{M_{\eta'}^2}{\mu^2}\right] c_{\theta}^7 M_0^8 M_{\pi}^4 s_{\theta}^5}{972 \sqrt{2} \pi^2 M_{\eta}^2 M_{\eta'}^6} - \frac{5 \sqrt{2} \text{Log}\left[\frac{M_{\eta'}^2}{\mu^2}\right] c_{\theta}^7 M_0^8 M_{\pi}^4 s_{\theta}^5}{243 \pi^2 M_{\eta}^2 M_{\eta'}^6} + \\
& \frac{112 \sqrt{2} c_{\theta}^3 L_6^r M_0^8 M_{\pi}^4 s_{\theta}^5}{81 M_{\eta}^2 M_{\eta'}^6} + \frac{112 \sqrt{2} c_{\theta}^3 L_7^r M_0^8 M_{\pi}^4 s_{\theta}^5}{81 M_{\eta}^2 M_{\eta'}^6} + \frac{896 \sqrt{2} c_{\theta}^3 C_{19} M_0^8 M_K^2 M_{\pi}^4 s_{\theta}^5}{9 M_{\eta}^2 M_{\eta'}^6} + \\
& \frac{2560 \sqrt{2} c_{\theta}^3 C_{31} M_0^8 M_K^2 M_{\pi}^4 s_{\theta}^5}{27 M_{\eta}^2 M_{\eta'}^6} - \frac{560 \sqrt{2} c_{\theta}^3 C_{19} M_0^8 M_{\pi}^6 s_{\theta}^5}{27 M_{\eta}^2 M_{\eta'}^6} - \frac{1600 \sqrt{2} c_{\theta}^3 C_{31} M_0^8 M_{\pi}^6 s_{\theta}^5}{81 M_{\eta}^2 M_{\eta'}^6} + \\
& \frac{13434880 \sqrt{2} c_{\theta}^7 L_8^r M_0^8 M_K^{10} s_{\theta}^5}{729 F^2 M_{\eta}^8 M_{\eta'}^4} - \frac{3457024 \sqrt{2} c_{\theta}^7 L_8^r M_0^8 M_K^8 M_{\pi}^2 s_{\theta}^5}{81 F^2 M_{\eta}^8 M_{\eta'}^4} +
\end{aligned}$$

$$\begin{aligned}
& \frac{7\,585\,792\,\sqrt{2}\,c_\theta^7 L_8^2 r M_\theta^8 M_K^4 M_\pi^4 s_\theta^5}{243 F^2 M_\eta^8 M_{\eta'}^4} - \frac{5\,343\,232\,\sqrt{2}\,c_\theta^7 L_8^2 r M_\theta^8 M_K^4 M_\pi^6 s_\theta^5}{729 F^2 M_\eta^8 M_{\eta'}^4} + \\
& \frac{106\,496\,\sqrt{2}\,c_\theta^7 L_8^2 r M_\theta^8 M_K^2 M_\pi^8 s_\theta^5}{243 F^2 M_\eta^8 M_{\eta'}^4} + \frac{1024\,\sqrt{2}\,c_\theta^7 L_8^2 r M_\theta^8 M_\pi^{10} s_\theta^5}{27 F^2 M_\eta^8 M_{\eta'}^4} - \frac{128\,\sqrt{2}\,F^2 v_2^{(2)} c_\theta^5 M_\theta^8 M_K^4 s_\theta^5}{9 M_\eta^6 M_{\eta'}^4} + \\
& \frac{53\,\sqrt{2}\,\text{Log}\left[\frac{M_K^2}{\mu^2}\right] c_\theta^5 M_\theta^8 M_K^6 s_\theta^5}{243 \pi^2 M_\eta^6 M_{\eta'}^4} - \frac{1024\,\sqrt{2}\,c_\theta^5 L_6^r M_\theta^8 M_K^6 s_\theta^5}{27 M_\eta^6 M_{\eta'}^4} - \frac{1024\,\sqrt{2}\,c_\theta^5 L_7^r M_\theta^8 M_K^6 s_\theta^5}{27 M_\eta^6 M_{\eta'}^4} + \\
& \frac{13\,568\,\sqrt{2}\,c_\theta^5 L_{25}^r M_\theta^8 M_K^6 s_\theta^5}{81 M_\eta^6 M_{\eta'}^4} - \frac{2048\,\sqrt{2}\,c_\theta^5 C_{19} M_\theta^8 M_K^8 s_\theta^5}{9 M_\eta^6 M_{\eta'}^4} - \frac{4096\,\sqrt{2}\,c_\theta^5 C_{31} M_\theta^8 M_K^8 s_\theta^5}{27 M_\eta^6 M_{\eta'}^4} - \\
& \frac{32\,\sqrt{2}\,F^2 v_2^{(2)} c_\theta^5 M_\theta^8 M_K^2 M_\pi^2 s_\theta^5}{9 M_\eta^6 M_{\eta'}^4} + \frac{5\,\text{Log}\left[\frac{M_K^2}{\mu^2}\right] c_\theta^5 M_\theta^8 M_K^4 M_\pi^2 s_\theta^5}{162\,\sqrt{2}\,\pi^2 M_\eta^6 M_{\eta'}^4} - \frac{25\,\sqrt{2}\,\text{Log}\left[\frac{M_K^2}{\mu^2}\right] c_\theta^5 M_\theta^8 M_K^4 M_\pi^2 s_\theta^5}{243 \pi^2 M_\eta^6 M_{\eta'}^4} + \\
& \frac{640\,\sqrt{2}\,c_\theta^5 L_6^r M_\theta^8 M_K^4 M_\pi^2 s_\theta^5}{27 M_\eta^6 M_{\eta'}^4} - \frac{256\,\sqrt{2}\,c_\theta^5 L_7^r M_\theta^8 M_K^4 M_\pi^2 s_\theta^5}{3 M_\eta^6 M_{\eta'}^4} - \frac{16\,768\,\sqrt{2}\,c_\theta^5 L_{25}^r M_\theta^8 M_K^4 M_\pi^2 s_\theta^5}{81 M_\eta^6 M_{\eta'}^4} + \\
& \frac{10\,240\,\sqrt{2}\,c_\theta^5 C_{19} M_\theta^8 M_K^6 M_\pi^2 s_\theta^5}{27 M_\eta^6 M_{\eta'}^4} + \frac{20\,480\,\sqrt{2}\,c_\theta^5 C_{31} M_\theta^8 M_K^6 M_\pi^2 s_\theta^5}{81 M_\eta^6 M_{\eta'}^4} + \frac{16\,\sqrt{2}\,F^2 v_2^{(2)} c_\theta^5 M_\theta^8 M_\pi^4 s_\theta^5}{9 M_\eta^6 M_{\eta'}^4} + \\
& \frac{5\,\text{Log}\left[\frac{M_K^2}{\mu^2}\right] c_\theta^5 M_\theta^8 M_K^2 M_\pi^4 s_\theta^5}{972\,\sqrt{2}\,\pi^2 M_\eta^6 M_{\eta'}^4} + \frac{\sqrt{2}\,\text{Log}\left[\frac{M_K^2}{\mu^2}\right] c_\theta^5 M_\theta^8 M_K^2 M_\pi^4 s_\theta^5}{243 \pi^2 M_\eta^6 M_{\eta'}^4} + \frac{5\,\text{Log}\left[\frac{M_\pi^2}{\mu^2}\right] c_\theta^5 M_\theta^8 M_K^2 M_\pi^4 s_\theta^5}{108\,\sqrt{2}\,\pi^2 M_\eta^6 M_{\eta'}^4} - \\
& \frac{2\,\sqrt{2}\,\text{Log}\left[\frac{M_\pi^2}{\mu^2}\right] c_\theta^5 M_\theta^8 M_K^2 M_\pi^4 s_\theta^5}{27 \pi^2 M_\eta^6 M_{\eta'}^4} + \frac{128\,\sqrt{2}\,c_\theta^5 L_6^r M_\theta^8 M_K^2 M_\pi^4 s_\theta^5}{9 M_\eta^6 M_{\eta'}^4} + \frac{896\,\sqrt{2}\,c_\theta^5 L_7^r M_\theta^8 M_K^2 M_\pi^4 s_\theta^5}{9 M_\eta^6 M_{\eta'}^4} + \\
& \frac{7808\,\sqrt{2}\,c_\theta^5 L_{25}^r M_\theta^8 M_K^2 M_\pi^4 s_\theta^5}{81 M_\eta^6 M_{\eta'}^4} - \frac{2048\,\sqrt{2}\,c_\theta^5 C_{19} M_\theta^8 M_K^4 M_\pi^4 s_\theta^5}{9 M_\eta^6 M_{\eta'}^4} - \frac{4096\,\sqrt{2}\,c_\theta^5 C_{31} M_\theta^8 M_K^4 M_\pi^4 s_\theta^5}{27 M_\eta^6 M_{\eta'}^4} + \\
& \frac{5\,\text{Log}\left[\frac{M_\pi^2}{\mu^2}\right] c_\theta^5 M_\theta^8 M_\pi^6 s_\theta^5}{216\,\sqrt{2}\,\pi^2 M_\eta^6 M_{\eta'}^4} - \frac{32\,\sqrt{2}\,c_\theta^5 L_6^r M_\theta^8 M_\pi^6 s_\theta^5}{9 M_\eta^6 M_{\eta'}^4} - \frac{512\,\sqrt{2}\,c_\theta^5 L_7^r M_\theta^8 M_\pi^6 s_\theta^5}{27 M_\eta^6 M_{\eta'}^4} - \\
& \frac{128\,\sqrt{2}\,c_\theta^5 L_{25}^r M_\theta^8 M_\pi^6 s_\theta^5}{9 M_\eta^6 M_{\eta'}^4} + \frac{2240\,\sqrt{2}\,c_\theta^5 C_{19} M_\theta^8 M_K^2 M_\pi^6 s_\theta^5}{27 M_\eta^6 M_{\eta'}^4} + \frac{4480\,\sqrt{2}\,c_\theta^5 C_{31} M_\theta^8 M_K^2 M_\pi^6 s_\theta^5}{81 M_\eta^6 M_{\eta'}^4} - \\
& \frac{32\,\sqrt{2}\,c_\theta^5 C_{19} M_\theta^8 M_\pi^8 s_\theta^5}{3 M_\eta^6 M_{\eta'}^4} - \frac{64\,\sqrt{2}\,c_\theta^5 C_{31} M_\theta^8 M_\pi^8 s_\theta^5}{9 M_\eta^6 M_{\eta'}^4} + \frac{8\,\sqrt{2}\,F^2 v_2^{(2)} c_\theta^3 M_\theta^8 M_K^2 s_\theta^5}{M_\eta^4 M_{\eta'}^4} - \\
& \frac{64\,\sqrt{2}\,F^2 v_2^{(2)} c_\theta^3 M_\theta^8 M_K^4 s_\theta^5}{9 M_\eta^4 M_{\eta'}^4} - \frac{c_\theta^3 M_\theta^8 M_K^4 s_\theta^5}{18\,\sqrt{2}\,\pi^2 M_\eta^4 M_{\eta'}^4} - \frac{17\,\text{Log}\left[\frac{M_K^2}{\mu^2}\right] c_\theta^3 M_\theta^8 M_K^4 s_\theta^5}{180\,\sqrt{2}\,\pi^2 M_\eta^4 M_{\eta'}^4} - \\
& \frac{29\,c_\theta^7 M_\theta^8 M_K^4 s_\theta^5}{81\,\sqrt{2}\,\pi^2 M_\eta^4 M_{\eta'}^4} + \frac{56\,\sqrt{2}\,\text{Log}\left[\frac{M_\eta^2}{\mu^2}\right] c_\theta^7 M_\theta^8 M_K^4 s_\theta^5}{729 \pi^2 M_\eta^4 M_{\eta'}^4} - \frac{13\,\text{Log}\left[\frac{M_\eta^2}{\mu^2}\right] c_\theta^7 M_\theta^8 M_K^4 s_\theta^5}{81\,\sqrt{2}\,\pi^2 M_\eta^4 M_{\eta'}^4} +
\end{aligned}$$



$$\begin{aligned}
& \frac{128 \sqrt{2} \operatorname{Log}\left[\frac{M_\eta^2}{\mu^2}\right] c_\theta^7 M_\theta^8 M_K^4 s_\theta^5}{729 \pi^2 M_\eta^4 M_{\eta'}^4} - \frac{512 \sqrt{2} c_\theta^3 L_6^r M_\theta^8 M_K^4 s_\theta^5}{27 M_\eta^4 M_{\eta'}^4} - \frac{512 \sqrt{2} c_\theta^3 L_7^r M_\theta^8 M_K^4 s_\theta^5}{27 M_\eta^4 M_{\eta'}^4} - \\
& \frac{1792 \sqrt{2} c_\theta^3 C_{19} M_\theta^8 M_K^6 s_\theta^5}{9 M_\eta^4 M_{\eta'}^4} - \frac{5120 \sqrt{2} c_\theta^3 C_{31} M_\theta^8 M_K^6 s_\theta^5}{27 M_\eta^4 M_{\eta'}^4} - \frac{8 \sqrt{2} F^2 v_2^{(2)} c_\theta^3 M_\theta^8 M_\pi^2 s_\theta^5}{M_\eta^4 M_{\eta'}^4} - \\
& \frac{16 \sqrt{2} F^2 v_2^{(2)} c_\theta^3 M_\theta^8 M_K^2 M_\pi^2 s_\theta^5}{9 M_\eta^4 M_{\eta'}^4} + \frac{c_\theta^3 M_\theta^8 M_K^2 M_\pi^2 s_\theta^5}{72 \sqrt{2} \pi^2 M_\eta^4 M_{\eta'}^4} + \frac{37 \operatorname{Log}\left[\frac{M_K^2}{\mu^2}\right] c_\theta^3 M_\theta^8 M_K^2 M_\pi^2 s_\theta^5}{1080 \sqrt{2} \pi^2 M_\eta^4 M_{\eta'}^4} + \\
& \frac{35 c_\theta^7 M_\theta^8 M_K^2 M_\pi^2 s_\theta^5}{162 \sqrt{2} \pi^2 M_\eta^4 M_{\eta'}^4} - \frac{565 \operatorname{Log}\left[\frac{M_\eta^2}{\mu^2}\right] c_\theta^7 M_\theta^8 M_K^2 M_\pi^2 s_\theta^5}{2916 \sqrt{2} \pi^2 M_\eta^4 M_{\eta'}^4} + \frac{40 \sqrt{2} \operatorname{Log}\left[\frac{M_\eta^2}{\mu^2}\right] c_\theta^7 M_\theta^8 M_K^2 M_\pi^2 s_\theta^5}{729 \pi^2 M_\eta^4 M_{\eta'}^4} + \\
& \frac{49 \operatorname{Log}\left[\frac{M_\eta^2}{\mu^2}\right] c_\theta^7 M_\theta^8 M_K^2 M_\pi^2 s_\theta^5}{972 \sqrt{2} \pi^2 M_\eta^4 M_{\eta'}^4} - \frac{52 \sqrt{2} \operatorname{Log}\left[\frac{M_\eta^2}{\mu^2}\right] c_\theta^7 M_\theta^8 M_K^2 M_\pi^2 s_\theta^5}{729 \pi^2 M_\eta^4 M_{\eta'}^4} + \frac{736 \sqrt{2} c_\theta^3 L_6^r M_\theta^8 M_K^2 M_\pi^2 s_\theta^5}{27 M_\eta^4 M_{\eta'}^4} + \\
& \frac{736 \sqrt{2} c_\theta^3 L_7^r M_\theta^8 M_K^2 M_\pi^2 s_\theta^5}{27 M_\eta^4 M_{\eta'}^4} + \frac{896 \sqrt{2} c_\theta^3 C_{19} M_\theta^8 M_K^4 M_\pi^2 s_\theta^5}{3 M_\eta^4 M_{\eta'}^4} + \frac{2560 \sqrt{2} c_\theta^3 C_{31} M_\theta^8 M_K^4 M_\pi^2 s_\theta^5}{9 M_\eta^4 M_{\eta'}^4} + \\
& \frac{8 \sqrt{2} F^2 v_2^{(2)} c_\theta^3 M_\theta^8 M_\pi^4 s_\theta^5}{9 M_\eta^4 M_{\eta'}^4} + \frac{c_\theta^3 M_\theta^8 M_\pi^4 s_\theta^5}{36 \sqrt{2} \pi^2 M_\eta^4 M_{\eta'}^4} + \frac{\operatorname{Log}\left[\frac{M_K^2}{\mu^2}\right] c_\theta^3 M_\theta^8 M_\pi^4 s_\theta^5}{144 \sqrt{2} \pi^2 M_\eta^4 M_{\eta'}^4} + \frac{\operatorname{Log}\left[\frac{M_\pi^2}{\mu^2}\right] c_\theta^3 M_\theta^8 M_\pi^4 s_\theta^5}{36 \sqrt{2} \pi^2 M_\eta^4 M_{\eta'}^4} - \\
& \frac{53 c_\theta^7 M_\theta^8 M_\pi^4 s_\theta^5}{1296 \sqrt{2} \pi^2 M_\eta^4 M_{\eta'}^4} + \frac{805 \operatorname{Log}\left[\frac{M_\eta^2}{\mu^2}\right] c_\theta^7 M_\theta^8 M_\pi^4 s_\theta^5}{11664 \sqrt{2} \pi^2 M_\eta^4 M_{\eta'}^4} - \frac{7 \sqrt{2} \operatorname{Log}\left[\frac{M_\eta^2}{\mu^2}\right] c_\theta^7 M_\theta^8 M_\pi^4 s_\theta^5}{243 \pi^2 M_\eta^4 M_{\eta'}^4} + \\
& \frac{65 \operatorname{Log}\left[\frac{M_\eta^2}{\mu^2}\right] c_\theta^7 M_\theta^8 M_\pi^4 s_\theta^5}{5832 \sqrt{2} \pi^2 M_\eta^4 M_{\eta'}^4} - \frac{368 \sqrt{2} c_\theta^3 L_6^r M_\theta^8 M_\pi^4 s_\theta^5}{27 M_\eta^4 M_{\eta'}^4} - \frac{368 \sqrt{2} c_\theta^3 L_7^r M_\theta^8 M_\pi^4 s_\theta^5}{27 M_\eta^4 M_{\eta'}^4} - \\
& \frac{448 \sqrt{2} c_\theta^3 C_{19} M_\theta^8 M_K^2 M_\pi^4 s_\theta^5}{3 M_\eta^4 M_{\eta'}^4} - \frac{1280 \sqrt{2} c_\theta^3 C_{31} M_\theta^8 M_K^2 M_\pi^4 s_\theta^5}{9 M_\eta^4 M_{\eta'}^4} + \frac{112 \sqrt{2} c_\theta^3 C_{19} M_\theta^8 M_\pi^6 s_\theta^5}{9 M_\eta^4 M_{\eta'}^4} + \\
& \frac{320 \sqrt{2} c_\theta^3 C_{31} M_\theta^8 M_\pi^6 s_\theta^5}{27 M_\eta^4 M_{\eta'}^4} - \frac{\operatorname{Log}\left[\frac{M_\eta^2}{\mu^2}\right] c_\theta^5 M_\theta^8 M_K^2 s_\theta^5}{81 \sqrt{2} \pi^2 M_\eta^2 M_{\eta'}^4} + \frac{5 \operatorname{Log}\left[\frac{M_\eta^2}{\mu^2}\right] c_\theta^5 M_\theta^8 M_\pi^2 s_\theta^5}{648 \sqrt{2} \pi^2 M_\eta^2 M_{\eta'}^4} + \\
& \frac{5 \operatorname{Log}\left[\frac{M_\eta^2}{\mu^2}\right] c_\theta^5 M_\theta^8 M_\pi^2 s_\theta^5}{1296 \sqrt{2} \pi^2 M_\eta^2 M_{\eta'}^4} - \frac{5242880 \sqrt{2} c_\theta^7 L_8^{2r} M_\theta^8 M_K^{10} s_\theta^5}{729 F^2 M_\eta^{10} M_{\eta'}^2} + \frac{4136960 \sqrt{2} c_\theta^7 L_8^{2r} M_\theta^8 M_K^8 M_\pi^2 s_\theta^5}{243 F^2 M_\eta^{10} M_{\eta'}^2} - \\
& \frac{1097728 \sqrt{2} c_\theta^7 L_8^{2r} M_\theta^8 M_K^6 M_\pi^4 s_\theta^5}{81 F^2 M_\eta^{10} M_{\eta'}^2} + \frac{2797568 \sqrt{2} c_\theta^7 L_8^{2r} M_\theta^8 M_K^4 M_\pi^6 s_\theta^5}{729 F^2 M_\eta^{10} M_{\eta'}^2} - \\
& \frac{47104 \sqrt{2} c_\theta^7 L_8^{2r} M_\theta^8 M_K^2 M_\pi^8 s_\theta^5}{243 F^2 M_\eta^{10} M_{\eta'}^2} + \frac{3584 \sqrt{2} c_\theta^7 L_8^{2r} M_\theta^8 M_\pi^{10} s_\theta^5}{27 F^2 M_\eta^{10} M_{\eta'}^2} + \frac{256 \sqrt{2} F^2 v_2^{(2)} c_\theta^5 M_\theta^8 M_K^4 s_\theta^5}{27 M_\eta^8 M_{\eta'}^2} - \\
& \frac{\sqrt{2} \operatorname{Log}\left[\frac{M_K^2}{\mu^2}\right] c_\theta^5 M_\theta^8 M_K^6 s_\theta^5}{9 \pi^2 M_\eta^8 M_{\eta'}^2} - \frac{256 \sqrt{2} c_\theta^5 L_{25}^r M_\theta^8 M_K^6 s_\theta^5}{3 M_\eta^8 M_{\eta'}^2} - \frac{32 \sqrt{2} F^2 v_2^{(2)} c_\theta^5 M_\theta^8 M_K^2 M_\pi^2 s_\theta^5}{27 M_\eta^8 M_{\eta'}^2} +
\end{aligned}$$

$$\begin{aligned}
& \frac{5 \operatorname{Log}\left[\frac{M_K^2}{\mu^2}\right] c_\theta^5 M_0^8 M_K^4 M_\pi^2 s_\theta^5}{81 \sqrt{2} \pi^2 M_\eta^8 M_{\eta'}^2} + \frac{\sqrt{2} \operatorname{Log}\left[\frac{M_K^2}{\mu^2}\right] c_\theta^5 M_0^8 M_K^4 M_\pi^2 s_\theta^5}{81 \pi^2 M_\eta^8 M_{\eta'}^2} + \frac{256 \sqrt{2} c_\theta^5 L_6^r M_0^8 M_K^4 M_\pi^2 s_\theta^5}{81 M_\eta^8 M_{\eta'}^2} + \\
& \frac{7552 \sqrt{2} c_\theta^5 L_7^r M_0^8 M_K^4 M_\pi^2 s_\theta^5}{81 M_\eta^8 M_{\eta'}^2} + \frac{3136 \sqrt{2} c_\theta^5 L_{25}^r M_0^8 M_K^4 M_\pi^2 s_\theta^5}{27 M_\eta^8 M_{\eta'}^2} + \frac{1280 \sqrt{2} c_\theta^5 C_{19} M_0^8 M_K^6 M_\pi^2 s_\theta^5}{27 M_\eta^8 M_{\eta'}^2} + \\
& \frac{2560 \sqrt{2} c_\theta^5 C_{31} M_0^8 M_K^6 M_\pi^2 s_\theta^5}{81 M_\eta^8 M_{\eta'}^2} - \frac{80 \sqrt{2} F^2 v_2^{(2)} c_\theta^5 M_0^8 M_K^4 s_\theta^5}{27 M_\eta^8 M_{\eta'}^2} + \frac{\operatorname{Log}\left[\frac{M_K^2}{\mu^2}\right] c_\theta^5 M_0^8 M_K^2 M_\pi^4 s_\theta^5}{486 \sqrt{2} \pi^2 M_\eta^8 M_{\eta'}^2} + \\
& \frac{2 \sqrt{2} \operatorname{Log}\left[\frac{M_\pi^2}{\mu^2}\right] c_\theta^5 M_0^8 M_K^2 M_\pi^4 s_\theta^5}{243 \pi^2 M_\eta^8 M_{\eta'}^2} + \frac{\operatorname{Log}\left[\frac{M_\pi^2}{\mu^2}\right] c_\theta^5 M_0^8 M_K^2 M_\pi^4 s_\theta^5}{36 \sqrt{2} \pi^2 M_\eta^8 M_{\eta'}^2} - \frac{704 \sqrt{2} c_\theta^5 L_6^r M_0^8 M_K^2 M_\pi^4 s_\theta^5}{81 M_\eta^8 M_{\eta'}^2} - \\
& \frac{7616 \sqrt{2} c_\theta^5 L_7^r M_0^8 M_K^2 M_\pi^4 s_\theta^5}{81 M_\eta^8 M_{\eta'}^2} - \frac{1856 \sqrt{2} c_\theta^5 L_{25}^r M_0^8 M_K^2 M_\pi^4 s_\theta^5}{27 M_\eta^8 M_{\eta'}^2} - \frac{640 \sqrt{2} c_\theta^5 C_{19} M_0^8 M_K^4 M_\pi^4 s_\theta^5}{9 M_\eta^8 M_{\eta'}^2} - \\
& \frac{1280 \sqrt{2} c_\theta^5 C_{31} M_0^8 M_K^4 M_\pi^4 s_\theta^5}{27 M_\eta^8 M_{\eta'}^2} + \frac{\operatorname{Log}\left[\frac{M_\pi^2}{\mu^2}\right] c_\theta^5 M_0^8 M_\pi^6 s_\theta^5}{81 \sqrt{2} \pi^2 M_\eta^8 M_{\eta'}^2} + \frac{\sqrt{2} \operatorname{Log}\left[\frac{M_\pi^2}{\mu^2}\right] c_\theta^5 M_0^8 M_\pi^6 s_\theta^5}{81 \pi^2 M_\eta^8 M_{\eta'}^2} - \\
& \frac{416 \sqrt{2} c_\theta^5 L_6^r M_0^8 M_\pi^6 s_\theta^5}{81 M_\eta^8 M_{\eta'}^2} + \frac{1216 \sqrt{2} c_\theta^5 L_7^r M_0^8 M_\pi^6 s_\theta^5}{81 M_\eta^8 M_{\eta'}^2} + \frac{640 \sqrt{2} c_\theta^5 L_{25}^r M_0^8 M_\pi^6 s_\theta^5}{27 M_\eta^8 M_{\eta'}^2} + \\
& \frac{256 \sqrt{2} c_\theta^5 C_{19} M_0^8 M_K^2 M_\pi^6 s_\theta^5}{9 M_\eta^8 M_{\eta'}^2} + \frac{512 \sqrt{2} c_\theta^5 C_{31} M_0^8 M_K^2 M_\pi^6 s_\theta^5}{27 M_\eta^8 M_{\eta'}^2} - \frac{416 \sqrt{2} c_\theta^5 C_{19} M_0^8 M_\pi^8 s_\theta^5}{27 M_\eta^8 M_{\eta'}^2} - \\
& \frac{832 \sqrt{2} c_\theta^5 C_{31} M_0^8 M_\pi^8 s_\theta^5}{81 M_\eta^8 M_{\eta'}^2} - \frac{8 \sqrt{2} F^2 v_2^{(2)} c_\theta^3 M_0^8 M_K^2 s_\theta^5}{M_\eta^6 M_{\eta'}^2} + \frac{64 \sqrt{2} F^2 v_2^{(2)} c_\theta^3 M_0^6 M_K^4 s_\theta^5}{9 M_\eta^6 M_{\eta'}^2} + \\
& \frac{c_\theta^3 M_0^8 M_K^4 s_\theta^5}{18 \sqrt{2} \pi^2 M_\eta^6 M_{\eta'}^2} + \frac{17 \operatorname{Log}\left[\frac{M_K^2}{\mu^2}\right] c_\theta^3 M_0^8 M_K^4 s_\theta^5}{180 \sqrt{2} \pi^2 M_\eta^6 M_{\eta'}^2} + \frac{41 c_\theta^7 M_0^8 M_K^4 s_\theta^5}{243 \sqrt{2} \pi^2 M_\eta^6 M_{\eta'}^2} - \frac{2 \sqrt{2} \operatorname{Log}\left[\frac{M_\eta^2}{\mu^2}\right] c_\theta^7 M_0^8 M_K^4 s_\theta^5}{81 \pi^2 M_\eta^6 M_{\eta'}^2} + \\
& \frac{13 \operatorname{Log}\left[\frac{M_\eta^2}{\mu^2}\right] c_\theta^7 M_0^8 M_K^4 s_\theta^5}{243 \sqrt{2} \pi^2 M_\eta^6 M_{\eta'}^2} - \frac{86 \sqrt{2} \operatorname{Log}\left[\frac{M_\eta^2}{\mu^2}\right] c_\theta^7 M_0^8 M_K^4 s_\theta^5}{729 \pi^2 M_\eta^6 M_{\eta'}^2} + \frac{512 \sqrt{2} c_\theta^3 L_6^r M_0^8 M_K^4 s_\theta^5}{27 M_\eta^6 M_{\eta'}^2} + \\
& \frac{512 \sqrt{2} c_\theta^3 L_7^r M_0^8 M_K^4 s_\theta^5}{27 M_\eta^6 M_{\eta'}^2} + \frac{1792 \sqrt{2} c_\theta^3 C_{19} M_0^8 M_K^6 s_\theta^5}{9 M_\eta^6 M_{\eta'}^2} + \frac{5120 \sqrt{2} c_\theta^3 C_{31} M_0^8 M_K^6 s_\theta^5}{27 M_\eta^6 M_{\eta'}^2} + \\
& \frac{8 \sqrt{2} F^2 v_2^{(2)} c_\theta^3 M_0^8 M_\pi^2 s_\theta^5}{M_\eta^6 M_{\eta'}^2} + \frac{16 \sqrt{2} F^2 v_2^{(2)} c_\theta^3 M_0^6 M_K^2 M_\pi^2 s_\theta^5}{9 M_\eta^6 M_{\eta'}^2} - \frac{c_\theta^3 M_0^8 M_K^2 M_\pi^2 s_\theta^5}{72 \sqrt{2} \pi^2 M_\eta^6 M_{\eta'}^2} - \\
& \frac{37 \operatorname{Log}\left[\frac{M_K^2}{\mu^2}\right] c_\theta^3 M_0^8 M_K^2 M_\pi^2 s_\theta^5}{1080 \sqrt{2} \pi^2 M_\eta^6 M_{\eta'}^2} - \frac{5 c_\theta^7 M_0^8 M_K^2 M_\pi^2 s_\theta^5}{486 \sqrt{2} \pi^2 M_\eta^6 M_{\eta'}^2} - \frac{4 \sqrt{2} c_\theta^7 M_0^8 M_K^2 M_\pi^2 s_\theta^5}{81 \pi^2 M_\eta^6 M_{\eta'}^2} + \\
& \frac{17 \operatorname{Log}\left[\frac{M_\eta^2}{\mu^2}\right] c_\theta^7 M_0^8 M_K^2 M_\pi^2 s_\theta^5}{972 \sqrt{2} \pi^2 M_\eta^6 M_{\eta'}^2} + \frac{2 \sqrt{2} \operatorname{Log}\left[\frac{M_\eta^2}{\mu^2}\right] c_\theta^7 M_0^8 M_K^2 M_\pi^2 s_\theta^5}{243 \pi^2 M_\eta^6 M_{\eta'}^2} + \frac{205 \operatorname{Log}\left[\frac{M_\eta^2}{\mu^2}\right] c_\theta^7 M_0^8 M_K^2 M_\pi^2 s_\theta^5}{2916 \sqrt{2} \pi^2 M_\eta^6 M_{\eta'}^2} +
\end{aligned}$$

$$\begin{aligned}
& \frac{5 \sqrt{2} \operatorname{Log} \left[ \frac{M_{\eta'}^2}{\mu^2} \right] c_{\theta}^7 M_{\theta}^8 M_K^2 M_{\pi}^2 s_{\theta}^5}{729 \pi^2 M_{\eta}^6 M_{\eta'}^2} - \frac{736 \sqrt{2} c_{\theta}^3 L_6^r M_{\theta}^8 M_K^2 M_{\pi}^2 s_{\theta}^5}{27 M_{\eta}^6 M_{\eta'}^2} - \frac{736 \sqrt{2} c_{\theta}^3 L_7^r M_{\theta}^8 M_K^2 M_{\pi}^2 s_{\theta}^5}{27 M_{\eta}^6 M_{\eta'}^2} - \\
& \frac{896 \sqrt{2} c_{\theta}^3 C_{19} M_{\theta}^8 M_K^4 M_{\pi}^2 s_{\theta}^5}{3 M_{\eta}^6 M_{\eta'}^2} - \frac{2560 \sqrt{2} c_{\theta}^3 C_{31} M_{\theta}^8 M_K^4 M_{\pi}^2 s_{\theta}^5}{9 M_{\eta}^6 M_{\eta'}^2} - \frac{8 \sqrt{2} F^2 v_2^{(2)} c_{\theta}^3 M_{\theta}^6 M_{\pi}^4 s_{\theta}^5}{9 M_{\eta}^6 M_{\eta'}^2} - \\
& \frac{c_{\theta}^3 M_{\theta}^8 M_{\pi}^4 s_{\theta}^5}{36 \sqrt{2} \pi^2 M_{\eta}^6 M_{\eta'}^2} - \frac{\operatorname{Log} \left[ \frac{M_K^2}{\mu^2} \right] c_{\theta}^3 M_{\theta}^8 M_{\pi}^4 s_{\theta}^5}{144 \sqrt{2} \pi^2 M_{\eta}^6 M_{\eta'}^2} - \frac{\operatorname{Log} \left[ \frac{M_{\pi}^2}{\mu^2} \right] c_{\theta}^3 M_{\theta}^8 M_{\pi}^4 s_{\theta}^5}{36 \sqrt{2} \pi^2 M_{\eta}^6 M_{\eta'}^2} - \frac{11 c_{\theta}^7 M_{\theta}^8 M_{\pi}^4 s_{\theta}^5}{432 \sqrt{2} \pi^2 M_{\eta}^6 M_{\eta'}^2} + \\
& \frac{4 \sqrt{2} c_{\theta}^7 M_{\theta}^8 M_{\pi}^4 s_{\theta}^5}{243 \pi^2 M_{\eta}^6 M_{\eta'}^2} - \frac{\operatorname{Log} \left[ \frac{M_{\eta}^2}{\mu^2} \right] c_{\theta}^7 M_{\theta}^8 M_{\pi}^4 s_{\theta}^5}{1296 \sqrt{2} \pi^2 M_{\eta}^6 M_{\eta'}^2} - \frac{47 \operatorname{Log} \left[ \frac{M_{\eta'}^2}{\mu^2} \right] c_{\theta}^7 M_{\theta}^8 M_{\pi}^4 s_{\theta}^5}{5832 \sqrt{2} \pi^2 M_{\eta}^6 M_{\eta'}^2} + \frac{368 \sqrt{2} c_{\theta}^3 L_6^r M_{\theta}^8 M_{\pi}^4 s_{\theta}^5}{27 M_{\eta}^6 M_{\eta'}^2} + \\
& \frac{368 \sqrt{2} c_{\theta}^3 L_7^r M_{\theta}^8 M_{\pi}^4 s_{\theta}^5}{27 M_{\eta}^6 M_{\eta'}^2} + \frac{448 \sqrt{2} c_{\theta}^3 C_{19} M_{\theta}^8 M_K^2 M_{\pi}^4 s_{\theta}^5}{3 M_{\eta}^6 M_{\eta'}^2} + \frac{1280 \sqrt{2} c_{\theta}^3 C_{31} M_{\theta}^8 M_K^2 M_{\pi}^4 s_{\theta}^5}{9 M_{\eta}^6 M_{\eta'}^2} - \\
& \frac{112 \sqrt{2} c_{\theta}^3 C_{19} M_{\theta}^8 M_{\pi}^6 s_{\theta}^5}{9 M_{\eta}^6 M_{\eta'}^2} - \frac{320 \sqrt{2} c_{\theta}^3 C_{31} M_{\theta}^8 M_{\pi}^6 s_{\theta}^5}{27 M_{\eta}^6 M_{\eta'}^2} + \frac{\operatorname{Log} \left[ \frac{M_{\eta'}^2}{\mu^2} \right] c_{\theta}^5 M_{\theta}^8 M_K^2 s_{\theta}^5}{81 \sqrt{2} \pi^2 M_{\eta}^4 M_{\eta'}^2} - \\
& \frac{5 \operatorname{Log} \left[ \frac{M_{\eta}^2}{\mu^2} \right] c_{\theta}^5 M_{\theta}^8 M_{\pi}^2 s_{\theta}^5}{1296 \sqrt{2} \pi^2 M_{\eta}^4 M_{\eta'}^2} - \frac{5 \operatorname{Log} \left[ \frac{M_{\eta'}^2}{\mu^2} \right] c_{\theta}^5 M_{\theta}^8 M_{\pi}^2 s_{\theta}^5}{648 \sqrt{2} \pi^2 M_{\eta}^4 M_{\eta'}^2} - \frac{4 \sqrt{2} \operatorname{Log} \left[ \frac{M_{\eta}^2}{\mu^2} \right] c_{\theta}^7 M_{\theta}^8 M_K^4 M_{\eta'}^2 s_{\theta}^5}{729 \pi^2 M_{\eta}^{10}} - \\
& \frac{7 \operatorname{Log} \left[ \frac{M_{\eta'}^2}{\mu^2} \right] c_{\theta}^7 M_{\theta}^8 M_K^2 M_{\pi}^2 M_{\eta'}^2 s_{\theta}^5}{1458 \sqrt{2} \pi^2 M_{\eta}^{10}} + \frac{2 \sqrt{2} \operatorname{Log} \left[ \frac{M_{\eta'}^2}{\mu^2} \right] c_{\theta}^7 M_{\theta}^8 M_K^2 M_{\pi}^2 M_{\eta'}^2 s_{\theta}^5}{243 \pi^2 M_{\eta}^{10}} - \\
& \frac{13 \operatorname{Log} \left[ \frac{M_{\eta}^2}{\mu^2} \right] c_{\theta}^7 M_{\theta}^8 M_{\pi}^4 M_{\eta'}^2 s_{\theta}^5}{5832 \sqrt{2} \pi^2 M_{\eta}^{10}} - \frac{\operatorname{Log} \left[ \frac{M_{\eta}^2}{\mu^2} \right] c_{\theta}^5 M_{\theta}^8 M_{\pi}^2 M_{\eta'}^2 s_{\theta}^5}{2592 \sqrt{2} \pi^2 M_{\eta}^8} + \frac{2 \sqrt{2} \operatorname{Log} \left[ \frac{M_{\eta}^2}{\mu^2} \right] c_{\theta}^7 M_{\theta}^8 M_K^4 s_{\theta}^5}{243 \pi^2 M_{\eta}^6 (M_{\eta}^2 - M_{\eta'}^2)} + \\
& \frac{16 \sqrt{2} \operatorname{Log} \left[ \frac{M_{\eta'}^2}{\mu^2} \right] c_{\theta}^7 M_{\theta}^8 M_K^4 s_{\theta}^5}{243 \pi^2 M_{\eta}^6 (M_{\eta}^2 - M_{\eta'}^2)} - \frac{\sqrt{2} \operatorname{Log} \left[ \frac{M_{\eta}^2}{\mu^2} \right] c_{\theta}^7 M_{\theta}^8 M_K^2 M_{\pi}^2 s_{\theta}^5}{243 \pi^2 M_{\eta}^6 (M_{\eta}^2 - M_{\eta'}^2)} + \frac{29 \operatorname{Log} \left[ \frac{M_{\eta}^2}{\mu^2} \right] c_{\theta}^7 M_{\theta}^8 M_K^2 M_{\pi}^2 s_{\theta}^5}{486 \sqrt{2} \pi^2 M_{\eta}^6 (M_{\eta}^2 - M_{\eta'}^2)} - \\
& \frac{16 \sqrt{2} \operatorname{Log} \left[ \frac{M_{\eta}^2}{\mu^2} \right] c_{\theta}^7 M_{\theta}^8 M_K^2 M_{\pi}^2 s_{\theta}^5}{243 \pi^2 M_{\eta}^6 (M_{\eta}^2 - M_{\eta'}^2)} - \frac{5 \operatorname{Log} \left[ \frac{M_{\eta}^2}{\mu^2} \right] c_{\theta}^7 M_{\theta}^8 M_{\pi}^4 s_{\theta}^5}{3888 \sqrt{2} \pi^2 M_{\eta}^6 (M_{\eta}^2 - M_{\eta'}^2)} - \frac{5 \operatorname{Log} \left[ \frac{M_{\eta}^2}{\mu^2} \right] c_{\theta}^7 M_{\theta}^8 M_{\pi}^4 s_{\theta}^5}{216 \sqrt{2} \pi^2 M_{\eta}^6 (M_{\eta}^2 - M_{\eta'}^2)} + \\
& \frac{4 \sqrt{2} \operatorname{Log} \left[ \frac{M_{\eta'}^2}{\mu^2} \right] c_{\theta}^7 M_{\theta}^8 M_{\pi}^4 s_{\theta}^5}{243 \pi^2 M_{\eta}^6 (M_{\eta}^2 - M_{\eta'}^2)} + \frac{8 \sqrt{2} \operatorname{Log} \left[ \frac{M_{\eta}^2}{\mu^2} \right] c_{\theta}^7 M_{\theta}^8 M_K^4 M_{\eta'}^2 s_{\theta}^5}{243 \pi^2 M_{\eta'}^8 (M_{\eta}^2 - M_{\eta'}^2)} - \frac{11 \operatorname{Log} \left[ \frac{M_{\eta}^2}{\mu^2} \right] c_{\theta}^7 M_{\theta}^8 M_K^2 M_{\pi}^2 M_{\eta'}^2 s_{\theta}^5}{243 \sqrt{2} \pi^2 M_{\eta'}^8 (M_{\eta}^2 - M_{\eta'}^2)} - \\
& \frac{\operatorname{Log} \left[ \frac{M_{\eta}^2}{\mu^2} \right] c_{\theta}^7 M_{\theta}^8 M_{\pi}^4 M_{\eta'}^2 s_{\theta}^5}{144 \sqrt{2} \pi^2 M_{\eta'}^8 (M_{\eta}^2 - M_{\eta'}^2)} + \frac{2 \sqrt{2} \operatorname{Log} \left[ \frac{M_{\eta}^2}{\mu^2} \right] c_{\theta}^7 M_{\theta}^8 M_{\pi}^4 M_{\eta'}^2 s_{\theta}^5}{243 \pi^2 M_{\eta'}^8 (M_{\eta}^2 - M_{\eta'}^2)} - \frac{25 \sqrt{2} \operatorname{Log} \left[ \frac{M_{\eta}^2}{\mu^2} \right] c_{\theta}^7 M_{\theta}^8 M_K^4 s_{\theta}^5}{243 \pi^2 M_{\eta'}^6 (M_{\eta}^2 - M_{\eta'}^2)} - \\
& \frac{8 \sqrt{2} \operatorname{Log} \left[ \frac{M_{\eta}^2}{\mu^2} \right] c_{\theta}^7 M_{\theta}^8 M_K^4 s_{\theta}^5}{243 \pi^2 M_{\eta'}^6 (M_{\eta}^2 - M_{\eta'}^2)} + \frac{25 \operatorname{Log} \left[ \frac{M_{\eta}^2}{\mu^2} \right] c_{\theta}^7 M_{\theta}^8 M_K^2 M_{\pi}^2 s_{\theta}^5}{243 \sqrt{2} \pi^2 M_{\eta'}^6 (M_{\eta}^2 - M_{\eta'}^2)} + \frac{11 \operatorname{Log} \left[ \frac{M_{\eta}^2}{\mu^2} \right] c_{\theta}^7 M_{\theta}^8 M_K^2 M_{\pi}^2 s_{\theta}^5}{243 \sqrt{2} \pi^2 M_{\eta'}^6 (M_{\eta}^2 - M_{\eta'}^2)} -
\end{aligned}$$

$$\begin{aligned}
& \frac{25 \operatorname{Log}\left[\frac{M_{\eta'}^2}{\mu^2}\right] c_{\theta}^7 M_{\theta}^8 M_{\pi}^4 s_{\theta}^5}{1944 \sqrt{2} \pi^2 M_{\eta'}^6 (M_{\eta}^2 - M_{\eta'}^2)} + \frac{\operatorname{Log}\left[\frac{M_{\eta'}^2}{\mu^2}\right] c_{\theta}^7 M_{\theta}^8 M_{\pi}^4 s_{\theta}^5}{144 \sqrt{2} \pi^2 M_{\eta'}^6 (M_{\eta}^2 - M_{\eta'}^2)} - \frac{2 \sqrt{2} \operatorname{Log}\left[\frac{M_{\eta'}^2}{\mu^2}\right] c_{\theta}^7 M_{\theta}^8 M_{\pi}^4 s_{\theta}^5}{243 \pi^2 M_{\eta'}^6 (M_{\eta}^2 - M_{\eta'}^2)} + \\
& \frac{10 \sqrt{2} \operatorname{Log}\left[\frac{M_{\eta'}^2}{\mu^2}\right] c_{\theta}^7 M_{\theta}^8 M_{\pi}^4 s_{\theta}^5}{81 \pi^2 M_{\eta'}^4 M_{\eta'}^4 (M_{\eta}^2 - M_{\eta'}^2)} + \frac{25 \sqrt{2} \operatorname{Log}\left[\frac{M_{\eta'}^2}{\mu^2}\right] c_{\theta}^7 M_{\theta}^8 M_{\pi}^4 s_{\theta}^5}{243 \pi^2 M_{\eta'}^4 M_{\eta'}^4 (M_{\eta}^2 - M_{\eta'}^2)} + \frac{23 \operatorname{Log}\left[\frac{M_{\eta'}^2}{\mu^2}\right] c_{\theta}^7 M_{\theta}^8 M_{\pi}^4 s_{\theta}^5}{162 \sqrt{2} \pi^2 M_{\eta'}^4 M_{\eta'}^4 (M_{\eta}^2 - M_{\eta'}^2)} - \\
& \frac{10 \sqrt{2} \operatorname{Log}\left[\frac{M_{\eta'}^2}{\mu^2}\right] c_{\theta}^7 M_{\theta}^8 M_{\pi}^4 s_{\theta}^5}{81 \pi^2 M_{\eta'}^4 M_{\eta'}^4 (M_{\eta}^2 - M_{\eta'}^2)} - \frac{25 \operatorname{Log}\left[\frac{M_{\eta'}^2}{\mu^2}\right] c_{\theta}^7 M_{\theta}^8 M_{\pi}^4 s_{\theta}^5}{243 \sqrt{2} \pi^2 M_{\eta'}^4 M_{\eta'}^4 (M_{\eta}^2 - M_{\eta'}^2)} + \frac{\operatorname{Log}\left[\frac{M_{\eta'}^2}{\mu^2}\right] c_{\theta}^7 M_{\theta}^8 M_{\pi}^4 s_{\theta}^5}{162 \sqrt{2} \pi^2 M_{\eta'}^4 M_{\eta'}^4 (M_{\eta}^2 - M_{\eta'}^2)} + \\
& \frac{25 \operatorname{Log}\left[\frac{M_{\eta'}^2}{\mu^2}\right] c_{\theta}^7 M_{\theta}^8 M_{\pi}^4 s_{\theta}^5}{1944 \sqrt{2} \pi^2 M_{\eta'}^4 M_{\eta'}^4 (M_{\eta}^2 - M_{\eta'}^2)} - \frac{16 \sqrt{2} \operatorname{Log}\left[\frac{M_{\eta'}^2}{\mu^2}\right] c_{\theta}^7 M_{\theta}^8 M_{\pi}^4 s_{\theta}^5}{243 \pi^2 M_{\eta'}^4 M_{\eta'}^4 (M_{\eta}^2 - M_{\eta'}^2)} - \frac{10 \sqrt{2} \operatorname{Log}\left[\frac{M_{\eta'}^2}{\mu^2}\right] c_{\theta}^7 M_{\theta}^8 M_{\pi}^4 s_{\theta}^5}{81 \pi^2 M_{\eta'}^4 M_{\eta'}^4 (M_{\eta}^2 - M_{\eta'}^2)} - \\
& \frac{29 \operatorname{Log}\left[\frac{M_{\eta'}^2}{\mu^2}\right] c_{\theta}^7 M_{\theta}^8 M_{\pi}^4 s_{\theta}^5}{486 \sqrt{2} \pi^2 M_{\eta'}^4 M_{\eta'}^4 (M_{\eta}^2 - M_{\eta'}^2)} + \frac{16 \sqrt{2} \operatorname{Log}\left[\frac{M_{\eta'}^2}{\mu^2}\right] c_{\theta}^7 M_{\theta}^8 M_{\pi}^4 s_{\theta}^5}{243 \pi^2 M_{\eta'}^4 M_{\eta'}^4 (M_{\eta}^2 - M_{\eta'}^2)} - \frac{23 \operatorname{Log}\left[\frac{M_{\eta'}^2}{\mu^2}\right] c_{\theta}^7 M_{\theta}^8 M_{\pi}^4 s_{\theta}^5}{162 \sqrt{2} \pi^2 M_{\eta'}^4 M_{\eta'}^4 (M_{\eta}^2 - M_{\eta'}^2)} + \\
& \frac{10 \sqrt{2} \operatorname{Log}\left[\frac{M_{\eta'}^2}{\mu^2}\right] c_{\theta}^7 M_{\theta}^8 M_{\pi}^4 s_{\theta}^5}{81 \pi^2 M_{\eta'}^4 M_{\eta'}^4 (M_{\eta}^2 - M_{\eta'}^2)} + \frac{5 \operatorname{Log}\left[\frac{M_{\eta'}^2}{\mu^2}\right] c_{\theta}^7 M_{\theta}^8 M_{\pi}^4 s_{\theta}^5}{216 \sqrt{2} \pi^2 M_{\eta'}^4 M_{\eta'}^4 (M_{\eta}^2 - M_{\eta'}^2)} - \frac{4 \sqrt{2} \operatorname{Log}\left[\frac{M_{\eta'}^2}{\mu^2}\right] c_{\theta}^7 M_{\theta}^8 M_{\pi}^4 s_{\theta}^5}{243 \pi^2 M_{\eta'}^4 M_{\eta'}^4 (M_{\eta}^2 - M_{\eta'}^2)} - \\
& \frac{\operatorname{Log}\left[\frac{M_{\eta'}^2}{\mu^2}\right] c_{\theta}^7 M_{\theta}^8 M_{\pi}^4 s_{\theta}^5}{162 \sqrt{2} \pi^2 M_{\eta'}^4 M_{\eta'}^4 (M_{\eta}^2 - M_{\eta'}^2)} - \frac{2 \sqrt{2} \operatorname{Log}\left[\frac{M_{\eta'}^2}{\mu^2}\right] c_{\theta}^7 M_{\theta}^8 M_{\pi}^4 s_{\theta}^5}{243 \pi^2 M_{\eta'}^4 M_{\eta'}^4 (M_{\eta}^2 - M_{\eta'}^2)} + \frac{\sqrt{2} \operatorname{Log}\left[\frac{M_{\eta'}^2}{\mu^2}\right] c_{\theta}^7 M_{\theta}^8 M_{\pi}^4 s_{\theta}^5}{243 \pi^2 M_{\eta'}^4 M_{\eta'}^4 (M_{\eta}^2 - M_{\eta'}^2)} + \\
& \frac{5 \operatorname{Log}\left[\frac{M_{\eta'}^2}{\mu^2}\right] c_{\theta}^7 M_{\theta}^8 M_{\pi}^4 s_{\theta}^5}{3888 \sqrt{2} \pi^2 M_{\eta'}^4 M_{\eta'}^4 (M_{\eta}^2 - M_{\eta'}^2)} - \frac{9175040 c_{\theta}^6 L_8^2 r M_{\theta}^8 M_{\pi}^{10} s_{\theta}^6}{729 F^2 M_{\eta}^{12}} + \frac{7659520 c_{\theta}^6 L_8^2 r M_{\theta}^8 M_{\pi}^8 s_{\theta}^6}{243 F^2 M_{\eta}^{12}} - \\
& \frac{7536640 c_{\theta}^6 L_8^2 r M_{\theta}^8 M_{\pi}^6 s_{\theta}^6}{243 F^2 M_{\eta}^{12}} + \frac{10726400 c_{\theta}^6 L_8^2 r M_{\theta}^8 M_{\pi}^4 s_{\theta}^6}{729 F^2 M_{\eta}^{12}} - \frac{793600 c_{\theta}^6 L_8^2 r M_{\theta}^8 M_{\pi}^2 s_{\theta}^6}{243 F^2 M_{\eta}^{12}} + \\
& \frac{16640 c_{\theta}^6 L_8^2 r M_{\theta}^8 M_{\pi}^{10} s_{\theta}^6}{81 F^2 M_{\eta}^{12}} + \frac{64 F^2 v_2^{(2)} c_{\theta}^4 M_{\theta}^8 M_{\pi}^4 s_{\theta}^6}{27 M_{\eta}^{10}} - \frac{20 \operatorname{Log}\left[\frac{M_K^2}{\mu^2}\right] c_{\theta}^4 M_{\theta}^8 M_{\pi}^6 s_{\theta}^6}{243 \pi^2 M_{\eta}^{10}} + \\
& \frac{5120 c_{\theta}^4 L_6^r M_{\theta}^8 M_{\pi}^6 s_{\theta}^6}{81 M_{\eta}^{10}} + \frac{5120 c_{\theta}^4 L_7^r M_{\theta}^8 M_{\pi}^6 s_{\theta}^6}{81 M_{\eta}^{10}} - \frac{5120 c_{\theta}^4 L_{25}^r M_{\theta}^8 M_{\pi}^6 s_{\theta}^6}{81 M_{\eta}^{10}} + \frac{10240 c_{\theta}^4 C_{19} M_{\theta}^8 M_{\pi}^8 s_{\theta}^6}{27 M_{\eta}^{10}} + \\
& \frac{20480 c_{\theta}^4 C_{31} M_{\theta}^8 M_{\pi}^8 s_{\theta}^6}{81 M_{\eta}^{10}} + \frac{4 F^2 v_2^{(2)} c_{\theta}^4 M_{\theta}^8 M_{\pi}^2 s_{\theta}^6}{27 M_{\eta}^{10}} + \frac{91 \operatorname{Log}\left[\frac{M_K^2}{\mu^2}\right] c_{\theta}^4 M_{\theta}^8 M_{\pi}^4 s_{\theta}^6}{972 \pi^2 M_{\eta}^{10}} - \\
& \frac{320 c_{\theta}^4 L_6^r M_{\theta}^8 M_{\pi}^4 s_{\theta}^6}{9 M_{\eta}^{10}} - \frac{832 c_{\theta}^4 L_7^r M_{\theta}^8 M_{\pi}^4 s_{\theta}^6}{9 M_{\eta}^{10}} + \frac{8128 c_{\theta}^4 L_{25}^r M_{\theta}^8 M_{\pi}^4 s_{\theta}^6}{81 M_{\eta}^{10}} - \\
& \frac{20096 c_{\theta}^4 C_{19} M_{\theta}^8 M_{\pi}^6 s_{\theta}^6}{27 M_{\eta}^{10}} - \frac{40192 c_{\theta}^4 C_{31} M_{\theta}^8 M_{\pi}^6 s_{\theta}^6}{81 M_{\eta}^{10}} - \frac{14 F^2 v_2^{(2)} c_{\theta}^4 M_{\theta}^8 M_{\pi}^4 s_{\theta}^6}{27 M_{\eta}^{10}} - \\
& \frac{23 \operatorname{Log}\left[\frac{M_K^2}{\mu^2}\right] c_{\theta}^4 M_{\theta}^8 M_{\pi}^2 s_{\theta}^6}{972 \pi^2 M_{\eta}^{10}} + \frac{\operatorname{Log}\left[\frac{M_K^2}{\mu^2}\right] c_{\theta}^4 M_{\theta}^8 M_{\pi}^2 s_{\theta}^6}{54 \pi^2 M_{\eta}^{10}} - \frac{320 c_{\theta}^4 L_6^r M_{\theta}^8 M_{\pi}^4 s_{\theta}^6}{27 M_{\eta}^{10}} +
\end{aligned}$$

$$\begin{aligned}
& \frac{832 c_{\theta}^4 L_7^r M_0^8 M_K^2 M_{\pi}^4 s_{\theta}^6}{27 M_{\eta}^{10}} - \frac{3776 c_{\theta}^4 L_{25}^r M_0^8 M_K^2 M_{\pi}^4 s_{\theta}^6}{81 M_{\eta}^{10}} + \frac{4928 c_{\theta}^4 C_{19} M_0^8 M_K^4 M_{\pi}^4 s_{\theta}^6}{9 M_{\eta}^{10}} + \\
& \frac{9856 c_{\theta}^4 C_{31} M_0^8 M_K^4 M_{\pi}^4 s_{\theta}^6}{27 M_{\eta}^{10}} - \frac{\text{Log}\left[\frac{M_{\pi}^2}{\mu^2}\right] c_{\theta}^4 M_0^8 M_{\pi}^6 s_{\theta}^6}{48 \pi^2 M_{\eta}^{10}} + \frac{880 c_{\theta}^4 L_6^r M_0^8 M_{\pi}^6 s_{\theta}^6}{81 M_{\eta}^{10}} + \frac{304 c_{\theta}^4 L_7^r M_0^8 M_{\pi}^6 s_{\theta}^6}{81 M_{\eta}^{10}} + \\
& \frac{112 c_{\theta}^4 L_{25}^r M_0^8 M_{\pi}^6 s_{\theta}^6}{27 M_{\eta}^{10}} - \frac{1696 c_{\theta}^4 C_{19} M_0^8 M_K^2 M_{\pi}^6 s_{\theta}^6}{9 M_{\eta}^{10}} - \frac{3392 c_{\theta}^4 C_{31} M_0^8 M_K^2 M_{\pi}^6 s_{\theta}^6}{27 M_{\eta}^{10}} + \\
& \frac{880 c_{\theta}^4 C_{19} M_0^8 M_{\pi}^6 s_{\theta}^6}{27 M_{\eta}^{10}} + \frac{1760 c_{\theta}^4 C_{31} M_0^8 M_{\pi}^6 s_{\theta}^6}{81 M_{\eta}^{10}} - \frac{8 F^2 v_2^{(2)} c_{\theta}^2 M_0^8 M_K^2 s_{\theta}^6}{3 M_{\eta}^8} - \frac{64 F^2 v_2^{(2)} c_{\theta}^2 M_0^6 M_K^4 s_{\theta}^6}{9 M_{\eta}^8} + \\
& \frac{c_{\theta}^2 M_0^8 M_K^4 s_{\theta}^6}{108 \pi^2 M_{\eta}^8} + \frac{\text{Log}\left[\frac{M_K^2}{\mu^2}\right] c_{\theta}^2 M_0^8 M_K^4 s_{\theta}^6}{108 \pi^2 M_{\eta}^8} + \frac{55 c_{\theta}^6 M_0^8 M_K^4 s_{\theta}^6}{486 \pi^2 M_{\eta}^8} - \frac{28 \text{Log}\left[\frac{M_{\eta}^2}{\mu^2}\right] c_{\theta}^6 M_0^8 M_K^4 s_{\theta}^6}{729 \pi^2 M_{\eta}^8} - \\
& \frac{5 \text{Log}\left[\frac{M_{\eta}^2}{\mu^2}\right] c_{\theta}^6 M_0^8 M_K^4 s_{\theta}^6}{486 \pi^2 M_{\eta}^8} - \frac{512 c_{\theta}^2 L_6^r M_0^8 M_K^4 s_{\theta}^6}{27 M_{\eta}^8} - \frac{512 c_{\theta}^2 L_7^r M_0^8 M_K^4 s_{\theta}^6}{27 M_{\eta}^8} - \frac{1792 c_{\theta}^2 C_{19} M_0^8 M_K^6 s_{\theta}^6}{9 M_{\eta}^8} - \\
& \frac{5120 c_{\theta}^2 C_{31} M_0^8 M_K^6 s_{\theta}^6}{27 M_{\eta}^8} + \frac{2 F^2 v_2^{(2)} c_{\theta}^2 M_0^8 M_{\pi}^2 s_{\theta}^6}{3 M_{\eta}^8} - \frac{16 F^2 v_2^{(2)} c_{\theta}^2 M_0^6 M_K^2 M_{\pi}^2 s_{\theta}^6}{9 M_{\eta}^8} - \frac{5 c_{\theta}^2 M_0^8 M_K^2 M_{\pi}^2 s_{\theta}^6}{432 \pi^2 M_{\eta}^8} - \\
& \frac{\text{Log}\left[\frac{M_K^2}{\mu^2}\right] c_{\theta}^2 M_0^8 M_K^2 M_{\pi}^2 s_{\theta}^6}{72 \pi^2 M_{\eta}^8} - \frac{28 c_{\theta}^6 M_0^8 M_K^2 M_{\pi}^2 s_{\theta}^6}{243 \pi^2 M_{\eta}^8} + \frac{113 \text{Log}\left[\frac{M_{\eta}^2}{\mu^2}\right] c_{\theta}^6 M_0^8 M_K^2 M_{\pi}^2 s_{\theta}^6}{2916 \pi^2 M_{\eta}^8} + \\
& \frac{\text{Log}\left[\frac{M_{\eta}^2}{\mu^2}\right] c_{\theta}^6 M_0^8 M_K^2 M_{\pi}^2 s_{\theta}^6}{36 \pi^2 M_{\eta}^8} + \frac{448 c_{\theta}^2 L_6^r M_0^8 M_K^2 M_{\pi}^2 s_{\theta}^6}{27 M_{\eta}^8} + \frac{448 c_{\theta}^2 L_7^r M_0^8 M_K^2 M_{\pi}^2 s_{\theta}^6}{27 M_{\eta}^8} + \\
& \frac{896 c_{\theta}^2 C_{19} M_0^8 M_K^4 M_{\pi}^2 s_{\theta}^6}{3 M_{\eta}^8} + \frac{2560 c_{\theta}^2 C_{31} M_0^8 M_K^4 M_{\pi}^2 s_{\theta}^6}{9 M_{\eta}^8} + \frac{8 F^2 v_2^{(2)} c_{\theta}^2 M_0^6 M_{\pi}^4 s_{\theta}^6}{9 M_{\eta}^8} + \frac{11 c_{\theta}^2 M_0^8 M_{\pi}^4 s_{\theta}^6}{864 \pi^2 M_{\eta}^8} + \\
& \frac{\text{Log}\left[\frac{M_K^2}{\mu^2}\right] c_{\theta}^2 M_0^8 M_{\pi}^4 s_{\theta}^6}{432 \pi^2 M_{\eta}^8} + \frac{\text{Log}\left[\frac{M_{\pi}^2}{\mu^2}\right] c_{\theta}^2 M_0^8 M_{\pi}^4 s_{\theta}^6}{72 \pi^2 M_{\eta}^8} + \frac{241 c_{\theta}^6 M_0^8 M_{\pi}^4 s_{\theta}^6}{7776 \pi^2 M_{\eta}^8} - \frac{121 \text{Log}\left[\frac{M_{\eta}^2}{\mu^2}\right] c_{\theta}^6 M_0^8 M_{\pi}^4 s_{\theta}^6}{11664 \pi^2 M_{\eta}^8} - \\
& \frac{73 \text{Log}\left[\frac{M_{\eta}^2}{\mu^2}\right] c_{\theta}^6 M_0^8 M_{\pi}^4 s_{\theta}^6}{7776 \pi^2 M_{\eta}^8} - \frac{224 c_{\theta}^2 L_6^r M_0^8 M_{\pi}^4 s_{\theta}^6}{27 M_{\eta}^8} - \frac{224 c_{\theta}^2 L_7^r M_0^8 M_{\pi}^4 s_{\theta}^6}{27 M_{\eta}^8} - \frac{448 c_{\theta}^2 C_{19} M_0^8 M_K^2 M_{\pi}^4 s_{\theta}^6}{3 M_{\eta}^8} - \\
& \frac{1280 c_{\theta}^2 C_{31} M_0^8 M_K^2 M_{\pi}^4 s_{\theta}^6}{9 M_{\eta}^8} + \frac{112 c_{\theta}^2 C_{19} M_0^8 M_{\pi}^6 s_{\theta}^6}{9 M_{\eta}^8} + \frac{320 c_{\theta}^2 C_{31} M_0^8 M_{\pi}^6 s_{\theta}^6}{27 M_{\eta}^8} + \frac{24 F^2 v_4^{(0)} M_0^6 s_{\theta}^6}{M_{\eta}^6} + \\
& \frac{8 F^2 v_2^{(2)} M_0^6 M_K^2 s_{\theta}^6}{3 M_{\eta}^6} + \frac{5 \text{Log}\left[\frac{M_{\eta}^2}{\mu^2}\right] c_{\theta}^4 M_0^8 M_K^2 s_{\theta}^6}{324 \pi^2 M_{\eta}^6} + \frac{11 \text{Log}\left[\frac{M_{\eta}^2}{\mu^2}\right] c_{\theta}^4 M_0^8 M_K^2 s_{\theta}^6}{972 \pi^2 M_{\eta}^6} + \frac{4 F^2 v_2^{(2)} M_0^6 M_{\pi}^2 s_{\theta}^6}{3 M_{\eta}^6} - \\
& \frac{35 \text{Log}\left[\frac{M_{\eta}^2}{\mu^2}\right] c_{\theta}^4 M_0^8 M_{\pi}^2 s_{\theta}^6}{5184 \pi^2 M_{\eta}^6} - \frac{55 \text{Log}\left[\frac{M_{\eta}^2}{\mu^2}\right] c_{\theta}^4 M_0^8 M_{\pi}^2 s_{\theta}^6}{7776 \pi^2 M_{\eta}^6} - \frac{9175040 c_{\theta}^6 L_8^2 r M_0^8 M_K^{10} s_{\theta}^6}{729 F^2 M_{\eta}^{12}} +
\end{aligned}$$

$$\begin{aligned}
& \frac{7\,659\,520\,c_\theta^6\,L_8^2\,r\,M_\theta^8\,M_K^8\,M_\pi^2\,s_\theta^6}{243\,F^2\,M_{\eta'}^{12}} - \frac{7\,536\,640\,c_\theta^6\,L_8^2\,r\,M_\theta^8\,M_K^6\,M_\pi^4\,s_\theta^6}{243\,F^2\,M_{\eta'}^{12}} + \frac{10\,726\,400\,c_\theta^6\,L_8^2\,r\,M_\theta^8\,M_K^4\,M_\pi^6\,s_\theta^6}{729\,F^2\,M_{\eta'}^{12}} - \\
& \frac{793\,600\,c_\theta^6\,L_8^2\,r\,M_\theta^8\,M_K^2\,M_\pi^8\,s_\theta^6}{243\,F^2\,M_{\eta'}^{12}} + \frac{16\,640\,c_\theta^6\,L_8^2\,r\,M_\theta^8\,M_\pi^{10}\,s_\theta^6}{81\,F^2\,M_{\eta'}^{12}} + \frac{2048\,c_\theta^4\,L_6^r\,M_\theta^8\,M_K^6\,s_\theta^6}{243\,M_{\eta'}^{10}} + \\
& \frac{2048\,c_\theta^4\,L_7^r\,M_\theta^8\,M_K^6\,s_\theta^6}{243\,M_{\eta'}^{10}} + \frac{4096\,c_\theta^4\,C_{19}\,M_\theta^8\,M_K^8\,s_\theta^6}{81\,M_{\eta'}^{10}} + \frac{8192\,c_\theta^4\,C_{31}\,M_\theta^8\,M_K^8\,s_\theta^6}{243\,M_{\eta'}^{10}} + \frac{\text{Log}\left[\frac{M_K^2}{\mu^2}\right]\,c_\theta^4\,M_\theta^8\,M_K^4\,M_\pi^2\,s_\theta^6}{243\,\pi^2\,M_{\eta'}^{10}} - \\
& \frac{128\,c_\theta^4\,L_6^r\,M_\theta^8\,M_K^4\,M_\pi^2\,s_\theta^6}{81\,M_{\eta'}^{10}} - \frac{1664\,c_\theta^4\,L_7^r\,M_\theta^8\,M_K^4\,M_\pi^2\,s_\theta^6}{81\,M_{\eta'}^{10}} - \frac{7936\,c_\theta^4\,C_{19}\,M_\theta^8\,M_K^6\,M_\pi^2\,s_\theta^6}{81\,M_{\eta'}^{10}} - \\
& \frac{15\,872\,c_\theta^4\,C_{31}\,M_\theta^8\,M_K^6\,M_\pi^2\,s_\theta^6}{243\,M_{\eta'}^{10}} - \frac{7\,\text{Log}\left[\frac{M_K^2}{\mu^2}\right]\,c_\theta^4\,M_\theta^8\,M_K^2\,M_\pi^4\,s_\theta^6}{3888\,\pi^2\,M_{\eta'}^{10}} - \frac{\text{Log}\left[\frac{M_\pi^2}{\mu^2}\right]\,c_\theta^4\,M_\theta^8\,M_K^2\,M_\pi^4\,s_\theta^6}{162\,\pi^2\,M_{\eta'}^{10}} - \\
& \frac{160\,c_\theta^4\,L_6^r\,M_\theta^8\,M_K^4\,M_\pi^4\,s_\theta^6}{81\,M_{\eta'}^{10}} + \frac{1280\,c_\theta^4\,L_7^r\,M_\theta^8\,M_K^4\,M_\pi^4\,s_\theta^6}{81\,M_{\eta'}^{10}} + \frac{640\,c_\theta^4\,C_{19}\,M_\theta^8\,M_K^4\,M_\pi^4\,s_\theta^6}{9\,M_{\eta'}^{10}} + \\
& \frac{1280\,c_\theta^4\,C_{31}\,M_\theta^8\,M_K^4\,M_\pi^4\,s_\theta^6}{27\,M_{\eta'}^{10}} + \frac{7\,\text{Log}\left[\frac{M_\pi^2}{\mu^2}\right]\,c_\theta^4\,M_\theta^8\,M_\pi^6\,s_\theta^6}{2592\,\pi^2\,M_{\eta'}^{10}} + \frac{112\,c_\theta^4\,L_6^r\,M_\theta^8\,M_\pi^6\,s_\theta^6}{243\,M_{\eta'}^{10}} - \frac{896\,c_\theta^4\,L_7^r\,M_\theta^8\,M_\pi^6\,s_\theta^6}{243\,M_{\eta'}^{10}} - \\
& \frac{1600\,c_\theta^4\,C_{19}\,M_\theta^8\,M_K^6\,M_\pi^6\,s_\theta^6}{81\,M_{\eta'}^{10}} - \frac{3200\,c_\theta^4\,C_{31}\,M_\theta^8\,M_K^6\,M_\pi^6\,s_\theta^6}{243\,M_{\eta'}^{10}} + \frac{112\,c_\theta^4\,C_{19}\,M_\theta^8\,M_\pi^8\,s_\theta^6}{81\,M_{\eta'}^{10}} + \frac{224\,c_\theta^4\,C_{31}\,M_\theta^8\,M_\pi^8\,s_\theta^6}{243\,M_{\eta'}^{10}} + \\
& \frac{6\,225\,920\,c_\theta^6\,L_8^2\,r\,M_\theta^8\,M_K^{10}\,s_\theta^6}{729\,F^2\,M_{\eta'}^{10}} - \frac{5\,287\,936\,c_\theta^6\,L_8^2\,r\,M_\theta^8\,M_K^8\,M_\pi^2\,s_\theta^6}{243\,F^2\,M_{\eta'}^{10}} + \frac{5\,005\,312\,c_\theta^6\,L_8^2\,r\,M_\theta^8\,M_K^6\,M_\pi^4\,s_\theta^6}{243\,F^2\,M_{\eta'}^{10}} - \\
& \frac{5\,685\,248\,c_\theta^6\,L_8^2\,r\,M_\theta^8\,M_K^4\,M_\pi^6\,s_\theta^6}{729\,F^2\,M_{\eta'}^{10}} + \frac{120\,832\,c_\theta^6\,L_8^2\,r\,M_\theta^8\,M_K^2\,M_\pi^8\,s_\theta^6}{243\,F^2\,M_{\eta'}^{10}} - \frac{5120\,c_\theta^6\,L_8^2\,r\,M_\theta^8\,M_\pi^{10}\,s_\theta^6}{27\,F^2\,M_{\eta'}^{10}} + \\
& \frac{10\,\text{Log}\left[\frac{M_\pi^2}{\mu^2}\right]\,c_\theta^6\,M_\theta^8\,M_K^4\,M_\pi^2\,s_\theta^6}{729\,\pi^2\,M_{\eta'}^{10}} - \frac{97\,\text{Log}\left[\frac{M_\pi^2}{\mu^2}\right]\,c_\theta^6\,M_\theta^8\,M_K^2\,M_\pi^2\,M_\pi^2\,s_\theta^6}{5832\,\pi^2\,M_{\eta'}^{10}} + \frac{77\,\text{Log}\left[\frac{M_\pi^2}{\mu^2}\right]\,c_\theta^6\,M_\theta^8\,M_\pi^4\,M_\pi^2\,s_\theta^6}{23\,328\,\pi^2\,M_{\eta'}^{10}} + \\
& \frac{55\,c_\theta^6\,M_\theta^8\,M_K^4\,s_\theta^6}{486\,\pi^2\,M_{\eta'}^8} - \frac{5\,\text{Log}\left[\frac{M_\pi^2}{\mu^2}\right]\,c_\theta^6\,M_\theta^8\,M_K^4\,s_\theta^6}{486\,\pi^2\,M_{\eta'}^8} - \frac{28\,\text{Log}\left[\frac{M_{\eta'}^2}{\mu^2}\right]\,c_\theta^6\,M_\theta^8\,M_K^4\,s_\theta^6}{729\,\pi^2\,M_{\eta'}^8} - \frac{28\,c_\theta^6\,M_\theta^8\,M_K^2\,M_\pi^2\,s_\theta^6}{243\,\pi^2\,M_{\eta'}^8} + \\
& \frac{\text{Log}\left[\frac{M_\pi^2}{\mu^2}\right]\,c_\theta^6\,M_\theta^8\,M_K^2\,M_\pi^2\,s_\theta^6}{36\,\pi^2\,M_{\eta'}^8} + \frac{113\,\text{Log}\left[\frac{M_{\eta'}^2}{\mu^2}\right]\,c_\theta^6\,M_\theta^8\,M_K^2\,M_\pi^2\,s_\theta^6}{2916\,\pi^2\,M_{\eta'}^8} + \frac{241\,c_\theta^6\,M_\theta^8\,M_\pi^4\,s_\theta^6}{7776\,\pi^2\,M_{\eta'}^8} - \\
& \frac{73\,\text{Log}\left[\frac{M_\pi^2}{\mu^2}\right]\,c_\theta^6\,M_\theta^8\,M_\pi^4\,s_\theta^6}{7776\,\pi^2\,M_{\eta'}^8} - \frac{121\,\text{Log}\left[\frac{M_{\eta'}^2}{\mu^2}\right]\,c_\theta^6\,M_\theta^8\,M_\pi^4\,s_\theta^6}{11\,664\,\pi^2\,M_{\eta'}^8} + \frac{1\,310\,720\,c_\theta^6\,L_8^2\,r\,M_\theta^8\,M_K^{10}\,s_\theta^6}{729\,F^2\,M_{\eta'}^8} - \\
& \frac{704\,512\,c_\theta^6\,L_8^2\,r\,M_\theta^8\,M_K^8\,M_\pi^2\,s_\theta^6}{243\,F^2\,M_{\eta'}^8} + \frac{237\,568\,c_\theta^6\,L_8^2\,r\,M_\theta^8\,M_K^6\,M_\pi^4\,s_\theta^6}{243\,F^2\,M_{\eta'}^8} - \frac{355\,328\,c_\theta^6\,L_8^2\,r\,M_\theta^8\,M_K^4\,M_\pi^6\,s_\theta^6}{729\,F^2\,M_{\eta'}^8} + \\
& \frac{185\,344\,c_\theta^6\,L_8^2\,r\,M_\theta^8\,M_K^2\,M_\pi^8\,s_\theta^6}{243\,F^2\,M_{\eta'}^8} - \frac{3328\,c_\theta^6\,L_8^2\,r\,M_\theta^8\,M_\pi^{10}\,s_\theta^6}{27\,F^2\,M_{\eta'}^8} + \frac{64\,F^2\,v_2^{(2)}\,c_\theta^4\,M_\theta^8\,M_K^4\,s_\theta^6}{27\,M_{\eta'}^8} -
\end{aligned}$$

$$\begin{aligned}
& \frac{26 \operatorname{Log}\left[\frac{M_K^2}{\mu^2}\right] c_\theta^4 M_\theta^8 M_K^6 s_\theta^6}{243 \pi^2 M_\eta^2 M_{\eta'}^8} + \frac{13\,312 c_\theta^4 L_6^r M_\theta^8 M_K^6 s_\theta^6}{243 M_\eta^2 M_{\eta'}^8} + \frac{13\,312 c_\theta^4 L_7^r M_\theta^8 M_K^6 s_\theta^6}{243 M_\eta^2 M_{\eta'}^8} - \\
& \frac{6656 c_\theta^4 L_{25}^r M_\theta^8 M_K^6 s_\theta^6}{81 M_\eta^2 M_{\eta'}^8} + \frac{26\,624 c_\theta^4 C_{19} M_\theta^8 M_K^6 s_\theta^6}{81 M_\eta^2 M_{\eta'}^8} + \frac{53\,248 c_\theta^4 C_{31} M_\theta^8 M_K^6 s_\theta^6}{243 M_\eta^2 M_{\eta'}^8} + \\
& \frac{4 F^2 v_2^{(2)} c_\theta^4 M_\theta^8 M_K^4 M_\pi^2 s_\theta^6}{27 M_\eta^2 M_{\eta'}^8} + \frac{\operatorname{Log}\left[\frac{M_K^2}{\mu^2}\right] c_\theta^4 M_\theta^8 M_K^4 M_\pi^2 s_\theta^6}{9 \pi^2 M_\eta^2 M_{\eta'}^8} - \frac{3520 c_\theta^4 L_6^r M_\theta^8 M_K^4 M_\pi^2 s_\theta^6}{81 M_\eta^2 M_{\eta'}^8} - \\
& \frac{4288 c_\theta^4 L_7^r M_\theta^8 M_K^4 M_\pi^2 s_\theta^6}{81 M_\eta^2 M_{\eta'}^8} + \frac{10\,624 c_\theta^4 L_{25}^r M_\theta^8 M_K^4 M_\pi^2 s_\theta^6}{81 M_\eta^2 M_{\eta'}^8} - \frac{52\,352 c_\theta^4 C_{19} M_\theta^8 M_K^4 M_\pi^2 s_\theta^6}{81 M_\eta^2 M_{\eta'}^8} - \\
& \frac{104\,704 c_\theta^4 C_{31} M_\theta^8 M_K^4 M_\pi^2 s_\theta^6}{243 M_\eta^2 M_{\eta'}^8} - \frac{14 F^2 v_2^{(2)} c_\theta^4 M_\theta^8 M_K^4 s_\theta^6}{27 M_\eta^2 M_{\eta'}^8} - \frac{25 \operatorname{Log}\left[\frac{M_K^2}{\mu^2}\right] c_\theta^4 M_\theta^8 M_K^4 M_\pi^2 s_\theta^6}{972 \pi^2 M_\eta^2 M_{\eta'}^8} + \\
& \frac{17 \operatorname{Log}\left[\frac{M_\pi^2}{\mu^2}\right] c_\theta^4 M_\theta^8 M_K^4 M_\pi^2 s_\theta^6}{324 \pi^2 M_\eta^2 M_{\eta'}^8} - \frac{704 c_\theta^4 L_6^r M_\theta^8 M_K^4 M_\pi^2 s_\theta^6}{81 M_\eta^2 M_{\eta'}^8} - \frac{1280 c_\theta^4 L_7^r M_\theta^8 M_K^4 M_\pi^2 s_\theta^6}{81 M_\eta^2 M_{\eta'}^8} - \\
& \frac{4736 c_\theta^4 L_{25}^r M_\theta^8 M_K^4 M_\pi^2 s_\theta^6}{81 M_\eta^2 M_{\eta'}^8} + \frac{4288 c_\theta^4 C_{19} M_\theta^8 M_K^4 M_\pi^2 s_\theta^6}{9 M_\eta^2 M_{\eta'}^8} + \frac{8576 c_\theta^4 C_{31} M_\theta^8 M_K^4 M_\pi^2 s_\theta^6}{27 M_\eta^2 M_{\eta'}^8} - \\
& \frac{53 \operatorname{Log}\left[\frac{M_\pi^2}{\mu^2}\right] c_\theta^4 M_\theta^8 M_\pi^6 s_\theta^6}{1296 \pi^2 M_\eta^2 M_{\eta'}^8} + \frac{3248 c_\theta^4 L_6^r M_\theta^8 M_\pi^6 s_\theta^6}{243 M_\eta^2 M_{\eta'}^8} + \frac{4688 c_\theta^4 L_7^r M_\theta^8 M_\pi^6 s_\theta^6}{243 M_\eta^2 M_{\eta'}^8} + \frac{112 c_\theta^4 L_{25}^r M_\theta^8 M_\pi^6 s_\theta^6}{27 M_\eta^2 M_{\eta'}^8} - \\
& \frac{14\,816 c_\theta^4 C_{19} M_\theta^8 M_\pi^6 s_\theta^6}{81 M_\eta^2 M_{\eta'}^8} - \frac{29\,632 c_\theta^4 C_{31} M_\theta^8 M_\pi^6 s_\theta^6}{243 M_\eta^2 M_{\eta'}^8} + \frac{3248 c_\theta^4 C_{19} M_\theta^8 M_\pi^8 s_\theta^6}{81 M_\eta^2 M_{\eta'}^8} + \\
& \frac{6496 c_\theta^4 C_{31} M_\theta^8 M_\pi^8 s_\theta^6}{243 M_\eta^2 M_{\eta'}^8} + \frac{\operatorname{Log}\left[\frac{M_\eta^2}{\mu^2}\right] c_\theta^4 M_\theta^8 M_K^2 M_\eta^2 s_\theta^6}{972 \pi^2 M_{\eta'}^8} - \frac{7 \operatorname{Log}\left[\frac{M_\eta^2}{\mu^2}\right] c_\theta^4 M_\theta^8 M_\pi^2 M_\eta^2 s_\theta^6}{15\,552 \pi^2 M_{\eta'}^8} - \\
& \frac{\operatorname{Log}\left[\frac{M_\eta^2}{\mu^2}\right] c_\theta^4 M_\theta^8 M_K^2 s_\theta^6}{162 \pi^2 M_{\eta'}^6} + \frac{\operatorname{Log}\left[\frac{M_{\eta'}^2}{\mu^2}\right] c_\theta^4 M_\theta^8 M_K^2 s_\theta^6}{486 \pi^2 M_{\eta'}^6} + \frac{5 \operatorname{Log}\left[\frac{M_\eta^2}{\mu^2}\right] c_\theta^4 M_\theta^8 M_\pi^2 s_\theta^6}{1296 \pi^2 M_{\eta'}^6} - \frac{31 \operatorname{Log}\left[\frac{M_{\eta'}^2}{\mu^2}\right] c_\theta^4 M_\theta^8 M_\pi^2 s_\theta^6}{31\,104 \pi^2 M_{\eta'}^6} - \\
& \frac{4\,096\,000 c_\theta^6 L_8^{2r} M_\theta^8 M_K^{10} s_\theta^6}{729 F^2 M_\eta^6 M_{\eta'}^6} + \frac{2\,809\,856 c_\theta^6 L_8^{2r} M_\theta^8 M_K^8 M_\pi^2 s_\theta^6}{243 F^2 M_\eta^6 M_{\eta'}^6} - \frac{1\,556\,480 c_\theta^6 L_8^{2r} M_\theta^8 M_K^6 M_\pi^4 s_\theta^6}{243 F^2 M_\eta^6 M_{\eta'}^6} - \\
& \frac{155\,648 c_\theta^6 L_8^{2r} M_\theta^8 M_K^4 M_\pi^6 s_\theta^6}{729 F^2 M_\eta^6 M_{\eta'}^6} + \frac{206\,848 c_\theta^6 L_8^{2r} M_\theta^8 M_K^2 M_\pi^8 s_\theta^6}{243 F^2 M_\eta^6 M_{\eta'}^6} - \frac{8192 c_\theta^6 L_8^{2r} M_\theta^8 M_\pi^{10} s_\theta^6}{81 F^2 M_\eta^6 M_{\eta'}^6} + \\
& \frac{320 F^2 v_2^{(2)} c_\theta^4 M_\theta^8 M_K^4 s_\theta^6}{27 M_\eta^4 M_{\eta'}^6} + \frac{17 \operatorname{Log}\left[\frac{M_K^2}{\mu^2}\right] c_\theta^4 M_\theta^8 M_K^6 s_\theta^6}{243 \pi^2 M_\eta^4 M_{\eta'}^6} - \frac{8192 c_\theta^4 L_6^r M_\theta^8 M_K^6 s_\theta^6}{81 M_\eta^4 M_{\eta'}^6} - \\
& \frac{8192 c_\theta^4 L_7^r M_\theta^8 M_K^6 s_\theta^6}{81 M_\eta^4 M_{\eta'}^6} + \frac{4352 c_\theta^4 L_{25}^r M_\theta^8 M_K^6 s_\theta^6}{81 M_\eta^4 M_{\eta'}^6} - \frac{16\,384 c_\theta^4 C_{19} M_\theta^8 M_K^6 s_\theta^6}{27 M_\eta^4 M_{\eta'}^6} - \frac{32\,768 c_\theta^4 C_{31} M_\theta^8 M_K^6 s_\theta^6}{81 M_\eta^4 M_{\eta'}^6} + \\
& \frac{128 F^2 v_2^{(2)} c_\theta^4 M_\theta^8 M_K^4 M_\pi^2 s_\theta^6}{27 M_\eta^4 M_{\eta'}^6} - \frac{139 \operatorname{Log}\left[\frac{M_K^2}{\mu^2}\right] c_\theta^4 M_\theta^8 M_K^4 M_\pi^2 s_\theta^6}{972 \pi^2 M_\eta^4 M_{\eta'}^6} + \frac{2176 c_\theta^4 L_6^r M_\theta^8 M_K^4 M_\pi^2 s_\theta^6}{27 M_\eta^4 M_{\eta'}^6} +
\end{aligned}$$

$$\begin{aligned}
& \frac{4864 c_{\theta}^4 L_7^r M_0^8 M_K^4 M_{\pi}^2 s_{\theta}^6}{27 M_{\eta}^4 M_{\eta'}^6} - \frac{7168 c_{\theta}^4 L_{25}^r M_0^8 M_K^4 M_{\pi}^2 s_{\theta}^6}{81 M_{\eta}^4 M_{\eta'}^6} + \frac{29\,696 c_{\theta}^4 C_{19} M_0^8 M_K^6 M_{\pi}^2 s_{\theta}^6}{27 M_{\eta}^4 M_{\eta'}^6} + \\
& \frac{59\,392 c_{\theta}^4 C_{31} M_0^8 M_K^6 M_{\pi}^2 s_{\theta}^6}{81 M_{\eta}^4 M_{\eta'}^6} - \frac{16 F^2 v_2^{(2)} c_{\theta}^4 M_0^8 M_{\pi}^4 s_{\theta}^6}{27 M_{\eta}^4 M_{\eta'}^6} + \frac{29 \operatorname{Log}\left[\frac{M_K^2}{\mu^2}\right] c_{\theta}^4 M_0^8 M_K^2 M_{\pi}^4 s_{\theta}^6}{972 \pi^2 M_{\eta}^4 M_{\eta'}^6} - \\
& \frac{31 \operatorname{Log}\left[\frac{M_{\pi}^2}{\mu^2}\right] c_{\theta}^4 M_0^8 M_K^2 M_{\pi}^4 s_{\theta}^6}{216 \pi^2 M_{\eta}^4 M_{\eta'}^6} + \frac{320 c_{\theta}^4 L_6^r M_0^8 M_K^2 M_{\pi}^4 s_{\theta}^6}{9 M_{\eta}^4 M_{\eta'}^6} - \frac{256 c_{\theta}^4 L_7^r M_0^8 M_K^2 M_{\pi}^4 s_{\theta}^6}{9 M_{\eta}^4 M_{\eta'}^6} - \\
& \frac{1024 c_{\theta}^4 L_{25}^r M_0^8 M_K^2 M_{\pi}^4 s_{\theta}^6}{81 M_{\eta}^4 M_{\eta'}^6} - \frac{6656 c_{\theta}^4 C_{19} M_0^8 M_K^4 M_{\pi}^4 s_{\theta}^6}{9 M_{\eta}^4 M_{\eta'}^6} - \frac{13\,312 c_{\theta}^4 C_{31} M_0^8 M_K^4 M_{\pi}^4 s_{\theta}^6}{27 M_{\eta}^4 M_{\eta'}^6} + \\
& \frac{\operatorname{Log}\left[\frac{M_{\pi}^2}{\mu^2}\right] c_{\theta}^4 M_0^8 M_{\pi}^6 s_{\theta}^6}{24 \pi^2 M_{\eta}^4 M_{\eta'}^6} - \frac{1216 c_{\theta}^4 L_6^r M_0^8 M_{\pi}^6 s_{\theta}^6}{81 M_{\eta}^4 M_{\eta'}^6} - \frac{640 c_{\theta}^4 L_7^r M_0^8 M_{\pi}^6 s_{\theta}^6}{81 M_{\eta}^4 M_{\eta'}^6} + \frac{128 c_{\theta}^4 L_{25}^r M_0^8 M_{\pi}^6 s_{\theta}^6}{27 M_{\eta}^4 M_{\eta'}^6} + \\
& \frac{2624 c_{\theta}^4 C_{19} M_0^8 M_K^2 M_{\pi}^6 s_{\theta}^6}{9 M_{\eta}^4 M_{\eta'}^6} + \frac{5248 c_{\theta}^4 C_{31} M_0^8 M_K^2 M_{\pi}^6 s_{\theta}^6}{27 M_{\eta}^4 M_{\eta'}^6} - \frac{1216 c_{\theta}^4 C_{19} M_0^8 M_{\pi}^8 s_{\theta}^6}{27 M_{\eta}^4 M_{\eta'}^6} - \\
& \frac{2432 c_{\theta}^4 C_{31} M_0^8 M_{\pi}^8 s_{\theta}^6}{81 M_{\eta}^4 M_{\eta'}^6} - \frac{17 c_{\theta}^6 M_0^8 M_K^4 s_{\theta}^6}{486 \pi^2 M_{\eta}^2 M_{\eta'}^6} - \frac{17 \operatorname{Log}\left[\frac{M_{\eta}^2}{\mu^2}\right] c_{\theta}^6 M_0^8 M_K^4 s_{\theta}^6}{1458 \pi^2 M_{\eta}^2 M_{\eta'}^6} + \frac{8 \operatorname{Log}\left[\frac{M_{\eta'}^2}{\mu^2}\right] c_{\theta}^6 M_0^8 M_K^4 s_{\theta}^6}{243 \pi^2 M_{\eta}^2 M_{\eta'}^6} + \\
& \frac{41 c_{\theta}^6 M_0^8 M_K^2 M_{\pi}^2 s_{\theta}^6}{972 \pi^2 M_{\eta}^2 M_{\eta'}^6} - \frac{17 \operatorname{Log}\left[\frac{M_{\eta}^2}{\mu^2}\right] c_{\theta}^6 M_0^8 M_K^2 M_{\pi}^2 s_{\theta}^6}{1458 \pi^2 M_{\eta}^2 M_{\eta'}^6} - \frac{23 \operatorname{Log}\left[\frac{M_{\eta'}^2}{\mu^2}\right] c_{\theta}^6 M_0^8 M_K^2 M_{\pi}^2 s_{\theta}^6}{648 \pi^2 M_{\eta}^2 M_{\eta'}^6} - \frac{c_{\theta}^6 M_0^8 M_{\pi}^4 s_{\theta}^6}{3888 \pi^2 M_{\eta}^2 M_{\eta'}^6} + \\
& \frac{101 \operatorname{Log}\left[\frac{M_{\eta}^2}{\mu^2}\right] c_{\theta}^6 M_0^8 M_{\pi}^4 s_{\theta}^6}{11\,664 \pi^2 M_{\eta}^2 M_{\eta'}^6} + \frac{29 \operatorname{Log}\left[\frac{M_{\eta'}^2}{\mu^2}\right] c_{\theta}^6 M_0^8 M_{\pi}^4 s_{\theta}^6}{7776 \pi^2 M_{\eta}^2 M_{\eta'}^6} + \frac{1\,310\,720 c_{\theta}^6 L_8^2 r M_0^8 M_K^{10} s_{\theta}^6}{729 F^2 M_{\eta}^8 M_{\eta'}^4} - \\
& \frac{704\,512 c_{\theta}^6 L_8^2 r M_0^8 M_K^8 M_{\pi}^2 s_{\theta}^6}{243 F^2 M_{\eta}^8 M_{\eta'}^4} + \frac{237\,568 c_{\theta}^6 L_8^2 r M_0^8 M_K^6 M_{\pi}^4 s_{\theta}^6}{243 F^2 M_{\eta}^8 M_{\eta'}^4} - \frac{355\,328 c_{\theta}^6 L_8^2 r M_0^8 M_K^4 M_{\pi}^6 s_{\theta}^6}{729 F^2 M_{\eta}^8 M_{\eta'}^4} + \\
& \frac{185\,344 c_{\theta}^6 L_8^2 r M_0^8 M_K^2 M_{\pi}^8 s_{\theta}^6}{243 F^2 M_{\eta}^8 M_{\eta'}^4} - \frac{3328 c_{\theta}^6 L_8^2 r M_0^8 M_{\pi}^{10} s_{\theta}^6}{27 F^2 M_{\eta}^8 M_{\eta'}^4} - \frac{608 F^2 v_2^{(2)} c_{\theta}^4 M_0^8 M_K^4 s_{\theta}^6}{27 M_{\eta}^6 M_{\eta'}^4} + \\
& \frac{2 \operatorname{Log}\left[\frac{M_K^2}{\mu^2}\right] c_{\theta}^4 M_0^8 M_K^6 s_{\theta}^6}{243 \pi^2 M_{\eta}^6 M_{\eta'}^4} + \frac{25\,088 c_{\theta}^4 L_6^r M_0^8 M_K^6 s_{\theta}^6}{243 M_{\eta}^6 M_{\eta'}^4} + \frac{25\,088 c_{\theta}^4 L_7^r M_0^8 M_K^6 s_{\theta}^6}{243 M_{\eta}^6 M_{\eta'}^4} + \frac{512 c_{\theta}^4 L_{25}^r M_0^8 M_K^6 s_{\theta}^6}{81 M_{\eta}^6 M_{\eta'}^4} + \\
& \frac{50\,176 c_{\theta}^4 C_{19} M_0^8 M_K^8 s_{\theta}^6}{81 M_{\eta}^6 M_{\eta'}^4} + \frac{100\,352 c_{\theta}^4 C_{31} M_0^8 M_K^8 s_{\theta}^6}{243 M_{\eta}^6 M_{\eta'}^4} - \frac{104 F^2 v_2^{(2)} c_{\theta}^4 M_0^8 M_K^2 M_{\pi}^2 s_{\theta}^6}{27 M_{\eta}^6 M_{\eta'}^4} + \\
& \frac{\operatorname{Log}\left[\frac{M_K^2}{\mu^2}\right] c_{\theta}^4 M_0^8 M_K^4 M_{\pi}^2 s_{\theta}^6}{12 \pi^2 M_{\eta}^6 M_{\eta'}^4} - \frac{6656 c_{\theta}^4 L_6^r M_0^8 M_K^4 M_{\pi}^2 s_{\theta}^6}{81 M_{\eta}^6 M_{\eta'}^4} - \frac{18\,944 c_{\theta}^4 L_7^r M_0^8 M_K^4 M_{\pi}^2 s_{\theta}^6}{81 M_{\eta}^6 M_{\eta'}^4} - \\
& \frac{1984 c_{\theta}^4 L_{25}^r M_0^8 M_K^4 M_{\pi}^2 s_{\theta}^6}{81 M_{\eta}^6 M_{\eta'}^4} - \frac{85\,504 c_{\theta}^4 C_{19} M_0^8 M_K^6 M_{\pi}^2 s_{\theta}^6}{81 M_{\eta}^6 M_{\eta'}^4} - \frac{171\,008 c_{\theta}^4 C_{31} M_0^8 M_K^6 M_{\pi}^2 s_{\theta}^6}{243 M_{\eta}^6 M_{\eta'}^4} +
\end{aligned}$$



$$\begin{aligned}
& \frac{100 F^2 v_2^{(2)} c_\theta^4 M_0^8 M_\pi^4 s_\theta^6}{27 M_\eta^6 M_{\eta'}^4} - \frac{23 \text{Log}\left[\frac{M_K^2}{\mu^2}\right] c_\theta^4 M_0^8 M_K^2 M_\pi^4 s_\theta^6}{972 \pi^2 M_\eta^6 M_{\eta'}^4} + \frac{29 \text{Log}\left[\frac{M_\pi^2}{\mu^2}\right] c_\theta^4 M_0^8 M_K^2 M_\pi^4 s_\theta^6}{162 \pi^2 M_\eta^6 M_{\eta'}^4} - \\
& \frac{3328 c_\theta^4 L_6^r M_0^8 M_K^2 M_\pi^4 s_\theta^6}{81 M_\eta^6 M_{\eta'}^4} + \frac{6464 c_\theta^4 L_7^r M_0^8 M_K^2 M_\pi^4 s_\theta^6}{81 M_\eta^6 M_{\eta'}^4} + \frac{8768 c_\theta^4 L_{25}^r M_0^8 M_K^2 M_\pi^4 s_\theta^6}{81 M_\eta^6 M_{\eta'}^4} + \\
& \frac{5888 c_\theta^4 C_{19} M_0^8 M_K^4 M_\pi^4 s_\theta^6}{9 M_\eta^6 M_{\eta'}^4} + \frac{11776 c_\theta^4 C_{31} M_0^8 M_K^4 M_\pi^4 s_\theta^6}{27 M_\eta^6 M_{\eta'}^4} - \frac{29 \text{Log}\left[\frac{M_\pi^2}{\mu^2}\right] c_\theta^4 M_0^8 M_\pi^6 s_\theta^6}{648 \pi^2 M_\eta^6 M_{\eta'}^4} + \\
& \frac{3136 c_\theta^4 L_6^r M_0^8 M_\pi^6 s_\theta^6}{243 M_\eta^6 M_{\eta'}^4} - \frac{2336 c_\theta^4 L_7^r M_0^8 M_\pi^6 s_\theta^6}{243 M_\eta^6 M_{\eta'}^4} - \frac{800 c_\theta^4 L_{25}^r M_0^8 M_\pi^6 s_\theta^6}{27 M_\eta^6 M_{\eta'}^4} - \frac{21376 c_\theta^4 C_{19} M_0^8 M_K^2 M_\pi^6 s_\theta^6}{81 M_\eta^6 M_{\eta'}^4} - \\
& \frac{42752 c_\theta^4 C_{31} M_0^8 M_K^2 M_\pi^6 s_\theta^6}{243 M_\eta^6 M_{\eta'}^4} + \frac{3136 c_\theta^4 C_{19} M_0^8 M_\pi^8 s_\theta^6}{81 M_\eta^6 M_{\eta'}^4} + \frac{6272 c_\theta^4 C_{31} M_0^8 M_\pi^8 s_\theta^6}{243 M_\eta^6 M_{\eta'}^4} - \\
& \frac{8 F^2 v_2^{(2)} c_\theta^2 M_0^8 M_K^2 s_\theta^6}{3 M_\eta^4 M_{\eta'}^4} - \frac{64 F^2 v_2^{(2)} c_\theta^2 M_0^6 M_K^4 s_\theta^6}{9 M_\eta^4 M_{\eta'}^4} + \frac{c_\theta^2 M_0^8 M_K^4 s_\theta^6}{108 \pi^2 M_\eta^4 M_{\eta'}^4} + \frac{\text{Log}\left[\frac{M_K^2}{\mu^2}\right] c_\theta^2 M_0^8 M_K^4 s_\theta^6}{108 \pi^2 M_\eta^4 M_{\eta'}^4} - \\
& \frac{5 c_\theta^6 M_0^8 M_K^4 s_\theta^6}{81 \pi^2 M_\eta^4 M_{\eta'}^4} - \frac{\text{Log}\left[\frac{M_\eta^2}{\mu^2}\right] c_\theta^6 M_0^8 M_K^4 s_\theta^6}{1458 \pi^2 M_\eta^4 M_{\eta'}^4} - \frac{\text{Log}\left[\frac{M_{\eta'}^2}{\mu^2}\right] c_\theta^6 M_0^8 M_K^4 s_\theta^6}{1458 \pi^2 M_\eta^4 M_{\eta'}^4} - \frac{512 c_\theta^2 L_6^r M_0^8 M_K^4 s_\theta^6}{27 M_\eta^4 M_{\eta'}^4} - \\
& \frac{512 c_\theta^2 L_7^r M_0^8 M_K^4 s_\theta^6}{27 M_\eta^4 M_{\eta'}^4} - \frac{1792 c_\theta^2 C_{19} M_0^8 M_K^6 s_\theta^6}{9 M_\eta^4 M_{\eta'}^4} - \frac{5120 c_\theta^2 C_{31} M_0^8 M_K^6 s_\theta^6}{27 M_\eta^4 M_{\eta'}^4} + \frac{2 F^2 v_2^{(2)} c_\theta^2 M_0^8 M_\pi^2 s_\theta^6}{3 M_\eta^4 M_{\eta'}^4} - \\
& \frac{16 F^2 v_2^{(2)} c_\theta^2 M_0^6 M_K^2 M_\pi^2 s_\theta^6}{9 M_\eta^4 M_{\eta'}^4} - \frac{5 c_\theta^2 M_0^8 M_K^2 M_\pi^2 s_\theta^6}{432 \pi^2 M_\eta^4 M_{\eta'}^4} - \frac{\text{Log}\left[\frac{M_K^2}{\mu^2}\right] c_\theta^2 M_0^8 M_K^2 M_\pi^2 s_\theta^6}{72 \pi^2 M_\eta^4 M_{\eta'}^4} + \frac{4 c_\theta^6 M_0^8 M_K^2 M_\pi^2 s_\theta^6}{81 \pi^2 M_\eta^4 M_{\eta'}^4} + \\
& \frac{31 \text{Log}\left[\frac{M_\pi^2}{\mu^2}\right] c_\theta^6 M_0^8 M_K^2 M_\pi^2 s_\theta^6}{2916 \pi^2 M_\eta^4 M_{\eta'}^4} + \frac{31 \text{Log}\left[\frac{M_{\eta'}^2}{\mu^2}\right] c_\theta^6 M_0^8 M_K^2 M_\pi^2 s_\theta^6}{2916 \pi^2 M_\eta^4 M_{\eta'}^4} + \frac{448 c_\theta^2 L_6^r M_0^8 M_K^2 M_\pi^2 s_\theta^6}{27 M_\eta^4 M_{\eta'}^4} + \\
& \frac{448 c_\theta^2 L_7^r M_0^8 M_K^2 M_\pi^2 s_\theta^6}{27 M_\eta^4 M_{\eta'}^4} + \frac{896 c_\theta^2 C_{19} M_0^8 M_K^4 M_\pi^2 s_\theta^6}{3 M_\eta^4 M_{\eta'}^4} + \frac{2560 c_\theta^2 C_{31} M_0^8 M_K^4 M_\pi^2 s_\theta^6}{9 M_\eta^4 M_{\eta'}^4} + \\
& \frac{8 F^2 v_2^{(2)} c_\theta^2 M_0^6 M_\pi^4 s_\theta^6}{9 M_\eta^4 M_{\eta'}^4} + \frac{11 c_\theta^2 M_0^8 M_\pi^4 s_\theta^6}{864 \pi^2 M_\eta^4 M_{\eta'}^4} + \frac{\text{Log}\left[\frac{M_K^2}{\mu^2}\right] c_\theta^2 M_0^8 M_\pi^4 s_\theta^6}{432 \pi^2 M_\eta^4 M_{\eta'}^4} + \frac{\text{Log}\left[\frac{M_\pi^2}{\mu^2}\right] c_\theta^2 M_0^8 M_\pi^4 s_\theta^6}{72 \pi^2 M_\eta^4 M_{\eta'}^4} - \\
& \frac{17 c_\theta^6 M_0^8 M_\pi^4 s_\theta^6}{1296 \pi^2 M_\eta^4 M_{\eta'}^4} - \frac{61 \text{Log}\left[\frac{M_\eta^2}{\mu^2}\right] c_\theta^6 M_0^8 M_\pi^4 s_\theta^6}{23328 \pi^2 M_\eta^4 M_{\eta'}^4} - \frac{61 \text{Log}\left[\frac{M_{\eta'}^2}{\mu^2}\right] c_\theta^6 M_0^8 M_\pi^4 s_\theta^6}{23328 \pi^2 M_\eta^4 M_{\eta'}^4} - \frac{224 c_\theta^2 L_6^r M_0^8 M_\pi^4 s_\theta^6}{27 M_\eta^4 M_{\eta'}^4} - \\
& \frac{224 c_\theta^2 L_7^r M_0^8 M_\pi^4 s_\theta^6}{27 M_\eta^4 M_{\eta'}^4} - \frac{448 c_\theta^2 C_{19} M_0^8 M_K^2 M_\pi^4 s_\theta^6}{3 M_\eta^4 M_{\eta'}^4} - \frac{1280 c_\theta^2 C_{31} M_0^8 M_K^2 M_\pi^4 s_\theta^6}{9 M_\eta^4 M_{\eta'}^4} + \frac{112 c_\theta^2 C_{19} M_0^8 M_\pi^6 s_\theta^6}{9 M_\eta^4 M_{\eta'}^4} + \\
& \frac{320 c_\theta^2 C_{31} M_0^8 M_\pi^6 s_\theta^6}{27 M_\eta^4 M_{\eta'}^4} + \frac{\text{Log}\left[\frac{M_\eta^2}{\mu^2}\right] c_\theta^4 M_0^8 M_K^2 s_\theta^6}{72 \pi^2 M_\eta^2 M_{\eta'}^4} + \frac{\text{Log}\left[\frac{M_{\eta'}^2}{\mu^2}\right] c_\theta^4 M_0^8 M_K^2 s_\theta^6}{81 \pi^2 M_\eta^2 M_{\eta'}^4} - \frac{\text{Log}\left[\frac{M_\pi^2}{\mu^2}\right] c_\theta^4 M_0^8 M_\pi^2 s_\theta^6}{108 \pi^2 M_\eta^2 M_{\eta'}^4} -
\end{aligned}$$

$$\begin{aligned}
& \frac{13 \operatorname{Log}\left[\frac{M_\eta^2}{\mu^2}\right] c_\theta^4 M_\theta^8 M_\pi^2 s_\theta^6}{2592 \pi^2 M_\eta^2 M_{\eta'}^4} + \frac{6\,225\,920 c_\theta^6 L_8^2 r M_\theta^8 M_K^{10} s_\theta^6}{729 F^2 M_\eta^{10} M_{\eta'}^2} - \frac{5\,287\,936 c_\theta^6 L_8^2 r M_\theta^8 M_K^8 M_\pi^2 s_\theta^6}{243 F^2 M_\eta^{10} M_{\eta'}^2} + \\
& \frac{5\,005\,312 c_\theta^6 L_8^2 r M_\theta^8 M_K^6 M_\pi^4 s_\theta^6}{243 F^2 M_\eta^{10} M_{\eta'}^2} - \frac{5\,685\,248 c_\theta^6 L_8^2 r M_\theta^8 M_K^4 M_\pi^6 s_\theta^6}{729 F^2 M_\eta^{10} M_{\eta'}^2} + \frac{120\,832 c_\theta^6 L_8^2 r M_\theta^8 M_K^2 M_\pi^8 s_\theta^6}{243 F^2 M_\eta^{10} M_{\eta'}^2} - \\
& \frac{5120 c_\theta^6 L_8^2 r M_\theta^8 M_\pi^{10} s_\theta^6}{27 F^2 M_\eta^{10} M_{\eta'}^2} + \frac{320 F^2 v_2^{(2)} c_\theta^4 M_\theta^8 M_K^4 s_\theta^6}{27 M_\eta^8 M_{\eta'}^2} + \frac{7 \operatorname{Log}\left[\frac{M_K^2}{\mu^2}\right] c_\theta^4 M_\theta^8 M_K^6 s_\theta^6}{243 \pi^2 M_\eta^8 M_{\eta'}^2} - \frac{23\,552 c_\theta^4 L_6^r M_\theta^8 M_K^6 s_\theta^6}{243 M_\eta^8 M_{\eta'}^2} - \\
& \frac{23\,552 c_\theta^4 L_7^r M_\theta^8 M_K^6 s_\theta^6}{243 M_\eta^8 M_{\eta'}^2} + \frac{1792 c_\theta^4 L_{25}^r M_\theta^8 M_K^6 s_\theta^6}{81 M_\eta^8 M_{\eta'}^2} - \frac{47\,104 c_\theta^4 C_{19} M_\theta^8 M_K^6 s_\theta^6}{81 M_\eta^8 M_{\eta'}^2} - \frac{94\,208 c_\theta^4 C_{31} M_\theta^8 M_K^6 s_\theta^6}{243 M_\eta^8 M_{\eta'}^2} + \\
& \frac{128 F^2 v_2^{(2)} c_\theta^4 M_\theta^8 M_K^2 M_\pi^2 s_\theta^6}{27 M_\eta^8 M_{\eta'}^2} - \frac{35 \operatorname{Log}\left[\frac{M_K^2}{\mu^2}\right] c_\theta^4 M_\theta^8 M_K^4 M_\pi^2 s_\theta^6}{324 \pi^2 M_\eta^8 M_{\eta'}^2} + \frac{1792 c_\theta^4 L_6^r M_\theta^8 M_K^4 M_\pi^2 s_\theta^6}{27 M_\eta^8 M_{\eta'}^2} + \\
& \frac{5504 c_\theta^4 L_7^r M_\theta^8 M_K^4 M_\pi^2 s_\theta^6}{27 M_\eta^8 M_{\eta'}^2} - \frac{3200 c_\theta^4 L_{25}^r M_\theta^8 M_K^4 M_\pi^2 s_\theta^6}{81 M_\eta^8 M_{\eta'}^2} + \frac{86\,272 c_\theta^4 C_{19} M_\theta^8 M_K^4 M_\pi^2 s_\theta^6}{81 M_\eta^8 M_{\eta'}^2} + \\
& \frac{172\,544 c_\theta^4 C_{31} M_\theta^8 M_K^4 M_\pi^2 s_\theta^6}{243 M_\eta^8 M_{\eta'}^2} - \frac{16 F^2 v_2^{(2)} c_\theta^4 M_\theta^8 M_\pi^4 s_\theta^6}{27 M_\eta^8 M_{\eta'}^2} + \frac{95 \operatorname{Log}\left[\frac{M_K^2}{\mu^2}\right] c_\theta^4 M_\theta^8 M_K^2 M_\pi^4 s_\theta^6}{3888 \pi^2 M_\eta^8 M_{\eta'}^2} - \\
& \frac{65 \operatorname{Log}\left[\frac{M_\pi^2}{\mu^2}\right] c_\theta^4 M_\theta^8 M_K^2 M_\pi^4 s_\theta^6}{648 \pi^2 M_\eta^8 M_{\eta'}^2} + \frac{2912 c_\theta^4 L_6^r M_\theta^8 M_K^2 M_\pi^4 s_\theta^6}{81 M_\eta^8 M_{\eta'}^2} - \frac{6016 c_\theta^4 L_7^r M_\theta^8 M_K^2 M_\pi^4 s_\theta^6}{81 M_\eta^8 M_{\eta'}^2} - \\
& \frac{2432 c_\theta^4 L_{25}^r M_\theta^8 M_K^2 M_\pi^4 s_\theta^6}{81 M_\eta^8 M_{\eta'}^2} - \frac{2176 c_\theta^4 C_{19} M_\theta^8 M_K^2 M_\pi^4 s_\theta^6}{3 M_\eta^8 M_{\eta'}^2} - \frac{4352 c_\theta^4 C_{31} M_\theta^8 M_K^2 M_\pi^4 s_\theta^6}{9 M_\eta^8 M_{\eta'}^2} + \\
& \frac{41 \operatorname{Log}\left[\frac{M_\pi^2}{\mu^2}\right] c_\theta^4 M_\theta^8 M_\pi^6 s_\theta^6}{2592 \pi^2 M_\eta^8 M_{\eta'}^2} - \frac{2608 c_\theta^4 L_6^r M_\theta^8 M_\pi^6 s_\theta^6}{243 M_\eta^8 M_{\eta'}^2} + \frac{2432 c_\theta^4 L_7^r M_\theta^8 M_\pi^6 s_\theta^6}{243 M_\eta^8 M_{\eta'}^2} + \frac{128 c_\theta^4 L_{25}^r M_\theta^8 M_\pi^6 s_\theta^6}{27 M_\eta^8 M_{\eta'}^2} + \\
& \frac{21\,760 c_\theta^4 C_{19} M_\theta^8 M_K^6 M_\pi^6 s_\theta^6}{81 M_\eta^8 M_{\eta'}^2} + \frac{43\,520 c_\theta^4 C_{31} M_\theta^8 M_K^6 M_\pi^6 s_\theta^6}{243 M_\eta^8 M_{\eta'}^2} - \frac{2608 c_\theta^4 C_{19} M_\theta^8 M_\pi^8 s_\theta^6}{81 M_\eta^8 M_{\eta'}^2} - \\
& \frac{5216 c_\theta^4 C_{31} M_\theta^8 M_\pi^8 s_\theta^6}{243 M_\eta^8 M_{\eta'}^2} + \frac{320 F^2 v_2^{(2)} c_\theta^2 M_\theta^6 M_K^4 s_\theta^6}{27 M_\eta^6 M_{\eta'}^2} + \frac{\operatorname{Log}\left[\frac{M_K^2}{\mu^2}\right] c_\theta^2 M_\theta^8 M_K^4 s_\theta^6}{162 \pi^2 M_\eta^6 M_{\eta'}^2} - \frac{17 c_\theta^6 M_\theta^8 M_K^4 s_\theta^6}{486 \pi^2 M_\eta^6 M_{\eta'}^2} + \\
& \frac{8 \operatorname{Log}\left[\frac{M_\eta^2}{\mu^2}\right] c_\theta^6 M_\theta^8 M_K^4 s_\theta^6}{243 \pi^2 M_\eta^6 M_{\eta'}^2} - \frac{17 \operatorname{Log}\left[\frac{M_\eta^2}{\mu^2}\right] c_\theta^6 M_\theta^8 M_K^4 s_\theta^6}{1458 \pi^2 M_\eta^6 M_{\eta'}^2} + \frac{2560 c_\theta^2 L_6^r M_\theta^8 M_K^4 s_\theta^6}{81 M_\eta^6 M_{\eta'}^2} + \\
& \frac{2560 c_\theta^2 L_7^r M_\theta^8 M_K^4 s_\theta^6}{81 M_\eta^6 M_{\eta'}^2} + \frac{8960 c_\theta^2 C_{19} M_\theta^8 M_K^6 s_\theta^6}{27 M_\eta^6 M_{\eta'}^2} + \frac{25\,600 c_\theta^2 C_{31} M_\theta^8 M_K^6 s_\theta^6}{81 M_\eta^6 M_{\eta'}^2} - \frac{4 F^2 v_2^{(2)} c_\theta^2 M_\theta^8 M_\pi^2 s_\theta^6}{M_\eta^6 M_{\eta'}^2} + \\
& \frac{32 F^2 v_2^{(2)} c_\theta^2 M_\theta^6 M_K^2 M_\pi^2 s_\theta^6}{27 M_\eta^6 M_{\eta'}^2} + \frac{5 c_\theta^2 M_\theta^8 M_K^2 M_\pi^2 s_\theta^6}{216 \pi^2 M_\eta^6 M_{\eta'}^2} + \frac{\operatorname{Log}\left[\frac{M_K^2}{\mu^2}\right] c_\theta^2 M_\theta^8 M_K^2 M_\pi^2 s_\theta^6}{36 \pi^2 M_\eta^6 M_{\eta'}^2} + \frac{41 c_\theta^6 M_\theta^8 M_K^2 M_\pi^2 s_\theta^6}{972 \pi^2 M_\eta^6 M_{\eta'}^2} -
\end{aligned}$$

$$\begin{aligned}
& \frac{23 \operatorname{Log} \left[ \frac{M_\eta^2}{\mu^2} \right] c_\theta^6 M_0^8 M_K^2 M_\pi^2 s_\theta^6}{648 \pi^2 M_\eta^6 M_{\eta'}^2} - \frac{17 \operatorname{Log} \left[ \frac{M_{\eta'}^2}{\mu^2} \right] c_\theta^6 M_0^8 M_K^2 M_\pi^2 s_\theta^6}{1458 \pi^2 M_\eta^6 M_{\eta'}^2} - \frac{3200 c_\theta^2 L_6^r M_0^8 M_K^2 M_\pi^2 s_\theta^6}{81 M_\eta^6 M_{\eta'}^2} \\
& \frac{3200 c_\theta^2 L_7^r M_0^8 M_K^2 M_\pi^2 s_\theta^6}{81 M_\eta^6 M_{\eta'}^2} - \frac{4480 c_\theta^2 C_{19} M_0^8 M_K^4 M_\pi^2 s_\theta^6}{9 M_\eta^6 M_{\eta'}^2} - \frac{12\,800 c_\theta^2 C_{31} M_0^8 M_K^4 M_\pi^2 s_\theta^6}{27 M_\eta^6 M_{\eta'}^2} - \\
& \frac{64 F^2 v_2^{(2)} c_\theta^2 M_0^6 M_\pi^4 s_\theta^6}{27 M_\eta^6 M_{\eta'}^2} - \frac{5 c_\theta^2 M_0^8 M_\pi^4 s_\theta^6}{432 \pi^2 M_\eta^6 M_{\eta'}^2} - \frac{\operatorname{Log} \left[ \frac{M_K^2}{\mu^2} \right] c_\theta^2 M_0^8 M_\pi^4 s_\theta^6}{216 \pi^2 M_\eta^6 M_{\eta'}^2} - \frac{\operatorname{Log} \left[ \frac{M_\pi^2}{\mu^2} \right] c_\theta^2 M_0^8 M_\pi^4 s_\theta^6}{108 \pi^2 M_\eta^6 M_{\eta'}^2} - \\
& \frac{c_\theta^6 M_0^8 M_\pi^4 s_\theta^6}{3888 \pi^2 M_\eta^6 M_{\eta'}^2} + \frac{29 \operatorname{Log} \left[ \frac{M_\eta^2}{\mu^2} \right] c_\theta^6 M_0^8 M_\pi^4 s_\theta^6}{7776 \pi^2 M_\eta^6 M_{\eta'}^2} + \frac{101 \operatorname{Log} \left[ \frac{M_{\eta'}^2}{\mu^2} \right] c_\theta^6 M_0^8 M_\pi^4 s_\theta^6}{11\,664 \pi^2 M_\eta^6 M_{\eta'}^2} + \frac{1216 c_\theta^2 L_6^r M_0^8 M_\pi^4 s_\theta^6}{81 M_\eta^6 M_{\eta'}^2} + \\
& \frac{1216 c_\theta^2 L_7^r M_0^8 M_\pi^4 s_\theta^6}{81 M_\eta^6 M_{\eta'}^2} + \frac{2240 c_\theta^2 C_{19} M_0^8 M_K^2 M_\pi^4 s_\theta^6}{9 M_\eta^6 M_{\eta'}^2} + \frac{6400 c_\theta^2 C_{31} M_0^8 M_K^2 M_\pi^4 s_\theta^6}{27 M_\eta^6 M_{\eta'}^2} - \frac{896 c_\theta^2 C_{19} M_0^8 M_\pi^6 s_\theta^6}{27 M_\eta^6 M_{\eta'}^2} - \\
& \frac{2560 c_\theta^2 C_{31} M_0^8 M_\pi^6 s_\theta^6}{81 M_\eta^6 M_{\eta'}^2} - \frac{5 \operatorname{Log} \left[ \frac{M_\eta^2}{\mu^2} \right] c_\theta^4 M_0^8 M_K^2 s_\theta^6}{243 \pi^2 M_\eta^4 M_{\eta'}^2} - \frac{\operatorname{Log} \left[ \frac{M_{\eta'}^2}{\mu^2} \right] c_\theta^4 M_0^8 M_K^2 s_\theta^6}{54 \pi^2 M_\eta^4 M_{\eta'}^2} + \frac{25 \operatorname{Log} \left[ \frac{M_\eta^2}{\mu^2} \right] c_\theta^4 M_0^8 M_\pi^2 s_\theta^6}{1944 \pi^2 M_\eta^4 M_{\eta'}^2} + \\
& \frac{19 \operatorname{Log} \left[ \frac{M_{\eta'}^2}{\mu^2} \right] c_\theta^4 M_0^8 M_\pi^2 s_\theta^6}{1728 \pi^2 M_\eta^4 M_{\eta'}^2} + \frac{10 \operatorname{Log} \left[ \frac{M_{\eta'}^2}{\mu^2} \right] c_\theta^6 M_0^8 M_K^4 M_{\eta'}^2 s_\theta^6}{729 \pi^2 M_\eta^{10}} - \frac{97 \operatorname{Log} \left[ \frac{M_{\eta'}^2}{\mu^2} \right] c_\theta^6 M_0^8 M_K^2 M_\pi^2 M_{\eta'}^2 s_\theta^6}{5832 \pi^2 M_\eta^{10}} + \\
& \frac{77 \operatorname{Log} \left[ \frac{M_{\eta'}^2}{\mu^2} \right] c_\theta^6 M_0^8 M_\pi^4 M_{\eta'}^2 s_\theta^6}{23\,328 \pi^2 M_\eta^{10}} - \frac{\operatorname{Log} \left[ \frac{M_{\eta'}^2}{\mu^2} \right] c_\theta^4 M_0^8 M_K^2 M_{\eta'}^2 s_\theta^6}{324 \pi^2 M_\eta^8} + \frac{19 \operatorname{Log} \left[ \frac{M_{\eta'}^2}{\mu^2} \right] c_\theta^4 M_0^8 M_\pi^2 M_{\eta'}^2 s_\theta^6}{10\,368 \pi^2 M_\eta^8} - \\
& \frac{5 \operatorname{Log} \left[ \frac{M_\eta^2}{\mu^2} \right] c_\theta^6 M_0^8 M_K^4 s_\theta^6}{243 \pi^2 M_\eta^6 (M_\eta^2 - M_{\eta'}^2)} - \frac{4 \operatorname{Log} \left[ \frac{M_{\eta'}^2}{\mu^2} \right] c_\theta^6 M_0^8 M_K^4 s_\theta^6}{243 \pi^2 M_\eta^6 (M_\eta^2 - M_{\eta'}^2)} + \frac{11 \operatorname{Log} \left[ \frac{M_\eta^2}{\mu^2} \right] c_\theta^6 M_0^8 M_K^2 M_\pi^2 s_\theta^6}{486 \pi^2 M_\eta^6 (M_\eta^2 - M_{\eta'}^2)} + \\
& \frac{23 \operatorname{Log} \left[ \frac{M_{\eta'}^2}{\mu^2} \right] c_\theta^6 M_0^8 M_K^2 M_\pi^2 s_\theta^6}{972 \pi^2 M_\eta^6 (M_\eta^2 - M_{\eta'}^2)} - \frac{59 \operatorname{Log} \left[ \frac{M_\eta^2}{\mu^2} \right] c_\theta^6 M_0^8 M_\pi^4 s_\theta^6}{15\,552 \pi^2 M_\eta^6 (M_\eta^2 - M_{\eta'}^2)} - \frac{19 \operatorname{Log} \left[ \frac{M_{\eta'}^2}{\mu^2} \right] c_\theta^6 M_0^8 M_\pi^4 s_\theta^6}{3888 \pi^2 M_\eta^6 (M_\eta^2 - M_{\eta'}^2)} - \\
& \frac{5 \operatorname{Log} \left[ \frac{M_\eta^2}{\mu^2} \right] c_\theta^6 M_0^8 M_K^4 M_{\eta'}^2 s_\theta^6}{243 \pi^2 M_\eta^8 (M_\eta^2 - M_{\eta'}^2)} + \frac{11 \operatorname{Log} \left[ \frac{M_\eta^2}{\mu^2} \right] c_\theta^6 M_0^8 M_K^2 M_\pi^2 M_{\eta'}^2 s_\theta^6}{486 \pi^2 M_\eta^8 (M_\eta^2 - M_{\eta'}^2)} - \frac{59 \operatorname{Log} \left[ \frac{M_\eta^2}{\mu^2} \right] c_\theta^6 M_0^8 M_\pi^4 M_{\eta'}^2 s_\theta^6}{15\,552 \pi^2 M_\eta^8 (M_\eta^2 - M_{\eta'}^2)} + \\
& \frac{4 \operatorname{Log} \left[ \frac{M_\eta^2}{\mu^2} \right] c_\theta^6 M_0^8 M_K^4 s_\theta^6}{243 \pi^2 M_\eta^6 (M_\eta^2 - M_{\eta'}^2)} + \frac{5 \operatorname{Log} \left[ \frac{M_{\eta'}^2}{\mu^2} \right] c_\theta^6 M_0^8 M_K^4 s_\theta^6}{243 \pi^2 M_\eta^6 (M_\eta^2 - M_{\eta'}^2)} - \frac{23 \operatorname{Log} \left[ \frac{M_\eta^2}{\mu^2} \right] c_\theta^6 M_0^8 M_K^2 M_\pi^2 s_\theta^6}{972 \pi^2 M_\eta^6 (M_\eta^2 - M_{\eta'}^2)} - \\
& \frac{11 \operatorname{Log} \left[ \frac{M_{\eta'}^2}{\mu^2} \right] c_\theta^6 M_0^8 M_K^2 M_\pi^2 s_\theta^6}{486 \pi^2 M_\eta^6 (M_\eta^2 - M_{\eta'}^2)} + \frac{19 \operatorname{Log} \left[ \frac{M_\eta^2}{\mu^2} \right] c_\theta^6 M_0^8 M_\pi^4 s_\theta^6}{3888 \pi^2 M_\eta^6 (M_\eta^2 - M_{\eta'}^2)} + \frac{59 \operatorname{Log} \left[ \frac{M_{\eta'}^2}{\mu^2} \right] c_\theta^6 M_0^8 M_\pi^4 s_\theta^6}{15\,552 \pi^2 M_\eta^6 (M_\eta^2 - M_{\eta'}^2)} + \\
& \frac{\operatorname{Log} \left[ \frac{M_\eta^2}{\mu^2} \right] c_\theta^6 M_0^8 M_K^4 s_\theta^6}{162 \pi^2 M_\eta^2 M_{\eta'}^4 (M_\eta^2 - M_{\eta'}^2)} - \frac{4 \operatorname{Log} \left[ \frac{M_{\eta'}^2}{\mu^2} \right] c_\theta^6 M_0^8 M_K^4 s_\theta^6}{243 \pi^2 M_\eta^2 M_{\eta'}^4 (M_\eta^2 - M_{\eta'}^2)} + \frac{\operatorname{Log} \left[ \frac{M_\eta^2}{\mu^2} \right] c_\theta^6 M_0^8 M_K^2 M_\pi^2 s_\theta^6}{162 \pi^2 M_\eta^2 M_{\eta'}^4 (M_\eta^2 - M_{\eta'}^2)} +
\end{aligned}$$

$$\begin{aligned}
& \frac{23 \operatorname{Log}\left[\frac{M_\eta^2}{\mu^2}\right] c_\theta^6 M_\theta^8 M_K^2 M_\pi^2 s_\theta^6}{972 \pi^2 M_\eta^2 M_\eta^4 (M_\eta^2 - M_\eta'^2)} - \frac{11 \operatorname{Log}\left[\frac{M_\eta^2}{\mu^2}\right] c_\theta^6 M_\theta^8 M_\pi^4 s_\theta^6}{2592 \pi^2 M_\eta^2 M_\eta^4 (M_\eta^2 - M_\eta'^2)} - \frac{19 \operatorname{Log}\left[\frac{M_\eta^2}{\mu^2}\right] c_\theta^6 M_\theta^8 M_\pi^4 s_\theta^6}{3888 \pi^2 M_\eta^2 M_\eta^4 (M_\eta^2 - M_\eta'^2)} + \\
& \frac{4 \operatorname{Log}\left[\frac{M_\eta^2}{\mu^2}\right] c_\theta^6 M_\theta^8 M_K^4 s_\theta^6}{243 \pi^2 M_\eta^4 M_\eta^2 (M_\eta^2 - M_\eta'^2)} - \frac{\operatorname{Log}\left[\frac{M_\eta^2}{\mu^2}\right] c_\theta^6 M_\theta^8 M_K^4 s_\theta^6}{162 \pi^2 M_\eta^4 M_\eta^2 (M_\eta^2 - M_\eta'^2)} - \frac{23 \operatorname{Log}\left[\frac{M_\eta^2}{\mu^2}\right] c_\theta^6 M_\theta^8 M_K^2 M_\pi^2 s_\theta^6}{972 \pi^2 M_\eta^4 M_\eta^2 (M_\eta^2 - M_\eta'^2)} - \\
& \frac{\operatorname{Log}\left[\frac{M_\eta^2}{\mu^2}\right] c_\theta^6 M_\theta^8 M_K^2 M_\pi^2 s_\theta^6}{162 \pi^2 M_\eta^4 M_\eta^2 (M_\eta^2 - M_\eta'^2)} + \frac{19 \operatorname{Log}\left[\frac{M_\eta^2}{\mu^2}\right] c_\theta^6 M_\theta^8 M_\pi^4 s_\theta^6}{3888 \pi^2 M_\eta^4 M_\eta^2 (M_\eta^2 - M_\eta'^2)} + \frac{11 \operatorname{Log}\left[\frac{M_\eta^2}{\mu^2}\right] c_\theta^6 M_\theta^8 M_\pi^4 s_\theta^6}{2592 \pi^2 M_\eta^4 M_\eta^2 (M_\eta^2 - M_\eta'^2)} + \\
& \frac{5 \operatorname{Log}\left[\frac{M_\eta^2}{\mu^2}\right] c_\theta^6 M_\theta^8 M_K^4 M_\eta^2 s_\theta^6}{243 \pi^2 M_\eta^8 (M_\eta^2 - M_\eta'^2)} - \frac{11 \operatorname{Log}\left[\frac{M_\eta^2}{\mu^2}\right] c_\theta^6 M_\theta^8 M_K^2 M_\pi^2 M_\eta^2 s_\theta^6}{486 \pi^2 M_\eta^8 (M_\eta^2 - M_\eta'^2)} + \frac{59 \operatorname{Log}\left[\frac{M_\eta^2}{\mu^2}\right] c_\theta^6 M_\theta^8 M_\pi^4 M_\eta^2 s_\theta^6}{15552 \pi^2 M_\eta^8 (M_\eta^2 - M_\eta'^2)} - \\
& \frac{9175040 \sqrt{2} c_\theta^5 L_8^2 r M_\theta^8 M_K^{10} s_\theta^7}{729 F^2 M_\eta^{12}} + \frac{7577600 \sqrt{2} c_\theta^5 L_8^2 r M_\theta^8 M_K^8 M_\pi^2 s_\theta^7}{243 F^2 M_\eta^{12}} - \\
& \frac{7290880 \sqrt{2} c_\theta^5 L_8^2 r M_\theta^8 M_K^6 M_\pi^4 s_\theta^7}{243 F^2 M_\eta^{12}} + \frac{10311680 \sqrt{2} c_\theta^5 L_8^2 r M_\theta^8 M_K^4 M_\pi^6 s_\theta^7}{729 F^2 M_\eta^{12}} - \\
& \frac{819200 \sqrt{2} c_\theta^5 L_8^2 r M_\theta^8 M_K^2 M_\pi^8 s_\theta^7}{243 F^2 M_\eta^{12}} + \frac{35840 \sqrt{2} c_\theta^5 L_8^2 r M_\theta^8 M_\pi^{10} s_\theta^7}{81 F^2 M_\eta^{12}} + \frac{128 \sqrt{2} F^2 v_2^{(2)} c_\theta^5 M_\theta^8 M_K^4 s_\theta^7}{27 M_\eta^{10}} - \\
& \frac{20 \sqrt{2} \operatorname{Log}\left[\frac{M_K^2}{\mu^2}\right] c_\theta^3 M_\theta^8 M_K^6 s_\theta^7}{243 \pi^2 M_\eta^{10}} + \frac{10240 \sqrt{2} c_\theta^3 L_6^r M_\theta^8 M_K^6 s_\theta^7}{243 M_\eta^{10}} + \frac{10240 \sqrt{2} c_\theta^3 L_7^r M_\theta^8 M_K^6 s_\theta^7}{243 M_\eta^{10}} - \\
& \frac{5120 \sqrt{2} c_\theta^3 L_{25}^r M_\theta^8 M_K^6 s_\theta^7}{81 M_\eta^{10}} + \frac{20480 \sqrt{2} c_\theta^3 C_{19} M_\theta^8 M_K^8 s_\theta^7}{81 M_\eta^{10}} + \frac{40960 \sqrt{2} c_\theta^3 C_{31} M_\theta^8 M_K^8 s_\theta^7}{243 M_\eta^{10}} - \\
& \frac{16 \sqrt{2} F^2 v_2^{(2)} c_\theta^3 M_\theta^8 M_K^2 M_\pi^2 s_\theta^7}{27 M_\eta^{10}} + \frac{5 \sqrt{2} \operatorname{Log}\left[\frac{M_K^2}{\mu^2}\right] c_\theta^3 M_\theta^8 M_K^4 M_\pi^2 s_\theta^7}{81 \pi^2 M_\eta^{10}} - \frac{1792 \sqrt{2} c_\theta^3 L_6^r M_\theta^8 M_K^4 M_\pi^2 s_\theta^7}{81 M_\eta^{10}} - \\
& \frac{3328 \sqrt{2} c_\theta^3 L_7^r M_\theta^8 M_K^4 M_\pi^2 s_\theta^7}{81 M_\eta^{10}} + \frac{7168 \sqrt{2} c_\theta^3 L_{25}^r M_\theta^8 M_K^4 M_\pi^2 s_\theta^7}{81 M_\eta^{10}} - \frac{40448 \sqrt{2} c_\theta^3 C_{19} M_\theta^8 M_K^6 M_\pi^2 s_\theta^7}{81 M_\eta^{10}} - \\
& \frac{80896 \sqrt{2} c_\theta^3 C_{31} M_\theta^8 M_K^6 M_\pi^2 s_\theta^7}{243 M_\eta^{10}} - \frac{40 \sqrt{2} F^2 v_2^{(2)} c_\theta^3 M_\theta^8 M_\pi^4 s_\theta^7}{27 M_\eta^{10}} - \frac{\operatorname{Log}\left[\frac{M_K^2}{\mu^2}\right] c_\theta^3 M_\theta^8 M_K^2 M_\pi^4 s_\theta^7}{81 \sqrt{2} \pi^2 M_\eta^{10}} - \\
& \frac{\sqrt{2} \operatorname{Log}\left[\frac{M_K^2}{\mu^2}\right] c_\theta^3 M_\theta^8 M_K^2 M_\pi^4 s_\theta^7}{243 \pi^2 M_\eta^{10}} - \frac{\operatorname{Log}\left[\frac{M_\pi^2}{\mu^2}\right] c_\theta^3 M_\theta^8 M_K^2 M_\pi^4 s_\theta^7}{81 \sqrt{2} \pi^2 M_\eta^{10}} + \frac{\sqrt{2} \operatorname{Log}\left[\frac{M_\pi^2}{\mu^2}\right] c_\theta^3 M_\theta^8 M_K^2 M_\pi^4 s_\theta^7}{81 \pi^2 M_\eta^{10}} - \\
& \frac{1280 \sqrt{2} c_\theta^3 L_6^r M_\theta^8 M_K^2 M_\pi^4 s_\theta^7}{81 M_\eta^{10}} + \frac{1024 \sqrt{2} c_\theta^3 L_7^r M_\theta^8 M_K^2 M_\pi^4 s_\theta^7}{81 M_\eta^{10}} - \frac{3584 \sqrt{2} c_\theta^3 L_{25}^r M_\theta^8 M_K^2 M_\pi^4 s_\theta^7}{81 M_\eta^{10}} + \\
& \frac{3328 \sqrt{2} c_\theta^3 C_{19} M_\theta^8 M_K^4 M_\pi^4 s_\theta^7}{9 M_\eta^{10}} + \frac{6656 \sqrt{2} c_\theta^3 C_{31} M_\theta^8 M_K^4 M_\pi^4 s_\theta^7}{27 M_\eta^{10}} + \frac{\sqrt{2} \operatorname{Log}\left[\frac{M_\pi^2}{\mu^2}\right] c_\theta^3 M_\theta^8 M_\pi^6 s_\theta^7}{81 \pi^2 M_\eta^{10}} +
\end{aligned}$$

$$\begin{aligned}
& \frac{704 \sqrt{2} c_\theta^3 L_6^r M_0^8 M_\pi^6 s_\theta^7}{243 M_\eta^{10}} - \frac{1600 \sqrt{2} c_\theta^3 L_7^r M_0^8 M_\pi^6 s_\theta^7}{243 M_\eta^{10}} + \frac{320 \sqrt{2} c_\theta^3 L_{25}^r M_0^8 M_\pi^6 s_\theta^7}{27 M_\eta^{10}} - \\
& \frac{10112 \sqrt{2} c_\theta^3 C_{19} M_0^8 M_K^2 M_\pi^6 s_\theta^7}{81 M_\eta^{10}} - \frac{20224 \sqrt{2} c_\theta^3 C_{31} M_0^8 M_K^2 M_\pi^6 s_\theta^7}{243 M_\eta^{10}} + \frac{704 \sqrt{2} c_\theta^3 C_{19} M_0^8 M_\pi^8 s_\theta^7}{81 M_\eta^{10}} + \\
& \frac{1408 \sqrt{2} c_\theta^3 C_{31} M_0^8 M_\pi^8 s_\theta^7}{243 M_\eta^{10}} - \frac{8 \sqrt{2} F^2 v_2^{(2)} c_\theta M_0^8 M_K^2 s_\theta^7}{3 M_\eta^8} - \frac{64 \sqrt{2} F^2 v_2^{(2)} c_\theta M_0^6 M_K^4 s_\theta^7}{27 M_\eta^8} - \\
& \frac{c_\theta M_0^8 M_K^4 s_\theta^7}{162 \sqrt{2} \pi^2 M_\eta^8} + \frac{\sqrt{2} c_\theta M_0^8 M_K^4 s_\theta^7}{81 \pi^2 M_\eta^8} + \frac{\sqrt{2} \text{Log} \left[ \frac{M_K^2}{\mu^2} \right] c_\theta M_0^8 M_K^4 s_\theta^7}{81 \pi^2 M_\eta^8} + \frac{61 c_\theta^5 M_0^8 M_K^4 s_\theta^7}{243 \sqrt{2} \pi^2 M_\eta^8} - \\
& \frac{28 \sqrt{2} \text{Log} \left[ \frac{M_\eta^2}{\mu^2} \right] c_\theta^5 M_0^8 M_K^4 s_\theta^7}{729 \pi^2 M_\eta^8} + \frac{5 \text{Log} \left[ \frac{M_\eta^2}{\mu^2} \right] c_\theta^5 M_0^8 M_K^4 s_\theta^7}{243 \sqrt{2} \pi^2 M_\eta^8} - \frac{20 \sqrt{2} \text{Log} \left[ \frac{M_\eta^2}{\mu^2} \right] c_\theta^5 M_0^8 M_K^4 s_\theta^7}{243 \pi^2 M_\eta^8} - \\
& \frac{512 \sqrt{2} c_\theta L_6^r M_0^8 M_K^4 s_\theta^7}{81 M_\eta^8} - \frac{512 \sqrt{2} c_\theta L_7^r M_0^8 M_K^4 s_\theta^7}{81 M_\eta^8} - \frac{1792 \sqrt{2} c_\theta C_{19} M_0^8 M_K^6 s_\theta^7}{27 M_\eta^8} - \\
& \frac{5120 \sqrt{2} c_\theta C_{31} M_0^8 M_K^6 s_\theta^7}{81 M_\eta^8} + \frac{8 \sqrt{2} F^2 v_2^{(2)} c_\theta M_0^8 M_\pi^2 s_\theta^7}{3 M_\eta^8} + \frac{32 \sqrt{2} F^2 v_2^{(2)} c_\theta M_0^6 M_K^2 M_\pi^2 s_\theta^7}{27 M_\eta^8} - \\
& \frac{c_\theta M_0^8 M_K^2 M_\pi^2 s_\theta^7}{108 \sqrt{2} \pi^2 M_\eta^8} - \frac{\text{Log} \left[ \frac{M_K^2}{\mu^2} \right] c_\theta M_0^8 M_K^2 M_\pi^2 s_\theta^7}{81 \sqrt{2} \pi^2 M_\eta^8} - \frac{28 \sqrt{2} c_\theta^5 M_0^8 M_K^2 M_\pi^2 s_\theta^7}{243 \pi^2 M_\eta^8} + \frac{5 \text{Log} \left[ \frac{M_\eta^2}{\mu^2} \right] c_\theta^5 M_0^8 M_K^2 M_\pi^2 s_\theta^7}{486 \sqrt{2} \pi^2 M_\eta^8} + \\
& \frac{23 \sqrt{2} \text{Log} \left[ \frac{M_\eta^2}{\mu^2} \right] c_\theta^5 M_0^8 M_K^2 M_\pi^2 s_\theta^7}{729 \pi^2 M_\eta^8} + \frac{\text{Log} \left[ \frac{M_\eta^2}{\mu^2} \right] c_\theta^5 M_0^8 M_K^2 M_\pi^2 s_\theta^7}{54 \sqrt{2} \pi^2 M_\eta^8} + \frac{2 \sqrt{2} \text{Log} \left[ \frac{M_\eta^2}{\mu^2} \right] c_\theta^5 M_0^8 M_K^2 M_\pi^2 s_\theta^7}{243 \pi^2 M_\eta^8} + \\
& \frac{256 \sqrt{2} c_\theta L_6^r M_0^8 M_K^2 M_\pi^2 s_\theta^7}{81 M_\eta^8} + \frac{256 \sqrt{2} c_\theta L_7^r M_0^8 M_K^2 M_\pi^2 s_\theta^7}{81 M_\eta^8} + \frac{896 \sqrt{2} c_\theta C_{19} M_0^8 M_K^4 M_\pi^2 s_\theta^7}{9 M_\eta^8} + \\
& \frac{2560 \sqrt{2} c_\theta C_{31} M_0^8 M_K^4 M_\pi^2 s_\theta^7}{27 M_\eta^8} + \frac{32 \sqrt{2} F^2 v_2^{(2)} c_\theta M_0^6 M_\pi^4 s_\theta^7}{27 M_\eta^8} - \frac{c_\theta M_0^8 M_\pi^4 s_\theta^7}{72 \sqrt{2} \pi^2 M_\eta^8} - \\
& \frac{\text{Log} \left[ \frac{M_\pi^2}{\mu^2} \right] c_\theta M_0^8 M_\pi^4 s_\theta^7}{54 \sqrt{2} \pi^2 M_\eta^8} - \frac{43 c_\theta^5 M_0^8 M_\pi^4 s_\theta^7}{3888 \sqrt{2} \pi^2 M_\eta^8} + \frac{7 \sqrt{2} c_\theta^5 M_0^8 M_\pi^4 s_\theta^7}{243 \pi^2 M_\eta^8} + \frac{11 \text{Log} \left[ \frac{M_\pi^2}{\mu^2} \right] c_\theta^5 M_0^8 M_\pi^4 s_\theta^7}{243 \sqrt{2} \pi^2 M_\eta^8} - \\
& \frac{22 \sqrt{2} \text{Log} \left[ \frac{M_\pi^2}{\mu^2} \right] c_\theta^5 M_0^8 M_\pi^4 s_\theta^7}{729 \pi^2 M_\eta^8} + \frac{5 \text{Log} \left[ \frac{M_\pi^2}{\mu^2} \right] c_\theta^5 M_0^8 M_\pi^4 s_\theta^7}{3888 \sqrt{2} \pi^2 M_\eta^8} + \frac{\sqrt{2} \text{Log} \left[ \frac{M_\pi^2}{\mu^2} \right] c_\theta^5 M_0^8 M_\pi^4 s_\theta^7}{243 \pi^2 M_\eta^8} + \\
& \frac{256 \sqrt{2} c_\theta L_6^r M_0^8 M_\pi^4 s_\theta^7}{81 M_\eta^8} + \frac{256 \sqrt{2} c_\theta L_7^r M_0^8 M_\pi^4 s_\theta^7}{81 M_\eta^8} - \frac{448 \sqrt{2} c_\theta C_{19} M_0^8 M_K^2 M_\pi^4 s_\theta^7}{9 M_\eta^8} - \\
& \frac{1280 \sqrt{2} c_\theta C_{31} M_0^8 M_K^2 M_\pi^4 s_\theta^7}{27 M_\eta^8} + \frac{448 \sqrt{2} c_\theta C_{19} M_0^8 M_\pi^6 s_\theta^7}{27 M_\eta^8} + \frac{1280 \sqrt{2} c_\theta C_{31} M_0^8 M_\pi^6 s_\theta^7}{81 M_\eta^8} +
\end{aligned}$$

$$\begin{aligned}
& \frac{5 \operatorname{Log}\left[\frac{M_\eta^2}{\mu^2}\right] c_\theta^3 M_0^8 M_K^2 s_\theta^7}{243 \sqrt{2} \pi^2 M_\eta^6} + \frac{\operatorname{Log}\left[\frac{M_{\eta'}^2}{\mu^2}\right] c_\theta^3 M_0^8 M_K^2 s_\theta^7}{162 \sqrt{2} \pi^2 M_\eta^6} - \frac{25 \operatorname{Log}\left[\frac{M_\eta^2}{\mu^2}\right] c_\theta^3 M_0^8 M_\pi^2 s_\theta^7}{1944 \sqrt{2} \pi^2 M_\eta^6} - \\
& \frac{5 \operatorname{Log}\left[\frac{M_\eta^2}{\mu^2}\right] c_\theta^3 M_0^8 M_\pi^2 s_\theta^7}{1296 \sqrt{2} \pi^2 M_\eta^6} + \frac{2\,621\,440 \sqrt{2} c_\theta^5 L_8^2 r M_0^8 M_K^{10} s_\theta^7}{729 F^2 M_\eta^{12}} - \frac{81\,920 \sqrt{2} c_\theta^5 L_8^2 r M_0^8 M_K^8 M_\pi^2 s_\theta^7}{9 F^2 M_\eta^{12}} + \\
& \frac{2\,293\,760 \sqrt{2} c_\theta^5 L_8^2 r M_0^8 M_K^6 M_\pi^4 s_\theta^7}{243 F^2 M_\eta^{12}} - \frac{3\,696\,640 \sqrt{2} c_\theta^5 L_8^2 r M_0^8 M_K^4 M_\pi^6 s_\theta^7}{729 F^2 M_\eta^{12}} + \\
& \frac{112\,640 \sqrt{2} c_\theta^5 L_8^2 r M_0^8 M_K^2 M_\pi^8 s_\theta^7}{81 F^2 M_\eta^{12}} - \frac{12\,800 \sqrt{2} c_\theta^5 L_8^2 r M_0^8 M_\pi^{10} s_\theta^7}{81 F^2 M_\eta^{12}} + \frac{5\,242\,880 \sqrt{2} c_\theta^5 L_8^2 r M_0^8 M_K^{10} s_\theta^7}{729 F^2 M_\eta^2 M_\eta^{10}} - \\
& \frac{4\,136\,960 \sqrt{2} c_\theta^5 L_8^2 r M_0^8 M_K^8 M_\pi^2 s_\theta^7}{243 F^2 M_\eta^2 M_\eta^{10}} + \frac{1\,097\,728 \sqrt{2} c_\theta^5 L_8^2 r M_0^8 M_K^6 M_\pi^4 s_\theta^7}{81 F^2 M_\eta^2 M_\eta^{10}} - \\
& \frac{2\,797\,568 \sqrt{2} c_\theta^5 L_8^2 r M_0^8 M_K^4 M_\pi^6 s_\theta^7}{729 F^2 M_\eta^2 M_\eta^{10}} + \frac{47\,104 \sqrt{2} c_\theta^5 L_8^2 r M_0^8 M_K^2 M_\pi^8 s_\theta^7}{243 F^2 M_\eta^2 M_\eta^{10}} - \\
& \frac{3584 \sqrt{2} c_\theta^5 L_8^2 r M_0^8 M_\pi^{10} s_\theta^7}{27 F^2 M_\eta^2 M_\eta^{10}} + \frac{4 \sqrt{2} \operatorname{Log}\left[\frac{M_\eta^2}{\mu^2}\right] c_\theta^5 M_0^8 M_K^4 M_\eta^2 s_\theta^7}{729 \pi^2 M_\eta^{10}} + \frac{7 \operatorname{Log}\left[\frac{M_\eta^2}{\mu^2}\right] c_\theta^5 M_0^8 M_K^2 M_\pi^2 M_\eta^2 s_\theta^7}{1458 \sqrt{2} \pi^2 M_\eta^{10}} - \\
& \frac{2 \sqrt{2} \operatorname{Log}\left[\frac{M_\eta^2}{\mu^2}\right] c_\theta^5 M_0^8 M_K^2 M_\pi^2 M_\eta^2 s_\theta^7}{243 \pi^2 M_\eta^{10}} + \frac{13 \operatorname{Log}\left[\frac{M_\eta^2}{\mu^2}\right] c_\theta^5 M_0^8 M_\pi^4 M_\eta^2 s_\theta^7}{5832 \sqrt{2} \pi^2 M_\eta^{10}} - \frac{7 \sqrt{2} c_\theta^5 M_0^8 M_K^4 s_\theta^7}{243 \pi^2 M_\eta^8} - \\
& \frac{11 \sqrt{2} \operatorname{Log}\left[\frac{M_\eta^2}{\mu^2}\right] c_\theta^5 M_0^8 M_K^4 s_\theta^7}{243 \pi^2 M_\eta^8} + \frac{8 \sqrt{2} \operatorname{Log}\left[\frac{M_{\eta'}^2}{\mu^2}\right] c_\theta^5 M_0^8 M_K^4 s_\theta^7}{729 \pi^2 M_\eta^8} + \frac{8 \sqrt{2} c_\theta^5 M_0^8 M_K^2 M_\pi^2 s_\theta^7}{243 \pi^2 M_\eta^8} + \\
& \frac{29 \operatorname{Log}\left[\frac{M_\eta^2}{\mu^2}\right] c_\theta^5 M_0^8 M_K^2 M_\pi^2 s_\theta^7}{486 \sqrt{2} \pi^2 M_\eta^8} + \frac{\sqrt{2} \operatorname{Log}\left[\frac{M_\eta^2}{\mu^2}\right] c_\theta^5 M_0^8 M_K^2 M_\pi^2 s_\theta^7}{243 \pi^2 M_\eta^8} + \frac{17 \operatorname{Log}\left[\frac{M_{\eta'}^2}{\mu^2}\right] c_\theta^5 M_0^8 M_K^2 M_\pi^2 s_\theta^7}{243 \sqrt{2} \pi^2 M_\eta^8} - \\
& \frac{34 \sqrt{2} \operatorname{Log}\left[\frac{M_\eta^2}{\mu^2}\right] c_\theta^5 M_0^8 M_K^2 M_\pi^2 s_\theta^7}{729 \pi^2 M_\eta^8} - \frac{c_\theta^5 M_0^8 M_\pi^4 s_\theta^7}{972 \sqrt{2} \pi^2 M_\eta^8} - \frac{2 \sqrt{2} c_\theta^5 M_0^8 M_\pi^4 s_\theta^7}{243 \pi^2 M_\eta^8} + \frac{\operatorname{Log}\left[\frac{M_\eta^2}{\mu^2}\right] c_\theta^5 M_0^8 M_\pi^4 s_\theta^7}{1944 \sqrt{2} \pi^2 M_\eta^8} - \\
& \frac{2 \sqrt{2} \operatorname{Log}\left[\frac{M_\eta^2}{\mu^2}\right] c_\theta^5 M_0^8 M_\pi^4 s_\theta^7}{243 \pi^2 M_\eta^8} + \frac{131 \operatorname{Log}\left[\frac{M_\eta^2}{\mu^2}\right] c_\theta^5 M_0^8 M_\pi^4 s_\theta^7}{5832 \sqrt{2} \pi^2 M_\eta^8} - \frac{2 \sqrt{2} \operatorname{Log}\left[\frac{M_{\eta'}^2}{\mu^2}\right] c_\theta^5 M_0^8 M_\pi^4 s_\theta^7}{243 \pi^2 M_\eta^8} - \\
& \frac{13\,434\,880 \sqrt{2} c_\theta^5 L_8^2 r M_0^8 M_K^{10} s_\theta^7}{729 F^2 M_\eta^4 M_\eta^8} + \frac{3\,457\,024 \sqrt{2} c_\theta^5 L_8^2 r M_0^8 M_K^8 M_\pi^2 s_\theta^7}{81 F^2 M_\eta^4 M_\eta^8} - \\
& \frac{7\,585\,792 \sqrt{2} c_\theta^5 L_8^2 r M_0^8 M_K^6 M_\pi^4 s_\theta^7}{243 F^2 M_\eta^4 M_\eta^8} + \frac{5\,343\,232 \sqrt{2} c_\theta^5 L_8^2 r M_0^8 M_K^4 M_\pi^6 s_\theta^7}{729 F^2 M_\eta^4 M_\eta^8} - \\
& \frac{106\,496 \sqrt{2} c_\theta^5 L_8^2 r M_0^8 M_K^2 M_\pi^8 s_\theta^7}{243 F^2 M_\eta^4 M_\eta^8} - \frac{1024 \sqrt{2} c_\theta^5 L_8^2 r M_0^8 M_\pi^{10} s_\theta^7}{27 F^2 M_\eta^4 M_\eta^8} + \frac{2 \sqrt{2} \operatorname{Log}\left[\frac{M_K^2}{\mu^2}\right] c_\theta^3 M_0^8 M_K^6 s_\theta^7}{243 \pi^2 M_\eta^2 M_\eta^8} -
\end{aligned}$$

$$\begin{aligned}
& \frac{4096 \sqrt{2} c_{\theta}^3 L_6^r M_0^8 M_K^6 s_{\theta}^7}{243 M_{\eta}^2 M_{\eta'}^8} - \frac{4096 \sqrt{2} c_{\theta}^3 L_7^r M_0^8 M_K^6 s_{\theta}^7}{243 M_{\eta}^2 M_{\eta'}^8} + \frac{512 \sqrt{2} c_{\theta}^3 L_{25}^r M_0^8 M_K^6 s_{\theta}^7}{81 M_{\eta}^2 M_{\eta'}^8} - \\
& \frac{8192 \sqrt{2} c_{\theta}^3 C_{19} M_0^8 M_K^8 s_{\theta}^7}{81 M_{\eta}^2 M_{\eta'}^8} - \frac{16384 \sqrt{2} c_{\theta}^3 C_{31} M_0^8 M_K^8 s_{\theta}^7}{243 M_{\eta}^2 M_{\eta'}^8} - \frac{19 \text{Log}\left[\frac{M_K^2}{\mu^2}\right] c_{\theta}^3 M_0^8 M_K^4 M_{\pi}^2 s_{\theta}^7}{972 \sqrt{2} \pi^2 M_{\eta}^2 M_{\eta'}^8} - \\
& \frac{\sqrt{2} \text{Log}\left[\frac{M_K^2}{\mu^2}\right] c_{\theta}^3 M_0^8 M_K^4 M_{\pi}^2 s_{\theta}^7}{243 \pi^2 M_{\eta}^2 M_{\eta'}^8} + \frac{704 \sqrt{2} c_{\theta}^3 L_6^r M_0^8 M_K^4 M_{\pi}^2 s_{\theta}^7}{81 M_{\eta}^2 M_{\eta'}^8} + \frac{3008 \sqrt{2} c_{\theta}^3 L_7^r M_0^8 M_K^4 M_{\pi}^2 s_{\theta}^7}{81 M_{\eta}^2 M_{\eta'}^8} - \\
& \frac{736 \sqrt{2} c_{\theta}^3 L_{25}^r M_0^8 M_K^4 M_{\pi}^2 s_{\theta}^7}{81 M_{\eta}^2 M_{\eta'}^8} + \frac{17024 \sqrt{2} c_{\theta}^3 C_{19} M_0^8 M_K^4 M_{\pi}^2 s_{\theta}^7}{81 M_{\eta}^2 M_{\eta'}^8} + \frac{34048 \sqrt{2} c_{\theta}^3 C_{31} M_0^8 M_K^4 M_{\pi}^2 s_{\theta}^7}{243 M_{\eta}^2 M_{\eta'}^8} + \\
& \frac{11 \text{Log}\left[\frac{M_K^2}{\mu^2}\right] c_{\theta}^3 M_0^8 M_K^4 M_{\pi}^2 s_{\theta}^7}{972 \sqrt{2} \pi^2 M_{\eta}^2 M_{\eta'}^8} + \frac{\text{Log}\left[\frac{M_{\pi}^2}{\mu^2}\right] c_{\theta}^3 M_0^8 M_K^4 M_{\pi}^2 s_{\theta}^7}{162 \sqrt{2} \pi^2 M_{\eta}^2 M_{\eta'}^8} + \frac{128 \sqrt{2} c_{\theta}^3 L_6^r M_0^8 M_K^4 M_{\pi}^2 s_{\theta}^7}{27 M_{\eta}^2 M_{\eta'}^8} - \\
& \frac{736 \sqrt{2} c_{\theta}^3 L_7^r M_0^8 M_K^4 M_{\pi}^2 s_{\theta}^7}{27 M_{\eta}^2 M_{\eta'}^8} + \frac{224 \sqrt{2} c_{\theta}^3 L_{25}^r M_0^8 M_K^4 M_{\pi}^2 s_{\theta}^7}{81 M_{\eta}^2 M_{\eta'}^8} - \frac{1472 \sqrt{2} c_{\theta}^3 C_{19} M_0^8 M_K^4 M_{\pi}^2 s_{\theta}^7}{9 M_{\eta}^2 M_{\eta'}^8} - \\
& \frac{2944 \sqrt{2} c_{\theta}^3 C_{31} M_0^8 M_K^4 M_{\pi}^2 s_{\theta}^7}{27 M_{\eta}^2 M_{\eta'}^8} - \frac{\text{Log}\left[\frac{M_{\pi}^2}{\mu^2}\right] c_{\theta}^3 M_0^8 M_{\pi}^6 s_{\theta}^7}{162 \sqrt{2} \pi^2 M_{\eta}^2 M_{\eta'}^8} - \frac{464 \sqrt{2} c_{\theta}^3 L_6^r M_0^8 M_{\pi}^6 s_{\theta}^7}{243 M_{\eta}^2 M_{\eta'}^8} + \\
& \frac{1696 \sqrt{2} c_{\theta}^3 L_7^r M_0^8 M_{\pi}^6 s_{\theta}^7}{243 M_{\eta}^2 M_{\eta'}^8} + \frac{4448 \sqrt{2} c_{\theta}^3 C_{19} M_0^8 M_{\pi}^6 s_{\theta}^7}{81 M_{\eta}^2 M_{\eta'}^8} + \frac{8896 \sqrt{2} c_{\theta}^3 C_{31} M_0^8 M_{\pi}^6 s_{\theta}^7}{243 M_{\eta}^2 M_{\eta'}^8} - \\
& \frac{464 \sqrt{2} c_{\theta}^3 C_{19} M_0^8 M_{\pi}^8 s_{\theta}^7}{81 M_{\eta}^2 M_{\eta'}^8} - \frac{928 \sqrt{2} c_{\theta}^3 C_{31} M_0^8 M_{\pi}^8 s_{\theta}^7}{243 M_{\eta}^2 M_{\eta'}^8} - \frac{\text{Log}\left[\frac{M_{\eta}^2}{\mu^2}\right] c_{\theta}^3 M_0^8 M_K^2 s_{\theta}^7}{243 \sqrt{2} \pi^2 M_{\eta}^6 M_{\eta'}^8} + \\
& \frac{5 \text{Log}\left[\frac{M_{\eta}^2}{\mu^2}\right] c_{\theta}^3 M_0^8 M_{\pi}^2 s_{\theta}^7}{1944 \sqrt{2} \pi^2 M_{\eta}^6 M_{\eta'}^8} + \frac{16056320 \sqrt{2} c_{\theta}^5 L_8^2 r M_0^8 M_K^{10} s_{\theta}^7}{729 F^2 M_{\eta}^6 M_{\eta'}^6} - \frac{11886592 \sqrt{2} c_{\theta}^5 L_8^2 r M_0^8 M_K^8 M_{\pi}^2 s_{\theta}^7}{243 F^2 M_{\eta}^6 M_{\eta'}^6} + \\
& \frac{7389184 \sqrt{2} c_{\theta}^5 L_8^2 r M_0^8 M_K^4 M_{\pi}^2 s_{\theta}^7}{243 F^2 M_{\eta}^6 M_{\eta'}^6} - \frac{2097152 \sqrt{2} c_{\theta}^5 L_8^2 r M_0^8 M_K^4 M_{\pi}^2 s_{\theta}^7}{729 F^2 M_{\eta}^6 M_{\eta'}^6} - \\
& \frac{174080 \sqrt{2} c_{\theta}^5 L_8^2 r M_0^8 M_K^2 M_{\pi}^2 s_{\theta}^7}{243 F^2 M_{\eta}^6 M_{\eta'}^6} - \frac{128 \sqrt{2} F^2 v_2^{(2)} c_{\theta}^3 M_0^8 M_K^4 s_{\theta}^7}{27 M_{\eta}^4 M_{\eta'}^6} + \frac{20 \sqrt{2} \text{Log}\left[\frac{M_K^2}{\mu^2}\right] c_{\theta}^3 M_0^8 M_K^6 s_{\theta}^7}{243 \pi^2 M_{\eta}^4 M_{\eta'}^6} - \\
& \frac{2048 \sqrt{2} c_{\theta}^3 L_6^r M_0^8 M_K^6 s_{\theta}^7}{243 M_{\eta}^4 M_{\eta'}^6} - \frac{2048 \sqrt{2} c_{\theta}^3 L_7^r M_0^8 M_K^6 s_{\theta}^7}{243 M_{\eta}^4 M_{\eta'}^6} + \frac{5120 \sqrt{2} c_{\theta}^3 L_{25}^r M_0^8 M_K^6 s_{\theta}^7}{81 M_{\eta}^4 M_{\eta'}^6} - \\
& \frac{4096 \sqrt{2} c_{\theta}^3 C_{19} M_0^8 M_K^8 s_{\theta}^7}{81 M_{\eta}^4 M_{\eta'}^6} - \frac{8192 \sqrt{2} c_{\theta}^3 C_{31} M_0^8 M_K^8 s_{\theta}^7}{243 M_{\eta}^4 M_{\eta'}^6} + \frac{16 \sqrt{2} F^2 v_2^{(2)} c_{\theta}^3 M_0^8 M_K^2 M_{\pi}^2 s_{\theta}^7}{27 M_{\eta}^4 M_{\eta'}^6} - \\
& \frac{31 \text{Log}\left[\frac{M_K^2}{\mu^2}\right] c_{\theta}^3 M_0^8 M_K^4 M_{\pi}^2 s_{\theta}^7}{972 \sqrt{2} \pi^2 M_{\eta}^4 M_{\eta'}^6} - \frac{2 \sqrt{2} \text{Log}\left[\frac{M_K^2}{\mu^2}\right] c_{\theta}^3 M_0^8 M_K^4 M_{\pi}^2 s_{\theta}^7}{81 \pi^2 M_{\eta}^4 M_{\eta'}^6} + \frac{704 \sqrt{2} c_{\theta}^3 L_6^r M_0^8 M_K^4 M_{\pi}^2 s_{\theta}^7}{81 M_{\eta}^4 M_{\eta'}^6} -
\end{aligned}$$

$$\begin{aligned}
& \frac{3904 \sqrt{2} c_{\theta}^3 L_7^r M_0^8 M_K^4 M_{\pi}^2 s_{\theta}^7}{81 M_{\eta}^4 M_{\eta'}^6} - \frac{6880 \sqrt{2} c_{\theta}^3 L_{25}^r M_0^8 M_K^4 M_{\pi}^2 s_{\theta}^7}{81 M_{\eta}^4 M_{\eta'}^6} + \frac{5248 \sqrt{2} c_{\theta}^3 C_{19} M_0^8 M_K^6 M_{\pi}^2 s_{\theta}^7}{81 M_{\eta}^4 M_{\eta'}^6} + \\
& \frac{10\,496 \sqrt{2} c_{\theta}^3 C_{31} M_0^8 M_K^6 M_{\pi}^2 s_{\theta}^7}{243 M_{\eta}^4 M_{\eta'}^6} + \frac{40 \sqrt{2} F^2 v_2^{(2)} c_{\theta}^3 M_0^8 M_{\pi}^4 s_{\theta}^7}{27 M_{\eta}^4 M_{\eta'}^6} - \frac{\text{Log}\left[\frac{M_K^2}{\mu^2}\right] c_{\theta}^3 M_0^8 M_K^2 M_{\pi}^4 s_{\theta}^7}{324 \sqrt{2} \pi^2 M_{\eta}^4 M_{\eta'}^6} - \\
& \frac{5 \text{Log}\left[\frac{M_{\pi}^2}{\mu^2}\right] c_{\theta}^3 M_0^8 M_K^2 M_{\pi}^4 s_{\theta}^7}{81 \sqrt{2} \pi^2 M_{\eta}^4 M_{\eta'}^6} + \frac{640 \sqrt{2} c_{\theta}^3 L_6^r M_0^8 M_K^2 M_{\pi}^4 s_{\theta}^7}{81 M_{\eta}^4 M_{\eta'}^6} + \frac{4960 \sqrt{2} c_{\theta}^3 L_7^r M_0^8 M_K^2 M_{\pi}^4 s_{\theta}^7}{81 M_{\eta}^4 M_{\eta'}^6} + \\
& \frac{3296 \sqrt{2} c_{\theta}^3 L_{25}^r M_0^8 M_K^2 M_{\pi}^4 s_{\theta}^7}{81 M_{\eta}^4 M_{\eta'}^6} - \frac{64 \sqrt{2} c_{\theta}^3 C_{19} M_0^8 M_K^4 M_{\pi}^4 s_{\theta}^7}{3 M_{\eta}^4 M_{\eta'}^6} - \frac{128 \sqrt{2} c_{\theta}^3 C_{31} M_0^8 M_K^4 M_{\pi}^4 s_{\theta}^7}{9 M_{\eta}^4 M_{\eta'}^6} - \\
& \frac{\text{Log}\left[\frac{M_{\pi}^2}{\mu^2}\right] c_{\theta}^3 M_0^8 M_{\pi}^6 s_{\theta}^7}{324 \sqrt{2} \pi^2 M_{\eta}^4 M_{\eta'}^6} + \frac{176 \sqrt{2} c_{\theta}^3 L_6^r M_0^8 M_{\pi}^6 s_{\theta}^7}{243 M_{\eta}^4 M_{\eta'}^6} - \frac{2848 \sqrt{2} c_{\theta}^3 L_7^r M_0^8 M_{\pi}^6 s_{\theta}^7}{243 M_{\eta}^4 M_{\eta'}^6} - \\
& \frac{320 \sqrt{2} c_{\theta}^3 L_{25}^r M_0^8 M_{\pi}^6 s_{\theta}^7}{27 M_{\eta}^4 M_{\eta'}^6} + \frac{1120 \sqrt{2} c_{\theta}^3 C_{19} M_0^8 M_K^2 M_{\pi}^6 s_{\theta}^7}{81 M_{\eta}^4 M_{\eta'}^6} + \frac{2240 \sqrt{2} c_{\theta}^3 C_{31} M_0^8 M_K^2 M_{\pi}^6 s_{\theta}^7}{243 M_{\eta}^4 M_{\eta'}^6} + \\
& \frac{176 \sqrt{2} c_{\theta}^3 C_{19} M_0^8 M_{\pi}^8 s_{\theta}^7}{81 M_{\eta}^4 M_{\eta'}^6} + \frac{352 \sqrt{2} c_{\theta}^3 C_{31} M_0^8 M_{\pi}^8 s_{\theta}^7}{243 M_{\eta}^4 M_{\eta'}^6} - \frac{41 c_{\theta}^5 M_0^8 M_K^4 s_{\theta}^7}{243 \sqrt{2} \pi^2 M_{\eta}^2 M_{\eta'}^6} - \\
& \frac{13 \text{Log}\left[\frac{M_{\eta}^2}{\mu^2}\right] c_{\theta}^5 M_0^8 M_K^4 s_{\theta}^7}{243 \sqrt{2} \pi^2 M_{\eta}^2 M_{\eta'}^6} + \frac{86 \sqrt{2} \text{Log}\left[\frac{M_{\eta}^2}{\mu^2}\right] c_{\theta}^5 M_0^8 M_K^4 s_{\theta}^7}{729 \pi^2 M_{\eta}^2 M_{\eta'}^6} + \frac{2 \sqrt{2} \text{Log}\left[\frac{M_{\eta}^2}{\mu^2}\right] c_{\theta}^5 M_0^8 M_K^4 s_{\theta}^7}{81 \pi^2 M_{\eta}^2 M_{\eta'}^6} + \\
& \frac{23 c_{\theta}^5 M_0^8 M_K^2 M_{\pi}^2 s_{\theta}^7}{1458 \sqrt{2} \pi^2 M_{\eta}^2 M_{\eta'}^6} + \frac{34 \sqrt{2} c_{\theta}^5 M_0^8 M_K^2 M_{\pi}^2 s_{\theta}^7}{729 \pi^2 M_{\eta}^2 M_{\eta'}^6} - \frac{31 \text{Log}\left[\frac{M_{\eta}^2}{\mu^2}\right] c_{\theta}^5 M_0^8 M_K^2 M_{\pi}^2 s_{\theta}^7}{972 \sqrt{2} \pi^2 M_{\eta}^2 M_{\eta'}^6} - \\
& \frac{19 \sqrt{2} \text{Log}\left[\frac{M_{\eta}^2}{\mu^2}\right] c_{\theta}^5 M_0^8 M_K^2 M_{\pi}^2 s_{\theta}^7}{729 \pi^2 M_{\eta}^2 M_{\eta'}^6} - \frac{49 \text{Log}\left[\frac{M_{\eta}^2}{\mu^2}\right] c_{\theta}^5 M_0^8 M_K^2 M_{\pi}^2 s_{\theta}^7}{972 \sqrt{2} \pi^2 M_{\eta}^2 M_{\eta'}^6} + \frac{2 \sqrt{2} \text{Log}\left[\frac{M_{\eta}^2}{\mu^2}\right] c_{\theta}^5 M_0^8 M_K^2 M_{\pi}^2 s_{\theta}^7}{243 \pi^2 M_{\eta}^2 M_{\eta'}^6} + \\
& \frac{11 c_{\theta}^5 M_0^8 M_{\pi}^4 s_{\theta}^7}{432 \sqrt{2} \pi^2 M_{\eta}^2 M_{\eta'}^6} - \frac{4 \sqrt{2} c_{\theta}^5 M_0^8 M_{\pi}^4 s_{\theta}^7}{243 \pi^2 M_{\eta}^2 M_{\eta'}^6} + \frac{47 \text{Log}\left[\frac{M_{\eta}^2}{\mu^2}\right] c_{\theta}^5 M_0^8 M_{\pi}^4 s_{\theta}^7}{5832 \sqrt{2} \pi^2 M_{\eta}^2 M_{\eta'}^6} + \frac{\text{Log}\left[\frac{M_{\eta}^2}{\mu^2}\right] c_{\theta}^5 M_0^8 M_{\pi}^4 s_{\theta}^7}{1296 \sqrt{2} \pi^2 M_{\eta}^2 M_{\eta'}^6} - \\
& \frac{15\,400\,960 \sqrt{2} c_{\theta}^5 L_8^{2r} M_0^8 M_K^{10} s_{\theta}^7}{729 F^2 M_{\eta}^8 M_{\eta'}^4} + \frac{11\,542\,528 \sqrt{2} c_{\theta}^5 L_8^{2r} M_0^8 M_K^8 M_{\pi}^2 s_{\theta}^7}{243 F^2 M_{\eta}^8 M_{\eta'}^4} - \\
& \frac{2\,523\,136 \sqrt{2} c_{\theta}^5 L_8^{2r} M_0^8 M_K^6 M_{\pi}^4 s_{\theta}^7}{81 F^2 M_{\eta}^8 M_{\eta'}^4} + \frac{3\,450\,880 \sqrt{2} c_{\theta}^5 L_8^{2r} M_0^8 M_K^4 M_{\pi}^6 s_{\theta}^7}{729 F^2 M_{\eta}^8 M_{\eta'}^4} + \\
& \frac{28\,672 \sqrt{2} c_{\theta}^5 L_8^{2r} M_0^8 M_K^2 M_{\pi}^8 s_{\theta}^7}{243 F^2 M_{\eta}^8 M_{\eta'}^4} - \frac{512 \sqrt{2} c_{\theta}^5 L_8^{2r} M_0^8 M_{\pi}^{10} s_{\theta}^7}{27 F^2 M_{\eta}^8 M_{\eta'}^4} + \frac{128 \sqrt{2} F^2 v_2^{(2)} c_{\theta}^3 M_0^8 M_K^4 s_{\theta}^7}{27 M_{\eta}^6 M_{\eta'}^4} - \\
& \frac{34 \sqrt{2} \text{Log}\left[\frac{M_K^2}{\mu^2}\right] c_{\theta}^3 M_0^8 M_K^6 s_{\theta}^7}{243 \pi^2 M_{\eta}^6 M_{\eta'}^4} + \frac{4096 \sqrt{2} c_{\theta}^3 L_6^r M_0^8 M_K^6 s_{\theta}^7}{81 M_{\eta}^6 M_{\eta'}^4} + \frac{4096 \sqrt{2} c_{\theta}^3 L_7^r M_0^8 M_K^6 s_{\theta}^7}{81 M_{\eta}^6 M_{\eta'}^4} -
\end{aligned}$$



$$\begin{aligned}
& \frac{8704 \sqrt{2} c_{\theta}^3 L_{25}^r M_0^8 M_K^6 s_{\theta}^7}{81 M_{\eta}^6 M_{\eta'}^4} + \frac{8192 \sqrt{2} c_{\theta}^3 C_{19} M_0^8 M_K^8 s_{\theta}^7}{27 M_{\eta}^6 M_{\eta'}^4} + \frac{16384 \sqrt{2} c_{\theta}^3 C_{31} M_0^8 M_K^8 s_{\theta}^7}{81 M_{\eta}^6 M_{\eta'}^4} + \\
& \frac{80 \sqrt{2} F^2 v_2^{(2)} c_{\theta}^3 M_0^8 M_K^2 M_{\pi}^2 s_{\theta}^7}{27 M_{\eta}^6 M_{\eta'}^4} + \frac{47 \text{Log}\left[\frac{M_K^2}{\mu^2}\right] c_{\theta}^3 M_0^8 M_K^4 M_{\pi}^2 s_{\theta}^7}{972 \sqrt{2} \pi^2 M_{\eta}^6 M_{\eta'}^4} + \frac{13 \sqrt{2} \text{Log}\left[\frac{M_K^2}{\mu^2}\right] c_{\theta}^3 M_0^8 M_K^4 M_{\pi}^2 s_{\theta}^7}{243 \pi^2 M_{\eta}^6 M_{\eta'}^4} - \\
& \frac{1088 \sqrt{2} c_{\theta}^3 L_6^r M_0^8 M_K^4 M_{\pi}^2 s_{\theta}^7}{27 M_{\eta}^6 M_{\eta'}^4} - \frac{320 \sqrt{2} c_{\theta}^3 L_7^r M_0^8 M_K^4 M_{\pi}^2 s_{\theta}^7}{27 M_{\eta}^6 M_{\eta'}^4} + \frac{10592 \sqrt{2} c_{\theta}^3 L_{25}^r M_0^8 M_K^4 M_{\pi}^2 s_{\theta}^7}{81 M_{\eta}^6 M_{\eta'}^4} - \\
& \frac{15232 \sqrt{2} c_{\theta}^3 C_{19} M_0^8 M_K^6 M_{\pi}^2 s_{\theta}^7}{27 M_{\eta}^6 M_{\eta'}^4} - \frac{30464 \sqrt{2} c_{\theta}^3 C_{31} M_0^8 M_K^6 M_{\pi}^2 s_{\theta}^7}{81 M_{\eta}^6 M_{\eta'}^4} + \frac{8 \sqrt{2} F^2 v_2^{(2)} c_{\theta}^3 M_0^8 M_K^4 s_{\theta}^7}{27 M_{\eta}^6 M_{\eta'}^4} - \\
& \frac{\text{Log}\left[\frac{M_K^2}{\mu^2}\right] c_{\theta}^3 M_0^8 M_K^2 M_{\pi}^4 s_{\theta}^7}{36 \sqrt{2} \pi^2 M_{\eta}^6 M_{\eta'}^4} - \frac{\sqrt{2} \text{Log}\left[\frac{M_K^2}{\mu^2}\right] c_{\theta}^3 M_0^8 M_K^2 M_{\pi}^4 s_{\theta}^7}{243 \pi^2 M_{\eta}^6 M_{\eta'}^4} + \frac{\text{Log}\left[\frac{M_{\pi}^2}{\mu^2}\right] c_{\theta}^3 M_0^8 M_K^2 M_{\pi}^4 s_{\theta}^7}{18 \sqrt{2} \pi^2 M_{\eta}^6 M_{\eta'}^4} + \\
& \frac{\sqrt{2} \text{Log}\left[\frac{M_{\pi}^2}{\mu^2}\right] c_{\theta}^3 M_0^8 M_K^2 M_{\pi}^4 s_{\theta}^7}{27 \pi^2 M_{\eta}^6 M_{\eta'}^4} - \frac{128 \sqrt{2} c_{\theta}^3 L_6^r M_0^8 M_K^2 M_{\pi}^4 s_{\theta}^7}{9 M_{\eta}^6 M_{\eta'}^4} - \frac{224 \sqrt{2} c_{\theta}^3 L_7^r M_0^8 M_K^2 M_{\pi}^4 s_{\theta}^7}{9 M_{\eta}^6 M_{\eta'}^4} - \\
& \frac{3424 \sqrt{2} c_{\theta}^3 L_{25}^r M_0^8 M_K^2 M_{\pi}^4 s_{\theta}^7}{81 M_{\eta}^6 M_{\eta'}^4} + \frac{3520 \sqrt{2} c_{\theta}^3 C_{19} M_0^8 M_K^4 M_{\pi}^4 s_{\theta}^7}{9 M_{\eta}^6 M_{\eta'}^4} + \frac{7040 \sqrt{2} c_{\theta}^3 C_{31} M_0^8 M_K^4 M_{\pi}^4 s_{\theta}^7}{27 M_{\eta}^6 M_{\eta'}^4} - \\
& \frac{\text{Log}\left[\frac{M_{\pi}^2}{\mu^2}\right] c_{\theta}^3 M_0^8 M_{\pi}^6 s_{\theta}^7}{18 \sqrt{2} \pi^2 M_{\eta}^6 M_{\eta'}^4} + \frac{752 \sqrt{2} c_{\theta}^3 L_6^r M_0^8 M_{\pi}^6 s_{\theta}^7}{81 M_{\eta}^6 M_{\eta'}^4} + \frac{608 \sqrt{2} c_{\theta}^3 L_7^r M_0^8 M_{\pi}^6 s_{\theta}^7}{81 M_{\eta}^6 M_{\eta'}^4} - \\
& \frac{64 \sqrt{2} c_{\theta}^3 L_{25}^r M_0^8 M_{\pi}^6 s_{\theta}^7}{27 M_{\eta}^6 M_{\eta'}^4} - \frac{1376 \sqrt{2} c_{\theta}^3 C_{19} M_0^8 M_K^2 M_{\pi}^6 s_{\theta}^7}{9 M_{\eta}^6 M_{\eta'}^4} - \frac{2752 \sqrt{2} c_{\theta}^3 C_{31} M_0^8 M_K^2 M_{\pi}^6 s_{\theta}^7}{27 M_{\eta}^6 M_{\eta'}^4} + \\
& \frac{752 \sqrt{2} c_{\theta}^3 C_{19} M_0^8 M_{\pi}^8 s_{\theta}^7}{27 M_{\eta}^6 M_{\eta'}^4} + \frac{1504 \sqrt{2} c_{\theta}^3 C_{31} M_0^8 M_{\pi}^8 s_{\theta}^7}{81 M_{\eta}^6 M_{\eta'}^4} + \frac{29 c_{\theta}^5 M_0^8 M_K^4 s_{\theta}^7}{81 \sqrt{2} \pi^2 M_{\eta}^4 M_{\eta'}^4} + \\
& \frac{13 \text{Log}\left[\frac{M_{\eta}^2}{\mu^2}\right] c_{\theta}^5 M_0^8 M_K^4 s_{\theta}^7}{81 \sqrt{2} \pi^2 M_{\eta}^4 M_{\eta'}^4} - \frac{128 \sqrt{2} \text{Log}\left[\frac{M_{\eta}^2}{\mu^2}\right] c_{\theta}^5 M_0^8 M_K^4 s_{\theta}^7}{729 \pi^2 M_{\eta}^4 M_{\eta'}^4} - \frac{56 \sqrt{2} \text{Log}\left[\frac{M_{\eta}^2}{\mu^2}\right] c_{\theta}^5 M_0^8 M_K^4 s_{\theta}^7}{729 \pi^2 M_{\eta}^4 M_{\eta'}^4} - \\
& \frac{35 c_{\theta}^5 M_0^8 M_K^2 M_{\pi}^2 s_{\theta}^7}{162 \sqrt{2} \pi^2 M_{\eta}^4 M_{\eta'}^4} - \frac{139 \text{Log}\left[\frac{M_{\eta}^2}{\mu^2}\right] c_{\theta}^5 M_0^8 M_K^2 M_{\pi}^2 s_{\theta}^7}{2916 \sqrt{2} \pi^2 M_{\eta}^4 M_{\eta'}^4} + \frac{17 \sqrt{2} \text{Log}\left[\frac{M_{\eta}^2}{\mu^2}\right] c_{\theta}^5 M_0^8 M_K^2 M_{\pi}^2 s_{\theta}^7}{243 \pi^2 M_{\eta}^4 M_{\eta'}^4} + \\
& \frac{581 \text{Log}\left[\frac{M_{\eta}^2}{\mu^2}\right] c_{\theta}^5 M_0^8 M_K^2 M_{\pi}^2 s_{\theta}^7}{2916 \sqrt{2} \pi^2 M_{\eta}^4 M_{\eta'}^4} - \frac{14 \sqrt{2} \text{Log}\left[\frac{M_{\eta}^2}{\mu^2}\right] c_{\theta}^5 M_0^8 M_K^2 M_{\pi}^2 s_{\theta}^7}{243 \pi^2 M_{\eta}^4 M_{\eta'}^4} + \frac{53 c_{\theta}^5 M_0^8 M_{\pi}^4 s_{\theta}^7}{1296 \sqrt{2} \pi^2 M_{\eta}^4 M_{\eta'}^4} - \\
& \frac{11 \text{Log}\left[\frac{M_{\eta}^2}{\mu^2}\right] c_{\theta}^5 M_0^8 M_{\pi}^4 s_{\theta}^7}{1944 \sqrt{2} \pi^2 M_{\eta}^4 M_{\eta'}^4} - \frac{2 \sqrt{2} \text{Log}\left[\frac{M_{\eta}^2}{\mu^2}\right] c_{\theta}^5 M_0^8 M_{\pi}^4 s_{\theta}^7}{729 \pi^2 M_{\eta}^4 M_{\eta'}^4} - \frac{805 \text{Log}\left[\frac{M_{\eta}^2}{\mu^2}\right] c_{\theta}^5 M_0^8 M_{\pi}^4 s_{\theta}^7}{11664 \sqrt{2} \pi^2 M_{\eta}^4 M_{\eta'}^4} + \\
& \frac{7 \sqrt{2} \text{Log}\left[\frac{M_{\eta}^2}{\mu^2}\right] c_{\theta}^5 M_0^8 M_{\pi}^4 s_{\theta}^7}{243 \pi^2 M_{\eta}^4 M_{\eta'}^4} + \frac{\text{Log}\left[\frac{M_{\eta}^2}{\mu^2}\right] c_{\theta}^3 M_0^8 M_K^2 s_{\theta}^7}{54 \sqrt{2} \pi^2 M_{\eta}^2 M_{\eta'}^4} - \frac{\sqrt{2} \text{Log}\left[\frac{M_{\eta}^2}{\mu^2}\right] c_{\theta}^3 M_0^8 M_K^2 s_{\theta}^7}{243 \pi^2 M_{\eta}^2 M_{\eta'}^4} -
\end{aligned}$$

$$\begin{aligned}
& \frac{\text{Log}\left[\frac{M_\eta^2}{\mu^2}\right] c_\theta^3 M_\theta^8 M_\pi^2 s_\theta^7}{108 \sqrt{2} \pi^2 M_\eta^2 M_\eta'^4} + \frac{17 \text{Log}\left[\frac{M_\eta^2}{\mu^2}\right] c_\theta^3 M_\theta^8 M_\pi^2 s_\theta^7}{3888 \sqrt{2} \pi^2 M_\eta^2 M_\eta'^4} + \frac{14\,090\,240 \sqrt{2} c_\theta^5 L_8^2 r M_\theta^8 M_K^{10} s_\theta^7}{729 F^2 M_\eta^{10} M_\eta'^2} - \\
& \frac{3\,751\,936 \sqrt{2} c_\theta^5 L_8^2 r M_\theta^8 M_K^8 M_\pi^2 s_\theta^7}{81 F^2 M_\eta^{10} M_\eta'^2} + \frac{9\,469\,952 \sqrt{2} c_\theta^5 L_8^2 r M_\theta^8 M_K^6 M_\pi^4 s_\theta^7}{243 F^2 M_\eta^{10} M_\eta'^2} - \\
& \frac{10\,514\,432 \sqrt{2} c_\theta^5 L_8^2 r M_\theta^8 M_K^4 M_\pi^6 s_\theta^7}{729 F^2 M_\eta^{10} M_\eta'^2} + \frac{686\,080 \sqrt{2} c_\theta^5 L_8^2 r M_\theta^8 M_K^2 M_\pi^8 s_\theta^7}{243 F^2 M_\eta^{10} M_\eta'^2} - \\
& \frac{2560 \sqrt{2} c_\theta^5 L_8^2 r M_\theta^8 M_\pi^{10} s_\theta^7}{27 F^2 M_\eta^{10} M_\eta'^2} - \frac{128 \sqrt{2} F^2 v_2^{(2)} c_\theta^3 M_\theta^8 M_K^4 s_\theta^7}{27 M_\eta^8 M_\eta'^2} + \frac{32 \sqrt{2} \text{Log}\left[\frac{M_K^2}{\mu^2}\right] c_\theta^3 M_\theta^8 M_K^6 s_\theta^7}{243 \pi^2 M_\eta^8 M_\eta'^2} - \\
& \frac{16\,384 \sqrt{2} c_\theta^3 L_6^r M_\theta^8 M_K^6 s_\theta^7}{243 M_\eta^8 M_\eta'^2} - \frac{16\,384 \sqrt{2} c_\theta^3 L_7^r M_\theta^8 M_K^6 s_\theta^7}{243 M_\eta^8 M_\eta'^2} + \frac{8192 \sqrt{2} c_\theta^3 L_{25}^r M_\theta^8 M_K^6 s_\theta^7}{81 M_\eta^8 M_\eta'^2} - \\
& \frac{32\,768 \sqrt{2} c_\theta^3 C_{19} M_\theta^8 M_K^8 s_\theta^7}{81 M_\eta^8 M_\eta'^2} - \frac{65\,536 \sqrt{2} c_\theta^3 C_{31} M_\theta^8 M_K^8 s_\theta^7}{243 M_\eta^8 M_\eta'^2} - \frac{80 \sqrt{2} F^2 v_2^{(2)} c_\theta^3 M_\theta^8 M_K^2 M_\pi^2 s_\theta^7}{27 M_\eta^8 M_\eta'^2} - \\
& \frac{125 \text{Log}\left[\frac{M_K^2}{\mu^2}\right] c_\theta^3 M_\theta^8 M_K^4 M_\pi^2 s_\theta^7}{972 \sqrt{2} \pi^2 M_\eta^8 M_\eta'^2} - \frac{5 \sqrt{2} \text{Log}\left[\frac{M_K^2}{\mu^2}\right] c_\theta^3 M_\theta^8 M_K^4 M_\pi^2 s_\theta^7}{243 \pi^2 M_\eta^8 M_\eta'^2} + \frac{1216 \sqrt{2} c_\theta^3 L_6^r M_\theta^8 M_K^4 M_\pi^2 s_\theta^7}{27 M_\eta^8 M_\eta'^2} + \\
& \frac{64 \sqrt{2} c_\theta^3 L_7^r M_\theta^8 M_K^4 M_\pi^2 s_\theta^7}{M_\eta^8 M_\eta'^2} - \frac{10\,144 \sqrt{2} c_\theta^3 L_{25}^r M_\theta^8 M_K^4 M_\pi^2 s_\theta^7}{81 M_\eta^8 M_\eta'^2} + \frac{63\,872 \sqrt{2} c_\theta^3 C_{19} M_\theta^8 M_K^6 M_\pi^2 s_\theta^7}{81 M_\eta^8 M_\eta'^2} + \\
& \frac{127\,744 \sqrt{2} c_\theta^3 C_{31} M_\theta^8 M_K^6 M_\pi^2 s_\theta^7}{243 M_\eta^8 M_\eta'^2} - \frac{8 \sqrt{2} F^2 v_2^{(2)} c_\theta^3 M_\theta^8 M_K^4 s_\theta^7}{27 M_\eta^8 M_\eta'^2} + \frac{23 \text{Log}\left[\frac{M_K^2}{\mu^2}\right] c_\theta^3 M_\theta^8 M_K^2 M_\pi^4 s_\theta^7}{972 \sqrt{2} \pi^2 M_\eta^8 M_\eta'^2} + \\
& \frac{\sqrt{2} \text{Log}\left[\frac{M_K^2}{\mu^2}\right] c_\theta^3 M_\theta^8 M_K^2 M_\pi^4 s_\theta^7}{81 \pi^2 M_\eta^8 M_\eta'^2} - \frac{7 \text{Log}\left[\frac{M_\pi^2}{\mu^2}\right] c_\theta^3 M_\theta^8 M_K^2 M_\pi^4 s_\theta^7}{81 \sqrt{2} \pi^2 M_\eta^8 M_\eta'^2} + \frac{1408 \sqrt{2} c_\theta^3 L_6^r M_\theta^8 M_K^2 M_\pi^4 s_\theta^7}{81 M_\eta^8 M_\eta'^2} - \\
& \frac{1760 \sqrt{2} c_\theta^3 L_7^r M_\theta^8 M_K^2 M_\pi^4 s_\theta^7}{81 M_\eta^8 M_\eta'^2} + \frac{3488 \sqrt{2} c_\theta^3 L_{25}^r M_\theta^8 M_K^2 M_\pi^4 s_\theta^7}{81 M_\eta^8 M_\eta'^2} - \frac{576 \sqrt{2} c_\theta^3 C_{19} M_\theta^8 M_K^4 M_\pi^4 s_\theta^7}{M_\eta^8 M_\eta'^2} - \\
& \frac{384 \sqrt{2} c_\theta^3 C_{31} M_\theta^8 M_K^4 M_\pi^4 s_\theta^7}{M_\eta^8 M_\eta'^2} + \frac{13 \text{Log}\left[\frac{M_\pi^2}{\mu^2}\right] c_\theta^3 M_\theta^8 M_\pi^6 s_\theta^7}{324 \sqrt{2} \pi^2 M_\eta^8 M_\eta'^2} - \frac{2672 \sqrt{2} c_\theta^3 L_6^r M_\theta^8 M_\pi^6 s_\theta^7}{243 M_\eta^8 M_\eta'^2} + \\
& \frac{928 \sqrt{2} c_\theta^3 L_7^r M_\theta^8 M_\pi^6 s_\theta^7}{243 M_\eta^8 M_\eta'^2} + \frac{64 \sqrt{2} c_\theta^3 L_{25}^r M_\theta^8 M_\pi^6 s_\theta^7}{27 M_\eta^8 M_\eta'^2} + \frac{16\,928 \sqrt{2} c_\theta^3 C_{19} M_\theta^8 M_K^2 M_\pi^6 s_\theta^7}{81 M_\eta^8 M_\eta'^2} + \\
& \frac{33\,856 \sqrt{2} c_\theta^3 C_{31} M_\theta^8 M_K^2 M_\pi^6 s_\theta^7}{243 M_\eta^8 M_\eta'^2} - \frac{2672 \sqrt{2} c_\theta^3 C_{19} M_\theta^8 M_\pi^8 s_\theta^7}{81 M_\eta^8 M_\eta'^2} - \frac{5344 \sqrt{2} c_\theta^3 C_{31} M_\theta^8 M_\pi^8 s_\theta^7}{243 M_\eta^8 M_\eta'^2} + \\
& \frac{8 \sqrt{2} F^2 v_2^{(2)} c_\theta M_\theta^8 M_K^2 s_\theta^7}{3 M_\eta^6 M_\eta'^2} + \frac{64 \sqrt{2} F^2 v_2^{(2)} c_\theta M_\theta^6 M_K^4 s_\theta^7}{27 M_\eta^6 M_\eta'^2} + \frac{c_\theta M_\theta^8 M_K^4 s_\theta^7}{162 \sqrt{2} \pi^2 M_\eta^6 M_\eta'^2} - \frac{\sqrt{2} c_\theta M_\theta^8 M_K^4 s_\theta^7}{81 \pi^2 M_\eta^6 M_\eta'^2} -
\end{aligned}$$

$$\begin{aligned}
& \frac{\sqrt{2} \operatorname{Log}\left[\frac{M_K^2}{\mu^2}\right] c_\theta M_0^8 M_K^4 s_\theta^7}{81 \pi^2 M_\eta^6 M_\eta'^2} - \frac{95 c_\theta^5 M_0^8 M_K^4 s_\theta^7}{243 \sqrt{2} \pi^2 M_\eta^6 M_\eta'^2} + \frac{17 \sqrt{2} \operatorname{Log}\left[\frac{M_\eta'^2}{\mu^2}\right] c_\theta^5 M_0^8 M_K^4 s_\theta^7}{243 \pi^2 M_\eta^6 M_\eta'^2} - \\
& \frac{25 \operatorname{Log}\left[\frac{M_\eta'^2}{\mu^2}\right] c_\theta^5 M_0^8 M_K^4 s_\theta^7}{243 \sqrt{2} \pi^2 M_\eta^6 M_\eta'^2} + \frac{110 \sqrt{2} \operatorname{Log}\left[\frac{M_\eta'^2}{\mu^2}\right] c_\theta^5 M_0^8 M_K^4 s_\theta^7}{729 \pi^2 M_\eta^6 M_\eta'^2} + \frac{512 \sqrt{2} c_\theta L_6^r M_0^8 M_K^4 s_\theta^7}{81 M_\eta^6 M_\eta'^2} + \\
& \frac{512 \sqrt{2} c_\theta L_7^r M_0^8 M_K^4 s_\theta^7}{81 M_\eta^6 M_\eta'^2} + \frac{1792 \sqrt{2} c_\theta C_{19} M_0^8 M_K^6 s_\theta^7}{27 M_\eta^6 M_\eta'^2} + \frac{5120 \sqrt{2} c_\theta C_{31} M_0^8 M_K^6 s_\theta^7}{81 M_\eta^6 M_\eta'^2} - \\
& \frac{8 \sqrt{2} F^2 v_2^{(2)} c_\theta M_0^8 M_\pi^2 s_\theta^7}{3 M_\eta^6 M_\eta'^2} - \frac{32 \sqrt{2} F^2 v_2^{(2)} c_\theta M_0^6 M_K^2 M_\pi^2 s_\theta^7}{27 M_\eta^6 M_\eta'^2} + \frac{c_\theta M_0^8 M_K^2 M_\pi^2 s_\theta^7}{108 \sqrt{2} \pi^2 M_\eta^6 M_\eta'^2} + \\
& \frac{\operatorname{Log}\left[\frac{M_K^2}{\mu^2}\right] c_\theta M_0^8 M_K^2 M_\pi^2 s_\theta^7}{81 \sqrt{2} \pi^2 M_\eta^6 M_\eta'^2} + \frac{35 \sqrt{2} c_\theta^5 M_0^8 M_K^2 M_\pi^2 s_\theta^7}{243 \pi^2 M_\eta^6 M_\eta'^2} - \frac{25 \operatorname{Log}\left[\frac{M_\eta'^2}{\mu^2}\right] c_\theta^5 M_0^8 M_K^2 M_\pi^2 s_\theta^7}{486 \sqrt{2} \pi^2 M_\eta^6 M_\eta'^2} - \\
& \frac{7 \sqrt{2} \operatorname{Log}\left[\frac{M_\eta'^2}{\mu^2}\right] c_\theta^5 M_0^8 M_K^2 M_\pi^2 s_\theta^7}{243 \pi^2 M_\eta^6 M_\eta'^2} + \frac{25 \operatorname{Log}\left[\frac{M_\eta'^2}{\mu^2}\right] c_\theta^5 M_0^8 M_K^2 M_\pi^2 s_\theta^7}{486 \sqrt{2} \pi^2 M_\eta^6 M_\eta'^2} - \frac{37 \sqrt{2} \operatorname{Log}\left[\frac{M_\eta'^2}{\mu^2}\right] c_\theta^5 M_0^8 M_K^2 M_\pi^2 s_\theta^7}{729 \pi^2 M_\eta^6 M_\eta'^2} - \\
& \frac{256 \sqrt{2} c_\theta L_6^r M_0^8 M_K^2 M_\pi^2 s_\theta^7}{81 M_\eta^6 M_\eta'^2} - \frac{256 \sqrt{2} c_\theta L_7^r M_0^8 M_K^2 M_\pi^2 s_\theta^7}{81 M_\eta^6 M_\eta'^2} - \frac{896 \sqrt{2} c_\theta C_{19} M_0^8 M_K^4 M_\pi^2 s_\theta^7}{9 M_\eta^6 M_\eta'^2} - \\
& \frac{2560 \sqrt{2} c_\theta C_{31} M_0^8 M_K^4 M_\pi^2 s_\theta^7}{27 M_\eta^6 M_\eta'^2} - \frac{32 \sqrt{2} F^2 v_2^{(2)} c_\theta M_0^6 M_\pi^4 s_\theta^7}{27 M_\eta^6 M_\eta'^2} + \frac{c_\theta M_0^8 M_\pi^4 s_\theta^7}{72 \sqrt{2} \pi^2 M_\eta^6 M_\eta'^2} + \\
& \frac{\operatorname{Log}\left[\frac{M_\pi^2}{\mu^2}\right] c_\theta M_0^8 M_\pi^4 s_\theta^7}{54 \sqrt{2} \pi^2 M_\eta^6 M_\eta'^2} - \frac{275 c_\theta^5 M_0^8 M_\pi^4 s_\theta^7}{3888 \sqrt{2} \pi^2 M_\eta^6 M_\eta'^2} - \frac{13 \operatorname{Log}\left[\frac{M_\eta'^2}{\mu^2}\right] c_\theta^5 M_0^8 M_\pi^4 s_\theta^7}{972 \sqrt{2} \pi^2 M_\eta^6 M_\eta'^2} + \\
& \frac{5 \sqrt{2} \operatorname{Log}\left[\frac{M_\eta'^2}{\mu^2}\right] c_\theta^5 M_0^8 M_\pi^4 s_\theta^7}{243 \pi^2 M_\eta^6 M_\eta'^2} - \frac{5 \operatorname{Log}\left[\frac{M_\eta'^2}{\mu^2}\right] c_\theta^5 M_0^8 M_\pi^4 s_\theta^7}{3888 \sqrt{2} \pi^2 M_\eta^6 M_\eta'^2} - \frac{4 \sqrt{2} \operatorname{Log}\left[\frac{M_\eta'^2}{\mu^2}\right] c_\theta^5 M_0^8 M_\pi^4 s_\theta^7}{729 \pi^2 M_\eta^6 M_\eta'^2} - \\
& \frac{256 \sqrt{2} c_\theta L_6^r M_0^8 M_\pi^4 s_\theta^7}{81 M_\eta^6 M_\eta'^2} - \frac{256 \sqrt{2} c_\theta L_7^r M_0^8 M_\pi^4 s_\theta^7}{81 M_\eta^6 M_\eta'^2} + \frac{448 \sqrt{2} c_\theta C_{19} M_0^8 M_K^2 M_\pi^4 s_\theta^7}{9 M_\eta^6 M_\eta'^2} + \\
& \frac{1280 \sqrt{2} c_\theta C_{31} M_0^8 M_K^2 M_\pi^4 s_\theta^7}{27 M_\eta^6 M_\eta'^2} - \frac{448 \sqrt{2} c_\theta C_{19} M_0^8 M_\pi^6 s_\theta^7}{27 M_\eta^6 M_\eta'^2} - \frac{1280 \sqrt{2} c_\theta C_{31} M_0^8 M_\pi^6 s_\theta^7}{81 M_\eta^6 M_\eta'^2} - \\
& \frac{5 \operatorname{Log}\left[\frac{M_\eta'^2}{\mu^2}\right] c_\theta^3 M_0^8 M_K^2 s_\theta^7}{162 \sqrt{2} \pi^2 M_\eta^4 M_\eta'^2} + \frac{5 \operatorname{Log}\left[\frac{M_\eta'^2}{\mu^2}\right] c_\theta^3 M_0^8 M_\pi^2 s_\theta^7}{324 \sqrt{2} \pi^2 M_\eta^4 M_\eta'^2} + \frac{\operatorname{Log}\left[\frac{M_\eta'^2}{\mu^2}\right] c_\theta^3 M_0^8 M_\pi^2 s_\theta^7}{432 \sqrt{2} \pi^2 M_\eta^4 M_\eta'^2} + \\
& \frac{16 \sqrt{2} \operatorname{Log}\left[\frac{M_\eta'^2}{\mu^2}\right] c_\theta^5 M_0^8 M_K^4 M_\eta'^2 s_\theta^7}{729 \pi^2 M_\eta^{10}} - \frac{23 \operatorname{Log}\left[\frac{M_\eta'^2}{\mu^2}\right] c_\theta^5 M_0^8 M_K^2 M_\pi^2 M_\eta'^2 s_\theta^7}{1458 \sqrt{2} \pi^2 M_\eta^{10}} -
\end{aligned}$$

[illegible]

$$\begin{aligned}
& \frac{8 \sqrt{2} \operatorname{Log}\left[\frac{M_{\eta'}^2}{\mu^2}\right] c_{\theta}^5 M_{\theta}^8 M_K^4 M_{\pi}^2 s_{\theta}^7}{243 \pi^2 M_{\eta}^8 (M_{\eta}^2 - M_{\eta'}^2)} - \frac{11 \operatorname{Log}\left[\frac{M_{\eta'}^2}{\mu^2}\right] c_{\theta}^5 M_{\theta}^8 M_K^2 M_{\pi}^2 M_{\eta'}^2 s_{\theta}^7}{243 \sqrt{2} \pi^2 M_{\eta}^8 (M_{\eta}^2 - M_{\eta'}^2)} - \frac{\operatorname{Log}\left[\frac{M_{\eta'}^2}{\mu^2}\right] c_{\theta}^5 M_{\theta}^8 M_{\pi}^4 M_{\eta'}^2 s_{\theta}^7}{144 \sqrt{2} \pi^2 M_{\eta}^8 (M_{\eta}^2 - M_{\eta'}^2)} + \\
& \frac{2 \sqrt{2} \operatorname{Log}\left[\frac{M_{\eta'}^2}{\mu^2}\right] c_{\theta}^5 M_{\theta}^8 M_{\pi}^4 M_{\eta'}^2 s_{\theta}^7}{243 \pi^2 M_{\eta}^8 (M_{\eta}^2 - M_{\eta'}^2)} - \frac{11 468 800 c_{\theta}^4 L_8^2 r M_{\theta}^8 M_K^{10} s_{\theta}^8}{729 F^2 M_{\eta}^{12}} + \frac{3 184 640 c_{\theta}^4 L_8^2 r M_{\theta}^8 M_K^8 M_{\pi}^2 s_{\theta}^8}{81 F^2 M_{\eta}^{12}} - \\
& \frac{9 482 240 c_{\theta}^4 L_8^2 r M_{\theta}^8 M_K^6 M_{\pi}^4 s_{\theta}^8}{243 F^2 M_{\eta}^{12}} + \frac{14 064 640 c_{\theta}^4 L_8^2 r M_{\theta}^8 M_K^4 M_{\pi}^6 s_{\theta}^8}{729 F^2 M_{\eta}^{12}} - \frac{386 560 c_{\theta}^4 L_8^2 r M_{\theta}^8 M_K^2 M_{\pi}^8 s_{\theta}^8}{81 F^2 M_{\eta}^{12}} + \\
& \frac{18 560 c_{\theta}^4 L_8^2 r M_{\theta}^8 M_K^{10} s_{\theta}^8}{81 F^2 M_{\eta}^{12}} + \frac{64 F^2 v_2^{(2)} c_{\theta}^2 M_{\theta}^8 M_K^4 s_{\theta}^8}{9 M_{\eta}^{10}} - \frac{20 \operatorname{Log}\left[\frac{M_K^2}{\mu^2}\right] c_{\theta}^2 M_{\theta}^8 M_K^6 s_{\theta}^8}{243 \pi^2 M_{\eta}^{10}} + \\
& \frac{2560 c_{\theta}^2 L_6^r M_{\theta}^8 M_K^6 s_{\theta}^8}{81 M_{\eta}^{10}} + \frac{2560 c_{\theta}^2 L_7^r M_{\theta}^8 M_K^6 s_{\theta}^8}{81 M_{\eta}^{10}} - \frac{5120 c_{\theta}^2 L_{25}^r M_{\theta}^8 M_K^6 s_{\theta}^8}{81 M_{\eta}^{10}} + \frac{5120 c_{\theta}^2 C_{19} M_{\theta}^8 M_K^8 s_{\theta}^8}{27 M_{\eta}^{10}} + \\
& \frac{10 240 c_{\theta}^2 C_{31} M_{\theta}^8 M_K^8 s_{\theta}^8}{81 M_{\eta}^{10}} + \frac{16 F^2 v_2^{(2)} c_{\theta}^2 M_{\theta}^8 M_K^2 M_{\pi}^2 s_{\theta}^8}{9 M_{\eta}^{10}} + \frac{61 \operatorname{Log}\left[\frac{M_K^2}{\mu^2}\right] c_{\theta}^2 M_{\theta}^8 M_K^4 M_{\pi}^2 s_{\theta}^8}{972 \pi^2 M_{\eta}^{10}} - \\
& \frac{128 c_{\theta}^2 L_6^r M_{\theta}^8 M_K^4 M_{\pi}^2 s_{\theta}^8}{9 M_{\eta}^{10}} - \frac{512 c_{\theta}^2 L_7^r M_{\theta}^8 M_K^4 M_{\pi}^2 s_{\theta}^8}{27 M_{\eta}^{10}} + \frac{7936 c_{\theta}^2 L_{25}^r M_{\theta}^8 M_K^4 M_{\pi}^2 s_{\theta}^8}{81 M_{\eta}^{10}} - \\
& \frac{3584 c_{\theta}^2 C_{19} M_{\theta}^8 M_K^6 M_{\pi}^2 s_{\theta}^8}{9 M_{\eta}^{10}} - \frac{7168 c_{\theta}^2 C_{31} M_{\theta}^8 M_K^6 M_{\pi}^2 s_{\theta}^8}{27 M_{\eta}^{10}} - \frac{8 F^2 v_2^{(2)} c_{\theta}^2 M_{\theta}^8 M_{\pi}^4 s_{\theta}^8}{9 M_{\eta}^{10}} - \\
& \frac{31 \operatorname{Log}\left[\frac{M_K^2}{\mu^2}\right] c_{\theta}^2 M_{\theta}^8 M_K^2 M_{\pi}^4 s_{\theta}^8}{1944 \pi^2 M_{\eta}^{10}} - \frac{\operatorname{Log}\left[\frac{M_{\pi}^2}{\mu^2}\right] c_{\theta}^2 M_{\theta}^8 M_K^2 M_{\pi}^4 s_{\theta}^8}{72 \pi^2 M_{\eta}^{10}} - \frac{5120 c_{\theta}^2 L_{25}^r M_{\theta}^8 M_K^2 M_{\pi}^4 s_{\theta}^8}{81 M_{\eta}^{10}} + \\
& \frac{2816 c_{\theta}^2 C_{19} M_{\theta}^8 M_K^4 M_{\pi}^4 s_{\theta}^8}{9 M_{\eta}^{10}} + \frac{5632 c_{\theta}^2 C_{31} M_{\theta}^8 M_K^4 M_{\pi}^4 s_{\theta}^8}{27 M_{\eta}^{10}} - \frac{7 \operatorname{Log}\left[\frac{M_{\pi}^2}{\mu^2}\right] c_{\theta}^2 M_{\theta}^8 M_{\pi}^6 s_{\theta}^8}{432 \pi^2 M_{\eta}^{10}} + \\
& \frac{608 c_{\theta}^2 L_6^r M_{\theta}^8 M_{\pi}^6 s_{\theta}^8}{81 M_{\eta}^{10}} + \frac{704 c_{\theta}^2 L_7^r M_{\theta}^8 M_{\pi}^6 s_{\theta}^8}{81 M_{\eta}^{10}} + \frac{64 c_{\theta}^2 L_{25}^r M_{\theta}^8 M_{\pi}^6 s_{\theta}^8}{9 M_{\eta}^{10}} - \frac{2752 c_{\theta}^2 C_{19} M_{\theta}^8 M_K^2 M_{\pi}^6 s_{\theta}^8}{27 M_{\eta}^{10}} - \\
& \frac{5504 c_{\theta}^2 C_{31} M_{\theta}^8 M_K^2 M_{\pi}^6 s_{\theta}^8}{81 M_{\eta}^{10}} + \frac{608 c_{\theta}^2 C_{19} M_{\theta}^8 M_{\pi}^8 s_{\theta}^8}{27 M_{\eta}^{10}} + \frac{1216 c_{\theta}^2 C_{31} M_{\theta}^8 M_{\pi}^8 s_{\theta}^8}{81 M_{\eta}^{10}} - \frac{4 F^2 v_2^{(2)} M_{\theta}^8 M_K^2 s_{\theta}^8}{3 M_{\eta}^8} - \\
& \frac{16 F^2 v_2^{(2)} M_{\theta}^6 M_K^4 s_{\theta}^8}{27 M_{\eta}^8} + \frac{M_{\theta}^8 M_K^4 s_{\theta}^8}{216 \pi^2 M_{\eta}^8} + \frac{\operatorname{Log}\left[\frac{M_K^2}{\mu^2}\right] M_{\theta}^8 M_K^4 s_{\theta}^8}{162 \pi^2 M_{\eta}^8} + \frac{281 c_{\theta}^4 M_{\theta}^8 M_K^4 s_{\theta}^8}{1944 \pi^2 M_{\eta}^8} - \frac{35 \operatorname{Log}\left[\frac{M_{\eta}^2}{\mu^2}\right] c_{\theta}^4 M_{\theta}^8 M_K^4 s_{\theta}^8}{729 \pi^2 M_{\eta}^8} - \\
& \frac{59 \operatorname{Log}\left[\frac{M_{\eta}^2}{\mu^2}\right] c_{\theta}^4 M_{\theta}^8 M_K^4 s_{\theta}^8}{1944 \pi^2 M_{\eta}^8} - \frac{128 L_6^r M_{\theta}^8 M_K^4 s_{\theta}^8}{81 M_{\eta}^8} - \frac{128 L_7^r M_{\theta}^8 M_K^4 s_{\theta}^8}{81 M_{\eta}^8} - \frac{448 C_{19} M_{\theta}^8 M_K^6 s_{\theta}^8}{27 M_{\eta}^8} - \\
& \frac{1280 C_{31} M_{\theta}^8 M_K^6 s_{\theta}^8}{81 M_{\eta}^8} - \frac{2 F^2 v_2^{(2)} M_{\theta}^8 M_{\pi}^2 s_{\theta}^8}{3 M_{\eta}^8} - \frac{16 F^2 v_2^{(2)} M_{\theta}^6 M_K^2 M_{\pi}^2 s_{\theta}^8}{27 M_{\eta}^8} - \frac{35 c_{\theta}^4 M_{\theta}^8 M_K^2 M_{\pi}^2 s_{\theta}^8}{243 \pi^2 M_{\eta}^8} +
\end{aligned}$$

$$\begin{aligned}
& \frac{559 \operatorname{Log}\left[\frac{M_\eta^2}{\mu^2}\right] c_\theta^4 M_\theta^8 M_K^2 M_\pi^2 s_\theta^8}{11\,664 \pi^2 M_\eta^8} + \frac{5 \operatorname{Log}\left[\frac{M_{\eta'}^2}{\mu^2}\right] c_\theta^4 M_\theta^8 M_K^2 M_\pi^2 s_\theta^8}{432 \pi^2 M_\eta^8} - \frac{128 L_6^r M_\theta^8 M_K^2 M_\pi^2 s_\theta^8}{81 M_\eta^8} - \\
& \frac{128 L_7^r M_\theta^8 M_K^2 M_\pi^2 s_\theta^8}{81 M_\eta^8} + \frac{224 C_{19} M_\theta^8 M_K^4 M_\pi^2 s_\theta^8}{9 M_\eta^8} + \frac{640 C_{31} M_\theta^8 M_K^4 M_\pi^2 s_\theta^8}{27 M_\eta^8} - \frac{4 F^2 v_2^{(2)} M_\theta^6 M_\pi^4 s_\theta^8}{27 M_\eta^8} + \\
& \frac{M_\theta^8 M_\pi^4 s_\theta^8}{288 \pi^2 M_\eta^8} + \frac{\operatorname{Log}\left[\frac{M_\pi^2}{\mu^2}\right] M_\theta^8 M_\pi^4 s_\theta^8}{216 \pi^2 M_\eta^8} + \frac{1397 c_\theta^4 M_\theta^8 M_\pi^4 s_\theta^8}{31\,104 \pi^2 M_\eta^8} - \frac{349 \operatorname{Log}\left[\frac{M_\eta^2}{\mu^2}\right] c_\theta^4 M_\theta^8 M_\pi^4 s_\theta^8}{23\,328 \pi^2 M_\eta^8} + \\
& \frac{77 \operatorname{Log}\left[\frac{M_{\eta'}^2}{\mu^2}\right] c_\theta^4 M_\theta^8 M_\pi^4 s_\theta^8}{31\,104 \pi^2 M_\eta^8} - \frac{32 L_6^r M_\theta^8 M_\pi^4 s_\theta^8}{81 M_\eta^8} - \frac{32 L_7^r M_\theta^8 M_\pi^4 s_\theta^8}{81 M_\eta^8} - \frac{112 C_{19} M_\theta^8 M_K^2 M_\pi^4 s_\theta^8}{9 M_\eta^8} - \\
& \frac{320 C_{31} M_\theta^8 M_K^2 M_\pi^4 s_\theta^8}{27 M_\eta^8} - \frac{56 C_{19} M_\theta^8 M_\pi^6 s_\theta^8}{27 M_\eta^8} - \frac{160 C_{31} M_\theta^8 M_\pi^6 s_\theta^8}{81 M_\eta^8} + \frac{5 \operatorname{Log}\left[\frac{M_\eta^2}{\mu^2}\right] c_\theta^2 M_\theta^8 M_K^2 s_\theta^8}{648 \pi^2 M_\eta^6} - \\
& \frac{\operatorname{Log}\left[\frac{M_{\eta'}^2}{\mu^2}\right] c_\theta^2 M_\theta^8 M_K^2 s_\theta^8}{162 \pi^2 M_\eta^6} - \frac{5 \operatorname{Log}\left[\frac{M_\eta^2}{\mu^2}\right] c_\theta^2 M_\theta^8 M_\pi^2 s_\theta^8}{2592 \pi^2 M_\eta^6} + \frac{5 \operatorname{Log}\left[\frac{M_{\eta'}^2}{\mu^2}\right] c_\theta^2 M_\theta^8 M_\pi^2 s_\theta^8}{1296 \pi^2 M_\eta^6} - \\
& \frac{655\,360 c_\theta^4 L_8^2 r M_\theta^8 M_K^{10} s_\theta^8}{729 F^2 M_\eta^{12}} + \frac{532\,480 c_\theta^4 L_8^2 r M_\theta^8 M_K^8 M_\pi^2 s_\theta^8}{243 F^2 M_\eta^{12}} - \frac{573\,440 c_\theta^4 L_8^2 r M_\theta^8 M_K^6 M_\pi^4 s_\theta^8}{243 F^2 M_\eta^{12}} + \\
& \frac{993\,280 c_\theta^4 L_8^2 r M_\theta^8 M_K^4 M_\pi^6 s_\theta^8}{729 F^2 M_\eta^{12}} - \frac{102\,400 c_\theta^4 L_8^2 r M_\theta^8 M_K^2 M_\pi^8 s_\theta^8}{243 F^2 M_\eta^{12}} + \frac{4480 c_\theta^4 L_8^2 r M_\theta^8 M_K^{10} s_\theta^8}{81 F^2 M_\eta^{12}} - \\
& \frac{7\,208\,960 c_\theta^4 L_8^2 r M_\theta^8 M_K^{10} s_\theta^8}{729 F^2 M_\eta^{10}} + \frac{2\,023\,424 c_\theta^4 L_8^2 r M_\theta^8 M_K^8 M_\pi^2 s_\theta^8}{81 F^2 M_\eta^{10}} - \frac{5\,783\,552 c_\theta^4 L_8^2 r M_\theta^8 M_K^6 M_\pi^4 s_\theta^8}{243 F^2 M_\eta^{10}} + \\
& \frac{7\,540\,736 c_\theta^4 L_8^2 r M_\theta^8 M_K^4 M_\pi^6 s_\theta^8}{729 F^2 M_\eta^{10}} - \frac{434\,176 c_\theta^4 L_8^2 r M_\theta^8 M_K^2 M_\pi^8 s_\theta^8}{243 F^2 M_\eta^{10}} - \frac{512 c_\theta^4 L_8^2 r M_\theta^8 M_\pi^{10} s_\theta^8}{27 F^2 M_\eta^{10}} - \\
& \frac{4 \operatorname{Log}\left[\frac{M_\eta^2}{\mu^2}\right] c_\theta^4 M_\theta^8 M_K^4 M_\pi^2 s_\theta^8}{729 \pi^2 M_\eta^{10}} + \frac{11 \operatorname{Log}\left[\frac{M_{\eta'}^2}{\mu^2}\right] c_\theta^4 M_\theta^8 M_K^2 M_\pi^2 s_\theta^8}{2916 \pi^2 M_\eta^{10}} - \frac{7 \operatorname{Log}\left[\frac{M_{\eta'}^2}{\mu^2}\right] c_\theta^4 M_\theta^8 M_\pi^4 M_\eta^2 s_\theta^8}{11\,664 \pi^2 M_\eta^{10}} + \\
& \frac{5 c_\theta^4 M_\theta^8 M_K^4 s_\theta^8}{486 \pi^2 M_{\eta'}^8} + \frac{5 \operatorname{Log}\left[\frac{M_\eta^2}{\mu^2}\right] c_\theta^4 M_\theta^8 M_K^4 s_\theta^8}{486 \pi^2 M_{\eta'}^8} - \frac{2 \operatorname{Log}\left[\frac{M_{\eta'}^2}{\mu^2}\right] c_\theta^4 M_\theta^8 M_K^4 s_\theta^8}{729 \pi^2 M_{\eta'}^8} - \frac{2 c_\theta^4 M_\theta^8 M_K^2 M_\pi^2 s_\theta^8}{243 \pi^2 M_{\eta'}^8} - \\
& \frac{7 \operatorname{Log}\left[\frac{M_\eta^2}{\mu^2}\right] c_\theta^4 M_\theta^8 M_K^2 M_\pi^2 s_\theta^8}{1944 \pi^2 M_{\eta'}^8} + \frac{7 \operatorname{Log}\left[\frac{M_{\eta'}^2}{\mu^2}\right] c_\theta^4 M_\theta^8 M_K^2 M_\pi^2 s_\theta^8}{2916 \pi^2 M_{\eta'}^8} + \frac{53 c_\theta^4 M_\theta^8 M_\pi^4 s_\theta^8}{31\,104 \pi^2 M_{\eta'}^8} - \\
& \frac{25 \operatorname{Log}\left[\frac{M_\eta^2}{\mu^2}\right] c_\theta^4 M_\theta^8 M_\pi^4 s_\theta^8}{7776 \pi^2 M_{\eta'}^8} - \frac{49 \operatorname{Log}\left[\frac{M_{\eta'}^2}{\mu^2}\right] c_\theta^4 M_\theta^8 M_\pi^4 s_\theta^8}{93\,312 \pi^2 M_{\eta'}^8} + \frac{6\,062\,080 c_\theta^4 L_8^2 r M_\theta^8 M_K^{10} s_\theta^8}{729 F^2 M_\eta^8 M_{\eta'}^8} - \\
& \frac{5\,183\,488 c_\theta^4 L_8^2 r M_\theta^8 M_K^8 M_\pi^2 s_\theta^8}{243 F^2 M_\eta^4 M_{\eta'}^8} + \frac{20\,480 c_\theta^4 L_8^2 r M_\theta^8 M_K^6 M_\pi^4 s_\theta^8}{F^2 M_\eta^4 M_{\eta'}^8} - \frac{5\,862\,400 c_\theta^4 L_8^2 r M_\theta^8 M_K^4 M_\pi^6 s_\theta^8}{729 F^2 M_\eta^4 M_{\eta'}^8} +
\end{aligned}$$

$$\begin{aligned}
& \frac{108\,032\,c_\theta^4\,L_8^2\,r\,M_\theta^8\,M_K^2\,M_\pi^8\,s_\theta^8}{243\,F^2\,M_\eta^4\,M_{\eta'}^8} + \frac{128\,c_\theta^4\,L_8^2\,r\,M_\theta^8\,M_\pi^{10}\,s_\theta^8}{27\,F^2\,M_\eta^4\,M_{\eta'}^8} + \frac{3\,604\,480\,c_\theta^4\,L_8^2\,r\,M_\theta^8\,M_K^{10}\,s_\theta^8}{729\,F^2\,M_\eta^6\,M_{\eta'}^6} - \\
& \frac{2\,711\,552\,c_\theta^4\,L_8^2\,r\,M_\theta^8\,M_K^2\,M_\pi^2\,s_\theta^8}{243\,F^2\,M_\eta^6\,M_{\eta'}^6} + \frac{1\,703\,936\,c_\theta^4\,L_8^2\,r\,M_\theta^8\,M_K^6\,M_\pi^4\,s_\theta^8}{243\,F^2\,M_\eta^6\,M_{\eta'}^6} - \frac{495\,616\,c_\theta^4\,L_8^2\,r\,M_\theta^8\,M_K^4\,M_\pi^6\,s_\theta^8}{729\,F^2\,M_\eta^6\,M_{\eta'}^6} - \\
& \frac{28\,672\,c_\theta^4\,L_8^2\,r\,M_\theta^8\,M_K^2\,M_\pi^8\,s_\theta^8}{243\,F^2\,M_\eta^6\,M_{\eta'}^6} - \frac{1024\,c_\theta^4\,L_8^2\,r\,M_\theta^8\,M_\pi^{10}\,s_\theta^8}{27\,F^2\,M_\eta^6\,M_{\eta'}^6} - \frac{2\,\text{Log}\left[\frac{M_K^2}{\mu^2}\right]\,c_\theta^2\,M_\theta^8\,M_K^6\,s_\theta^8}{81\,\pi^2\,M_\eta^4\,M_{\eta'}^6} + \\
& \frac{2048\,c_\theta^2\,L_6^r\,M_\theta^8\,M_K^6\,s_\theta^8}{81\,M_\eta^4\,M_{\eta'}^6} + \frac{2048\,c_\theta^2\,L_7^r\,M_\theta^8\,M_K^6\,s_\theta^8}{81\,M_\eta^4\,M_{\eta'}^6} - \frac{512\,c_\theta^2\,L_{25}^r\,M_\theta^8\,M_K^6\,s_\theta^8}{27\,M_\eta^4\,M_{\eta'}^6} + \frac{4096\,c_\theta^2\,C_{19}\,M_\theta^8\,M_K^8\,s_\theta^8}{27\,M_\eta^4\,M_{\eta'}^6} + \\
& \frac{8192\,c_\theta^2\,C_{31}\,M_\theta^8\,M_K^8\,s_\theta^8}{81\,M_\eta^4\,M_{\eta'}^6} + \frac{11\,\text{Log}\left[\frac{M_K^2}{\mu^2}\right]\,c_\theta^2\,M_\theta^8\,M_K^4\,M_\pi^2\,s_\theta^8}{324\,\pi^2\,M_\eta^4\,M_{\eta'}^6} - \frac{128\,c_\theta^2\,L_6^r\,M_\theta^8\,M_K^4\,M_\pi^2\,s_\theta^8}{9\,M_\eta^4\,M_{\eta'}^6} - \\
& \frac{128\,c_\theta^2\,L_7^r\,M_\theta^8\,M_K^4\,M_\pi^2\,s_\theta^8}{3\,M_\eta^4\,M_{\eta'}^6} + \frac{832\,c_\theta^2\,L_{25}^r\,M_\theta^8\,M_K^4\,M_\pi^2\,s_\theta^8}{27\,M_\eta^4\,M_{\eta'}^6} - \frac{7936\,c_\theta^2\,C_{19}\,M_\theta^8\,M_K^6\,M_\pi^2\,s_\theta^8}{27\,M_\eta^4\,M_{\eta'}^6} - \\
& \frac{15\,872\,c_\theta^2\,C_{31}\,M_\theta^8\,M_K^6\,M_\pi^2\,s_\theta^8}{81\,M_\eta^4\,M_{\eta'}^6} - \frac{\text{Log}\left[\frac{M_K^2}{\mu^2}\right]\,c_\theta^2\,M_\theta^8\,M_K^2\,M_\pi^4\,s_\theta^8}{108\,\pi^2\,M_\eta^4\,M_{\eta'}^6} + \frac{\text{Log}\left[\frac{M_\pi^2}{\mu^2}\right]\,c_\theta^2\,M_\theta^8\,M_K^2\,M_\pi^4\,s_\theta^8}{108\,\pi^2\,M_\eta^4\,M_{\eta'}^6} - \\
& \frac{128\,c_\theta^2\,L_6^r\,M_\theta^8\,M_K^2\,M_\pi^4\,s_\theta^8}{27\,M_\eta^4\,M_{\eta'}^6} + \frac{448\,c_\theta^2\,L_7^r\,M_\theta^8\,M_K^2\,M_\pi^4\,s_\theta^8}{27\,M_\eta^4\,M_{\eta'}^6} - \frac{320\,c_\theta^2\,L_{25}^r\,M_\theta^8\,M_K^2\,M_\pi^4\,s_\theta^8}{27\,M_\eta^4\,M_{\eta'}^6} + \\
& \frac{640\,c_\theta^2\,C_{19}\,M_\theta^8\,M_K^4\,M_\pi^4\,s_\theta^8}{3\,M_\eta^4\,M_{\eta'}^6} + \frac{1280\,c_\theta^2\,C_{31}\,M_\theta^8\,M_K^4\,M_\pi^4\,s_\theta^8}{9\,M_\eta^4\,M_{\eta'}^6} - \frac{\text{Log}\left[\frac{M_\pi^2}{\mu^2}\right]\,c_\theta^2\,M_\theta^8\,M_\pi^6\,s_\theta^8}{108\,\pi^2\,M_\eta^4\,M_{\eta'}^6} + \\
& \frac{352\,c_\theta^2\,L_6^r\,M_\theta^8\,M_\pi^6\,s_\theta^8}{81\,M_\eta^4\,M_{\eta'}^6} + \frac{64\,c_\theta^2\,L_7^r\,M_\theta^8\,M_\pi^6\,s_\theta^8}{81\,M_\eta^4\,M_{\eta'}^6} - \frac{1984\,c_\theta^2\,C_{19}\,M_\theta^8\,M_K^2\,M_\pi^6\,s_\theta^8}{27\,M_\eta^4\,M_{\eta'}^6} - \frac{3968\,c_\theta^2\,C_{31}\,M_\theta^8\,M_K^2\,M_\pi^6\,s_\theta^8}{81\,M_\eta^4\,M_{\eta'}^6} + \\
& \frac{352\,c_\theta^2\,C_{19}\,M_\theta^8\,M_\pi^8\,s_\theta^8}{27\,M_\eta^4\,M_{\eta'}^6} + \frac{704\,c_\theta^2\,C_{31}\,M_\theta^8\,M_\pi^8\,s_\theta^8}{81\,M_\eta^4\,M_{\eta'}^6} + \frac{13\,c_\theta^4\,M_\theta^8\,M_K^4\,s_\theta^8}{243\,\pi^2\,M_\eta^2\,M_{\eta'}^6} + \frac{19\,\text{Log}\left[\frac{M_\eta^2}{\mu^2}\right]\,c_\theta^4\,M_\theta^8\,M_K^4\,s_\theta^8}{729\,\pi^2\,M_\eta^2\,M_{\eta'}^6} - \\
& \frac{8\,\text{Log}\left[\frac{M_\eta^2}{\mu^2}\right]\,c_\theta^4\,M_\theta^8\,M_K^4\,s_\theta^8}{243\,\pi^2\,M_\eta^2\,M_{\eta'}^6} - \frac{31\,c_\theta^4\,M_\theta^8\,M_K^2\,M_\pi^2\,s_\theta^8}{486\,\pi^2\,M_\eta^2\,M_{\eta'}^6} - \frac{65\,\text{Log}\left[\frac{M_\eta^2}{\mu^2}\right]\,c_\theta^4\,M_\theta^8\,M_K^2\,M_\pi^2\,s_\theta^8}{2916\,\pi^2\,M_\eta^2\,M_{\eta'}^6} + \\
& \frac{35\,\text{Log}\left[\frac{M_\eta^2}{\mu^2}\right]\,c_\theta^4\,M_\theta^8\,M_K^2\,M_\pi^2\,s_\theta^8}{972\,\pi^2\,M_\eta^2\,M_{\eta'}^6} + \frac{161\,c_\theta^4\,M_\theta^8\,M_\pi^4\,s_\theta^8}{7776\,\pi^2\,M_\eta^2\,M_{\eta'}^6} + \frac{4\,\text{Log}\left[\frac{M_\eta^2}{\mu^2}\right]\,c_\theta^4\,M_\theta^8\,M_\pi^4\,s_\theta^8}{729\,\pi^2\,M_\eta^2\,M_{\eta'}^6} - \\
& \frac{\text{Log}\left[\frac{M_\eta^2}{\mu^2}\right]\,c_\theta^4\,M_\theta^8\,M_\pi^4\,s_\theta^8}{96\,\pi^2\,M_\eta^2\,M_{\eta'}^6} - \frac{12\,738\,560\,c_\theta^4\,L_8^2\,r\,M_\theta^8\,M_K^{10}\,s_\theta^8}{729\,F^2\,M_\eta^8\,M_{\eta'}^4} + \frac{1\,146\,880\,c_\theta^4\,L_8^2\,r\,M_\theta^8\,M_K^8\,M_\pi^2\,s_\theta^8}{27\,F^2\,M_\eta^8\,M_{\eta'}^4} - \\
& \frac{8\,474\,624\,c_\theta^4\,L_8^2\,r\,M_\theta^8\,M_K^6\,M_\pi^4\,s_\theta^8}{243\,F^2\,M_\eta^8\,M_{\eta'}^4} + \frac{7\,374\,848\,c_\theta^4\,L_8^2\,r\,M_\theta^8\,M_K^4\,M_\pi^6\,s_\theta^8}{729\,F^2\,M_\eta^8\,M_{\eta'}^4} + \frac{512\,c_\theta^4\,L_8^2\,r\,M_\theta^8\,M_K^2\,M_\pi^8\,s_\theta^8}{243\,F^2\,M_\eta^8\,M_{\eta'}^4} - \\
& \frac{3968\,c_\theta^4\,L_8^2\,r\,M_\theta^8\,M_\pi^{10}\,s_\theta^8}{27\,F^2\,M_\eta^8\,M_{\eta'}^4} + \frac{64\,F^2\,v_2^{(2)}\,c_\theta^2\,M_\theta^8\,M_K^4\,s_\theta^8}{9\,M_\eta^6\,M_{\eta'}^4} - \frac{11\,\text{Log}\left[\frac{M_K^2}{\mu^2}\right]\,c_\theta^2\,M_\theta^8\,M_K^6\,s_\theta^8}{243\,\pi^2\,M_\eta^6\,M_{\eta'}^4} - \frac{1024\,c_\theta^2\,L_6^r\,M_\theta^8\,M_K^6\,s_\theta^8}{81\,M_\eta^6\,M_{\eta'}^4} -
\end{aligned}$$

$$\begin{aligned}
& \frac{1024 c_{\theta}^2 L_7^r M_0^8 M_K^6 S_{\theta}^8}{81 M_{\eta}^6 M_{\eta'}^4} - \frac{2816 c_{\theta}^2 L_{25}^r M_0^8 M_K^6 S_{\theta}^8}{81 M_{\eta}^6 M_{\eta'}^4} - \frac{2048 c_{\theta}^2 C_{19} M_0^8 M_K^8 S_{\theta}^8}{27 M_{\eta}^6 M_{\eta'}^4} - \frac{4096 c_{\theta}^2 C_{31} M_0^8 M_K^8 S_{\theta}^8}{81 M_{\eta}^6 M_{\eta'}^4} + \\
& \frac{16 F^2 v_2^{(2)} c_{\theta}^2 M_0^8 M_K^2 M_{\pi}^2 S_{\theta}^8}{9 M_{\eta}^6 M_{\eta'}^4} + \frac{13 \text{Log}\left[\frac{M_K^2}{\mu^2}\right] c_{\theta}^2 M_0^8 M_K^4 M_{\pi}^2 S_{\theta}^8}{972 \pi^2 M_{\eta}^6 M_{\eta'}^4} + \frac{128 c_{\theta}^2 L_6^r M_0^8 M_K^4 M_{\pi}^2 S_{\theta}^8}{27 M_{\eta}^6 M_{\eta'}^4} + \\
& \frac{512 c_{\theta}^2 L_7^r M_0^8 M_K^4 M_{\pi}^2 S_{\theta}^8}{9 M_{\eta}^6 M_{\eta'}^4} + \frac{4480 c_{\theta}^2 L_{25}^r M_0^8 M_K^4 M_{\pi}^2 S_{\theta}^8}{81 M_{\eta}^6 M_{\eta'}^4} + \frac{2560 c_{\theta}^2 C_{19} M_0^8 M_K^6 M_{\pi}^2 S_{\theta}^8}{27 M_{\eta}^6 M_{\eta'}^4} + \\
& \frac{5120 c_{\theta}^2 C_{31} M_0^8 M_K^6 M_{\pi}^2 S_{\theta}^8}{81 M_{\eta}^6 M_{\eta'}^4} - \frac{8 F^2 v_2^{(2)} c_{\theta}^2 M_0^8 M_K^4 S_{\theta}^8}{9 M_{\eta}^6 M_{\eta'}^4} - \frac{7 \text{Log}\left[\frac{M_K^2}{\mu^2}\right] c_{\theta}^2 M_0^8 M_K^2 M_{\pi}^4 S_{\theta}^8}{1944 \pi^2 M_{\eta}^6 M_{\eta'}^4} - \\
& \frac{5 \text{Log}\left[\frac{M_{\pi}^2}{\mu^2}\right] c_{\theta}^2 M_0^8 M_K^2 M_{\pi}^4 S_{\theta}^8}{216 \pi^2 M_{\eta}^6 M_{\eta'}^4} + \frac{256 c_{\theta}^2 L_6^r M_0^8 M_K^2 M_{\pi}^4 S_{\theta}^8}{27 M_{\eta}^6 M_{\eta'}^4} - \frac{896 c_{\theta}^2 L_7^r M_0^8 M_K^2 M_{\pi}^4 S_{\theta}^8}{27 M_{\eta}^6 M_{\eta'}^4} - \\
& \frac{3968 c_{\theta}^2 L_{25}^r M_0^8 M_K^2 M_{\pi}^4 S_{\theta}^8}{81 M_{\eta}^6 M_{\eta'}^4} - \frac{256 c_{\theta}^2 C_{19} M_0^8 M_K^4 M_{\pi}^4 S_{\theta}^8}{9 M_{\eta}^6 M_{\eta'}^4} - \frac{512 c_{\theta}^2 C_{31} M_0^8 M_K^4 M_{\pi}^4 S_{\theta}^8}{27 M_{\eta}^6 M_{\eta'}^4} - \\
& \frac{\text{Log}\left[\frac{M_{\pi}^2}{\mu^2}\right] c_{\theta}^2 M_0^8 M_{\pi}^6 S_{\theta}^8}{144 \pi^2 M_{\eta}^6 M_{\eta'}^4} + \frac{160 c_{\theta}^2 L_6^r M_0^8 M_{\pi}^6 S_{\theta}^8}{81 M_{\eta}^6 M_{\eta'}^4} + \frac{832 c_{\theta}^2 L_7^r M_0^8 M_{\pi}^6 S_{\theta}^8}{81 M_{\eta}^6 M_{\eta'}^4} + \frac{64 c_{\theta}^2 L_{25}^r M_0^8 M_{\pi}^6 S_{\theta}^8}{9 M_{\eta}^6 M_{\eta'}^4} + \\
& \frac{64 c_{\theta}^2 C_{19} M_0^8 M_K^2 M_{\pi}^6 S_{\theta}^8}{9 M_{\eta}^6 M_{\eta'}^4} + \frac{128 c_{\theta}^2 C_{31} M_0^8 M_K^2 M_{\pi}^6 S_{\theta}^8}{27 M_{\eta}^6 M_{\eta'}^4} + \frac{160 c_{\theta}^2 C_{19} M_0^8 M_{\pi}^8 S_{\theta}^8}{27 M_{\eta}^6 M_{\eta'}^4} + \frac{320 c_{\theta}^2 C_{31} M_0^8 M_{\pi}^8 S_{\theta}^8}{81 M_{\eta}^6 M_{\eta'}^4} + \\
& \frac{17 c_{\theta}^4 M_0^8 M_K^4 S_{\theta}^8}{324 \pi^2 M_{\eta}^4 M_{\eta'}^4} - \frac{199 \text{Log}\left[\frac{M_{\eta}^2}{\mu^2}\right] c_{\theta}^4 M_0^8 M_K^4 S_{\theta}^8}{2916 \pi^2 M_{\eta}^4 M_{\eta'}^4} + \frac{23 \text{Log}\left[\frac{M_{\eta}^2}{\mu^2}\right] c_{\theta}^4 M_0^8 M_K^4 S_{\theta}^8}{729 \pi^2 M_{\eta}^4 M_{\eta'}^4} - \frac{23 c_{\theta}^4 M_0^8 M_K^2 M_{\pi}^2 S_{\theta}^8}{648 \pi^2 M_{\eta}^4 M_{\eta'}^4} + \\
& \frac{689 \text{Log}\left[\frac{M_{\eta}^2}{\mu^2}\right] c_{\theta}^4 M_0^8 M_K^2 M_{\pi}^2 S_{\theta}^8}{11\,664 \pi^2 M_{\eta}^4 M_{\eta'}^4} - \frac{499 \text{Log}\left[\frac{M_{\eta}^2}{\mu^2}\right] c_{\theta}^4 M_0^8 M_K^2 M_{\pi}^2 S_{\theta}^8}{11\,664 \pi^2 M_{\eta}^4 M_{\eta'}^4} + \frac{41 c_{\theta}^4 M_0^8 M_{\pi}^4 S_{\theta}^8}{5184 \pi^2 M_{\eta}^4 M_{\eta'}^4} - \\
& \frac{245 \text{Log}\left[\frac{M_{\eta}^2}{\mu^2}\right] c_{\theta}^4 M_0^8 M_{\pi}^4 S_{\theta}^8}{23\,328 \pi^2 M_{\eta}^4 M_{\eta'}^4} + \frac{407 \text{Log}\left[\frac{M_{\eta}^2}{\mu^2}\right] c_{\theta}^4 M_0^8 M_{\pi}^4 S_{\theta}^8}{46\,656 \pi^2 M_{\eta}^4 M_{\eta'}^4} + \frac{\text{Log}\left[\frac{M_{\eta}^2}{\mu^2}\right] c_{\theta}^2 M_0^8 M_K^2 S_{\theta}^8}{324 \pi^2 M_{\eta}^2 M_{\eta'}^4} - \\
& \frac{\text{Log}\left[\frac{M_{\eta}^2}{\mu^2}\right] c_{\theta}^2 M_0^8 M_{\pi}^2 S_{\theta}^8}{1296 \pi^2 M_{\eta}^2 M_{\eta'}^4} + \frac{16\,875\,520 c_{\theta}^4 L_8^2 r M_0^8 M_K^{10} S_{\theta}^8}{729 F^2 M_{\eta}^{10} M_{\eta'}^2} - \frac{13\,975\,552 c_{\theta}^4 L_8^2 r M_0^8 M_K^8 M_{\pi}^2 S_{\theta}^8}{243 F^2 M_{\eta}^{10} M_{\eta'}^2} + \\
& \frac{4\,341\,760 c_{\theta}^4 L_8^2 r M_0^8 M_K^6 M_{\pi}^4 S_{\theta}^8}{81 F^2 M_{\eta}^{10} M_{\eta'}^2} - \frac{16\,703\,488 c_{\theta}^4 L_8^2 r M_0^8 M_K^4 M_{\pi}^6 S_{\theta}^8}{729 F^2 M_{\eta}^{10} M_{\eta'}^2} + \frac{1\,040\,384 c_{\theta}^4 L_8^2 r M_0^8 M_K^2 M_{\pi}^8 S_{\theta}^8}{243 F^2 M_{\eta}^{10} M_{\eta'}^2} - \\
& \frac{8704 c_{\theta}^4 L_8^2 r M_0^8 M_{\pi}^{10} S_{\theta}^8}{27 F^2 M_{\eta}^{10} M_{\eta'}^2} - \frac{304 F^2 v_2^{(2)} c_{\theta}^2 M_0^8 M_K^4 S_{\theta}^8}{27 M_{\eta}^8 M_{\eta'}^2} + \frac{\text{Log}\left[\frac{M_K^2}{\mu^2}\right] c_{\theta}^2 M_0^8 M_K^6 S_{\theta}^8}{9 \pi^2 M_{\eta}^8 M_{\eta'}^2} - \frac{256 c_{\theta}^2 L_6^r M_0^8 M_K^6 S_{\theta}^8}{9 M_{\eta}^8 M_{\eta'}^2} - \\
& \frac{256 c_{\theta}^2 L_7^r M_0^8 M_K^6 S_{\theta}^8}{9 M_{\eta}^8 M_{\eta'}^2} + \frac{256 c_{\theta}^2 L_{25}^r M_0^8 M_K^6 S_{\theta}^8}{3 M_{\eta}^8 M_{\eta'}^2} - \frac{512 c_{\theta}^2 C_{19} M_0^8 M_K^8 S_{\theta}^8}{3 M_{\eta}^8 M_{\eta'}^2} - \frac{1024 c_{\theta}^2 C_{31} M_0^8 M_K^8 S_{\theta}^8}{9 M_{\eta}^8 M_{\eta'}^2} -
\end{aligned}$$



$$\begin{aligned}
& \frac{16 F^2 v_2^{(2)} c_\theta^2 M_\theta^8 M_K^2 M_\pi^2 s_\theta^8}{27 M_\eta^8 M_{\eta'}^2} - \frac{29 \text{Log}\left[\frac{M_K^2}{\mu^2}\right] c_\theta^2 M_\theta^8 M_K^4 M_\pi^2 s_\theta^8}{324 \pi^2 M_\eta^8 M_{\eta'}^2} + \frac{1280 c_\theta^2 L_6^r M_\theta^8 M_K^4 M_\pi^2 s_\theta^8}{81 M_\eta^8 M_{\eta'}^2} - \\
& \frac{256 c_\theta^2 L_7^r M_\theta^8 M_K^4 M_\pi^2 s_\theta^8}{81 M_\eta^8 M_{\eta'}^2} - \frac{3904 c_\theta^2 L_{25}^r M_\theta^8 M_K^4 M_\pi^2 s_\theta^8}{27 M_\eta^8 M_{\eta'}^2} + \frac{11\,008 c_\theta^2 C_{19} M_\theta^8 M_K^6 M_\pi^2 s_\theta^8}{27 M_\eta^8 M_{\eta'}^2} + \\
& \frac{22\,016 c_\theta^2 C_{31} M_\theta^8 M_K^6 M_\pi^2 s_\theta^8}{81 M_\eta^8 M_{\eta'}^2} + \frac{68 F^2 v_2^{(2)} c_\theta^2 M_\theta^8 M_K^4 s_\theta^8}{27 M_\eta^8 M_{\eta'}^2} + \frac{\text{Log}\left[\frac{M_K^2}{\mu^2}\right] c_\theta^2 M_\theta^8 M_K^2 M_\pi^4 s_\theta^8}{54 \pi^2 M_\eta^8 M_{\eta'}^2} + \\
& \frac{\text{Log}\left[\frac{M_\pi^2}{\mu^2}\right] c_\theta^2 M_\theta^8 M_K^2 M_\pi^4 s_\theta^8}{36 \pi^2 M_\eta^8 M_{\eta'}^2} - \frac{64 c_\theta^2 L_6^r M_\theta^8 M_K^2 M_\pi^4 s_\theta^8}{81 M_\eta^8 M_{\eta'}^2} + \frac{1664 c_\theta^2 L_7^r M_\theta^8 M_K^2 M_\pi^4 s_\theta^8}{81 M_\eta^8 M_{\eta'}^2} + \\
& \frac{2816 c_\theta^2 L_{25}^r M_\theta^8 M_K^2 M_\pi^4 s_\theta^8}{27 M_\eta^8 M_{\eta'}^2} - \frac{3200 c_\theta^2 C_{19} M_\theta^8 M_K^4 M_\pi^4 s_\theta^8}{9 M_\eta^8 M_{\eta'}^2} - \frac{6400 c_\theta^2 C_{31} M_\theta^8 M_K^4 M_\pi^4 s_\theta^8}{27 M_\eta^8 M_{\eta'}^2} + \\
& \frac{\text{Log}\left[\frac{M_\pi^2}{\mu^2}\right] c_\theta^2 M_\theta^8 M_\pi^6 s_\theta^8}{108 \pi^2 M_\eta^8 M_{\eta'}^2} - \frac{640 c_\theta^2 L_6^r M_\theta^8 M_\pi^6 s_\theta^8}{81 M_\eta^8 M_{\eta'}^2} - \frac{1120 c_\theta^2 L_7^r M_\theta^8 M_\pi^6 s_\theta^8}{81 M_\eta^8 M_{\eta'}^2} - \frac{544 c_\theta^2 L_{25}^r M_\theta^8 M_\pi^6 s_\theta^8}{27 M_\eta^8 M_{\eta'}^2} + \\
& \frac{1088 c_\theta^2 C_{19} M_\theta^8 M_K^2 M_\pi^6 s_\theta^8}{9 M_\eta^8 M_{\eta'}^2} + \frac{2176 c_\theta^2 C_{31} M_\theta^8 M_K^2 M_\pi^6 s_\theta^8}{27 M_\eta^8 M_{\eta'}^2} - \frac{640 c_\theta^2 C_{19} M_\theta^8 M_\pi^8 s_\theta^8}{27 M_\eta^8 M_{\eta'}^2} - \\
& \frac{1280 c_\theta^2 C_{31} M_\theta^8 M_\pi^8 s_\theta^8}{81 M_\eta^8 M_{\eta'}^2} - \frac{47 c_\theta^4 M_\theta^8 M_K^4 s_\theta^8}{243 \pi^2 M_\eta^6 M_{\eta'}^2} + \frac{2 \text{Log}\left[\frac{M_\eta^2}{\mu^2}\right] c_\theta^4 M_\theta^8 M_K^4 s_\theta^8}{27 \pi^2 M_\eta^6 M_{\eta'}^2} + \frac{10 \text{Log}\left[\frac{M_{\eta'}^2}{\mu^2}\right] c_\theta^4 M_\theta^8 M_K^4 s_\theta^8}{729 \pi^2 M_\eta^6 M_{\eta'}^2} + \\
& \frac{181 c_\theta^4 M_\theta^8 M_K^2 M_\pi^2 s_\theta^8}{972 \pi^2 M_\eta^6 M_{\eta'}^2} - \frac{47 \text{Log}\left[\frac{M_\eta^2}{\mu^2}\right] c_\theta^4 M_\theta^8 M_K^2 M_\pi^2 s_\theta^8}{648 \pi^2 M_\eta^6 M_{\eta'}^2} + \frac{65 \text{Log}\left[\frac{M_{\eta'}^2}{\mu^2}\right] c_\theta^4 M_\theta^8 M_K^2 M_\pi^2 s_\theta^8}{5832 \pi^2 M_\eta^6 M_{\eta'}^2} - \\
& \frac{331 c_\theta^4 M_\theta^8 M_\pi^4 s_\theta^8}{7776 \pi^2 M_\eta^6 M_{\eta'}^2} + \frac{11 \text{Log}\left[\frac{M_\eta^2}{\mu^2}\right] c_\theta^4 M_\theta^8 M_\pi^4 s_\theta^8}{648 \pi^2 M_\eta^6 M_{\eta'}^2} - \frac{175 \text{Log}\left[\frac{M_{\eta'}^2}{\mu^2}\right] c_\theta^4 M_\theta^8 M_\pi^4 s_\theta^8}{23\,328 \pi^2 M_\eta^6 M_{\eta'}^2} - \\
& \frac{\text{Log}\left[\frac{M_\eta^2}{\mu^2}\right] c_\theta^2 M_\theta^8 M_K^2 s_\theta^8}{108 \pi^2 M_\eta^4 M_{\eta'}^2} + \frac{\text{Log}\left[\frac{M_{\eta'}^2}{\mu^2}\right] c_\theta^2 M_\theta^8 M_K^2 s_\theta^8}{162 \pi^2 M_\eta^4 M_{\eta'}^2} + \frac{\text{Log}\left[\frac{M_\pi^2}{\mu^2}\right] c_\theta^2 M_\theta^8 M_\pi^2 s_\theta^8}{324 \pi^2 M_\eta^4 M_{\eta'}^2} - \\
& \frac{7 \text{Log}\left[\frac{M_\eta^2}{\mu^2}\right] c_\theta^2 M_\theta^8 M_\pi^2 s_\theta^8}{2592 \pi^2 M_\eta^4 M_{\eta'}^2} + \frac{5 \text{Log}\left[\frac{M_{\eta'}^2}{\mu^2}\right] c_\theta^4 M_\theta^8 M_K^4 M_{\eta'}^2 s_\theta^8}{729 \pi^2 M_\eta^{10}} - \frac{5 \text{Log}\left[\frac{M_\pi^2}{\mu^2}\right] c_\theta^4 M_\theta^8 M_K^2 M_\pi^2 M_{\eta'}^2 s_\theta^8}{1458 \pi^2 M_\eta^{10}} + \\
& \frac{5 \text{Log}\left[\frac{M_\eta^2}{\mu^2}\right] c_\theta^4 M_\theta^8 M_\pi^4 M_{\eta'}^2 s_\theta^8}{11\,664 \pi^2 M_\eta^{10}} + \frac{\text{Log}\left[\frac{M_\eta^2}{\mu^2}\right] c_\theta^2 M_\theta^8 M_K^2 M_{\eta'}^2 s_\theta^8}{432 \pi^2 M_\eta^8} - \frac{\text{Log}\left[\frac{M_{\eta'}^2}{\mu^2}\right] c_\theta^2 M_\theta^8 M_\pi^2 M_{\eta'}^2 s_\theta^8}{648 \pi^2 M_\eta^8} - \\
& \frac{5 \text{Log}\left[\frac{M_\eta^2}{\mu^2}\right] c_\theta^4 M_\theta^8 M_K^4 s_\theta^8}{486 \pi^2 M_\eta^6 (M_\eta^2 - M_{\eta'}^2)} - \frac{11 \text{Log}\left[\frac{M_{\eta'}^2}{\mu^2}\right] c_\theta^4 M_\theta^8 M_K^4 s_\theta^8}{243 \pi^2 M_\eta^6 (M_\eta^2 - M_{\eta'}^2)} + \frac{19 \text{Log}\left[\frac{M_\pi^2}{\mu^2}\right] c_\theta^4 M_\theta^8 M_K^2 M_\pi^2 s_\theta^8}{1944 \pi^2 M_\eta^6 (M_\eta^2 - M_{\eta'}^2)} + \\
& \frac{37 \text{Log}\left[\frac{M_\eta^2}{\mu^2}\right] c_\theta^4 M_\theta^8 M_K^2 M_\pi^2 s_\theta^8}{972 \pi^2 M_\eta^6 (M_\eta^2 - M_{\eta'}^2)} - \frac{23 \text{Log}\left[\frac{M_\eta^2}{\mu^2}\right] c_\theta^4 M_\theta^8 M_\pi^4 s_\theta^8}{7776 \pi^2 M_\eta^6 (M_\eta^2 - M_{\eta'}^2)} - \frac{13 \text{Log}\left[\frac{M_{\eta'}^2}{\mu^2}\right] c_\theta^4 M_\theta^8 M_\pi^4 s_\theta^8}{1944 \pi^2 M_\eta^6 (M_\eta^2 - M_{\eta'}^2)} +
\end{aligned}$$

$$\begin{aligned}
& \frac{2 \operatorname{Log}\left[\frac{M_\eta^2}{\mu^2}\right] c_\theta^4 M_0^8 M_K^4 M_\pi^2 s_\theta^8}{243 \pi^2 M_{\eta'}^8 (M_\eta^2 - M_{\eta'}^2)} - \frac{5 \operatorname{Log}\left[\frac{M_\eta^2}{\mu^2}\right] c_\theta^4 M_0^8 M_K^2 M_\pi^2 M_\eta^2 s_\theta^8}{486 \pi^2 M_{\eta'}^8 (M_\eta^2 - M_{\eta'}^2)} + \frac{25 \operatorname{Log}\left[\frac{M_\eta^2}{\mu^2}\right] c_\theta^4 M_0^8 M_\pi^4 M_\eta^2 s_\theta^8}{7776 \pi^2 M_{\eta'}^8 (M_\eta^2 - M_{\eta'}^2)} - \\
& \frac{4 \operatorname{Log}\left[\frac{M_\eta^2}{\mu^2}\right] c_\theta^4 M_0^8 M_K^4 s_\theta^8}{243 \pi^2 M_{\eta'}^6 (M_\eta^2 - M_{\eta'}^2)} - \frac{2 \operatorname{Log}\left[\frac{M_\eta^2}{\mu^2}\right] c_\theta^4 M_0^8 M_K^4 s_\theta^8}{243 \pi^2 M_{\eta'}^6 (M_\eta^2 - M_{\eta'}^2)} + \frac{13 \operatorname{Log}\left[\frac{M_\eta^2}{\mu^2}\right] c_\theta^4 M_0^8 M_K^2 M_\pi^2 s_\theta^8}{486 \pi^2 M_{\eta'}^6 (M_\eta^2 - M_{\eta'}^2)} + \\
& \frac{5 \operatorname{Log}\left[\frac{M_\eta^2}{\mu^2}\right] c_\theta^4 M_0^8 M_K^2 M_\pi^2 s_\theta^8}{486 \pi^2 M_{\eta'}^6 (M_\eta^2 - M_{\eta'}^2)} - \frac{11 \operatorname{Log}\left[\frac{M_\eta^2}{\mu^2}\right] c_\theta^4 M_0^8 M_\pi^4 s_\theta^8}{1944 \pi^2 M_{\eta'}^6 (M_\eta^2 - M_{\eta'}^2)} - \frac{25 \operatorname{Log}\left[\frac{M_\eta^2}{\mu^2}\right] c_\theta^4 M_0^8 M_\pi^4 s_\theta^8}{7776 \pi^2 M_{\eta'}^6 (M_\eta^2 - M_{\eta'}^2)} - \\
& \frac{2 \operatorname{Log}\left[\frac{M_\eta^2}{\mu^2}\right] c_\theta^4 M_0^8 M_K^4 s_\theta^8}{81 \pi^2 M_\eta^2 M_{\eta'}^4 (M_\eta^2 - M_{\eta'}^2)} + \frac{4 \operatorname{Log}\left[\frac{M_\eta^2}{\mu^2}\right] c_\theta^4 M_0^8 M_K^4 s_\theta^8}{243 \pi^2 M_\eta^2 M_{\eta'}^4 (M_\eta^2 - M_{\eta'}^2)} + \frac{5 \operatorname{Log}\left[\frac{M_\eta^2}{\mu^2}\right] c_\theta^4 M_0^8 M_K^2 M_\pi^2 s_\theta^8}{648 \pi^2 M_\eta^2 M_{\eta'}^4 (M_\eta^2 - M_{\eta'}^2)} - \\
& \frac{13 \operatorname{Log}\left[\frac{M_\eta^2}{\mu^2}\right] c_\theta^4 M_0^8 M_K^2 M_\pi^2 s_\theta^8}{486 \pi^2 M_\eta^2 M_{\eta'}^4 (M_\eta^2 - M_{\eta'}^2)} + \frac{\operatorname{Log}\left[\frac{M_\eta^2}{\mu^2}\right] c_\theta^4 M_0^8 M_\pi^4 s_\theta^8}{1296 \pi^2 M_\eta^2 M_{\eta'}^4 (M_\eta^2 - M_{\eta'}^2)} + \frac{11 \operatorname{Log}\left[\frac{M_\eta^2}{\mu^2}\right] c_\theta^4 M_0^8 M_\pi^4 s_\theta^8}{1944 \pi^2 M_\eta^2 M_{\eta'}^4 (M_\eta^2 - M_{\eta'}^2)} + \\
& \frac{11 \operatorname{Log}\left[\frac{M_\eta^2}{\mu^2}\right] c_\theta^4 M_0^8 M_K^4 s_\theta^8}{243 \pi^2 M_\eta^2 M_{\eta'}^2 (M_\eta^2 - M_{\eta'}^2)} + \frac{2 \operatorname{Log}\left[\frac{M_\eta^2}{\mu^2}\right] c_\theta^4 M_0^8 M_K^4 s_\theta^8}{81 \pi^2 M_\eta^2 M_{\eta'}^2 (M_\eta^2 - M_{\eta'}^2)} - \frac{37 \operatorname{Log}\left[\frac{M_\eta^2}{\mu^2}\right] c_\theta^4 M_0^8 M_K^2 M_\pi^2 s_\theta^8}{972 \pi^2 M_\eta^2 M_{\eta'}^2 (M_\eta^2 - M_{\eta'}^2)} - \\
& \frac{5 \operatorname{Log}\left[\frac{M_\eta^2}{\mu^2}\right] c_\theta^4 M_0^8 M_K^2 M_\pi^2 s_\theta^8}{648 \pi^2 M_\eta^2 M_{\eta'}^2 (M_\eta^2 - M_{\eta'}^2)} + \frac{13 \operatorname{Log}\left[\frac{M_\eta^2}{\mu^2}\right] c_\theta^4 M_0^8 M_\pi^4 s_\theta^8}{1944 \pi^2 M_\eta^2 M_{\eta'}^2 (M_\eta^2 - M_{\eta'}^2)} - \frac{\operatorname{Log}\left[\frac{M_\eta^2}{\mu^2}\right] c_\theta^4 M_0^8 M_\pi^4 s_\theta^8}{1296 \pi^2 M_\eta^2 M_{\eta'}^2 (M_\eta^2 - M_{\eta'}^2)} + \\
& \frac{5 \operatorname{Log}\left[\frac{M_\eta^2}{\mu^2}\right] c_\theta^4 M_0^8 M_K^4 M_\eta^2 s_\theta^8}{486 \pi^2 M_\eta^8 (M_\eta^2 - M_{\eta'}^2)} - \frac{19 \operatorname{Log}\left[\frac{M_\eta^2}{\mu^2}\right] c_\theta^4 M_0^8 M_K^2 M_\pi^2 M_\eta^2 s_\theta^8}{1944 \pi^2 M_\eta^8 (M_\eta^2 - M_{\eta'}^2)} + \frac{23 \operatorname{Log}\left[\frac{M_\eta^2}{\mu^2}\right] c_\theta^4 M_0^8 M_\pi^4 M_\eta^2 s_\theta^8}{7776 \pi^2 M_\eta^8 (M_\eta^2 - M_{\eta'}^2)} - \\
& \frac{4 587 520 \sqrt{2} c_\theta^3 L_8^2 r M_0^8 M_K^{10} s_\theta^9}{729 F^2 M_\eta^{12}} + \frac{3 891 200 \sqrt{2} c_\theta^3 L_8^2 r M_0^8 M_K^8 M_\pi^2 s_\theta^9}{243 F^2 M_\eta^{12}} - \\
& \frac{4 136 960 \sqrt{2} c_\theta^3 L_8^2 r M_0^8 M_K^6 M_\pi^4 s_\theta^9}{243 F^2 M_\eta^{12}} + \frac{6 676 480 \sqrt{2} c_\theta^3 L_8^2 r M_0^8 M_K^4 M_\pi^6 s_\theta^9}{729 F^2 M_\eta^{12}} - \\
& \frac{573 440 \sqrt{2} c_\theta^3 L_8^2 r M_0^8 M_K^2 M_\pi^8 s_\theta^9}{243 F^2 M_\eta^{12}} + \frac{33 280 \sqrt{2} c_\theta^3 L_8^2 r M_0^8 M_\pi^{10} s_\theta^9}{81 F^2 M_\eta^{12}} + \frac{64 \sqrt{2} F^2 v_2^{(2)} c_\theta M_0^8 M_K^4 s_\theta^9}{27 M_\eta^{10}} - \\
& \frac{5 \sqrt{2} \operatorname{Log}\left[\frac{M_K^2}{\mu^2}\right] c_\theta M_0^8 M_K^6 s_\theta^9}{243 \pi^2 M_\eta^{10}} + \frac{512 \sqrt{2} c_\theta L_6^r M_0^8 M_K^6 s_\theta^9}{81 M_\eta^{10}} + \frac{512 \sqrt{2} c_\theta L_7^r M_0^8 M_K^6 s_\theta^9}{81 M_\eta^{10}} - \\
& \frac{1280 \sqrt{2} c_\theta L_{25}^r M_0^8 M_K^6 s_\theta^9}{81 M_\eta^{10}} + \frac{1024 \sqrt{2} c_\theta C_{19} M_0^8 M_K^8 s_\theta^9}{27 M_\eta^{10}} + \frac{2048 \sqrt{2} c_\theta C_{31} M_0^8 M_K^8 s_\theta^9}{81 M_\eta^{10}} - \\
& \frac{32 \sqrt{2} F^2 v_2^{(2)} c_\theta M_0^8 M_K^2 M_\pi^2 s_\theta^9}{27 M_\eta^{10}} + \frac{4 \sqrt{2} \operatorname{Log}\left[\frac{M_K^2}{\mu^2}\right] c_\theta M_0^8 M_K^4 M_\pi^2 s_\theta^9}{243 \pi^2 M_\eta^{10}} + \frac{2176 \sqrt{2} c_\theta L_{25}^r M_0^8 M_K^4 M_\pi^2 s_\theta^9}{81 M_\eta^{10}} - \\
& \frac{2048 \sqrt{2} c_\theta C_{19} M_0^8 M_K^6 M_\pi^2 s_\theta^9}{27 M_\eta^{10}} - \frac{4096 \sqrt{2} c_\theta C_{31} M_0^8 M_K^6 M_\pi^2 s_\theta^9}{81 M_\eta^{10}} - \frac{32 \sqrt{2} F^2 v_2^{(2)} c_\theta M_0^8 M_\pi^4 s_\theta^9}{27 M_\eta^{10}} +
\end{aligned}$$

$$\begin{aligned}
& \frac{\text{Log}\left[\frac{M_K^2}{\mu^2}\right] c_\theta M_0^8 M_K^2 M_\pi^4 s_\theta^9}{486 \sqrt{2} \pi^2 M_\eta^{10}} + \frac{\text{Log}\left[\frac{M_\pi^2}{\mu^2}\right] c_\theta M_0^8 M_K^2 M_\pi^4 s_\theta^9}{162 \sqrt{2} \pi^2 M_\eta^{10}} - \frac{\sqrt{2} \text{Log}\left[\frac{M_\pi^2}{\mu^2}\right] c_\theta M_0^8 M_K^2 M_\pi^4 s_\theta^9}{81 \pi^2 M_\eta^{10}} - \\
& \frac{128 \sqrt{2} c_\theta L_6^r M_0^8 M_K^2 M_\pi^4 s_\theta^9}{27 M_\eta^{10}} - \frac{128 \sqrt{2} c_\theta L_7^r M_0^8 M_K^2 M_\pi^4 s_\theta^9}{27 M_\eta^{10}} - \frac{1664 \sqrt{2} c_\theta L_{25}^r M_0^8 M_K^2 M_\pi^4 s_\theta^9}{81 M_\eta^{10}} + \\
& \frac{512 \sqrt{2} c_\theta C_{19} M_0^8 M_K^4 M_\pi^4 s_\theta^9}{9 M_\eta^{10}} + \frac{1024 \sqrt{2} c_\theta C_{31} M_0^8 M_K^4 M_\pi^4 s_\theta^9}{27 M_\eta^{10}} + \frac{\text{Log}\left[\frac{M_\pi^2}{\mu^2}\right] c_\theta M_0^8 M_\pi^6 s_\theta^9}{324 \sqrt{2} \pi^2 M_\eta^{10}} + \\
& \frac{\sqrt{2} \text{Log}\left[\frac{M_\pi^2}{\mu^2}\right] c_\theta M_0^8 M_\pi^6 s_\theta^9}{81 \pi^2 M_\eta^{10}} - \frac{128 \sqrt{2} c_\theta L_6^r M_0^8 M_\pi^6 s_\theta^9}{81 M_\eta^{10}} - \frac{128 \sqrt{2} c_\theta L_7^r M_0^8 M_\pi^6 s_\theta^9}{81 M_\eta^{10}} + \\
& \frac{256 \sqrt{2} c_\theta L_{25}^r M_0^8 M_\pi^6 s_\theta^9}{27 M_\eta^{10}} - \frac{128 \sqrt{2} c_\theta C_{19} M_0^8 M_K^2 M_\pi^6 s_\theta^9}{9 M_\eta^{10}} - \frac{256 \sqrt{2} c_\theta C_{31} M_0^8 M_K^2 M_\pi^6 s_\theta^9}{27 M_\eta^{10}} - \\
& \frac{128 \sqrt{2} c_\theta C_{19} M_0^8 M_\pi^8 s_\theta^9}{27 M_\eta^{10}} - \frac{256 \sqrt{2} c_\theta C_{31} M_0^8 M_\pi^8 s_\theta^9}{81 M_\eta^{10}} + \frac{23 c_\theta^3 M_0^8 M_K^4 s_\theta^9}{243 \sqrt{2} \pi^2 M_\eta^8} - \\
& \frac{14 \sqrt{2} \text{Log}\left[\frac{M_\eta^2}{\mu^2}\right] c_\theta^3 M_0^8 M_K^4 s_\theta^9}{729 \pi^2 M_\eta^8} - \frac{5 \text{Log}\left[\frac{M_\eta^2}{\mu^2}\right] c_\theta^3 M_0^8 M_K^4 s_\theta^9}{243 \sqrt{2} \pi^2 M_\eta^8} + \frac{4 \sqrt{2} \text{Log}\left[\frac{M_\eta^2}{\mu^2}\right] c_\theta^3 M_0^8 M_K^4 s_\theta^9}{81 \pi^2 M_\eta^8} - \\
& \frac{14 \sqrt{2} c_\theta^3 M_0^8 M_K^2 M_\pi^2 s_\theta^9}{243 \pi^2 M_\eta^8} - \frac{5 \text{Log}\left[\frac{M_\eta^2}{\mu^2}\right] c_\theta^3 M_0^8 M_K^2 M_\pi^2 s_\theta^9}{486 \sqrt{2} \pi^2 M_\eta^8} + \frac{19 \sqrt{2} \text{Log}\left[\frac{M_\eta^2}{\mu^2}\right] c_\theta^3 M_0^8 M_K^2 M_\pi^2 s_\theta^9}{729 \pi^2 M_\eta^8} - \\
& \frac{5 \sqrt{2} \text{Log}\left[\frac{M_\eta^2}{\mu^2}\right] c_\theta^3 M_0^8 M_K^2 M_\pi^2 s_\theta^9}{243 \pi^2 M_\eta^8} + \frac{71 c_\theta^3 M_0^8 M_\pi^4 s_\theta^9}{3888 \sqrt{2} \pi^2 M_\eta^8} + \frac{77 \text{Log}\left[\frac{M_\eta^2}{\mu^2}\right] c_\theta^3 M_0^8 M_\pi^4 s_\theta^9}{2916 \sqrt{2} \pi^2 M_\eta^8} - \\
& \frac{4 \sqrt{2} \text{Log}\left[\frac{M_\eta^2}{\mu^2}\right] c_\theta^3 M_0^8 M_\pi^4 s_\theta^9}{243 \pi^2 M_\eta^8} - \frac{5 \text{Log}\left[\frac{M_\eta^2}{\mu^2}\right] c_\theta^3 M_0^8 M_\pi^4 s_\theta^9}{3888 \sqrt{2} \pi^2 M_\eta^8} + \frac{\sqrt{2} \text{Log}\left[\frac{M_\eta^2}{\mu^2}\right] c_\theta^3 M_0^8 M_\pi^4 s_\theta^9}{243 \pi^2 M_\eta^8} + \\
& \frac{\text{Log}\left[\frac{M_\eta^2}{\mu^2}\right] c_\theta M_0^8 M_K^2 s_\theta^9}{324 \sqrt{2} \pi^2 M_\eta^6} - \frac{\text{Log}\left[\frac{M_\eta^2}{\mu^2}\right] c_\theta M_0^8 M_K^2 s_\theta^9}{243 \sqrt{2} \pi^2 M_\eta^6} - \frac{\text{Log}\left[\frac{M_\eta^2}{\mu^2}\right] c_\theta M_0^8 M_\pi^2 s_\theta^9}{324 \sqrt{2} \pi^2 M_\eta^6} + \frac{5 \text{Log}\left[\frac{M_\eta^2}{\mu^2}\right] c_\theta M_0^8 M_\pi^2 s_\theta^9}{1944 \sqrt{2} \pi^2 M_\eta^6} + \\
& \frac{1310720 \sqrt{2} c_\theta^3 L_8^2 r M_0^8 M_K^8 M_\pi^2 s_\theta^9}{729 F^2 M_\eta^2 M_\eta^{10}} - \frac{1114112 \sqrt{2} c_\theta^3 L_8^2 r M_0^8 M_K^8 M_\pi^2 s_\theta^9}{243 F^2 M_\eta^2 M_\eta^{10}} + \\
& \frac{131072 \sqrt{2} c_\theta^3 L_8^2 r M_0^8 M_K^6 M_\pi^4 s_\theta^9}{27 F^2 M_\eta^2 M_\eta^{10}} - \frac{1961984 \sqrt{2} c_\theta^3 L_8^2 r M_0^8 M_K^6 M_\pi^4 s_\theta^9}{729 F^2 M_\eta^2 M_\eta^{10}} + \\
& \frac{188416 \sqrt{2} c_\theta^3 L_8^2 r M_0^8 M_K^8 M_\pi^8 s_\theta^9}{243 F^2 M_\eta^2 M_\eta^{10}} - \frac{2560 \sqrt{2} c_\theta^3 L_8^2 r M_0^8 M_\pi^{10} s_\theta^9}{27 F^2 M_\eta^2 M_\eta^{10}} + \frac{8 \sqrt{2} \text{Log}\left[\frac{M_\eta^2}{\mu^2}\right] c_\theta^3 M_0^8 M_K^4 s_\theta^9}{729 \pi^2 M_\eta^8} -
\end{aligned}$$

$$\begin{aligned}
& \frac{49 \operatorname{Log}\left[\frac{M_\eta^2}{\mu^2}\right] c_\theta^3 M_\theta^8 M_K^2 M_\pi^2 s_\theta^9}{2916 \sqrt{2} \pi^2 M_\eta^8} - \frac{2 \sqrt{2} \operatorname{Log}\left[\frac{M_\eta^2}{\mu^2}\right] c_\theta^3 M_\theta^8 M_K^2 M_\pi^2 s_\theta^9}{729 \pi^2 M_\eta^8} + \frac{29 \operatorname{Log}\left[\frac{M_\eta^2}{\mu^2}\right] c_\theta^3 M_\theta^8 M_\pi^4 s_\theta^9}{5832 \sqrt{2} \pi^2 M_\eta^8} + \\
& \frac{3\,276\,800 \sqrt{2} c_\theta^3 L_8^2 r M_\theta^8 M_K^{10} s_\theta^9}{729 F^2 M_\eta^4 M_\eta^8} - \frac{286\,720 \sqrt{2} c_\theta^3 L_8^2 r M_\theta^8 M_K^8 M_\pi^2 s_\theta^9}{27 F^2 M_\eta^4 M_\eta^8} + \\
& \frac{2\,048\,000 \sqrt{2} c_\theta^3 L_8^2 r M_\theta^8 M_K^6 M_\pi^4 s_\theta^9}{243 F^2 M_\eta^4 M_\eta^8} - \frac{1\,728\,512 \sqrt{2} c_\theta^3 L_8^2 r M_\theta^8 M_K^4 M_\pi^6 s_\theta^9}{729 F^2 M_\eta^4 M_\eta^8} + \\
& \frac{7168 \sqrt{2} c_\theta^3 L_8^2 r M_\theta^8 M_K^2 M_\pi^8 s_\theta^9}{243 F^2 M_\eta^4 M_\eta^8} - \frac{512 \sqrt{2} c_\theta^3 L_8^2 r M_\theta^8 M_\pi^{10} s_\theta^9}{27 F^2 M_\eta^4 M_\eta^8} - \frac{6\,225\,920 \sqrt{2} c_\theta^3 L_8^2 r M_\theta^8 M_K^{10} s_\theta^9}{729 F^2 M_\eta^6 M_\eta^6} + \\
& \frac{4\,784\,128 \sqrt{2} c_\theta^3 L_8^2 r M_\theta^8 M_K^8 M_\pi^2 s_\theta^9}{243 F^2 M_\eta^6 M_\eta^6} - \frac{3\,604\,480 \sqrt{2} c_\theta^3 L_8^2 r M_\theta^8 M_K^6 M_\pi^4 s_\theta^9}{243 F^2 M_\eta^6 M_\eta^6} + \\
& \frac{3\,067\,904 \sqrt{2} c_\theta^3 L_8^2 r M_\theta^8 M_K^4 M_\pi^6 s_\theta^9}{729 F^2 M_\eta^6 M_\eta^6} - \frac{142\,336 \sqrt{2} c_\theta^3 L_8^2 r M_\theta^8 M_K^2 M_\pi^8 s_\theta^9}{243 F^2 M_\eta^6 M_\eta^6} - \\
& \frac{1024 \sqrt{2} c_\theta^3 L_8^2 r M_\theta^8 M_\pi^{10} s_\theta^9}{81 F^2 M_\eta^6 M_\eta^6} - \frac{5 \sqrt{2} c_\theta^3 M_\theta^8 M_K^4 s_\theta^9}{243 \pi^2 M_\eta^2 M_\eta^6} - \frac{23 \sqrt{2} \operatorname{Log}\left[\frac{M_\eta^2}{\mu^2}\right] c_\theta^3 M_\theta^8 M_K^4 s_\theta^9}{729 \pi^2 M_\eta^2 M_\eta^6} + \\
& \frac{4 \sqrt{2} \operatorname{Log}\left[\frac{M_\eta^2}{\mu^2}\right] c_\theta^3 M_\theta^8 M_K^4 s_\theta^9}{729 \pi^2 M_\eta^2 M_\eta^6} + \frac{11 c_\theta^3 M_\theta^8 M_K^2 M_\pi^2 s_\theta^9}{243 \sqrt{2} \pi^2 M_\eta^2 M_\eta^6} + \frac{5 \operatorname{Log}\left[\frac{M_\eta^2}{\mu^2}\right] c_\theta^3 M_\theta^8 M_K^2 M_\pi^2 s_\theta^9}{2916 \sqrt{2} \pi^2 M_\eta^2 M_\eta^6} + \\
& \frac{2 \sqrt{2} \operatorname{Log}\left[\frac{M_\eta^2}{\mu^2}\right] c_\theta^3 M_\theta^8 M_K^2 M_\pi^2 s_\theta^9}{81 \pi^2 M_\eta^2 M_\eta^6} + \frac{\operatorname{Log}\left[\frac{M_\eta^2}{\mu^2}\right] c_\theta^3 M_\theta^8 M_K^2 M_\pi^2 s_\theta^9}{486 \sqrt{2} \pi^2 M_\eta^2 M_\eta^6} - \frac{5 \sqrt{2} \operatorname{Log}\left[\frac{M_\eta^2}{\mu^2}\right] c_\theta^3 M_\theta^8 M_K^2 M_\pi^2 s_\theta^9}{729 \pi^2 M_\eta^2 M_\eta^6} - \\
& \frac{11 c_\theta^3 M_\theta^8 M_\pi^4 s_\theta^9}{3888 \sqrt{2} \pi^2 M_\eta^2 M_\eta^6} - \frac{\sqrt{2} c_\theta^3 M_\theta^8 M_\pi^4 s_\theta^9}{243 \pi^2 M_\eta^2 M_\eta^6} - \frac{83 \operatorname{Log}\left[\frac{M_\eta^2}{\mu^2}\right] c_\theta^3 M_\theta^8 M_\pi^4 s_\theta^9}{5832 \sqrt{2} \pi^2 M_\eta^2 M_\eta^6} + \frac{131 \operatorname{Log}\left[\frac{M_\eta^2}{\mu^2}\right] c_\theta^3 M_\theta^8 M_\pi^4 s_\theta^9}{11\,664 \sqrt{2} \pi^2 M_\eta^2 M_\eta^6} - \\
& \frac{\sqrt{2} \operatorname{Log}\left[\frac{M_\eta^2}{\mu^2}\right] c_\theta^3 M_\theta^8 M_\pi^4 s_\theta^9}{243 \pi^2 M_\eta^2 M_\eta^6} + \frac{2\,621\,440 \sqrt{2} c_\theta^3 L_8^2 r M_\theta^8 M_K^{10} s_\theta^9}{729 F^2 M_\eta^8 M_\eta^4} - \frac{1\,630\,208 \sqrt{2} c_\theta^3 L_8^2 r M_\theta^8 M_K^8 M_\pi^2 s_\theta^9}{243 F^2 M_\eta^8 M_\eta^4} + \\
& \frac{401\,408 \sqrt{2} c_\theta^3 L_8^2 r M_\theta^8 M_K^6 M_\pi^4 s_\theta^9}{243 F^2 M_\eta^8 M_\eta^4} + \frac{1\,224\,704 \sqrt{2} c_\theta^3 L_8^2 r M_\theta^8 M_K^4 M_\pi^6 s_\theta^9}{729 F^2 M_\eta^8 M_\eta^4} - \\
& \frac{34\,816 \sqrt{2} c_\theta^3 L_8^2 r M_\theta^8 M_K^2 M_\pi^8 s_\theta^9}{243 F^2 M_\eta^8 M_\eta^4} - \frac{2048 \sqrt{2} c_\theta^3 L_8^2 r M_\theta^8 M_\pi^{10} s_\theta^9}{27 F^2 M_\eta^8 M_\eta^4} + \frac{\sqrt{2} \operatorname{Log}\left[\frac{M_K^2}{\mu^2}\right] c_\theta M_\theta^8 M_K^6 s_\theta^9}{81 \pi^2 M_\eta^6 M_\eta^4} - \\
& \frac{2048 \sqrt{2} c_\theta L_6^r M_\theta^8 M_K^6 s_\theta^9}{243 M_\eta^6 M_\eta^4} - \frac{2048 \sqrt{2} c_\theta L_7^r M_\theta^8 M_K^6 s_\theta^9}{243 M_\eta^6 M_\eta^4} + \frac{256 \sqrt{2} c_\theta L_{25}^r M_\theta^8 M_K^6 s_\theta^9}{27 M_\eta^6 M_\eta^4} - \\
& \frac{4096 \sqrt{2} c_\theta C_{19} M_\theta^8 M_K^8 s_\theta^9}{81 M_\eta^6 M_\eta^4} - \frac{8192 \sqrt{2} c_\theta C_{31} M_\theta^8 M_K^8 s_\theta^9}{243 M_\eta^6 M_\eta^4} - \frac{\operatorname{Log}\left[\frac{M_K^2}{\mu^2}\right] c_\theta M_\theta^8 M_K^4 M_\pi^2 s_\theta^9}{81 \sqrt{2} \pi^2 M_\eta^6 M_\eta^4} -
\end{aligned}$$

$$\begin{aligned}
& \frac{\sqrt{2} \operatorname{Log}\left[\frac{M_K^2}{\mu^2}\right] c_\theta M_0^8 M_K^4 M_\pi^2 s_\theta^9}{243 \pi^2 M_\eta^6 M_{\eta'}^4} + \frac{512 \sqrt{2} c_\theta L_6^r M_0^8 M_K^4 M_\pi^2 s_\theta^9}{81 M_\eta^6 M_{\eta'}^4} + \frac{896 \sqrt{2} c_\theta L_7^r M_0^8 M_K^4 M_\pi^2 s_\theta^9}{81 M_\eta^6 M_{\eta'}^4} - \\
& \frac{320 \sqrt{2} c_\theta L_{25}^r M_0^8 M_K^4 M_\pi^2 s_\theta^9}{27 M_\eta^6 M_{\eta'}^4} + \frac{7936 \sqrt{2} c_\theta C_{19} M_0^8 M_K^4 M_\pi^2 s_\theta^9}{81 M_\eta^6 M_{\eta'}^4} + \frac{15872 \sqrt{2} c_\theta C_{31} M_0^8 M_K^4 M_\pi^2 s_\theta^9}{243 M_\eta^6 M_{\eta'}^4} + \\
& \frac{5 \operatorname{Log}\left[\frac{M_K^2}{\mu^2}\right] c_\theta M_0^8 M_K^2 M_\pi^4 s_\theta^9}{972 \sqrt{2} \pi^2 M_\eta^6 M_{\eta'}^4} - \frac{5 \operatorname{Log}\left[\frac{M_\pi^2}{\mu^2}\right] c_\theta M_0^8 M_K^2 M_\pi^4 s_\theta^9}{324 \sqrt{2} \pi^2 M_\eta^6 M_{\eta'}^4} + \frac{256 \sqrt{2} c_\theta L_6^r M_0^8 M_K^2 M_\pi^4 s_\theta^9}{81 M_\eta^6 M_{\eta'}^4} - \\
& \frac{320 \sqrt{2} c_\theta L_7^r M_0^8 M_K^2 M_\pi^4 s_\theta^9}{81 M_\eta^6 M_{\eta'}^4} + \frac{64 \sqrt{2} c_\theta L_{25}^r M_0^8 M_K^2 M_\pi^4 s_\theta^9}{27 M_\eta^6 M_{\eta'}^4} - \frac{640 \sqrt{2} c_\theta C_{19} M_0^8 M_K^2 M_\pi^4 s_\theta^9}{9 M_\eta^6 M_{\eta'}^4} - \\
& \frac{1280 \sqrt{2} c_\theta C_{31} M_0^8 M_K^2 M_\pi^4 s_\theta^9}{27 M_\eta^6 M_{\eta'}^4} + \frac{\operatorname{Log}\left[\frac{M_\pi^2}{\mu^2}\right] c_\theta M_0^8 M_\pi^6 s_\theta^9}{648 \sqrt{2} \pi^2 M_\eta^6 M_{\eta'}^4} - \frac{256 \sqrt{2} c_\theta L_6^r M_0^8 M_\pi^6 s_\theta^9}{243 M_\eta^6 M_{\eta'}^4} + \\
& \frac{320 \sqrt{2} c_\theta L_7^r M_0^8 M_\pi^6 s_\theta^9}{243 M_\eta^6 M_{\eta'}^4} + \frac{2176 \sqrt{2} c_\theta C_{19} M_0^8 M_\pi^6 s_\theta^9}{81 M_\eta^6 M_{\eta'}^4} + \frac{4352 \sqrt{2} c_\theta C_{31} M_0^8 M_\pi^6 s_\theta^9}{243 M_\eta^6 M_{\eta'}^4} - \\
& \frac{256 \sqrt{2} c_\theta C_{19} M_0^8 M_\pi^8 s_\theta^9}{81 M_\eta^6 M_{\eta'}^4} - \frac{512 \sqrt{2} c_\theta C_{31} M_0^8 M_\pi^8 s_\theta^9}{243 M_\eta^6 M_{\eta'}^4} + \frac{c_\theta^3 M_0^8 M_K^4 s_\theta^9}{81 \sqrt{2} \pi^2 M_\eta^4 M_{\eta'}^4} + \\
& \frac{5 \operatorname{Log}\left[\frac{M_\pi^2}{\mu^2}\right] c_\theta^3 M_0^8 M_K^4 s_\theta^9}{81 \sqrt{2} \pi^2 M_\eta^4 M_{\eta'}^4} - \frac{4 \sqrt{2} \operatorname{Log}\left[\frac{M_\eta^2}{\mu^2}\right] c_\theta^3 M_0^8 M_K^4 s_\theta^9}{729 \pi^2 M_\eta^4 M_{\eta'}^4} + \frac{14 \sqrt{2} \operatorname{Log}\left[\frac{M_{\eta'}^2}{\mu^2}\right] c_\theta^3 M_0^8 M_K^4 s_\theta^9}{729 \pi^2 M_\eta^4 M_{\eta'}^4} - \\
& \frac{7 c_\theta^3 M_0^8 M_K^2 M_\pi^2 s_\theta^9}{162 \sqrt{2} \pi^2 M_\eta^4 M_{\eta'}^4} - \frac{\operatorname{Log}\left[\frac{M_\eta^2}{\mu^2}\right] c_\theta^3 M_0^8 M_K^2 M_\pi^2 s_\theta^9}{12 \sqrt{2} \pi^2 M_\eta^4 M_{\eta'}^4} + \frac{26 \sqrt{2} \operatorname{Log}\left[\frac{M_{\eta'}^2}{\mu^2}\right] c_\theta^3 M_0^8 M_K^2 M_\pi^2 s_\theta^9}{729 \pi^2 M_\eta^4 M_{\eta'}^4} - \\
& \frac{107 \operatorname{Log}\left[\frac{M_{\eta'}^2}{\mu^2}\right] c_\theta^3 M_0^8 M_K^2 M_\pi^2 s_\theta^9}{2916 \sqrt{2} \pi^2 M_\eta^4 M_{\eta'}^4} + \frac{25 c_\theta^3 M_0^8 M_\pi^4 s_\theta^9}{1296 \sqrt{2} \pi^2 M_\eta^4 M_{\eta'}^4} + \frac{47 \operatorname{Log}\left[\frac{M_\eta^2}{\mu^2}\right] c_\theta^3 M_0^8 M_\pi^4 s_\theta^9}{5832 \sqrt{2} \pi^2 M_\eta^4 M_{\eta'}^4} - \\
& \frac{\sqrt{2} \operatorname{Log}\left[\frac{M_{\eta'}^2}{\mu^2}\right] c_\theta^3 M_0^8 M_\pi^4 s_\theta^9}{243 \pi^2 M_\eta^4 M_{\eta'}^4} + \frac{79 \operatorname{Log}\left[\frac{M_{\eta'}^2}{\mu^2}\right] c_\theta^3 M_0^8 M_\pi^4 s_\theta^9}{11664 \sqrt{2} \pi^2 M_\eta^4 M_{\eta'}^4} + \frac{3604480 \sqrt{2} c_\theta^3 L_8^2 r M_0^8 M_K^{10} s_\theta^9}{729 F^2 M_\eta^{10} M_{\eta'}^2} - \\
& \frac{3350528 \sqrt{2} c_\theta^3 L_8^2 r M_0^8 M_K^8 M_\pi^2 s_\theta^9}{243 F^2 M_\eta^{10} M_{\eta'}^2} + \frac{4112384 \sqrt{2} c_\theta^3 L_8^2 r M_0^8 M_K^6 M_\pi^4 s_\theta^9}{243 F^2 M_\eta^{10} M_{\eta'}^2} - \\
& \frac{7278592 \sqrt{2} c_\theta^3 L_8^2 r M_0^8 M_K^4 M_\pi^6 s_\theta^9}{729 F^2 M_\eta^{10} M_{\eta'}^2} + \frac{555008 \sqrt{2} c_\theta^3 L_8^2 r M_0^8 M_K^2 M_\pi^8 s_\theta^9}{243 F^2 M_\eta^{10} M_{\eta'}^2} - \\
& \frac{5632 \sqrt{2} c_\theta^3 L_8^2 r M_0^8 M_\pi^{10} s_\theta^9}{27 F^2 M_\eta^{10} M_{\eta'}^2} - \frac{64 \sqrt{2} F^2 v_2^{(2)} c_\theta M_0^8 M_K^4 s_\theta^9}{27 M_\eta^8 M_{\eta'}^2} + \frac{2 \sqrt{2} \operatorname{Log}\left[\frac{M_K^2}{\mu^2}\right] c_\theta M_0^8 M_K^6 s_\theta^9}{243 \pi^2 M_\eta^8 M_{\eta'}^2} + \\
& \frac{512 \sqrt{2} c_\theta L_6^r M_0^8 M_K^6 s_\theta^9}{243 M_\eta^8 M_{\eta'}^2} + \frac{512 \sqrt{2} c_\theta L_7^r M_0^8 M_K^6 s_\theta^9}{243 M_\eta^8 M_{\eta'}^2} + \frac{512 \sqrt{2} c_\theta L_{25}^r M_0^8 M_K^6 s_\theta^9}{81 M_\eta^8 M_{\eta'}^2} +
\end{aligned}$$

$$\begin{aligned}
& \frac{1024 \sqrt{2} c_{\theta} C_{19} M_0^8 M_K^8 s_{\theta}^9}{81 M_{\eta}^8 M_{\eta'}^2} + \frac{2048 \sqrt{2} c_{\theta} C_{31} M_0^8 M_K^8 s_{\theta}^9}{243 M_{\eta}^8 M_{\eta'}^2} + \frac{32 \sqrt{2} F^2 v_2^{(2)} c_{\theta} M_0^8 M_K^2 M_{\pi}^2 s_{\theta}^9}{27 M_{\eta}^8 M_{\eta'}^2} + \\
& \frac{\text{Log}\left[\frac{M_K^2}{\mu^2}\right] c_{\theta} M_0^8 M_K^4 M_{\pi}^2 s_{\theta}^9}{81 \sqrt{2} \pi^2 M_{\eta}^8 M_{\eta'}^2} - \frac{\sqrt{2} \text{Log}\left[\frac{M_K^2}{\mu^2}\right] c_{\theta} M_0^8 M_K^4 M_{\pi}^2 s_{\theta}^9}{81 \pi^2 M_{\eta}^8 M_{\eta'}^2} - \frac{512 \sqrt{2} c_{\theta} L_6^r M_0^8 M_K^4 M_{\pi}^2 s_{\theta}^9}{81 M_{\eta}^8 M_{\eta'}^2} - \\
& \frac{896 \sqrt{2} c_{\theta} L_7^r M_0^8 M_K^4 M_{\pi}^2 s_{\theta}^9}{81 M_{\eta}^8 M_{\eta'}^2} - \frac{1216 \sqrt{2} c_{\theta} L_{25}^r M_0^8 M_K^4 M_{\pi}^2 s_{\theta}^9}{81 M_{\eta}^8 M_{\eta'}^2} - \frac{1792 \sqrt{2} c_{\theta} C_{19} M_0^8 M_K^6 M_{\pi}^2 s_{\theta}^9}{81 M_{\eta}^8 M_{\eta'}^2} - \\
& \frac{3584 \sqrt{2} c_{\theta} C_{31} M_0^8 M_K^6 M_{\pi}^2 s_{\theta}^9}{243 M_{\eta}^8 M_{\eta'}^2} + \frac{32 \sqrt{2} F^2 v_2^{(2)} c_{\theta} M_0^8 M_{\pi}^4 s_{\theta}^9}{27 M_{\eta}^8 M_{\eta'}^2} - \frac{7 \text{Log}\left[\frac{M_K^2}{\mu^2}\right] c_{\theta} M_0^8 M_K^2 M_{\pi}^4 s_{\theta}^9}{972 \sqrt{2} \pi^2 M_{\eta}^8 M_{\eta'}^2} + \\
& \frac{11 \text{Log}\left[\frac{M_{\pi}^2}{\mu^2}\right] c_{\theta} M_0^8 M_K^2 M_{\pi}^4 s_{\theta}^9}{324 \sqrt{2} \pi^2 M_{\eta}^8 M_{\eta'}^2} + \frac{128 \sqrt{2} c_{\theta} L_6^r M_0^8 M_K^2 M_{\pi}^4 s_{\theta}^9}{81 M_{\eta}^8 M_{\eta'}^2} + \frac{704 \sqrt{2} c_{\theta} L_7^r M_0^8 M_K^2 M_{\pi}^4 s_{\theta}^9}{81 M_{\eta}^8 M_{\eta'}^2} + \\
& \frac{1472 \sqrt{2} c_{\theta} L_{25}^r M_0^8 M_K^2 M_{\pi}^4 s_{\theta}^9}{81 M_{\eta}^8 M_{\eta'}^2} + \frac{128 \sqrt{2} c_{\theta} C_{19} M_0^8 M_K^4 M_{\pi}^4 s_{\theta}^9}{9 M_{\eta}^8 M_{\eta'}^2} + \frac{256 \sqrt{2} c_{\theta} C_{31} M_0^8 M_K^4 M_{\pi}^4 s_{\theta}^9}{27 M_{\eta}^8 M_{\eta'}^2} - \\
& \frac{19 \text{Log}\left[\frac{M_{\pi}^2}{\mu^2}\right] c_{\theta} M_0^8 M_{\pi}^6 s_{\theta}^9}{648 \sqrt{2} \pi^2 M_{\eta}^8 M_{\eta'}^2} + \frac{640 \sqrt{2} c_{\theta} L_6^r M_0^8 M_{\pi}^6 s_{\theta}^9}{243 M_{\eta}^8 M_{\eta'}^2} + \frac{64 \sqrt{2} c_{\theta} L_7^r M_0^8 M_{\pi}^6 s_{\theta}^9}{243 M_{\eta}^8 M_{\eta'}^2} - \\
& \frac{256 \sqrt{2} c_{\theta} L_{25}^r M_0^8 M_{\pi}^6 s_{\theta}^9}{27 M_{\eta}^8 M_{\eta'}^2} - \frac{1024 \sqrt{2} c_{\theta} C_{19} M_0^8 M_K^2 M_{\pi}^6 s_{\theta}^9}{81 M_{\eta}^8 M_{\eta'}^2} - \frac{2048 \sqrt{2} c_{\theta} C_{31} M_0^8 M_K^2 M_{\pi}^6 s_{\theta}^9}{243 M_{\eta}^8 M_{\eta'}^2} + \\
& \frac{640 \sqrt{2} c_{\theta} C_{19} M_0^8 M_{\pi}^8 s_{\theta}^9}{81 M_{\eta}^8 M_{\eta'}^2} + \frac{1280 \sqrt{2} c_{\theta} C_{31} M_0^8 M_{\pi}^8 s_{\theta}^9}{243 M_{\eta}^8 M_{\eta'}^2} - \frac{19 c_{\theta}^3 M_0^8 M_K^4 s_{\theta}^9}{243 \sqrt{2} \pi^2 M_{\eta}^6 M_{\eta'}^2} - \\
& \frac{35 \text{Log}\left[\frac{M_{\eta}^2}{\mu^2}\right] c_{\theta}^3 M_0^8 M_K^4 s_{\theta}^9}{243 \sqrt{2} \pi^2 M_{\eta}^6 M_{\eta'}^2} + \frac{19 \sqrt{2} \text{Log}\left[\frac{M_{\eta}^2}{\mu^2}\right] c_{\theta}^3 M_0^8 M_K^4 s_{\theta}^9}{243 \pi^2 M_{\eta}^6 M_{\eta'}^2} - \frac{32 \sqrt{2} \text{Log}\left[\frac{M_{\eta}^2}{\mu^2}\right] c_{\theta}^3 M_0^8 M_K^4 s_{\theta}^9}{729 \pi^2 M_{\eta}^6 M_{\eta'}^2} + \\
& \frac{67 c_{\theta}^3 M_0^8 M_K^2 M_{\pi}^2 s_{\theta}^9}{486 \sqrt{2} \pi^2 M_{\eta}^6 M_{\eta'}^2} + \frac{511 \text{Log}\left[\frac{M_{\eta}^2}{\mu^2}\right] c_{\theta}^3 M_0^8 M_K^2 M_{\pi}^2 s_{\theta}^9}{2916 \sqrt{2} \pi^2 M_{\eta}^6 M_{\eta'}^2} - \frac{77 \sqrt{2} \text{Log}\left[\frac{M_{\eta}^2}{\mu^2}\right] c_{\theta}^3 M_0^8 M_K^2 M_{\pi}^2 s_{\theta}^9}{729 \pi^2 M_{\eta}^6 M_{\eta'}^2} + \\
& \frac{31 \text{Log}\left[\frac{M_{\eta}^2}{\mu^2}\right] c_{\theta}^3 M_0^8 M_K^2 M_{\pi}^2 s_{\theta}^9}{972 \sqrt{2} \pi^2 M_{\eta}^6 M_{\eta'}^2} + \frac{16 \sqrt{2} \text{Log}\left[\frac{M_{\eta}^2}{\mu^2}\right] c_{\theta}^3 M_0^8 M_K^2 M_{\pi}^2 s_{\theta}^9}{729 \pi^2 M_{\eta}^6 M_{\eta'}^2} - \frac{215 c_{\theta}^3 M_0^8 M_{\pi}^4 s_{\theta}^9}{3888 \sqrt{2} \pi^2 M_{\eta}^6 M_{\eta'}^2} + \\
& \frac{2 \sqrt{2} c_{\theta}^3 M_0^8 M_{\pi}^4 s_{\theta}^9}{243 \pi^2 M_{\eta}^6 M_{\eta'}^2} - \frac{5 \text{Log}\left[\frac{M_{\eta}^2}{\mu^2}\right] c_{\theta}^3 M_0^8 M_{\pi}^4 s_{\theta}^9}{216 \sqrt{2} \pi^2 M_{\eta}^6 M_{\eta'}^2} + \frac{4 \sqrt{2} \text{Log}\left[\frac{M_{\eta}^2}{\mu^2}\right] c_{\theta}^3 M_0^8 M_{\pi}^4 s_{\theta}^9}{243 \pi^2 M_{\eta}^6 M_{\eta'}^2} - \\
& \frac{31 \text{Log}\left[\frac{M_{\eta}^2}{\mu^2}\right] c_{\theta}^3 M_0^8 M_{\pi}^4 s_{\theta}^9}{1296 \sqrt{2} \pi^2 M_{\eta}^6 M_{\eta'}^2} + \frac{\sqrt{2} \text{Log}\left[\frac{M_{\eta}^2}{\mu^2}\right] c_{\theta}^3 M_0^8 M_{\pi}^4 s_{\theta}^9}{729 \pi^2 M_{\eta}^6 M_{\eta'}^2} - \frac{\text{Log}\left[\frac{M_{\eta}^2}{\mu^2}\right] c_{\theta} M_0^8 M_K^2 s_{\theta}^9}{486 \sqrt{2} \pi^2 M_{\eta}^4 M_{\eta'}^2} +
\end{aligned}$$



$$\begin{aligned}
& \frac{1\,925\,120\,c_\theta^2\,L_8^2\,r\,M_0^8\,M_K^8\,M_\pi^2\,s_\theta^{10}}{243\,F^2\,M_\eta^{12}} - \frac{2\,191\,360\,c_\theta^2\,L_8^2\,r\,M_0^8\,M_K^6\,M_\pi^4\,s_\theta^{10}}{243\,F^2\,M_\eta^{12}} + \frac{4\,167\,680\,c_\theta^2\,L_8^2\,r\,M_0^8\,M_K^4\,M_\pi^6\,s_\theta^{10}}{729\,F^2\,M_\eta^{12}} - \\
& \frac{465\,920\,c_\theta^2\,L_8^2\,r\,M_0^8\,M_K^2\,M_\pi^8\,s_\theta^{10}}{243\,F^2\,M_\eta^{12}} + \frac{5120\,c_\theta^2\,L_8^2\,r\,M_0^8\,M_\pi^{10}\,s_\theta^{10}}{81\,F^2\,M_\eta^{12}} + \frac{16\,F^2\,v_2^{(2)}\,M_0^8\,M_K^4\,s_\theta^{10}}{27\,M_\eta^{10}} - \\
& \frac{\text{Log}\left[\frac{M_K^2}{\mu^2}\right]M_0^8\,M_K^6\,s_\theta^{10}}{243\,\pi^2\,M_\eta^{10}} + \frac{256\,L_6^r\,M_0^8\,M_K^6\,s_\theta^{10}}{243\,M_\eta^{10}} + \frac{256\,L_7^r\,M_0^8\,M_K^6\,s_\theta^{10}}{243\,M_\eta^{10}} - \frac{256\,L_{25}^r\,M_0^8\,M_K^6\,s_\theta^{10}}{81\,M_\eta^{10}} + \\
& \frac{512\,C_{19}\,M_0^8\,M_K^8\,s_\theta^{10}}{81\,M_\eta^{10}} + \frac{1024\,C_{31}\,M_0^8\,M_K^8\,s_\theta^{10}}{243\,M_\eta^{10}} + \frac{16\,F^2\,v_2^{(2)}\,M_0^8\,M_K^2\,M_\pi^2\,s_\theta^{10}}{27\,M_\eta^{10}} - \frac{\text{Log}\left[\frac{M_K^2}{\mu^2}\right]M_0^8\,M_K^4\,M_\pi^2\,s_\theta^{10}}{486\,\pi^2\,M_\eta^{10}} + \\
& \frac{128\,L_6^r\,M_0^8\,M_K^4\,M_\pi^2\,s_\theta^{10}}{81\,M_\eta^{10}} + \frac{128\,L_7^r\,M_0^8\,M_K^4\,M_\pi^2\,s_\theta^{10}}{81\,M_\eta^{10}} + \frac{128\,L_{25}^r\,M_0^8\,M_K^4\,M_\pi^2\,s_\theta^{10}}{81\,M_\eta^{10}} - \frac{512\,C_{19}\,M_0^8\,M_K^6\,M_\pi^2\,s_\theta^{10}}{81\,M_\eta^{10}} - \\
& \frac{1024\,C_{31}\,M_0^8\,M_K^6\,M_\pi^2\,s_\theta^{10}}{243\,M_\eta^{10}} + \frac{4\,F^2\,v_2^{(2)}\,M_0^8\,M_\pi^4\,s_\theta^{10}}{27\,M_\eta^{10}} - \frac{\text{Log}\left[\frac{M_\pi^2}{\mu^2}\right]M_0^8\,M_K^2\,M_\pi^4\,s_\theta^{10}}{324\,\pi^2\,M_\eta^{10}} + \frac{64\,L_6^r\,M_0^8\,M_K^2\,M_\pi^4\,s_\theta^{10}}{81\,M_\eta^{10}} + \\
& \frac{64\,L_7^r\,M_0^8\,M_K^2\,M_\pi^4\,s_\theta^{10}}{81\,M_\eta^{10}} - \frac{64\,L_{25}^r\,M_0^8\,M_K^2\,M_\pi^4\,s_\theta^{10}}{81\,M_\eta^{10}} - \frac{\text{Log}\left[\frac{M_\pi^2}{\mu^2}\right]M_0^8\,M_\pi^6\,s_\theta^{10}}{648\,\pi^2\,M_\eta^{10}} + \frac{32\,L_6^r\,M_0^8\,M_\pi^6\,s_\theta^{10}}{243\,M_\eta^{10}} + \\
& \frac{32\,L_7^r\,M_0^8\,M_\pi^6\,s_\theta^{10}}{243\,M_\eta^{10}} - \frac{32\,L_{25}^r\,M_0^8\,M_\pi^6\,s_\theta^{10}}{27\,M_\eta^{10}} + \frac{256\,C_{19}\,M_0^8\,M_K^2\,M_\pi^6\,s_\theta^{10}}{81\,M_\eta^{10}} + \frac{512\,C_{31}\,M_0^8\,M_K^2\,M_\pi^6\,s_\theta^{10}}{243\,M_\eta^{10}} + \\
& \frac{32\,C_{19}\,M_0^8\,M_\pi^8\,s_\theta^{10}}{81\,M_\eta^{10}} + \frac{64\,C_{31}\,M_0^8\,M_\pi^8\,s_\theta^{10}}{243\,M_\eta^{10}} + \frac{13\,c_\theta^2\,M_0^8\,M_K^4\,s_\theta^{10}}{486\,\pi^2\,M_\eta^8} - \frac{7\,\text{Log}\left[\frac{M_\eta^2}{\mu^2}\right]c_\theta^2\,M_0^8\,M_K^4\,s_\theta^{10}}{729\,\pi^2\,M_\eta^8} + \\
& \frac{19\,\text{Log}\left[\frac{M_\eta^2}{\mu^2}\right]c_\theta^2\,M_0^8\,M_K^4\,s_\theta^{10}}{486\,\pi^2\,M_\eta^8} - \frac{7\,c_\theta^2\,M_0^8\,M_K^2\,M_\pi^2\,s_\theta^{10}}{243\,\pi^2\,M_\eta^8} + \frac{29\,\text{Log}\left[\frac{M_\eta^2}{\mu^2}\right]c_\theta^2\,M_0^8\,M_K^2\,M_\pi^2\,s_\theta^{10}}{2916\,\pi^2\,M_\eta^8} - \\
& \frac{10\,\text{Log}\left[\frac{M_\eta^2}{\mu^2}\right]c_\theta^2\,M_0^8\,M_K^2\,M_\pi^2\,s_\theta^{10}}{243\,\pi^2\,M_\eta^8} + \frac{115\,c_\theta^2\,M_0^8\,M_\pi^4\,s_\theta^{10}}{7776\,\pi^2\,M_\eta^8} - \frac{29\,\text{Log}\left[\frac{M_\eta^2}{\mu^2}\right]c_\theta^2\,M_0^8\,M_\pi^4\,s_\theta^{10}}{5832\,\pi^2\,M_\eta^8} + \\
& \frac{79\,\text{Log}\left[\frac{M_\eta^2}{\mu^2}\right]c_\theta^2\,M_0^8\,M_\pi^4\,s_\theta^{10}}{7776\,\pi^2\,M_\eta^8} + \frac{\text{Log}\left[\frac{M_\eta^2}{\mu^2}\right]M_0^8\,M_K^2\,s_\theta^{10}}{3888\,\pi^2\,M_\eta^6} + \frac{\text{Log}\left[\frac{M_\eta^2}{\mu^2}\right]M_0^8\,M_\pi^2\,s_\theta^{10}}{7776\,\pi^2\,M_\eta^6} - \frac{655\,360\,c_\theta^2\,L_8^2\,r\,M_0^8\,M_K^{10}\,s_\theta^{10}}{243\,F^2\,M_\eta^4\,M_{\eta'}^8} + \\
& \frac{544\,768\,c_\theta^2\,L_8^2\,r\,M_0^8\,M_K^8\,M_\pi^2\,s_\theta^{10}}{81\,F^2\,M_\eta^4\,M_{\eta'}^8} - \frac{532\,480\,c_\theta^2\,L_8^2\,r\,M_0^8\,M_K^6\,M_\pi^4\,s_\theta^{10}}{81\,F^2\,M_\eta^4\,M_{\eta'}^8} + \frac{747\,520\,c_\theta^2\,L_8^2\,r\,M_0^8\,M_K^4\,M_\pi^6\,s_\theta^{10}}{243\,F^2\,M_\eta^4\,M_{\eta'}^8} - \\
& \frac{17\,408\,c_\theta^2\,L_8^2\,r\,M_0^8\,M_K^2\,M_\pi^8\,s_\theta^{10}}{27\,F^2\,M_\eta^4\,M_{\eta'}^8} + \frac{256\,c_\theta^2\,L_8^2\,r\,M_0^8\,M_\pi^{10}\,s_\theta^{10}}{9\,F^2\,M_\eta^4\,M_{\eta'}^8} - \frac{1\,310\,720\,c_\theta^2\,L_8^2\,r\,M_0^8\,M_K^{10}\,s_\theta^{10}}{729\,F^2\,M_\eta^6\,M_{\eta'}^6} + \\
& \frac{40\,960\,c_\theta^2\,L_8^2\,r\,M_0^8\,M_K^8\,M_\pi^2\,s_\theta^{10}}{9\,F^2\,M_\eta^6\,M_{\eta'}^6} - \frac{999\,424\,c_\theta^2\,L_8^2\,r\,M_0^8\,M_K^6\,M_\pi^4\,s_\theta^{10}}{243\,F^2\,M_\eta^6\,M_{\eta'}^6} + \frac{1\,323\,008\,c_\theta^2\,L_8^2\,r\,M_0^8\,M_K^4\,M_\pi^6\,s_\theta^{10}}{729\,F^2\,M_\eta^6\,M_{\eta'}^6} -
\end{aligned}$$



$$\begin{aligned}
& \frac{44\,032\,c_\theta^2\,L_8^2\,r\,M_\theta^8\,M_K^2\,M_\pi^8\,s_\theta^{10}}{81\,F^2\,M_\eta^6\,M_{\eta'}^6} + \frac{1024\,c_\theta^2\,L_8^2\,r\,M_\theta^8\,M_\pi^{10}\,s_\theta^{10}}{81\,F^2\,M_\eta^6\,M_{\eta'}^6} - \frac{4\,\text{Log}\left[\frac{M_\eta^2}{\mu^2}\right]\,c_\theta^2\,M_\theta^8\,M_K^4\,s_\theta^{10}}{243\,\pi^2\,M_\eta^2\,M_{\eta'}^6} + \\
& \frac{17\,\text{Log}\left[\frac{M_\eta^2}{\mu^2}\right]\,c_\theta^2\,M_\theta^8\,M_K^2\,M_\pi^2\,s_\theta^{10}}{972\,\pi^2\,M_\eta^2\,M_{\eta'}^6} - \frac{11\,\text{Log}\left[\frac{M_\eta^2}{\mu^2}\right]\,c_\theta^2\,M_\theta^8\,M_\pi^4\,s_\theta^{10}}{1944\,\pi^2\,M_\eta^2\,M_{\eta'}^6} + \frac{4\,259\,840\,c_\theta^2\,L_8^2\,r\,M_\theta^8\,M_K^{10}\,s_\theta^{10}}{729\,F^2\,M_\eta^8\,M_{\eta'}^4} - \\
& \frac{3\,485\,696\,c_\theta^2\,L_8^2\,r\,M_\theta^8\,M_K^8\,M_\pi^2\,s_\theta^{10}}{243\,F^2\,M_\eta^8\,M_{\eta'}^4} + \frac{987\,136\,c_\theta^2\,L_8^2\,r\,M_\theta^8\,M_K^6\,M_\pi^4\,s_\theta^{10}}{81\,F^2\,M_\eta^8\,M_{\eta'}^4} - \frac{2\,846\,720\,c_\theta^2\,L_8^2\,r\,M_\theta^8\,M_K^4\,M_\pi^6\,s_\theta^{10}}{729\,F^2\,M_\eta^8\,M_{\eta'}^4} + \\
& \frac{71\,680\,c_\theta^2\,L_8^2\,r\,M_\theta^8\,M_K^2\,M_\pi^8\,s_\theta^{10}}{243\,F^2\,M_\eta^8\,M_{\eta'}^4} - \frac{1280\,c_\theta^2\,L_8^2\,r\,M_\theta^8\,M_\pi^{10}\,s_\theta^{10}}{27\,F^2\,M_\eta^8\,M_{\eta'}^4} + \frac{5\,c_\theta^2\,M_\theta^8\,M_K^4\,s_\theta^{10}}{162\,\pi^2\,M_\eta^4\,M_{\eta'}^4} + \frac{53\,\text{Log}\left[\frac{M_\eta^2}{\mu^2}\right]\,c_\theta^2\,M_\theta^8\,M_K^4\,s_\theta^{10}}{1458\,\pi^2\,M_\eta^4\,M_{\eta'}^4} - \\
& \frac{2\,\text{Log}\left[\frac{M_\eta^2}{\mu^2}\right]\,c_\theta^2\,M_\theta^8\,M_K^4\,s_\theta^{10}}{243\,\pi^2\,M_\eta^4\,M_{\eta'}^4} - \frac{11\,c_\theta^2\,M_\theta^8\,M_K^2\,M_\pi^2\,s_\theta^{10}}{324\,\pi^2\,M_\eta^4\,M_{\eta'}^4} - \frac{187\,\text{Log}\left[\frac{M_\eta^2}{\mu^2}\right]\,c_\theta^2\,M_\theta^8\,M_K^2\,M_\pi^2\,s_\theta^{10}}{5832\,\pi^2\,M_\eta^4\,M_{\eta'}^4} + \\
& \frac{11\,\text{Log}\left[\frac{M_\eta^2}{\mu^2}\right]\,c_\theta^2\,M_\theta^8\,M_K^2\,M_\pi^2\,s_\theta^{10}}{1944\,\pi^2\,M_\eta^4\,M_{\eta'}^4} + \frac{29\,c_\theta^2\,M_\theta^8\,M_\pi^4\,s_\theta^{10}}{2592\,\pi^2\,M_\eta^4\,M_{\eta'}^4} + \frac{67\,\text{Log}\left[\frac{M_\eta^2}{\mu^2}\right]\,c_\theta^2\,M_\theta^8\,M_\pi^4\,s_\theta^{10}}{11\,664\,\pi^2\,M_\eta^4\,M_{\eta'}^4} - \\
& \frac{7\,\text{Log}\left[\frac{M_\eta^2}{\mu^2}\right]\,c_\theta^2\,M_\theta^8\,M_\pi^4\,s_\theta^{10}}{7776\,\pi^2\,M_\eta^4\,M_{\eta'}^4} - \frac{901\,120\,c_\theta^2\,L_8^2\,r\,M_\theta^8\,M_K^{10}\,s_\theta^{10}}{729\,F^2\,M_\eta^{10}\,M_{\eta'}^2} + \frac{8192\,c_\theta^2\,L_8^2\,r\,M_\theta^8\,M_K^8\,M_\pi^2\,s_\theta^{10}}{3\,F^2\,M_\eta^{10}\,M_{\eta'}^2} - \\
& \frac{16\,384\,c_\theta^2\,L_8^2\,r\,M_\theta^8\,M_K^6\,M_\pi^4\,s_\theta^{10}}{243\,F^2\,M_\eta^{10}\,M_{\eta'}^2} - \frac{2\,121\,728\,c_\theta^2\,L_8^2\,r\,M_\theta^8\,M_K^4\,M_\pi^6\,s_\theta^{10}}{729\,F^2\,M_\eta^{10}\,M_{\eta'}^2} + \frac{452\,608\,c_\theta^2\,L_8^2\,r\,M_\theta^8\,M_K^2\,M_\pi^8\,s_\theta^{10}}{243\,F^2\,M_\eta^{10}\,M_{\eta'}^2} - \\
& \frac{4096\,c_\theta^2\,L_8^2\,r\,M_\theta^8\,M_\pi^{10}\,s_\theta^{10}}{27\,F^2\,M_\eta^{10}\,M_{\eta'}^2} - \frac{\text{Log}\left[\frac{M_K^2}{\mu^2}\right]\,M_\theta^8\,M_K^6\,s_\theta^{10}}{243\,\pi^2\,M_\eta^8\,M_{\eta'}^2} + \frac{512\,L_6^r\,M_\theta^8\,M_K^6\,s_\theta^{10}}{243\,M_\eta^8\,M_{\eta'}^2} + \frac{512\,L_7^r\,M_\theta^8\,M_K^6\,s_\theta^{10}}{243\,M_\eta^8\,M_{\eta'}^2} - \\
& \frac{256\,L_{25}^r\,M_\theta^8\,M_K^6\,s_\theta^{10}}{81\,M_\eta^8\,M_{\eta'}^2} + \frac{1024\,C_{19}\,M_\theta^8\,M_K^8\,s_\theta^{10}}{81\,M_\eta^8\,M_{\eta'}^2} + \frac{2048\,C_{31}\,M_\theta^8\,M_K^8\,s_\theta^{10}}{243\,M_\eta^8\,M_{\eta'}^2} + \frac{\text{Log}\left[\frac{M_K^2}{\mu^2}\right]\,M_\theta^8\,M_K^4\,M_\pi^2\,s_\theta^{10}}{162\,\pi^2\,M_\eta^8\,M_{\eta'}^2} - \\
& \frac{256\,L_6^r\,M_\theta^8\,M_K^4\,M_\pi^2\,s_\theta^{10}}{81\,M_\eta^8\,M_{\eta'}^2} - \frac{256\,L_7^r\,M_\theta^8\,M_K^4\,M_\pi^2\,s_\theta^{10}}{81\,M_\eta^8\,M_{\eta'}^2} + \frac{512\,L_{25}^r\,M_\theta^8\,M_K^4\,M_\pi^2\,s_\theta^{10}}{81\,M_\eta^8\,M_{\eta'}^2} - \frac{2560\,C_{19}\,M_\theta^8\,M_K^6\,M_\pi^2\,s_\theta^{10}}{81\,M_\eta^8\,M_{\eta'}^2} - \\
& \frac{5120\,C_{31}\,M_\theta^8\,M_K^6\,M_\pi^2\,s_\theta^{10}}{243\,M_\eta^8\,M_{\eta'}^2} - \frac{\text{Log}\left[\frac{M_K^2}{\mu^2}\right]\,M_\theta^8\,M_K^2\,M_\pi^4\,s_\theta^{10}}{486\,\pi^2\,M_\eta^8\,M_{\eta'}^2} + \frac{\text{Log}\left[\frac{M_\pi^2}{\mu^2}\right]\,M_\theta^8\,M_K^2\,M_\pi^4\,s_\theta^{10}}{324\,\pi^2\,M_\eta^8\,M_{\eta'}^2} - \frac{256\,L_{25}^r\,M_\theta^8\,M_K^2\,M_\pi^4\,s_\theta^{10}}{81\,M_\eta^8\,M_{\eta'}^2} + \\
& \frac{256\,C_{19}\,M_\theta^8\,M_K^4\,M_\pi^4\,s_\theta^{10}}{9\,M_\eta^8\,M_{\eta'}^2} + \frac{512\,C_{31}\,M_\theta^8\,M_K^4\,M_\pi^4\,s_\theta^{10}}{27\,M_\eta^8\,M_{\eta'}^2} - \frac{\text{Log}\left[\frac{M_\pi^2}{\mu^2}\right]\,M_\theta^8\,M_\pi^6\,s_\theta^{10}}{324\,\pi^2\,M_\eta^8\,M_{\eta'}^2} + \frac{256\,L_6^r\,M_\theta^8\,M_\pi^6\,s_\theta^{10}}{243\,M_\eta^8\,M_{\eta'}^2} + \\
& \frac{256\,L_7^r\,M_\theta^8\,M_\pi^6\,s_\theta^{10}}{243\,M_\eta^8\,M_{\eta'}^2} - \frac{1024\,C_{19}\,M_\theta^8\,M_K^2\,M_\pi^6\,s_\theta^{10}}{81\,M_\eta^8\,M_{\eta'}^2} - \frac{2048\,C_{31}\,M_\theta^8\,M_K^2\,M_\pi^6\,s_\theta^{10}}{243\,M_\eta^8\,M_{\eta'}^2} + \frac{256\,C_{19}\,M_\theta^8\,M_\pi^8\,s_\theta^{10}}{81\,M_\eta^8\,M_{\eta'}^2} + \\
& \frac{512\,C_{31}\,M_\theta^8\,M_\pi^8\,s_\theta^{10}}{243\,M_\eta^8\,M_{\eta'}^2} - \frac{17\,c_\theta^2\,M_\theta^8\,M_K^4\,s_\theta^{10}}{486\,\pi^2\,M_\eta^6\,M_{\eta'}^2} - \frac{4\,\text{Log}\left[\frac{M_\eta^2}{\mu^2}\right]\,c_\theta^2\,M_\theta^8\,M_K^4\,s_\theta^{10}}{243\,\pi^2\,M_\eta^6\,M_{\eta'}^2} - \frac{10\,\text{Log}\left[\frac{M_\eta^2}{\mu^2}\right]\,c_\theta^2\,M_\theta^8\,M_K^4\,s_\theta^{10}}{729\,\pi^2\,M_\eta^6\,M_{\eta'}^2} +
\end{aligned}$$

$$\begin{aligned}
& \frac{11 c_\theta^2 M_0^8 M_K^2 M_\pi^2 s_\theta^{10}}{243 \pi^2 M_\eta^6 M_{\eta'}^2} + \frac{13 \operatorname{Log}\left[\frac{M_\eta^2}{\mu^2}\right] c_\theta^2 M_0^8 M_K^2 M_\pi^2 s_\theta^{10}}{972 \pi^2 M_\eta^6 M_{\eta'}^2} + \frac{139 \operatorname{Log}\left[\frac{M_{\eta'}^2}{\mu^2}\right] c_\theta^2 M_0^8 M_K^2 M_\pi^2 s_\theta^{10}}{5832 \pi^2 M_\eta^6 M_{\eta'}^2} - \\
& \frac{67 c_\theta^2 M_0^8 M_\pi^4 s_\theta^{10}}{3888 \pi^2 M_\eta^6 M_{\eta'}^2} - \frac{59 \operatorname{Log}\left[\frac{M_{\eta'}^2}{\mu^2}\right] c_\theta^2 M_0^8 M_\pi^4 s_\theta^{10}}{5832 \pi^2 M_\eta^6 M_{\eta'}^2} - \frac{37 \operatorname{Log}\left[\frac{M_\eta^2}{\mu^2}\right] c_\theta^2 M_0^8 M_K^4 M_{\eta'}^2 s_\theta^{10}}{1458 \pi^2 M_\eta^{10}} + \\
& \frac{131 \operatorname{Log}\left[\frac{M_\eta^2}{\mu^2}\right] c_\theta^2 M_0^8 M_K^2 M_\pi^2 M_{\eta'}^2 s_\theta^{10}}{5832 \pi^2 M_\eta^{10}} - \frac{47 \operatorname{Log}\left[\frac{M_\eta^2}{\mu^2}\right] c_\theta^2 M_0^8 M_\pi^4 M_{\eta'}^2 s_\theta^{10}}{11664 \pi^2 M_\eta^{10}} + \frac{\operatorname{Log}\left[\frac{M_{\eta'}^2}{\mu^2}\right] M_0^8 M_K^2 M_{\eta'}^2 s_\theta^{10}}{1944 \pi^2 M_\eta^8} - \\
& \frac{\operatorname{Log}\left[\frac{M_\eta^2}{\mu^2}\right] M_0^8 M_\pi^2 M_{\eta'}^2 s_\theta^{10}}{7776 \pi^2 M_\eta^8} + \frac{37 \operatorname{Log}\left[\frac{M_\eta^2}{\mu^2}\right] c_\theta^2 M_0^8 M_K^4 s_\theta^{10}}{972 \pi^2 M_\eta^6 (M_\eta^2 - M_{\eta'}^2)} + \frac{14 \operatorname{Log}\left[\frac{M_{\eta'}^2}{\mu^2}\right] c_\theta^2 M_0^8 M_K^4 s_\theta^{10}}{243 \pi^2 M_\eta^6 (M_\eta^2 - M_{\eta'}^2)} - \\
& \frac{35 \operatorname{Log}\left[\frac{M_\eta^2}{\mu^2}\right] c_\theta^2 M_0^8 M_K^2 M_\pi^2 s_\theta^{10}}{972 \pi^2 M_\eta^6 (M_\eta^2 - M_{\eta'}^2)} - \frac{23 \operatorname{Log}\left[\frac{M_{\eta'}^2}{\mu^2}\right] c_\theta^2 M_0^8 M_K^2 M_\pi^2 s_\theta^{10}}{486 \pi^2 M_\eta^6 (M_\eta^2 - M_{\eta'}^2)} + \frac{7 \operatorname{Log}\left[\frac{M_\eta^2}{\mu^2}\right] c_\theta^2 M_0^8 M_\pi^4 s_\theta^{10}}{972 \pi^2 M_\eta^6 (M_\eta^2 - M_{\eta'}^2)} + \\
& \frac{2 \operatorname{Log}\left[\frac{M_{\eta'}^2}{\mu^2}\right] c_\theta^2 M_0^8 M_\pi^4 s_\theta^{10}}{243 \pi^2 M_\eta^6 (M_\eta^2 - M_{\eta'}^2)} + \frac{2 \operatorname{Log}\left[\frac{M_\eta^2}{\mu^2}\right] c_\theta^2 M_0^8 M_K^4 s_\theta^{10}}{81 \pi^2 M_\eta^4 M_{\eta'}^2 (M_\eta^2 - M_{\eta'}^2)} - \frac{7 \operatorname{Log}\left[\frac{M_\eta^2}{\mu^2}\right] c_\theta^2 M_0^8 M_K^2 M_\pi^2 s_\theta^{10}}{324 \pi^2 M_\eta^4 M_{\eta'}^2 (M_\eta^2 - M_{\eta'}^2)} + \\
& \frac{\operatorname{Log}\left[\frac{M_\eta^2}{\mu^2}\right] c_\theta^2 M_0^8 M_\pi^4 s_\theta^{10}}{162 \pi^2 M_\eta^4 M_{\eta'}^2 (M_\eta^2 - M_{\eta'}^2)} - \frac{14 \operatorname{Log}\left[\frac{M_\eta^2}{\mu^2}\right] c_\theta^2 M_0^8 M_K^4 s_\theta^{10}}{243 \pi^2 M_\eta^4 M_{\eta'}^2 (M_\eta^2 - M_{\eta'}^2)} - \frac{2 \operatorname{Log}\left[\frac{M_{\eta'}^2}{\mu^2}\right] c_\theta^2 M_0^8 M_K^4 s_\theta^{10}}{81 \pi^2 M_\eta^4 M_{\eta'}^2 (M_\eta^2 - M_{\eta'}^2)} + \\
& \frac{23 \operatorname{Log}\left[\frac{M_\eta^2}{\mu^2}\right] c_\theta^2 M_0^8 M_K^2 M_\pi^2 s_\theta^{10}}{486 \pi^2 M_\eta^4 M_{\eta'}^2 (M_\eta^2 - M_{\eta'}^2)} + \frac{7 \operatorname{Log}\left[\frac{M_{\eta'}^2}{\mu^2}\right] c_\theta^2 M_0^8 M_K^2 M_\pi^2 s_\theta^{10}}{324 \pi^2 M_\eta^4 M_{\eta'}^2 (M_\eta^2 - M_{\eta'}^2)} - \frac{2 \operatorname{Log}\left[\frac{M_\eta^2}{\mu^2}\right] c_\theta^2 M_0^8 M_\pi^4 s_\theta^{10}}{243 \pi^2 M_\eta^4 M_{\eta'}^2 (M_\eta^2 - M_{\eta'}^2)} - \\
& \frac{\operatorname{Log}\left[\frac{M_\eta^2}{\mu^2}\right] c_\theta^2 M_0^8 M_\pi^4 s_\theta^{10}}{162 \pi^2 M_\eta^4 M_{\eta'}^2 (M_\eta^2 - M_{\eta'}^2)} - \frac{37 \operatorname{Log}\left[\frac{M_\eta^2}{\mu^2}\right] c_\theta^2 M_0^8 M_K^4 M_{\eta'}^2 s_\theta^{10}}{972 \pi^2 M_\eta^8 (M_\eta^2 - M_{\eta'}^2)} + \frac{35 \operatorname{Log}\left[\frac{M_{\eta'}^2}{\mu^2}\right] c_\theta^2 M_0^8 M_K^2 M_\pi^2 M_{\eta'}^2 s_\theta^{10}}{972 \pi^2 M_\eta^8 (M_\eta^2 - M_{\eta'}^2)} - \\
& \frac{7 \operatorname{Log}\left[\frac{M_{\eta'}^2}{\mu^2}\right] c_\theta^2 M_0^8 M_\pi^4 M_{\eta'}^2 s_\theta^{10}}{972 \pi^2 M_\eta^8 (M_\eta^2 - M_{\eta'}^2)} - \frac{327680 \sqrt{2} c_\theta L_8^2 r M_0^8 M_K^{10} s_\theta^{11}}{729 F^2 M_\eta^{12}} + \frac{81920 \sqrt{2} c_\theta L_8^2 r M_0^8 M_K^8 M_\pi^2 s_\theta^{11}}{81 F^2 M_\eta^{12}} - \\
& \frac{286720 \sqrt{2} c_\theta L_8^2 r M_0^8 M_K^6 M_\pi^4 s_\theta^{11}}{243 F^2 M_\eta^{12}} + \frac{634880 \sqrt{2} c_\theta L_8^2 r M_0^8 M_K^4 M_\pi^6 s_\theta^{11}}{729 F^2 M_\eta^{12}} - \\
& \frac{10240 \sqrt{2} c_\theta L_8^2 r M_0^8 M_K^2 M_\pi^8 s_\theta^{11}}{27 F^2 M_\eta^{12}} + \frac{10240 \sqrt{2} c_\theta L_8^2 r M_0^8 M_\pi^{10} s_\theta^{11}}{81 F^2 M_\eta^{12}} + \frac{2 \sqrt{2} c_\theta M_0^8 M_K^4 s_\theta^{11}}{243 \pi^2 M_\eta^8} - \\
& \frac{\sqrt{2} \operatorname{Log}\left[\frac{M_\eta^2}{\mu^2}\right] c_\theta M_0^8 M_K^4 s_\theta^{11}}{729 \pi^2 M_\eta^8} + \frac{\sqrt{2} \operatorname{Log}\left[\frac{M_{\eta'}^2}{\mu^2}\right] c_\theta M_0^8 M_K^4 s_\theta^{11}}{243 \pi^2 M_\eta^8} - \frac{\sqrt{2} c_\theta M_0^8 M_K^2 M_\pi^2 s_\theta^{11}}{243 \pi^2 M_\eta^8} - \\
& \frac{\operatorname{Log}\left[\frac{M_\eta^2}{\mu^2}\right] c_\theta M_0^8 M_K^2 M_\pi^2 s_\theta^{11}}{243 \sqrt{2} \pi^2 M_\eta^8} + \frac{2 \sqrt{2} \operatorname{Log}\left[\frac{M_\eta^2}{\mu^2}\right] c_\theta M_0^8 M_K^2 M_\pi^2 s_\theta^{11}}{729 \pi^2 M_\eta^8} + \frac{23 \operatorname{Log}\left[\frac{M_{\eta'}^2}{\mu^2}\right] c_\theta M_0^8 M_K^2 M_\pi^2 s_\theta^{11}}{2916 \sqrt{2} \pi^2 M_\eta^8} -
\end{aligned}$$

$$\begin{aligned}
& \frac{4 \sqrt{2} \operatorname{Log} \left[ \frac{M_\eta^2}{\mu^2} \right] c_\theta M_\theta^8 M_K^2 M_\pi^2 s_\theta^{11}}{729 \pi^2 M_\eta^8} - \frac{7 c_\theta M_\theta^8 M_\pi^4 s_\theta^{11}}{1944 \sqrt{2} \pi^2 M_\eta^8} - \frac{\operatorname{Log} \left[ \frac{M_\eta^2}{\mu^2} \right] c_\theta M_\theta^8 M_\pi^4 s_\theta^{11}}{243 \sqrt{2} \pi^2 M_\eta^8} + \\
& \frac{2 \sqrt{2} \operatorname{Log} \left[ \frac{M_\eta^2}{\mu^2} \right] c_\theta M_\theta^8 M_\pi^4 s_\theta^{11}}{729 \pi^2 M_\eta^8} - \frac{\operatorname{Log} \left[ \frac{M_\eta^2}{\mu^2} \right] c_\theta M_\theta^8 M_\pi^4 s_\theta^{11}}{486 \sqrt{2} \pi^2 M_\eta^8} + \frac{655360 \sqrt{2} c_\theta L_8^2 r M_\theta^8 M_K^{10} s_\theta^{11}}{729 F^2 M_\eta^6 M_{\eta'}^6} - \\
& \frac{532480 \sqrt{2} c_\theta L_8^2 r M_\theta^8 M_K^8 M_\pi^2 s_\theta^{11}}{243 F^2 M_\eta^6 M_{\eta'}^6} + \frac{475136 \sqrt{2} c_\theta L_8^2 r M_\theta^8 M_K^6 M_\pi^4 s_\theta^{11}}{243 F^2 M_\eta^6 M_{\eta'}^6} - \\
& \frac{569344 \sqrt{2} c_\theta L_8^2 r M_\theta^8 M_K^4 M_\pi^6 s_\theta^{11}}{729 F^2 M_\eta^6 M_{\eta'}^6} + \frac{31744 \sqrt{2} c_\theta L_8^2 r M_\theta^8 M_K^2 M_\pi^8 s_\theta^{11}}{243 F^2 M_\eta^6 M_{\eta'}^6} - \\
& \frac{1024 \sqrt{2} c_\theta L_8^2 r M_\theta^8 M_\pi^{10} s_\theta^{11}}{81 F^2 M_\eta^6 M_{\eta'}^6} + \frac{327680 \sqrt{2} c_\theta L_8^2 r M_\theta^8 M_K^{10} s_\theta^{11}}{729 F^2 M_\eta^8 M_{\eta'}^4} - \frac{106496 \sqrt{2} c_\theta L_8^2 r M_\theta^8 M_K^8 M_\pi^2 s_\theta^{11}}{81 F^2 M_\eta^8 M_{\eta'}^4} + \\
& \frac{401408 \sqrt{2} c_\theta L_8^2 r M_\theta^8 M_K^6 M_\pi^4 s_\theta^{11}}{243 F^2 M_\eta^8 M_{\eta'}^4} - \frac{696320 \sqrt{2} c_\theta L_8^2 r M_\theta^8 M_K^4 M_\pi^6 s_\theta^{11}}{729 F^2 M_\eta^8 M_{\eta'}^4} + \\
& \frac{50176 \sqrt{2} c_\theta L_8^2 r M_\theta^8 M_K^2 M_\pi^8 s_\theta^{11}}{243 F^2 M_\eta^8 M_{\eta'}^4} - \frac{1024 \sqrt{2} c_\theta L_8^2 r M_\theta^8 M_\pi^{10} s_\theta^{11}}{27 F^2 M_\eta^8 M_{\eta'}^4} + \frac{4 \sqrt{2} \operatorname{Log} \left[ \frac{M_\eta^2}{\mu^2} \right] c_\theta M_\theta^8 M_\pi^4 s_\theta^{11}}{729 \pi^2 M_\eta^4 M_{\eta'}^4} - \\
& \frac{5 \sqrt{2} \operatorname{Log} \left[ \frac{M_\eta^2}{\mu^2} \right] c_\theta M_\theta^8 M_K^2 M_\pi^2 s_\theta^{11}}{729 \pi^2 M_\eta^4 M_{\eta'}^4} + \frac{\sqrt{2} \operatorname{Log} \left[ \frac{M_\eta^2}{\mu^2} \right] c_\theta M_\theta^8 M_\pi^4 s_\theta^{11}}{729 \pi^2 M_\eta^4 M_{\eta'}^4} - \frac{655360 \sqrt{2} c_\theta L_8^2 r M_\theta^8 M_K^{10} s_\theta^{11}}{729 F^2 M_\eta^{10} M_{\eta'}^2} + \\
& \frac{606208 \sqrt{2} c_\theta L_8^2 r M_\theta^8 M_K^8 M_\pi^2 s_\theta^{11}}{243 F^2 M_\eta^{10} M_{\eta'}^2} - \frac{65536 \sqrt{2} c_\theta L_8^2 r M_\theta^8 M_K^6 M_\pi^4 s_\theta^{11}}{27 F^2 M_\eta^{10} M_{\eta'}^2} + \\
& \frac{630784 \sqrt{2} c_\theta L_8^2 r M_\theta^8 M_K^4 M_\pi^6 s_\theta^{11}}{729 F^2 M_\eta^{10} M_{\eta'}^2} + \frac{10240 \sqrt{2} c_\theta L_8^2 r M_\theta^8 M_K^2 M_\pi^8 s_\theta^{11}}{243 F^2 M_\eta^{10} M_{\eta'}^2} - \\
& \frac{2048 \sqrt{2} c_\theta L_8^2 r M_\theta^8 M_\pi^{10} s_\theta^{11}}{27 F^2 M_\eta^{10} M_{\eta'}^2} - \frac{5 c_\theta M_\theta^8 M_\pi^4 s_\theta^{11}}{243 \sqrt{2} \pi^2 M_\eta^6 M_{\eta'}^2} - \frac{\operatorname{Log} \left[ \frac{M_\eta^2}{\mu^2} \right] c_\theta M_\theta^8 M_\pi^4 s_\theta^{11}}{243 \sqrt{2} \pi^2 M_\eta^6 M_{\eta'}^2} - \\
& \frac{\sqrt{2} \operatorname{Log} \left[ \frac{M_\eta^2}{\mu^2} \right] c_\theta M_\theta^8 M_\pi^4 s_\theta^{11}}{243 \pi^2 M_\eta^6 M_{\eta'}^2} + \frac{2 \sqrt{2} \operatorname{Log} \left[ \frac{M_\eta^2}{\mu^2} \right] c_\theta M_\theta^8 M_\pi^4 s_\theta^{11}}{729 \pi^2 M_\eta^6 M_{\eta'}^2} + \frac{2 \sqrt{2} c_\theta M_\theta^8 M_K^2 M_\pi^2 s_\theta^{11}}{243 \pi^2 M_\eta^6 M_{\eta'}^2} + \\
& \frac{\operatorname{Log} \left[ \frac{M_\eta^2}{\mu^2} \right] c_\theta M_\theta^8 M_K^2 M_\pi^2 s_\theta^{11}}{486 \sqrt{2} \pi^2 M_\eta^6 M_{\eta'}^2} + \frac{2 \sqrt{2} \operatorname{Log} \left[ \frac{M_\eta^2}{\mu^2} \right] c_\theta M_\theta^8 M_K^2 M_\pi^2 s_\theta^{11}}{243 \pi^2 M_\eta^6 M_{\eta'}^2} - \frac{55 \operatorname{Log} \left[ \frac{M_\eta^2}{\mu^2} \right] c_\theta M_\theta^8 M_K^2 M_\pi^2 s_\theta^{11}}{2916 \sqrt{2} \pi^2 M_\eta^6 M_{\eta'}^2} + \\
& \frac{4 \sqrt{2} \operatorname{Log} \left[ \frac{M_\eta^2}{\mu^2} \right] c_\theta M_\theta^8 M_K^2 M_\pi^2 s_\theta^{11}}{729 \pi^2 M_\eta^6 M_{\eta'}^2} - \frac{c_\theta M_\theta^8 M_\pi^4 s_\theta^{11}}{1944 \sqrt{2} \pi^2 M_\eta^6 M_{\eta'}^2} + \frac{\operatorname{Log} \left[ \frac{M_\eta^2}{\mu^2} \right] c_\theta M_\theta^8 M_\pi^4 s_\theta^{11}}{486 \sqrt{2} \pi^2 M_\eta^6 M_{\eta'}^2} - \\
& \frac{\sqrt{2} \operatorname{Log} \left[ \frac{M_\eta^2}{\mu^2} \right] c_\theta M_\theta^8 M_\pi^4 s_\theta^{11}}{243 \pi^2 M_\eta^6 M_{\eta'}^2} + \frac{7 \operatorname{Log} \left[ \frac{M_\eta^2}{\mu^2} \right] c_\theta M_\theta^8 M_\pi^4 s_\theta^{11}}{2916 \sqrt{2} \pi^2 M_\eta^6 M_{\eta'}^2} - \frac{5 \sqrt{2} \operatorname{Log} \left[ \frac{M_\eta^2}{\mu^2} \right] c_\theta M_\theta^8 M_K^4 M_\pi^2 s_\theta^{11}}{729 \pi^2 M_\eta^{10}} -
\end{aligned}$$

$$\begin{aligned}
& \frac{\text{Log}\left[\frac{M_{\eta'}^2}{\mu^2}\right] c_{\theta} M_0^8 M_K^2 M_{\pi}^2 M_{\eta'}^2 s_{\theta}^{11}}{1458 \sqrt{2} \pi^2 M_{\eta}^{10}} + \frac{5 \sqrt{2} \text{Log}\left[\frac{M_{\eta'}^2}{\mu^2}\right] c_{\theta} M_0^8 M_K^2 M_{\pi}^2 M_{\eta'}^2 s_{\theta}^{11}}{729 \pi^2 M_{\eta}^{10}} + \\
& \frac{\text{Log}\left[\frac{M_{\eta'}^2}{\mu^2}\right] c_{\theta} M_0^8 M_{\pi}^4 M_{\eta'}^2 s_{\theta}^{11}}{2916 \sqrt{2} \pi^2 M_{\eta}^{10}} - \frac{\sqrt{2} \text{Log}\left[\frac{M_{\eta'}^2}{\mu^2}\right] c_{\theta} M_0^8 M_{\pi}^4 M_{\eta'}^2 s_{\theta}^{11}}{729 \pi^2 M_{\eta}^{10}} + \frac{5 \text{Log}\left[\frac{M_{\eta'}^2}{\mu^2}\right] c_{\theta} M_0^8 M_K^4 s_{\theta}^{11}}{243 \sqrt{2} \pi^2 M_{\eta}^6 (M_{\eta}^2 - M_{\eta'}^2)} + \\
& \frac{2 \sqrt{2} \text{Log}\left[\frac{M_{\eta'}^2}{\mu^2}\right] c_{\theta} M_0^8 M_K^4 s_{\theta}^{11}}{243 \pi^2 M_{\eta}^6 (M_{\eta}^2 - M_{\eta'}^2)} - \frac{7 \text{Log}\left[\frac{M_{\eta'}^2}{\mu^2}\right] c_{\theta} M_0^8 M_K^2 M_{\pi}^2 s_{\theta}^{11}}{243 \sqrt{2} \pi^2 M_{\eta}^6 (M_{\eta}^2 - M_{\eta'}^2)} - \frac{5 \text{Log}\left[\frac{M_{\eta'}^2}{\mu^2}\right] c_{\theta} M_0^8 M_K^2 M_{\pi}^2 s_{\theta}^{11}}{243 \sqrt{2} \pi^2 M_{\eta}^6 (M_{\eta}^2 - M_{\eta'}^2)} + \\
& \frac{\sqrt{2} \text{Log}\left[\frac{M_{\eta'}^2}{\mu^2}\right] c_{\theta} M_0^8 M_{\pi}^4 s_{\theta}^{11}}{243 \pi^2 M_{\eta}^6 (M_{\eta}^2 - M_{\eta'}^2)} + \frac{\text{Log}\left[\frac{M_{\eta'}^2}{\mu^2}\right] c_{\theta} M_0^8 M_{\pi}^4 s_{\theta}^{11}}{243 \sqrt{2} \pi^2 M_{\eta}^6 (M_{\eta}^2 - M_{\eta'}^2)} - \frac{2 \sqrt{2} \text{Log}\left[\frac{M_{\eta'}^2}{\mu^2}\right] c_{\theta} M_0^8 M_K^4 s_{\theta}^{11}}{243 \pi^2 M_{\eta}^4 M_{\eta'}^2 (M_{\eta}^2 - M_{\eta'}^2)} + \\
& \frac{5 \text{Log}\left[\frac{M_{\eta'}^2}{\mu^2}\right] c_{\theta} M_0^8 M_K^2 M_{\pi}^2 s_{\theta}^{11}}{243 \sqrt{2} \pi^2 M_{\eta}^4 M_{\eta'}^2 (M_{\eta}^2 - M_{\eta'}^2)} - \frac{\text{Log}\left[\frac{M_{\eta'}^2}{\mu^2}\right] c_{\theta} M_0^8 M_{\pi}^4 s_{\theta}^{11}}{243 \sqrt{2} \pi^2 M_{\eta}^4 M_{\eta'}^2 (M_{\eta}^2 - M_{\eta'}^2)} - \frac{5 \text{Log}\left[\frac{M_{\eta'}^2}{\mu^2}\right] c_{\theta} M_0^8 M_K^4 M_{\eta'}^2 s_{\theta}^{11}}{243 \sqrt{2} \pi^2 M_{\eta}^8 (M_{\eta}^2 - M_{\eta'}^2)} + \\
& \frac{7 \text{Log}\left[\frac{M_{\eta'}^2}{\mu^2}\right] c_{\theta} M_0^8 M_K^2 M_{\pi}^2 M_{\eta'}^2 s_{\theta}^{11}}{243 \sqrt{2} \pi^2 M_{\eta}^8 (M_{\eta}^2 - M_{\eta'}^2)} - \frac{\sqrt{2} \text{Log}\left[\frac{M_{\eta'}^2}{\mu^2}\right] c_{\theta} M_0^8 M_{\pi}^4 M_{\eta'}^2 s_{\theta}^{11}}{243 \pi^2 M_{\eta}^8 (M_{\eta}^2 - M_{\eta'}^2)} - \frac{40960 L_8^2 r M_0^8 M_K^{10} s_{\theta}^{12}}{729 F^2 M_{\eta}^{12}} + \\
& \frac{20480 L_8^2 r M_0^8 M_K^8 M_{\pi}^2 s_{\theta}^{12}}{243 F^2 M_{\eta}^{12}} - \frac{20480 L_8^2 r M_0^8 M_K^6 M_{\pi}^4 s_{\theta}^{12}}{243 F^2 M_{\eta}^{12}} + \frac{10240 L_8^2 r M_0^8 M_K^4 M_{\pi}^6 s_{\theta}^{12}}{729 F^2 M_{\eta}^{12}} + \\
& \frac{2560 L_8^2 r M_0^8 M_K^2 M_{\pi}^8 s_{\theta}^{12}}{243 F^2 M_{\eta}^{12}} - \frac{1280 L_8^2 r M_0^8 M_{\pi}^{10} s_{\theta}^{12}}{81 F^2 M_{\eta}^{12}} + \frac{5 M_0^8 M_K^4 s_{\theta}^{12}}{1944 \pi^2 M_{\eta}^8} - \frac{\text{Log}\left[\frac{M_{\eta'}^2}{\mu^2}\right] M_0^8 M_K^4 s_{\theta}^{12}}{5832 \pi^2 M_{\eta}^8} - \\
& \frac{\text{Log}\left[\frac{M_{\eta'}^2}{\mu^2}\right] M_0^8 M_K^4 s_{\theta}^{12}}{1458 \pi^2 M_{\eta}^8} - \frac{M_0^8 M_K^2 M_{\pi}^2 s_{\theta}^{12}}{1944 \pi^2 M_{\eta}^8} - \frac{\text{Log}\left[\frac{M_{\eta'}^2}{\mu^2}\right] M_0^8 M_K^2 M_{\pi}^2 s_{\theta}^{12}}{5832 \pi^2 M_{\eta}^8} + \frac{5 \text{Log}\left[\frac{M_{\eta'}^2}{\mu^2}\right] M_0^8 M_K^2 M_{\pi}^2 s_{\theta}^{12}}{1458 \pi^2 M_{\eta}^8} + \\
& \frac{M_0^8 M_{\pi}^4 s_{\theta}^{12}}{3888 \pi^2 M_{\eta}^8} - \frac{\text{Log}\left[\frac{M_{\eta'}^2}{\mu^2}\right] M_0^8 M_{\pi}^4 s_{\theta}^{12}}{23328 \pi^2 M_{\eta}^8} - \frac{37 \text{Log}\left[\frac{M_{\eta'}^2}{\mu^2}\right] M_0^8 M_{\pi}^4 s_{\theta}^{12}}{23328 \pi^2 M_{\eta}^8} - \frac{163840 L_8^2 r M_0^8 M_K^{10} s_{\theta}^{12}}{729 F^2 M_{\eta}^8 M_{\eta'}^4} + \\
& \frac{139264 L_8^2 r M_0^8 M_K^8 M_{\pi}^2 s_{\theta}^{12}}{243 F^2 M_{\eta}^8 M_{\eta'}^4} - \frac{40960 L_8^2 r M_0^8 M_K^6 M_{\pi}^4 s_{\theta}^{12}}{81 F^2 M_{\eta}^8 M_{\eta'}^4} + \frac{139264 L_8^2 r M_0^8 M_K^4 M_{\pi}^6 s_{\theta}^{12}}{729 F^2 M_{\eta}^8 M_{\eta'}^4} - \\
& \frac{8192 L_8^2 r M_0^8 M_K^2 M_{\pi}^8 s_{\theta}^{12}}{243 F^2 M_{\eta}^8 M_{\eta'}^4} - \frac{163840 L_8^2 r M_0^8 M_K^{10} s_{\theta}^{12}}{729 F^2 M_{\eta}^{10} M_{\eta'}^2} + \frac{16384 L_8^2 r M_0^8 M_K^8 M_{\pi}^2 s_{\theta}^{12}}{27 F^2 M_{\eta}^{10} M_{\eta'}^2} - \\
& \frac{163840 L_8^2 r M_0^8 M_K^6 M_{\pi}^4 s_{\theta}^{12}}{243 F^2 M_{\eta}^{10} M_{\eta'}^2} + \frac{311296 L_8^2 r M_0^8 M_K^4 M_{\pi}^6 s_{\theta}^{12}}{729 F^2 M_{\eta}^{10} M_{\eta'}^2} - \frac{32768 L_8^2 r M_0^8 M_K^2 M_{\pi}^8 s_{\theta}^{12}}{243 F^2 M_{\eta}^{10} M_{\eta'}^2} - \\
& \frac{\text{Log}\left[\frac{M_{\eta'}^2}{\mu^2}\right] M_0^8 M_K^4 s_{\theta}^{12}}{729 \pi^2 M_{\eta}^6 M_{\eta'}^2} + \frac{2 \text{Log}\left[\frac{M_{\eta'}^2}{\mu^2}\right] M_0^8 M_K^2 M_{\pi}^2 s_{\theta}^{12}}{729 \pi^2 M_{\eta}^6 M_{\eta'}^2} - \frac{\text{Log}\left[\frac{M_{\eta'}^2}{\mu^2}\right] M_0^8 M_{\pi}^4 s_{\theta}^{12}}{729 \pi^2 M_{\eta}^6 M_{\eta'}^2} - \frac{\text{Log}\left[\frac{M_{\eta'}^2}{\mu^2}\right] M_0^8 M_K^4 M_{\eta'}^2 s_{\theta}^{12}}{729 \pi^2 M_{\eta}^{10}} - \\
& \frac{\text{Log}\left[\frac{M_{\eta'}^2}{\mu^2}\right] M_0^8 M_K^2 M_{\pi}^2 M_{\eta'}^2 s_{\theta}^{12}}{2916 \pi^2 M_{\eta}^{10}} + \frac{\text{Log}\left[\frac{M_{\eta'}^2}{\mu^2}\right] M_0^8 M_{\pi}^4 M_{\eta'}^2 s_{\theta}^{12}}{5832 \pi^2 M_{\eta}^{10}} + \frac{\text{Log}\left[\frac{M_{\eta'}^2}{\mu^2}\right] M_0^8 M_K^4 s_{\theta}^{12}}{486 \pi^2 M_{\eta}^6 (M_{\eta}^2 - M_{\eta'}^2)} -
\end{aligned}$$

$$\begin{aligned}
& \frac{\text{Log} \left[ \frac{M_\eta^2}{\mu^2} \right] M_\theta^8 M_K^2 M_\pi^2 s_\theta^{12}}{243 \pi^2 M_\eta^6 (M_\eta^2 - M_{\eta'}^2)} + \frac{\text{Log} \left[ \frac{M_\eta^2}{\mu^2} \right] M_\theta^8 M_\pi^4 s_\theta^{12}}{486 \pi^2 M_\eta^6 (M_\eta^2 - M_{\eta'}^2)} - \frac{\text{Log} \left[ \frac{M_{\eta'}^2}{\mu^2} \right] M_\theta^8 M_K^4 M_{\eta'}^2 s_\theta^{12}}{486 \pi^2 M_\eta^6 (M_\eta^2 - M_{\eta'}^2)} + \\
& \frac{\text{Log} \left[ \frac{M_{\eta'}^2}{\mu^2} \right] M_\theta^8 M_K^2 M_\pi^2 M_{\eta'}^2 s_\theta^{12}}{243 \pi^2 M_\eta^6 (M_\eta^2 - M_{\eta'}^2)} - \frac{\text{Log} \left[ \frac{M_{\eta'}^2}{\mu^2} \right] M_\theta^8 M_\pi^4 M_{\eta'}^2 s_\theta^{12}}{486 \pi^2 M_\eta^6 (M_\eta^2 - M_{\eta'}^2)} - \frac{5120 c_\theta^{12} L_8^r M_\theta^8 M_K^8 \Lambda_2}{729 M_{\eta'}^{12}} - \\
& \frac{2560 c_\theta^{12} L_8^r M_\theta^8 M_K^2 M_\pi^6 \Lambda_2}{729 M_{\eta'}^{12}} - \frac{320 c_\theta^{12} L_8^r M_\theta^8 M_\pi^8 \Lambda_2}{243 M_{\eta'}^{12}} + \frac{1024 c_\theta^{10} L_8^r M_\theta^8 M_K^6 \Lambda_2}{243 M_{\eta'}^{10}} + \frac{2048 c_\theta^{10} L_8^r M_\theta^6 M_K^8 \Lambda_2}{729 M_{\eta'}^{10}} - \\
& \frac{512 c_\theta^{10} L_8^r M_\theta^8 M_K^4 M_\pi^2 \Lambda_2}{243 M_{\eta'}^{10}} + \frac{256 c_\theta^{10} L_8^r M_\theta^8 M_K^2 M_\pi^4 \Lambda_2}{243 M_{\eta'}^{10}} + \frac{128 c_\theta^{10} L_8^r M_\theta^8 M_\pi^6 \Lambda_2}{81 M_{\eta'}^{10}} + \frac{1024 c_\theta^{10} L_8^r M_\theta^6 M_K^2 M_\pi^6 \Lambda_2}{729 M_{\eta'}^{10}} + \\
& \frac{128 c_\theta^{10} L_8^r M_\theta^6 M_\pi^8 \Lambda_2}{243 M_{\eta'}^{10}} - \frac{14 336 c_\theta^{12} L_8^r M_\theta^8 M_K^8 \Lambda_2}{729 M_\eta^2 M_{\eta'}^{10}} + \frac{1024 c_\theta^{12} L_8^r M_\theta^8 M_K^6 M_\pi^2 \Lambda_2}{27 M_\eta^2 M_{\eta'}^{10}} - \\
& \frac{5120 c_\theta^{12} L_8^r M_\theta^8 M_K^4 M_\pi^4 \Lambda_2}{243 M_\eta^2 M_{\eta'}^{10}} + \frac{5120 c_\theta^{12} L_8^r M_\theta^8 M_K^2 M_\pi^6 \Lambda_2}{729 M_\eta^2 M_{\eta'}^{10}} - \frac{1024 c_\theta^{12} L_8^r M_\theta^8 M_\pi^8 \Lambda_2}{243 M_\eta^2 M_{\eta'}^{10}} - \frac{1024 c_\theta^8 L_8^r M_\theta^6 M_K^6 \Lambda_2}{243 M_{\eta'}^8} + \\
& \frac{512 c_\theta^8 L_8^r M_\theta^6 M_K^4 M_\pi^2 \Lambda_2}{243 M_{\eta'}^8} - \frac{256 c_\theta^8 L_8^r M_\theta^6 M_K^2 M_\pi^4 \Lambda_2}{243 M_{\eta'}^8} - \frac{128 c_\theta^8 L_8^r M_\theta^6 M_\pi^6 \Lambda_2}{81 M_{\eta'}^8} - \frac{8192 c_\theta^{12} L_8^r M_\theta^8 M_K^8 \Lambda_2}{729 M_\eta^4 M_{\eta'}^8} + \\
& \frac{6656 c_\theta^{12} L_8^r M_\theta^8 M_K^6 M_\pi^2 \Lambda_2}{243 M_\eta^4 M_{\eta'}^8} - \frac{1792 c_\theta^{12} L_8^r M_\theta^8 M_K^4 M_\pi^4 \Lambda_2}{81 M_\eta^4 M_{\eta'}^8} + \frac{5120 c_\theta^{12} L_8^r M_\theta^8 M_K^2 M_\pi^6 \Lambda_2}{729 M_\eta^4 M_{\eta'}^8} - \\
& \frac{256 c_\theta^{12} L_8^r M_\theta^8 M_\pi^8 \Lambda_2}{243 M_\eta^4 M_{\eta'}^8} + \frac{512 c_\theta^{10} L_8^r M_\theta^8 M_K^6 \Lambda_2}{81 M_\eta^2 M_{\eta'}^8} + \frac{8192 c_\theta^{10} L_8^r M_\theta^6 M_K^8 \Lambda_2}{729 M_\eta^2 M_{\eta'}^8} - \frac{1024 c_\theta^{10} L_8^r M_\theta^6 M_K^4 M_\pi^2 \Lambda_2}{81 M_\eta^2 M_{\eta'}^8} - \\
& \frac{5632 c_\theta^{10} L_8^r M_\theta^6 M_K^6 M_\pi^2 \Lambda_2}{243 M_\eta^2 M_{\eta'}^8} + \frac{512 c_\theta^{10} L_8^r M_\theta^8 M_K^2 M_\pi^4 \Lambda_2}{81 M_\eta^2 M_{\eta'}^8} + \frac{1280 c_\theta^{10} L_8^r M_\theta^6 M_K^4 M_\pi^4 \Lambda_2}{81 M_\eta^2 M_{\eta'}^8} - \\
& \frac{5120 c_\theta^{10} L_8^r M_\theta^6 M_K^2 M_\pi^6 \Lambda_2}{729 M_\eta^2 M_{\eta'}^8} + \frac{256 c_\theta^{10} L_8^r M_\theta^6 M_\pi^8 \Lambda_2}{81 M_\eta^2 M_{\eta'}^8} + \frac{8192 c_\theta^{10} L_8^r M_\theta^6 M_K^8 \Lambda_2}{729 M_\eta^4 M_{\eta'}^6} - \frac{6656 c_\theta^{10} L_8^r M_\theta^6 M_K^6 M_\pi^2 \Lambda_2}{243 M_\eta^4 M_{\eta'}^6} + \\
& \frac{1792 c_\theta^{10} L_8^r M_\theta^6 M_K^4 M_\pi^4 \Lambda_2}{81 M_\eta^4 M_{\eta'}^6} - \frac{5120 c_\theta^{10} L_8^r M_\theta^6 M_K^2 M_\pi^6 \Lambda_2}{729 M_\eta^4 M_{\eta'}^6} + \frac{256 c_\theta^{10} L_8^r M_\theta^6 M_\pi^8 \Lambda_2}{243 M_\eta^4 M_{\eta'}^6} - \frac{2048 c_\theta^8 L_8^r M_\theta^6 M_K^6 \Lambda_2}{243 M_\eta^2 M_{\eta'}^6} + \\
& \frac{4096 c_\theta^8 L_8^r M_\theta^6 M_K^4 M_\pi^2 \Lambda_2}{243 M_\eta^2 M_{\eta'}^6} - \frac{2048 c_\theta^8 L_8^r M_\theta^6 M_K^2 M_\pi^4 \Lambda_2}{243 M_\eta^2 M_{\eta'}^6} + \frac{35 840 \sqrt{2} c_\theta^{11} L_8^r M_\theta^8 M_K^8 s_\theta \Lambda_2}{729 M_{\eta'}^{12}} - \\
& \frac{12 800 \sqrt{2} c_\theta^{11} L_8^r M_\theta^8 M_K^6 M_\pi^2 s_\theta \Lambda_2}{243 M_{\eta'}^{12}} + \frac{1280 \sqrt{2} c_\theta^{11} L_8^r M_\theta^8 M_K^4 M_\pi^4 s_\theta \Lambda_2}{81 M_{\eta'}^{12}} + \\
& \frac{640 \sqrt{2} c_\theta^{11} L_8^r M_\theta^8 M_K^2 M_\pi^6 s_\theta \Lambda_2}{729 M_{\eta'}^{12}} - \frac{3200 \sqrt{2} c_\theta^{11} L_8^r M_\theta^8 M_\pi^8 s_\theta \Lambda_2}{243 M_{\eta'}^{12}} - \frac{5120 \sqrt{2} c_\theta^9 L_8^r M_\theta^8 M_K^6 s_\theta \Lambda_2}{243 M_{\eta'}^{10}} - \\
& \frac{14 336 \sqrt{2} c_\theta^9 L_8^r M_\theta^6 M_K^8 s_\theta \Lambda_2}{729 M_{\eta'}^{10}} + \frac{7168 \sqrt{2} c_\theta^9 L_8^r M_\theta^8 M_K^4 M_\pi^2 s_\theta \Lambda_2}{243 M_{\eta'}^{10}} + \frac{5120 \sqrt{2} c_\theta^9 L_8^r M_\theta^6 M_K^6 M_\pi^2 s_\theta \Lambda_2}{243 M_{\eta'}^{10}} - \\
& \frac{4352 \sqrt{2} c_\theta^9 L_8^r M_\theta^8 M_K^2 M_\pi^4 s_\theta \Lambda_2}{243 M_{\eta'}^{10}} - \frac{512 \sqrt{2} c_\theta^9 L_8^r M_\theta^6 M_K^4 M_\pi^4 s_\theta \Lambda_2}{81 M_{\eta'}^{10}} + \frac{256 \sqrt{2} c_\theta^9 L_8^r M_\theta^6 M_\pi^6 s_\theta \Lambda_2}{27 M_{\eta'}^{10}} -
\end{aligned}$$

$$\begin{aligned}
& \frac{256 \sqrt{2} c_{\theta}^9 L_8^r M_0^6 M_K^2 M_{\pi}^6 s_{\theta} \Lambda_2}{729 M_{\eta'}^{10}} + \frac{1280 \sqrt{2} c_{\theta}^9 L_8^r M_0^6 M_{\pi}^8 s_{\theta} \Lambda_2}{243 M_{\eta'}^{10}} + \frac{35840 \sqrt{2} c_{\theta}^{11} L_8^r M_0^8 M_K^8 s_{\theta} \Lambda_2}{729 M_{\eta'}^2 M_{\eta'}^{10}} - \\
& \frac{3584 \sqrt{2} c_{\theta}^{11} L_8^r M_0^8 M_K^6 M_{\pi}^2 s_{\theta} \Lambda_2}{27 M_{\eta'}^2 M_{\eta'}^{10}} + \frac{28160 \sqrt{2} c_{\theta}^{11} L_8^r M_0^8 M_K^4 M_{\pi}^4 s_{\theta} \Lambda_2}{243 M_{\eta'}^2 M_{\eta'}^{10}} - \\
& \frac{33536 \sqrt{2} c_{\theta}^{11} L_8^r M_0^8 M_K^2 M_{\pi}^6 s_{\theta} \Lambda_2}{729 M_{\eta'}^2 M_{\eta'}^{10}} + \frac{3328 \sqrt{2} c_{\theta}^{11} L_8^r M_0^8 M_{\pi}^8 s_{\theta} \Lambda_2}{243 M_{\eta'}^2 M_{\eta'}^{10}} + \frac{5120 \sqrt{2} c_{\theta}^7 L_8^r M_0^6 M_K^6 s_{\theta} \Lambda_2}{243 M_{\eta'}^8} - \\
& \frac{4096 \sqrt{2} c_{\theta}^7 L_8^r M_0^6 M_K^4 M_{\pi}^2 s_{\theta} \Lambda_2}{243 M_{\eta'}^8} - \frac{256 \sqrt{2} c_{\theta}^7 L_8^r M_0^6 M_K^2 M_{\pi}^4 s_{\theta} \Lambda_2}{243 M_{\eta'}^8} - \frac{256 \sqrt{2} c_{\theta}^7 L_8^r M_0^6 M_{\pi}^6 s_{\theta} \Lambda_2}{81 M_{\eta'}^8} - \\
& \frac{47104 \sqrt{2} c_{\theta}^{11} L_8^r M_0^8 M_K^8 s_{\theta} \Lambda_2}{729 M_{\eta'}^4 M_{\eta'}^8} + \frac{25088 \sqrt{2} c_{\theta}^{11} L_8^r M_0^8 M_K^6 M_{\pi}^2 s_{\theta} \Lambda_2}{243 M_{\eta'}^4 M_{\eta'}^8} - \\
& \frac{15104 \sqrt{2} c_{\theta}^{11} L_8^r M_0^8 M_K^4 M_{\pi}^4 s_{\theta} \Lambda_2}{243 M_{\eta'}^4 M_{\eta'}^8} + \frac{16384 \sqrt{2} c_{\theta}^{11} L_8^r M_0^8 M_K^2 M_{\pi}^6 s_{\theta} \Lambda_2}{729 M_{\eta'}^4 M_{\eta'}^8} + \\
& \frac{256 \sqrt{2} c_{\theta}^{11} L_8^r M_0^8 M_{\pi}^8 s_{\theta} \Lambda_2}{243 M_{\eta'}^4 M_{\eta'}^8} + \frac{512 \sqrt{2} c_{\theta}^9 L_8^r M_0^8 M_K^6 s_{\theta} \Lambda_2}{243 M_{\eta'}^2 M_{\eta'}^8} - \frac{26624 \sqrt{2} c_{\theta}^9 L_8^r M_0^6 M_K^8 s_{\theta} \Lambda_2}{729 M_{\eta'}^2 M_{\eta'}^8} - \\
& \frac{256 \sqrt{2} c_{\theta}^9 L_8^r M_0^8 M_K^4 M_{\pi}^2 s_{\theta} \Lambda_2}{243 M_{\eta'}^2 M_{\eta'}^8} + \frac{21760 \sqrt{2} c_{\theta}^9 L_8^r M_0^6 M_K^6 M_{\pi}^2 s_{\theta} \Lambda_2}{243 M_{\eta'}^2 M_{\eta'}^8} + \frac{1472 \sqrt{2} c_{\theta}^9 L_8^r M_0^8 M_K^2 M_{\pi}^4 s_{\theta} \Lambda_2}{243 M_{\eta'}^2 M_{\eta'}^8} - \\
& \frac{6272 \sqrt{2} c_{\theta}^9 L_8^r M_0^6 M_K^4 M_{\pi}^4 s_{\theta} \Lambda_2}{81 M_{\eta'}^2 M_{\eta'}^8} - \frac{64 \sqrt{2} c_{\theta}^9 L_8^r M_0^8 M_{\pi}^6 s_{\theta} \Lambda_2}{9 M_{\eta'}^2 M_{\eta'}^8} + \frac{22400 \sqrt{2} c_{\theta}^9 L_8^r M_0^6 M_K^2 M_{\pi}^6 s_{\theta} \Lambda_2}{729 M_{\eta'}^2 M_{\eta'}^8} - \\
& \frac{512 \sqrt{2} c_{\theta}^9 L_8^r M_0^6 M_{\pi}^8 s_{\theta} \Lambda_2}{81 M_{\eta'}^2 M_{\eta'}^8} - \frac{8192 \sqrt{2} c_{\theta}^{11} L_8^r M_0^8 M_K^8 s_{\theta} \Lambda_2}{243 M_{\eta'}^6 M_{\eta'}^6} + \frac{6656 \sqrt{2} c_{\theta}^{11} L_8^r M_0^8 M_K^6 M_{\pi}^2 s_{\theta} \Lambda_2}{81 M_{\eta'}^6 M_{\eta'}^6} - \\
& \frac{5632 \sqrt{2} c_{\theta}^{11} L_8^r M_0^8 M_K^4 M_{\pi}^4 s_{\theta} \Lambda_2}{81 M_{\eta'}^6 M_{\eta'}^6} + \frac{5504 \sqrt{2} c_{\theta}^{11} L_8^r M_0^8 M_K^2 M_{\pi}^6 s_{\theta} \Lambda_2}{243 M_{\eta'}^6 M_{\eta'}^6} - \frac{128 \sqrt{2} c_{\theta}^{11} L_8^r M_0^8 M_{\pi}^8 s_{\theta} \Lambda_2}{81 M_{\eta'}^6 M_{\eta'}^6} + \\
& \frac{512 \sqrt{2} c_{\theta}^9 L_8^r M_0^8 M_K^6 s_{\theta} \Lambda_2}{27 M_{\eta'}^4 M_{\eta'}^6} + \frac{16384 \sqrt{2} c_{\theta}^9 L_8^r M_0^6 M_K^8 s_{\theta} \Lambda_2}{729 M_{\eta'}^4 M_{\eta'}^6} - \frac{256 \sqrt{2} c_{\theta}^9 L_8^r M_0^8 M_K^4 M_{\pi}^2 s_{\theta} \Lambda_2}{9 M_{\eta'}^4 M_{\eta'}^6} - \\
& \frac{256 \sqrt{2} c_{\theta}^9 L_8^r M_0^6 M_K^6 M_{\pi}^2 s_{\theta} \Lambda_2}{9 M_{\eta'}^4 M_{\eta'}^6} + \frac{320 \sqrt{2} c_{\theta}^9 L_8^r M_0^8 M_K^2 M_{\pi}^4 s_{\theta} \Lambda_2}{27 M_{\eta'}^4 M_{\eta'}^6} + \frac{128 \sqrt{2} c_{\theta}^9 L_8^r M_0^6 M_K^4 M_{\pi}^4 s_{\theta} \Lambda_2}{9 M_{\eta'}^4 M_{\eta'}^6} - \\
& \frac{64 \sqrt{2} c_{\theta}^9 L_8^r M_0^8 M_{\pi}^6 s_{\theta} \Lambda_2}{27 M_{\eta'}^4 M_{\eta'}^6} - \frac{5632 \sqrt{2} c_{\theta}^9 L_8^r M_0^6 M_K^2 M_{\pi}^6 s_{\theta} \Lambda_2}{729 M_{\eta'}^4 M_{\eta'}^6} - \frac{128 \sqrt{2} c_{\theta}^9 L_8^r M_0^6 M_{\pi}^8 s_{\theta} \Lambda_2}{243 M_{\eta'}^4 M_{\eta'}^6} + \\
& \frac{1024 \sqrt{2} c_{\theta}^7 L_8^r M_0^6 M_K^6 s_{\theta} \Lambda_2}{243 M_{\eta'}^2 M_{\eta'}^6} - \frac{8192 \sqrt{2} c_{\theta}^7 L_8^r M_0^6 M_K^4 M_{\pi}^2 s_{\theta} \Lambda_2}{243 M_{\eta'}^2 M_{\eta'}^6} + \frac{8704 \sqrt{2} c_{\theta}^7 L_8^r M_0^6 M_K^2 M_{\pi}^4 s_{\theta} \Lambda_2}{243 M_{\eta'}^2 M_{\eta'}^6} - \\
& \frac{512 \sqrt{2} c_{\theta}^7 L_8^r M_0^6 M_{\pi}^6 s_{\theta} \Lambda_2}{81 M_{\eta'}^2 M_{\eta'}^6} + \frac{8192 \sqrt{2} c_{\theta}^9 L_8^r M_0^6 M_K^8 s_{\theta} \Lambda_2}{243 M_{\eta'}^6 M_{\eta'}^4} - \frac{6656 \sqrt{2} c_{\theta}^9 L_8^r M_0^6 M_K^6 M_{\pi}^2 s_{\theta} \Lambda_2}{81 M_{\eta'}^6 M_{\eta'}^4} +
\end{aligned}$$

$$\begin{aligned}
& \frac{5632 \sqrt{2} c_{\theta}^9 L_8^r M_0^6 M_K^4 M_{\pi}^4 s_{\theta} \Lambda_2}{81 M_{\eta}^6 M_{\eta'}^4} - \frac{5504 \sqrt{2} c_{\theta}^9 L_8^r M_0^6 M_K^2 M_{\pi}^6 s_{\theta} \Lambda_2}{243 M_{\eta}^6 M_{\eta'}^4} + \frac{128 \sqrt{2} c_{\theta}^9 L_8^r M_0^6 M_{\pi}^8 s_{\theta} \Lambda_2}{81 M_{\eta}^6 M_{\eta'}^4} - \\
& \frac{2048 \sqrt{2} c_{\theta}^7 L_8^r M_0^6 M_K^6 s_{\theta} \Lambda_2}{81 M_{\eta}^4 M_{\eta'}^4} + \frac{4096 \sqrt{2} c_{\theta}^7 L_8^r M_0^6 M_K^4 M_{\pi}^2 s_{\theta} \Lambda_2}{81 M_{\eta}^4 M_{\eta'}^4} - \frac{2816 \sqrt{2} c_{\theta}^7 L_8^r M_0^6 M_K^2 M_{\pi}^4 s_{\theta} \Lambda_2}{81 M_{\eta}^4 M_{\eta'}^4} + \\
& \frac{256 \sqrt{2} c_{\theta}^7 L_8^r M_0^6 M_{\pi}^6 s_{\theta} \Lambda_2}{27 M_{\eta}^4 M_{\eta'}^4} - \frac{71\,680 c_{\theta}^{10} L_8^r M_0^8 M_K^8 s_{\theta}^2 \Lambda_2}{243 M_{\eta}^{12}} + \frac{35\,840 c_{\theta}^{10} L_8^r M_0^8 M_K^6 M_{\pi}^2 s_{\theta}^2 \Lambda_2}{81 M_{\eta}^{12}} - \\
& \frac{6400 c_{\theta}^{10} L_8^r M_0^8 M_K^4 M_{\pi}^4 s_{\theta}^2 \Lambda_2}{27 M_{\eta}^{12}} + \frac{10\,240 c_{\theta}^{10} L_8^r M_0^8 M_K^2 M_{\pi}^6 s_{\theta}^2 \Lambda_2}{243 M_{\eta}^{12}} - \frac{320 c_{\theta}^{10} L_8^r M_0^8 M_{\pi}^8 s_{\theta}^2 \Lambda_2}{9 M_{\eta}^{12}} + \\
& \frac{20\,480 c_{\theta}^8 L_8^r M_0^8 M_K^6 s_{\theta}^2 \Lambda_2}{243 M_{\eta}^{10}} + \frac{28\,672 c_{\theta}^8 L_8^r M_0^8 M_K^4 s_{\theta}^2 \Lambda_2}{243 M_{\eta}^{10}} - \frac{33\,280 c_{\theta}^8 L_8^r M_0^8 M_K^2 M_{\pi}^2 s_{\theta}^2 \Lambda_2}{243 M_{\eta}^{10}} - \\
& \frac{14\,336 c_{\theta}^8 L_8^r M_0^8 M_K^6 M_{\pi}^2 s_{\theta}^2 \Lambda_2}{81 M_{\eta}^{10}} + \frac{18\,176 c_{\theta}^8 L_8^r M_0^8 M_K^4 M_{\pi}^4 s_{\theta}^2 \Lambda_2}{243 M_{\eta}^{10}} + \frac{2560 c_{\theta}^8 L_8^r M_0^8 M_K^2 M_{\pi}^6 s_{\theta}^2 \Lambda_2}{27 M_{\eta}^{10}} - \\
& \frac{256 c_{\theta}^8 L_8^r M_0^8 M_{\pi}^8 s_{\theta}^2 \Lambda_2}{81 M_{\eta}^{10}} - \frac{4096 c_{\theta}^8 L_8^r M_0^8 M_K^2 M_{\pi}^6 s_{\theta}^2 \Lambda_2}{243 M_{\eta}^{10}} + \frac{128 c_{\theta}^8 L_8^r M_0^8 M_{\pi}^8 s_{\theta}^2 \Lambda_2}{9 M_{\eta}^{10}} + \\
& \frac{83\,968 c_{\theta}^{10} L_8^r M_0^8 M_K^8 s_{\theta}^2 \Lambda_2}{729 M_{\eta}^2 M_{\eta'}^{10}} - \frac{11\,264 c_{\theta}^{10} L_8^r M_0^8 M_K^6 M_{\pi}^2 s_{\theta}^2 \Lambda_2}{243 M_{\eta}^2 M_{\eta'}^{10}} - \frac{24\,064 c_{\theta}^{10} L_8^r M_0^8 M_K^4 M_{\pi}^4 s_{\theta}^2 \Lambda_2}{243 M_{\eta}^2 M_{\eta'}^{10}} + \\
& \frac{55\,040 c_{\theta}^{10} L_8^r M_0^8 M_K^2 M_{\pi}^6 s_{\theta}^2 \Lambda_2}{729 M_{\eta}^2 M_{\eta'}^{10}} + \frac{5120 c_{\theta}^{10} L_8^r M_0^8 M_{\pi}^8 s_{\theta}^2 \Lambda_2}{243 M_{\eta}^2 M_{\eta'}^{10}} - \frac{20\,480 c_{\theta}^6 L_8^r M_0^6 M_K^6 s_{\theta}^2 \Lambda_2}{243 M_{\eta'}^8} + \\
& \frac{22\,528 c_{\theta}^6 L_8^r M_0^6 M_K^4 M_{\pi}^2 s_{\theta}^2 \Lambda_2}{243 M_{\eta'}^8} - \frac{6656 c_{\theta}^6 L_8^r M_0^6 M_K^2 M_{\pi}^4 s_{\theta}^2 \Lambda_2}{243 M_{\eta'}^8} - \frac{256 c_{\theta}^6 L_8^r M_0^6 M_{\pi}^6 s_{\theta}^2 \Lambda_2}{27 M_{\eta'}^8} + \\
& \frac{219\,136 c_{\theta}^{10} L_8^r M_0^8 M_K^8 s_{\theta}^2 \Lambda_2}{729 M_{\eta}^4 M_{\eta'}^8} - \frac{52\,480 c_{\theta}^{10} L_8^r M_0^8 M_K^6 M_{\pi}^2 s_{\theta}^2 \Lambda_2}{81 M_{\eta}^4 M_{\eta'}^8} + \frac{118\,528 c_{\theta}^{10} L_8^r M_0^8 M_K^4 M_{\pi}^4 s_{\theta}^2 \Lambda_2}{243 M_{\eta}^4 M_{\eta'}^8} - \\
& \frac{120\,640 c_{\theta}^{10} L_8^r M_0^8 M_K^2 M_{\pi}^6 s_{\theta}^2 \Lambda_2}{729 M_{\eta}^4 M_{\eta'}^8} - \frac{256 c_{\theta}^{10} L_8^r M_0^8 M_{\pi}^8 s_{\theta}^2 \Lambda_2}{243 M_{\eta}^4 M_{\eta'}^8} - \frac{23\,552 c_{\theta}^8 L_8^r M_0^8 M_K^6 s_{\theta}^2 \Lambda_2}{243 M_{\eta}^2 M_{\eta'}^8} + \\
& \frac{2048 c_{\theta}^8 L_8^r M_0^8 M_K^4 s_{\theta}^2 \Lambda_2}{81 M_{\eta}^2 M_{\eta'}^8} + \frac{45\,184 c_{\theta}^8 L_8^r M_0^8 M_K^2 M_{\pi}^2 s_{\theta}^2 \Lambda_2}{243 M_{\eta}^2 M_{\eta'}^8} - \frac{1280 c_{\theta}^8 L_8^r M_0^8 M_K M_{\pi}^4 s_{\theta}^2 \Lambda_2}{9 M_{\eta}^2 M_{\eta'}^8} - \\
& \frac{26\,240 c_{\theta}^8 L_8^r M_0^8 M_K^2 M_{\pi}^4 s_{\theta}^2 \Lambda_2}{243 M_{\eta}^2 M_{\eta'}^8} + \frac{13\,568 c_{\theta}^8 L_8^r M_0^8 M_K M_{\pi}^6 s_{\theta}^2 \Lambda_2}{81 M_{\eta}^2 M_{\eta'}^8} + \frac{320 c_{\theta}^8 L_8^r M_0^8 M_{\pi}^8 s_{\theta}^2 \Lambda_2}{27 M_{\eta}^2 M_{\eta'}^8} - \\
& \frac{6592 c_{\theta}^8 L_8^r M_0^6 M_K^2 M_{\pi}^6 s_{\theta}^2 \Lambda_2}{81 M_{\eta}^2 M_{\eta'}^8} + \frac{64 c_{\theta}^8 L_8^r M_0^6 M_{\pi}^8 s_{\theta}^2 \Lambda_2}{27 M_{\eta}^2 M_{\eta'}^8} - \frac{204\,800 c_{\theta}^{10} L_8^r M_0^8 M_K^8 s_{\theta}^2 \Lambda_2}{729 M_{\eta}^6 M_{\eta'}^6} + \\
& \frac{114\,176 c_{\theta}^{10} L_8^r M_0^8 M_K^6 M_{\pi}^2 s_{\theta}^2 \Lambda_2}{243 M_{\eta}^6 M_{\eta'}^6} - \frac{6656 c_{\theta}^{10} L_8^r M_0^8 M_K^4 M_{\pi}^4 s_{\theta}^2 \Lambda_2}{27 M_{\eta}^6 M_{\eta'}^6} + \frac{30\,080 c_{\theta}^{10} L_8^r M_0^8 M_K^2 M_{\pi}^6 s_{\theta}^2 \Lambda_2}{729 M_{\eta}^6 M_{\eta'}^6} - \\
& \frac{2944 c_{\theta}^{10} L_8^r M_0^8 M_{\pi}^8 s_{\theta}^2 \Lambda_2}{243 M_{\eta}^6 M_{\eta'}^6} + \frac{6656 c_{\theta}^8 L_8^r M_0^8 M_K^6 s_{\theta}^2 \Lambda_2}{243 M_{\eta}^4 M_{\eta'}^6} - \frac{45\,056 c_{\theta}^8 L_8^r M_0^8 M_K^4 s_{\theta}^2 \Lambda_2}{243 M_{\eta}^4 M_{\eta'}^6} -
\end{aligned}$$

$$\begin{aligned}
& \frac{17\,152\,c_{\theta}^8 L_8^r M_0^8 M_K^4 M_{\pi}^2 s_{\theta}^2 \Lambda_2}{243\,M_{\eta}^4 M_{\eta'}^6} + \frac{3328\,c_{\theta}^8 L_8^r M_0^6 M_K^6 M_{\pi}^2 s_{\theta}^2 \Lambda_2}{9\,M_{\eta}^4 M_{\eta'}^6} + \frac{11\,264\,c_{\theta}^8 L_8^r M_0^8 M_K^2 M_{\pi}^4 s_{\theta}^2 \Lambda_2}{243\,M_{\eta}^4 M_{\eta'}^6} - \\
& \frac{256\,c_{\theta}^8 L_8^r M_0^6 M_K^4 M_{\pi}^4 s_{\theta}^2 \Lambda_2}{M_{\eta}^4 M_{\eta'}^6} + \frac{128\,c_{\theta}^8 L_8^r M_0^8 M_{\pi}^6 s_{\theta}^2 \Lambda_2}{81\,M_{\eta}^4 M_{\eta'}^6} + \frac{19\,520\,c_{\theta}^8 L_8^r M_0^6 M_K^2 M_{\pi}^6 s_{\theta}^2 \Lambda_2}{243\,M_{\eta}^4 M_{\eta'}^6} - \\
& \frac{320\,c_{\theta}^8 L_8^r M_0^6 M_{\pi}^8 s_{\theta}^2 \Lambda_2}{81\,M_{\eta}^4 M_{\eta'}^6} + \frac{20\,480\,c_{\theta}^6 L_8^r M_0^6 M_K^6 s_{\theta}^2 \Lambda_2}{243\,M_{\eta}^2 M_{\eta'}^6} - \frac{10\,240\,c_{\theta}^6 L_8^r M_0^6 M_K^4 M_{\pi}^2 s_{\theta}^2 \Lambda_2}{243\,M_{\eta}^2 M_{\eta'}^6} - \\
& \frac{6400\,c_{\theta}^6 L_8^r M_0^6 M_K^2 M_{\pi}^4 s_{\theta}^2 \Lambda_2}{243\,M_{\eta}^2 M_{\eta'}^6} + \frac{1792\,c_{\theta}^6 L_8^r M_0^6 M_{\pi}^6 s_{\theta}^2 \Lambda_2}{81\,M_{\eta}^2 M_{\eta'}^6} - \frac{16\,384\,c_{\theta}^{10} L_8^r M_0^8 M_K^8 s_{\theta}^2 \Lambda_2}{243\,M_{\eta}^8 M_{\eta'}^4} + \\
& \frac{14\,080\,c_{\theta}^{10} L_8^r M_0^8 M_K^6 M_{\pi}^2 s_{\theta}^2 \Lambda_2}{81\,M_{\eta}^8 M_{\eta'}^4} - \frac{13\,312\,c_{\theta}^{10} L_8^r M_0^8 M_K^4 M_{\pi}^4 s_{\theta}^2 \Lambda_2}{81\,M_{\eta}^8 M_{\eta'}^4} + \frac{16\,960\,c_{\theta}^{10} L_8^r M_0^8 M_K^2 M_{\pi}^6 s_{\theta}^2 \Lambda_2}{243\,M_{\eta}^8 M_{\eta'}^4} - \\
& \frac{320\,c_{\theta}^{10} L_8^r M_0^8 M_{\pi}^8 s_{\theta}^2 \Lambda_2}{27\,M_{\eta}^8 M_{\eta'}^4} + \frac{1024\,c_{\theta}^8 L_8^r M_0^8 M_K^6 s_{\theta}^2 \Lambda_2}{27\,M_{\eta}^6 M_{\eta'}^4} + \frac{8192\,c_{\theta}^8 L_8^r M_0^6 M_K^8 s_{\theta}^2 \Lambda_2}{81\,M_{\eta}^6 M_{\eta'}^4} - \\
& \frac{1408\,c_{\theta}^8 L_8^r M_0^8 M_K^4 M_{\pi}^2 s_{\theta}^2 \Lambda_2}{27\,M_{\eta}^6 M_{\eta'}^4} - \frac{10\,496\,c_{\theta}^8 L_8^r M_0^6 M_K^6 M_{\pi}^2 s_{\theta}^2 \Lambda_2}{81\,M_{\eta}^6 M_{\eta'}^4} + \frac{640\,c_{\theta}^8 L_8^r M_0^8 M_K^2 M_{\pi}^4 s_{\theta}^2 \Lambda_2}{27\,M_{\eta}^6 M_{\eta'}^4} + \\
& \frac{512\,c_{\theta}^8 L_8^r M_0^6 M_K^4 M_{\pi}^4 s_{\theta}^2 \Lambda_2}{27\,M_{\eta}^6 M_{\eta'}^4} - \frac{64\,c_{\theta}^8 L_8^r M_0^8 M_{\pi}^6 s_{\theta}^2 \Lambda_2}{27\,M_{\eta}^6 M_{\eta'}^4} + \frac{1984\,c_{\theta}^8 L_8^r M_0^6 M_K^2 M_{\pi}^6 s_{\theta}^2 \Lambda_2}{81\,M_{\eta}^6 M_{\eta'}^4} - \\
& \frac{64\,c_{\theta}^8 L_8^r M_0^6 M_{\pi}^8 s_{\theta}^2 \Lambda_2}{81\,M_{\eta}^6 M_{\eta'}^4} - \frac{2048\,c_{\theta}^6 L_8^r M_0^6 M_K^4 M_{\pi}^2 s_{\theta}^2 \Lambda_2}{27\,M_{\eta}^4 M_{\eta'}^4} + \frac{2048\,c_{\theta}^6 L_8^r M_0^6 M_K^2 M_{\pi}^4 s_{\theta}^2 \Lambda_2}{27\,M_{\eta}^4 M_{\eta'}^4} - \\
& \frac{256\,c_{\theta}^6 L_8^r M_0^6 M_{\pi}^6 s_{\theta}^2 \Lambda_2}{9\,M_{\eta}^4 M_{\eta'}^4} + \frac{16\,384\,c_{\theta}^8 L_8^r M_0^6 M_K^8 s_{\theta}^2 \Lambda_2}{243\,M_{\eta}^8 M_{\eta'}^2} - \frac{14\,080\,c_{\theta}^8 L_8^r M_0^6 M_K^6 M_{\pi}^2 s_{\theta}^2 \Lambda_2}{81\,M_{\eta}^8 M_{\eta'}^2} + \\
& \frac{13\,312\,c_{\theta}^8 L_8^r M_0^6 M_K^4 M_{\pi}^4 s_{\theta}^2 \Lambda_2}{81\,M_{\eta}^8 M_{\eta'}^2} - \frac{16\,960\,c_{\theta}^8 L_8^r M_0^6 M_K^2 M_{\pi}^6 s_{\theta}^2 \Lambda_2}{243\,M_{\eta}^8 M_{\eta'}^2} + \frac{320\,c_{\theta}^8 L_8^r M_0^6 M_{\pi}^8 s_{\theta}^2 \Lambda_2}{27\,M_{\eta}^8 M_{\eta'}^2} - \\
& \frac{4096\,c_{\theta}^6 L_8^r M_0^6 M_K^6 s_{\theta}^2 \Lambda_2}{81\,M_{\eta}^6 M_{\eta'}^2} + \frac{8192\,c_{\theta}^6 L_8^r M_0^6 M_K^4 M_{\pi}^2 s_{\theta}^2 \Lambda_2}{81\,M_{\eta}^6 M_{\eta'}^2} - \frac{4864\,c_{\theta}^6 L_8^r M_0^6 M_K^2 M_{\pi}^4 s_{\theta}^2 \Lambda_2}{81\,M_{\eta}^6 M_{\eta'}^2} + \\
& \frac{256\,c_{\theta}^6 L_8^r M_0^6 M_{\pi}^6 s_{\theta}^2 \Lambda_2}{27\,M_{\eta}^6 M_{\eta'}^2} + \frac{16\,384\,\sqrt{2}\,c_{\theta}^7 L_8^r M_0^6 M_K^8 s_{\theta}^3 \Lambda_2}{729\,M_{\eta}^{10}} - \frac{13\,312\,\sqrt{2}\,c_{\theta}^7 L_8^r M_0^6 M_K^6 M_{\pi}^2 s_{\theta}^3 \Lambda_2}{243\,M_{\eta}^{10}} + \\
& \frac{4096\,\sqrt{2}\,c_{\theta}^7 L_8^r M_0^6 M_K^4 M_{\pi}^4 s_{\theta}^3 \Lambda_2}{81\,M_{\eta}^{10}} - \frac{16\,000\,\sqrt{2}\,c_{\theta}^7 L_8^r M_0^6 M_K^2 M_{\pi}^6 s_{\theta}^3 \Lambda_2}{729\,M_{\eta}^{10}} + \frac{896\,\sqrt{2}\,c_{\theta}^7 L_8^r M_0^6 M_{\pi}^8 s_{\theta}^3 \Lambda_2}{243\,M_{\eta}^{10}} - \\
& \frac{4096\,\sqrt{2}\,c_{\theta}^5 L_8^r M_0^6 M_K^6 s_{\theta}^3 \Lambda_2}{243\,M_{\eta}^8} + \frac{8192\,\sqrt{2}\,c_{\theta}^5 L_8^r M_0^6 M_K^4 M_{\pi}^2 s_{\theta}^3 \Lambda_2}{243\,M_{\eta}^8} - \frac{5248\,\sqrt{2}\,c_{\theta}^5 L_8^r M_0^6 M_K^2 M_{\pi}^4 s_{\theta}^3 \Lambda_2}{243\,M_{\eta}^8} + \\
& \frac{128\,\sqrt{2}\,c_{\theta}^5 L_8^r M_0^6 M_{\pi}^6 s_{\theta}^3 \Lambda_2}{27\,M_{\eta}^8} + \frac{358\,400\,\sqrt{2}\,c_{\theta}^9 L_8^r M_0^8 M_K^8 s_{\theta}^3 \Lambda_2}{729\,M_{\eta}^{12}} - \frac{66\,560\,\sqrt{2}\,c_{\theta}^9 L_8^r M_0^8 M_K^6 M_{\pi}^2 s_{\theta}^3 \Lambda_2}{81\,M_{\eta}^{12}} + \\
& \frac{14\,080\,\sqrt{2}\,c_{\theta}^9 L_8^r M_0^8 M_K^4 M_{\pi}^4 s_{\theta}^3 \Lambda_2}{27\,M_{\eta}^{12}} - \frac{114\,560\,\sqrt{2}\,c_{\theta}^9 L_8^r M_0^8 M_K^2 M_{\pi}^6 s_{\theta}^3 \Lambda_2}{729\,M_{\eta}^{12}} -
\end{aligned}$$



$$\begin{aligned}
& \frac{2560 \sqrt{2} c_{\theta}^9 L_8^r M_0^8 M_{\pi}^8 s_{\theta}^3 \Lambda_2}{243 M_{\eta'}^{12}} - \frac{20480 \sqrt{2} c_{\theta}^7 L_8^r M_0^8 M_K^6 s_{\theta}^3 \Lambda_2}{243 M_{\eta'}^{10}} - \frac{143360 \sqrt{2} c_{\theta}^7 L_8^r M_0^6 M_K^8 s_{\theta}^3 \Lambda_2}{729 M_{\eta'}^{10}} + \\
& \frac{30976 \sqrt{2} c_{\theta}^7 L_8^r M_0^8 M_K^4 M_{\pi}^2 s_{\theta}^3 \Lambda_2}{243 M_{\eta'}^{10}} + \frac{26624 \sqrt{2} c_{\theta}^7 L_8^r M_0^6 M_K^6 M_{\pi}^2 s_{\theta}^3 \Lambda_2}{81 M_{\eta'}^{10}} - \\
& \frac{14336 \sqrt{2} c_{\theta}^7 L_8^r M_0^8 M_K^2 M_{\pi}^4 s_{\theta}^3 \Lambda_2}{243 M_{\eta'}^{10}} - \frac{5632 \sqrt{2} c_{\theta}^7 L_8^r M_0^6 M_K^4 M_{\pi}^4 s_{\theta}^3 \Lambda_2}{27 M_{\eta'}^{10}} + \frac{1088 \sqrt{2} c_{\theta}^7 L_8^r M_0^8 M_{\pi}^6 s_{\theta}^3 \Lambda_2}{81 M_{\eta'}^{10}} + \\
& \frac{45824 \sqrt{2} c_{\theta}^7 L_8^r M_0^6 M_K^2 M_{\pi}^6 s_{\theta}^3 \Lambda_2}{729 M_{\eta'}^{10}} + \frac{1024 \sqrt{2} c_{\theta}^7 L_8^r M_0^8 M_{\pi}^8 s_{\theta}^3 \Lambda_2}{243 M_{\eta'}^{10}} - \frac{465920 \sqrt{2} c_{\theta}^9 L_8^r M_0^8 M_K^8 s_{\theta}^3 \Lambda_2}{729 M_{\eta}^2 M_{\eta'}^{10}} + \\
& \frac{240640 \sqrt{2} c_{\theta}^9 L_8^r M_0^8 M_K^6 M_{\pi}^2 s_{\theta}^3 \Lambda_2}{243 M_{\eta}^2 M_{\eta'}^{10}} - \frac{140800 \sqrt{2} c_{\theta}^9 L_8^r M_0^8 M_K^4 M_{\pi}^4 s_{\theta}^3 \Lambda_2}{243 M_{\eta}^2 M_{\eta'}^{10}} + \\
& \frac{142976 \sqrt{2} c_{\theta}^9 L_8^r M_0^8 M_K^2 M_{\pi}^6 s_{\theta}^3 \Lambda_2}{729 M_{\eta}^2 M_{\eta'}^{10}} - \frac{6016 \sqrt{2} c_{\theta}^9 L_8^r M_0^8 M_{\pi}^8 s_{\theta}^3 \Lambda_2}{243 M_{\eta}^2 M_{\eta'}^{10}} + \frac{20480 \sqrt{2} c_{\theta}^5 L_8^r M_0^6 M_K^6 s_{\theta}^3 \Lambda_2}{243 M_{\eta}^8} - \\
& \frac{28672 \sqrt{2} c_{\theta}^5 L_8^r M_0^6 M_K^4 M_{\pi}^2 s_{\theta}^3 \Lambda_2}{243 M_{\eta}^8} + \frac{14336 \sqrt{2} c_{\theta}^5 L_8^r M_0^6 M_K^2 M_{\pi}^4 s_{\theta}^3 \Lambda_2}{243 M_{\eta}^8} - \\
& \frac{1280 \sqrt{2} c_{\theta}^5 L_8^r M_0^6 M_{\pi}^6 s_{\theta}^3 \Lambda_2}{81 M_{\eta}^8} + \frac{222208 \sqrt{2} c_{\theta}^9 L_8^r M_0^8 M_K^8 s_{\theta}^3 \Lambda_2}{729 M_{\eta}^4 M_{\eta'}^8} - \frac{60416 \sqrt{2} c_{\theta}^9 L_8^r M_0^8 M_K^6 M_{\pi}^2 s_{\theta}^3 \Lambda_2}{243 M_{\eta}^4 M_{\eta'}^8} + \\
& \frac{4352 \sqrt{2} c_{\theta}^9 L_8^r M_0^8 M_K^4 M_{\pi}^4 s_{\theta}^3 \Lambda_2}{243 M_{\eta}^4 M_{\eta'}^8} - \frac{47488 \sqrt{2} c_{\theta}^9 L_8^r M_0^8 M_K^2 M_{\pi}^6 s_{\theta}^3 \Lambda_2}{729 M_{\eta}^4 M_{\eta'}^8} + \frac{4736 \sqrt{2} c_{\theta}^9 L_8^r M_0^8 M_{\pi}^8 s_{\theta}^3 \Lambda_2}{243 M_{\eta}^4 M_{\eta'}^8} + \\
& \frac{28672 \sqrt{2} c_{\theta}^7 L_8^r M_0^8 M_K^6 s_{\theta}^3 \Lambda_2}{243 M_{\eta}^2 M_{\eta'}^8} + \frac{126976 \sqrt{2} c_{\theta}^7 L_8^r M_0^6 M_K^8 s_{\theta}^3 \Lambda_2}{729 M_{\eta}^2 M_{\eta'}^8} - \frac{45440 \sqrt{2} c_{\theta}^7 L_8^r M_0^8 M_K^4 M_{\pi}^2 s_{\theta}^3 \Lambda_2}{243 M_{\eta}^2 M_{\eta'}^8} - \\
& \frac{46208 \sqrt{2} c_{\theta}^7 L_8^r M_0^6 M_K^6 M_{\pi}^2 s_{\theta}^3 \Lambda_2}{243 M_{\eta}^2 M_{\eta'}^8} + \frac{16768 \sqrt{2} c_{\theta}^7 L_8^r M_0^8 M_K^2 M_{\pi}^4 s_{\theta}^3 \Lambda_2}{243 M_{\eta}^2 M_{\eta'}^8} + \\
& \frac{4096 \sqrt{2} c_{\theta}^7 L_8^r M_0^6 M_K^4 M_{\pi}^4 s_{\theta}^3 \Lambda_2}{81 M_{\eta}^2 M_{\eta'}^8} + \frac{16 \sqrt{2} c_{\theta}^7 L_8^r M_0^8 M_{\pi}^6 s_{\theta}^3 \Lambda_2}{3 M_{\eta}^2 M_{\eta'}^8} - \frac{9952 \sqrt{2} c_{\theta}^7 L_8^r M_0^6 M_K^2 M_{\pi}^6 s_{\theta}^3 \Lambda_2}{729 M_{\eta}^2 M_{\eta'}^8} + \\
& \frac{32 \sqrt{2} c_{\theta}^7 L_8^r M_0^6 M_{\pi}^8 s_{\theta}^3 \Lambda_2}{81 M_{\eta}^2 M_{\eta'}^8} + \frac{163840 \sqrt{2} c_{\theta}^9 L_8^r M_0^8 M_K^8 s_{\theta}^3 \Lambda_2}{729 M_{\eta}^6 M_{\eta'}^6} - \frac{59392 \sqrt{2} c_{\theta}^9 L_8^r M_0^8 M_K^6 M_{\pi}^2 s_{\theta}^3 \Lambda_2}{81 M_{\eta}^6 M_{\eta'}^6} + \\
& \frac{52736 \sqrt{2} c_{\theta}^9 L_8^r M_0^8 M_K^4 M_{\pi}^4 s_{\theta}^3 \Lambda_2}{81 M_{\eta}^6 M_{\eta'}^6} - \frac{103552 \sqrt{2} c_{\theta}^9 L_8^r M_0^8 M_K^2 M_{\pi}^6 s_{\theta}^3 \Lambda_2}{729 M_{\eta}^6 M_{\eta'}^6} + \\
& \frac{4480 \sqrt{2} c_{\theta}^9 L_8^r M_0^8 M_{\pi}^8 s_{\theta}^3 \Lambda_2}{243 M_{\eta}^6 M_{\eta'}^6} - \frac{31744 \sqrt{2} c_{\theta}^7 L_8^r M_0^8 M_K^6 s_{\theta}^3 \Lambda_2}{243 M_{\eta}^4 M_{\eta'}^6} + \frac{4096 \sqrt{2} c_{\theta}^7 L_8^r M_0^6 M_K^8 s_{\theta}^3 \Lambda_2}{729 M_{\eta}^4 M_{\eta'}^6} + \\
& \frac{49280 \sqrt{2} c_{\theta}^7 L_8^r M_0^8 M_K^4 M_{\pi}^2 s_{\theta}^3 \Lambda_2}{243 M_{\eta}^4 M_{\eta'}^6} - \frac{45184 \sqrt{2} c_{\theta}^7 L_8^r M_0^6 M_K^6 M_{\pi}^2 s_{\theta}^3 \Lambda_2}{243 M_{\eta}^4 M_{\eta'}^6} -
\end{aligned}$$

$$\begin{aligned}
& \frac{16\,384\sqrt{2}\,c_{\theta}^7L_8^rM_0^8M_K^2M_{\pi}^4s_{\theta}^3\Lambda_2}{243M_{\eta}^4M_{\eta'}^6} + \frac{5888\sqrt{2}\,c_{\theta}^7L_8^rM_0^6M_K^4M_{\pi}^4s_{\theta}^3\Lambda_2}{27M_{\eta}^4M_{\eta'}^6} - \frac{176\sqrt{2}\,c_{\theta}^7L_8^rM_0^8M_{\pi}^6s_{\theta}^3\Lambda_2}{27M_{\eta}^4M_{\eta'}^6} - \\
& \frac{32\,224\sqrt{2}\,c_{\theta}^7L_8^rM_0^6M_K^2M_{\pi}^6s_{\theta}^3\Lambda_2}{729M_{\eta}^4M_{\eta'}^6} - \frac{160\sqrt{2}\,c_{\theta}^7L_8^rM_0^6M_{\pi}^8s_{\theta}^3\Lambda_2}{243M_{\eta}^4M_{\eta'}^6} - \frac{29\,696\sqrt{2}\,c_{\theta}^5L_8^rM_0^6M_K^6s_{\theta}^3\Lambda_2}{243M_{\eta}^2M_{\eta'}^6} + \\
& \frac{40\,960\sqrt{2}\,c_{\theta}^5L_8^rM_0^6M_K^4M_{\pi}^2s_{\theta}^3\Lambda_2}{243M_{\eta}^2M_{\eta'}^6} - \frac{21\,632\sqrt{2}\,c_{\theta}^5L_8^rM_0^6M_K^2M_{\pi}^4s_{\theta}^3\Lambda_2}{243M_{\eta}^2M_{\eta'}^6} + \\
& \frac{128\sqrt{2}\,c_{\theta}^5L_8^rM_0^6M_{\pi}^6s_{\theta}^3\Lambda_2}{9M_{\eta}^2M_{\eta'}^6} - \frac{262\,144\sqrt{2}\,c_{\theta}^9L_8^rM_0^8M_K^8s_{\theta}^3\Lambda_2}{729M_{\eta}^8M_{\eta'}^4} + \frac{20\,480\sqrt{2}\,c_{\theta}^9L_8^rM_0^8M_K^6M_{\pi}^2s_{\theta}^3\Lambda_2}{27M_{\eta}^8M_{\eta'}^4} - \\
& \frac{136\,192\sqrt{2}\,c_{\theta}^9L_8^rM_0^8M_K^4M_{\pi}^4s_{\theta}^3\Lambda_2}{243M_{\eta}^8M_{\eta'}^4} + \frac{106\,624\sqrt{2}\,c_{\theta}^9L_8^rM_0^8M_K^2M_{\pi}^6s_{\theta}^3\Lambda_2}{729M_{\eta}^8M_{\eta'}^4} + \\
& \frac{256\sqrt{2}\,c_{\theta}^9L_8^rM_0^8M_{\pi}^8s_{\theta}^3\Lambda_2}{243M_{\eta}^8M_{\eta'}^4} + \frac{20\,480\sqrt{2}\,c_{\theta}^7L_8^rM_0^8M_K^6s_{\theta}^3\Lambda_2}{243M_{\eta}^6M_{\eta'}^4} - \frac{118\,784\sqrt{2}\,c_{\theta}^7L_8^rM_0^6M_K^8s_{\theta}^3\Lambda_2}{729M_{\eta}^6M_{\eta'}^4} - \\
& \frac{29\,824\sqrt{2}\,c_{\theta}^7L_8^rM_0^8M_K^4M_{\pi}^2s_{\theta}^3\Lambda_2}{243M_{\eta}^6M_{\eta'}^4} + \frac{34\,688\sqrt{2}\,c_{\theta}^7L_8^rM_0^6M_K^6M_{\pi}^2s_{\theta}^3\Lambda_2}{81M_{\eta}^6M_{\eta'}^4} + \\
& \frac{10\,880\sqrt{2}\,c_{\theta}^7L_8^rM_0^8M_K^2M_{\pi}^4s_{\theta}^3\Lambda_2}{243M_{\eta}^6M_{\eta'}^4} - \frac{1024\sqrt{2}\,c_{\theta}^7L_8^rM_0^6M_K^4M_{\pi}^4s_{\theta}^3\Lambda_2}{3M_{\eta}^6M_{\eta'}^4} - \\
& \frac{752\sqrt{2}\,c_{\theta}^7L_8^rM_0^8M_{\pi}^6s_{\theta}^3\Lambda_2}{81M_{\eta}^6M_{\eta'}^4} + \frac{48\,608\sqrt{2}\,c_{\theta}^7L_8^rM_0^6M_K^2M_{\pi}^6s_{\theta}^3\Lambda_2}{729M_{\eta}^6M_{\eta'}^4} - \frac{608\sqrt{2}\,c_{\theta}^7L_8^rM_0^6M_{\pi}^8s_{\theta}^3\Lambda_2}{243M_{\eta}^6M_{\eta'}^4} + \\
& \frac{1024\sqrt{2}\,c_{\theta}^5L_8^rM_0^6M_K^6s_{\theta}^3\Lambda_2}{9M_{\eta}^4M_{\eta'}^4} - \frac{4096\sqrt{2}\,c_{\theta}^5L_8^rM_0^6M_K^4M_{\pi}^2s_{\theta}^3\Lambda_2}{27M_{\eta}^4M_{\eta'}^4} + \frac{2176\sqrt{2}\,c_{\theta}^5L_8^rM_0^6M_K^2M_{\pi}^4s_{\theta}^3\Lambda_2}{27M_{\eta}^4M_{\eta'}^4} - \\
& \frac{128\sqrt{2}\,c_{\theta}^5L_8^rM_0^6M_{\pi}^6s_{\theta}^3\Lambda_2}{9M_{\eta}^4M_{\eta'}^4} - \frac{16\,384\sqrt{2}\,c_{\theta}^9L_8^rM_0^8M_K^8s_{\theta}^3\Lambda_2}{729M_{\eta}^{10}M_{\eta'}^2} + \frac{13\,312\sqrt{2}\,c_{\theta}^9L_8^rM_0^8M_K^6M_{\pi}^2s_{\theta}^3\Lambda_2}{243M_{\eta}^{10}M_{\eta'}^2} - \\
& \frac{4096\sqrt{2}\,c_{\theta}^9L_8^rM_0^8M_K^4M_{\pi}^4s_{\theta}^3\Lambda_2}{81M_{\eta}^{10}M_{\eta'}^2} + \frac{16\,000\sqrt{2}\,c_{\theta}^9L_8^rM_0^8M_K^2M_{\pi}^6s_{\theta}^3\Lambda_2}{729M_{\eta}^{10}M_{\eta'}^2} - \\
& \frac{896\sqrt{2}\,c_{\theta}^9L_8^rM_0^8M_{\pi}^8s_{\theta}^3\Lambda_2}{243M_{\eta}^{10}M_{\eta'}^2} + \frac{1024\sqrt{2}\,c_{\theta}^7L_8^rM_0^8M_K^6s_{\theta}^3\Lambda_2}{81M_{\eta}^8M_{\eta'}^2} + \frac{114\,688\sqrt{2}\,c_{\theta}^7L_8^rM_0^6M_K^8s_{\theta}^3\Lambda_2}{729M_{\eta}^8M_{\eta'}^2} - \\
& \frac{1664\sqrt{2}\,c_{\theta}^7L_8^rM_0^8M_K^4M_{\pi}^2s_{\theta}^3\Lambda_2}{81M_{\eta}^8M_{\eta'}^2} - \frac{79\,232\sqrt{2}\,c_{\theta}^7L_8^rM_0^6M_K^6M_{\pi}^2s_{\theta}^3\Lambda_2}{243M_{\eta}^8M_{\eta'}^2} + \\
& \frac{1024\sqrt{2}\,c_{\theta}^7L_8^rM_0^8M_K^2M_{\pi}^4s_{\theta}^3\Lambda_2}{81M_{\eta}^8M_{\eta'}^2} + \frac{18\,688\sqrt{2}\,c_{\theta}^7L_8^rM_0^6M_K^4M_{\pi}^4s_{\theta}^3\Lambda_2}{81M_{\eta}^8M_{\eta'}^2} - \frac{80\sqrt{2}\,c_{\theta}^7L_8^rM_0^8M_{\pi}^6s_{\theta}^3\Lambda_2}{27M_{\eta}^8M_{\eta'}^2} - \\
& \frac{36\,256\sqrt{2}\,c_{\theta}^7L_8^rM_0^6M_K^2M_{\pi}^6s_{\theta}^3\Lambda_2}{729M_{\eta}^8M_{\eta'}^2} - \frac{416\sqrt{2}\,c_{\theta}^7L_8^rM_0^6M_{\pi}^8s_{\theta}^3\Lambda_2}{81M_{\eta}^8M_{\eta'}^2} - \frac{14\,336\sqrt{2}\,c_{\theta}^5L_8^rM_0^6M_K^6s_{\theta}^3\Lambda_2}{243M_{\eta}^6M_{\eta'}^2} +
\end{aligned}$$

$$\begin{aligned}
& \frac{16\,384\sqrt{2}\,c_{\theta}^5L_8^rM_0^6M_K^4M_{\pi}^2s_{\theta}^3\Lambda_2}{243M_{\eta}^6M_{\eta'}^2} - \frac{7040\sqrt{2}\,c_{\theta}^5L_8^rM_0^6M_K^2M_{\pi}^4s_{\theta}^3\Lambda_2}{243M_{\eta}^6M_{\eta'}^2} + \frac{896\sqrt{2}\,c_{\theta}^5L_8^rM_0^6M_{\pi}^6s_{\theta}^3\Lambda_2}{81M_{\eta}^6M_{\eta'}^2} + \\
& \frac{114\,688\,c_{\theta}^6L_8^rM_0^6M_K^8s_{\theta}^4\Lambda_2}{729M_{\eta}^{10}} - \frac{29\,696\,c_{\theta}^6L_8^rM_0^6M_K^6M_{\pi}^2s_{\theta}^4\Lambda_2}{81M_{\eta}^{10}} + \frac{8704\,c_{\theta}^6L_8^rM_0^6M_K^4M_{\pi}^4s_{\theta}^4\Lambda_2}{27M_{\eta}^{10}} - \\
& \frac{91\,264\,c_{\theta}^6L_8^rM_0^6M_K^2M_{\pi}^6s_{\theta}^4\Lambda_2}{729M_{\eta}^{10}} + \frac{4672\,c_{\theta}^6L_8^rM_0^6M_{\pi}^8s_{\theta}^4\Lambda_2}{243M_{\eta}^{10}} - \frac{20\,480\,c_{\theta}^4L_8^rM_0^6M_K^6s_{\theta}^4\Lambda_2}{243M_{\eta}^8} + \\
& \frac{34\,816\,c_{\theta}^4L_8^rM_0^6M_K^4M_{\pi}^2s_{\theta}^4\Lambda_2}{243M_{\eta}^8} - \frac{18\,560\,c_{\theta}^4L_8^rM_0^6M_K^2M_{\pi}^4s_{\theta}^4\Lambda_2}{243M_{\eta}^8} + \frac{832\,c_{\theta}^4L_8^rM_0^6M_{\pi}^6s_{\theta}^4\Lambda_2}{81M_{\eta}^8} - \\
& \frac{716\,800\,c_{\theta}^8L_8^rM_0^8M_K^8s_{\theta}^4\Lambda_2}{729M_{\eta}^{12}} + \frac{436\,480\,c_{\theta}^8L_8^rM_0^8M_K^6M_{\pi}^2s_{\theta}^4\Lambda_2}{243M_{\eta}^{12}} - \frac{96\,640\,c_{\theta}^8L_8^rM_0^8M_K^4M_{\pi}^4s_{\theta}^4\Lambda_2}{81M_{\eta}^{12}} + \\
& \frac{272\,320\,c_{\theta}^8L_8^rM_0^8M_K^2M_{\pi}^6s_{\theta}^4\Lambda_2}{729M_{\eta'}^{12}} - \frac{20\,000\,c_{\theta}^8L_8^rM_0^8M_{\pi}^8s_{\theta}^4\Lambda_2}{243M_{\eta'}^{12}} + \frac{20\,480\,c_{\theta}^6L_8^rM_0^8M_K^6s_{\theta}^4\Lambda_2}{243M_{\eta'}^{10}} + \\
& \frac{286\,720\,c_{\theta}^6L_8^rM_0^6M_K^8s_{\theta}^4\Lambda_2}{729M_{\eta'}^{10}} - \frac{28\,672\,c_{\theta}^6L_8^rM_0^8M_K^4M_{\pi}^2s_{\theta}^4\Lambda_2}{243M_{\eta'}^{10}} - \frac{174\,592\,c_{\theta}^6L_8^rM_0^6M_K^6M_{\pi}^2s_{\theta}^4\Lambda_2}{243M_{\eta'}^{10}} + \\
& \frac{12\,800\,c_{\theta}^6L_8^rM_0^8M_K^2M_{\pi}^4s_{\theta}^4\Lambda_2}{243M_{\eta'}^{10}} + \frac{38\,656\,c_{\theta}^6L_8^rM_0^6M_K^4M_{\pi}^4s_{\theta}^4\Lambda_2}{81M_{\eta'}^{10}} - \frac{128\,c_{\theta}^6L_8^rM_0^8M_{\pi}^6s_{\theta}^4\Lambda_2}{27M_{\eta'}^{10}} - \\
& \frac{108\,928\,c_{\theta}^6L_8^rM_0^6M_K^2M_{\pi}^6s_{\theta}^4\Lambda_2}{729M_{\eta'}^{10}} + \frac{8000\,c_{\theta}^6L_8^rM_0^6M_{\pi}^8s_{\theta}^4\Lambda_2}{243M_{\eta'}^{10}} + \frac{1\,132\,544\,c_{\theta}^8L_8^rM_0^8M_K^8s_{\theta}^4\Lambda_2}{729M_{\eta'}^2M_{\eta'}^{10}} - \\
& \frac{236\,032\,c_{\theta}^8L_8^rM_0^8M_K^6M_{\pi}^2s_{\theta}^4\Lambda_2}{81M_{\eta'}^2M_{\eta'}^{10}} + \frac{461\,312\,c_{\theta}^8L_8^rM_0^8M_K^4M_{\pi}^4s_{\theta}^4\Lambda_2}{243M_{\eta'}^2M_{\eta'}^{10}} - \frac{471\,296\,c_{\theta}^8L_8^rM_0^8M_K^2M_{\pi}^6s_{\theta}^4\Lambda_2}{729M_{\eta'}^2M_{\eta'}^{10}} + \\
& \frac{14\,848\,c_{\theta}^8L_8^rM_0^8M_{\pi}^8s_{\theta}^4\Lambda_2}{243M_{\eta'}^2M_{\eta'}^{10}} - \frac{20\,480\,c_{\theta}^4L_8^rM_0^6M_K^6s_{\theta}^4\Lambda_2}{243M_{\eta'}^8} + \frac{34\,816\,c_{\theta}^4L_8^rM_0^6M_K^4M_{\pi}^2s_{\theta}^4\Lambda_2}{243M_{\eta'}^8} - \\
& \frac{18\,560\,c_{\theta}^4L_8^rM_0^6M_K^2M_{\pi}^4s_{\theta}^4\Lambda_2}{243M_{\eta'}^8} + \frac{832\,c_{\theta}^4L_8^rM_0^6M_{\pi}^6s_{\theta}^4\Lambda_2}{81M_{\eta'}^8} - \frac{1\,297\,408\,c_{\theta}^8L_8^rM_0^8M_K^8s_{\theta}^4\Lambda_2}{729M_{\eta'}^4M_{\eta'}^8} + \\
& \frac{759\,296\,c_{\theta}^8L_8^rM_0^8M_K^6M_{\pi}^2s_{\theta}^4\Lambda_2}{243M_{\eta'}^4M_{\eta'}^8} - \frac{434\,432\,c_{\theta}^8L_8^rM_0^8M_K^4M_{\pi}^4s_{\theta}^4\Lambda_2}{243M_{\eta'}^4M_{\eta'}^8} + \frac{394\,624\,c_{\theta}^8L_8^rM_0^8M_K^2M_{\pi}^6s_{\theta}^4\Lambda_2}{729M_{\eta'}^4M_{\eta'}^8} - \\
& \frac{7808\,c_{\theta}^8L_8^rM_0^8M_{\pi}^8s_{\theta}^4\Lambda_2}{243M_{\eta'}^4M_{\eta'}^8} - \frac{512\,c_{\theta}^6L_8^rM_0^8M_K^6s_{\theta}^4\Lambda_2}{243M_{\eta'}^2M_{\eta'}^8} - \frac{389\,120\,c_{\theta}^6L_8^rM_0^6M_K^8s_{\theta}^4\Lambda_2}{729M_{\eta'}^2M_{\eta'}^8} - \\
& \frac{13\,568\,c_{\theta}^6L_8^rM_0^8M_K^4M_{\pi}^2s_{\theta}^4\Lambda_2}{243M_{\eta'}^2M_{\eta'}^8} + \frac{213\,760\,c_{\theta}^6L_8^rM_0^6M_K^6M_{\pi}^2s_{\theta}^4\Lambda_2}{243M_{\eta'}^2M_{\eta'}^8} + \frac{16\,384\,c_{\theta}^6L_8^rM_0^8M_K^2M_{\pi}^4s_{\theta}^4\Lambda_2}{243M_{\eta'}^2M_{\eta'}^8} - \\
& \frac{38\,144\,c_{\theta}^6L_8^rM_0^6M_K^4M_{\pi}^4s_{\theta}^4\Lambda_2}{81M_{\eta'}^2M_{\eta'}^8} + \frac{128\,c_{\theta}^6L_8^rM_0^8M_{\pi}^6s_{\theta}^4\Lambda_2}{27M_{\eta'}^2M_{\eta'}^8} + \frac{94\,016\,c_{\theta}^6L_8^rM_0^6M_K^2M_{\pi}^6s_{\theta}^4\Lambda_2}{729M_{\eta'}^2M_{\eta'}^8} - \\
& \frac{896\,c_{\theta}^6L_8^rM_0^6M_{\pi}^8s_{\theta}^4\Lambda_2}{81M_{\eta'}^2M_{\eta'}^8} + \frac{1\,101\,824\,c_{\theta}^8L_8^rM_0^8M_K^8s_{\theta}^4\Lambda_2}{729M_{\eta'}^6M_{\eta'}^6} - \frac{548\,864\,c_{\theta}^8L_8^rM_0^8M_K^6M_{\pi}^2s_{\theta}^4\Lambda_2}{243M_{\eta'}^6M_{\eta'}^6} +
\end{aligned}$$

$$\begin{aligned}
& \frac{68\,096\,c_{\theta}^8\,L_8^r\,M_0^8\,M_K^4\,M_{\pi}^4\,s_{\theta}^4\,\Lambda_2}{81\,M_{\eta}^6\,M_{\eta'}^6} - \frac{64\,256\,c_{\theta}^8\,L_8^r\,M_0^8\,M_K^2\,M_{\pi}^6\,s_{\theta}^4\,\Lambda_2}{729\,M_{\eta}^6\,M_{\eta'}^6} - \frac{2432\,c_{\theta}^8\,L_8^r\,M_0^8\,M_{\pi}^8\,s_{\theta}^4\,\Lambda_2}{243\,M_{\eta}^6\,M_{\eta'}^6} - \\
& \frac{8192\,c_{\theta}^6\,L_8^r\,M_0^8\,M_K^6\,s_{\theta}^4\,\Lambda_2}{243\,M_{\eta}^4\,M_{\eta'}^6} + \frac{372\,736\,c_{\theta}^6\,L_8^r\,M_0^8\,M_K^6\,s_{\theta}^4\,\Lambda_2}{729\,M_{\eta}^4\,M_{\eta'}^6} + \frac{42\,112\,c_{\theta}^6\,L_8^r\,M_0^8\,M_K^4\,M_{\pi}^2\,s_{\theta}^4\,\Lambda_2}{243\,M_{\eta}^4\,M_{\eta'}^6} - \\
& \frac{59\,648\,c_{\theta}^6\,L_8^r\,M_0^6\,M_K^6\,M_{\pi}^2\,s_{\theta}^4\,\Lambda_2}{81\,M_{\eta}^4\,M_{\eta'}^6} - \frac{37\,760\,c_{\theta}^6\,L_8^r\,M_0^6\,M_K^2\,M_{\pi}^4\,s_{\theta}^4\,\Lambda_2}{243\,M_{\eta}^4\,M_{\eta'}^6} + \frac{256\,c_{\theta}^6\,L_8^r\,M_0^6\,M_K^4\,M_{\pi}^4\,s_{\theta}^4\,\Lambda_2}{M_{\eta}^4\,M_{\eta'}^6} + \\
& \frac{1088\,c_{\theta}^6\,L_8^r\,M_0^8\,M_{\pi}^6\,s_{\theta}^4\,\Lambda_2}{81\,M_{\eta}^4\,M_{\eta'}^6} - \frac{29\,632\,c_{\theta}^6\,L_8^r\,M_0^6\,M_K^2\,M_{\pi}^6\,s_{\theta}^4\,\Lambda_2}{729\,M_{\eta}^4\,M_{\eta'}^6} + \frac{64\,c_{\theta}^6\,L_8^r\,M_0^8\,M_{\pi}^8\,s_{\theta}^4\,\Lambda_2}{243\,M_{\eta}^4\,M_{\eta'}^6} + \\
& \frac{14\,336\,c_{\theta}^4\,L_8^r\,M_0^6\,M_K^6\,s_{\theta}^4\,\Lambda_2}{243\,M_{\eta}^2\,M_{\eta'}^6} - \frac{40\,960\,c_{\theta}^4\,L_8^r\,M_0^6\,M_K^4\,M_{\pi}^2\,s_{\theta}^4\,\Lambda_2}{243\,M_{\eta}^2\,M_{\eta'}^6} + \frac{29\,696\,c_{\theta}^4\,L_8^r\,M_0^6\,M_K^2\,M_{\pi}^4\,s_{\theta}^4\,\Lambda_2}{243\,M_{\eta}^2\,M_{\eta'}^6} - \\
& \frac{3328\,c_{\theta}^4\,L_8^r\,M_0^6\,M_{\pi}^6\,s_{\theta}^4\,\Lambda_2}{81\,M_{\eta}^2\,M_{\eta'}^6} - \frac{348\,160\,c_{\theta}^8\,L_8^r\,M_0^8\,M_K^8\,s_{\theta}^4\,\Lambda_2}{729\,M_{\eta}^8\,M_{\eta'}^4} + \frac{7936\,c_{\theta}^8\,L_8^r\,M_0^8\,M_K^6\,M_{\pi}^2\,s_{\theta}^4\,\Lambda_2}{27\,M_{\eta}^8\,M_{\eta'}^4} + \\
& \frac{106\,112\,c_{\theta}^8\,L_8^r\,M_0^8\,M_K^4\,M_{\pi}^4\,s_{\theta}^4\,\Lambda_2}{243\,M_{\eta}^8\,M_{\eta'}^4} - \frac{262\,976\,c_{\theta}^8\,L_8^r\,M_0^8\,M_K^2\,M_{\pi}^6\,s_{\theta}^4\,\Lambda_2}{729\,M_{\eta}^8\,M_{\eta'}^4} + \frac{4576\,c_{\theta}^8\,L_8^r\,M_0^8\,M_{\pi}^8\,s_{\theta}^4\,\Lambda_2}{243\,M_{\eta}^8\,M_{\eta'}^4} - \\
& \frac{15\,872\,c_{\theta}^6\,L_8^r\,M_0^8\,M_K^6\,s_{\theta}^4\,\Lambda_2}{243\,M_{\eta}^6\,M_{\eta'}^4} - \frac{290\,816\,c_{\theta}^6\,L_8^r\,M_0^6\,M_K^8\,s_{\theta}^4\,\Lambda_2}{729\,M_{\eta}^6\,M_{\eta'}^4} + \frac{5632\,c_{\theta}^6\,L_8^r\,M_0^8\,M_K^4\,M_{\pi}^2\,s_{\theta}^4\,\Lambda_2}{243\,M_{\eta}^6\,M_{\eta'}^4} + \\
& \frac{118\,016\,c_{\theta}^6\,L_8^r\,M_0^6\,M_K^6\,M_{\pi}^2\,s_{\theta}^4\,\Lambda_2}{243\,M_{\eta}^6\,M_{\eta'}^4} + \frac{7936\,c_{\theta}^6\,L_8^r\,M_0^8\,M_K^2\,M_{\pi}^4\,s_{\theta}^4\,\Lambda_2}{243\,M_{\eta}^6\,M_{\eta'}^4} - \frac{1280\,c_{\theta}^6\,L_8^r\,M_0^6\,M_K^4\,M_{\pi}^4\,s_{\theta}^4\,\Lambda_2}{27\,M_{\eta}^6\,M_{\eta'}^4} + \\
& \frac{256\,c_{\theta}^6\,L_8^r\,M_0^8\,M_{\pi}^6\,s_{\theta}^4\,\Lambda_2}{27\,M_{\eta}^6\,M_{\eta'}^4} - \frac{31\,936\,c_{\theta}^6\,L_8^r\,M_0^6\,M_K^2\,M_{\pi}^6\,s_{\theta}^4\,\Lambda_2}{729\,M_{\eta}^6\,M_{\eta'}^4} + \frac{1088\,c_{\theta}^6\,L_8^r\,M_0^8\,M_{\pi}^8\,s_{\theta}^4\,\Lambda_2}{243\,M_{\eta}^6\,M_{\eta'}^4} - \\
& \frac{2048\,c_{\theta}^4\,L_8^r\,M_0^6\,M_K^6\,s_{\theta}^4\,\Lambda_2}{81\,M_{\eta}^4\,M_{\eta'}^4} + \frac{13\,312\,c_{\theta}^4\,L_8^r\,M_0^6\,M_K^4\,M_{\pi}^2\,s_{\theta}^4\,\Lambda_2}{81\,M_{\eta}^4\,M_{\eta'}^4} - \frac{12\,032\,c_{\theta}^4\,L_8^r\,M_0^6\,M_K^2\,M_{\pi}^4\,s_{\theta}^4\,\Lambda_2}{81\,M_{\eta}^4\,M_{\eta'}^4} + \\
& \frac{1408\,c_{\theta}^4\,L_8^r\,M_0^6\,M_{\pi}^6\,s_{\theta}^4\,\Lambda_2}{27\,M_{\eta}^4\,M_{\eta'}^4} - \frac{286\,720\,c_{\theta}^8\,L_8^r\,M_0^8\,M_K^8\,s_{\theta}^4\,\Lambda_2}{729\,M_{\eta}^{10}\,M_{\eta'}^2} + \frac{227\,840\,c_{\theta}^8\,L_8^r\,M_0^8\,M_K^6\,M_{\pi}^2\,s_{\theta}^4\,\Lambda_2}{243\,M_{\eta}^{10}\,M_{\eta'}^2} - \\
& \frac{204\,800\,c_{\theta}^8\,L_8^r\,M_0^8\,M_K^4\,M_{\pi}^4\,s_{\theta}^4\,\Lambda_2}{243\,M_{\eta}^{10}\,M_{\eta'}^2} + \frac{246\,784\,c_{\theta}^8\,L_8^r\,M_0^8\,M_K^2\,M_{\pi}^6\,s_{\theta}^4\,\Lambda_2}{729\,M_{\eta}^{10}\,M_{\eta'}^2} - \frac{13\,184\,c_{\theta}^8\,L_8^r\,M_0^8\,M_{\pi}^8\,s_{\theta}^4\,\Lambda_2}{243\,M_{\eta}^{10}\,M_{\eta'}^2} + \\
& \frac{29\,696\,c_{\theta}^6\,L_8^r\,M_0^8\,M_K^6\,s_{\theta}^4\,\Lambda_2}{243\,M_{\eta}^8\,M_{\eta'}^2} + \frac{90\,112\,c_{\theta}^6\,L_8^r\,M_0^6\,M_K^8\,s_{\theta}^4\,\Lambda_2}{729\,M_{\eta}^8\,M_{\eta'}^2} - \frac{41\,344\,c_{\theta}^6\,L_8^r\,M_0^8\,M_K^4\,M_{\pi}^2\,s_{\theta}^4\,\Lambda_2}{243\,M_{\eta}^8\,M_{\eta'}^2} - \\
& \frac{12\,032\,c_{\theta}^6\,L_8^r\,M_0^6\,M_K^6\,M_{\pi}^2\,s_{\theta}^4\,\Lambda_2}{243\,M_{\eta}^8\,M_{\eta'}^2} + \frac{18\,560\,c_{\theta}^6\,L_8^r\,M_0^6\,M_K^2\,M_{\pi}^4\,s_{\theta}^4\,\Lambda_2}{243\,M_{\eta}^8\,M_{\eta'}^2} - \frac{12\,800\,c_{\theta}^6\,L_8^r\,M_0^6\,M_K^4\,M_{\pi}^4\,s_{\theta}^4\,\Lambda_2}{81\,M_{\eta}^8\,M_{\eta'}^2} - \\
& \frac{64\,c_{\theta}^6\,L_8^r\,M_0^8\,M_{\pi}^6\,s_{\theta}^4\,\Lambda_2}{9\,M_{\eta}^8\,M_{\eta'}^2} + \frac{75\,584\,c_{\theta}^6\,L_8^r\,M_0^6\,M_K^2\,M_{\pi}^6\,s_{\theta}^4\,\Lambda_2}{729\,M_{\eta}^8\,M_{\eta'}^2} + \frac{128\,c_{\theta}^6\,L_8^r\,M_0^8\,M_{\pi}^8\,s_{\theta}^4\,\Lambda_2}{81\,M_{\eta}^8\,M_{\eta'}^2} + \\
& \frac{14\,336\,c_{\theta}^4\,L_8^r\,M_0^6\,M_K^6\,s_{\theta}^4\,\Lambda_2}{243\,M_{\eta}^6\,M_{\eta'}^2} - \frac{40\,960\,c_{\theta}^4\,L_8^r\,M_0^6\,M_K^4\,M_{\pi}^2\,s_{\theta}^4\,\Lambda_2}{243\,M_{\eta}^6\,M_{\eta'}^2} + \frac{29\,696\,c_{\theta}^4\,L_8^r\,M_0^6\,M_K^2\,M_{\pi}^4\,s_{\theta}^4\,\Lambda_2}{243\,M_{\eta}^6\,M_{\eta'}^2} -
\end{aligned}$$

$$\begin{aligned}
& \frac{3328 c_{\theta}^4 L_8^r M_0^6 M_{\pi}^6 s_{\theta}^4 \Lambda_2}{81 M_{\eta}^6 M_{\eta'}^2} - \frac{40960 \sqrt{2} c_{\theta}^7 L_8^r M_0^8 M_K^8 s_{\theta}^5 \Lambda_2}{729 M_{\eta}^{12}} + \frac{33280 \sqrt{2} c_{\theta}^7 L_8^r M_0^8 M_K^6 M_{\pi}^2 s_{\theta}^5 \Lambda_2}{243 M_{\eta}^{12}} - \\
& \frac{10240 \sqrt{2} c_{\theta}^7 L_8^r M_0^8 M_K^4 M_{\pi}^4 s_{\theta}^5 \Lambda_2}{81 M_{\eta}^{12}} + \frac{40000 \sqrt{2} c_{\theta}^7 L_8^r M_0^8 M_K^2 M_{\pi}^6 s_{\theta}^5 \Lambda_2}{729 M_{\eta}^{12}} - \frac{2240 \sqrt{2} c_{\theta}^7 L_8^r M_0^8 M_{\pi}^8 s_{\theta}^5 \Lambda_2}{243 M_{\eta}^{12}} + \\
& \frac{4096 \sqrt{2} c_{\theta}^5 L_8^r M_0^8 M_K^6 s_{\theta}^5 \Lambda_2}{243 M_{\eta}^{10}} + \frac{57344 \sqrt{2} c_{\theta}^5 L_8^r M_0^8 M_K^8 s_{\theta}^5 \Lambda_2}{243 M_{\eta}^{10}} - \frac{6656 \sqrt{2} c_{\theta}^5 L_8^r M_0^8 M_K^4 M_{\pi}^2 s_{\theta}^5 \Lambda_2}{243 M_{\eta}^{10}} - \\
& \frac{39424 \sqrt{2} c_{\theta}^5 L_8^r M_0^6 M_K^6 M_{\pi}^2 s_{\theta}^5 \Lambda_2}{81 M_{\eta}^{10}} + \frac{4096 \sqrt{2} c_{\theta}^5 L_8^r M_0^8 M_K^2 M_{\pi}^4 s_{\theta}^5 \Lambda_2}{243 M_{\eta}^{10}} + \\
& \frac{9728 \sqrt{2} c_{\theta}^5 L_8^r M_0^6 M_K^4 M_{\pi}^4 s_{\theta}^5 \Lambda_2}{27 M_{\eta}^{10}} - \frac{320 \sqrt{2} c_{\theta}^5 L_8^r M_0^8 M_{\pi}^6 s_{\theta}^5 \Lambda_2}{81 M_{\eta}^{10}} - \frac{25472 \sqrt{2} c_{\theta}^5 L_8^r M_0^6 M_K^2 M_{\pi}^6 s_{\theta}^5 \Lambda_2}{243 M_{\eta}^{10}} + \\
& \frac{128 \sqrt{2} c_{\theta}^5 L_8^r M_0^6 M_{\pi}^8 s_{\theta}^5 \Lambda_2}{27 M_{\eta}^{10}} - \frac{20480 \sqrt{2} c_{\theta}^3 L_8^r M_0^6 M_K^6 s_{\theta}^5 \Lambda_2}{243 M_{\eta}^8} + \frac{28672 \sqrt{2} c_{\theta}^3 L_8^r M_0^6 M_K^4 M_{\pi}^2 s_{\theta}^5 \Lambda_2}{243 M_{\eta}^8} - \\
& \frac{14336 \sqrt{2} c_{\theta}^3 L_8^r M_0^6 M_K^2 M_{\pi}^4 s_{\theta}^5 \Lambda_2}{243 M_{\eta}^8} + \frac{1280 \sqrt{2} c_{\theta}^3 L_8^r M_0^6 M_{\pi}^6 s_{\theta}^5 \Lambda_2}{81 M_{\eta}^8} + \frac{143360 \sqrt{2} c_{\theta}^7 L_8^r M_0^8 M_K^8 s_{\theta}^5 \Lambda_2}{243 M_{\eta'}^{12}} - \\
& \frac{98560 \sqrt{2} c_{\theta}^7 L_8^r M_0^8 M_K^6 M_{\pi}^2 s_{\theta}^5 \Lambda_2}{81 M_{\eta'}^{12}} + \frac{24320 \sqrt{2} c_{\theta}^7 L_8^r M_0^8 M_K^4 M_{\pi}^4 s_{\theta}^5 \Lambda_2}{27 M_{\eta'}^{12}} - \\
& \frac{63680 \sqrt{2} c_{\theta}^7 L_8^r M_0^8 M_K^2 M_{\pi}^6 s_{\theta}^5 \Lambda_2}{243 M_{\eta'}^{12}} + \frac{320 \sqrt{2} c_{\theta}^7 L_8^r M_0^8 M_{\pi}^8 s_{\theta}^5 \Lambda_2}{27 M_{\eta'}^{12}} - \frac{4096 \sqrt{2} c_{\theta}^5 L_8^r M_0^8 M_K^6 s_{\theta}^5 \Lambda_2}{243 M_{\eta'}^{10}} - \\
& \frac{57344 \sqrt{2} c_{\theta}^5 L_8^r M_0^6 M_K^8 s_{\theta}^5 \Lambda_2}{243 M_{\eta'}^{10}} + \frac{6656 \sqrt{2} c_{\theta}^5 L_8^r M_0^8 M_K^4 M_{\pi}^2 s_{\theta}^5 \Lambda_2}{243 M_{\eta'}^{10}} + \frac{39424 \sqrt{2} c_{\theta}^5 L_8^r M_0^6 M_K^6 M_{\pi}^2 s_{\theta}^5 \Lambda_2}{81 M_{\eta'}^{10}} - \\
& \frac{4096 \sqrt{2} c_{\theta}^5 L_8^r M_0^8 M_K^2 M_{\pi}^4 s_{\theta}^5 \Lambda_2}{243 M_{\eta'}^{10}} - \frac{9728 \sqrt{2} c_{\theta}^5 L_8^r M_0^6 M_K^4 M_{\pi}^4 s_{\theta}^5 \Lambda_2}{27 M_{\eta'}^{10}} + \frac{320 \sqrt{2} c_{\theta}^5 L_8^r M_0^8 M_{\pi}^6 s_{\theta}^5 \Lambda_2}{81 M_{\eta'}^{10}} + \\
& \frac{25472 \sqrt{2} c_{\theta}^5 L_8^r M_0^6 M_K^2 M_{\pi}^6 s_{\theta}^5 \Lambda_2}{243 M_{\eta'}^{10}} - \frac{128 \sqrt{2} c_{\theta}^5 L_8^r M_0^8 M_{\pi}^8 s_{\theta}^5 \Lambda_2}{27 M_{\eta'}^{10}} - \frac{372736 \sqrt{2} c_{\theta}^7 L_8^r M_0^8 M_K^8 s_{\theta}^5 \Lambda_2}{729 M_{\eta}^2 M_{\eta'}^{10}} + \\
& \frac{379136 \sqrt{2} c_{\theta}^7 L_8^r M_0^8 M_K^6 M_{\pi}^2 s_{\theta}^5 \Lambda_2}{243 M_{\eta}^2 M_{\eta'}^{10}} - \frac{326912 \sqrt{2} c_{\theta}^7 L_8^r M_0^8 M_K^4 M_{\pi}^4 s_{\theta}^5 \Lambda_2}{243 M_{\eta}^2 M_{\eta'}^{10}} + \\
& \frac{246400 \sqrt{2} c_{\theta}^7 L_8^r M_0^8 M_K^2 M_{\pi}^6 s_{\theta}^5 \Lambda_2}{729 M_{\eta}^2 M_{\eta'}^{10}} - \frac{14720 \sqrt{2} c_{\theta}^7 L_8^r M_0^8 M_{\pi}^8 s_{\theta}^5 \Lambda_2}{243 M_{\eta}^2 M_{\eta'}^{10}} + \frac{4096 \sqrt{2} c_{\theta}^3 L_8^r M_0^6 M_K^6 s_{\theta}^5 \Lambda_2}{243 M_{\eta'}^8} - \\
& \frac{8192 \sqrt{2} c_{\theta}^3 L_8^r M_0^6 M_K^4 M_{\pi}^2 s_{\theta}^5 \Lambda_2}{243 M_{\eta'}^8} + \frac{5248 \sqrt{2} c_{\theta}^3 L_8^r M_0^6 M_K^2 M_{\pi}^4 s_{\theta}^5 \Lambda_2}{243 M_{\eta'}^8} - \frac{128 \sqrt{2} c_{\theta}^3 L_8^r M_0^6 M_{\pi}^6 s_{\theta}^5 \Lambda_2}{27 M_{\eta'}^8} + \\
& \frac{284672 \sqrt{2} c_{\theta}^7 L_8^r M_0^8 M_K^8 s_{\theta}^5 \Lambda_2}{729 M_{\eta}^4 M_{\eta'}^8} - \frac{143872 \sqrt{2} c_{\theta}^7 L_8^r M_0^8 M_K^6 M_{\pi}^2 s_{\theta}^5 \Lambda_2}{81 M_{\eta}^4 M_{\eta'}^8} +
\end{aligned}$$

$$\begin{aligned}
& \frac{401\,408 \sqrt{2} \, c_{\theta}^7 L_8^r M_0^8 M_K^4 M_{\pi}^4 s_{\theta}^5 \Lambda_2}{243 M_{\eta}^4 M_{\eta'}^8} - \frac{229\,952 \sqrt{2} \, c_{\theta}^7 L_8^r M_0^8 M_K^2 M_{\pi}^6 s_{\theta}^5 \Lambda_2}{729 M_{\eta}^4 M_{\eta'}^8} + \\
& \frac{448 \sqrt{2} \, c_{\theta}^7 L_8^r M_0^8 M_{\pi}^8 s_{\theta}^5 \Lambda_2}{243 M_{\eta}^4 M_{\eta'}^8} - \frac{31\,232 \sqrt{2} \, c_{\theta}^5 L_8^r M_0^8 M_K^6 s_{\theta}^5 \Lambda_2}{243 M_{\eta}^2 M_{\eta'}^8} + \frac{57\,344 \sqrt{2} \, c_{\theta}^5 L_8^r M_0^6 M_K^8 s_{\theta}^5 \Lambda_2}{243 M_{\eta}^2 M_{\eta'}^8} + \\
& \frac{45\,568 \sqrt{2} \, c_{\theta}^5 L_8^r M_0^8 M_K^4 M_{\pi}^2 s_{\theta}^5 \Lambda_2}{243 M_{\eta}^2 M_{\eta'}^8} - \frac{46\,592 \sqrt{2} \, c_{\theta}^5 L_8^r M_0^6 M_K^6 M_{\pi}^2 s_{\theta}^5 \Lambda_2}{81 M_{\eta}^2 M_{\eta'}^8} - \\
& \frac{17\,216 \sqrt{2} \, c_{\theta}^5 L_8^r M_0^8 M_K^2 M_{\pi}^4 s_{\theta}^5 \Lambda_2}{243 M_{\eta}^2 M_{\eta'}^8} + \frac{35\,200 \sqrt{2} \, c_{\theta}^5 L_8^r M_0^6 M_K^4 M_{\pi}^4 s_{\theta}^5 \Lambda_2}{81 M_{\eta}^2 M_{\eta'}^8} + \\
& \frac{416 \sqrt{2} \, c_{\theta}^5 L_8^r M_0^8 M_{\pi}^6 s_{\theta}^5 \Lambda_2}{27 M_{\eta}^2 M_{\eta'}^8} - \frac{22\,592 \sqrt{2} \, c_{\theta}^5 L_8^r M_0^6 M_K^2 M_{\pi}^6 s_{\theta}^5 \Lambda_2}{243 M_{\eta}^2 M_{\eta'}^8} + \frac{320 \sqrt{2} \, c_{\theta}^5 L_8^r M_0^6 M_{\pi}^8 s_{\theta}^5 \Lambda_2}{27 M_{\eta}^2 M_{\eta'}^8} - \\
& \frac{477\,184 \sqrt{2} \, c_{\theta}^7 L_8^r M_0^8 M_K^8 s_{\theta}^5 \Lambda_2}{729 M_{\eta}^6 M_{\eta'}^6} + \frac{557\,056 \sqrt{2} \, c_{\theta}^7 L_8^r M_0^8 M_K^6 M_{\pi}^2 s_{\theta}^5 \Lambda_2}{243 M_{\eta}^6 M_{\eta'}^6} - \\
& \frac{159\,232 \sqrt{2} \, c_{\theta}^7 L_8^r M_0^8 M_K^4 M_{\pi}^4 s_{\theta}^5 \Lambda_2}{81 M_{\eta}^6 M_{\eta'}^6} + \frac{238\,336 \sqrt{2} \, c_{\theta}^7 L_8^r M_0^8 M_K^2 M_{\pi}^6 s_{\theta}^5 \Lambda_2}{729 M_{\eta}^6 M_{\eta'}^6} + \\
& \frac{4864 \sqrt{2} \, c_{\theta}^7 L_8^r M_0^8 M_{\pi}^8 s_{\theta}^5 \Lambda_2}{243 M_{\eta}^6 M_{\eta'}^6} + \frac{55\,808 \sqrt{2} \, c_{\theta}^5 L_8^r M_0^8 M_K^6 s_{\theta}^5 \Lambda_2}{243 M_{\eta}^4 M_{\eta'}^6} - \frac{45\,056 \sqrt{2} \, c_{\theta}^5 L_8^r M_0^6 M_K^8 s_{\theta}^5 \Lambda_2}{243 M_{\eta}^4 M_{\eta'}^6} - \\
& \frac{85\,504 \sqrt{2} \, c_{\theta}^5 L_8^r M_0^8 M_K^4 M_{\pi}^2 s_{\theta}^5 \Lambda_2}{243 M_{\eta}^4 M_{\eta'}^6} + \frac{46\,592 \sqrt{2} \, c_{\theta}^5 L_8^r M_0^6 M_K^6 M_{\pi}^2 s_{\theta}^5 \Lambda_2}{81 M_{\eta}^4 M_{\eta'}^6} + \\
& \frac{28\,736 \sqrt{2} \, c_{\theta}^5 L_8^r M_0^8 M_K^2 M_{\pi}^4 s_{\theta}^5 \Lambda_2}{243 M_{\eta}^4 M_{\eta'}^6} - \frac{12\,416 \sqrt{2} \, c_{\theta}^5 L_8^r M_0^6 M_K^4 M_{\pi}^4 s_{\theta}^5 \Lambda_2}{27 M_{\eta}^4 M_{\eta'}^6} + \frac{416 \sqrt{2} \, c_{\theta}^5 L_8^r M_0^8 M_{\pi}^6 s_{\theta}^5 \Lambda_2}{81 M_{\eta}^4 M_{\eta'}^6} + \\
& \frac{17\,216 \sqrt{2} \, c_{\theta}^5 L_8^r M_0^6 M_K^2 M_{\pi}^6 s_{\theta}^5 \Lambda_2}{243 M_{\eta}^4 M_{\eta'}^6} + \frac{320 \sqrt{2} \, c_{\theta}^5 L_8^r M_0^6 M_{\pi}^8 s_{\theta}^5 \Lambda_2}{81 M_{\eta}^4 M_{\eta'}^6} + \frac{14\,336 \sqrt{2} \, c_{\theta}^3 L_8^r M_0^6 M_K^6 s_{\theta}^5 \Lambda_2}{243 M_{\eta}^2 M_{\eta'}^6} - \\
& \frac{16\,384 \sqrt{2} \, c_{\theta}^3 L_8^r M_0^6 M_K^4 M_{\pi}^2 s_{\theta}^5 \Lambda_2}{243 M_{\eta}^2 M_{\eta'}^6} + \frac{7040 \sqrt{2} \, c_{\theta}^3 L_8^r M_0^6 M_K^2 M_{\pi}^4 s_{\theta}^5 \Lambda_2}{243 M_{\eta}^2 M_{\eta'}^6} - \frac{896 \sqrt{2} \, c_{\theta}^3 L_8^r M_0^6 M_{\pi}^6 s_{\theta}^5 \Lambda_2}{81 M_{\eta}^2 M_{\eta'}^6} + \\
& \frac{720\,896 \sqrt{2} \, c_{\theta}^7 L_8^r M_0^8 M_K^8 s_{\theta}^5 \Lambda_2}{729 M_{\eta}^8 M_{\eta'}^4} - \frac{602\,368 \sqrt{2} \, c_{\theta}^7 L_8^r M_0^8 M_K^6 M_{\pi}^2 s_{\theta}^5 \Lambda_2}{243 M_{\eta}^8 M_{\eta'}^4} + \\
& \frac{461\,056 \sqrt{2} \, c_{\theta}^7 L_8^r M_0^8 M_K^4 M_{\pi}^4 s_{\theta}^5 \Lambda_2}{243 M_{\eta}^8 M_{\eta'}^4} - \frac{264\,896 \sqrt{2} \, c_{\theta}^7 L_8^r M_0^8 M_K^2 M_{\pi}^6 s_{\theta}^5 \Lambda_2}{729 M_{\eta}^8 M_{\eta'}^4} + \\
& \frac{4288 \sqrt{2} \, c_{\theta}^7 L_8^r M_0^8 M_{\pi}^8 s_{\theta}^5 \Lambda_2}{243 M_{\eta}^8 M_{\eta'}^4} - \frac{55\,808 \sqrt{2} \, c_{\theta}^5 L_8^r M_0^8 M_K^6 s_{\theta}^5 \Lambda_2}{243 M_{\eta}^6 M_{\eta'}^4} + \frac{45\,056 \sqrt{2} \, c_{\theta}^5 L_8^r M_0^6 M_K^8 s_{\theta}^5 \Lambda_2}{243 M_{\eta}^6 M_{\eta'}^4} + \\
& \frac{85\,504 \sqrt{2} \, c_{\theta}^5 L_8^r M_0^8 M_K^4 M_{\pi}^2 s_{\theta}^5 \Lambda_2}{243 M_{\eta}^6 M_{\eta'}^4} - \frac{46\,592 \sqrt{2} \, c_{\theta}^5 L_8^r M_0^6 M_K^6 M_{\pi}^2 s_{\theta}^5 \Lambda_2}{81 M_{\eta}^6 M_{\eta'}^4} -
\end{aligned}$$

$$\begin{aligned}
& \frac{28\,736\sqrt{2}\,c_\theta^5 L_8^r M_0^8 M_K^2 M_\pi^4 s_\theta^5 \Lambda_2}{243 M_\eta^6 M_{\eta'}^4} + \frac{12\,416\sqrt{2}\,c_\theta^5 L_8^r M_0^6 M_K^4 M_\pi^4 s_\theta^5 \Lambda_2}{27 M_\eta^6 M_{\eta'}^4} - \\
& \frac{416\sqrt{2}\,c_\theta^5 L_8^r M_0^8 M_\pi^6 s_\theta^5 \Lambda_2}{81 M_\eta^6 M_{\eta'}^4} - \frac{17\,216\sqrt{2}\,c_\theta^5 L_8^r M_0^6 M_K^2 M_\pi^6 s_\theta^5 \Lambda_2}{243 M_\eta^6 M_{\eta'}^4} - \frac{320\sqrt{2}\,c_\theta^5 L_8^r M_0^6 M_\pi^8 s_\theta^5 \Lambda_2}{81 M_\eta^6 M_{\eta'}^4} - \\
& \frac{1024\sqrt{2}\,c_\theta^3 L_8^r M_0^6 M_K^6 s_\theta^5 \Lambda_2}{9 M_\eta^4 M_{\eta'}^4} + \frac{4096\sqrt{2}\,c_\theta^3 L_8^r M_0^6 M_K^4 M_\pi^2 s_\theta^5 \Lambda_2}{27 M_\eta^4 M_{\eta'}^4} - \frac{2176\sqrt{2}\,c_\theta^3 L_8^r M_0^6 M_K^2 M_\pi^4 s_\theta^5 \Lambda_2}{27 M_\eta^4 M_{\eta'}^4} + \\
& \frac{128\sqrt{2}\,c_\theta^3 L_8^r M_0^6 M_\pi^6 s_\theta^5 \Lambda_2}{9 M_\eta^4 M_{\eta'}^4} - \frac{544\,768\sqrt{2}\,c_\theta^7 L_8^r M_0^8 M_K^8 s_\theta^5 \Lambda_2}{729 M_\eta^{10} M_{\eta'}^2} + \frac{120\,064\sqrt{2}\,c_\theta^7 L_8^r M_0^8 M_K^6 M_\pi^2 s_\theta^5 \Lambda_2}{81 M_\eta^{10} M_{\eta'}^2} - \\
& \frac{246\,016\sqrt{2}\,c_\theta^7 L_8^r M_0^8 M_K^4 M_\pi^4 s_\theta^5 \Lambda_2}{243 M_\eta^{10} M_{\eta'}^2} + \frac{161\,152\sqrt{2}\,c_\theta^7 L_8^r M_0^8 M_K^2 M_\pi^6 s_\theta^5 \Lambda_2}{729 M_\eta^{10} M_{\eta'}^2} + \\
& \frac{4480\sqrt{2}\,c_\theta^7 L_8^r M_0^8 M_\pi^8 s_\theta^5 \Lambda_2}{243 M_\eta^{10} M_{\eta'}^2} + \frac{31\,232\sqrt{2}\,c_\theta^5 L_8^r M_0^8 M_K^6 s_\theta^5 \Lambda_2}{243 M_\eta^8 M_{\eta'}^2} - \frac{57\,344\sqrt{2}\,c_\theta^5 L_8^r M_0^6 M_K^8 s_\theta^5 \Lambda_2}{243 M_\eta^8 M_{\eta'}^2} - \\
& \frac{45\,568\sqrt{2}\,c_\theta^5 L_8^r M_0^8 M_K^4 M_\pi^2 s_\theta^5 \Lambda_2}{243 M_\eta^8 M_{\eta'}^2} + \frac{46\,592\sqrt{2}\,c_\theta^5 L_8^r M_0^6 M_K^6 M_\pi^2 s_\theta^5 \Lambda_2}{81 M_\eta^8 M_{\eta'}^2} + \\
& \frac{17\,216\sqrt{2}\,c_\theta^5 L_8^r M_0^8 M_K^2 M_\pi^4 s_\theta^5 \Lambda_2}{243 M_\eta^8 M_{\eta'}^2} - \frac{35\,200\sqrt{2}\,c_\theta^5 L_8^r M_0^6 M_K^4 M_\pi^4 s_\theta^5 \Lambda_2}{81 M_\eta^8 M_{\eta'}^2} - \frac{416\sqrt{2}\,c_\theta^5 L_8^r M_0^8 M_\pi^6 s_\theta^5 \Lambda_2}{27 M_\eta^8 M_{\eta'}^2} + \\
& \frac{22\,592\sqrt{2}\,c_\theta^5 L_8^r M_0^6 M_K^2 M_\pi^6 s_\theta^5 \Lambda_2}{243 M_\eta^8 M_{\eta'}^2} - \frac{320\sqrt{2}\,c_\theta^5 L_8^r M_0^6 M_\pi^8 s_\theta^5 \Lambda_2}{27 M_\eta^8 M_{\eta'}^2} + \frac{29\,696\sqrt{2}\,c_\theta^3 L_8^r M_0^6 M_K^6 s_\theta^5 \Lambda_2}{243 M_\eta^6 M_{\eta'}^2} - \\
& \frac{40\,960\sqrt{2}\,c_\theta^3 L_8^r M_0^6 M_K^4 M_\pi^2 s_\theta^5 \Lambda_2}{243 M_\eta^6 M_{\eta'}^2} + \frac{21\,632\sqrt{2}\,c_\theta^3 L_8^r M_0^6 M_K^2 M_\pi^4 s_\theta^5 \Lambda_2}{243 M_\eta^6 M_{\eta'}^2} - \frac{128\sqrt{2}\,c_\theta^3 L_8^r M_0^6 M_\pi^6 s_\theta^5 \Lambda_2}{9 M_\eta^6 M_{\eta'}^2} - \\
& \frac{286\,720\,c_\theta^6 L_8^r M_0^8 M_K^8 s_\theta^6 \Lambda_2}{729 M_\eta^{12}} + \frac{74\,240\,c_\theta^6 L_8^r M_0^8 M_K^6 M_\pi^2 s_\theta^6 \Lambda_2}{81 M_\eta^{12}} - \frac{21\,760\,c_\theta^6 L_8^r M_0^8 M_K^4 M_\pi^4 s_\theta^6 \Lambda_2}{27 M_\eta^{12}} + \\
& \frac{228\,160\,c_\theta^6 L_8^r M_0^8 M_K^2 M_\pi^6 s_\theta^6 \Lambda_2}{729 M_\eta^{12}} - \frac{11\,680\,c_\theta^6 L_8^r M_0^8 M_\pi^8 s_\theta^6 \Lambda_2}{243 M_\eta^{12}} + \frac{20\,480\,c_\theta^4 L_8^r M_0^8 M_K^6 s_\theta^6 \Lambda_2}{243 M_\eta^{10}} + \\
& \frac{286\,720\,c_\theta^4 L_8^r M_0^6 M_K^8 s_\theta^6 \Lambda_2}{729 M_\eta^{10}} - \frac{28\,672\,c_\theta^4 L_8^r M_0^8 M_K^4 M_\pi^2 s_\theta^6 \Lambda_2}{243 M_\eta^{10}} - \frac{174\,592\,c_\theta^4 L_8^r M_0^6 M_K^6 M_\pi^2 s_\theta^6 \Lambda_2}{243 M_\eta^{10}} + \\
& \frac{12\,800\,c_\theta^4 L_8^r M_0^8 M_K^2 M_\pi^4 s_\theta^6 \Lambda_2}{243 M_\eta^{10}} + \frac{38\,656\,c_\theta^4 L_8^r M_0^6 M_K^4 M_\pi^4 s_\theta^6 \Lambda_2}{81 M_\eta^{10}} - \frac{128\,c_\theta^4 L_8^r M_0^8 M_\pi^6 s_\theta^6 \Lambda_2}{27 M_\eta^{10}} - \\
& \frac{108\,928\,c_\theta^4 L_8^r M_0^6 M_K^2 M_\pi^6 s_\theta^6 \Lambda_2}{729 M_\eta^{10}} + \frac{80\,000\,c_\theta^4 L_8^r M_0^6 M_\pi^8 s_\theta^6 \Lambda_2}{243 M_\eta^{10}} - \frac{20\,480\,c_\theta^2 L_8^r M_0^6 M_K^6 s_\theta^6 \Lambda_2}{243 M_\eta^8} + \\
& \frac{22\,528\,c_\theta^2 L_8^r M_0^6 M_K^4 M_\pi^2 s_\theta^6 \Lambda_2}{243 M_\eta^8} - \frac{66\,560\,c_\theta^2 L_8^r M_0^6 M_K^2 M_\pi^4 s_\theta^6 \Lambda_2}{243 M_\eta^8} - \frac{256\,c_\theta^2 L_8^r M_0^6 M_\pi^6 s_\theta^6 \Lambda_2}{27 M_\eta^8} - \\
& \frac{286\,720\,c_\theta^6 L_8^r M_0^8 M_K^8 s_\theta^6 \Lambda_2}{729 M_\eta^{12}} + \frac{74\,240\,c_\theta^6 L_8^r M_0^8 M_K^6 M_\pi^2 s_\theta^6 \Lambda_2}{81 M_\eta^{12}} - \frac{21\,760\,c_\theta^6 L_8^r M_0^8 M_K^4 M_\pi^4 s_\theta^6 \Lambda_2}{27 M_\eta^{12}} +
\end{aligned}$$

$$\begin{aligned}
& \frac{228\,160\,c_{\theta}^6 L_8^r M_0^8 M_K^2 M_{\pi}^6 s_{\theta}^6 \Lambda_2}{729 M_{\eta'}^{12}} - \frac{11\,680\,c_{\theta}^6 L_8^r M_0^8 M_{\pi}^8 s_{\theta}^6 \Lambda_2}{243 M_{\eta'}^{12}} + \frac{114\,688\,c_{\theta}^4 L_8^r M_0^6 M_K^8 s_{\theta}^6 \Lambda_2}{729 M_{\eta'}^{10}} - \\
& \frac{29\,696\,c_{\theta}^4 L_8^r M_0^6 M_K^2 M_{\pi}^6 s_{\theta}^6 \Lambda_2}{81 M_{\eta'}^{10}} + \frac{8704\,c_{\theta}^4 L_8^r M_0^6 M_K^4 M_{\pi}^6 s_{\theta}^6 \Lambda_2}{27 M_{\eta'}^{10}} - \frac{91\,264\,c_{\theta}^4 L_8^r M_0^6 M_K^2 M_{\pi}^6 s_{\theta}^6 \Lambda_2}{729 M_{\eta'}^{10}} + \\
& \frac{4672\,c_{\theta}^4 L_8^r M_0^6 M_{\pi}^8 s_{\theta}^6 \Lambda_2}{243 M_{\eta'}^{10}} - \frac{573\,440\,c_{\theta}^6 L_8^r M_0^8 M_K^8 s_{\theta}^6 \Lambda_2}{729 M_{\eta'}^2 M_{\eta'}^{10}} + \frac{177\,664\,c_{\theta}^6 L_8^r M_0^6 M_K^2 M_{\pi}^6 s_{\theta}^6 \Lambda_2}{243 M_{\eta'}^2 M_{\eta'}^{10}} + \\
& \frac{56\,576\,c_{\theta}^6 L_8^r M_0^8 M_K^4 M_{\pi}^4 s_{\theta}^6 \Lambda_2}{243 M_{\eta'}^2 M_{\eta'}^{10}} - \frac{209\,152\,c_{\theta}^6 L_8^r M_0^8 M_K^2 M_{\pi}^6 s_{\theta}^6 \Lambda_2}{729 M_{\eta'}^2 M_{\eta'}^{10}} - \frac{4480\,c_{\theta}^6 L_8^r M_0^8 M_{\pi}^8 s_{\theta}^6 \Lambda_2}{243 M_{\eta'}^2 M_{\eta'}^{10}} + \\
& \frac{1\,478\,656\,c_{\theta}^6 L_8^r M_0^8 M_K^8 s_{\theta}^6 \Lambda_2}{729 M_{\eta'}^4 M_{\eta'}^8} - \frac{641\,024\,c_{\theta}^6 L_8^r M_0^8 M_K^2 M_{\pi}^6 s_{\theta}^6 \Lambda_2}{243 M_{\eta'}^4 M_{\eta'}^8} + \frac{134\,912\,c_{\theta}^6 L_8^r M_0^8 M_K^4 M_{\pi}^4 s_{\theta}^6 \Lambda_2}{243 M_{\eta'}^4 M_{\eta'}^8} + \\
& \frac{43\,328\,c_{\theta}^6 L_8^r M_0^8 M_K^2 M_{\pi}^6 s_{\theta}^6 \Lambda_2}{729 M_{\eta'}^4 M_{\eta'}^8} - \frac{352\,c_{\theta}^6 L_8^r M_0^8 M_{\pi}^8 s_{\theta}^6 \Lambda_2}{243 M_{\eta'}^4 M_{\eta'}^8} + \frac{29\,696\,c_{\theta}^4 L_8^r M_0^8 M_K^6 s_{\theta}^6 \Lambda_2}{243 M_{\eta'}^2 M_{\eta'}^8} + \\
& \frac{90\,112\,c_{\theta}^4 L_8^r M_0^6 M_K^8 s_{\theta}^6 \Lambda_2}{729 M_{\eta'}^2 M_{\eta'}^8} - \frac{41\,344\,c_{\theta}^4 L_8^r M_0^8 M_K^4 M_{\pi}^2 s_{\theta}^6 \Lambda_2}{243 M_{\eta'}^2 M_{\eta'}^8} - \frac{12\,032\,c_{\theta}^4 L_8^r M_0^6 M_K^2 M_{\pi}^6 s_{\theta}^6 \Lambda_2}{243 M_{\eta'}^2 M_{\eta'}^8} + \\
& \frac{18\,560\,c_{\theta}^4 L_8^r M_0^8 M_K^2 M_{\pi}^4 s_{\theta}^6 \Lambda_2}{243 M_{\eta'}^2 M_{\eta'}^8} - \frac{12\,800\,c_{\theta}^4 L_8^r M_0^6 M_K^4 M_{\pi}^4 s_{\theta}^6 \Lambda_2}{81 M_{\eta'}^2 M_{\eta'}^8} - \frac{64\,c_{\theta}^4 L_8^r M_0^8 M_{\pi}^6 s_{\theta}^6 \Lambda_2}{9 M_{\eta'}^2 M_{\eta'}^8} + \\
& \frac{75\,584\,c_{\theta}^4 L_8^r M_0^6 M_K^2 M_{\pi}^6 s_{\theta}^6 \Lambda_2}{729 M_{\eta'}^2 M_{\eta'}^8} + \frac{128\,c_{\theta}^4 L_8^r M_0^6 M_{\pi}^8 s_{\theta}^6 \Lambda_2}{81 M_{\eta'}^2 M_{\eta'}^8} - \frac{1\,789\,952\,c_{\theta}^6 L_8^r M_0^8 M_K^8 s_{\theta}^6 \Lambda_2}{729 M_{\eta'}^6 M_{\eta'}^6} + \\
& \frac{266\,240\,c_{\theta}^6 L_8^r M_0^8 M_K^2 M_{\pi}^6 s_{\theta}^6 \Lambda_2}{81 M_{\eta'}^6 M_{\eta'}^6} - \frac{67\,072\,c_{\theta}^6 L_8^r M_0^8 M_K^4 M_{\pi}^4 s_{\theta}^6 \Lambda_2}{81 M_{\eta'}^6 M_{\eta'}^6} + \frac{28\,928\,c_{\theta}^6 L_8^r M_0^8 M_K^2 M_{\pi}^6 s_{\theta}^6 \Lambda_2}{729 M_{\eta'}^6 M_{\eta'}^6} + \\
& \frac{1024\,c_{\theta}^6 L_8^r M_0^8 M_{\pi}^8 s_{\theta}^6 \Lambda_2}{243 M_{\eta'}^6 M_{\eta'}^6} - \frac{15\,872\,c_{\theta}^4 L_8^r M_0^8 M_K^6 s_{\theta}^6 \Lambda_2}{243 M_{\eta'}^4 M_{\eta'}^6} - \frac{290\,816\,c_{\theta}^4 L_8^r M_0^6 M_K^8 s_{\theta}^6 \Lambda_2}{729 M_{\eta'}^4 M_{\eta'}^6} + \\
& \frac{5632\,c_{\theta}^4 L_8^r M_0^8 M_K^4 M_{\pi}^2 s_{\theta}^6 \Lambda_2}{243 M_{\eta'}^4 M_{\eta'}^6} + \frac{118\,016\,c_{\theta}^4 L_8^r M_0^6 M_K^6 M_{\pi}^2 s_{\theta}^6 \Lambda_2}{243 M_{\eta'}^4 M_{\eta'}^6} + \frac{7936\,c_{\theta}^4 L_8^r M_0^8 M_K^2 M_{\pi}^4 s_{\theta}^6 \Lambda_2}{243 M_{\eta'}^4 M_{\eta'}^6} - \\
& \frac{1280\,c_{\theta}^4 L_8^r M_0^6 M_K^4 M_{\pi}^4 s_{\theta}^6 \Lambda_2}{27 M_{\eta'}^4 M_{\eta'}^6} + \frac{256\,c_{\theta}^4 L_8^r M_0^8 M_{\pi}^6 s_{\theta}^6 \Lambda_2}{27 M_{\eta'}^4 M_{\eta'}^6} - \frac{31\,936\,c_{\theta}^4 L_8^r M_0^6 M_K^2 M_{\pi}^6 s_{\theta}^6 \Lambda_2}{729 M_{\eta'}^4 M_{\eta'}^6} + \\
& \frac{1088\,c_{\theta}^4 L_8^r M_0^6 M_{\pi}^8 s_{\theta}^6 \Lambda_2}{243 M_{\eta'}^4 M_{\eta'}^6} - \frac{4096\,c_{\theta}^2 L_8^r M_0^6 M_K^6 s_{\theta}^6 \Lambda_2}{81 M_{\eta'}^2 M_{\eta'}^6} + \frac{8192\,c_{\theta}^2 L_8^r M_0^6 M_K^4 M_{\pi}^2 s_{\theta}^6 \Lambda_2}{81 M_{\eta'}^2 M_{\eta'}^6} - \\
& \frac{4864\,c_{\theta}^2 L_8^r M_0^6 M_K^2 M_{\pi}^4 s_{\theta}^6 \Lambda_2}{81 M_{\eta'}^2 M_{\eta'}^6} + \frac{256\,c_{\theta}^2 L_8^r M_0^6 M_{\pi}^6 s_{\theta}^6 \Lambda_2}{27 M_{\eta'}^2 M_{\eta'}^6} + \frac{1\,478\,656\,c_{\theta}^6 L_8^r M_0^8 M_K^8 s_{\theta}^6 \Lambda_2}{729 M_{\eta'}^8 M_{\eta'}^4} - \\
& \frac{641\,024\,c_{\theta}^6 L_8^r M_0^8 M_K^2 M_{\pi}^6 s_{\theta}^6 \Lambda_2}{243 M_{\eta'}^8 M_{\eta'}^4} + \frac{134\,912\,c_{\theta}^6 L_8^r M_0^8 M_K^4 M_{\pi}^4 s_{\theta}^6 \Lambda_2}{243 M_{\eta'}^8 M_{\eta'}^4} + \frac{43\,328\,c_{\theta}^6 L_8^r M_0^8 M_K^2 M_{\pi}^6 s_{\theta}^6 \Lambda_2}{729 M_{\eta'}^8 M_{\eta'}^4} - \\
& \frac{352\,c_{\theta}^6 L_8^r M_0^8 M_{\pi}^8 s_{\theta}^6 \Lambda_2}{243 M_{\eta'}^8 M_{\eta'}^4} - \frac{8192\,c_{\theta}^4 L_8^r M_0^8 M_K^6 s_{\theta}^6 \Lambda_2}{243 M_{\eta'}^6 M_{\eta'}^4} + \frac{372\,736\,c_{\theta}^4 L_8^r M_0^6 M_K^8 s_{\theta}^6 \Lambda_2}{729 M_{\eta'}^6 M_{\eta'}^4} +
\end{aligned}$$



$$\begin{aligned}
& \frac{42\,112\,c_{\theta}^4\,L_8^r\,M_0^8\,M_K^4\,M_{\pi}^2\,s_{\theta}^6\,\Lambda_2}{243\,M_{\eta}^6\,M_{\eta'}^4} - \frac{59\,648\,c_{\theta}^4\,L_8^r\,M_0^6\,M_K^6\,M_{\pi}^2\,s_{\theta}^6\,\Lambda_2}{81\,M_{\eta}^6\,M_{\eta'}^4} - \frac{37\,760\,c_{\theta}^4\,L_8^r\,M_0^8\,M_K^2\,M_{\pi}^4\,s_{\theta}^6\,\Lambda_2}{243\,M_{\eta}^6\,M_{\eta'}^4} + \\
& \frac{256\,c_{\theta}^4\,L_8^r\,M_0^6\,M_K^4\,M_{\pi}^4\,s_{\theta}^6\,\Lambda_2}{M_{\eta}^6\,M_{\eta'}^4} + \frac{1088\,c_{\theta}^4\,L_8^r\,M_0^8\,M_{\pi}^6\,s_{\theta}^6\,\Lambda_2}{81\,M_{\eta}^6\,M_{\eta'}^4} - \frac{29\,632\,c_{\theta}^4\,L_8^r\,M_0^6\,M_K^2\,M_{\pi}^6\,s_{\theta}^6\,\Lambda_2}{729\,M_{\eta}^6\,M_{\eta'}^4} + \\
& \frac{64\,c_{\theta}^4\,L_8^r\,M_0^6\,M_{\pi}^8\,s_{\theta}^6\,\Lambda_2}{243\,M_{\eta}^6\,M_{\eta'}^4} - \frac{2048\,c_{\theta}^2\,L_8^r\,M_0^6\,M_K^4\,M_{\pi}^2\,s_{\theta}^6\,\Lambda_2}{27\,M_{\eta}^4\,M_{\eta'}^4} + \frac{2048\,c_{\theta}^2\,L_8^r\,M_0^6\,M_K^2\,M_{\pi}^4\,s_{\theta}^6\,\Lambda_2}{27\,M_{\eta}^4\,M_{\eta'}^4} - \\
& \frac{256\,c_{\theta}^2\,L_8^r\,M_0^6\,M_{\pi}^6\,s_{\theta}^6\,\Lambda_2}{9\,M_{\eta}^4\,M_{\eta'}^4} - \frac{573\,440\,c_{\theta}^6\,L_8^r\,M_0^8\,M_K^8\,s_{\theta}^6\,\Lambda_2}{729\,M_{\eta}^{10}\,M_{\eta'}^2} + \frac{177\,664\,c_{\theta}^6\,L_8^r\,M_0^8\,M_K^6\,M_{\pi}^2\,s_{\theta}^6\,\Lambda_2}{243\,M_{\eta}^{10}\,M_{\eta'}^2} + \\
& \frac{56\,576\,c_{\theta}^6\,L_8^r\,M_0^8\,M_K^4\,M_{\pi}^4\,s_{\theta}^6\,\Lambda_2}{243\,M_{\eta}^{10}\,M_{\eta'}^2} - \frac{209\,152\,c_{\theta}^6\,L_8^r\,M_0^8\,M_K^2\,M_{\pi}^6\,s_{\theta}^6\,\Lambda_2}{729\,M_{\eta}^{10}\,M_{\eta'}^2} - \frac{4480\,c_{\theta}^6\,L_8^r\,M_0^8\,M_{\pi}^8\,s_{\theta}^6\,\Lambda_2}{243\,M_{\eta}^{10}\,M_{\eta'}^2} - \\
& \frac{512\,c_{\theta}^4\,L_8^r\,M_0^6\,M_K^6\,s_{\theta}^6\,\Lambda_2}{243\,M_{\eta}^8\,M_{\eta'}^2} - \frac{389\,120\,c_{\theta}^4\,L_8^r\,M_0^6\,M_K^8\,s_{\theta}^6\,\Lambda_2}{729\,M_{\eta}^8\,M_{\eta'}^2} - \frac{13\,568\,c_{\theta}^4\,L_8^r\,M_0^8\,M_K^4\,M_{\pi}^2\,s_{\theta}^6\,\Lambda_2}{243\,M_{\eta}^8\,M_{\eta'}^2} + \\
& \frac{213\,760\,c_{\theta}^4\,L_8^r\,M_0^6\,M_K^6\,M_{\pi}^2\,s_{\theta}^6\,\Lambda_2}{243\,M_{\eta}^8\,M_{\eta'}^2} + \frac{16\,384\,c_{\theta}^4\,L_8^r\,M_0^6\,M_K^2\,M_{\pi}^4\,s_{\theta}^6\,\Lambda_2}{243\,M_{\eta}^8\,M_{\eta'}^2} - \frac{38\,144\,c_{\theta}^4\,L_8^r\,M_0^6\,M_K^4\,M_{\pi}^4\,s_{\theta}^6\,\Lambda_2}{81\,M_{\eta}^8\,M_{\eta'}^2} + \\
& \frac{128\,c_{\theta}^4\,L_8^r\,M_0^8\,M_{\pi}^6\,s_{\theta}^6\,\Lambda_2}{27\,M_{\eta}^8\,M_{\eta'}^2} + \frac{94\,016\,c_{\theta}^4\,L_8^r\,M_0^6\,M_K^2\,M_{\pi}^6\,s_{\theta}^6\,\Lambda_2}{729\,M_{\eta}^8\,M_{\eta'}^2} - \frac{896\,c_{\theta}^4\,L_8^r\,M_0^6\,M_{\pi}^8\,s_{\theta}^6\,\Lambda_2}{81\,M_{\eta}^8\,M_{\eta'}^2} + \\
& \frac{20\,480\,c_{\theta}^2\,L_8^r\,M_0^6\,M_K^6\,s_{\theta}^6\,\Lambda_2}{243\,M_{\eta}^6\,M_{\eta'}^2} - \frac{10\,240\,c_{\theta}^2\,L_8^r\,M_0^6\,M_K^4\,M_{\pi}^2\,s_{\theta}^6\,\Lambda_2}{243\,M_{\eta}^6\,M_{\eta'}^2} - \frac{6400\,c_{\theta}^2\,L_8^r\,M_0^6\,M_K^2\,M_{\pi}^4\,s_{\theta}^6\,\Lambda_2}{243\,M_{\eta}^6\,M_{\eta'}^2} + \\
& \frac{1792\,c_{\theta}^2\,L_8^r\,M_0^6\,M_{\pi}^6\,s_{\theta}^6\,\Lambda_2}{81\,M_{\eta}^6\,M_{\eta'}^2} - \frac{143\,360\,\sqrt{2}\,c_{\theta}^5\,L_8^r\,M_0^8\,M_K^8\,s_{\theta}^7\,\Lambda_2}{243\,M_{\eta}^{12}} + \frac{98\,560\,\sqrt{2}\,c_{\theta}^5\,L_8^r\,M_0^8\,M_K^6\,M_{\pi}^2\,s_{\theta}^7\,\Lambda_2}{81\,M_{\eta}^{12}} - \\
& \frac{24\,320\,\sqrt{2}\,c_{\theta}^5\,L_8^r\,M_0^8\,M_K^4\,M_{\pi}^4\,s_{\theta}^7\,\Lambda_2}{27\,M_{\eta}^{12}} + \frac{63\,680\,\sqrt{2}\,c_{\theta}^5\,L_8^r\,M_0^8\,M_K^2\,M_{\pi}^6\,s_{\theta}^7\,\Lambda_2}{243\,M_{\eta}^{12}} - \\
& \frac{320\,\sqrt{2}\,c_{\theta}^5\,L_8^r\,M_0^8\,M_{\pi}^8\,s_{\theta}^7\,\Lambda_2}{27\,M_{\eta}^{12}} + \frac{20\,480\,\sqrt{2}\,c_{\theta}^3\,L_8^r\,M_0^8\,M_K^6\,s_{\theta}^7\,\Lambda_2}{243\,M_{\eta}^{10}} + \frac{143\,360\,\sqrt{2}\,c_{\theta}^3\,L_8^r\,M_0^6\,M_K^8\,s_{\theta}^7\,\Lambda_2}{729\,M_{\eta}^{10}} - \\
& \frac{30\,976\,\sqrt{2}\,c_{\theta}^3\,L_8^r\,M_0^8\,M_K^4\,M_{\pi}^2\,s_{\theta}^7\,\Lambda_2}{243\,M_{\eta}^{10}} - \frac{26\,624\,\sqrt{2}\,c_{\theta}^3\,L_8^r\,M_0^6\,M_K^6\,M_{\pi}^2\,s_{\theta}^7\,\Lambda_2}{81\,M_{\eta}^{10}} + \\
& \frac{14\,336\,\sqrt{2}\,c_{\theta}^3\,L_8^r\,M_0^8\,M_K^2\,M_{\pi}^4\,s_{\theta}^7\,\Lambda_2}{243\,M_{\eta}^{10}} + \frac{5632\,\sqrt{2}\,c_{\theta}^3\,L_8^r\,M_0^6\,M_K^4\,M_{\pi}^4\,s_{\theta}^7\,\Lambda_2}{27\,M_{\eta}^{10}} - \\
& \frac{1088\,\sqrt{2}\,c_{\theta}^3\,L_8^r\,M_0^8\,M_{\pi}^6\,s_{\theta}^7\,\Lambda_2}{81\,M_{\eta}^{10}} - \frac{45\,824\,\sqrt{2}\,c_{\theta}^3\,L_8^r\,M_0^6\,M_K^2\,M_{\pi}^6\,s_{\theta}^7\,\Lambda_2}{729\,M_{\eta}^{10}} - \frac{1024\,\sqrt{2}\,c_{\theta}^3\,L_8^r\,M_0^6\,M_{\pi}^8\,s_{\theta}^7\,\Lambda_2}{243\,M_{\eta}^{10}} - \\
& \frac{5120\,\sqrt{2}\,c_{\theta}\,L_8^r\,M_0^6\,M_K^6\,s_{\theta}^7\,\Lambda_2}{243\,M_{\eta}^8} + \frac{4096\,\sqrt{2}\,c_{\theta}\,L_8^r\,M_0^6\,M_K^4\,M_{\pi}^2\,s_{\theta}^7\,\Lambda_2}{243\,M_{\eta}^8} + \frac{256\,\sqrt{2}\,c_{\theta}\,L_8^r\,M_0^6\,M_K^2\,M_{\pi}^4\,s_{\theta}^7\,\Lambda_2}{243\,M_{\eta}^8} + \\
& \frac{256\,\sqrt{2}\,c_{\theta}\,L_8^r\,M_0^6\,M_{\pi}^6\,s_{\theta}^7\,\Lambda_2}{81\,M_{\eta}^8} + \frac{40\,960\,\sqrt{2}\,c_{\theta}^5\,L_8^r\,M_0^8\,M_K^8\,s_{\theta}^7\,\Lambda_2}{729\,M_{\eta}^{12}} - \frac{33\,280\,\sqrt{2}\,c_{\theta}^5\,L_8^r\,M_0^8\,M_K^6\,M_{\pi}^2\,s_{\theta}^7\,\Lambda_2}{243\,M_{\eta}^{12}} +
\end{aligned}$$

$$\begin{aligned}
& \frac{10\,240\sqrt{2}\,c_{\theta}^5 L_8^r M_0^8 M_K^4 M_{\pi}^4 s_{\theta}^7 \Lambda_2}{81 M_{\eta'}^{12}} - \frac{40\,000\sqrt{2}\,c_{\theta}^5 L_8^r M_0^8 M_K^2 M_{\pi}^6 s_{\theta}^7 \Lambda_2}{729 M_{\eta'}^{12}} + \frac{2240\sqrt{2}\,c_{\theta}^5 L_8^r M_0^8 M_{\pi}^8 s_{\theta}^7 \Lambda_2}{243 M_{\eta'}^{12}} - \\
& \frac{16\,384\sqrt{2}\,c_{\theta}^3 L_8^r M_0^6 M_K^8 s_{\theta}^7 \Lambda_2}{729 M_{\eta'}^{10}} + \frac{13\,312\sqrt{2}\,c_{\theta}^3 L_8^r M_0^6 M_K^2 M_{\pi}^2 s_{\theta}^7 \Lambda_2}{243 M_{\eta'}^{10}} - \frac{4096\sqrt{2}\,c_{\theta}^3 L_8^r M_0^6 M_K^4 M_{\pi}^4 s_{\theta}^7 \Lambda_2}{81 M_{\eta'}^{10}} + \\
& \frac{16\,000\sqrt{2}\,c_{\theta}^3 L_8^r M_0^6 M_K^2 M_{\pi}^6 s_{\theta}^7 \Lambda_2}{729 M_{\eta'}^{10}} - \frac{896\sqrt{2}\,c_{\theta}^3 L_8^r M_0^6 M_{\pi}^8 s_{\theta}^7 \Lambda_2}{243 M_{\eta'}^{10}} + \frac{544\,768\sqrt{2}\,c_{\theta}^5 L_8^r M_0^8 M_K^8 s_{\theta}^7 \Lambda_2}{729 M_{\eta'}^2 M_{\eta'}^{10}} - \\
& \frac{120\,064\sqrt{2}\,c_{\theta}^5 L_8^r M_0^8 M_K^6 M_{\pi}^2 s_{\theta}^7 \Lambda_2}{81 M_{\eta'}^2 M_{\eta'}^{10}} + \frac{246\,016\sqrt{2}\,c_{\theta}^5 L_8^r M_0^8 M_K^4 M_{\pi}^4 s_{\theta}^7 \Lambda_2}{243 M_{\eta'}^2 M_{\eta'}^{10}} - \\
& \frac{161\,152\sqrt{2}\,c_{\theta}^5 L_8^r M_0^8 M_K^2 M_{\pi}^6 s_{\theta}^7 \Lambda_2}{729 M_{\eta'}^2 M_{\eta'}^{10}} - \frac{4480\sqrt{2}\,c_{\theta}^5 L_8^r M_0^8 M_{\pi}^8 s_{\theta}^7 \Lambda_2}{243 M_{\eta'}^2 M_{\eta'}^{10}} - \frac{720\,896\sqrt{2}\,c_{\theta}^5 L_8^r M_0^8 M_K^8 s_{\theta}^7 \Lambda_2}{729 M_{\eta'}^4 M_{\eta'}^8} + \\
& \frac{602\,368\sqrt{2}\,c_{\theta}^5 L_8^r M_0^8 M_K^6 M_{\pi}^2 s_{\theta}^7 \Lambda_2}{243 M_{\eta'}^4 M_{\eta'}^8} - \frac{461\,056\sqrt{2}\,c_{\theta}^5 L_8^r M_0^8 M_K^4 M_{\pi}^4 s_{\theta}^7 \Lambda_2}{243 M_{\eta'}^4 M_{\eta'}^8} + \\
& \frac{264\,896\sqrt{2}\,c_{\theta}^5 L_8^r M_0^8 M_K^2 M_{\pi}^6 s_{\theta}^7 \Lambda_2}{729 M_{\eta'}^4 M_{\eta'}^8} - \frac{4288\sqrt{2}\,c_{\theta}^5 L_8^r M_0^8 M_{\pi}^8 s_{\theta}^7 \Lambda_2}{243 M_{\eta'}^4 M_{\eta'}^8} - \\
& \frac{1024\sqrt{2}\,c_{\theta}^3 L_8^r M_0^8 M_K^6 s_{\theta}^7 \Lambda_2}{81 M_{\eta'}^2 M_{\eta'}^8} - \frac{114\,688\sqrt{2}\,c_{\theta}^3 L_8^r M_0^8 M_K^8 s_{\theta}^7 \Lambda_2}{729 M_{\eta'}^2 M_{\eta'}^8} + \frac{1664\sqrt{2}\,c_{\theta}^3 L_8^r M_0^8 M_K^4 M_{\pi}^2 s_{\theta}^7 \Lambda_2}{81 M_{\eta'}^2 M_{\eta'}^8} + \\
& \frac{79\,232\sqrt{2}\,c_{\theta}^3 L_8^r M_0^6 M_K^6 M_{\pi}^2 s_{\theta}^7 \Lambda_2}{243 M_{\eta'}^2 M_{\eta'}^8} - \frac{1024\sqrt{2}\,c_{\theta}^3 L_8^r M_0^8 M_K^2 M_{\pi}^4 s_{\theta}^7 \Lambda_2}{81 M_{\eta'}^2 M_{\eta'}^8} - \\
& \frac{18\,688\sqrt{2}\,c_{\theta}^3 L_8^r M_0^6 M_K^4 M_{\pi}^4 s_{\theta}^7 \Lambda_2}{81 M_{\eta'}^2 M_{\eta'}^8} + \frac{80\sqrt{2}\,c_{\theta}^3 L_8^r M_0^8 M_{\pi}^6 s_{\theta}^7 \Lambda_2}{27 M_{\eta'}^2 M_{\eta'}^8} + \frac{36\,256\sqrt{2}\,c_{\theta}^3 L_8^r M_0^6 M_K^2 M_{\pi}^6 s_{\theta}^7 \Lambda_2}{729 M_{\eta'}^2 M_{\eta'}^8} + \\
& \frac{416\sqrt{2}\,c_{\theta}^3 L_8^r M_0^6 M_{\pi}^8 s_{\theta}^7 \Lambda_2}{81 M_{\eta'}^2 M_{\eta'}^8} + \frac{477\,184\sqrt{2}\,c_{\theta}^5 L_8^r M_0^8 M_K^8 s_{\theta}^7 \Lambda_2}{729 M_{\eta'}^6 M_{\eta'}^6} - \frac{557\,056\sqrt{2}\,c_{\theta}^5 L_8^r M_0^8 M_K^6 M_{\pi}^2 s_{\theta}^7 \Lambda_2}{243 M_{\eta'}^6 M_{\eta'}^6} + \\
& \frac{159\,232\sqrt{2}\,c_{\theta}^5 L_8^r M_0^8 M_K^4 M_{\pi}^4 s_{\theta}^7 \Lambda_2}{81 M_{\eta'}^6 M_{\eta'}^6} - \frac{238\,336\sqrt{2}\,c_{\theta}^5 L_8^r M_0^8 M_K^2 M_{\pi}^6 s_{\theta}^7 \Lambda_2}{729 M_{\eta'}^6 M_{\eta'}^6} - \\
& \frac{4864\sqrt{2}\,c_{\theta}^5 L_8^r M_0^8 M_{\pi}^8 s_{\theta}^7 \Lambda_2}{243 M_{\eta'}^6 M_{\eta'}^6} - \frac{20\,480\sqrt{2}\,c_{\theta}^3 L_8^r M_0^8 M_K^6 s_{\theta}^7 \Lambda_2}{243 M_{\eta'}^4 M_{\eta'}^6} + \frac{118\,784\sqrt{2}\,c_{\theta}^3 L_8^r M_0^6 M_K^8 s_{\theta}^7 \Lambda_2}{729 M_{\eta'}^4 M_{\eta'}^6} + \\
& \frac{29\,824\sqrt{2}\,c_{\theta}^3 L_8^r M_0^8 M_K^4 M_{\pi}^2 s_{\theta}^7 \Lambda_2}{243 M_{\eta'}^4 M_{\eta'}^6} - \frac{34\,688\sqrt{2}\,c_{\theta}^3 L_8^r M_0^6 M_K^6 M_{\pi}^2 s_{\theta}^7 \Lambda_2}{81 M_{\eta'}^4 M_{\eta'}^6} - \\
& \frac{10\,880\sqrt{2}\,c_{\theta}^3 L_8^r M_0^8 M_K^2 M_{\pi}^4 s_{\theta}^7 \Lambda_2}{243 M_{\eta'}^4 M_{\eta'}^6} + \frac{1024\sqrt{2}\,c_{\theta}^3 L_8^r M_0^6 M_K^4 M_{\pi}^4 s_{\theta}^7 \Lambda_2}{3 M_{\eta'}^4 M_{\eta'}^6} + \frac{752\sqrt{2}\,c_{\theta}^3 L_8^r M_0^8 M_{\pi}^6 s_{\theta}^7 \Lambda_2}{81 M_{\eta'}^4 M_{\eta'}^6} - \\
& \frac{48\,608\sqrt{2}\,c_{\theta}^3 L_8^r M_0^6 M_K^2 M_{\pi}^6 s_{\theta}^7 \Lambda_2}{729 M_{\eta'}^4 M_{\eta'}^6} + \frac{608\sqrt{2}\,c_{\theta}^3 L_8^r M_0^6 M_{\pi}^8 s_{\theta}^7 \Lambda_2}{243 M_{\eta'}^4 M_{\eta'}^6} - \frac{284\,672\sqrt{2}\,c_{\theta}^5 L_8^r M_0^8 M_K^8 s_{\theta}^7 \Lambda_2}{729 M_{\eta'}^8 M_{\eta'}^4} +
\end{aligned}$$

$$\begin{aligned}
& \frac{143\,872\sqrt{2}\,c_\theta^5 L_8^r M_0^8 M_K^6 M_\pi^2 s_\theta^7 \Lambda_2}{81 M_\eta^8 M_{\eta'}^4} - \frac{401\,408\sqrt{2}\,c_\theta^5 L_8^r M_0^8 M_K^4 M_\pi^4 s_\theta^7 \Lambda_2}{243 M_\eta^8 M_{\eta'}^4} + \\
& \frac{229\,952\sqrt{2}\,c_\theta^5 L_8^r M_0^8 M_K^2 M_\pi^6 s_\theta^7 \Lambda_2}{729 M_\eta^8 M_{\eta'}^4} - \frac{448\sqrt{2}\,c_\theta^5 L_8^r M_0^8 M_\pi^8 s_\theta^7 \Lambda_2}{243 M_\eta^8 M_{\eta'}^4} + \frac{31\,744\sqrt{2}\,c_\theta^3 L_8^r M_0^8 M_K^6 s_\theta^7 \Lambda_2}{243 M_\eta^6 M_{\eta'}^4} - \\
& \frac{4096\sqrt{2}\,c_\theta^3 L_8^r M_0^6 M_K^8 s_\theta^7 \Lambda_2}{729 M_\eta^6 M_{\eta'}^4} - \frac{49\,280\sqrt{2}\,c_\theta^3 L_8^r M_0^8 M_K^4 M_\pi^2 s_\theta^7 \Lambda_2}{243 M_\eta^6 M_{\eta'}^4} + \frac{45\,184\sqrt{2}\,c_\theta^3 L_8^r M_0^6 M_K^6 M_\pi^2 s_\theta^7 \Lambda_2}{243 M_\eta^6 M_{\eta'}^4} + \\
& \frac{16\,384\sqrt{2}\,c_\theta^3 L_8^r M_0^8 M_K^2 M_\pi^4 s_\theta^7 \Lambda_2}{243 M_\eta^6 M_{\eta'}^4} - \frac{5888\sqrt{2}\,c_\theta^3 L_8^r M_0^6 M_K^4 M_\pi^4 s_\theta^7 \Lambda_2}{27 M_\eta^6 M_{\eta'}^4} + \frac{176\sqrt{2}\,c_\theta^3 L_8^r M_0^8 M_\pi^6 s_\theta^7 \Lambda_2}{27 M_\eta^6 M_{\eta'}^4} + \\
& \frac{32\,224\sqrt{2}\,c_\theta^3 L_8^r M_0^6 M_K^2 M_\pi^6 s_\theta^7 \Lambda_2}{729 M_\eta^6 M_{\eta'}^4} + \frac{160\sqrt{2}\,c_\theta^3 L_8^r M_0^6 M_\pi^8 s_\theta^7 \Lambda_2}{243 M_\eta^6 M_{\eta'}^4} + \frac{2048\sqrt{2}\,c_\theta L_8^r M_0^6 M_K^6 s_\theta^7 \Lambda_2}{81 M_\eta^4 M_{\eta'}^4} - \\
& \frac{4096\sqrt{2}\,c_\theta L_8^r M_0^6 M_K^4 M_\pi^2 s_\theta^7 \Lambda_2}{81 M_\eta^4 M_{\eta'}^4} + \frac{2816\sqrt{2}\,c_\theta L_8^r M_0^6 M_K^2 M_\pi^4 s_\theta^7 \Lambda_2}{81 M_\eta^4 M_{\eta'}^4} - \frac{256\sqrt{2}\,c_\theta L_8^r M_0^6 M_\pi^6 s_\theta^7 \Lambda_2}{27 M_\eta^4 M_{\eta'}^4} + \\
& \frac{372\,736\sqrt{2}\,c_\theta^5 L_8^r M_0^8 M_K^8 s_\theta^7 \Lambda_2}{729 M_\eta^{10} M_{\eta'}^2} - \frac{379\,136\sqrt{2}\,c_\theta^5 L_8^r M_0^8 M_K^6 M_\pi^2 s_\theta^7 \Lambda_2}{243 M_\eta^{10} M_{\eta'}^2} + \\
& \frac{326\,912\sqrt{2}\,c_\theta^5 L_8^r M_0^8 M_K^4 M_\pi^4 s_\theta^7 \Lambda_2}{243 M_\eta^{10} M_{\eta'}^2} - \frac{246\,400\sqrt{2}\,c_\theta^5 L_8^r M_0^8 M_K^2 M_\pi^6 s_\theta^7 \Lambda_2}{729 M_\eta^{10} M_{\eta'}^2} + \\
& \frac{14\,720\sqrt{2}\,c_\theta^5 L_8^r M_0^8 M_\pi^8 s_\theta^7 \Lambda_2}{243 M_\eta^{10} M_{\eta'}^2} - \frac{28\,672\sqrt{2}\,c_\theta^3 L_8^r M_0^8 M_K^6 s_\theta^7 \Lambda_2}{243 M_\eta^8 M_{\eta'}^2} - \frac{126\,976\sqrt{2}\,c_\theta^3 L_8^r M_0^6 M_K^8 s_\theta^7 \Lambda_2}{729 M_\eta^8 M_{\eta'}^2} + \\
& \frac{45\,440\sqrt{2}\,c_\theta^3 L_8^r M_0^8 M_K^4 M_\pi^2 s_\theta^7 \Lambda_2}{243 M_\eta^8 M_{\eta'}^2} + \frac{46\,208\sqrt{2}\,c_\theta^3 L_8^r M_0^6 M_K^6 M_\pi^2 s_\theta^7 \Lambda_2}{243 M_\eta^8 M_{\eta'}^2} - \\
& \frac{16\,768\sqrt{2}\,c_\theta^3 L_8^r M_0^8 M_K^2 M_\pi^4 s_\theta^7 \Lambda_2}{243 M_\eta^8 M_{\eta'}^2} - \frac{4096\sqrt{2}\,c_\theta^3 L_8^r M_0^6 M_K^4 M_\pi^4 s_\theta^7 \Lambda_2}{81 M_\eta^8 M_{\eta'}^2} - \frac{16\sqrt{2}\,c_\theta^3 L_8^r M_0^8 M_\pi^6 s_\theta^7 \Lambda_2}{3 M_\eta^8 M_{\eta'}^2} + \\
& \frac{9952\sqrt{2}\,c_\theta^3 L_8^r M_0^6 M_K^2 M_\pi^6 s_\theta^7 \Lambda_2}{729 M_\eta^8 M_{\eta'}^2} - \frac{32\sqrt{2}\,c_\theta^3 L_8^r M_0^6 M_\pi^8 s_\theta^7 \Lambda_2}{81 M_\eta^8 M_{\eta'}^2} - \frac{1024\sqrt{2}\,c_\theta L_8^r M_0^6 M_K^6 s_\theta^7 \Lambda_2}{243 M_\eta^6 M_{\eta'}^2} + \\
& \frac{8192\sqrt{2}\,c_\theta L_8^r M_0^6 M_K^4 M_\pi^2 s_\theta^7 \Lambda_2}{243 M_\eta^6 M_{\eta'}^2} - \frac{8704\sqrt{2}\,c_\theta L_8^r M_0^6 M_K^2 M_\pi^4 s_\theta^7 \Lambda_2}{243 M_\eta^6 M_{\eta'}^2} + \frac{512\sqrt{2}\,c_\theta L_8^r M_0^6 M_\pi^6 s_\theta^7 \Lambda_2}{81 M_\eta^6 M_{\eta'}^2} - \\
& \frac{716\,800\,c_\theta^4 L_8^r M_0^8 M_K^8 s_\theta^8 \Lambda_2}{729 M_\eta^{12}} + \frac{436\,480\,c_\theta^4 L_8^r M_0^8 M_K^6 M_\pi^2 s_\theta^8 \Lambda_2}{243 M_\eta^{12}} - \frac{96\,640\,c_\theta^4 L_8^r M_0^8 M_K^4 M_\pi^4 s_\theta^8 \Lambda_2}{81 M_\eta^{12}} + \\
& \frac{272\,320\,c_\theta^4 L_8^r M_0^8 M_K^2 M_\pi^6 s_\theta^8 \Lambda_2}{729 M_\eta^{12}} - \frac{20\,000\,c_\theta^4 L_8^r M_0^8 M_\pi^8 s_\theta^8 \Lambda_2}{243 M_\eta^{12}} + \frac{20\,480\,c_\theta^2 L_8^r M_0^8 M_K^6 s_\theta^8 \Lambda_2}{243 M_\eta^{10}} + \\
& \frac{28\,672\,c_\theta^2 L_8^r M_0^6 M_K^8 s_\theta^8 \Lambda_2}{243 M_\eta^{10}} - \frac{33\,280\,c_\theta^2 L_8^r M_0^6 M_K^4 M_\pi^2 s_\theta^8 \Lambda_2}{243 M_\eta^{10}} - \frac{14\,336\,c_\theta^2 L_8^r M_0^6 M_K^6 M_\pi^2 s_\theta^8 \Lambda_2}{81 M_\eta^{10}} + \\
& \frac{18\,176\,c_\theta^2 L_8^r M_0^8 M_K^2 M_\pi^4 s_\theta^8 \Lambda_2}{243 M_\eta^{10}} + \frac{2560\,c_\theta^2 L_8^r M_0^6 M_K^4 M_\pi^4 s_\theta^8 \Lambda_2}{27 M_\eta^{10}} - \frac{256\,c_\theta^2 L_8^r M_0^8 M_\pi^6 s_\theta^8 \Lambda_2}{81 M_\eta^{10}} -
\end{aligned}$$

$$\begin{aligned}
& \frac{4096 c_{\theta}^2 L_8^r M_0^6 M_K^2 M_{\pi}^6 s_{\theta}^8 \Lambda_2}{243 M_{\eta}^{10}} + \frac{128 c_{\theta}^2 L_8^r M_0^6 M_{\pi}^8 s_{\theta}^8 \Lambda_2}{9 M_{\eta}^{10}} - \frac{1024 L_8^r M_0^6 M_K^6 s_{\theta}^8 \Lambda_2}{243 M_{\eta}^8} + \\
& \frac{512 L_8^r M_0^6 M_K^4 M_{\pi}^2 s_{\theta}^8 \Lambda_2}{243 M_{\eta}^8} - \frac{256 L_8^r M_0^6 M_K^2 M_{\pi}^4 s_{\theta}^8 \Lambda_2}{243 M_{\eta}^8} - \frac{128 L_8^r M_0^6 M_{\pi}^6 s_{\theta}^8 \Lambda_2}{81 M_{\eta}^8} - \frac{286720 c_{\theta}^4 L_8^r M_0^8 M_K^8 s_{\theta}^8 \Lambda_2}{729 M_{\eta}^2 M_{\eta'}^{10}} + \\
& \frac{227840 c_{\theta}^4 L_8^r M_0^8 M_K^6 M_{\pi}^2 s_{\theta}^8 \Lambda_2}{243 M_{\eta}^2 M_{\eta'}^{10}} - \frac{204800 c_{\theta}^4 L_8^r M_0^8 M_K^4 M_{\pi}^4 s_{\theta}^8 \Lambda_2}{243 M_{\eta}^2 M_{\eta'}^{10}} + \frac{246784 c_{\theta}^4 L_8^r M_0^8 M_K^2 M_{\pi}^6 s_{\theta}^8 \Lambda_2}{729 M_{\eta}^2 M_{\eta'}^{10}} - \\
& \frac{13184 c_{\theta}^4 L_8^r M_0^8 M_{\pi}^8 s_{\theta}^8 \Lambda_2}{243 M_{\eta}^2 M_{\eta'}^{10}} - \frac{348160 c_{\theta}^4 L_8^r M_0^8 M_K^8 s_{\theta}^8 \Lambda_2}{729 M_{\eta}^4 M_{\eta'}^8} + \frac{7936 c_{\theta}^4 L_8^r M_0^8 M_K^6 M_{\pi}^2 s_{\theta}^8 \Lambda_2}{27 M_{\eta}^4 M_{\eta'}^8} + \\
& \frac{106112 c_{\theta}^4 L_8^r M_0^8 M_K^4 M_{\pi}^4 s_{\theta}^8 \Lambda_2}{243 M_{\eta}^4 M_{\eta'}^8} - \frac{262976 c_{\theta}^4 L_8^r M_0^8 M_K^2 M_{\pi}^6 s_{\theta}^8 \Lambda_2}{729 M_{\eta}^4 M_{\eta'}^8} + \frac{4576 c_{\theta}^4 L_8^r M_0^8 M_{\pi}^8 s_{\theta}^8 \Lambda_2}{243 M_{\eta}^4 M_{\eta'}^8} + \\
& \frac{16384 c_{\theta}^2 L_8^r M_0^6 M_K^8 s_{\theta}^8 \Lambda_2}{243 M_{\eta}^2 M_{\eta'}^8} - \frac{14080 c_{\theta}^2 L_8^r M_0^6 M_K^6 M_{\pi}^2 s_{\theta}^8 \Lambda_2}{81 M_{\eta}^2 M_{\eta'}^8} + \frac{13312 c_{\theta}^2 L_8^r M_0^6 M_K^4 M_{\pi}^4 s_{\theta}^8 \Lambda_2}{81 M_{\eta}^2 M_{\eta'}^8} - \\
& \frac{16960 c_{\theta}^2 L_8^r M_0^6 M_K^2 M_{\pi}^6 s_{\theta}^8 \Lambda_2}{243 M_{\eta}^2 M_{\eta'}^8} + \frac{320 c_{\theta}^2 L_8^r M_0^6 M_{\pi}^8 s_{\theta}^8 \Lambda_2}{27 M_{\eta}^2 M_{\eta'}^8} + \frac{1101824 c_{\theta}^4 L_8^r M_0^8 M_K^8 s_{\theta}^8 \Lambda_2}{729 M_{\eta}^6 M_{\eta'}^6} - \\
& \frac{548864 c_{\theta}^4 L_8^r M_0^8 M_K^6 M_{\pi}^2 s_{\theta}^8 \Lambda_2}{243 M_{\eta}^6 M_{\eta'}^6} + \frac{68096 c_{\theta}^4 L_8^r M_0^8 M_K^4 M_{\pi}^4 s_{\theta}^8 \Lambda_2}{81 M_{\eta}^6 M_{\eta'}^6} - \frac{64256 c_{\theta}^4 L_8^r M_0^8 M_K^2 M_{\pi}^6 s_{\theta}^8 \Lambda_2}{729 M_{\eta}^6 M_{\eta'}^6} - \\
& \frac{2432 c_{\theta}^4 L_8^r M_0^8 M_{\pi}^8 s_{\theta}^8 \Lambda_2}{243 M_{\eta}^6 M_{\eta'}^6} + \frac{1024 c_{\theta}^2 L_8^r M_0^8 M_K^6 s_{\theta}^8 \Lambda_2}{27 M_{\eta}^4 M_{\eta'}^6} + \frac{8192 c_{\theta}^2 L_8^r M_0^6 M_K^8 s_{\theta}^8 \Lambda_2}{81 M_{\eta}^4 M_{\eta'}^6} - \\
& \frac{1408 c_{\theta}^2 L_8^r M_0^8 M_K^4 M_{\pi}^2 s_{\theta}^8 \Lambda_2}{27 M_{\eta}^4 M_{\eta'}^6} - \frac{10496 c_{\theta}^2 L_8^r M_0^6 M_K^6 M_{\pi}^2 s_{\theta}^8 \Lambda_2}{81 M_{\eta}^4 M_{\eta'}^6} + \frac{640 c_{\theta}^2 L_8^r M_0^8 M_K^2 M_{\pi}^4 s_{\theta}^8 \Lambda_2}{27 M_{\eta}^4 M_{\eta'}^6} + \\
& \frac{512 c_{\theta}^2 L_8^r M_0^6 M_K^4 M_{\pi}^4 s_{\theta}^8 \Lambda_2}{27 M_{\eta}^4 M_{\eta'}^6} - \frac{64 c_{\theta}^2 L_8^r M_0^8 M_{\pi}^6 s_{\theta}^8 \Lambda_2}{27 M_{\eta}^4 M_{\eta'}^6} + \frac{1984 c_{\theta}^2 L_8^r M_0^6 M_K^2 M_{\pi}^6 s_{\theta}^8 \Lambda_2}{81 M_{\eta}^4 M_{\eta'}^6} - \\
& \frac{64 c_{\theta}^2 L_8^r M_0^6 M_{\pi}^8 s_{\theta}^8 \Lambda_2}{81 M_{\eta}^4 M_{\eta'}^6} - \frac{1297408 c_{\theta}^4 L_8^r M_0^8 M_K^8 s_{\theta}^8 \Lambda_2}{729 M_{\eta}^8 M_{\eta'}^4} + \frac{759296 c_{\theta}^4 L_8^r M_0^8 M_K^6 M_{\pi}^2 s_{\theta}^8 \Lambda_2}{243 M_{\eta}^8 M_{\eta'}^4} - \\
& \frac{434432 c_{\theta}^4 L_8^r M_0^8 M_K^4 M_{\pi}^4 s_{\theta}^8 \Lambda_2}{243 M_{\eta}^8 M_{\eta'}^4} + \frac{394624 c_{\theta}^4 L_8^r M_0^8 M_K^2 M_{\pi}^6 s_{\theta}^8 \Lambda_2}{729 M_{\eta}^8 M_{\eta'}^4} - \frac{7808 c_{\theta}^4 L_8^r M_0^8 M_{\pi}^8 s_{\theta}^8 \Lambda_2}{243 M_{\eta}^8 M_{\eta'}^4} + \\
& \frac{6656 c_{\theta}^2 L_8^r M_0^8 M_K^6 s_{\theta}^8 \Lambda_2}{243 M_{\eta}^6 M_{\eta'}^4} - \frac{45056 c_{\theta}^2 L_8^r M_0^6 M_K^8 s_{\theta}^8 \Lambda_2}{243 M_{\eta}^6 M_{\eta'}^4} - \frac{17152 c_{\theta}^2 L_8^r M_0^8 M_K^4 M_{\pi}^2 s_{\theta}^8 \Lambda_2}{243 M_{\eta}^6 M_{\eta'}^4} + \\
& \frac{3328 c_{\theta}^2 L_8^r M_0^6 M_K^6 M_{\pi}^2 s_{\theta}^8 \Lambda_2}{9 M_{\eta}^6 M_{\eta'}^4} + \frac{11264 c_{\theta}^2 L_8^r M_0^8 M_K^2 M_{\pi}^4 s_{\theta}^8 \Lambda_2}{243 M_{\eta}^6 M_{\eta'}^4} - \frac{256 c_{\theta}^2 L_8^r M_0^6 M_K^4 M_{\pi}^4 s_{\theta}^8 \Lambda_2}{M_{\eta}^6 M_{\eta'}^4} + \\
& \frac{128 c_{\theta}^2 L_8^r M_0^8 M_{\pi}^6 s_{\theta}^8 \Lambda_2}{81 M_{\eta}^6 M_{\eta'}^4} + \frac{19520 c_{\theta}^2 L_8^r M_0^6 M_K^2 M_{\pi}^6 s_{\theta}^8 \Lambda_2}{243 M_{\eta}^6 M_{\eta'}^4} - \frac{320 c_{\theta}^2 L_8^r M_0^6 M_{\pi}^8 s_{\theta}^8 \Lambda_2}{81 M_{\eta}^6 M_{\eta'}^4} + \\
& \frac{1132544 c_{\theta}^4 L_8^r M_0^8 M_K^8 s_{\theta}^8 \Lambda_2}{729 M_{\eta}^{10} M_{\eta'}^2} - \frac{236032 c_{\theta}^4 L_8^r M_0^8 M_K^6 M_{\pi}^2 s_{\theta}^8 \Lambda_2}{81 M_{\eta}^{10} M_{\eta'}^2} + \frac{461312 c_{\theta}^4 L_8^r M_0^8 M_K^4 M_{\pi}^4 s_{\theta}^8 \Lambda_2}{243 M_{\eta}^{10} M_{\eta'}^2} -
\end{aligned}$$

$$\begin{aligned}
& \frac{471\,296\,c_{\theta}^4\,L_8^r\,M_0^8\,M_K^2\,M_{\pi}^6\,s_{\theta}^8\,\Lambda_2}{729\,M_{\eta}^{10}\,M_{\eta'}^2} + \frac{14\,848\,c_{\theta}^4\,L_8^r\,M_0^8\,M_{\pi}^8\,s_{\theta}^8\,\Lambda_2}{243\,M_{\eta}^{10}\,M_{\eta'}^2} - \frac{23\,552\,c_{\theta}^2\,L_8^r\,M_0^8\,M_K^6\,s_{\theta}^8\,\Lambda_2}{243\,M_{\eta}^8\,M_{\eta'}^2} + \\
& \frac{2048\,c_{\theta}^2\,L_8^r\,M_0^6\,M_K^8\,s_{\theta}^8\,\Lambda_2}{81\,M_{\eta}^8\,M_{\eta'}^2} + \frac{45\,184\,c_{\theta}^2\,L_8^r\,M_0^8\,M_K^4\,M_{\pi}^2\,s_{\theta}^8\,\Lambda_2}{243\,M_{\eta}^8\,M_{\eta'}^2} - \frac{1280\,c_{\theta}^2\,L_8^r\,M_0^6\,M_K^6\,M_{\pi}^2\,s_{\theta}^8\,\Lambda_2}{9\,M_{\eta}^8\,M_{\eta'}^2} - \\
& \frac{26\,240\,c_{\theta}^2\,L_8^r\,M_0^8\,M_K^2\,M_{\pi}^4\,s_{\theta}^8\,\Lambda_2}{243\,M_{\eta}^8\,M_{\eta'}^2} + \frac{13\,568\,c_{\theta}^2\,L_8^r\,M_0^6\,M_K^4\,M_{\pi}^4\,s_{\theta}^8\,\Lambda_2}{81\,M_{\eta}^8\,M_{\eta'}^2} + \frac{320\,c_{\theta}^2\,L_8^r\,M_0^8\,M_{\pi}^6\,s_{\theta}^8\,\Lambda_2}{27\,M_{\eta}^8\,M_{\eta'}^2} - \\
& \frac{6592\,c_{\theta}^2\,L_8^r\,M_0^6\,M_K^2\,M_{\pi}^6\,s_{\theta}^8\,\Lambda_2}{81\,M_{\eta}^8\,M_{\eta'}^2} + \frac{64\,c_{\theta}^2\,L_8^r\,M_0^6\,M_{\pi}^8\,s_{\theta}^8\,\Lambda_2}{27\,M_{\eta}^8\,M_{\eta'}^2} - \frac{2048\,L_8^r\,M_0^6\,M_K^6\,s_{\theta}^8\,\Lambda_2}{243\,M_{\eta}^6\,M_{\eta'}^2} + \frac{4096\,L_8^r\,M_0^6\,M_K^4\,M_{\pi}^2\,s_{\theta}^8\,\Lambda_2}{243\,M_{\eta}^6\,M_{\eta'}^2} - \\
& \frac{2048\,L_8^r\,M_0^6\,M_K^2\,M_{\pi}^4\,s_{\theta}^8\,\Lambda_2}{243\,M_{\eta}^6\,M_{\eta'}^2} - \frac{358\,400\,\sqrt{2}\,c_{\theta}^3\,L_8^r\,M_0^8\,M_K^8\,s_{\theta}^9\,\Lambda_2}{729\,M_{\eta}^{12}} + \frac{66\,560\,\sqrt{2}\,c_{\theta}^3\,L_8^r\,M_0^8\,M_K^6\,M_{\pi}^2\,s_{\theta}^9\,\Lambda_2}{81\,M_{\eta}^{12}} - \\
& \frac{14\,080\,\sqrt{2}\,c_{\theta}^3\,L_8^r\,M_0^8\,M_K^4\,M_{\pi}^4\,s_{\theta}^9\,\Lambda_2}{27\,M_{\eta}^{12}} + \frac{114\,560\,\sqrt{2}\,c_{\theta}^3\,L_8^r\,M_0^8\,M_K^2\,M_{\pi}^6\,s_{\theta}^9\,\Lambda_2}{729\,M_{\eta}^{12}} + \\
& \frac{2560\,\sqrt{2}\,c_{\theta}^3\,L_8^r\,M_0^8\,M_{\pi}^8\,s_{\theta}^9\,\Lambda_2}{243\,M_{\eta}^{12}} + \frac{5120\,\sqrt{2}\,c_{\theta}\,L_8^r\,M_0^8\,M_K^6\,s_{\theta}^9\,\Lambda_2}{243\,M_{\eta}^{10}} + \frac{14\,336\,\sqrt{2}\,c_{\theta}\,L_8^r\,M_0^6\,M_K^8\,s_{\theta}^9\,\Lambda_2}{729\,M_{\eta}^{10}} - \\
& \frac{7168\,\sqrt{2}\,c_{\theta}\,L_8^r\,M_0^8\,M_K^4\,M_{\pi}^2\,s_{\theta}^9\,\Lambda_2}{243\,M_{\eta}^{10}} - \frac{5120\,\sqrt{2}\,c_{\theta}\,L_8^r\,M_0^6\,M_K^6\,M_{\pi}^2\,s_{\theta}^9\,\Lambda_2}{243\,M_{\eta}^{10}} + \frac{4352\,\sqrt{2}\,c_{\theta}\,L_8^r\,M_0^8\,M_K^2\,M_{\pi}^4\,s_{\theta}^9\,\Lambda_2}{243\,M_{\eta}^{10}} + \\
& \frac{512\,\sqrt{2}\,c_{\theta}\,L_8^r\,M_0^6\,M_K^4\,M_{\pi}^4\,s_{\theta}^9\,\Lambda_2}{81\,M_{\eta}^{10}} - \frac{256\,\sqrt{2}\,c_{\theta}\,L_8^r\,M_0^8\,M_{\pi}^6\,s_{\theta}^9\,\Lambda_2}{27\,M_{\eta}^{10}} + \frac{256\,\sqrt{2}\,c_{\theta}\,L_8^r\,M_0^6\,M_K^2\,M_{\pi}^6\,s_{\theta}^9\,\Lambda_2}{729\,M_{\eta}^{10}} - \\
& \frac{1280\,\sqrt{2}\,c_{\theta}\,L_8^r\,M_0^6\,M_{\pi}^8\,s_{\theta}^9\,\Lambda_2}{243\,M_{\eta}^{10}} + \frac{16\,384\,\sqrt{2}\,c_{\theta}^3\,L_8^r\,M_0^8\,M_K^8\,s_{\theta}^9\,\Lambda_2}{729\,M_{\eta}^2\,M_{\eta'}^{10}} - \frac{13\,312\,\sqrt{2}\,c_{\theta}^3\,L_8^r\,M_0^8\,M_K^6\,M_{\pi}^2\,s_{\theta}^9\,\Lambda_2}{243\,M_{\eta}^2\,M_{\eta'}^{10}} + \\
& \frac{4096\,\sqrt{2}\,c_{\theta}^3\,L_8^r\,M_0^8\,M_K^4\,M_{\pi}^4\,s_{\theta}^9\,\Lambda_2}{81\,M_{\eta}^2\,M_{\eta'}^{10}} - \frac{16\,000\,\sqrt{2}\,c_{\theta}^3\,L_8^r\,M_0^6\,M_K^2\,M_{\pi}^6\,s_{\theta}^9\,\Lambda_2}{729\,M_{\eta}^2\,M_{\eta'}^{10}} + \frac{896\,\sqrt{2}\,c_{\theta}^3\,L_8^r\,M_0^8\,M_{\pi}^8\,s_{\theta}^9\,\Lambda_2}{243\,M_{\eta}^2\,M_{\eta'}^{10}} + \\
& \frac{262\,144\,\sqrt{2}\,c_{\theta}^3\,L_8^r\,M_0^8\,M_K^8\,s_{\theta}^9\,\Lambda_2}{729\,M_{\eta}^4\,M_{\eta'}^8} - \frac{20\,480\,\sqrt{2}\,c_{\theta}^3\,L_8^r\,M_0^8\,M_K^6\,M_{\pi}^2\,s_{\theta}^9\,\Lambda_2}{27\,M_{\eta}^4\,M_{\eta'}^8} + \\
& \frac{136\,192\,\sqrt{2}\,c_{\theta}^3\,L_8^r\,M_0^8\,M_K^4\,M_{\pi}^4\,s_{\theta}^9\,\Lambda_2}{243\,M_{\eta}^4\,M_{\eta'}^8} - \frac{106\,624\,\sqrt{2}\,c_{\theta}^3\,L_8^r\,M_0^8\,M_K^2\,M_{\pi}^6\,s_{\theta}^9\,\Lambda_2}{729\,M_{\eta}^4\,M_{\eta'}^8} - \\
& \frac{256\,\sqrt{2}\,c_{\theta}^3\,L_8^r\,M_0^8\,M_{\pi}^8\,s_{\theta}^9\,\Lambda_2}{243\,M_{\eta}^4\,M_{\eta'}^8} - \frac{163\,840\,\sqrt{2}\,c_{\theta}^3\,L_8^r\,M_0^8\,M_K^8\,s_{\theta}^9\,\Lambda_2}{729\,M_{\eta}^6\,M_{\eta'}^6} + \frac{59\,392\,\sqrt{2}\,c_{\theta}^3\,L_8^r\,M_0^8\,M_K^6\,M_{\pi}^2\,s_{\theta}^9\,\Lambda_2}{81\,M_{\eta}^6\,M_{\eta'}^6} - \\
& \frac{52\,736\,\sqrt{2}\,c_{\theta}^3\,L_8^r\,M_0^8\,M_K^4\,M_{\pi}^4\,s_{\theta}^9\,\Lambda_2}{81\,M_{\eta}^6\,M_{\eta'}^6} + \frac{103\,552\,\sqrt{2}\,c_{\theta}^3\,L_8^r\,M_0^8\,M_K^2\,M_{\pi}^6\,s_{\theta}^9\,\Lambda_2}{729\,M_{\eta}^6\,M_{\eta'}^6} - \\
& \frac{4480\,\sqrt{2}\,c_{\theta}^3\,L_8^r\,M_0^8\,M_{\pi}^8\,s_{\theta}^9\,\Lambda_2}{243\,M_{\eta}^6\,M_{\eta'}^6} - \frac{8192\,\sqrt{2}\,c_{\theta}\,L_8^r\,M_0^6\,M_K^8\,s_{\theta}^9\,\Lambda_2}{243\,M_{\eta}^4\,M_{\eta'}^6} + \frac{6656\,\sqrt{2}\,c_{\theta}\,L_8^r\,M_0^6\,M_K^6\,M_{\pi}^2\,s_{\theta}^9\,\Lambda_2}{81\,M_{\eta}^4\,M_{\eta'}^6} - \\
& \frac{5632\,\sqrt{2}\,c_{\theta}\,L_8^r\,M_0^6\,M_K^4\,M_{\pi}^4\,s_{\theta}^9\,\Lambda_2}{81\,M_{\eta}^4\,M_{\eta'}^6} + \frac{5504\,\sqrt{2}\,c_{\theta}\,L_8^r\,M_0^6\,M_K^2\,M_{\pi}^6\,s_{\theta}^9\,\Lambda_2}{243\,M_{\eta}^4\,M_{\eta'}^6} - \frac{128\,\sqrt{2}\,c_{\theta}\,L_8^r\,M_0^8\,M_{\pi}^8\,s_{\theta}^9\,\Lambda_2}{81\,M_{\eta}^4\,M_{\eta'}^6} -
\end{aligned}$$

$$\begin{aligned}
& \frac{222\,208\sqrt{2}\,c_\theta^3 L_8^r M_0^8 M_K^8 S_\theta^9 \Lambda_2}{729 M_\eta^8 M_{\eta'}^4} + \frac{60\,416\sqrt{2}\,c_\theta^3 L_8^r M_0^8 M_K^6 M_\pi^2 S_\theta^9 \Lambda_2}{243 M_\eta^8 M_{\eta'}^4} - \\
& \frac{4352\sqrt{2}\,c_\theta^3 L_8^r M_0^8 M_K^4 M_\pi^4 S_\theta^9 \Lambda_2}{243 M_\eta^8 M_{\eta'}^4} + \frac{47\,488\sqrt{2}\,c_\theta^3 L_8^r M_0^8 M_K^6 M_\pi^6 S_\theta^9 \Lambda_2}{729 M_\eta^8 M_{\eta'}^4} - \frac{4736\sqrt{2}\,c_\theta^3 L_8^r M_0^8 M_\pi^8 S_\theta^9 \Lambda_2}{243 M_\eta^8 M_{\eta'}^4} - \\
& \frac{512\sqrt{2}\,c_\theta L_8^r M_0^8 M_K^6 S_\theta^9 \Lambda_2}{27 M_\eta^6 M_{\eta'}^4} - \frac{16\,384\sqrt{2}\,c_\theta L_8^r M_0^6 M_K^8 S_\theta^9 \Lambda_2}{729 M_\eta^6 M_{\eta'}^4} + \frac{256\sqrt{2}\,c_\theta L_8^r M_0^8 M_K^4 M_\pi^2 S_\theta^9 \Lambda_2}{9 M_\eta^6 M_{\eta'}^4} + \\
& \frac{256\sqrt{2}\,c_\theta L_8^r M_0^6 M_K^6 M_\pi^2 S_\theta^9 \Lambda_2}{9 M_\eta^6 M_{\eta'}^4} - \frac{320\sqrt{2}\,c_\theta L_8^r M_0^8 M_K^2 M_\pi^4 S_\theta^9 \Lambda_2}{27 M_\eta^6 M_{\eta'}^4} - \frac{128\sqrt{2}\,c_\theta L_8^r M_0^6 M_K^4 M_\pi^4 S_\theta^9 \Lambda_2}{9 M_\eta^6 M_{\eta'}^4} + \\
& \frac{64\sqrt{2}\,c_\theta L_8^r M_0^8 M_\pi^6 S_\theta^9 \Lambda_2}{27 M_\eta^6 M_{\eta'}^4} + \frac{5632\sqrt{2}\,c_\theta L_8^r M_0^6 M_K^2 M_\pi^6 S_\theta^9 \Lambda_2}{729 M_\eta^6 M_{\eta'}^4} + \frac{128\sqrt{2}\,c_\theta L_8^r M_0^8 M_\pi^8 S_\theta^9 \Lambda_2}{243 M_\eta^6 M_{\eta'}^4} + \\
& \frac{465\,920\sqrt{2}\,c_\theta^3 L_8^r M_0^8 M_K^8 S_\theta^9 \Lambda_2}{729 M_\eta^{10} M_{\eta'}^2} - \frac{240\,640\sqrt{2}\,c_\theta^3 L_8^r M_0^8 M_K^6 M_\pi^2 S_\theta^9 \Lambda_2}{243 M_\eta^{10} M_{\eta'}^2} + \\
& \frac{140\,800\sqrt{2}\,c_\theta^3 L_8^r M_0^8 M_K^4 M_\pi^4 S_\theta^9 \Lambda_2}{243 M_\eta^{10} M_{\eta'}^2} - \frac{142\,976\sqrt{2}\,c_\theta^3 L_8^r M_0^8 M_K^2 M_\pi^6 S_\theta^9 \Lambda_2}{729 M_\eta^{10} M_{\eta'}^2} + \\
& \frac{6016\sqrt{2}\,c_\theta^3 L_8^r M_0^8 M_\pi^8 S_\theta^9 \Lambda_2}{243 M_\eta^{10} M_{\eta'}^2} - \frac{512\sqrt{2}\,c_\theta L_8^r M_0^8 M_K^6 S_\theta^9 \Lambda_2}{243 M_\eta^8 M_{\eta'}^2} + \frac{26\,624\sqrt{2}\,c_\theta L_8^r M_0^6 M_K^8 S_\theta^9 \Lambda_2}{729 M_\eta^8 M_{\eta'}^2} + \\
& \frac{256\sqrt{2}\,c_\theta L_8^r M_0^8 M_K^4 M_\pi^2 S_\theta^9 \Lambda_2}{243 M_\eta^8 M_{\eta'}^2} - \frac{21\,760\sqrt{2}\,c_\theta L_8^r M_0^6 M_K^6 M_\pi^2 S_\theta^9 \Lambda_2}{243 M_\eta^8 M_{\eta'}^2} - \frac{1472\sqrt{2}\,c_\theta L_8^r M_0^8 M_K^2 M_\pi^4 S_\theta^9 \Lambda_2}{243 M_\eta^8 M_{\eta'}^2} + \\
& \frac{6272\sqrt{2}\,c_\theta L_8^r M_0^6 M_K^4 M_\pi^4 S_\theta^9 \Lambda_2}{81 M_\eta^8 M_{\eta'}^2} + \frac{64\sqrt{2}\,c_\theta L_8^r M_0^8 M_\pi^6 S_\theta^9 \Lambda_2}{9 M_\eta^8 M_{\eta'}^2} - \frac{22\,400\sqrt{2}\,c_\theta L_8^r M_0^6 M_K^2 M_\pi^6 S_\theta^9 \Lambda_2}{729 M_\eta^8 M_{\eta'}^2} + \\
& \frac{512\sqrt{2}\,c_\theta L_8^r M_0^8 M_\pi^8 S_\theta^9 \Lambda_2}{81 M_\eta^8 M_{\eta'}^2} - \frac{71\,680 c_\theta^2 L_8^r M_0^8 M_K^8 S_\theta^{10} \Lambda_2}{243 M_\eta^{12}} + \frac{35\,840 c_\theta^2 L_8^r M_0^8 M_K^6 M_\pi^2 S_\theta^{10} \Lambda_2}{81 M_\eta^{12}} - \\
& \frac{6400 c_\theta^2 L_8^r M_0^8 M_K^4 M_\pi^4 S_\theta^{10} \Lambda_2}{27 M_\eta^{12}} + \frac{10\,240 c_\theta^2 L_8^r M_0^8 M_K^2 M_\pi^6 S_\theta^{10} \Lambda_2}{243 M_\eta^{12}} - \frac{320 c_\theta^2 L_8^r M_0^8 M_\pi^8 S_\theta^{10} \Lambda_2}{9 M_\eta^{12}} + \\
& \frac{1024 L_8^r M_0^8 M_K^6 S_\theta^{10} \Lambda_2}{243 M_\eta^{10}} + \frac{2048 L_8^r M_0^6 M_K^8 S_\theta^{10} \Lambda_2}{729 M_\eta^{10}} - \frac{512 L_8^r M_0^8 M_K^4 M_\pi^2 S_\theta^{10} \Lambda_2}{243 M_\eta^{10}} + \frac{256 L_8^r M_0^8 M_K^2 M_\pi^4 S_\theta^{10} \Lambda_2}{243 M_\eta^{10}} + \\
& \frac{128 L_8^r M_0^8 M_\pi^6 S_\theta^{10} \Lambda_2}{81 M_\eta^{10}} + \frac{1024 L_8^r M_0^6 M_K^2 M_\pi^6 S_\theta^{10} \Lambda_2}{729 M_\eta^{10}} + \frac{128 L_8^r M_0^6 M_\pi^8 S_\theta^{10} \Lambda_2}{243 M_\eta^{10}} - \frac{16\,384 c_\theta^2 L_8^r M_0^8 M_K^8 S_\theta^{10} \Lambda_2}{243 M_\eta^4 M_{\eta'}^8} + \\
& \frac{14\,080 c_\theta^2 L_8^r M_0^8 M_K^6 M_\pi^2 S_\theta^{10} \Lambda_2}{81 M_\eta^4 M_{\eta'}^8} - \frac{13\,312 c_\theta^2 L_8^r M_0^8 M_K^4 M_\pi^4 S_\theta^{10} \Lambda_2}{81 M_\eta^4 M_{\eta'}^8} + \frac{16\,960 c_\theta^2 L_8^r M_0^8 M_K^2 M_\pi^6 S_\theta^{10} \Lambda_2}{243 M_\eta^4 M_{\eta'}^8} - \\
& \frac{320 c_\theta^2 L_8^r M_0^8 M_\pi^8 S_\theta^{10} \Lambda_2}{27 M_\eta^4 M_{\eta'}^8} - \frac{204\,800 c_\theta^2 L_8^r M_0^8 M_K^8 S_\theta^{10} \Lambda_2}{729 M_\eta^6 M_{\eta'}^6} + \frac{114\,176 c_\theta^2 L_8^r M_0^8 M_K^6 M_\pi^2 S_\theta^{10} \Lambda_2}{243 M_\eta^6 M_{\eta'}^6} - \\
& \frac{6656 c_\theta^2 L_8^r M_0^8 M_K^4 M_\pi^4 S_\theta^{10} \Lambda_2}{27 M_\eta^6 M_{\eta'}^6} + \frac{30\,080 c_\theta^2 L_8^r M_0^8 M_K^2 M_\pi^6 S_\theta^{10} \Lambda_2}{729 M_\eta^6 M_{\eta'}^6} - \frac{2944 c_\theta^2 L_8^r M_0^8 M_\pi^8 S_\theta^{10} \Lambda_2}{243 M_\eta^6 M_{\eta'}^6} +
\end{aligned}$$

$$\begin{aligned}
& \frac{219\,136\,c_\theta^2\,L_8^r\,M_0^8\,M_K^8\,s_\theta^{10}\,\Lambda_2}{729\,M_\eta^8\,M_{\eta'}^4} - \frac{52\,480\,c_\theta^2\,L_8^r\,M_0^8\,M_K^6\,M_\pi^2\,s_\theta^{10}\,\Lambda_2}{81\,M_\eta^8\,M_{\eta'}^4} + \frac{118\,528\,c_\theta^2\,L_8^r\,M_0^8\,M_K^4\,M_\pi^4\,s_\theta^{10}\,\Lambda_2}{243\,M_\eta^8\,M_{\eta'}^4} - \\
& \frac{120\,640\,c_\theta^2\,L_8^r\,M_0^8\,M_K^2\,M_\pi^6\,s_\theta^{10}\,\Lambda_2}{729\,M_\eta^8\,M_{\eta'}^4} - \frac{256\,c_\theta^2\,L_8^r\,M_0^8\,M_\pi^8\,s_\theta^{10}\,\Lambda_2}{243\,M_\eta^8\,M_{\eta'}^4} + \frac{8192\,L_8^r\,M_0^6\,M_K^8\,s_\theta^{10}\,\Lambda_2}{729\,M_\eta^6\,M_{\eta'}^4} - \\
& \frac{6656\,L_8^r\,M_0^6\,M_K^6\,M_\pi^2\,s_\theta^{10}\,\Lambda_2}{243\,M_\eta^6\,M_{\eta'}^4} + \frac{1792\,L_8^r\,M_0^6\,M_K^4\,M_\pi^4\,s_\theta^{10}\,\Lambda_2}{81\,M_\eta^6\,M_{\eta'}^4} - \frac{5120\,L_8^r\,M_0^6\,M_K^2\,M_\pi^6\,s_\theta^{10}\,\Lambda_2}{729\,M_\eta^6\,M_{\eta'}^4} + \\
& \frac{256\,L_8^r\,M_0^6\,M_\pi^8\,s_\theta^{10}\,\Lambda_2}{243\,M_\eta^6\,M_{\eta'}^4} + \frac{83\,968\,c_\theta^2\,L_8^r\,M_0^8\,M_K^8\,s_\theta^{10}\,\Lambda_2}{729\,M_\eta^{10}\,M_{\eta'}^2} - \frac{11\,264\,c_\theta^2\,L_8^r\,M_0^8\,M_K^6\,M_\pi^2\,s_\theta^{10}\,\Lambda_2}{243\,M_\eta^{10}\,M_{\eta'}^2} - \\
& \frac{24\,064\,c_\theta^2\,L_8^r\,M_0^8\,M_K^4\,M_\pi^4\,s_\theta^{10}\,\Lambda_2}{243\,M_\eta^{10}\,M_{\eta'}^2} + \frac{55\,040\,c_\theta^2\,L_8^r\,M_0^8\,M_K^2\,M_\pi^6\,s_\theta^{10}\,\Lambda_2}{729\,M_\eta^{10}\,M_{\eta'}^2} + \frac{5120\,c_\theta^2\,L_8^r\,M_0^8\,M_\pi^8\,s_\theta^{10}\,\Lambda_2}{243\,M_\eta^{10}\,M_{\eta'}^2} + \\
& \frac{512\,L_8^r\,M_0^8\,M_K^6\,s_\theta^{10}\,\Lambda_2}{81\,M_\eta^8\,M_{\eta'}^2} + \frac{8192\,L_8^r\,M_0^6\,M_K^8\,s_\theta^{10}\,\Lambda_2}{729\,M_\eta^8\,M_{\eta'}^2} - \frac{1024\,L_8^r\,M_0^8\,M_K^4\,M_\pi^2\,s_\theta^{10}\,\Lambda_2}{81\,M_\eta^8\,M_{\eta'}^2} - \frac{5632\,L_8^r\,M_0^6\,M_K^6\,M_\pi^2\,s_\theta^{10}\,\Lambda_2}{243\,M_\eta^8\,M_{\eta'}^2} + \\
& \frac{512\,L_8^r\,M_0^8\,M_K^2\,M_\pi^4\,s_\theta^{10}\,\Lambda_2}{81\,M_\eta^8\,M_{\eta'}^2} + \frac{1280\,L_8^r\,M_0^6\,M_K^4\,M_\pi^4\,s_\theta^{10}\,\Lambda_2}{81\,M_\eta^8\,M_{\eta'}^2} - \frac{5120\,L_8^r\,M_0^6\,M_K^2\,M_\pi^6\,s_\theta^{10}\,\Lambda_2}{729\,M_\eta^8\,M_{\eta'}^2} + \\
& \frac{256\,L_8^r\,M_0^6\,M_\pi^8\,s_\theta^{10}\,\Lambda_2}{81\,M_\eta^8\,M_{\eta'}^2} - \frac{35\,840\,\sqrt{2}\,c_\theta\,L_8^r\,M_0^8\,M_K^8\,s_\theta^{11}\,\Lambda_2}{729\,M_\eta^{12}} + \frac{12\,800\,\sqrt{2}\,c_\theta\,L_8^r\,M_0^8\,M_K^6\,M_\pi^2\,s_\theta^{11}\,\Lambda_2}{243\,M_\eta^{12}} - \\
& \frac{1280\,\sqrt{2}\,c_\theta\,L_8^r\,M_0^8\,M_K^4\,M_\pi^4\,s_\theta^{11}\,\Lambda_2}{81\,M_\eta^{12}} - \frac{640\,\sqrt{2}\,c_\theta\,L_8^r\,M_0^8\,M_K^2\,M_\pi^6\,s_\theta^{11}\,\Lambda_2}{729\,M_\eta^{12}} + \frac{3200\,\sqrt{2}\,c_\theta\,L_8^r\,M_0^8\,M_\pi^8\,s_\theta^{11}\,\Lambda_2}{243\,M_\eta^{12}} + \\
& \frac{8192\,\sqrt{2}\,c_\theta\,L_8^r\,M_0^8\,M_K^8\,s_\theta^{11}\,\Lambda_2}{243\,M_\eta^6\,M_{\eta'}^6} - \frac{6656\,\sqrt{2}\,c_\theta\,L_8^r\,M_0^8\,M_K^6\,M_\pi^2\,s_\theta^{11}\,\Lambda_2}{81\,M_\eta^6\,M_{\eta'}^6} + \frac{5632\,\sqrt{2}\,c_\theta\,L_8^r\,M_0^8\,M_K^4\,M_\pi^4\,s_\theta^{11}\,\Lambda_2}{81\,M_\eta^6\,M_{\eta'}^6} - \\
& \frac{5504\,\sqrt{2}\,c_\theta\,L_8^r\,M_0^8\,M_K^2\,M_\pi^6\,s_\theta^{11}\,\Lambda_2}{243\,M_\eta^6\,M_{\eta'}^6} + \frac{128\,\sqrt{2}\,c_\theta\,L_8^r\,M_0^8\,M_\pi^8\,s_\theta^{11}\,\Lambda_2}{81\,M_\eta^6\,M_{\eta'}^6} + \frac{47\,104\,\sqrt{2}\,c_\theta\,L_8^r\,M_0^8\,M_K^8\,s_\theta^{11}\,\Lambda_2}{729\,M_\eta^8\,M_{\eta'}^4} - \\
& \frac{25\,088\,\sqrt{2}\,c_\theta\,L_8^r\,M_0^8\,M_K^6\,M_\pi^2\,s_\theta^{11}\,\Lambda_2}{243\,M_\eta^8\,M_{\eta'}^4} + \frac{15\,104\,\sqrt{2}\,c_\theta\,L_8^r\,M_0^8\,M_K^4\,M_\pi^4\,s_\theta^{11}\,\Lambda_2}{243\,M_\eta^8\,M_{\eta'}^4} - \\
& \frac{16\,384\,\sqrt{2}\,c_\theta\,L_8^r\,M_0^8\,M_K^2\,M_\pi^6\,s_\theta^{11}\,\Lambda_2}{729\,M_\eta^8\,M_{\eta'}^4} - \frac{256\,\sqrt{2}\,c_\theta\,L_8^r\,M_0^8\,M_\pi^8\,s_\theta^{11}\,\Lambda_2}{243\,M_\eta^8\,M_{\eta'}^4} - \frac{35\,840\,\sqrt{2}\,c_\theta\,L_8^r\,M_0^8\,M_K^8\,s_\theta^{11}\,\Lambda_2}{729\,M_\eta^{10}\,M_{\eta'}^2} + \\
& \frac{3584\,\sqrt{2}\,c_\theta\,L_8^r\,M_0^8\,M_K^6\,M_\pi^2\,s_\theta^{11}\,\Lambda_2}{27\,M_\eta^{10}\,M_{\eta'}^2} - \frac{28\,160\,\sqrt{2}\,c_\theta\,L_8^r\,M_0^8\,M_K^4\,M_\pi^4\,s_\theta^{11}\,\Lambda_2}{243\,M_\eta^{10}\,M_{\eta'}^2} + \\
& \frac{33\,536\,\sqrt{2}\,c_\theta\,L_8^r\,M_0^8\,M_K^2\,M_\pi^6\,s_\theta^{11}\,\Lambda_2}{729\,M_\eta^{10}\,M_{\eta'}^2} - \frac{3328\,\sqrt{2}\,c_\theta\,L_8^r\,M_0^8\,M_\pi^8\,s_\theta^{11}\,\Lambda_2}{243\,M_\eta^{10}\,M_{\eta'}^2} - \frac{5120\,L_8^r\,M_0^8\,M_K^8\,s_\theta^{12}\,\Lambda_2}{729\,M_\eta^{12}} - \\
& \frac{2560\,L_8^r\,M_0^8\,M_K^2\,M_\pi^6\,s_\theta^{12}\,\Lambda_2}{729\,M_\eta^{12}} - \frac{320\,L_8^r\,M_0^8\,M_\pi^8\,s_\theta^{12}\,\Lambda_2}{243\,M_\eta^{12}} - \frac{8192\,L_8^r\,M_0^8\,M_K^8\,s_\theta^{12}\,\Lambda_2}{729\,M_\eta^8\,M_{\eta'}^4} + \\
& \frac{6656\,L_8^r\,M_0^8\,M_K^6\,M_\pi^2\,s_\theta^{12}\,\Lambda_2}{243\,M_\eta^8\,M_{\eta'}^4} - \frac{1792\,L_8^r\,M_0^8\,M_K^4\,M_\pi^4\,s_\theta^{12}\,\Lambda_2}{81\,M_\eta^8\,M_{\eta'}^4} + \frac{5120\,L_8^r\,M_0^8\,M_K^2\,M_\pi^6\,s_\theta^{12}\,\Lambda_2}{729\,M_\eta^8\,M_{\eta'}^4} -
\end{aligned}$$

$$\begin{aligned}
& \frac{256 L_8^r M_0^8 M_\pi^8 S_\theta^{12} \Lambda_2}{243 M_\eta^8 M_{\eta'}^4} - \frac{14 \, 336 L_8^r M_0^8 M_K^8 S_\theta^{12} \Lambda_2}{729 M_\eta^{10} M_{\eta'}^2} + \frac{1024 L_8^r M_0^8 M_K^6 M_\pi^2 S_\theta^{12} \Lambda_2}{27 M_\eta^{10} M_{\eta'}^2} - \\
& \frac{5120 L_8^r M_0^8 M_K^4 M_\pi^4 S_\theta^{12} \Lambda_2}{243 M_\eta^{10} M_{\eta'}^2} + \frac{5120 L_8^r M_0^8 M_K^2 M_\pi^6 S_\theta^{12} \Lambda_2}{729 M_\eta^{10} M_{\eta'}^2} - \frac{1024 L_8^r M_0^8 M_\pi^8 S_\theta^{12} \Lambda_2}{243 M_\eta^{10} M_{\eta'}^2} - \\
& \frac{160 F^2 c_\theta^{12} M_0^8 M_K^6 \Lambda_2^2}{729 M_\eta^{12}} - \frac{80 F^2 c_\theta^{12} M_0^8 M_K^4 M_\pi^2 \Lambda_2^2}{243 M_\eta^{12}} - \frac{40 F^2 c_\theta^{12} M_0^8 M_K^2 M_\pi^4 \Lambda_2^2}{243 M_\eta^{12}} - \frac{20 F^2 c_\theta^{12} M_0^8 M_\pi^6 \Lambda_2^2}{729 M_\eta^{12}} + \\
& \frac{64 F^2 c_\theta^{10} M_0^8 M_K^4 \Lambda_2^2}{243 M_\eta^{10}} + \frac{128 F^2 c_\theta^{10} M_0^6 M_K^6 \Lambda_2^2}{729 M_\eta^{10}} + \frac{64 F^2 c_\theta^{10} M_0^8 M_K^2 M_\pi^2 \Lambda_2^2}{243 M_\eta^{10}} + \frac{64 F^2 c_\theta^{10} M_0^6 M_K^4 M_\pi^2 \Lambda_2^2}{243 M_\eta^{10}} + \\
& \frac{16 F^2 c_\theta^{10} M_0^8 M_K^4 \Lambda_2^2}{243 M_\eta^{10}} + \frac{32 F^2 c_\theta^{10} M_0^6 M_K^2 M_\pi^4 \Lambda_2^2}{243 M_\eta^{10}} + \frac{16 F^2 c_\theta^{10} M_0^6 M_\pi^6 \Lambda_2^2}{729 M_\eta^{10}} - \frac{32 F^2 c_\theta^{12} M_0^8 M_K^6 \Lambda_2^2}{81 M_\eta^2 M_{\eta'}^{10}} + \\
& \frac{16 F^2 c_\theta^{12} M_0^8 M_K^4 M_\pi^2 \Lambda_2^2}{27 M_\eta^2 M_{\eta'}^{10}} - \frac{16 F^2 c_\theta^{12} M_0^8 M_\pi^6 \Lambda_2^2}{81 M_\eta^2 M_{\eta'}^{10}} - \frac{32 F^2 c_\theta^8 M_0^6 M_K^4 \Lambda_2^2}{243 M_\eta^8} - \frac{8 F^2 c_\theta^8 M_0^4 M_K^6 \Lambda_2^2}{243 M_\eta^8} - \\
& \frac{32 F^2 c_\theta^8 M_0^6 M_K^2 M_\pi^2 \Lambda_2^2}{243 M_\eta^8} - \frac{4 F^2 c_\theta^8 M_0^4 M_K^4 M_\pi^2 \Lambda_2^2}{81 M_\eta^8} - \frac{8 F^2 c_\theta^8 M_0^6 M_\pi^4 \Lambda_2^2}{243 M_\eta^8} - \frac{2 F^2 c_\theta^8 M_0^4 M_K^2 M_\pi^4 \Lambda_2^2}{81 M_\eta^8} - \\
& \frac{F^2 c_\theta^8 M_0^4 M_\pi^6 \Lambda_2^2}{243 M_\eta^8} - \frac{32 F^2 c_\theta^{12} M_0^8 M_K^6 \Lambda_2^2}{243 M_\eta^4 M_{\eta'}^8} + \frac{8 F^2 c_\theta^{12} M_0^8 M_K^4 M_\pi^2 \Lambda_2^2}{27 M_\eta^4 M_{\eta'}^8} - \frac{16 F^2 c_\theta^{12} M_0^8 M_K^2 M_\pi^4 \Lambda_2^2}{81 M_\eta^4 M_{\eta'}^8} + \\
& \frac{8 F^2 c_\theta^{12} M_0^8 M_\pi^6 \Lambda_2^2}{243 M_\eta^4 M_{\eta'}^8} + \frac{16 F^2 c_\theta^{10} M_0^8 M_K^4 \Lambda_2^2}{81 M_\eta^2 M_{\eta'}^8} + \frac{352 F^2 c_\theta^{10} M_0^6 M_K^6 \Lambda_2^2}{729 M_\eta^2 M_{\eta'}^8} - \frac{32 F^2 c_\theta^{10} M_0^8 M_K^2 M_\pi^2 \Lambda_2^2}{81 M_\eta^2 M_{\eta'}^8} - \\
& \frac{176 F^2 c_\theta^{10} M_0^6 M_K^4 M_\pi^2 \Lambda_2^2}{243 M_\eta^2 M_{\eta'}^8} + \frac{16 F^2 c_\theta^{10} M_0^8 M_\pi^4 \Lambda_2^2}{81 M_\eta^2 M_{\eta'}^8} + \frac{176 F^2 c_\theta^{10} M_0^6 M_\pi^6 \Lambda_2^2}{729 M_\eta^2 M_{\eta'}^8} + \frac{8 F^2 c_\theta^6 M_0^4 M_K^4 \Lambda_2^2}{81 M_\eta^6} + \\
& \frac{8 F^2 c_\theta^6 M_0^6 M_K^2 M_\pi^2 \Lambda_2^2}{81 M_\eta^6} + \frac{2 F^2 c_\theta^6 M_0^4 M_\pi^4 \Lambda_2^2}{81 M_\eta^6} + \frac{64 F^2 c_\theta^{10} M_0^6 M_K^6 \Lambda_2^2}{243 M_\eta^4 M_{\eta'}^6} - \frac{16 F^2 c_\theta^{10} M_0^6 M_K^4 M_\pi^2 \Lambda_2^2}{27 M_\eta^4 M_{\eta'}^6} + \\
& \frac{32 F^2 c_\theta^{10} M_0^6 M_\pi^6 \Lambda_2^2}{81 M_\eta^4 M_{\eta'}^6} - \frac{16 F^2 c_\theta^{10} M_0^6 M_\pi^6 \Lambda_2^2}{243 M_\eta^4 M_{\eta'}^6} - \frac{16 F^2 c_\theta^8 M_0^6 M_K^4 \Lambda_2^2}{81 M_\eta^2 M_{\eta'}^6} - \frac{32 F^2 c_\theta^8 M_0^4 M_K^6 \Lambda_2^2}{243 M_\eta^2 M_{\eta'}^6} + \\
& \frac{32 F^2 c_\theta^8 M_0^6 M_K^2 M_\pi^2 \Lambda_2^2}{81 M_\eta^2 M_{\eta'}^6} + \frac{16 F^2 c_\theta^8 M_0^4 M_K^4 M_\pi^2 \Lambda_2^2}{81 M_\eta^2 M_{\eta'}^6} - \frac{16 F^2 c_\theta^8 M_0^6 M_\pi^4 \Lambda_2^2}{81 M_\eta^2 M_{\eta'}^6} - \frac{16 F^2 c_\theta^8 M_0^4 M_\pi^6 \Lambda_2^2}{243 M_\eta^2 M_{\eta'}^6} - \\
& \frac{32 F^2 c_\theta^8 M_0^4 M_K^6 \Lambda_2^2}{243 M_\eta^4 M_{\eta'}^4} + \frac{8 F^2 c_\theta^8 M_0^4 M_K^4 M_\pi^2 \Lambda_2^2}{27 M_\eta^4 M_{\eta'}^4} - \frac{16 F^2 c_\theta^8 M_0^6 M_K^2 M_\pi^2 \Lambda_2^2}{81 M_\eta^4 M_{\eta'}^4} + \frac{8 F^2 c_\theta^8 M_0^4 M_\pi^6 \Lambda_2^2}{243 M_\eta^4 M_{\eta'}^4} + \\
& \frac{320 \sqrt{2} F^2 c_\theta^{11} M_0^8 M_K^6 S_\theta \Lambda_2^2}{243 M_\eta^{12}} - \frac{80 \sqrt{2} F^2 c_\theta^{11} M_0^8 M_K^2 M_\pi^4 S_\theta \Lambda_2^2}{81 M_\eta^{12}} - \frac{80 \sqrt{2} F^2 c_\theta^{11} M_0^8 M_\pi^6 S_\theta \Lambda_2^2}{243 M_\eta^{12}} - \\
& \frac{256 \sqrt{2} F^2 c_\theta^9 M_0^8 M_K^4 S_\theta \Lambda_2^2}{243 M_\eta^{10}} - \frac{256 \sqrt{2} F^2 c_\theta^9 M_0^6 M_K^6 S_\theta \Lambda_2^2}{243 M_\eta^{10}} + \frac{128 \sqrt{2} F^2 c_\theta^9 M_0^8 M_K^2 M_\pi^2 S_\theta \Lambda_2^2}{243 M_\eta^{10}} + \\
& \frac{128 \sqrt{2} F^2 c_\theta^9 M_0^8 M_\pi^4 S_\theta \Lambda_2^2}{243 M_\eta^{10}} + \frac{64 \sqrt{2} F^2 c_\theta^9 M_0^6 M_K^2 M_\pi^4 S_\theta \Lambda_2^2}{81 M_\eta^{10}} + \frac{64 \sqrt{2} F^2 c_\theta^9 M_0^6 M_\pi^6 S_\theta \Lambda_2^2}{243 M_\eta^{10}} +
\end{aligned}$$



$$\begin{aligned}
& \frac{64 \sqrt{2} F^2 c_\theta^{11} M_\theta^8 M_K^6 s_\theta \Lambda_2^2}{243 M_\eta^2 M_{\eta'}^{10}} - \frac{64 \sqrt{2} F^2 c_\theta^{11} M_\theta^8 M_K^4 M_\pi^2 s_\theta \Lambda_2^2}{27 M_\eta^2 M_{\eta'}^{10}} + \frac{176 \sqrt{2} F^2 c_\theta^{11} M_\theta^8 M_K^2 M_\pi^4 s_\theta \Lambda_2^2}{81 M_\eta^2 M_{\eta'}^{10}} - \\
& \frac{16 \sqrt{2} F^2 c_\theta^{11} M_\theta^8 M_\pi^6 s_\theta \Lambda_2^2}{243 M_\eta^2 M_{\eta'}^{10}} + \frac{128 \sqrt{2} F^2 c_\theta^7 M_\theta^6 M_K^4 s_\theta \Lambda_2^2}{243 M_{\eta'}^8} + \frac{16 \sqrt{2} F^2 c_\theta^7 M_\theta^4 M_K^6 s_\theta \Lambda_2^2}{81 M_{\eta'}^8} - \\
& \frac{64 \sqrt{2} F^2 c_\theta^7 M_\theta^6 M_K^2 M_\pi^2 s_\theta \Lambda_2^2}{243 M_{\eta'}^8} - \frac{64 \sqrt{2} F^2 c_\theta^7 M_\theta^6 M_\pi^4 s_\theta \Lambda_2^2}{243 M_{\eta'}^8} - \frac{4 \sqrt{2} F^2 c_\theta^7 M_\theta^4 M_K^2 M_\pi^4 s_\theta \Lambda_2^2}{27 M_{\eta'}^8} - \\
& \frac{4 \sqrt{2} F^2 c_\theta^7 M_\theta^4 M_\pi^6 s_\theta \Lambda_2^2}{81 M_{\eta'}^8} - \frac{320 \sqrt{2} F^2 c_\theta^{11} M_\theta^8 M_K^6 s_\theta \Lambda_2^2}{243 M_\eta^4 M_{\eta'}^8} + \frac{136 \sqrt{2} F^2 c_\theta^{11} M_\theta^8 M_K^4 M_\pi^2 s_\theta \Lambda_2^2}{81 M_\eta^4 M_{\eta'}^8} - \\
& \frac{16 \sqrt{2} F^2 c_\theta^{11} M_\theta^8 M_K^2 M_\pi^4 s_\theta \Lambda_2^2}{27 M_\eta^4 M_{\eta'}^8} + \frac{56 \sqrt{2} F^2 c_\theta^{11} M_\theta^8 M_\pi^6 s_\theta \Lambda_2^2}{243 M_\eta^4 M_{\eta'}^8} + \frac{160 \sqrt{2} F^2 c_\theta^9 M_\theta^8 M_K^4 s_\theta \Lambda_2^2}{243 M_\eta^2 M_{\eta'}^8} - \\
& \frac{640 \sqrt{2} F^2 c_\theta^9 M_\theta^6 M_K^6 s_\theta \Lambda_2^2}{729 M_\eta^2 M_{\eta'}^8} - \frac{8 \sqrt{2} F^2 c_\theta^9 M_\theta^8 M_K^2 M_\pi^2 s_\theta \Lambda_2^2}{243 M_\eta^2 M_{\eta'}^8} + \frac{688 \sqrt{2} F^2 c_\theta^9 M_\theta^6 M_K^4 M_\pi^2 s_\theta \Lambda_2^2}{243 M_\eta^2 M_{\eta'}^8} - \\
& \frac{152 \sqrt{2} F^2 c_\theta^9 M_\theta^8 M_\pi^4 s_\theta \Lambda_2^2}{243 M_\eta^2 M_{\eta'}^8} - \frac{520 \sqrt{2} F^2 c_\theta^9 M_\theta^6 M_K^2 M_\pi^4 s_\theta \Lambda_2^2}{243 M_\eta^2 M_{\eta'}^8} + \frac{136 \sqrt{2} F^2 c_\theta^9 M_\theta^6 M_\pi^6 s_\theta \Lambda_2^2}{729 M_\eta^2 M_{\eta'}^8} - \\
& \frac{32 \sqrt{2} F^2 c_\theta^5 M_\theta^4 M_K^4 s_\theta \Lambda_2^2}{81 M_{\eta'}^6} + \frac{16 \sqrt{2} F^2 c_\theta^5 M_\theta^4 M_K^2 M_\pi^2 s_\theta \Lambda_2^2}{81 M_{\eta'}^6} + \frac{16 \sqrt{2} F^2 c_\theta^5 M_\theta^4 M_\pi^4 s_\theta \Lambda_2^2}{81 M_{\eta'}^6} - \\
& \frac{64 \sqrt{2} F^2 c_\theta^{11} M_\theta^8 M_K^6 s_\theta \Lambda_2^2}{243 M_\eta^6 M_{\eta'}^6} + \frac{56 \sqrt{2} F^2 c_\theta^{11} M_\theta^8 M_K^4 M_\pi^2 s_\theta \Lambda_2^2}{81 M_\eta^6 M_{\eta'}^6} - \frac{16 \sqrt{2} F^2 c_\theta^{11} M_\theta^8 M_K^2 M_\pi^4 s_\theta \Lambda_2^2}{27 M_\eta^6 M_{\eta'}^6} + \\
& \frac{40 \sqrt{2} F^2 c_\theta^{11} M_\theta^8 M_\pi^6 s_\theta \Lambda_2^2}{243 M_\eta^6 M_{\eta'}^6} + \frac{32 \sqrt{2} F^2 c_\theta^9 M_\theta^8 M_K^4 s_\theta \Lambda_2^2}{81 M_\eta^4 M_{\eta'}^6} + \frac{1024 \sqrt{2} F^2 c_\theta^9 M_\theta^6 M_K^6 s_\theta \Lambda_2^2}{729 M_\eta^4 M_{\eta'}^6} - \\
& \frac{40 \sqrt{2} F^2 c_\theta^9 M_\theta^8 M_K^2 M_\pi^2 s_\theta \Lambda_2^2}{81 M_\eta^4 M_{\eta'}^6} - \frac{352 \sqrt{2} F^2 c_\theta^9 M_\theta^6 M_K^4 M_\pi^2 s_\theta \Lambda_2^2}{243 M_\eta^4 M_{\eta'}^6} + \frac{8 \sqrt{2} F^2 c_\theta^9 M_\theta^8 M_\pi^4 s_\theta \Lambda_2^2}{81 M_\eta^4 M_{\eta'}^6} + \\
& \frac{40 \sqrt{2} F^2 c_\theta^9 M_\theta^6 M_K^2 M_\pi^4 s_\theta \Lambda_2^2}{243 M_\eta^4 M_{\eta'}^6} - \frac{88 \sqrt{2} F^2 c_\theta^9 M_\theta^6 M_\pi^6 s_\theta \Lambda_2^2}{729 M_\eta^4 M_{\eta'}^6} - \frac{32 \sqrt{2} F^2 c_\theta^7 M_\theta^6 M_K^4 s_\theta \Lambda_2^2}{243 M_\eta^2 M_{\eta'}^6} + \\
& \frac{80 \sqrt{2} F^2 c_\theta^7 M_\theta^4 M_K^6 s_\theta \Lambda_2^2}{243 M_\eta^2 M_{\eta'}^6} - \frac{56 \sqrt{2} F^2 c_\theta^7 M_\theta^6 M_K^2 M_\pi^2 s_\theta \Lambda_2^2}{243 M_\eta^2 M_{\eta'}^6} - \frac{56 \sqrt{2} F^2 c_\theta^7 M_\theta^4 M_K^4 M_\pi^2 s_\theta \Lambda_2^2}{81 M_\eta^2 M_{\eta'}^6} + \\
& \frac{88 \sqrt{2} F^2 c_\theta^7 M_\theta^6 M_\pi^4 s_\theta \Lambda_2^2}{243 M_\eta^2 M_{\eta'}^6} + \frac{32 \sqrt{2} F^2 c_\theta^7 M_\theta^4 M_K^2 M_\pi^4 s_\theta \Lambda_2^2}{81 M_\eta^2 M_{\eta'}^6} - \frac{8 \sqrt{2} F^2 c_\theta^7 M_\theta^4 M_\pi^6 s_\theta \Lambda_2^2}{243 M_\eta^2 M_{\eta'}^6} + \\
& \frac{128 \sqrt{2} F^2 c_\theta^9 M_\theta^6 M_K^6 s_\theta \Lambda_2^2}{243 M_\eta^6 M_{\eta'}^4} - \frac{112 \sqrt{2} F^2 c_\theta^9 M_\theta^6 M_K^4 M_\pi^2 s_\theta \Lambda_2^2}{81 M_\eta^6 M_{\eta'}^4} + \frac{32 \sqrt{2} F^2 c_\theta^9 M_\theta^6 M_K^2 M_\pi^4 s_\theta \Lambda_2^2}{27 M_\eta^6 M_{\eta'}^4} - \\
& \frac{80 \sqrt{2} F^2 c_\theta^9 M_\theta^6 M_\pi^6 s_\theta \Lambda_2^2}{243 M_\eta^6 M_{\eta'}^4} - \frac{32 \sqrt{2} F^2 c_\theta^7 M_\theta^6 M_K^4 s_\theta \Lambda_2^2}{81 M_\eta^4 M_{\eta'}^4} - \frac{64 \sqrt{2} F^2 c_\theta^7 M_\theta^4 M_K^6 s_\theta \Lambda_2^2}{243 M_\eta^4 M_{\eta'}^4} +
\end{aligned}$$

$$\begin{aligned}
& \frac{40 \sqrt{2} F^2 c_\theta^7 M_0^6 M_K^2 M_\pi^2 s_\theta \Lambda_2^2}{81 M_\eta^4 M_{\eta'}^4} - \frac{8 \sqrt{2} F^2 c_\theta^7 M_0^6 M_\pi^4 s_\theta \Lambda_2^2}{81 M_\eta^4 M_{\eta'}^4} + \frac{28 \sqrt{2} F^2 c_\theta^7 M_0^4 M_K^2 M_\pi^4 s_\theta \Lambda_2^2}{81 M_\eta^4 M_{\eta'}^4} - \\
& \frac{20 \sqrt{2} F^2 c_\theta^7 M_0^4 M_\pi^6 s_\theta \Lambda_2^2}{243 M_\eta^4 M_{\eta'}^4} - \frac{64 \sqrt{2} F^2 c_\theta^7 M_0^4 M_K^6 s_\theta \Lambda_2^2}{243 M_\eta^6 M_{\eta'}^2} + \frac{56 \sqrt{2} F^2 c_\theta^7 M_0^4 M_K^4 M_\pi^2 s_\theta \Lambda_2^2}{81 M_\eta^6 M_{\eta'}^2} - \\
& \frac{16 \sqrt{2} F^2 c_\theta^7 M_0^4 M_K^2 M_\pi^4 s_\theta \Lambda_2^2}{27 M_\eta^6 M_{\eta'}^2} + \frac{40 \sqrt{2} F^2 c_\theta^7 M_0^4 M_\pi^6 s_\theta \Lambda_2^2}{243 M_\eta^6 M_{\eta'}^2} - \frac{64 F^2 c_\theta^6 M_0^4 M_K^6 s_\theta^2 \Lambda_2^2}{243 M_\eta^8} + \\
& \frac{52 F^2 c_\theta^6 M_0^4 M_K^4 M_\pi^2 s_\theta^2 \Lambda_2^2}{81 M_\eta^8} - \frac{40 F^2 c_\theta^6 M_0^4 M_K^2 M_\pi^4 s_\theta^2 \Lambda_2^2}{81 M_\eta^8} + \frac{28 F^2 c_\theta^6 M_0^4 M_\pi^6 s_\theta^2 \Lambda_2^2}{243 M_\eta^8} + \frac{32 F^2 c_\theta^4 M_0^4 M_K^4 s_\theta^2 \Lambda_2^2}{81 M_\eta^6} - \\
& \frac{52 F^2 c_\theta^4 M_0^4 M_K^2 M_\pi^2 s_\theta^2 \Lambda_2^2}{81 M_\eta^6} + \frac{20 F^2 c_\theta^4 M_0^4 M_\pi^4 s_\theta^2 \Lambda_2^2}{81 M_\eta^6} - \frac{1600 F^2 c_\theta^{10} M_0^8 M_K^6 s_\theta^2 \Lambda_2^2}{243 M_{\eta'}^{12}} + \\
& \frac{320 F^2 c_\theta^{10} M_0^8 M_K^4 M_\pi^2 s_\theta^2 \Lambda_2^2}{81 M_{\eta'}^{12}} - \frac{440 F^2 c_\theta^{10} M_0^8 M_\pi^6 s_\theta^2 \Lambda_2^2}{243 M_{\eta'}^{12}} + \frac{256 F^2 c_\theta^8 M_0^8 M_K^4 s_\theta^2 \Lambda_2^2}{81 M_{\eta'}^{10}} + \\
& \frac{1280 F^2 c_\theta^8 M_0^6 M_K^6 s_\theta^2 \Lambda_2^2}{243 M_{\eta'}^{10}} - \frac{224 F^2 c_\theta^8 M_0^8 M_K^2 M_\pi^2 s_\theta^2 \Lambda_2^2}{81 M_{\eta'}^{10}} - \frac{256 F^2 c_\theta^8 M_0^6 M_K^4 M_\pi^2 s_\theta^2 \Lambda_2^2}{81 M_{\eta'}^{10}} + \\
& \frac{112 F^2 c_\theta^8 M_0^8 M_\pi^4 s_\theta^2 \Lambda_2^2}{81 M_{\eta'}^{10}} + \frac{352 F^2 c_\theta^8 M_0^6 M_\pi^6 s_\theta^2 \Lambda_2^2}{243 M_{\eta'}^{10}} + \frac{512 F^2 c_\theta^{10} M_0^8 M_K^6 s_\theta^2 \Lambda_2^2}{81 M_\eta^2 M_{\eta'}^{10}} - \\
& \frac{32 F^2 c_\theta^{10} M_0^8 M_K^4 M_\pi^2 s_\theta^2 \Lambda_2^2}{81 M_\eta^2 M_{\eta'}^{10}} - \frac{368 F^2 c_\theta^{10} M_0^8 M_K^2 M_\pi^4 s_\theta^2 \Lambda_2^2}{81 M_\eta^2 M_{\eta'}^{10}} + \frac{248 F^2 c_\theta^{10} M_0^8 M_\pi^6 s_\theta^2 \Lambda_2^2}{81 M_\eta^2 M_{\eta'}^{10}} - \\
& \frac{128 F^2 c_\theta^6 M_0^6 M_K^4 s_\theta^2 \Lambda_2^2}{81 M_{\eta'}^8} - \frac{80 F^2 c_\theta^6 M_0^4 M_K^6 s_\theta^2 \Lambda_2^2}{81 M_{\eta'}^8} + \frac{112 F^2 c_\theta^6 M_0^6 M_K^2 M_\pi^2 s_\theta^2 \Lambda_2^2}{81 M_{\eta'}^8} + \\
& \frac{16 F^2 c_\theta^6 M_0^4 M_K^4 M_\pi^2 s_\theta^2 \Lambda_2^2}{27 M_{\eta'}^8} - \frac{56 F^2 c_\theta^6 M_0^6 M_\pi^4 s_\theta^2 \Lambda_2^2}{81 M_{\eta'}^8} - \frac{22 F^2 c_\theta^6 M_0^4 M_\pi^6 s_\theta^2 \Lambda_2^2}{81 M_{\eta'}^8} + \frac{128 F^2 c_\theta^{10} M_0^8 M_K^6 s_\theta^2 \Lambda_2^2}{243 M_\eta^4 M_{\eta'}^8} - \\
& \frac{76 F^2 c_\theta^{10} M_0^8 M_K^4 M_\pi^2 s_\theta^2 \Lambda_2^2}{9 M_\eta^4 M_{\eta'}^8} + \frac{472 F^2 c_\theta^{10} M_0^8 M_K^2 M_\pi^4 s_\theta^2 \Lambda_2^2}{81 M_\eta^4 M_{\eta'}^8} - \frac{572 F^2 c_\theta^{10} M_0^8 M_\pi^6 s_\theta^2 \Lambda_2^2}{243 M_\eta^4 M_{\eta'}^8} - \\
& \frac{1024 F^2 c_\theta^8 M_0^8 M_K^4 s_\theta^2 \Lambda_2^2}{243 M_\eta^2 M_{\eta'}^8} - \frac{704 F^2 c_\theta^8 M_0^6 M_K^6 s_\theta^2 \Lambda_2^2}{243 M_\eta^2 M_{\eta'}^8} + \frac{1316 F^2 c_\theta^8 M_0^8 M_K^2 M_\pi^2 s_\theta^2 \Lambda_2^2}{243 M_\eta^2 M_{\eta'}^8} - \\
& \frac{944 F^2 c_\theta^8 M_0^6 M_K^4 M_\pi^2 s_\theta^2 \Lambda_2^2}{243 M_\eta^2 M_{\eta'}^8} - \frac{436 F^2 c_\theta^8 M_0^8 M_\pi^4 s_\theta^2 \Lambda_2^2}{243 M_\eta^2 M_{\eta'}^8} + \frac{1192 F^2 c_\theta^8 M_0^6 M_K^2 M_\pi^4 s_\theta^2 \Lambda_2^2}{243 M_\eta^2 M_{\eta'}^8} - \\
& \frac{184 F^2 c_\theta^8 M_0^6 M_\pi^6 s_\theta^2 \Lambda_2^2}{81 M_\eta^2 M_{\eta'}^8} + \frac{32 F^2 c_\theta^4 M_0^4 M_K^4 s_\theta^2 \Lambda_2^2}{27 M_{\eta'}^6} - \frac{28 F^2 c_\theta^4 M_0^4 M_K^2 M_\pi^2 s_\theta^2 \Lambda_2^2}{27 M_{\eta'}^6} + \frac{14 F^2 c_\theta^4 M_0^4 M_\pi^4 s_\theta^2 \Lambda_2^2}{27 M_{\eta'}^6} - \\
& \frac{1088 F^2 c_\theta^{10} M_0^8 M_K^6 s_\theta^2 \Lambda_2^2}{243 M_\eta^6 M_{\eta'}^6} + \frac{616 F^2 c_\theta^{10} M_0^8 M_K^4 M_\pi^2 s_\theta^2 \Lambda_2^2}{81 M_\eta^6 M_{\eta'}^6} - \frac{80 F^2 c_\theta^{10} M_0^8 M_K^2 M_\pi^4 s_\theta^2 \Lambda_2^2}{27 M_\eta^6 M_{\eta'}^6} - \\
& \frac{40 F^2 c_\theta^{10} M_0^8 M_\pi^6 s_\theta^2 \Lambda_2^2}{243 M_\eta^6 M_{\eta'}^6} + \frac{80 F^2 c_\theta^8 M_0^8 M_K^4 s_\theta^2 \Lambda_2^2}{27 M_\eta^4 M_{\eta'}^6} - \frac{800 F^2 c_\theta^8 M_0^6 M_K^6 s_\theta^2 \Lambda_2^2}{243 M_\eta^4 M_{\eta'}^6} - \frac{8 F^2 c_\theta^8 M_0^8 M_K^2 M_\pi^2 s_\theta^2 \Lambda_2^2}{3 M_\eta^4 M_{\eta'}^6} +
\end{aligned}$$

$$\begin{aligned}
& \frac{904 F^2 c_\theta^8 M_\theta^6 M_K^4 M_\pi^2 s_\theta^2 \Lambda_2^2}{81 M_\eta^4 M_{\eta'}^6} + \frac{40 F^2 c_\theta^8 M_\theta^8 M_\pi^4 s_\theta^2 \Lambda_2^2}{27 M_\eta^4 M_{\eta'}^6} - \frac{160 F^2 c_\theta^8 M_\theta^6 M_K^2 M_\pi^4 s_\theta^2 \Lambda_2^2}{27 M_\eta^4 M_{\eta'}^6} + \\
& \frac{392 F^2 c_\theta^8 M_\theta^6 M_\pi^6 s_\theta^2 \Lambda_2^2}{243 M_\eta^4 M_{\eta'}^6} + \frac{448 F^2 c_\theta^6 M_\theta^6 M_K^4 s_\theta^2 \Lambda_2^2}{243 M_\eta^2 M_{\eta'}^6} - \frac{452 F^2 c_\theta^6 M_\theta^6 M_K^2 M_\pi^2 s_\theta^2 \Lambda_2^2}{243 M_\eta^2 M_{\eta'}^6} + \\
& \frac{136 F^2 c_\theta^6 M_\theta^4 M_K^4 M_\pi^2 s_\theta^2 \Lambda_2^2}{81 M_\eta^2 M_{\eta'}^6} + \frac{148 F^2 c_\theta^6 M_\theta^6 M_\pi^4 s_\theta^2 \Lambda_2^2}{243 M_\eta^2 M_{\eta'}^6} - \frac{92 F^2 c_\theta^6 M_\theta^4 M_K^2 M_\pi^4 s_\theta^2 \Lambda_2^2}{81 M_\eta^2 M_{\eta'}^6} + \frac{28 F^2 c_\theta^6 M_\theta^4 M_\pi^6 s_\theta^2 \Lambda_2^2}{81 M_\eta^2 M_{\eta'}^6} - \\
& \frac{64 F^2 c_\theta^{10} M_\theta^8 M_K^6 s_\theta^2 \Lambda_2^2}{243 M_\eta^8 M_{\eta'}^4} + \frac{52 F^2 c_\theta^{10} M_\theta^8 M_K^4 M_\pi^2 s_\theta^2 \Lambda_2^2}{81 M_\eta^8 M_{\eta'}^4} - \frac{40 F^2 c_\theta^{10} M_\theta^8 M_K^2 M_\pi^4 s_\theta^2 \Lambda_2^2}{81 M_\eta^8 M_{\eta'}^4} + \\
& \frac{28 F^2 c_\theta^{10} M_\theta^8 M_\pi^6 s_\theta^2 \Lambda_2^2}{243 M_\eta^8 M_{\eta'}^4} + \frac{32 F^2 c_\theta^8 M_\theta^8 M_K^4 s_\theta^2 \Lambda_2^2}{81 M_\eta^6 M_{\eta'}^4} + \frac{1216 F^2 c_\theta^8 M_\theta^6 M_K^6 s_\theta^2 \Lambda_2^2}{243 M_\eta^6 M_{\eta'}^4} - \frac{52 F^2 c_\theta^8 M_\theta^8 M_K^2 M_\pi^2 s_\theta^2 \Lambda_2^2}{81 M_\eta^6 M_{\eta'}^4} - \\
& \frac{656 F^2 c_\theta^8 M_\theta^6 M_K^4 M_\pi^2 s_\theta^2 \Lambda_2^2}{81 M_\eta^6 M_{\eta'}^4} + \frac{20 F^2 c_\theta^8 M_\theta^8 M_\pi^4 s_\theta^2 \Lambda_2^2}{81 M_\eta^6 M_{\eta'}^4} + \frac{8 F^2 c_\theta^8 M_\theta^6 M_K^2 M_\pi^4 s_\theta^2 \Lambda_2^2}{3 M_\eta^6 M_{\eta'}^4} + \\
& \frac{104 F^2 c_\theta^8 M_\theta^6 M_\pi^6 s_\theta^2 \Lambda_2^2}{243 M_\eta^6 M_{\eta'}^4} - \frac{32 F^2 c_\theta^6 M_\theta^6 M_K^4 s_\theta^2 \Lambda_2^2}{27 M_\eta^4 M_{\eta'}^4} + \frac{272 F^2 c_\theta^6 M_\theta^4 M_K^6 s_\theta^2 \Lambda_2^2}{243 M_\eta^4 M_{\eta'}^4} + \frac{8 F^2 c_\theta^6 M_\theta^6 M_K^2 M_\pi^2 s_\theta^2 \Lambda_2^2}{9 M_\eta^4 M_{\eta'}^4} - \\
& \frac{68 F^2 c_\theta^6 M_\theta^4 M_K^4 M_\pi^2 s_\theta^2 \Lambda_2^2}{27 M_\eta^4 M_{\eta'}^4} - \frac{16 F^2 c_\theta^6 M_\theta^6 M_\pi^4 s_\theta^2 \Lambda_2^2}{27 M_\eta^4 M_{\eta'}^4} + \frac{64 F^2 c_\theta^6 M_\theta^4 M_K^2 M_\pi^4 s_\theta^2 \Lambda_2^2}{81 M_\eta^4 M_{\eta'}^4} - \frac{14 F^2 c_\theta^6 M_\theta^4 M_\pi^6 s_\theta^2 \Lambda_2^2}{243 M_\eta^4 M_{\eta'}^4} + \\
& \frac{128 F^2 c_\theta^8 M_\theta^6 M_K^6 s_\theta^2 \Lambda_2^2}{243 M_\eta^8 M_{\eta'}^2} - \frac{104 F^2 c_\theta^8 M_\theta^6 M_K^4 M_\pi^2 s_\theta^2 \Lambda_2^2}{81 M_\eta^8 M_{\eta'}^2} + \frac{80 F^2 c_\theta^8 M_\theta^6 M_K^2 M_\pi^4 s_\theta^2 \Lambda_2^2}{81 M_\eta^8 M_{\eta'}^2} - \\
& \frac{56 F^2 c_\theta^8 M_\theta^6 M_\pi^6 s_\theta^2 \Lambda_2^2}{243 M_\eta^8 M_{\eta'}^2} - \frac{32 F^2 c_\theta^6 M_\theta^6 M_K^4 s_\theta^2 \Lambda_2^2}{81 M_\eta^6 M_{\eta'}^2} - \frac{256 F^2 c_\theta^6 M_\theta^4 M_K^6 s_\theta^2 \Lambda_2^2}{243 M_\eta^6 M_{\eta'}^2} + \frac{52 F^2 c_\theta^6 M_\theta^6 M_K^2 M_\pi^2 s_\theta^2 \Lambda_2^2}{81 M_\eta^6 M_{\eta'}^2} + \\
& \frac{112 F^2 c_\theta^6 M_\theta^4 M_K^4 M_\pi^2 s_\theta^2 \Lambda_2^2}{81 M_\eta^6 M_{\eta'}^2} - \frac{20 F^2 c_\theta^6 M_\theta^6 M_\pi^4 s_\theta^2 \Lambda_2^2}{81 M_\eta^6 M_{\eta'}^2} - \frac{4 F^2 c_\theta^6 M_\theta^4 M_K^2 M_\pi^4 s_\theta^2 \Lambda_2^2}{81 M_\eta^6 M_{\eta'}^2} - \frac{68 F^2 c_\theta^6 M_\theta^4 M_\pi^6 s_\theta^2 \Lambda_2^2}{243 M_\eta^6 M_{\eta'}^2} - \\
& \frac{64 \sqrt{2} F^2 c_\theta^5 M_\theta^4 M_K^6 s_\theta^3 \Lambda_2^2}{81 M_\eta^8} + \frac{44 \sqrt{2} F^2 c_\theta^5 M_\theta^4 M_K^4 M_\pi^2 s_\theta^3 \Lambda_2^2}{27 M_\eta^8} - \frac{10 \sqrt{2} F^2 c_\theta^5 M_\theta^4 M_K^2 M_\pi^4 s_\theta^3 \Lambda_2^2}{9 M_\eta^8} + \\
& \frac{22 \sqrt{2} F^2 c_\theta^5 M_\theta^4 M_\pi^6 s_\theta^3 \Lambda_2^2}{81 M_\eta^8} + \frac{64 \sqrt{2} F^2 c_\theta^3 M_\theta^4 M_K^4 s_\theta^3 \Lambda_2^2}{81 M_\eta^6} - \frac{62 \sqrt{2} F^2 c_\theta^3 M_\theta^4 M_K^2 M_\pi^2 s_\theta^3 \Lambda_2^2}{81 M_\eta^6} + \\
& \frac{7 \sqrt{2} F^2 c_\theta^3 M_\theta^4 M_\pi^4 s_\theta^3 \Lambda_2^2}{81 M_\eta^6} + \frac{6400 \sqrt{2} F^2 c_\theta^9 M_\theta^8 M_K^6 s_\theta^3 \Lambda_2^2}{729 M_{\eta'}^{12}} - \frac{2080 \sqrt{2} F^2 c_\theta^9 M_\theta^8 M_K^4 M_\pi^2 s_\theta^3 \Lambda_2^2}{243 M_{\eta'}^{12}} + \\
& \frac{640 \sqrt{2} F^2 c_\theta^9 M_\theta^8 M_K^2 M_\pi^4 s_\theta^3 \Lambda_2^2}{243 M_{\eta'}^{12}} - \frac{1000 \sqrt{2} F^2 c_\theta^9 M_\theta^8 M_\pi^6 s_\theta^3 \Lambda_2^2}{729 M_{\eta'}^{12}} - \frac{512 \sqrt{2} F^2 c_\theta^7 M_\theta^8 M_K^4 s_\theta^3 \Lambda_2^2}{243 M_{\eta'}^{10}} - \\
& \frac{5120 \sqrt{2} F^2 c_\theta^7 M_\theta^6 M_K^6 s_\theta^3 \Lambda_2^2}{729 M_{\eta'}^{10}} + \frac{496 \sqrt{2} F^2 c_\theta^7 M_\theta^8 M_K^2 M_\pi^2 s_\theta^3 \Lambda_2^2}{243 M_{\eta'}^{10}} + \frac{1664 \sqrt{2} F^2 c_\theta^7 M_\theta^6 M_K^4 M_\pi^2 s_\theta^3 \Lambda_2^2}{243 M_{\eta'}^{10}} - \\
& \frac{56 \sqrt{2} F^2 c_\theta^7 M_\theta^8 M_\pi^4 s_\theta^3 \Lambda_2^2}{243 M_{\eta'}^{10}} - \frac{512 \sqrt{2} F^2 c_\theta^7 M_\theta^6 M_K^2 M_\pi^4 s_\theta^3 \Lambda_2^2}{243 M_{\eta'}^{10}} + \frac{800 \sqrt{2} F^2 c_\theta^7 M_\theta^6 M_\pi^6 s_\theta^3 \Lambda_2^2}{729 M_{\eta'}^{10}} -
\end{aligned}$$

$$\begin{aligned}
& \frac{1088 \sqrt{2} F^2 c_\theta^9 M_\theta^8 M_K^6 s_\theta^3 \Lambda_2^2}{81 M_\eta^2 M_{\eta'}^{10}} + \frac{1120 \sqrt{2} F^2 c_\theta^9 M_\theta^8 M_K^4 M_\pi^2 s_\theta^3 \Lambda_2^2}{81 M_\eta^2 M_{\eta'}^{10}} - \frac{416 \sqrt{2} F^2 c_\theta^9 M_\theta^8 M_K^2 M_\pi^4 s_\theta^3 \Lambda_2^2}{81 M_\eta^2 M_{\eta'}^{10}} + \\
& \frac{8 \sqrt{2} F^2 c_\theta^9 M_\theta^8 M_\pi^6 s_\theta^3 \Lambda_2^2}{27 M_\eta^2 M_{\eta'}^{10}} + \frac{256 \sqrt{2} F^2 c_\theta^5 M_\theta^6 M_K^4 s_\theta^3 \Lambda_2^2}{243 M_{\eta'}^8} + \frac{320 \sqrt{2} F^2 c_\theta^5 M_\theta^6 M_K^2 s_\theta^3 \Lambda_2^2}{243 M_{\eta'}^8} - \\
& \frac{248 \sqrt{2} F^2 c_\theta^5 M_\theta^6 M_K^2 M_\pi^2 s_\theta^3 \Lambda_2^2}{243 M_{\eta'}^8} - \frac{104 \sqrt{2} F^2 c_\theta^5 M_\theta^4 M_K^4 M_\pi^2 s_\theta^3 \Lambda_2^2}{81 M_{\eta'}^8} + \frac{28 \sqrt{2} F^2 c_\theta^5 M_\theta^6 M_\pi^4 s_\theta^3 \Lambda_2^2}{243 M_{\eta'}^8} + \\
& \frac{32 \sqrt{2} F^2 c_\theta^5 M_\theta^4 M_K^4 M_\pi^2 s_\theta^3 \Lambda_2^2}{81 M_{\eta'}^8} - \frac{50 \sqrt{2} F^2 c_\theta^5 M_\theta^4 M_\pi^6 s_\theta^3 \Lambda_2^2}{243 M_{\eta'}^8} + \frac{3136 \sqrt{2} F^2 c_\theta^9 M_\theta^8 M_K^6 s_\theta^3 \Lambda_2^2}{243 M_\eta^4 M_{\eta'}^8} - \\
& \frac{256 \sqrt{2} F^2 c_\theta^9 M_\theta^8 M_K^4 M_\pi^2 s_\theta^3 \Lambda_2^2}{27 M_\eta^4 M_{\eta'}^8} + \frac{32 \sqrt{2} F^2 c_\theta^9 M_\theta^8 M_K^2 M_\pi^4 s_\theta^3 \Lambda_2^2}{81 M_\eta^4 M_{\eta'}^8} + \frac{152 \sqrt{2} F^2 c_\theta^9 M_\theta^8 M_\pi^6 s_\theta^3 \Lambda_2^2}{243 M_\eta^4 M_{\eta'}^8} + \\
& \frac{320 \sqrt{2} F^2 c_\theta^7 M_\theta^8 M_K^4 s_\theta^3 \Lambda_2^2}{243 M_\eta^2 M_{\eta'}^8} + \frac{6656 \sqrt{2} F^2 c_\theta^7 M_\theta^6 M_K^6 s_\theta^3 \Lambda_2^2}{729 M_\eta^2 M_{\eta'}^8} - \frac{736 \sqrt{2} F^2 c_\theta^7 M_\theta^8 M_K^2 M_\pi^2 s_\theta^3 \Lambda_2^2}{243 M_\eta^2 M_{\eta'}^8} - \\
& \frac{56 \sqrt{2} F^2 c_\theta^7 M_\theta^6 M_K^4 M_\pi^2 s_\theta^3 \Lambda_2^2}{9 M_\eta^2 M_{\eta'}^8} + \frac{632 \sqrt{2} F^2 c_\theta^7 M_\theta^8 M_\pi^4 s_\theta^3 \Lambda_2^2}{243 M_\eta^2 M_{\eta'}^8} + \frac{76 \sqrt{2} F^2 c_\theta^7 M_\theta^6 M_K^2 M_\pi^4 s_\theta^3 \Lambda_2^2}{243 M_\eta^2 M_{\eta'}^8} + \\
& \frac{244 \sqrt{2} F^2 c_\theta^7 M_\theta^6 M_\pi^6 s_\theta^3 \Lambda_2^2}{729 M_\eta^2 M_{\eta'}^8} - \frac{64 \sqrt{2} F^2 c_\theta^3 M_\theta^4 M_K^4 s_\theta^3 \Lambda_2^2}{81 M_{\eta'}^6} + \frac{62 \sqrt{2} F^2 c_\theta^3 M_\theta^4 M_K^2 M_\pi^2 s_\theta^3 \Lambda_2^2}{81 M_{\eta'}^6} - \\
& \frac{7 \sqrt{2} F^2 c_\theta^3 M_\theta^4 M_\pi^4 s_\theta^3 \Lambda_2^2}{81 M_{\eta'}^6} - \frac{3520 \sqrt{2} F^2 c_\theta^9 M_\theta^8 M_K^6 s_\theta^3 \Lambda_2^2}{729 M_\eta^6 M_{\eta'}^6} - \frac{872 \sqrt{2} F^2 c_\theta^9 M_\theta^8 M_K^4 M_\pi^2 s_\theta^3 \Lambda_2^2}{243 M_\eta^6 M_{\eta'}^6} + \\
& \frac{1952 \sqrt{2} F^2 c_\theta^9 M_\theta^8 M_K^2 M_\pi^4 s_\theta^3 \Lambda_2^2}{243 M_\eta^6 M_{\eta'}^6} - \frac{800 \sqrt{2} F^2 c_\theta^9 M_\theta^8 M_\pi^6 s_\theta^3 \Lambda_2^2}{729 M_\eta^6 M_{\eta'}^6} - \frac{512 \sqrt{2} F^2 c_\theta^7 M_\theta^8 M_K^4 s_\theta^3 \Lambda_2^2}{243 M_\eta^4 M_{\eta'}^6} - \\
& \frac{1792 \sqrt{2} F^2 c_\theta^7 M_\theta^6 M_K^6 s_\theta^3 \Lambda_2^2}{243 M_\eta^4 M_{\eta'}^6} + \frac{976 \sqrt{2} F^2 c_\theta^7 M_\theta^8 M_K^2 M_\pi^2 s_\theta^3 \Lambda_2^2}{243 M_\eta^4 M_{\eta'}^6} + \frac{8 \sqrt{2} F^2 c_\theta^7 M_\theta^6 M_K^4 M_\pi^2 s_\theta^3 \Lambda_2^2}{81 M_\eta^4 M_{\eta'}^6} - \\
& \frac{680 \sqrt{2} F^2 c_\theta^7 M_\theta^8 M_\pi^4 s_\theta^3 \Lambda_2^2}{243 M_\eta^4 M_{\eta'}^6} + \frac{140 \sqrt{2} F^2 c_\theta^7 M_\theta^6 M_K^2 M_\pi^4 s_\theta^3 \Lambda_2^2}{27 M_\eta^4 M_{\eta'}^6} - \frac{356 \sqrt{2} F^2 c_\theta^7 M_\theta^6 M_\pi^6 s_\theta^3 \Lambda_2^2}{243 M_\eta^4 M_{\eta'}^6} - \\
& \frac{64 \sqrt{2} F^2 c_\theta^5 M_\theta^6 M_K^4 s_\theta^3 \Lambda_2^2}{81 M_\eta^2 M_{\eta'}^6} - \frac{304 \sqrt{2} F^2 c_\theta^5 M_\theta^4 M_K^6 s_\theta^3 \Lambda_2^2}{243 M_\eta^2 M_{\eta'}^6} + \frac{104 \sqrt{2} F^2 c_\theta^5 M_\theta^6 M_K^2 M_\pi^2 s_\theta^3 \Lambda_2^2}{81 M_\eta^2 M_{\eta'}^6} + \\
& \frac{4 \sqrt{2} F^2 c_\theta^5 M_\theta^4 M_K^4 M_\pi^2 s_\theta^3 \Lambda_2^2}{27 M_\eta^2 M_{\eta'}^6} - \frac{76 \sqrt{2} F^2 c_\theta^5 M_\theta^6 M_\pi^4 s_\theta^3 \Lambda_2^2}{81 M_\eta^2 M_{\eta'}^6} + \frac{46 \sqrt{2} F^2 c_\theta^5 M_\theta^4 M_K^2 M_\pi^4 s_\theta^3 \Lambda_2^2}{81 M_\eta^2 M_{\eta'}^6} - \\
& \frac{32 \sqrt{2} F^2 c_\theta^5 M_\theta^4 M_\pi^6 s_\theta^3 \Lambda_2^2}{243 M_\eta^2 M_{\eta'}^6} - \frac{832 \sqrt{2} F^2 c_\theta^9 M_\theta^8 M_K^6 s_\theta^3 \Lambda_2^2}{243 M_\eta^8 M_{\eta'}^4} + \frac{632 \sqrt{2} F^2 c_\theta^9 M_\theta^8 M_K^4 M_\pi^2 s_\theta^3 \Lambda_2^2}{81 M_\eta^8 M_{\eta'}^4} - \\
& \frac{160 \sqrt{2} F^2 c_\theta^9 M_\theta^8 M_K^2 M_\pi^4 s_\theta^3 \Lambda_2^2}{27 M_\eta^8 M_{\eta'}^4} + \frac{376 \sqrt{2} F^2 c_\theta^9 M_\theta^8 M_\pi^6 s_\theta^3 \Lambda_2^2}{243 M_\eta^8 M_{\eta'}^4} + \frac{704 \sqrt{2} F^2 c_\theta^7 M_\theta^8 M_K^4 s_\theta^3 \Lambda_2^2}{243 M_\eta^6 M_{\eta'}^4} +
\end{aligned}$$

$$\begin{aligned}
& \frac{1024 \sqrt{2} F^2 c_\theta^7 M_\theta^6 M_K^6 s_\theta^3 \Lambda_2^2}{729 M_\eta^6 M_{\eta'}^4} - \frac{736 \sqrt{2} F^2 c_\theta^7 M_\theta^8 M_K^2 M_\pi^2 s_\theta^3 \Lambda_2^2}{243 M_\eta^6 M_{\eta'}^4} + \frac{1928 \sqrt{2} F^2 c_\theta^7 M_\theta^6 M_K^4 M_\pi^2 s_\theta^3 \Lambda_2^2}{243 M_\eta^6 M_{\eta'}^4} + \\
& \frac{104 \sqrt{2} F^2 c_\theta^7 M_\theta^8 M_K^4 s_\theta^3 \Lambda_2^2}{243 M_\eta^6 M_{\eta'}^4} - \frac{2396 \sqrt{2} F^2 c_\theta^7 M_\theta^6 M_K^2 M_\pi^4 s_\theta^3 \Lambda_2^2}{243 M_\eta^6 M_{\eta'}^4} + \frac{1244 \sqrt{2} F^2 c_\theta^7 M_\theta^6 M_\pi^6 s_\theta^3 \Lambda_2^2}{729 M_\eta^6 M_{\eta'}^4} + \\
& \frac{32 \sqrt{2} F^2 c_\theta^5 M_\theta^6 M_K^4 s_\theta^3 \Lambda_2^2}{27 M_\eta^4 M_{\eta'}^4} + \frac{176 \sqrt{2} F^2 c_\theta^5 M_\theta^4 M_K^6 s_\theta^3 \Lambda_2^2}{243 M_\eta^4 M_{\eta'}^4} - \frac{16 \sqrt{2} F^2 c_\theta^5 M_\theta^6 M_K^2 M_\pi^2 s_\theta^3 \Lambda_2^2}{9 M_\eta^4 M_{\eta'}^4} + \\
& \frac{28 \sqrt{2} F^2 c_\theta^5 M_\theta^4 M_K^4 M_\pi^2 s_\theta^3 \Lambda_2^2}{27 M_\eta^4 M_{\eta'}^4} + \frac{28 \sqrt{2} F^2 c_\theta^5 M_\theta^6 M_\pi^4 s_\theta^3 \Lambda_2^2}{27 M_\eta^4 M_{\eta'}^4} - \frac{110 \sqrt{2} F^2 c_\theta^5 M_\theta^4 M_K^2 M_\pi^4 s_\theta^3 \Lambda_2^2}{81 M_\eta^4 M_{\eta'}^4} + \\
& \frac{64 \sqrt{2} F^2 c_\theta^5 M_\theta^4 M_\pi^6 s_\theta^3 \Lambda_2^2}{243 M_\eta^4 M_{\eta'}^4} + \frac{2816 \sqrt{2} F^2 c_\theta^7 M_\theta^6 M_K^6 s_\theta^3 \Lambda_2^2}{729 M_\eta^8 M_{\eta'}^2} - \frac{2104 \sqrt{2} F^2 c_\theta^7 M_\theta^6 M_K^4 M_\pi^2 s_\theta^3 \Lambda_2^2}{243 M_\eta^8 M_{\eta'}^2} + \\
& \frac{524 \sqrt{2} F^2 c_\theta^7 M_\theta^6 M_K^2 M_\pi^4 s_\theta^3 \Lambda_2^2}{81 M_\eta^8 M_{\eta'}^2} - \frac{1220 \sqrt{2} F^2 c_\theta^7 M_\theta^6 M_\pi^6 s_\theta^3 \Lambda_2^2}{729 M_\eta^8 M_{\eta'}^2} - \frac{352 \sqrt{2} F^2 c_\theta^5 M_\theta^6 M_K^4 s_\theta^3 \Lambda_2^2}{243 M_\eta^6 M_{\eta'}^2} + \\
& \frac{368 \sqrt{2} F^2 c_\theta^5 M_\theta^6 M_K^2 M_\pi^2 s_\theta^3 \Lambda_2^2}{243 M_\eta^6 M_{\eta'}^2} - \frac{124 \sqrt{2} F^2 c_\theta^5 M_\theta^4 M_K^4 M_\pi^2 s_\theta^3 \Lambda_2^2}{81 M_\eta^6 M_{\eta'}^2} - \frac{52 \sqrt{2} F^2 c_\theta^5 M_\theta^6 M_\pi^4 s_\theta^3 \Lambda_2^2}{243 M_\eta^6 M_{\eta'}^2} + \\
& \frac{122 \sqrt{2} F^2 c_\theta^5 M_\theta^4 M_K^2 M_\pi^4 s_\theta^3 \Lambda_2^2}{81 M_\eta^6 M_{\eta'}^2} - \frac{16 \sqrt{2} F^2 c_\theta^5 M_\theta^4 M_\pi^6 s_\theta^3 \Lambda_2^2}{81 M_\eta^6 M_{\eta'}^2} + \frac{1024 F^2 c_\theta^6 M_\theta^6 M_K^6 s_\theta^4 \Lambda_2^2}{729 M_\eta^{10}} - \\
& \frac{832 F^2 c_\theta^6 M_\theta^6 M_K^4 M_\pi^2 s_\theta^4 \Lambda_2^2}{243 M_\eta^{10}} + \frac{640 F^2 c_\theta^6 M_\theta^6 M_K^2 M_\pi^4 s_\theta^4 \Lambda_2^2}{243 M_\eta^{10}} - \frac{448 F^2 c_\theta^6 M_\theta^6 M_\pi^6 s_\theta^4 \Lambda_2^2}{729 M_\eta^{10}} - \\
& \frac{128 F^2 c_\theta^4 M_\theta^6 M_K^4 s_\theta^4 \Lambda_2^2}{243 M_\eta^8} - \frac{160 F^2 c_\theta^4 M_\theta^4 M_K^6 s_\theta^4 \Lambda_2^2}{81 M_\eta^8} + \frac{208 F^2 c_\theta^4 M_\theta^6 M_K^2 M_\pi^2 s_\theta^4 \Lambda_2^2}{243 M_\eta^8} + \\
& \frac{26 F^2 c_\theta^4 M_\theta^4 M_K^4 M_\pi^2 s_\theta^4 \Lambda_2^2}{9 M_\eta^8} - \frac{80 F^2 c_\theta^4 M_\theta^6 M_\pi^4 s_\theta^4 \Lambda_2^2}{243 M_\eta^8} - \frac{26 F^2 c_\theta^4 M_\theta^4 M_K^2 M_\pi^4 s_\theta^4 \Lambda_2^2}{27 M_\eta^8} - \frac{19 F^2 c_\theta^4 M_\theta^4 M_\pi^6 s_\theta^4 \Lambda_2^2}{162 M_\eta^8} + \\
& \frac{32 F^2 c_\theta^2 M_\theta^4 M_K^4 s_\theta^4 \Lambda_2^2}{27 M_\eta^6} - \frac{28 F^2 c_\theta^2 M_\theta^4 M_K^2 M_\pi^2 s_\theta^4 \Lambda_2^2}{27 M_\eta^6} + \frac{14 F^2 c_\theta^2 M_\theta^4 M_\pi^4 s_\theta^4 \Lambda_2^2}{27 M_\eta^6} - \frac{3200 F^2 c_\theta^8 M_\theta^8 M_K^6 s_\theta^4 \Lambda_2^2}{243 M_\eta^{12}} + \\
& \frac{520 F^2 c_\theta^8 M_\theta^8 M_K^4 M_\pi^2 s_\theta^4 \Lambda_2^2}{27 M_\eta^{12}} - \frac{520 F^2 c_\theta^8 M_\theta^8 M_K^2 M_\pi^4 s_\theta^4 \Lambda_2^2}{81 M_\eta^{12}} - \frac{190 F^2 c_\theta^8 M_\theta^8 M_\pi^6 s_\theta^4 \Lambda_2^2}{243 M_\eta^{12}} + \\
& \frac{256 F^2 c_\theta^6 M_\theta^6 M_K^4 s_\theta^4 \Lambda_2^2}{243 M_\eta^{10}} + \frac{2560 F^2 c_\theta^6 M_\theta^6 M_K^6 s_\theta^4 \Lambda_2^2}{243 M_\eta^{10}} - \frac{416 F^2 c_\theta^6 M_\theta^8 M_K^2 M_\pi^2 s_\theta^4 \Lambda_2^2}{243 M_\eta^{10}} - \\
& \frac{416 F^2 c_\theta^6 M_\theta^6 M_K^4 M_\pi^2 s_\theta^4 \Lambda_2^2}{27 M_\eta^{10}} + \frac{160 F^2 c_\theta^6 M_\theta^8 M_\pi^4 s_\theta^4 \Lambda_2^2}{243 M_\eta^{10}} + \frac{416 F^2 c_\theta^6 M_\theta^6 M_K^2 M_\pi^4 s_\theta^4 \Lambda_2^2}{81 M_\eta^{10}} + \\
& \frac{152 F^2 c_\theta^6 M_\theta^6 M_\pi^6 s_\theta^4 \Lambda_2^2}{243 M_\eta^{10}} + \frac{3616 F^2 c_\theta^8 M_\theta^8 M_K^6 s_\theta^4 \Lambda_2^2}{243 M_\eta^2 M_\eta^{10}} - \frac{3256 F^2 c_\theta^8 M_\theta^8 M_K^4 M_\pi^2 s_\theta^4 \Lambda_2^2}{81 M_\eta^2 M_\eta^{10}} + \\
& \frac{1264 F^2 c_\theta^8 M_\theta^8 M_K^2 M_\pi^4 s_\theta^4 \Lambda_2^2}{81 M_\eta^2 M_\eta^{10}} - \frac{880 F^2 c_\theta^8 M_\theta^8 M_\pi^6 s_\theta^4 \Lambda_2^2}{243 M_\eta^2 M_\eta^{10}} - \frac{128 F^2 c_\theta^4 M_\theta^6 M_K^4 s_\theta^4 \Lambda_2^2}{243 M_\eta^8} -
\end{aligned}$$

$$\begin{aligned}
& \frac{160 F^2 c_\theta^4 M_\theta^4 M_K^6 s_\theta^4 \Lambda_2^2}{81 M_{\eta'}^8} + \frac{208 F^2 c_\theta^4 M_\theta^6 M_K^2 M_\pi^2 s_\theta^4 \Lambda_2^2}{243 M_{\eta'}^8} + \frac{26 F^2 c_\theta^4 M_\theta^4 M_K^4 M_\pi^2 s_\theta^4 \Lambda_2^2}{9 M_{\eta'}^8} - \\
& \frac{80 F^2 c_\theta^4 M_\theta^6 M_\pi^4 s_\theta^4 \Lambda_2^2}{243 M_{\eta'}^8} - \frac{26 F^2 c_\theta^4 M_\theta^4 M_K^2 M_\pi^4 s_\theta^4 \Lambda_2^2}{27 M_{\eta'}^8} - \frac{19 F^2 c_\theta^4 M_\theta^4 M_\pi^6 s_\theta^4 \Lambda_2^2}{162 M_{\eta'}^8} - \frac{4576 F^2 c_\theta^8 M_\theta^8 M_K^6 s_\theta^4 \Lambda_2^2}{243 M_\eta^4 M_{\eta'}^8} + \\
& \frac{4544 F^2 c_\theta^8 M_\theta^8 M_K^4 M_\pi^2 s_\theta^4 \Lambda_2^2}{81 M_\eta^4 M_{\eta'}^8} - \frac{680 F^2 c_\theta^8 M_\theta^8 M_K^2 M_\pi^4 s_\theta^4 \Lambda_2^2}{27 M_\eta^4 M_{\eta'}^8} + \frac{1384 F^2 c_\theta^8 M_\theta^8 M_\pi^6 s_\theta^4 \Lambda_2^2}{243 M_\eta^4 M_{\eta'}^8} + \\
& \frac{1520 F^2 c_\theta^6 M_\theta^6 M_K^4 s_\theta^4 \Lambda_2^2}{243 M_\eta^2 M_{\eta'}^8} - \frac{8992 F^2 c_\theta^6 M_\theta^6 M_K^6 s_\theta^4 \Lambda_2^2}{729 M_\eta^2 M_{\eta'}^8} - \frac{760 F^2 c_\theta^6 M_\theta^8 M_K^2 M_\pi^2 s_\theta^4 \Lambda_2^2}{243 M_\eta^2 M_{\eta'}^8} + \\
& \frac{2152 F^2 c_\theta^6 M_\theta^6 M_K^4 M_\pi^2 s_\theta^4 \Lambda_2^2}{81 M_\eta^2 M_{\eta'}^8} + \frac{536 F^2 c_\theta^6 M_\theta^8 M_\pi^4 s_\theta^4 \Lambda_2^2}{243 M_\eta^2 M_{\eta'}^8} - \frac{2048 F^2 c_\theta^6 M_\theta^6 M_K^2 M_\pi^4 s_\theta^4 \Lambda_2^2}{243 M_\eta^2 M_{\eta'}^8} + \\
& \frac{952 F^2 c_\theta^6 M_\theta^6 M_\pi^6 s_\theta^4 \Lambda_2^2}{729 M_\eta^2 M_{\eta'}^8} + \frac{32 F^2 c_\theta^2 M_\theta^4 M_K^4 s_\theta^4 \Lambda_2^2}{81 M_{\eta'}^6} - \frac{52 F^2 c_\theta^2 M_\theta^4 M_K^2 M_\pi^2 s_\theta^4 \Lambda_2^2}{81 M_{\eta'}^6} + \frac{20 F^2 c_\theta^2 M_\theta^4 M_\pi^4 s_\theta^4 \Lambda_2^2}{81 M_{\eta'}^6} + \\
& \frac{6080 F^2 c_\theta^8 M_\theta^8 M_K^6 s_\theta^4 \Lambda_2^2}{243 M_\eta^6 M_{\eta'}^6} - \frac{1456 F^2 c_\theta^8 M_\theta^8 M_K^4 M_\pi^2 s_\theta^4 \Lambda_2^2}{27 M_\eta^6 M_{\eta'}^6} + \frac{1408 F^2 c_\theta^8 M_\theta^8 M_K^2 M_\pi^4 s_\theta^4 \Lambda_2^2}{81 M_\eta^6 M_{\eta'}^6} - \\
& \frac{440 F^2 c_\theta^8 M_\theta^8 M_\pi^6 s_\theta^4 \Lambda_2^2}{243 M_\eta^6 M_{\eta'}^6} - \frac{2432 F^2 c_\theta^6 M_\theta^8 M_K^4 s_\theta^4 \Lambda_2^2}{243 M_\eta^4 M_{\eta'}^6} + \frac{10816 F^2 c_\theta^6 M_\theta^6 M_K^6 s_\theta^4 \Lambda_2^2}{729 M_\eta^4 M_{\eta'}^6} + \\
& \frac{2068 F^2 c_\theta^6 M_\theta^8 M_K^2 M_\pi^2 s_\theta^4 \Lambda_2^2}{243 M_\eta^4 M_{\eta'}^6} - \frac{8464 F^2 c_\theta^6 M_\theta^6 M_K^4 M_\pi^2 s_\theta^4 \Lambda_2^2}{243 M_\eta^4 M_{\eta'}^6} - \frac{788 F^2 c_\theta^6 M_\theta^8 M_\pi^4 s_\theta^4 \Lambda_2^2}{243 M_\eta^4 M_{\eta'}^6} + \\
& \frac{2728 F^2 c_\theta^6 M_\theta^6 M_K^2 M_\pi^4 s_\theta^4 \Lambda_2^2}{243 M_\eta^4 M_{\eta'}^6} - \frac{952 F^2 c_\theta^6 M_\theta^6 M_\pi^6 s_\theta^4 \Lambda_2^2}{729 M_\eta^4 M_{\eta'}^6} - \frac{496 F^2 c_\theta^4 M_\theta^6 M_K^4 s_\theta^4 \Lambda_2^2}{243 M_\eta^2 M_{\eta'}^6} + \\
& \frac{512 F^2 c_\theta^4 M_\theta^4 M_K^6 s_\theta^4 \Lambda_2^2}{243 M_\eta^2 M_{\eta'}^6} + \frac{248 F^2 c_\theta^4 M_\theta^6 M_K^2 M_\pi^2 s_\theta^4 \Lambda_2^2}{243 M_\eta^2 M_{\eta'}^6} - \frac{32 F^2 c_\theta^4 M_\theta^4 M_K^4 M_\pi^2 s_\theta^4 \Lambda_2^2}{9 M_\eta^2 M_{\eta'}^6} - \\
& \frac{184 F^2 c_\theta^4 M_\theta^6 M_\pi^4 s_\theta^4 \Lambda_2^2}{243 M_\eta^2 M_{\eta'}^6} + \frac{64 F^2 c_\theta^4 M_\theta^4 M_K^2 M_\pi^4 s_\theta^4 \Lambda_2^2}{81 M_\eta^2 M_{\eta'}^6} - \frac{2 F^2 c_\theta^4 M_\theta^4 M_\pi^6 s_\theta^4 \Lambda_2^2}{243 M_\eta^2 M_{\eta'}^6} - \frac{4256 F^2 c_\theta^8 M_\theta^8 M_K^6 s_\theta^4 \Lambda_2^2}{243 M_\eta^8 M_{\eta'}^4} + \\
& \frac{1888 F^2 c_\theta^8 M_\theta^8 M_K^4 M_\pi^2 s_\theta^4 \Lambda_2^2}{81 M_\eta^8 M_{\eta'}^4} - \frac{104 F^2 c_\theta^8 M_\theta^8 M_K^2 M_\pi^4 s_\theta^4 \Lambda_2^2}{27 M_\eta^8 M_{\eta'}^4} - \frac{742 F^2 c_\theta^8 M_\theta^8 M_\pi^6 s_\theta^4 \Lambda_2^2}{243 M_\eta^8 M_{\eta'}^4} + \\
& \frac{1424 F^2 c_\theta^6 M_\theta^8 M_K^4 s_\theta^4 \Lambda_2^2}{243 M_\eta^6 M_{\eta'}^4} - \frac{1376 F^2 c_\theta^6 M_\theta^6 M_K^6 s_\theta^4 \Lambda_2^2}{81 M_\eta^6 M_{\eta'}^4} - \frac{640 F^2 c_\theta^6 M_\theta^8 M_K^2 M_\pi^2 s_\theta^4 \Lambda_2^2}{243 M_\eta^6 M_{\eta'}^4} + \\
& \frac{2504 F^2 c_\theta^6 M_\theta^6 M_K^4 M_\pi^2 s_\theta^4 \Lambda_2^2}{81 M_\eta^6 M_{\eta'}^4} + \frac{512 F^2 c_\theta^6 M_\theta^8 M_\pi^4 s_\theta^4 \Lambda_2^2}{243 M_\eta^6 M_{\eta'}^4} - \frac{496 F^2 c_\theta^6 M_\theta^6 M_K^2 M_\pi^4 s_\theta^4 \Lambda_2^2}{81 M_\eta^6 M_{\eta'}^4} - \\
& \frac{56 F^2 c_\theta^6 M_\theta^6 M_\pi^6 s_\theta^4 \Lambda_2^2}{81 M_\eta^6 M_{\eta'}^4} + \frac{256 F^2 c_\theta^4 M_\theta^6 M_K^4 s_\theta^4 \Lambda_2^2}{81 M_\eta^4 M_{\eta'}^4} - \frac{496 F^2 c_\theta^4 M_\theta^4 M_K^6 s_\theta^4 \Lambda_2^2}{243 M_\eta^4 M_{\eta'}^4} - \frac{176 F^2 c_\theta^4 M_\theta^6 M_K^2 M_\pi^2 s_\theta^4 \Lambda_2^2}{81 M_\eta^4 M_{\eta'}^4} + \\
& \frac{4 F^2 c_\theta^4 M_\theta^4 M_K^4 M_\pi^2 s_\theta^4 \Lambda_2^2}{M_\eta^4 M_{\eta'}^4} + \frac{64 F^2 c_\theta^4 M_\theta^6 M_\pi^4 s_\theta^4 \Lambda_2^2}{81 M_\eta^4 M_{\eta'}^4} - \frac{80 F^2 c_\theta^4 M_\theta^4 M_K^2 M_\pi^4 s_\theta^4 \Lambda_2^2}{81 M_\eta^4 M_{\eta'}^4} + \frac{7 F^2 c_\theta^4 M_\theta^4 M_\pi^6 s_\theta^4 \Lambda_2^2}{243 M_\eta^4 M_{\eta'}^4} -
\end{aligned}$$

$$\begin{aligned}
& \frac{128 F^2 c_\theta^8 M_\theta^8 M_K^6 S_\theta^4 \Lambda_2^2}{81 M_\eta^{10} M_\eta^2} + \frac{104 F^2 c_\theta^8 M_\theta^8 M_K^4 M_\pi^2 S_\theta^4 \Lambda_2^2}{27 M_\eta^{10} M_\eta^2} - \frac{80 F^2 c_\theta^8 M_\theta^8 M_K^2 M_\pi^4 S_\theta^4 \Lambda_2^2}{27 M_\eta^{10} M_\eta^2} + \\
& \frac{56 F^2 c_\theta^8 M_\theta^8 M_\pi^6 S_\theta^4 \Lambda_2^2}{81 M_\eta^{10} M_\eta^2} + \frac{352 F^2 c_\theta^6 M_\theta^8 M_K^4 S_\theta^4 \Lambda_2^2}{243 M_\eta^8 M_\eta^2} + \frac{8576 F^2 c_\theta^6 M_\theta^6 M_K^6 S_\theta^4 \Lambda_2^2}{729 M_\eta^8 M_\eta^2} - \frac{572 F^2 c_\theta^6 M_\theta^8 M_K^2 M_\pi^2 S_\theta^4 \Lambda_2^2}{243 M_\eta^8 M_\eta^2} - \\
& \frac{3488 F^2 c_\theta^6 M_\theta^6 M_K^4 M_\pi^2 S_\theta^4 \Lambda_2^2}{243 M_\eta^8 M_\eta^2} + \frac{220 F^2 c_\theta^6 M_\theta^8 M_\pi^4 S_\theta^4 \Lambda_2^2}{243 M_\eta^8 M_\eta^2} + \frac{200 F^2 c_\theta^6 M_\theta^6 M_K^2 M_\pi^4 S_\theta^4 \Lambda_2^2}{243 M_\eta^8 M_\eta^2} + \\
& \frac{1936 F^2 c_\theta^6 M_\theta^6 M_\pi^6 S_\theta^4 \Lambda_2^2}{729 M_\eta^8 M_\eta^2} - \frac{496 F^2 c_\theta^4 M_\theta^6 M_K^4 S_\theta^4 \Lambda_2^2}{243 M_\eta^6 M_\eta^2} + \frac{512 F^2 c_\theta^4 M_\theta^4 M_K^6 S_\theta^4 \Lambda_2^2}{243 M_\eta^6 M_\eta^2} + \\
& \frac{248 F^2 c_\theta^4 M_\theta^6 M_K^2 M_\pi^2 S_\theta^4 \Lambda_2^2}{243 M_\eta^6 M_\eta^2} - \frac{32 F^2 c_\theta^4 M_\theta^4 M_K^4 M_\pi^2 S_\theta^4 \Lambda_2^2}{9 M_\eta^6 M_\eta^2} - \frac{184 F^2 c_\theta^4 M_\theta^6 M_\pi^4 S_\theta^4 \Lambda_2^2}{243 M_\eta^6 M_\eta^2} + \\
& \frac{64 F^2 c_\theta^4 M_\theta^4 M_K^2 M_\pi^4 S_\theta^4 \Lambda_2^2}{81 M_\eta^6 M_\eta^2} - \frac{2 F^2 c_\theta^4 M_\theta^4 M_\pi^6 S_\theta^4 \Lambda_2^2}{243 M_\eta^6 M_\eta^2} + \frac{1024 \sqrt{2} F^2 c_\theta^5 M_\theta^6 M_K^6 S_\theta^5 \Lambda_2^2}{243 M_\eta^{10}} - \\
& \frac{704 \sqrt{2} F^2 c_\theta^5 M_\theta^6 M_K^4 M_\pi^2 S_\theta^5 \Lambda_2^2}{81 M_\eta^{10}} + \frac{160 \sqrt{2} F^2 c_\theta^5 M_\theta^6 M_K^2 M_\pi^4 S_\theta^5 \Lambda_2^2}{27 M_\eta^{10}} - \frac{352 \sqrt{2} F^2 c_\theta^5 M_\theta^6 M_\pi^6 S_\theta^5 \Lambda_2^2}{243 M_\eta^{10}} - \\
& \frac{256 \sqrt{2} F^2 c_\theta^3 M_\theta^6 M_K^4 S_\theta^5 \Lambda_2^2}{243 M_\eta^8} - \frac{320 \sqrt{2} F^2 c_\theta^3 M_\theta^4 M_K^6 S_\theta^5 \Lambda_2^2}{243 M_\eta^8} + \frac{248 \sqrt{2} F^2 c_\theta^3 M_\theta^6 M_K^2 M_\pi^2 S_\theta^5 \Lambda_2^2}{243 M_\eta^8} + \\
& \frac{104 \sqrt{2} F^2 c_\theta^3 M_\theta^4 M_K^4 M_\pi^2 S_\theta^5 \Lambda_2^2}{81 M_\eta^8} - \frac{28 \sqrt{2} F^2 c_\theta^3 M_\theta^6 M_\pi^4 S_\theta^5 \Lambda_2^2}{243 M_\eta^8} - \frac{32 \sqrt{2} F^2 c_\theta^3 M_\theta^4 M_K^2 M_\pi^4 S_\theta^5 \Lambda_2^2}{81 M_\eta^8} + \\
& \frac{50 \sqrt{2} F^2 c_\theta^3 M_\theta^4 M_\pi^6 S_\theta^5 \Lambda_2^2}{243 M_\eta^8} + \frac{32 \sqrt{2} F^2 c_\theta M_\theta^4 M_K^4 S_\theta^5 \Lambda_2^2}{81 M_\eta^6} - \frac{16 \sqrt{2} F^2 c_\theta M_\theta^4 M_K^2 M_\pi^2 S_\theta^5 \Lambda_2^2}{81 M_\eta^6} - \\
& \frac{16 \sqrt{2} F^2 c_\theta M_\theta^4 M_\pi^4 S_\theta^5 \Lambda_2^2}{81 M_\eta^6} + \frac{1280 \sqrt{2} F^2 c_\theta^7 M_\theta^8 M_K^6 S_\theta^5 \Lambda_2^2}{243 M_\eta^{12}} - \frac{880 \sqrt{2} F^2 c_\theta^7 M_\theta^8 M_K^4 M_\pi^2 S_\theta^5 \Lambda_2^2}{81 M_\eta^{12}} + \\
& \frac{200 \sqrt{2} F^2 c_\theta^7 M_\theta^8 M_K^2 M_\pi^4 S_\theta^5 \Lambda_2^2}{27 M_\eta^{12}} - \frac{440 \sqrt{2} F^2 c_\theta^7 M_\theta^8 M_\pi^6 S_\theta^5 \Lambda_2^2}{243 M_\eta^{12}} - \frac{1024 \sqrt{2} F^2 c_\theta^5 M_\theta^6 M_K^6 S_\theta^5 \Lambda_2^2}{243 M_\eta^{10}} + \\
& \frac{704 \sqrt{2} F^2 c_\theta^5 M_\theta^6 M_K^4 M_\pi^2 S_\theta^5 \Lambda_2^2}{81 M_\eta^{10}} - \frac{160 \sqrt{2} F^2 c_\theta^5 M_\theta^6 M_K^2 M_\pi^4 S_\theta^5 \Lambda_2^2}{27 M_\eta^{10}} + \frac{352 \sqrt{2} F^2 c_\theta^5 M_\theta^6 M_\pi^6 S_\theta^5 \Lambda_2^2}{243 M_\eta^{10}} + \\
& \frac{640 \sqrt{2} F^2 c_\theta^7 M_\theta^8 M_K^6 S_\theta^5 \Lambda_2^2}{81 M_\eta^2 M_\eta^{10}} + \frac{976 \sqrt{2} F^2 c_\theta^7 M_\theta^8 M_K^4 M_\pi^2 S_\theta^5 \Lambda_2^2}{81 M_\eta^2 M_\eta^{10}} - \frac{1400 \sqrt{2} F^2 c_\theta^7 M_\theta^8 M_K^2 M_\pi^4 S_\theta^5 \Lambda_2^2}{81 M_\eta^2 M_\eta^{10}} + \\
& \frac{16 \sqrt{2} F^2 c_\theta^7 M_\theta^8 M_\pi^6 S_\theta^5 \Lambda_2^2}{9 M_\eta^2 M_\eta^{10}} + \frac{64 \sqrt{2} F^2 c_\theta^3 M_\theta^4 M_K^6 S_\theta^5 \Lambda_2^2}{81 M_\eta^8} - \frac{44 \sqrt{2} F^2 c_\theta^3 M_\theta^4 M_K^4 M_\pi^2 S_\theta^5 \Lambda_2^2}{27 M_\eta^8} + \\
& \frac{10 \sqrt{2} F^2 c_\theta^3 M_\theta^4 M_K^2 M_\pi^4 S_\theta^5 \Lambda_2^2}{9 M_\eta^8} - \frac{22 \sqrt{2} F^2 c_\theta^3 M_\theta^4 M_\pi^6 S_\theta^5 \Lambda_2^2}{81 M_\eta^8} - \frac{4736 \sqrt{2} F^2 c_\theta^7 M_\theta^8 M_K^6 S_\theta^5 \Lambda_2^2}{243 M_\eta^4 M_\eta^8} - \\
& \frac{976 \sqrt{2} F^2 c_\theta^7 M_\theta^8 M_K^4 M_\pi^2 S_\theta^5 \Lambda_2^2}{81 M_\eta^4 M_\eta^8} + \frac{1888 \sqrt{2} F^2 c_\theta^7 M_\theta^8 M_K^2 M_\pi^4 S_\theta^5 \Lambda_2^2}{81 M_\eta^4 M_\eta^8} - \frac{1240 \sqrt{2} F^2 c_\theta^7 M_\theta^8 M_\pi^6 S_\theta^5 \Lambda_2^2}{243 M_\eta^4 M_\eta^8} -
\end{aligned}$$

$$\begin{aligned}
& \frac{1120 \sqrt{2} F^2 c_\theta^5 M_0^8 M_K^4 s_\theta^5 \Lambda_2^2}{243 M_\eta^2 M_{\eta'}^8} - \frac{640 \sqrt{2} F^2 c_\theta^5 M_0^6 M_K^6 s_\theta^5 \Lambda_2^2}{243 M_\eta^2 M_{\eta'}^8} + \frac{1112 \sqrt{2} F^2 c_\theta^5 M_0^8 M_K^2 M_\pi^2 s_\theta^5 \Lambda_2^2}{243 M_\eta^2 M_{\eta'}^8} - \\
& \frac{2336 \sqrt{2} F^2 c_\theta^5 M_0^6 M_K^4 M_\pi^2 s_\theta^5 \Lambda_2^2}{243 M_\eta^2 M_{\eta'}^8} - \frac{136 \sqrt{2} F^2 c_\theta^5 M_0^8 M_\pi^8 s_\theta^5 \Lambda_2^2}{243 M_\eta^2 M_{\eta'}^8} + \frac{2704 \sqrt{2} F^2 c_\theta^5 M_0^6 M_K^4 M_\pi^2 s_\theta^5 \Lambda_2^2}{243 M_\eta^2 M_{\eta'}^8} - \\
& \frac{304 \sqrt{2} F^2 c_\theta^5 M_0^6 M_\pi^6 s_\theta^5 \Lambda_2^2}{243 M_\eta^2 M_{\eta'}^8} + \frac{1408 \sqrt{2} F^2 c_\theta^7 M_0^8 M_K^6 s_\theta^5 \Lambda_2^2}{81 M_\eta^6 M_{\eta'}^6} + \frac{1520 \sqrt{2} F^2 c_\theta^7 M_0^8 M_K^4 M_\pi^2 s_\theta^5 \Lambda_2^2}{81 M_\eta^6 M_{\eta'}^6} - \\
& \frac{2368 \sqrt{2} F^2 c_\theta^7 M_0^8 M_K^2 M_\pi^4 s_\theta^5 \Lambda_2^2}{81 M_\eta^6 M_{\eta'}^6} + \frac{520 \sqrt{2} F^2 c_\theta^7 M_0^8 M_\pi^6 s_\theta^5 \Lambda_2^2}{81 M_\eta^6 M_{\eta'}^6} + \frac{416 \sqrt{2} F^2 c_\theta^5 M_0^8 M_K^4 s_\theta^5 \Lambda_2^2}{81 M_\eta^4 M_{\eta'}^6} + \\
& \frac{640 \sqrt{2} F^2 c_\theta^5 M_0^6 M_K^6 s_\theta^5 \Lambda_2^2}{81 M_\eta^4 M_{\eta'}^6} - \frac{616 \sqrt{2} F^2 c_\theta^5 M_0^8 M_K^2 M_\pi^2 s_\theta^5 \Lambda_2^2}{81 M_\eta^4 M_{\eta'}^6} + \frac{32 \sqrt{2} F^2 c_\theta^5 M_0^6 M_K^4 M_\pi^2 s_\theta^5 \Lambda_2^2}{3 M_\eta^4 M_{\eta'}^6} + \\
& \frac{344 \sqrt{2} F^2 c_\theta^5 M_0^8 M_\pi^4 s_\theta^5 \Lambda_2^2}{81 M_\eta^4 M_{\eta'}^6} - \frac{128 \sqrt{2} F^2 c_\theta^5 M_0^6 M_K^2 M_\pi^4 s_\theta^5 \Lambda_2^2}{9 M_\eta^4 M_{\eta'}^6} + \frac{224 \sqrt{2} F^2 c_\theta^5 M_0^6 M_\pi^6 s_\theta^5 \Lambda_2^2}{81 M_\eta^4 M_{\eta'}^6} + \\
& \frac{352 \sqrt{2} F^2 c_\theta^3 M_0^6 M_K^4 s_\theta^5 \Lambda_2^2}{243 M_\eta^2 M_{\eta'}^6} - \frac{368 \sqrt{2} F^2 c_\theta^3 M_0^6 M_K^2 M_\pi^2 s_\theta^5 \Lambda_2^2}{243 M_\eta^2 M_{\eta'}^6} + \frac{124 \sqrt{2} F^2 c_\theta^3 M_0^4 M_K^4 M_\pi^2 s_\theta^5 \Lambda_2^2}{81 M_\eta^2 M_{\eta'}^6} + \\
& \frac{52 \sqrt{2} F^2 c_\theta^3 M_0^6 M_\pi^4 s_\theta^5 \Lambda_2^2}{243 M_\eta^2 M_{\eta'}^6} - \frac{122 \sqrt{2} F^2 c_\theta^3 M_0^4 M_K^2 M_\pi^4 s_\theta^5 \Lambda_2^2}{81 M_\eta^2 M_{\eta'}^6} + \frac{16 \sqrt{2} F^2 c_\theta^3 M_0^4 M_\pi^6 s_\theta^5 \Lambda_2^2}{81 M_\eta^2 M_{\eta'}^6} - \\
& \frac{640 \sqrt{2} F^2 c_\theta^7 M_0^8 M_K^6 s_\theta^5 \Lambda_2^2}{243 M_\eta^8 M_{\eta'}^4} - \frac{2096 \sqrt{2} F^2 c_\theta^7 M_0^8 M_K^4 M_\pi^2 s_\theta^5 \Lambda_2^2}{81 M_\eta^8 M_{\eta'}^4} + \frac{2312 \sqrt{2} F^2 c_\theta^7 M_0^8 M_K^2 M_\pi^4 s_\theta^5 \Lambda_2^2}{81 M_\eta^8 M_{\eta'}^4} - \\
& \frac{1088 \sqrt{2} F^2 c_\theta^7 M_0^8 M_\pi^6 s_\theta^5 \Lambda_2^2}{243 M_\eta^8 M_{\eta'}^4} - \frac{416 \sqrt{2} F^2 c_\theta^5 M_0^8 M_K^4 s_\theta^5 \Lambda_2^2}{81 M_\eta^6 M_{\eta'}^4} - \frac{640 \sqrt{2} F^2 c_\theta^5 M_0^6 M_K^6 s_\theta^5 \Lambda_2^2}{81 M_\eta^6 M_{\eta'}^4} + \\
& \frac{616 \sqrt{2} F^2 c_\theta^5 M_0^8 M_K^2 M_\pi^2 s_\theta^5 \Lambda_2^2}{81 M_\eta^6 M_{\eta'}^4} - \frac{32 \sqrt{2} F^2 c_\theta^5 M_0^6 M_K^4 M_\pi^2 s_\theta^5 \Lambda_2^2}{3 M_\eta^6 M_{\eta'}^4} - \frac{344 \sqrt{2} F^2 c_\theta^5 M_0^8 M_\pi^4 s_\theta^5 \Lambda_2^2}{81 M_\eta^6 M_{\eta'}^4} + \\
& \frac{128 \sqrt{2} F^2 c_\theta^5 M_0^6 M_K^2 M_\pi^4 s_\theta^5 \Lambda_2^2}{9 M_\eta^6 M_{\eta'}^4} - \frac{224 \sqrt{2} F^2 c_\theta^5 M_0^6 M_\pi^6 s_\theta^5 \Lambda_2^2}{81 M_\eta^6 M_{\eta'}^4} - \frac{32 \sqrt{2} F^2 c_\theta^3 M_0^6 M_K^4 s_\theta^5 \Lambda_2^2}{27 M_\eta^4 M_{\eta'}^4} - \\
& \frac{176 \sqrt{2} F^2 c_\theta^3 M_0^4 M_K^6 s_\theta^5 \Lambda_2^2}{243 M_\eta^4 M_{\eta'}^4} + \frac{16 \sqrt{2} F^2 c_\theta^3 M_0^6 M_K^2 M_\pi^2 s_\theta^5 \Lambda_2^2}{9 M_\eta^4 M_{\eta'}^4} - \frac{28 \sqrt{2} F^2 c_\theta^3 M_0^4 M_K^4 M_\pi^2 s_\theta^5 \Lambda_2^2}{27 M_\eta^4 M_{\eta'}^4} - \\
& \frac{28 \sqrt{2} F^2 c_\theta^3 M_0^6 M_\pi^4 s_\theta^5 \Lambda_2^2}{27 M_\eta^4 M_{\eta'}^4} + \frac{110 \sqrt{2} F^2 c_\theta^3 M_0^4 M_K^2 M_\pi^4 s_\theta^5 \Lambda_2^2}{81 M_\eta^4 M_{\eta'}^4} - \frac{64 \sqrt{2} F^2 c_\theta^3 M_0^4 M_\pi^6 s_\theta^5 \Lambda_2^2}{243 M_\eta^4 M_{\eta'}^4} - \\
& \frac{2048 \sqrt{2} F^2 c_\theta^7 M_0^8 M_K^6 s_\theta^5 \Lambda_2^2}{243 M_\eta^{10} M_{\eta'}^2} + \frac{1456 \sqrt{2} F^2 c_\theta^7 M_0^8 M_K^4 M_\pi^2 s_\theta^5 \Lambda_2^2}{81 M_\eta^{10} M_{\eta'}^2} - \frac{344 \sqrt{2} F^2 c_\theta^7 M_0^8 M_K^2 M_\pi^4 s_\theta^5 \Lambda_2^2}{27 M_\eta^{10} M_{\eta'}^2} + \\
& \frac{776 \sqrt{2} F^2 c_\theta^7 M_0^8 M_\pi^6 s_\theta^5 \Lambda_2^2}{243 M_\eta^{10} M_{\eta'}^2} + \frac{1120 \sqrt{2} F^2 c_\theta^5 M_0^8 M_K^4 s_\theta^5 \Lambda_2^2}{243 M_\eta^8 M_{\eta'}^2} + \frac{640 \sqrt{2} F^2 c_\theta^5 M_0^6 M_K^6 s_\theta^5 \Lambda_2^2}{243 M_\eta^8 M_{\eta'}^2} -
\end{aligned}$$



$$\begin{aligned}
& \frac{1112 \sqrt{2} F^2 c_\theta^5 M_0^8 M_K^2 M_\pi^2 s_\theta^5 \Lambda_2^2}{243 M_\eta^8 M_{\eta'}^2} + \frac{2336 \sqrt{2} F^2 c_\theta^5 M_0^6 M_K^4 M_\pi^2 s_\theta^5 \Lambda_2^2}{243 M_\eta^8 M_{\eta'}^2} + \frac{136 \sqrt{2} F^2 c_\theta^5 M_0^8 M_\pi^4 s_\theta^5 \Lambda_2^2}{243 M_\eta^8 M_{\eta'}^2} - \\
& \frac{2704 \sqrt{2} F^2 c_\theta^5 M_0^6 M_K^2 M_\pi^4 s_\theta^5 \Lambda_2^2}{243 M_\eta^8 M_{\eta'}^2} + \frac{304 \sqrt{2} F^2 c_\theta^5 M_0^6 M_\pi^6 s_\theta^5 \Lambda_2^2}{243 M_\eta^8 M_{\eta'}^2} + \frac{64 \sqrt{2} F^2 c_\theta^3 M_0^6 M_K^4 s_\theta^5 \Lambda_2^2}{81 M_\eta^6 M_{\eta'}^2} + \\
& \frac{304 \sqrt{2} F^2 c_\theta^3 M_0^4 M_K^6 s_\theta^5 \Lambda_2^2}{243 M_\eta^6 M_{\eta'}^2} - \frac{104 \sqrt{2} F^2 c_\theta^3 M_0^6 M_K^2 M_\pi^2 s_\theta^5 \Lambda_2^2}{81 M_\eta^6 M_{\eta'}^2} - \frac{4 \sqrt{2} F^2 c_\theta^3 M_0^4 M_K^4 M_\pi^2 s_\theta^5 \Lambda_2^2}{27 M_\eta^6 M_{\eta'}^2} + \\
& \frac{76 \sqrt{2} F^2 c_\theta^3 M_0^6 M_\pi^4 s_\theta^5 \Lambda_2^2}{81 M_\eta^6 M_{\eta'}^2} - \frac{46 \sqrt{2} F^2 c_\theta^3 M_0^4 M_K^2 M_\pi^2 s_\theta^5 \Lambda_2^2}{81 M_\eta^6 M_{\eta'}^2} + \frac{32 \sqrt{2} F^2 c_\theta^3 M_0^4 M_\pi^6 s_\theta^5 \Lambda_2^2}{243 M_\eta^6 M_{\eta'}^2} - \\
& \frac{1280 F^2 c_\theta^6 M_0^8 M_K^6 s_\theta^6 \Lambda_2^2}{729 M_\eta^{12}} + \frac{1040 F^2 c_\theta^6 M_0^8 M_K^4 M_\pi^2 s_\theta^6 \Lambda_2^2}{243 M_\eta^{12}} - \frac{800 F^2 c_\theta^6 M_0^8 M_K^2 M_\pi^4 s_\theta^6 \Lambda_2^2}{243 M_\eta^{12}} + \\
& \frac{560 F^2 c_\theta^6 M_0^8 M_\pi^6 s_\theta^6 \Lambda_2^2}{729 M_\eta^{12}} + \frac{256 F^2 c_\theta^4 M_0^8 M_K^4 s_\theta^6 \Lambda_2^2}{243 M_\eta^{10}} + \frac{2560 F^2 c_\theta^4 M_0^6 M_K^6 s_\theta^6 \Lambda_2^2}{243 M_\eta^{10}} - \\
& \frac{416 F^2 c_\theta^4 M_0^8 M_K^2 M_\pi^2 s_\theta^6 \Lambda_2^2}{243 M_\eta^{10}} - \frac{416 F^2 c_\theta^4 M_0^6 M_K^4 M_\pi^2 s_\theta^6 \Lambda_2^2}{27 M_\eta^{10}} + \frac{160 F^2 c_\theta^4 M_0^8 M_\pi^4 s_\theta^6 \Lambda_2^2}{243 M_\eta^{10}} + \\
& \frac{416 F^2 c_\theta^4 M_0^6 M_K^2 M_\pi^4 s_\theta^6 \Lambda_2^2}{81 M_\eta^{10}} + \frac{152 F^2 c_\theta^4 M_0^6 M_\pi^6 s_\theta^6 \Lambda_2^2}{243 M_\eta^{10}} - \frac{128 F^2 c_\theta^2 M_0^6 M_K^4 s_\theta^6 \Lambda_2^2}{81 M_\eta^8} - \frac{80 F^2 c_\theta^2 M_0^4 M_K^6 s_\theta^6 \Lambda_2^2}{81 M_\eta^8} + \\
& \frac{112 F^2 c_\theta^2 M_0^6 M_K^2 M_\pi^2 s_\theta^6 \Lambda_2^2}{81 M_\eta^8} + \frac{16 F^2 c_\theta^2 M_0^4 M_K^4 M_\pi^2 s_\theta^6 \Lambda_2^2}{27 M_\eta^8} - \frac{56 F^2 c_\theta^2 M_0^6 M_\pi^4 s_\theta^6 \Lambda_2^2}{81 M_\eta^8} - \\
& \frac{22 F^2 c_\theta^2 M_0^4 M_\pi^6 s_\theta^6 \Lambda_2^2}{81 M_\eta^8} + \frac{8 F^2 M_0^4 M_K^4 s_\theta^6 \Lambda_2^2}{81 M_\eta^6} + \frac{8 F^2 M_0^4 M_K^2 M_\pi^2 s_\theta^6 \Lambda_2^2}{81 M_\eta^6} + \frac{2 F^2 M_0^4 M_\pi^4 s_\theta^6 \Lambda_2^2}{81 M_\eta^6} - \\
& \frac{1280 F^2 c_\theta^6 M_0^8 M_K^6 s_\theta^6 \Lambda_2^2}{729 M_\eta^{12}} + \frac{1040 F^2 c_\theta^6 M_0^8 M_K^4 M_\pi^2 s_\theta^6 \Lambda_2^2}{243 M_\eta^{12}} - \frac{800 F^2 c_\theta^6 M_0^8 M_K^2 M_\pi^4 s_\theta^6 \Lambda_2^2}{243 M_\eta^{12}} + \\
& \frac{560 F^2 c_\theta^6 M_0^8 M_\pi^6 s_\theta^6 \Lambda_2^2}{729 M_{\eta'}^{12}} + \frac{1024 F^2 c_\theta^4 M_0^6 M_K^6 s_\theta^6 \Lambda_2^2}{729 M_{\eta'}^{10}} - \frac{832 F^2 c_\theta^4 M_0^6 M_K^4 M_\pi^2 s_\theta^6 \Lambda_2^2}{243 M_{\eta'}^{10}} + \\
& \frac{640 F^2 c_\theta^4 M_0^6 M_K^2 M_\pi^4 s_\theta^6 \Lambda_2^2}{243 M_{\eta'}^{10}} - \frac{448 F^2 c_\theta^4 M_0^6 M_\pi^6 s_\theta^6 \Lambda_2^2}{729 M_{\eta'}^{10}} - \frac{640 F^2 c_\theta^6 M_0^8 M_K^6 s_\theta^6 \Lambda_2^2}{27 M_\eta^2 M_{\eta'}^{10}} + \\
& \frac{2336 F^2 c_\theta^6 M_0^8 M_K^4 M_\pi^2 s_\theta^6 \Lambda_2^2}{81 M_\eta^2 M_{\eta'}^{10}} - \frac{208 F^2 c_\theta^6 M_0^8 M_K^2 M_\pi^4 s_\theta^6 \Lambda_2^2}{81 M_\eta^2 M_{\eta'}^{10}} - \frac{388 F^2 c_\theta^6 M_0^8 M_\pi^6 s_\theta^6 \Lambda_2^2}{81 M_\eta^2 M_{\eta'}^{10}} - \\
& \frac{64 F^2 c_\theta^2 M_0^4 M_K^6 s_\theta^6 \Lambda_2^2}{243 M_\eta^8} + \frac{52 F^2 c_\theta^2 M_0^4 M_K^4 M_\pi^2 s_\theta^6 \Lambda_2^2}{81 M_\eta^8} - \frac{40 F^2 c_\theta^2 M_0^4 M_K^2 M_\pi^4 s_\theta^6 \Lambda_2^2}{81 M_\eta^8} + \frac{28 F^2 c_\theta^2 M_0^4 M_\pi^6 s_\theta^6 \Lambda_2^2}{243 M_\eta^8} + \\
& \frac{9472 F^2 c_\theta^6 M_0^8 M_K^6 s_\theta^6 \Lambda_2^2}{243 M_\eta^4 M_{\eta'}^8} - \frac{5912 F^2 c_\theta^6 M_0^8 M_K^4 M_\pi^2 s_\theta^6 \Lambda_2^2}{81 M_\eta^4 M_{\eta'}^8} + \frac{400 F^2 c_\theta^6 M_0^8 M_K^2 M_\pi^4 s_\theta^6 \Lambda_2^2}{27 M_\eta^4 M_{\eta'}^8} + \\
& \frac{344 F^2 c_\theta^6 M_0^8 M_\pi^6 s_\theta^6 \Lambda_2^2}{243 M_\eta^4 M_{\eta'}^8} + \frac{352 F^2 c_\theta^4 M_0^8 M_K^4 s_\theta^6 \Lambda_2^2}{243 M_\eta^2 M_{\eta'}^8} + \frac{8576 F^2 c_\theta^4 M_0^6 M_K^6 s_\theta^6 \Lambda_2^2}{729 M_\eta^2 M_{\eta'}^8} -
\end{aligned}$$

$$\begin{aligned}
& \frac{572 F^2 c_\theta^4 M_\theta^8 M_K^2 M_\pi^2 s_\theta^6 \Lambda_2^2}{243 M_\eta^2 M_{\eta'}^8} - \frac{3488 F^2 c_\theta^4 M_\theta^6 M_K^4 M_\pi^2 s_\theta^6 \Lambda_2^2}{243 M_\eta^2 M_{\eta'}^8} + \frac{220 F^2 c_\theta^4 M_\theta^8 M_K^4 s_\theta^6 \Lambda_2^2}{243 M_\eta^2 M_{\eta'}^8} + \\
& \frac{200 F^2 c_\theta^6 M_\theta^6 M_K^2 M_\pi^4 s_\theta^6 \Lambda_2^2}{243 M_\eta^2 M_{\eta'}^8} + \frac{1936 F^2 c_\theta^4 M_\theta^6 M_\pi^6 s_\theta^6 \Lambda_2^2}{729 M_\eta^2 M_{\eta'}^8} - \frac{30592 F^2 c_\theta^6 M_\theta^8 M_K^6 s_\theta^6 \Lambda_2^2}{729 M_\eta^6 M_{\eta'}^6} + \\
& \frac{22096 F^2 c_\theta^6 M_\theta^8 M_K^4 M_\pi^2 s_\theta^6 \Lambda_2^2}{243 M_\eta^6 M_{\eta'}^6} - \frac{6112 F^2 c_\theta^6 M_\theta^8 M_K^2 M_\pi^4 s_\theta^6 \Lambda_2^2}{243 M_\eta^6 M_{\eta'}^6} + \frac{10000 F^2 c_\theta^6 M_\theta^8 M_\pi^6 s_\theta^6 \Lambda_2^2}{729 M_\eta^6 M_{\eta'}^6} + \\
& \frac{1424 F^2 c_\theta^4 M_\theta^8 M_K^4 s_\theta^6 \Lambda_2^2}{243 M_\eta^4 M_{\eta'}^6} - \frac{1376 F^2 c_\theta^4 M_\theta^6 M_K^6 s_\theta^6 \Lambda_2^2}{81 M_\eta^4 M_{\eta'}^6} - \frac{640 F^2 c_\theta^4 M_\theta^8 M_K^2 M_\pi^2 s_\theta^6 \Lambda_2^2}{243 M_\eta^4 M_{\eta'}^6} + \\
& \frac{2504 F^2 c_\theta^4 M_\theta^6 M_K^4 M_\pi^2 s_\theta^6 \Lambda_2^2}{81 M_\eta^4 M_{\eta'}^6} + \frac{512 F^2 c_\theta^4 M_\theta^8 M_K^4 s_\theta^6 \Lambda_2^2}{243 M_\eta^4 M_{\eta'}^6} - \frac{496 F^2 c_\theta^4 M_\theta^6 M_K^2 M_\pi^4 s_\theta^6 \Lambda_2^2}{81 M_\eta^4 M_{\eta'}^6} - \\
& \frac{56 F^2 c_\theta^4 M_\theta^6 M_\pi^6 s_\theta^6 \Lambda_2^2}{81 M_\eta^4 M_{\eta'}^6} - \frac{32 F^2 c_\theta^2 M_\theta^6 M_K^4 s_\theta^6 \Lambda_2^2}{81 M_\eta^2 M_{\eta'}^6} - \frac{256 F^2 c_\theta^2 M_\theta^4 M_K^6 s_\theta^6 \Lambda_2^2}{243 M_\eta^2 M_{\eta'}^6} + \frac{52 F^2 c_\theta^2 M_\theta^6 M_K^2 M_\pi^2 s_\theta^6 \Lambda_2^2}{81 M_\eta^2 M_{\eta'}^6} + \\
& \frac{112 F^2 c_\theta^2 M_\theta^4 M_K^4 M_\pi^2 s_\theta^6 \Lambda_2^2}{81 M_\eta^2 M_{\eta'}^6} - \frac{20 F^2 c_\theta^2 M_\theta^6 M_K^4 s_\theta^6 \Lambda_2^2}{81 M_\eta^2 M_{\eta'}^6} - \frac{4 F^2 c_\theta^2 M_\theta^4 M_K^2 M_\pi^4 s_\theta^6 \Lambda_2^2}{81 M_\eta^2 M_{\eta'}^6} - \frac{68 F^2 c_\theta^2 M_\theta^4 M_\pi^6 s_\theta^6 \Lambda_2^2}{243 M_\eta^2 M_{\eta'}^6} + \\
& \frac{9472 F^2 c_\theta^6 M_\theta^8 M_K^6 s_\theta^6 \Lambda_2^2}{243 M_\eta^8 M_{\eta'}^4} - \frac{5912 F^2 c_\theta^6 M_\theta^8 M_K^4 M_\pi^2 s_\theta^6 \Lambda_2^2}{81 M_\eta^8 M_{\eta'}^4} + \frac{400 F^2 c_\theta^6 M_\theta^8 M_K^2 M_\pi^4 s_\theta^6 \Lambda_2^2}{27 M_\eta^8 M_{\eta'}^4} + \\
& \frac{344 F^2 c_\theta^6 M_\theta^8 M_\pi^6 s_\theta^6 \Lambda_2^2}{243 M_\eta^8 M_{\eta'}^4} - \frac{2432 F^2 c_\theta^4 M_\theta^8 M_K^4 s_\theta^6 \Lambda_2^2}{243 M_\eta^6 M_{\eta'}^4} + \frac{10816 F^2 c_\theta^4 M_\theta^6 M_K^6 s_\theta^6 \Lambda_2^2}{729 M_\eta^6 M_{\eta'}^4} + \\
& \frac{2068 F^2 c_\theta^4 M_\theta^8 M_K^2 M_\pi^2 s_\theta^6 \Lambda_2^2}{243 M_\eta^6 M_{\eta'}^4} - \frac{8464 F^2 c_\theta^4 M_\theta^6 M_K^4 M_\pi^2 s_\theta^6 \Lambda_2^2}{243 M_\eta^6 M_{\eta'}^4} - \frac{788 F^2 c_\theta^4 M_\theta^8 M_K^4 s_\theta^6 \Lambda_2^2}{243 M_\eta^6 M_{\eta'}^4} + \\
& \frac{2728 F^2 c_\theta^4 M_\theta^6 M_K^2 M_\pi^4 s_\theta^6 \Lambda_2^2}{243 M_\eta^6 M_{\eta'}^4} - \frac{952 F^2 c_\theta^4 M_\theta^6 M_\pi^6 s_\theta^6 \Lambda_2^2}{729 M_\eta^6 M_{\eta'}^4} - \frac{32 F^2 c_\theta^2 M_\theta^6 M_K^4 s_\theta^6 \Lambda_2^2}{27 M_\eta^4 M_{\eta'}^4} + \\
& \frac{272 F^2 c_\theta^2 M_\theta^4 M_K^6 s_\theta^6 \Lambda_2^2}{243 M_\eta^4 M_{\eta'}^4} + \frac{8 F^2 c_\theta^2 M_\theta^6 M_K^2 M_\pi^2 s_\theta^6 \Lambda_2^2}{9 M_\eta^4 M_{\eta'}^4} - \frac{68 F^2 c_\theta^2 M_\theta^4 M_K^4 M_\pi^2 s_\theta^6 \Lambda_2^2}{27 M_\eta^4 M_{\eta'}^4} - \\
& \frac{16 F^2 c_\theta^2 M_\theta^6 M_K^4 s_\theta^6 \Lambda_2^2}{27 M_\eta^4 M_{\eta'}^4} + \frac{64 F^2 c_\theta^2 M_\theta^4 M_K^2 M_\pi^4 s_\theta^6 \Lambda_2^2}{81 M_\eta^4 M_{\eta'}^4} - \frac{14 F^2 c_\theta^2 M_\theta^4 M_\pi^6 s_\theta^6 \Lambda_2^2}{243 M_\eta^4 M_{\eta'}^4} - \frac{640 F^2 c_\theta^6 M_\theta^8 M_K^6 s_\theta^6 \Lambda_2^2}{27 M_\eta^{10} M_{\eta'}^2} + \\
& \frac{2336 F^2 c_\theta^6 M_\theta^8 M_K^4 M_\pi^2 s_\theta^6 \Lambda_2^2}{81 M_\eta^{10} M_{\eta'}^2} - \frac{208 F^2 c_\theta^6 M_\theta^8 M_K^2 M_\pi^4 s_\theta^6 \Lambda_2^2}{81 M_\eta^{10} M_{\eta'}^2} - \frac{388 F^2 c_\theta^6 M_\theta^8 M_\pi^6 s_\theta^6 \Lambda_2^2}{81 M_\eta^{10} M_{\eta'}^2} + \\
& \frac{1520 F^2 c_\theta^4 M_\theta^8 M_K^4 s_\theta^6 \Lambda_2^2}{243 M_\eta^8 M_{\eta'}^2} - \frac{8992 F^2 c_\theta^4 M_\theta^6 M_K^6 s_\theta^6 \Lambda_2^2}{729 M_\eta^8 M_{\eta'}^2} - \frac{760 F^2 c_\theta^4 M_\theta^8 M_K^2 M_\pi^2 s_\theta^6 \Lambda_2^2}{243 M_\eta^8 M_{\eta'}^2} + \\
& \frac{2152 F^2 c_\theta^4 M_\theta^6 M_K^4 M_\pi^2 s_\theta^6 \Lambda_2^2}{81 M_\eta^8 M_{\eta'}^2} + \frac{536 F^2 c_\theta^4 M_\theta^8 M_K^4 s_\theta^6 \Lambda_2^2}{243 M_\eta^8 M_{\eta'}^2} - \frac{2048 F^2 c_\theta^4 M_\theta^6 M_K^2 M_\pi^4 s_\theta^6 \Lambda_2^2}{243 M_\eta^8 M_{\eta'}^2} + \\
& \frac{952 F^2 c_\theta^4 M_\theta^6 M_\pi^6 s_\theta^6 \Lambda_2^2}{729 M_\eta^8 M_{\eta'}^2} + \frac{448 F^2 c_\theta^2 M_\theta^6 M_K^4 s_\theta^6 \Lambda_2^2}{243 M_\eta^6 M_{\eta'}^2} - \frac{452 F^2 c_\theta^2 M_\theta^6 M_K^2 M_\pi^2 s_\theta^6 \Lambda_2^2}{243 M_\eta^6 M_{\eta'}^2} +
\end{aligned}$$

$$\begin{aligned}
& \frac{136 F^2 c_\theta^2 M_0^4 M_K^4 M_\pi^2 s_\theta^6 \Lambda_2^2}{81 M_\eta^6 M_{\eta'}^2} + \frac{148 F^2 c_\theta^2 M_0^6 M_\pi^4 s_\theta^6 \Lambda_2^2}{243 M_\eta^6 M_{\eta'}^2} - \frac{92 F^2 c_\theta^2 M_0^4 M_K^2 M_\pi^4 s_\theta^6 \Lambda_2^2}{81 M_\eta^6 M_{\eta'}^2} + \\
& \frac{28 F^2 c_\theta^2 M_0^4 M_\pi^6 s_\theta^6 \Lambda_2^2}{81 M_\eta^6 M_{\eta'}^2} - \frac{1280 \sqrt{2} F^2 c_\theta^5 M_0^8 M_K^6 s_\theta^7 \Lambda_2^2}{243 M_\eta^{12}} + \frac{880 \sqrt{2} F^2 c_\theta^5 M_0^8 M_K^4 M_\pi^2 s_\theta^7 \Lambda_2^2}{81 M_\eta^{12}} - \\
& \frac{200 \sqrt{2} F^2 c_\theta^5 M_0^8 M_K^2 M_\pi^4 s_\theta^7 \Lambda_2^2}{27 M_\eta^{12}} + \frac{440 \sqrt{2} F^2 c_\theta^5 M_0^8 M_\pi^6 s_\theta^7 \Lambda_2^2}{243 M_\eta^{12}} + \frac{512 \sqrt{2} F^2 c_\theta^3 M_0^8 M_K^4 s_\theta^7 \Lambda_2^2}{243 M_\eta^{10}} + \\
& \frac{5120 \sqrt{2} F^2 c_\theta^3 M_0^6 M_K^6 s_\theta^7 \Lambda_2^2}{729 M_\eta^{10}} - \frac{496 \sqrt{2} F^2 c_\theta^3 M_0^8 M_K^2 M_\pi^2 s_\theta^7 \Lambda_2^2}{243 M_\eta^{10}} - \frac{1664 \sqrt{2} F^2 c_\theta^3 M_0^6 M_K^4 M_\pi^2 s_\theta^7 \Lambda_2^2}{243 M_\eta^{10}} + \\
& \frac{56 \sqrt{2} F^2 c_\theta^3 M_0^8 M_\pi^4 s_\theta^7 \Lambda_2^2}{243 M_\eta^{10}} + \frac{512 \sqrt{2} F^2 c_\theta^3 M_0^6 M_K^2 M_\pi^4 s_\theta^7 \Lambda_2^2}{243 M_\eta^{10}} - \frac{800 \sqrt{2} F^2 c_\theta^3 M_0^6 M_\pi^6 s_\theta^7 \Lambda_2^2}{729 M_\eta^{10}} - \\
& \frac{128 \sqrt{2} F^2 c_\theta M_0^6 M_K^4 s_\theta^7 \Lambda_2^2}{243 M_\eta^8} - \frac{16 \sqrt{2} F^2 c_\theta M_0^4 M_K^6 s_\theta^7 \Lambda_2^2}{81 M_\eta^8} + \frac{64 \sqrt{2} F^2 c_\theta M_0^6 M_K^2 M_\pi^2 s_\theta^7 \Lambda_2^2}{243 M_\eta^8} + \\
& \frac{64 \sqrt{2} F^2 c_\theta M_0^6 M_\pi^4 s_\theta^7 \Lambda_2^2}{243 M_\eta^8} + \frac{4 \sqrt{2} F^2 c_\theta M_0^4 M_K^2 M_\pi^4 s_\theta^7 \Lambda_2^2}{27 M_\eta^8} + \frac{4 \sqrt{2} F^2 c_\theta M_0^4 M_\pi^6 s_\theta^7 \Lambda_2^2}{81 M_\eta^8} + \\
& \frac{2048 \sqrt{2} F^2 c_\theta^5 M_0^8 M_K^6 s_\theta^7 \Lambda_2^2}{243 M_\eta^2 M_{\eta'}^{10}} - \frac{1456 \sqrt{2} F^2 c_\theta^5 M_0^8 M_K^4 M_\pi^2 s_\theta^7 \Lambda_2^2}{81 M_\eta^2 M_{\eta'}^{10}} + \frac{344 \sqrt{2} F^2 c_\theta^5 M_0^8 M_K^2 M_\pi^4 s_\theta^7 \Lambda_2^2}{27 M_\eta^2 M_{\eta'}^{10}} - \\
& \frac{776 \sqrt{2} F^2 c_\theta^5 M_0^8 M_\pi^6 s_\theta^7 \Lambda_2^2}{243 M_\eta^2 M_{\eta'}^{10}} + \frac{640 \sqrt{2} F^2 c_\theta^5 M_0^8 M_K^6 s_\theta^7 \Lambda_2^2}{243 M_\eta^4 M_{\eta'}^8} + \frac{2096 \sqrt{2} F^2 c_\theta^5 M_0^8 M_K^4 M_\pi^2 s_\theta^7 \Lambda_2^2}{81 M_\eta^4 M_{\eta'}^8} - \\
& \frac{2312 \sqrt{2} F^2 c_\theta^5 M_0^8 M_K^2 M_\pi^4 s_\theta^7 \Lambda_2^2}{81 M_\eta^4 M_{\eta'}^8} + \frac{1088 \sqrt{2} F^2 c_\theta^5 M_0^8 M_\pi^6 s_\theta^7 \Lambda_2^2}{243 M_\eta^4 M_{\eta'}^8} - \frac{2816 \sqrt{2} F^2 c_\theta^3 M_0^6 M_K^6 s_\theta^7 \Lambda_2^2}{729 M_\eta^2 M_{\eta'}^8} + \\
& \frac{2104 \sqrt{2} F^2 c_\theta^3 M_0^6 M_K^4 M_\pi^2 s_\theta^7 \Lambda_2^2}{243 M_\eta^2 M_{\eta'}^8} - \frac{524 \sqrt{2} F^2 c_\theta^3 M_0^6 M_K^2 M_\pi^4 s_\theta^7 \Lambda_2^2}{81 M_\eta^2 M_{\eta'}^8} + \frac{1220 \sqrt{2} F^2 c_\theta^3 M_0^6 M_\pi^6 s_\theta^7 \Lambda_2^2}{729 M_\eta^2 M_{\eta'}^8} - \\
& \frac{1408 \sqrt{2} F^2 c_\theta^5 M_0^8 M_K^6 s_\theta^7 \Lambda_2^2}{81 M_\eta^6 M_{\eta'}^6} - \frac{1520 \sqrt{2} F^2 c_\theta^5 M_0^8 M_K^4 M_\pi^2 s_\theta^7 \Lambda_2^2}{81 M_\eta^6 M_{\eta'}^6} + \frac{2368 \sqrt{2} F^2 c_\theta^5 M_0^8 M_K^2 M_\pi^4 s_\theta^7 \Lambda_2^2}{81 M_\eta^6 M_{\eta'}^6} - \\
& \frac{520 \sqrt{2} F^2 c_\theta^5 M_0^8 M_\pi^6 s_\theta^7 \Lambda_2^2}{81 M_\eta^6 M_{\eta'}^6} - \frac{704 \sqrt{2} F^2 c_\theta^3 M_0^8 M_K^4 s_\theta^7 \Lambda_2^2}{243 M_\eta^4 M_{\eta'}^6} - \frac{1024 \sqrt{2} F^2 c_\theta^3 M_0^6 M_K^6 s_\theta^7 \Lambda_2^2}{729 M_\eta^4 M_{\eta'}^6} + \\
& \frac{736 \sqrt{2} F^2 c_\theta^3 M_0^8 M_K^2 M_\pi^2 s_\theta^7 \Lambda_2^2}{243 M_\eta^4 M_{\eta'}^6} - \frac{1928 \sqrt{2} F^2 c_\theta^3 M_0^6 M_K^4 M_\pi^2 s_\theta^7 \Lambda_2^2}{243 M_\eta^4 M_{\eta'}^6} - \frac{104 \sqrt{2} F^2 c_\theta^3 M_0^8 M_\pi^4 s_\theta^7 \Lambda_2^2}{243 M_\eta^4 M_{\eta'}^6} + \\
& \frac{2396 \sqrt{2} F^2 c_\theta^3 M_0^6 M_K^2 M_\pi^4 s_\theta^7 \Lambda_2^2}{243 M_\eta^4 M_{\eta'}^6} - \frac{1244 \sqrt{2} F^2 c_\theta^3 M_0^6 M_\pi^6 s_\theta^7 \Lambda_2^2}{729 M_\eta^4 M_{\eta'}^6} + \frac{64 \sqrt{2} F^2 c_\theta M_0^4 M_K^6 s_\theta^7 \Lambda_2^2}{243 M_\eta^2 M_{\eta'}^6} - \\
& \frac{56 \sqrt{2} F^2 c_\theta M_0^4 M_K^4 M_\pi^2 s_\theta^7 \Lambda_2^2}{81 M_\eta^2 M_{\eta'}^6} + \frac{16 \sqrt{2} F^2 c_\theta M_0^4 M_K^2 M_\pi^4 s_\theta^7 \Lambda_2^2}{27 M_\eta^2 M_{\eta'}^6} - \frac{40 \sqrt{2} F^2 c_\theta M_0^4 M_\pi^6 s_\theta^7 \Lambda_2^2}{243 M_\eta^2 M_{\eta'}^6} +
\end{aligned}$$

$$\begin{aligned}
& \frac{4736 \sqrt{2} F^2 c_\theta^5 M_0^8 M_K^6 s_\theta^7 \Lambda_2^2}{243 M_\eta^8 M_{\eta'}^4} + \frac{976 \sqrt{2} F^2 c_\theta^5 M_0^8 M_K^4 M_\pi^2 s_\theta^7 \Lambda_2^2}{81 M_\eta^8 M_{\eta'}^4} - \frac{1888 \sqrt{2} F^2 c_\theta^5 M_0^8 M_K^2 M_\pi^4 s_\theta^7 \Lambda_2^2}{81 M_\eta^8 M_{\eta'}^4} + \\
& \frac{1240 \sqrt{2} F^2 c_\theta^5 M_0^8 M_\pi^6 s_\theta^7 \Lambda_2^2}{243 M_\eta^8 M_{\eta'}^4} + \frac{512 \sqrt{2} F^2 c_\theta^3 M_0^8 M_K^4 s_\theta^7 \Lambda_2^2}{243 M_\eta^6 M_{\eta'}^4} + \frac{1792 \sqrt{2} F^2 c_\theta^3 M_0^6 M_K^6 s_\theta^7 \Lambda_2^2}{243 M_\eta^6 M_{\eta'}^4} - \\
& \frac{976 \sqrt{2} F^2 c_\theta^3 M_0^8 M_K^2 M_\pi^2 s_\theta^7 \Lambda_2^2}{243 M_\eta^6 M_{\eta'}^4} - \frac{8 \sqrt{2} F^2 c_\theta^3 M_0^6 M_K^4 M_\pi^2 s_\theta^7 \Lambda_2^2}{81 M_\eta^6 M_{\eta'}^4} + \frac{680 \sqrt{2} F^2 c_\theta^3 M_0^8 M_\pi^4 s_\theta^7 \Lambda_2^2}{243 M_\eta^6 M_{\eta'}^4} - \\
& \frac{140 \sqrt{2} F^2 c_\theta^3 M_0^6 M_K^2 M_\pi^4 s_\theta^7 \Lambda_2^2}{27 M_\eta^6 M_{\eta'}^4} + \frac{356 \sqrt{2} F^2 c_\theta^3 M_0^6 M_\pi^6 s_\theta^7 \Lambda_2^2}{243 M_\eta^6 M_{\eta'}^4} + \frac{32 \sqrt{2} F^2 c_\theta M_0^6 M_K^4 s_\theta^7 \Lambda_2^2}{81 M_\eta^4 M_{\eta'}^4} + \\
& \frac{64 \sqrt{2} F^2 c_\theta M_0^4 M_K^6 s_\theta^7 \Lambda_2^2}{243 M_\eta^4 M_{\eta'}^4} - \frac{40 \sqrt{2} F^2 c_\theta M_0^6 M_K^2 M_\pi^2 s_\theta^7 \Lambda_2^2}{81 M_\eta^4 M_{\eta'}^4} + \frac{8 \sqrt{2} F^2 c_\theta M_0^6 M_\pi^4 s_\theta^7 \Lambda_2^2}{81 M_\eta^4 M_{\eta'}^4} - \\
& \frac{28 \sqrt{2} F^2 c_\theta M_0^4 M_K^2 M_\pi^4 s_\theta^7 \Lambda_2^2}{81 M_\eta^4 M_{\eta'}^4} + \frac{20 \sqrt{2} F^2 c_\theta M_0^4 M_\pi^6 s_\theta^7 \Lambda_2^2}{243 M_\eta^4 M_{\eta'}^4} - \frac{640 \sqrt{2} F^2 c_\theta^5 M_0^8 M_K^6 s_\theta^7 \Lambda_2^2}{81 M_\eta^{10} M_\pi^2} - \\
& \frac{976 \sqrt{2} F^2 c_\theta^5 M_0^8 M_K^4 M_\pi^2 s_\theta^7 \Lambda_2^2}{81 M_\eta^{10} M_\pi^2} + \frac{1400 \sqrt{2} F^2 c_\theta^5 M_0^8 M_K^2 M_\pi^4 s_\theta^7 \Lambda_2^2}{81 M_\eta^{10} M_\pi^2} - \frac{16 \sqrt{2} F^2 c_\theta^5 M_0^8 M_\pi^6 s_\theta^7 \Lambda_2^2}{9 M_\eta^{10} M_\pi^2} - \\
& \frac{320 \sqrt{2} F^2 c_\theta^3 M_0^8 M_K^4 s_\theta^7 \Lambda_2^2}{243 M_\eta^8 M_{\eta'}^2} - \frac{6656 \sqrt{2} F^2 c_\theta^3 M_0^6 M_K^6 s_\theta^7 \Lambda_2^2}{729 M_\eta^8 M_{\eta'}^2} + \frac{736 \sqrt{2} F^2 c_\theta^3 M_0^8 M_K^2 M_\pi^2 s_\theta^7 \Lambda_2^2}{243 M_\eta^8 M_{\eta'}^2} + \\
& \frac{56 \sqrt{2} F^2 c_\theta^3 M_0^6 M_K^4 M_\pi^2 s_\theta^7 \Lambda_2^2}{9 M_\eta^8 M_{\eta'}^2} - \frac{632 \sqrt{2} F^2 c_\theta^3 M_0^8 M_\pi^4 s_\theta^7 \Lambda_2^2}{243 M_\eta^8 M_{\eta'}^2} - \frac{76 \sqrt{2} F^2 c_\theta^3 M_0^6 M_K^2 M_\pi^4 s_\theta^7 \Lambda_2^2}{243 M_\eta^8 M_{\eta'}^2} - \\
& \frac{244 \sqrt{2} F^2 c_\theta^3 M_0^6 M_\pi^6 s_\theta^7 \Lambda_2^2}{729 M_\eta^8 M_{\eta'}^2} + \frac{32 \sqrt{2} F^2 c_\theta M_0^6 M_K^4 s_\theta^7 \Lambda_2^2}{243 M_\eta^6 M_{\eta'}^2} - \frac{80 \sqrt{2} F^2 c_\theta M_0^4 M_K^6 s_\theta^7 \Lambda_2^2}{243 M_\eta^6 M_{\eta'}^2} + \\
& \frac{56 \sqrt{2} F^2 c_\theta M_0^6 M_K^2 M_\pi^2 s_\theta^7 \Lambda_2^2}{243 M_\eta^6 M_{\eta'}^2} + \frac{56 \sqrt{2} F^2 c_\theta M_0^4 M_K^4 M_\pi^2 s_\theta^7 \Lambda_2^2}{81 M_\eta^6 M_{\eta'}^2} - \frac{88 \sqrt{2} F^2 c_\theta M_0^6 M_\pi^4 s_\theta^7 \Lambda_2^2}{243 M_\eta^6 M_{\eta'}^2} - \\
& \frac{32 \sqrt{2} F^2 c_\theta M_0^4 M_K^2 M_\pi^4 s_\theta^7 \Lambda_2^2}{81 M_\eta^6 M_{\eta'}^2} + \frac{8 \sqrt{2} F^2 c_\theta M_0^4 M_\pi^6 s_\theta^7 \Lambda_2^2}{243 M_\eta^6 M_{\eta'}^2} - \frac{3200 F^2 c_\theta^4 M_0^8 M_K^6 s_\theta^8 \Lambda_2^2}{243 M_\eta^{12}} + \\
& \frac{520 F^2 c_\theta^4 M_0^8 M_K^4 M_\pi^2 s_\theta^8 \Lambda_2^2}{27 M_\eta^{12}} - \frac{520 F^2 c_\theta^4 M_0^8 M_K^2 M_\pi^4 s_\theta^8 \Lambda_2^2}{81 M_\eta^{12}} - \frac{190 F^2 c_\theta^4 M_0^8 M_\pi^6 s_\theta^8 \Lambda_2^2}{243 M_\eta^{12}} + \\
& \frac{256 F^2 c_\theta^2 M_0^8 M_K^4 s_\theta^8 \Lambda_2^2}{81 M_\eta^{10}} + \frac{1280 F^2 c_\theta^2 M_0^6 M_K^6 s_\theta^8 \Lambda_2^2}{243 M_\eta^{10}} - \frac{224 F^2 c_\theta^2 M_0^8 M_K^2 M_\pi^2 s_\theta^8 \Lambda_2^2}{81 M_\eta^{10}} - \\
& \frac{256 F^2 c_\theta^2 M_0^6 M_K^4 M_\pi^2 s_\theta^8 \Lambda_2^2}{81 M_\eta^{10}} + \frac{112 F^2 c_\theta^2 M_0^8 M_\pi^4 s_\theta^8 \Lambda_2^2}{81 M_\eta^{10}} + \frac{352 F^2 c_\theta^2 M_0^6 M_\pi^6 s_\theta^8 \Lambda_2^2}{243 M_\eta^{10}} - \frac{32 F^2 M_0^6 M_K^4 s_\theta^8 \Lambda_2^2}{243 M_\eta^8} - \\
& \frac{8 F^2 M_0^4 M_K^6 s_\theta^8 \Lambda_2^2}{243 M_\eta^8} - \frac{32 F^2 M_0^6 M_K^2 M_\pi^2 s_\theta^8 \Lambda_2^2}{243 M_\eta^8} - \frac{4 F^2 M_0^4 M_K^4 M_\pi^2 s_\theta^8 \Lambda_2^2}{81 M_\eta^8} - \frac{8 F^2 M_0^6 M_\pi^4 s_\theta^8 \Lambda_2^2}{243 M_\eta^8} - \\
& \frac{2 F^2 M_0^4 M_K^2 M_\pi^4 s_\theta^8 \Lambda_2^2}{81 M_\eta^8} - \frac{F^2 M_0^4 M_\pi^6 s_\theta^8 \Lambda_2^2}{243 M_\eta^8} - \frac{128 F^2 c_\theta^4 M_0^8 M_K^6 s_\theta^8 \Lambda_2^2}{81 M_\eta^2 M_{\eta'}^{10}} + \frac{104 F^2 c_\theta^4 M_0^8 M_K^4 M_\pi^2 s_\theta^8 \Lambda_2^2}{27 M_\eta^2 M_{\eta'}^{10}} -
\end{aligned}$$

$$\begin{aligned}
& \frac{80 F^2 c_\theta^4 M_\theta^8 M_K^2 M_\pi^4 s_\theta^8 \Lambda_2^2}{27 M_\eta^2 M_{\eta'}^{10}} + \frac{56 F^2 c_\theta^4 M_\theta^8 M_\pi^6 s_\theta^8 \Lambda_2^2}{81 M_\eta^2 M_{\eta'}^{10}} - \frac{4256 F^2 c_\theta^4 M_\theta^8 M_K^6 s_\theta^8 \Lambda_2^2}{243 M_\eta^4 M_{\eta'}^8} + \\
& \frac{1888 F^2 c_\theta^4 M_\theta^8 M_K^4 M_\pi^2 s_\theta^8 \Lambda_2^2}{81 M_\eta^4 M_{\eta'}^8} - \frac{104 F^2 c_\theta^4 M_\theta^8 M_K^2 M_\pi^4 s_\theta^8 \Lambda_2^2}{27 M_\eta^4 M_{\eta'}^8} - \frac{742 F^2 c_\theta^4 M_\theta^8 M_\pi^6 s_\theta^8 \Lambda_2^2}{243 M_\eta^4 M_{\eta'}^8} + \\
& \frac{128 F^2 c_\theta^2 M_\theta^6 M_K^6 s_\theta^8 \Lambda_2^2}{243 M_\eta^2 M_{\eta'}^8} - \frac{104 F^2 c_\theta^2 M_\theta^6 M_K^4 M_\pi^2 s_\theta^8 \Lambda_2^2}{81 M_\eta^2 M_{\eta'}^8} + \frac{80 F^2 c_\theta^2 M_\theta^6 M_K^2 M_\pi^4 s_\theta^8 \Lambda_2^2}{81 M_\eta^2 M_{\eta'}^8} - \\
& \frac{56 F^2 c_\theta^2 M_\theta^6 M_\pi^6 s_\theta^8 \Lambda_2^2}{243 M_\eta^2 M_{\eta'}^8} + \frac{6080 F^2 c_\theta^4 M_\theta^8 M_K^6 s_\theta^8 \Lambda_2^2}{243 M_\eta^6 M_{\eta'}^6} - \frac{1456 F^2 c_\theta^4 M_\theta^8 M_K^4 M_\pi^2 s_\theta^8 \Lambda_2^2}{27 M_\eta^6 M_{\eta'}^6} + \\
& \frac{1408 F^2 c_\theta^4 M_\theta^8 M_K^2 M_\pi^4 s_\theta^8 \Lambda_2^2}{81 M_\eta^6 M_{\eta'}^6} - \frac{440 F^2 c_\theta^4 M_\theta^8 M_\pi^6 s_\theta^8 \Lambda_2^2}{243 M_\eta^6 M_{\eta'}^6} + \frac{32 F^2 c_\theta^2 M_\theta^8 M_K^4 s_\theta^8 \Lambda_2^2}{81 M_\eta^4 M_{\eta'}^6} + \\
& \frac{1216 F^2 c_\theta^2 M_\theta^6 M_K^6 s_\theta^8 \Lambda_2^2}{243 M_\eta^4 M_{\eta'}^6} - \frac{52 F^2 c_\theta^2 M_\theta^8 M_K^2 M_\pi^2 s_\theta^8 \Lambda_2^2}{81 M_\eta^4 M_{\eta'}^6} - \frac{656 F^2 c_\theta^2 M_\theta^6 M_K^4 M_\pi^2 s_\theta^8 \Lambda_2^2}{81 M_\eta^4 M_{\eta'}^6} + \\
& \frac{20 F^2 c_\theta^2 M_\theta^8 M_\pi^4 s_\theta^8 \Lambda_2^2}{81 M_\eta^4 M_{\eta'}^6} + \frac{8 F^2 c_\theta^2 M_\theta^6 M_K^2 M_\pi^4 s_\theta^8 \Lambda_2^2}{3 M_\eta^4 M_{\eta'}^6} + \frac{104 F^2 c_\theta^2 M_\theta^6 M_\pi^6 s_\theta^8 \Lambda_2^2}{243 M_\eta^4 M_{\eta'}^6} - \frac{4576 F^2 c_\theta^4 M_\theta^8 M_K^6 s_\theta^8 \Lambda_2^2}{243 M_\eta^8 M_{\eta'}^4} + \\
& \frac{4544 F^2 c_\theta^4 M_\theta^8 M_K^4 M_\pi^2 s_\theta^8 \Lambda_2^2}{81 M_\eta^8 M_{\eta'}^4} - \frac{680 F^2 c_\theta^4 M_\theta^8 M_K^2 M_\pi^4 s_\theta^8 \Lambda_2^2}{27 M_\eta^8 M_{\eta'}^4} + \frac{1384 F^2 c_\theta^4 M_\theta^8 M_\pi^6 s_\theta^8 \Lambda_2^2}{243 M_\eta^8 M_{\eta'}^4} + \\
& \frac{80 F^2 c_\theta^2 M_\theta^8 M_K^4 s_\theta^8 \Lambda_2^2}{27 M_\eta^6 M_{\eta'}^4} - \frac{800 F^2 c_\theta^2 M_\theta^6 M_K^6 s_\theta^8 \Lambda_2^2}{243 M_\eta^6 M_{\eta'}^4} - \frac{8 F^2 c_\theta^2 M_\theta^8 M_K^2 M_\pi^2 s_\theta^8 \Lambda_2^2}{3 M_\eta^6 M_{\eta'}^4} + \frac{904 F^2 c_\theta^2 M_\theta^6 M_K^4 M_\pi^2 s_\theta^8 \Lambda_2^2}{81 M_\eta^6 M_{\eta'}^4} + \\
& \frac{40 F^2 c_\theta^2 M_\theta^8 M_\pi^4 s_\theta^8 \Lambda_2^2}{27 M_\eta^6 M_{\eta'}^4} - \frac{160 F^2 c_\theta^2 M_\theta^6 M_K^2 M_\pi^4 s_\theta^8 \Lambda_2^2}{27 M_\eta^6 M_{\eta'}^4} + \frac{392 F^2 c_\theta^2 M_\theta^6 M_\pi^6 s_\theta^8 \Lambda_2^2}{243 M_\eta^6 M_{\eta'}^4} - \frac{32 F^2 M_\theta^4 M_K^6 s_\theta^8 \Lambda_2^2}{243 M_\eta^4 M_{\eta'}^4} + \\
& \frac{8 F^2 M_\theta^4 M_K^4 M_\pi^2 s_\theta^8 \Lambda_2^2}{27 M_\eta^4 M_{\eta'}^4} - \frac{16 F^2 M_\theta^4 M_K^2 M_\pi^4 s_\theta^8 \Lambda_2^2}{81 M_\eta^4 M_{\eta'}^4} + \frac{8 F^2 M_\theta^4 M_\pi^6 s_\theta^8 \Lambda_2^2}{243 M_\eta^4 M_{\eta'}^4} + \frac{3616 F^2 c_\theta^4 M_\theta^8 M_K^6 s_\theta^8 \Lambda_2^2}{243 M_\eta^{10} M_{\eta'}^2} - \\
& \frac{3256 F^2 c_\theta^4 M_\theta^8 M_K^4 M_\pi^2 s_\theta^8 \Lambda_2^2}{81 M_\eta^{10} M_{\eta'}^2} + \frac{1264 F^2 c_\theta^4 M_\theta^8 M_K^2 M_\pi^4 s_\theta^8 \Lambda_2^2}{81 M_\eta^{10} M_{\eta'}^2} - \frac{880 F^2 c_\theta^4 M_\theta^8 M_\pi^6 s_\theta^8 \Lambda_2^2}{243 M_\eta^{10} M_{\eta'}^2} - \\
& \frac{1024 F^2 c_\theta^2 M_\theta^8 M_K^4 s_\theta^8 \Lambda_2^2}{243 M_\eta^8 M_{\eta'}^2} - \frac{704 F^2 c_\theta^2 M_\theta^6 M_K^6 s_\theta^8 \Lambda_2^2}{243 M_\eta^8 M_{\eta'}^2} + \frac{1316 F^2 c_\theta^2 M_\theta^8 M_K^2 M_\pi^2 s_\theta^8 \Lambda_2^2}{243 M_\eta^8 M_{\eta'}^2} - \\
& \frac{944 F^2 c_\theta^2 M_\theta^6 M_K^4 M_\pi^2 s_\theta^8 \Lambda_2^2}{243 M_\eta^8 M_{\eta'}^2} - \frac{436 F^2 c_\theta^2 M_\theta^8 M_\pi^4 s_\theta^8 \Lambda_2^2}{243 M_\eta^8 M_{\eta'}^2} + \frac{1192 F^2 c_\theta^2 M_\theta^6 M_K^2 M_\pi^4 s_\theta^8 \Lambda_2^2}{243 M_\eta^8 M_{\eta'}^2} - \\
& \frac{184 F^2 c_\theta^2 M_\theta^6 M_\pi^6 s_\theta^8 \Lambda_2^2}{81 M_\eta^8 M_{\eta'}^2} - \frac{16 F^2 M_\theta^6 M_K^4 s_\theta^8 \Lambda_2^2}{81 M_\eta^6 M_{\eta'}^2} - \frac{32 F^2 M_\theta^4 M_K^6 s_\theta^8 \Lambda_2^2}{243 M_\eta^6 M_{\eta'}^2} + \frac{32 F^2 M_\theta^6 M_K^2 M_\pi^2 s_\theta^8 \Lambda_2^2}{81 M_\eta^6 M_{\eta'}^2} + \\
& \frac{16 F^2 M_\theta^4 M_K^4 M_\pi^2 s_\theta^8 \Lambda_2^2}{81 M_\eta^6 M_{\eta'}^2} - \frac{16 F^2 M_\theta^6 M_\pi^4 s_\theta^8 \Lambda_2^2}{81 M_\eta^6 M_{\eta'}^2} - \frac{16 F^2 M_\theta^4 M_\pi^6 s_\theta^8 \Lambda_2^2}{243 M_\eta^6 M_{\eta'}^2} - \frac{6400 \sqrt{2} F^2 c_\theta^3 M_\theta^8 M_K^6 s_\theta^9 \Lambda_2^2}{729 M_\eta^{12}} + \\
& \frac{2080 \sqrt{2} F^2 c_\theta^3 M_\theta^8 M_K^4 M_\pi^2 s_\theta^9 \Lambda_2^2}{243 M_\eta^{12}} - \frac{640 \sqrt{2} F^2 c_\theta^3 M_\theta^8 M_K^2 M_\pi^4 s_\theta^9 \Lambda_2^2}{243 M_\eta^{12}} + \frac{1000 \sqrt{2} F^2 c_\theta^3 M_\theta^8 M_\pi^6 s_\theta^9 \Lambda_2^2}{729 M_\eta^{12}} +
\end{aligned}$$

$$\begin{aligned}
& \frac{256 \sqrt{2} F^2 c_\theta M_0^8 M_K^4 s_\theta^9 \Lambda_2^2}{243 M_\eta^{10}} + \frac{256 \sqrt{2} F^2 c_\theta M_0^6 M_K^6 s_\theta^9 \Lambda_2^2}{243 M_\eta^{10}} - \frac{128 \sqrt{2} F^2 c_\theta M_0^8 M_K^2 M_\pi^2 s_\theta^9 \Lambda_2^2}{243 M_\eta^{10}} - \\
& \frac{128 \sqrt{2} F^2 c_\theta M_0^8 M_\pi^4 s_\theta^9 \Lambda_2^2}{243 M_\eta^{10}} - \frac{64 \sqrt{2} F^2 c_\theta M_0^6 M_K^2 M_\pi^4 s_\theta^9 \Lambda_2^2}{81 M_\eta^{10}} - \frac{64 \sqrt{2} F^2 c_\theta M_0^6 M_\pi^6 s_\theta^9 \Lambda_2^2}{243 M_\eta^{10}} + \\
& \frac{832 \sqrt{2} F^2 c_\theta^3 M_0^8 M_K^6 s_\theta^9 \Lambda_2^2}{243 M_\eta^4 M_{\eta'}^8} - \frac{632 \sqrt{2} F^2 c_\theta^3 M_0^8 M_K^4 M_\pi^2 s_\theta^9 \Lambda_2^2}{81 M_\eta^4 M_{\eta'}^8} + \frac{160 \sqrt{2} F^2 c_\theta^3 M_0^8 M_K^2 M_\pi^4 s_\theta^9 \Lambda_2^2}{27 M_\eta^4 M_{\eta'}^8} - \\
& \frac{376 \sqrt{2} F^2 c_\theta^3 M_0^8 M_\pi^6 s_\theta^9 \Lambda_2^2}{243 M_\eta^4 M_{\eta'}^8} + \frac{3520 \sqrt{2} F^2 c_\theta^3 M_0^8 M_K^6 s_\theta^9 \Lambda_2^2}{729 M_\eta^6 M_{\eta'}^6} + \frac{872 \sqrt{2} F^2 c_\theta^3 M_0^8 M_K^4 M_\pi^2 s_\theta^9 \Lambda_2^2}{243 M_\eta^6 M_{\eta'}^6} - \\
& \frac{1952 \sqrt{2} F^2 c_\theta^3 M_0^8 M_K^2 M_\pi^4 s_\theta^9 \Lambda_2^2}{243 M_\eta^6 M_{\eta'}^6} + \frac{800 \sqrt{2} F^2 c_\theta^3 M_0^8 M_\pi^6 s_\theta^9 \Lambda_2^2}{729 M_\eta^6 M_{\eta'}^6} - \frac{128 \sqrt{2} F^2 c_\theta M_0^6 M_K^6 s_\theta^9 \Lambda_2^2}{243 M_\eta^4 M_{\eta'}^6} + \\
& \frac{112 \sqrt{2} F^2 c_\theta M_0^6 M_K^4 M_\pi^2 s_\theta^9 \Lambda_2^2}{81 M_\eta^4 M_{\eta'}^6} - \frac{32 \sqrt{2} F^2 c_\theta M_0^6 M_K^2 M_\pi^4 s_\theta^9 \Lambda_2^2}{27 M_\eta^4 M_{\eta'}^6} + \frac{80 \sqrt{2} F^2 c_\theta M_0^6 M_\pi^6 s_\theta^9 \Lambda_2^2}{243 M_\eta^4 M_{\eta'}^6} - \\
& \frac{3136 \sqrt{2} F^2 c_\theta^3 M_0^8 M_K^6 s_\theta^9 \Lambda_2^2}{243 M_\eta^8 M_{\eta'}^4} + \frac{256 \sqrt{2} F^2 c_\theta^3 M_0^8 M_K^4 M_\pi^2 s_\theta^9 \Lambda_2^2}{27 M_\eta^8 M_{\eta'}^4} - \frac{32 \sqrt{2} F^2 c_\theta^3 M_0^8 M_K^2 M_\pi^4 s_\theta^9 \Lambda_2^2}{81 M_\eta^8 M_{\eta'}^4} - \\
& \frac{152 \sqrt{2} F^2 c_\theta^3 M_0^8 M_\pi^6 s_\theta^9 \Lambda_2^2}{243 M_\eta^8 M_{\eta'}^4} - \frac{32 \sqrt{2} F^2 c_\theta M_0^8 M_K^4 s_\theta^9 \Lambda_2^2}{81 M_\eta^6 M_{\eta'}^4} - \frac{1024 \sqrt{2} F^2 c_\theta M_0^6 M_K^6 s_\theta^9 \Lambda_2^2}{729 M_\eta^6 M_{\eta'}^4} + \\
& \frac{40 \sqrt{2} F^2 c_\theta M_0^8 M_K^2 M_\pi^4 s_\theta^9 \Lambda_2^2}{81 M_\eta^6 M_{\eta'}^4} + \frac{352 \sqrt{2} F^2 c_\theta M_0^6 M_K^4 M_\pi^2 s_\theta^9 \Lambda_2^2}{243 M_\eta^6 M_{\eta'}^4} - \frac{8 \sqrt{2} F^2 c_\theta M_0^8 M_\pi^4 s_\theta^9 \Lambda_2^2}{81 M_\eta^6 M_{\eta'}^4} - \\
& \frac{40 \sqrt{2} F^2 c_\theta M_0^6 M_K^2 M_\pi^4 s_\theta^9 \Lambda_2^2}{243 M_\eta^6 M_{\eta'}^4} + \frac{88 \sqrt{2} F^2 c_\theta M_0^6 M_\pi^6 s_\theta^9 \Lambda_2^2}{729 M_\eta^6 M_{\eta'}^4} + \frac{1088 \sqrt{2} F^2 c_\theta^3 M_0^8 M_K^6 s_\theta^9 \Lambda_2^2}{81 M_\eta^{10} M_{\eta'}^2} - \\
& \frac{1120 \sqrt{2} F^2 c_\theta^3 M_0^8 M_K^4 M_\pi^2 s_\theta^9 \Lambda_2^2}{81 M_\eta^{10} M_{\eta'}^2} + \frac{416 \sqrt{2} F^2 c_\theta^3 M_0^8 M_K^2 M_\pi^4 s_\theta^9 \Lambda_2^2}{81 M_\eta^{10} M_{\eta'}^2} - \frac{8 \sqrt{2} F^2 c_\theta^3 M_0^8 M_\pi^6 s_\theta^9 \Lambda_2^2}{27 M_\eta^{10} M_{\eta'}^2} - \\
& \frac{160 \sqrt{2} F^2 c_\theta M_0^8 M_K^4 s_\theta^9 \Lambda_2^2}{243 M_\eta^8 M_{\eta'}^2} + \frac{640 \sqrt{2} F^2 c_\theta M_0^6 M_K^6 s_\theta^9 \Lambda_2^2}{729 M_\eta^8 M_{\eta'}^2} + \frac{8 \sqrt{2} F^2 c_\theta M_0^8 M_K^2 M_\pi^2 s_\theta^9 \Lambda_2^2}{243 M_\eta^8 M_{\eta'}^2} - \\
& \frac{688 \sqrt{2} F^2 c_\theta M_0^6 M_K^4 M_\pi^2 s_\theta^9 \Lambda_2^2}{243 M_\eta^8 M_{\eta'}^2} + \frac{152 \sqrt{2} F^2 c_\theta M_0^8 M_\pi^4 s_\theta^9 \Lambda_2^2}{243 M_\eta^8 M_{\eta'}^2} + \frac{520 \sqrt{2} F^2 c_\theta M_0^6 M_K^2 M_\pi^4 s_\theta^9 \Lambda_2^2}{243 M_\eta^8 M_{\eta'}^2} - \\
& \frac{136 \sqrt{2} F^2 c_\theta M_0^6 M_\pi^6 s_\theta^9 \Lambda_2^2}{729 M_\eta^8 M_{\eta'}^2} - \frac{1600 F^2 c_\theta^2 M_0^8 M_K^6 s_\theta^{10} \Lambda_2^2}{243 M_\eta^{12}} + \frac{320 F^2 c_\theta^2 M_0^8 M_K^4 M_\pi^2 s_\theta^{10} \Lambda_2^2}{81 M_\eta^{12}} - \\
& \frac{440 F^2 c_\theta^2 M_0^8 M_\pi^6 s_\theta^{10} \Lambda_2^2}{243 M_\eta^{12}} + \frac{64 F^2 M_0^8 M_K^4 s_\theta^{10} \Lambda_2^2}{243 M_\eta^{10}} + \frac{128 F^2 M_0^6 M_K^6 s_\theta^{10} \Lambda_2^2}{729 M_\eta^{10}} + \frac{64 F^2 M_0^8 M_K^2 M_\pi^2 s_\theta^{10} \Lambda_2^2}{243 M_\eta^{10}} + \\
& \frac{64 F^2 M_0^6 M_K^4 M_\pi^2 s_\theta^{10} \Lambda_2^2}{243 M_\eta^{10}} + \frac{16 F^2 M_0^8 M_\pi^4 s_\theta^{10} \Lambda_2^2}{243 M_\eta^{10}} + \frac{32 F^2 M_0^6 M_K^2 M_\pi^4 s_\theta^{10} \Lambda_2^2}{243 M_\eta^{10}} + \frac{16 F^2 M_0^6 M_\pi^6 s_\theta^{10} \Lambda_2^2}{729 M_\eta^{10}} - \\
& \frac{64 F^2 c_\theta^2 M_0^8 M_K^6 s_\theta^{10} \Lambda_2^2}{243 M_\eta^4 M_{\eta'}^8} + \frac{52 F^2 c_\theta^2 M_0^8 M_K^4 M_\pi^2 s_\theta^{10} \Lambda_2^2}{81 M_\eta^4 M_{\eta'}^8} - \frac{40 F^2 c_\theta^2 M_0^8 M_K^2 M_\pi^4 s_\theta^{10} \Lambda_2^2}{81 M_\eta^4 M_{\eta'}^8} +
\end{aligned}$$

$$\begin{aligned}
& \frac{28 F^2 c_\theta^2 M_\theta^8 M_\pi^6 s_\theta^{10} \Lambda_2^2}{243 M_\eta^4 M_{\eta'}^8} - \frac{1088 F^2 c_\theta^2 M_\theta^8 M_K^6 s_\theta^{10} \Lambda_2^2}{243 M_\eta^6 M_{\eta'}^6} + \frac{616 F^2 c_\theta^2 M_\theta^8 M_K^4 M_\pi^2 s_\theta^{10} \Lambda_2^2}{81 M_\eta^6 M_{\eta'}^6} - \\
& \frac{80 F^2 c_\theta^2 M_\theta^8 M_K^4 M_\pi^4 s_\theta^{10} \Lambda_2^2}{27 M_\eta^6 M_{\eta'}^6} - \frac{40 F^2 c_\theta^2 M_\theta^8 M_\pi^6 s_\theta^{10} \Lambda_2^2}{243 M_\eta^6 M_{\eta'}^6} + \frac{128 F^2 c_\theta^2 M_\theta^8 M_K^6 s_\theta^{10} \Lambda_2^2}{243 M_\eta^8 M_{\eta'}^4} - \\
& \frac{76 F^2 c_\theta^2 M_\theta^8 M_K^4 M_\pi^2 s_\theta^{10} \Lambda_2^2}{9 M_\eta^8 M_{\eta'}^4} + \frac{472 F^2 c_\theta^2 M_\theta^8 M_K^2 M_\pi^4 s_\theta^{10} \Lambda_2^2}{81 M_\eta^8 M_{\eta'}^4} - \frac{572 F^2 c_\theta^2 M_\theta^8 M_\pi^6 s_\theta^{10} \Lambda_2^2}{243 M_\eta^8 M_{\eta'}^4} + \\
& \frac{64 F^2 M_\theta^6 M_K^6 s_\theta^{10} \Lambda_2^2}{243 M_\eta^6 M_{\eta'}^4} - \frac{16 F^2 M_\theta^6 M_K^4 M_\pi^2 s_\theta^{10} \Lambda_2^2}{27 M_\eta^6 M_{\eta'}^4} + \frac{32 F^2 M_\theta^6 M_K^2 M_\pi^4 s_\theta^{10} \Lambda_2^2}{81 M_\eta^6 M_{\eta'}^4} - \frac{16 F^2 M_\theta^6 M_\pi^6 s_\theta^{10} \Lambda_2^2}{243 M_\eta^6 M_{\eta'}^4} + \\
& \frac{512 F^2 c_\theta^2 M_\theta^8 M_K^6 s_\theta^{10} \Lambda_2^2}{81 M_\eta^{10} M_{\eta'}^2} - \frac{32 F^2 c_\theta^2 M_\theta^8 M_K^4 M_\pi^2 s_\theta^{10} \Lambda_2^2}{81 M_\eta^{10} M_{\eta'}^2} - \frac{368 F^2 c_\theta^2 M_\theta^8 M_K^2 M_\pi^4 s_\theta^{10} \Lambda_2^2}{81 M_\eta^{10} M_{\eta'}^2} + \\
& \frac{248 F^2 c_\theta^2 M_\theta^8 M_\pi^6 s_\theta^{10} \Lambda_2^2}{81 M_\eta^{10} M_{\eta'}^2} + \frac{16 F^2 M_\theta^8 M_K^4 s_\theta^{10} \Lambda_2^2}{81 M_\eta^8 M_{\eta'}^2} + \frac{352 F^2 M_\theta^6 M_K^6 s_\theta^{10} \Lambda_2^2}{729 M_\eta^8 M_{\eta'}^2} - \frac{32 F^2 M_\theta^8 M_K^2 M_\pi^2 s_\theta^{10} \Lambda_2^2}{81 M_\eta^8 M_{\eta'}^2} - \\
& \frac{176 F^2 M_\theta^6 M_K^4 M_\pi^2 s_\theta^{10} \Lambda_2^2}{243 M_\eta^8 M_{\eta'}^2} + \frac{16 F^2 M_\theta^8 M_\pi^4 s_\theta^{10} \Lambda_2^2}{81 M_\eta^8 M_{\eta'}^2} + \frac{176 F^2 M_\theta^6 M_\pi^6 s_\theta^{10} \Lambda_2^2}{729 M_\eta^8 M_{\eta'}^2} - \\
& \frac{320 \sqrt{2} F^2 c_\theta M_\theta^8 M_K^6 s_\theta^{11} \Lambda_2^2}{243 M_\eta^{12}} + \frac{80 \sqrt{2} F^2 c_\theta M_\theta^8 M_K^2 M_\pi^4 s_\theta^{11} \Lambda_2^2}{81 M_\eta^{12}} + \frac{80 \sqrt{2} F^2 c_\theta M_\theta^8 M_\pi^6 s_\theta^{11} \Lambda_2^2}{243 M_\eta^{12}} + \\
& \frac{64 \sqrt{2} F^2 c_\theta M_\theta^8 M_K^6 s_\theta^{11} \Lambda_2^2}{243 M_\eta^6 M_{\eta'}^6} - \frac{56 \sqrt{2} F^2 c_\theta M_\theta^8 M_K^4 M_\pi^2 s_\theta^{11} \Lambda_2^2}{81 M_\eta^6 M_{\eta'}^6} + \frac{16 \sqrt{2} F^2 c_\theta M_\theta^8 M_K^2 M_\pi^4 s_\theta^{11} \Lambda_2^2}{27 M_\eta^6 M_{\eta'}^6} - \\
& \frac{40 \sqrt{2} F^2 c_\theta M_\theta^8 M_\pi^6 s_\theta^{11} \Lambda_2^2}{243 M_\eta^6 M_{\eta'}^6} + \frac{320 \sqrt{2} F^2 c_\theta M_\theta^8 M_K^6 s_\theta^{11} \Lambda_2^2}{243 M_\eta^8 M_{\eta'}^4} - \frac{136 \sqrt{2} F^2 c_\theta M_\theta^8 M_K^4 M_\pi^2 s_\theta^{11} \Lambda_2^2}{81 M_\eta^8 M_{\eta'}^4} + \\
& \frac{16 \sqrt{2} F^2 c_\theta M_\theta^8 M_K^2 M_\pi^4 s_\theta^{11} \Lambda_2^2}{27 M_\eta^8 M_{\eta'}^4} - \frac{56 \sqrt{2} F^2 c_\theta M_\theta^8 M_\pi^6 s_\theta^{11} \Lambda_2^2}{243 M_\eta^8 M_{\eta'}^4} - \frac{64 \sqrt{2} F^2 c_\theta M_\theta^8 M_K^6 s_\theta^{11} \Lambda_2^2}{243 M_\eta^{10} M_{\eta'}^2} + \\
& \frac{64 \sqrt{2} F^2 c_\theta M_\theta^8 M_K^4 M_\pi^2 s_\theta^{11} \Lambda_2^2}{27 M_\eta^{10} M_{\eta'}^2} - \frac{176 \sqrt{2} F^2 c_\theta M_\theta^8 M_K^2 M_\pi^4 s_\theta^{11} \Lambda_2^2}{81 M_\eta^{10} M_{\eta'}^2} + \frac{16 \sqrt{2} F^2 c_\theta M_\theta^8 M_\pi^6 s_\theta^{11} \Lambda_2^2}{243 M_\eta^{10} M_{\eta'}^2} - \\
& \frac{160 F^2 M_\theta^8 M_K^6 s_\theta^{12} \Lambda_2^2}{729 M_\eta^{12}} - \frac{80 F^2 M_\theta^8 M_K^4 M_\pi^2 s_\theta^{12} \Lambda_2^2}{243 M_\eta^{12}} - \frac{40 F^2 M_\theta^8 M_K^2 M_\pi^4 s_\theta^{12} \Lambda_2^2}{243 M_\eta^{12}} - \frac{20 F^2 M_\theta^8 M_\pi^6 s_\theta^{12} \Lambda_2^2}{729 M_\eta^{12}} - \\
& \frac{32 F^2 M_\theta^8 M_K^6 s_\theta^{12} \Lambda_2^2}{243 M_\eta^8 M_{\eta'}^4} + \frac{8 F^2 M_\theta^8 M_K^4 M_\pi^2 s_\theta^{12} \Lambda_2^2}{27 M_\eta^8 M_{\eta'}^4} - \frac{16 F^2 M_\theta^8 M_K^2 M_\pi^4 s_\theta^{12} \Lambda_2^2}{81 M_\eta^8 M_{\eta'}^4} + \frac{8 F^2 M_\theta^8 M_\pi^6 s_\theta^{12} \Lambda_2^2}{243 M_\eta^8 M_{\eta'}^4} - \\
& \frac{32 F^2 M_\theta^8 M_K^6 s_\theta^{12} \Lambda_2^2}{81 M_\eta^{10} M_{\eta'}^2} + \frac{16 F^2 M_\theta^8 M_K^4 M_\pi^2 s_\theta^{12} \Lambda_2^2}{27 M_\eta^{10} M_{\eta'}^2} - \frac{16 F^2 M_\theta^8 M_\pi^6 s_\theta^{12} \Lambda_2^2}{81 M_\eta^{10} M_{\eta'}^2} - \frac{16 c_\theta^{10} M_\theta^8 M_K^4 g_1[M_K, T]}{243 M_\eta^{10}} - \\
& \frac{8 c_\theta^{10} M_\theta^8 M_K^2 M_\pi^2 g_1[M_K, T]}{243 M_\eta^{10}} + \frac{2 c_\theta^8 M_\theta^8 M_K^2 g_1[M_K, T]}{81 M_\eta^8} - \frac{16 c_\theta^{10} M_\theta^8 M_K^4 g_1[M_K, T]}{243 M_\eta^2 M_{\eta'}^8} + \\
& \frac{8 c_\theta^{10} M_\theta^8 M_K^2 M_\pi^2 g_1[M_K, T]}{81 M_\eta^2 M_{\eta'}^8} - \frac{8 c_\theta^{10} M_\theta^8 M_\pi^4 g_1[M_K, T]}{243 M_\eta^2 M_{\eta'}^8} + \frac{80 \sqrt{2} c_\theta^9 M_\theta^8 M_K^4 s_\theta g_1[M_K, T]}{243 M_\eta^{10}} -
\end{aligned}$$

$$\begin{aligned}
& \frac{64 \sqrt{2} c_{\theta}^9 M_0^8 M_K^2 M_{\pi}^2 s_{\theta} g_1 [M_K, T]}{243 M_{\eta'}^{10}} - \frac{4 \sqrt{2} c_{\theta}^9 M_0^8 M_{\pi}^4 s_{\theta} g_1 [M_K, T]}{243 M_{\eta'}^{10}} - \\
& \frac{4 \sqrt{2} c_{\theta}^7 M_0^8 M_K^2 s_{\theta} g_1 [M_K, T]}{81 M_{\eta'}^8} + \frac{2 \sqrt{2} c_{\theta}^7 M_0^8 M_{\pi}^2 s_{\theta} g_1 [M_K, T]}{81 M_{\eta'}^8} - \frac{32 \sqrt{2} c_{\theta}^9 M_0^8 M_K^4 s_{\theta} g_1 [M_K, T]}{243 M_{\eta'}^2 M_{\eta'}^8} + \\
& \frac{8 \sqrt{2} c_{\theta}^9 M_0^8 M_K^2 M_{\pi}^2 s_{\theta} g_1 [M_K, T]}{81 M_{\eta'}^2 M_{\eta'}^8} + \frac{14 \sqrt{2} c_{\theta}^9 M_0^8 M_{\pi}^4 s_{\theta} g_1 [M_K, T]}{243 M_{\eta'}^2 M_{\eta'}^8} - \\
& \frac{16 \sqrt{2} c_{\theta}^9 M_0^8 M_K^4 s_{\theta} g_1 [M_K, T]}{81 M_{\eta'}^4 M_{\eta'}^6} + \frac{40 \sqrt{2} c_{\theta}^9 M_0^8 M_K^2 M_{\pi}^2 s_{\theta} g_1 [M_K, T]}{243 M_{\eta'}^4 M_{\eta'}^6} - \\
& \frac{10 \sqrt{2} c_{\theta}^9 M_0^8 M_{\pi}^4 s_{\theta} g_1 [M_K, T]}{243 M_{\eta'}^4 M_{\eta'}^6} + \frac{4 \sqrt{2} c_{\theta}^7 M_0^8 M_K^2 s_{\theta} g_1 [M_K, T]}{81 M_{\eta'}^2 M_{\eta'}^6} - \frac{2 \sqrt{2} c_{\theta}^7 M_0^8 M_{\pi}^2 s_{\theta} g_1 [M_K, T]}{81 M_{\eta'}^2 M_{\eta'}^6} - \\
& \frac{320 c_{\theta}^8 M_0^8 M_K^4 s_{\theta}^2 g_1 [M_K, T]}{243 M_{\eta'}^{10}} + \frac{244 c_{\theta}^8 M_0^8 M_K^2 M_{\pi}^2 s_{\theta}^2 g_1 [M_K, T]}{243 M_{\eta'}^{10}} - \frac{62 c_{\theta}^8 M_0^8 M_{\pi}^4 s_{\theta}^2 g_1 [M_K, T]}{243 M_{\eta'}^{10}} - \\
& \frac{c_{\theta}^6 M_0^8 M_{\pi}^2 s_{\theta}^2 g_1 [M_K, T]}{27 M_{\eta'}^8} + \frac{16 c_{\theta}^8 M_0^8 M_K^4 s_{\theta}^2 g_1 [M_K, T]}{9 M_{\eta'}^2 M_{\eta'}^8} - \frac{116 c_{\theta}^8 M_0^8 M_K^2 M_{\pi}^2 s_{\theta}^2 g_1 [M_K, T]}{81 M_{\eta'}^2 M_{\eta'}^8} + \\
& \frac{8 c_{\theta}^8 M_0^8 M_{\pi}^4 s_{\theta}^2 g_1 [M_K, T]}{27 M_{\eta'}^2 M_{\eta'}^8} - \frac{176 c_{\theta}^8 M_0^8 M_K^4 s_{\theta}^2 g_1 [M_K, T]}{243 M_{\eta'}^4 M_{\eta'}^6} + \frac{52 c_{\theta}^8 M_0^8 M_K^2 M_{\pi}^2 s_{\theta}^2 g_1 [M_K, T]}{243 M_{\eta'}^4 M_{\eta'}^6} - \\
& \frac{14 c_{\theta}^8 M_0^8 M_{\pi}^4 s_{\theta}^2 g_1 [M_K, T]}{243 M_{\eta'}^4 M_{\eta'}^6} + \frac{8 c_{\theta}^6 M_0^8 M_K^2 s_{\theta}^2 g_1 [M_K, T]}{81 M_{\eta'}^2 M_{\eta'}^6} + \frac{2 c_{\theta}^6 M_0^8 M_{\pi}^2 s_{\theta}^2 g_1 [M_K, T]}{27 M_{\eta'}^2 M_{\eta'}^6} - \\
& \frac{32 c_{\theta}^8 M_0^8 M_K^4 s_{\theta}^2 g_1 [M_K, T]}{81 M_{\eta'}^6 M_{\eta'}^4} + \frac{44 c_{\theta}^8 M_0^8 M_K^2 M_{\pi}^2 s_{\theta}^2 g_1 [M_K, T]}{81 M_{\eta'}^6 M_{\eta'}^4} - \frac{4 c_{\theta}^8 M_0^8 M_{\pi}^4 s_{\theta}^2 g_1 [M_K, T]}{27 M_{\eta'}^6 M_{\eta'}^4} - \\
& \frac{c_{\theta}^6 M_0^8 M_{\pi}^2 s_{\theta}^2 g_1 [M_K, T]}{27 M_{\eta'}^4 M_{\eta'}^4} + \frac{320 \sqrt{2} c_{\theta}^7 M_0^8 M_K^4 s_{\theta}^3 g_1 [M_K, T]}{243 M_{\eta'}^{10}} - \frac{80 \sqrt{2} c_{\theta}^7 M_0^8 M_K^2 M_{\pi}^2 s_{\theta}^3 g_1 [M_K, T]}{81 M_{\eta'}^{10}} + \\
& \frac{40 \sqrt{2} c_{\theta}^7 M_0^8 M_{\pi}^4 s_{\theta}^3 g_1 [M_K, T]}{243 M_{\eta'}^{10}} + \frac{22 \sqrt{2} c_{\theta}^5 M_0^8 M_K^2 s_{\theta}^3 g_1 [M_K, T]}{405 M_{\eta'}^8} - \frac{4 \sqrt{2} c_{\theta}^5 M_0^8 M_{\pi}^2 s_{\theta}^3 g_1 [M_K, T]}{135 M_{\eta'}^8} - \\
& \frac{512 \sqrt{2} c_{\theta}^7 M_0^8 M_K^4 s_{\theta}^3 g_1 [M_K, T]}{243 M_{\eta'}^2 M_{\eta'}^8} + \frac{110 \sqrt{2} c_{\theta}^7 M_0^8 M_K^2 M_{\pi}^2 s_{\theta}^3 g_1 [M_K, T]}{81 M_{\eta'}^2 M_{\eta'}^8} - \\
& \frac{94 \sqrt{2} c_{\theta}^7 M_0^8 M_{\pi}^4 s_{\theta}^3 g_1 [M_K, T]}{243 M_{\eta'}^2 M_{\eta'}^8} + \frac{544 \sqrt{2} c_{\theta}^7 M_0^8 M_K^4 s_{\theta}^3 g_1 [M_K, T]}{243 M_{\eta'}^4 M_{\eta'}^6} - \\
& \frac{302 \sqrt{2} c_{\theta}^7 M_0^8 M_K^2 M_{\pi}^2 s_{\theta}^3 g_1 [M_K, T]}{243 M_{\eta'}^4 M_{\eta'}^6} + \frac{70 \sqrt{2} c_{\theta}^7 M_0^8 M_{\pi}^4 s_{\theta}^3 g_1 [M_K, T]}{243 M_{\eta'}^4 M_{\eta'}^6} - \\
& \frac{14 \sqrt{2} c_{\theta}^5 M_0^8 M_K^2 s_{\theta}^3 g_1 [M_K, T]}{45 M_{\eta'}^2 M_{\eta'}^6} + \frac{22 \sqrt{2} c_{\theta}^5 M_0^8 M_{\pi}^2 s_{\theta}^3 g_1 [M_K, T]}{135 M_{\eta'}^2 M_{\eta'}^6} - \frac{320 \sqrt{2} c_{\theta}^7 M_0^8 M_K^4 s_{\theta}^3 g_1 [M_K, T]}{243 M_{\eta'}^6 M_{\eta'}^4} + \\
& \frac{158 \sqrt{2} c_{\theta}^7 M_0^8 M_K^2 M_{\pi}^2 s_{\theta}^3 g_1 [M_K, T]}{243 M_{\eta'}^6 M_{\eta'}^4} + \frac{2 \sqrt{2} c_{\theta}^7 M_0^8 M_{\pi}^4 s_{\theta}^3 g_1 [M_K, T]}{81 M_{\eta'}^6 M_{\eta'}^4} +
\end{aligned}$$



$$\begin{aligned}
& \frac{14 \sqrt{2} c_{\theta}^5 M_0^8 M_K^2 s_{\theta}^3 g_1 [M_K, T]}{45 M_{\eta}^4 M_{\eta'}^4} - \frac{22 \sqrt{2} c_{\theta}^5 M_0^8 M_{\pi}^2 s_{\theta}^3 g_1 [M_K, T]}{135 M_{\eta}^4 M_{\eta'}^4} - \frac{32 \sqrt{2} c_{\theta}^7 M_0^8 M_K^4 s_{\theta}^3 g_1 [M_K, T]}{243 M_{\eta}^8 M_{\eta'}^2} + \\
& \frac{2 \sqrt{2} c_{\theta}^7 M_0^8 M_K^2 M_{\pi}^2 s_{\theta}^3 g_1 [M_K, T]}{9 M_{\eta}^8 M_{\eta'}^2} - \frac{22 \sqrt{2} c_{\theta}^7 M_0^8 M_{\pi}^4 s_{\theta}^3 g_1 [M_K, T]}{243 M_{\eta}^8 M_{\eta'}^2} - \\
& \frac{22 \sqrt{2} c_{\theta}^5 M_0^8 M_K^2 s_{\theta}^3 g_1 [M_K, T]}{405 M_{\eta}^6 M_{\eta'}^2} + \frac{4 \sqrt{2} c_{\theta}^5 M_0^8 M_{\pi}^2 s_{\theta}^3 g_1 [M_K, T]}{135 M_{\eta}^6 M_{\eta'}^2} + \frac{16 c_{\theta}^6 M_0^8 M_K^2 M_{\pi}^2 s_{\theta}^4 g_1 [M_K, T]}{243 M_{\eta}^{10}} - \\
& \frac{7 c_{\theta}^6 M_0^8 M_{\pi}^4 s_{\theta}^4 g_1 [M_K, T]}{243 M_{\eta}^{10}} + \frac{19 c_{\theta}^4 M_0^8 M_K^2 s_{\theta}^4 g_1 [M_K, T]}{810 M_{\eta}^8} + \frac{29 c_{\theta}^4 M_0^8 M_{\pi}^2 s_{\theta}^4 g_1 [M_K, T]}{1620 M_{\eta}^8} - \\
& \frac{320 c_{\theta}^6 M_0^8 M_K^4 s_{\theta}^4 g_1 [M_K, T]}{243 M_{\eta}^{10}} + \frac{364 c_{\theta}^6 M_0^8 M_K^2 M_{\pi}^2 s_{\theta}^4 g_1 [M_K, T]}{243 M_{\eta}^{10}} - \frac{92 c_{\theta}^6 M_0^8 M_{\pi}^4 s_{\theta}^4 g_1 [M_K, T]}{243 M_{\eta}^{10}} + \\
& \frac{19 c_{\theta}^4 M_0^8 M_K^2 s_{\theta}^4 g_1 [M_K, T]}{810 M_{\eta}^8} + \frac{29 c_{\theta}^4 M_0^8 M_{\pi}^2 s_{\theta}^4 g_1 [M_K, T]}{1620 M_{\eta}^8} + \frac{112 c_{\theta}^6 M_0^8 M_K^4 s_{\theta}^4 g_1 [M_K, T]}{243 M_{\eta}^2 M_{\eta'}^8} - \\
& \frac{140 c_{\theta}^6 M_0^8 M_K^2 M_{\pi}^2 s_{\theta}^4 g_1 [M_K, T]}{81 M_{\eta}^2 M_{\eta'}^8} + \frac{95 c_{\theta}^6 M_0^8 M_{\pi}^4 s_{\theta}^4 g_1 [M_K, T]}{243 M_{\eta}^2 M_{\eta'}^8} + \frac{32 c_{\theta}^6 M_0^8 M_K^4 s_{\theta}^4 g_1 [M_K, T]}{243 M_{\eta}^4 M_{\eta'}^6} + \\
& \frac{4 c_{\theta}^6 M_0^8 M_K^2 M_{\pi}^2 s_{\theta}^4 g_1 [M_K, T]}{3 M_{\eta}^4 M_{\eta'}^6} - \frac{92 c_{\theta}^6 M_0^8 M_{\pi}^4 s_{\theta}^4 g_1 [M_K, T]}{243 M_{\eta}^4 M_{\eta'}^6} - \frac{38 c_{\theta}^4 M_0^8 M_K^2 s_{\theta}^4 g_1 [M_K, T]}{405 M_{\eta}^2 M_{\eta'}^6} - \\
& \frac{59 c_{\theta}^4 M_0^8 M_{\pi}^2 s_{\theta}^4 g_1 [M_K, T]}{405 M_{\eta}^2 M_{\eta'}^6} + \frac{272 c_{\theta}^6 M_0^8 M_K^4 s_{\theta}^4 g_1 [M_K, T]}{243 M_{\eta}^6 M_{\eta'}^4} - \frac{556 c_{\theta}^6 M_0^8 M_K^2 M_{\pi}^2 s_{\theta}^4 g_1 [M_K, T]}{243 M_{\eta}^6 M_{\eta'}^4} + \\
& \frac{116 c_{\theta}^6 M_0^8 M_{\pi}^4 s_{\theta}^4 g_1 [M_K, T]}{243 M_{\eta}^6 M_{\eta'}^4} + \frac{13 c_{\theta}^4 M_0^8 M_K^2 s_{\theta}^4 g_1 [M_K, T]}{45 M_{\eta}^4 M_{\eta'}^4} + \frac{23 c_{\theta}^4 M_0^8 M_{\pi}^2 s_{\theta}^4 g_1 [M_K, T]}{90 M_{\eta}^4 M_{\eta'}^4} - \\
& \frac{416 c_{\theta}^6 M_0^8 M_K^4 s_{\theta}^4 g_1 [M_K, T]}{243 M_{\eta}^8 M_{\eta'}^2} + \frac{16 c_{\theta}^6 M_0^8 M_K^2 M_{\pi}^2 s_{\theta}^4 g_1 [M_K, T]}{9 M_{\eta}^8 M_{\eta'}^2} - \frac{100 c_{\theta}^6 M_0^8 M_{\pi}^4 s_{\theta}^4 g_1 [M_K, T]}{243 M_{\eta}^8 M_{\eta'}^2} - \\
& \frac{38 c_{\theta}^4 M_0^8 M_K^2 s_{\theta}^4 g_1 [M_K, T]}{405 M_{\eta}^6 M_{\eta'}^2} - \frac{59 c_{\theta}^4 M_0^8 M_{\pi}^2 s_{\theta}^4 g_1 [M_K, T]}{405 M_{\eta}^6 M_{\eta'}^2} - \frac{64 \sqrt{2} c_{\theta}^5 M_0^8 M_K^4 s_{\theta}^5 g_1 [M_K, T]}{243 M_{\eta}^{10}} + \\
& \frac{92 \sqrt{2} c_{\theta}^5 M_0^8 M_K^2 M_{\pi}^2 s_{\theta}^5 g_1 [M_K, T]}{243 M_{\eta}^{10}} - \frac{34 \sqrt{2} c_{\theta}^5 M_0^8 M_{\pi}^4 s_{\theta}^5 g_1 [M_K, T]}{243 M_{\eta}^{10}} - \\
& \frac{22 \sqrt{2} c_{\theta}^3 M_0^8 M_K^2 s_{\theta}^5 g_1 [M_K, T]}{405 M_{\eta}^8} + \frac{4 \sqrt{2} c_{\theta}^3 M_0^8 M_{\pi}^2 s_{\theta}^5 g_1 [M_K, T]}{135 M_{\eta}^8} + \frac{64 \sqrt{2} c_{\theta}^5 M_0^8 M_K^4 s_{\theta}^5 g_1 [M_K, T]}{243 M_{\eta}^{10}} - \\
& \frac{92 \sqrt{2} c_{\theta}^5 M_0^8 M_K^2 M_{\pi}^2 s_{\theta}^5 g_1 [M_K, T]}{243 M_{\eta}^{10}} + \frac{34 \sqrt{2} c_{\theta}^5 M_0^8 M_{\pi}^4 s_{\theta}^5 g_1 [M_K, T]}{243 M_{\eta}^{10}} + \\
& \frac{16 \sqrt{2} c_{\theta}^5 M_0^8 M_K^4 s_{\theta}^5 g_1 [M_K, T]}{9 M_{\eta}^2 M_{\eta'}^8} - \frac{56 \sqrt{2} c_{\theta}^5 M_0^8 M_K^2 M_{\pi}^2 s_{\theta}^5 g_1 [M_K, T]}{81 M_{\eta}^2 M_{\eta'}^8} - \\
& \frac{4 \sqrt{2} c_{\theta}^5 M_0^8 M_{\pi}^4 s_{\theta}^5 g_1 [M_K, T]}{27 M_{\eta}^2 M_{\eta'}^8} - \frac{848 \sqrt{2} c_{\theta}^5 M_0^8 M_K^4 s_{\theta}^5 g_1 [M_K, T]}{243 M_{\eta}^4 M_{\eta'}^6} +
\end{aligned}$$

$$\begin{aligned}
& \frac{340 \sqrt{2} c_{\theta}^5 M_0^8 M_K^2 M_{\pi}^2 s_{\theta}^5 g_1 [M_K, T]}{243 M_{\eta}^4 M_{\eta'}^6} - \frac{26 \sqrt{2} c_{\theta}^5 M_0^8 M_{\pi}^4 s_{\theta}^5 g_1 [M_K, T]}{243 M_{\eta}^4 M_{\eta'}^6} + \\
& \frac{22 \sqrt{2} c_{\theta}^3 M_0^8 M_K^2 s_{\theta}^5 g_1 [M_K, T]}{405 M_{\eta}^2 M_{\eta'}^6} - \frac{4 \sqrt{2} c_{\theta}^3 M_0^8 M_{\pi}^2 s_{\theta}^5 g_1 [M_K, T]}{135 M_{\eta}^2 M_{\eta'}^6} + \frac{848 \sqrt{2} c_{\theta}^5 M_0^8 M_K^4 s_{\theta}^5 g_1 [M_K, T]}{243 M_{\eta}^6 M_{\eta'}^4} - \\
& \frac{340 \sqrt{2} c_{\theta}^5 M_0^8 M_K^2 M_{\pi}^2 s_{\theta}^5 g_1 [M_K, T]}{243 M_{\eta}^6 M_{\eta'}^4} + \frac{26 \sqrt{2} c_{\theta}^5 M_0^8 M_{\pi}^4 s_{\theta}^5 g_1 [M_K, T]}{243 M_{\eta}^6 M_{\eta'}^4} - \\
& \frac{14 \sqrt{2} c_{\theta}^3 M_0^8 M_K^2 s_{\theta}^5 g_1 [M_K, T]}{45 M_{\eta}^4 M_{\eta'}^4} + \frac{22 \sqrt{2} c_{\theta}^3 M_0^8 M_{\pi}^2 s_{\theta}^5 g_1 [M_K, T]}{135 M_{\eta}^4 M_{\eta'}^4} - \frac{16 \sqrt{2} c_{\theta}^5 M_0^8 M_K^4 s_{\theta}^5 g_1 [M_K, T]}{9 M_{\eta}^8 M_{\eta'}^2} + \\
& \frac{56 \sqrt{2} c_{\theta}^5 M_0^8 M_K^2 M_{\pi}^2 s_{\theta}^5 g_1 [M_K, T]}{81 M_{\eta}^8 M_{\eta'}^2} + \frac{4 \sqrt{2} c_{\theta}^5 M_0^8 M_{\pi}^4 s_{\theta}^5 g_1 [M_K, T]}{27 M_{\eta}^8 M_{\eta'}^2} + \\
& \frac{14 \sqrt{2} c_{\theta}^3 M_0^8 M_K^2 s_{\theta}^5 g_1 [M_K, T]}{45 M_{\eta}^6 M_{\eta'}^2} - \frac{22 \sqrt{2} c_{\theta}^3 M_0^8 M_{\pi}^2 s_{\theta}^5 g_1 [M_K, T]}{135 M_{\eta}^6 M_{\eta'}^2} - \frac{320 c_{\theta}^4 M_0^8 M_K^4 s_{\theta}^6 g_1 [M_K, T]}{243 M_{\eta}^{10}} + \\
& \frac{364 c_{\theta}^4 M_0^8 M_K^2 M_{\pi}^2 s_{\theta}^6 g_1 [M_K, T]}{243 M_{\eta}^{10}} - \frac{92 c_{\theta}^4 M_0^8 M_{\pi}^4 s_{\theta}^6 g_1 [M_K, T]}{243 M_{\eta}^{10}} - \frac{c_{\theta}^2 M_0^8 M_{\pi}^2 s_{\theta}^6 g_1 [M_K, T]}{27 M_{\eta}^8} + \\
& \frac{16 c_{\theta}^4 M_0^8 M_K^2 M_{\pi}^2 s_{\theta}^6 g_1 [M_K, T]}{243 M_{\eta}^{10}} - \frac{7 c_{\theta}^4 M_0^8 M_{\pi}^4 s_{\theta}^6 g_1 [M_K, T]}{243 M_{\eta}^{10}} - \frac{416 c_{\theta}^4 M_0^8 M_K^4 s_{\theta}^6 g_1 [M_K, T]}{243 M_{\eta}^2 M_{\eta'}^8} + \\
& \frac{16 c_{\theta}^4 M_0^8 M_K^2 M_{\pi}^2 s_{\theta}^6 g_1 [M_K, T]}{9 M_{\eta}^2 M_{\eta'}^8} - \frac{100 c_{\theta}^4 M_0^8 M_{\pi}^4 s_{\theta}^6 g_1 [M_K, T]}{243 M_{\eta}^2 M_{\eta'}^8} + \frac{272 c_{\theta}^4 M_0^8 M_K^4 s_{\theta}^6 g_1 [M_K, T]}{243 M_{\eta}^4 M_{\eta'}^6} - \\
& \frac{556 c_{\theta}^4 M_0^8 M_K^2 M_{\pi}^2 s_{\theta}^6 g_1 [M_K, T]}{243 M_{\eta}^4 M_{\eta'}^6} + \frac{116 c_{\theta}^4 M_0^8 M_{\pi}^4 s_{\theta}^6 g_1 [M_K, T]}{243 M_{\eta}^4 M_{\eta'}^6} + \frac{32 c_{\theta}^4 M_0^8 M_K^4 s_{\theta}^6 g_1 [M_K, T]}{243 M_{\eta}^6 M_{\eta'}^4} + \\
& \frac{4 c_{\theta}^4 M_0^8 M_K^2 M_{\pi}^2 s_{\theta}^6 g_1 [M_K, T]}{3 M_{\eta}^6 M_{\eta'}^4} - \frac{92 c_{\theta}^4 M_0^8 M_{\pi}^4 s_{\theta}^6 g_1 [M_K, T]}{243 M_{\eta}^6 M_{\eta'}^4} - \frac{c_{\theta}^2 M_0^8 M_{\pi}^2 s_{\theta}^6 g_1 [M_K, T]}{27 M_{\eta}^4 M_{\eta'}^4} + \\
& \frac{112 c_{\theta}^4 M_0^8 M_K^4 s_{\theta}^6 g_1 [M_K, T]}{243 M_{\eta}^8 M_{\eta'}^2} - \frac{140 c_{\theta}^4 M_0^8 M_K^2 M_{\pi}^2 s_{\theta}^6 g_1 [M_K, T]}{81 M_{\eta}^8 M_{\eta'}^2} + \frac{95 c_{\theta}^4 M_0^8 M_{\pi}^4 s_{\theta}^6 g_1 [M_K, T]}{243 M_{\eta}^8 M_{\eta'}^2} + \\
& \frac{8 c_{\theta}^2 M_0^8 M_K^2 s_{\theta}^6 g_1 [M_K, T]}{81 M_{\eta}^6 M_{\eta'}^2} + \frac{2 c_{\theta}^2 M_0^8 M_{\pi}^2 s_{\theta}^6 g_1 [M_K, T]}{27 M_{\eta}^6 M_{\eta'}^2} - \frac{320 \sqrt{2} c_{\theta}^3 M_0^8 M_K^4 s_{\theta}^7 g_1 [M_K, T]}{243 M_{\eta}^{10}} + \\
& \frac{80 \sqrt{2} c_{\theta}^3 M_0^8 M_K^2 M_{\pi}^2 s_{\theta}^7 g_1 [M_K, T]}{81 M_{\eta}^{10}} - \frac{40 \sqrt{2} c_{\theta}^3 M_0^8 M_{\pi}^4 s_{\theta}^7 g_1 [M_K, T]}{243 M_{\eta}^{10}} + \\
& \frac{4 \sqrt{2} c_{\theta} M_0^8 M_K^2 s_{\theta}^7 g_1 [M_K, T]}{81 M_{\eta}^8} - \frac{2 \sqrt{2} c_{\theta} M_0^8 M_{\pi}^2 s_{\theta}^7 g_1 [M_K, T]}{81 M_{\eta}^8} + \frac{32 \sqrt{2} c_{\theta}^3 M_0^8 M_K^4 s_{\theta}^7 g_1 [M_K, T]}{243 M_{\eta}^2 M_{\eta'}^8} - \\
& \frac{2 \sqrt{2} c_{\theta}^3 M_0^8 M_K^2 M_{\pi}^2 s_{\theta}^7 g_1 [M_K, T]}{9 M_{\eta}^2 M_{\eta'}^8} + \frac{22 \sqrt{2} c_{\theta}^3 M_0^8 M_{\pi}^4 s_{\theta}^7 g_1 [M_K, T]}{243 M_{\eta}^2 M_{\eta'}^8} + \\
& \frac{320 \sqrt{2} c_{\theta}^3 M_0^8 M_K^4 s_{\theta}^7 g_1 [M_K, T]}{243 M_{\eta}^4 M_{\eta'}^6} - \frac{158 \sqrt{2} c_{\theta}^3 M_0^8 M_K^2 M_{\pi}^2 s_{\theta}^7 g_1 [M_K, T]}{243 M_{\eta}^4 M_{\eta'}^6} -
\end{aligned}$$

$$\begin{aligned}
& \frac{2\sqrt{2} c_\theta^3 M_0^8 M_\pi^4 s_\theta^7 g_1 [M_K, T]}{81 M_\eta^4 M_{\eta'}^6} - \frac{544\sqrt{2} c_\theta^3 M_0^8 M_K^4 s_\theta^7 g_1 [M_K, T]}{243 M_\eta^6 M_{\eta'}^4} + \\
& \frac{302\sqrt{2} c_\theta^3 M_0^8 M_K^2 M_\pi^2 s_\theta^7 g_1 [M_K, T]}{243 M_\eta^6 M_{\eta'}^4} - \frac{70\sqrt{2} c_\theta^3 M_0^8 M_\pi^4 s_\theta^7 g_1 [M_K, T]}{243 M_\eta^6 M_{\eta'}^4} + \\
& \frac{512\sqrt{2} c_\theta^3 M_0^8 M_K^4 s_\theta^7 g_1 [M_K, T]}{243 M_\eta^8 M_{\eta'}^2} - \frac{110\sqrt{2} c_\theta^3 M_0^8 M_K^2 M_\pi^2 s_\theta^7 g_1 [M_K, T]}{81 M_\eta^8 M_{\eta'}^2} + \\
& \frac{94\sqrt{2} c_\theta^3 M_0^8 M_\pi^4 s_\theta^7 g_1 [M_K, T]}{243 M_\eta^8 M_{\eta'}^2} - \frac{4\sqrt{2} c_\theta M_0^8 M_K^2 s_\theta^7 g_1 [M_K, T]}{81 M_\eta^6 M_{\eta'}^2} + \frac{2\sqrt{2} c_\theta M_0^8 M_\pi^2 s_\theta^7 g_1 [M_K, T]}{81 M_\eta^6 M_{\eta'}^2} - \\
& \frac{320 c_\theta^2 M_0^8 M_K^4 s_\theta^8 g_1 [M_K, T]}{243 M_\eta^{10}} + \frac{244 c_\theta^2 M_0^8 M_K^2 M_\pi^2 s_\theta^8 g_1 [M_K, T]}{243 M_\eta^{10}} - \frac{62 c_\theta^2 M_0^8 M_\pi^4 s_\theta^8 g_1 [M_K, T]}{243 M_\eta^{10}} + \\
& \frac{2 M_0^8 M_K^2 s_\theta^8 g_1 [M_K, T]}{81 M_\eta^8} - \frac{32 c_\theta^2 M_0^8 M_K^4 s_\theta^8 g_1 [M_K, T]}{81 M_\eta^4 M_{\eta'}^6} + \frac{44 c_\theta^2 M_0^8 M_K^2 M_\pi^2 s_\theta^8 g_1 [M_K, T]}{81 M_\eta^4 M_{\eta'}^6} - \\
& \frac{4 c_\theta^2 M_0^8 M_\pi^4 s_\theta^8 g_1 [M_K, T]}{27 M_\eta^4 M_{\eta'}^6} - \frac{176 c_\theta^2 M_0^8 M_K^4 s_\theta^8 g_1 [M_K, T]}{243 M_\eta^6 M_{\eta'}^4} + \frac{52 c_\theta^2 M_0^8 M_K^2 M_\pi^2 s_\theta^8 g_1 [M_K, T]}{243 M_\eta^6 M_{\eta'}^4} - \\
& \frac{14 c_\theta^2 M_0^8 M_\pi^4 s_\theta^8 g_1 [M_K, T]}{243 M_\eta^6 M_{\eta'}^4} + \frac{16 c_\theta^2 M_0^8 M_K^4 s_\theta^8 g_1 [M_K, T]}{9 M_\eta^8 M_{\eta'}^2} - \frac{116 c_\theta^2 M_0^8 M_K^2 M_\pi^2 s_\theta^8 g_1 [M_K, T]}{81 M_\eta^8 M_{\eta'}^2} + \\
& \frac{8 c_\theta^2 M_0^8 M_\pi^4 s_\theta^8 g_1 [M_K, T]}{27 M_\eta^8 M_{\eta'}^2} - \frac{80\sqrt{2} c_\theta M_0^8 M_K^4 s_\theta^9 g_1 [M_K, T]}{243 M_\eta^{10}} + \frac{64\sqrt{2} c_\theta M_0^8 M_K^2 M_\pi^2 s_\theta^9 g_1 [M_K, T]}{243 M_\eta^{10}} + \\
& \frac{4\sqrt{2} c_\theta M_0^8 M_\pi^4 s_\theta^9 g_1 [M_K, T]}{243 M_\eta^{10}} + \frac{16\sqrt{2} c_\theta M_0^8 M_K^4 s_\theta^9 g_1 [M_K, T]}{81 M_\eta^6 M_{\eta'}^4} - \\
& \frac{40\sqrt{2} c_\theta M_0^8 M_K^2 M_\pi^2 s_\theta^9 g_1 [M_K, T]}{243 M_\eta^6 M_{\eta'}^4} + \frac{10\sqrt{2} c_\theta M_0^8 M_\pi^4 s_\theta^9 g_1 [M_K, T]}{243 M_\eta^6 M_{\eta'}^4} + \\
& \frac{32\sqrt{2} c_\theta M_0^8 M_K^4 s_\theta^9 g_1 [M_K, T]}{243 M_\eta^8 M_{\eta'}^2} - \frac{8\sqrt{2} c_\theta M_0^8 M_K^2 M_\pi^2 s_\theta^9 g_1 [M_K, T]}{81 M_\eta^8 M_{\eta'}^2} - \\
& \frac{14\sqrt{2} c_\theta M_0^8 M_\pi^4 s_\theta^9 g_1 [M_K, T]}{243 M_\eta^8 M_{\eta'}^2} - \frac{16 M_0^8 M_K^4 s_\theta^{10} g_1 [M_K, T]}{243 M_\eta^{10}} - \frac{8 M_0^8 M_K^2 M_\pi^2 s_\theta^{10} g_1 [M_K, T]}{243 M_\eta^{10}} - \\
& \frac{16 M_0^8 M_K^4 s_\theta^{10} g_1 [M_K, T]}{243 M_\eta^8 M_{\eta'}^2} + \frac{8 M_0^8 M_K^2 M_\pi^2 s_\theta^{10} g_1 [M_K, T]}{81 M_\eta^8 M_{\eta'}^2} - \frac{8 M_0^8 M_\pi^4 s_\theta^{10} g_1 [M_K, T]}{243 M_\eta^8 M_{\eta'}^2} - \\
& \frac{4 c_\theta^{10} M_0^8 M_K^2 M_\pi^2 g_1 [M_\pi, T]}{81 M_\eta^{10}} - \frac{2 c_\theta^{10} M_0^8 M_\pi^4 g_1 [M_\pi, T]}{81 M_\eta^{10}} + \frac{c_\theta^8 M_0^8 M_\pi^2 g_1 [M_\pi, T]}{54 M_\eta^8} + \\
& \frac{4 c_\theta^{10} M_0^8 M_K^2 M_\pi^2 g_1 [M_\pi, T]}{81 M_\eta^2 M_{\eta'}^8} - \frac{4 c_\theta^{10} M_0^8 M_\pi^4 g_1 [M_\pi, T]}{81 M_\eta^2 M_{\eta'}^8} + \frac{4\sqrt{2} c_\theta^9 M_0^8 M_K^2 M_\pi^2 s_\theta g_1 [M_\pi, T]}{27 M_\eta^{10}} - \\
& \frac{2\sqrt{2} c_\theta^9 M_0^8 M_\pi^4 s_\theta g_1 [M_\pi, T]}{9 M_\eta^{10}} + \frac{\sqrt{2} c_\theta^7 M_0^8 M_\pi^2 s_\theta g_1 [M_\pi, T]}{27 M_\eta^8} - \frac{22\sqrt{2} c_\theta^9 M_0^8 M_K^2 M_\pi^2 s_\theta g_1 [M_\pi, T]}{81 M_\eta^2 M_{\eta'}^8} +
\end{aligned}$$

$$\begin{aligned}
& \frac{19 \sqrt{2} c_{\theta}^9 M_0^8 M_{\pi}^4 s_{\theta} g_1 [M_{\pi}, T]}{81 M_{\eta}^2 M_{\eta'}^8} + \frac{10 \sqrt{2} c_{\theta}^9 M_0^8 M_K^2 M_{\pi}^2 s_{\theta} g_1 [M_{\pi}, T]}{81 M_{\eta}^4 M_{\eta'}^6} - \\
& \frac{\sqrt{2} c_{\theta}^9 M_0^8 M_{\pi}^4 s_{\theta} g_1 [M_{\pi}, T]}{81 M_{\eta}^4 M_{\eta'}^6} - \frac{\sqrt{2} c_{\theta}^7 M_0^8 M_{\pi}^2 s_{\theta} g_1 [M_{\pi}, T]}{27 M_{\eta}^2 M_{\eta'}^6} - \frac{2 c_{\theta}^8 M_0^8 M_K^2 M_{\pi}^2 s_{\theta}^2 g_1 [M_{\pi}, T]}{9 M_{\eta'}^{10}} - \\
& \frac{7 c_{\theta}^8 M_0^8 M_{\pi}^4 s_{\theta}^2 g_1 [M_{\pi}, T]}{27 M_{\eta'}^{10}} + \frac{c_{\theta}^6 M_0^8 M_{\pi}^2 s_{\theta}^2 g_1 [M_{\pi}, T]}{18 M_{\eta'}^8} + \frac{4 c_{\theta}^8 M_0^8 M_K^2 M_{\pi}^2 s_{\theta}^2 g_1 [M_{\pi}, T]}{9 M_{\eta}^2 M_{\eta'}^8} + \\
& \frac{4 c_{\theta}^8 M_0^8 M_{\pi}^4 s_{\theta}^2 g_1 [M_{\pi}, T]}{27 M_{\eta}^2 M_{\eta'}^8} - \frac{10 c_{\theta}^8 M_0^8 M_K^2 M_{\pi}^2 s_{\theta}^2 g_1 [M_{\pi}, T]}{27 M_{\eta}^4 M_{\eta'}^6} - \frac{c_{\theta}^8 M_0^8 M_{\pi}^4 s_{\theta}^2 g_1 [M_{\pi}, T]}{9 M_{\eta}^4 M_{\eta'}^6} - \\
& \frac{c_{\theta}^6 M_0^8 M_{\pi}^2 s_{\theta}^2 g_1 [M_{\pi}, T]}{27 M_{\eta}^2 M_{\eta'}^6} + \frac{4 c_{\theta}^8 M_0^8 M_K^2 M_{\pi}^2 s_{\theta}^2 g_1 [M_{\pi}, T]}{27 M_{\eta}^6 M_{\eta'}^4} - \frac{4 c_{\theta}^8 M_0^8 M_{\pi}^4 s_{\theta}^2 g_1 [M_{\pi}, T]}{27 M_{\eta}^6 M_{\eta'}^4} + \\
& \frac{c_{\theta}^6 M_0^8 M_{\pi}^2 s_{\theta}^2 g_1 [M_{\pi}, T]}{18 M_{\eta}^4 M_{\eta'}^4} - \frac{8 \sqrt{2} c_{\theta}^7 M_0^8 M_K^2 M_{\pi}^2 s_{\theta}^3 g_1 [M_{\pi}, T]}{81 M_{\eta'}^{10}} - \frac{16 \sqrt{2} c_{\theta}^7 M_0^8 M_{\pi}^4 s_{\theta}^3 g_1 [M_{\pi}, T]}{81 M_{\eta'}^{10}} + \\
& \frac{c_{\theta}^5 M_0^8 M_{\pi}^2 s_{\theta}^3 g_1 [M_{\pi}, T]}{27 \sqrt{2} M_{\eta'}^8} + \frac{56 \sqrt{2} c_{\theta}^7 M_0^8 M_K^2 M_{\pi}^2 s_{\theta}^3 g_1 [M_{\pi}, T]}{81 M_{\eta}^2 M_{\eta'}^8} - \frac{26 \sqrt{2} c_{\theta}^7 M_0^8 M_{\pi}^4 s_{\theta}^3 g_1 [M_{\pi}, T]}{81 M_{\eta}^2 M_{\eta'}^8} - \\
& \frac{28 \sqrt{2} c_{\theta}^7 M_0^8 M_K^2 M_{\pi}^2 s_{\theta}^3 g_1 [M_{\pi}, T]}{27 M_{\eta}^4 M_{\eta'}^6} + \frac{4 \sqrt{2} c_{\theta}^7 M_0^8 M_{\pi}^4 s_{\theta}^3 g_1 [M_{\pi}, T]}{9 M_{\eta}^4 M_{\eta'}^6} + \\
& \frac{c_{\theta}^5 M_0^8 M_{\pi}^2 s_{\theta}^3 g_1 [M_{\pi}, T]}{9 \sqrt{2} M_{\eta}^2 M_{\eta'}^6} + \frac{40 \sqrt{2} c_{\theta}^7 M_0^8 M_K^2 M_{\pi}^2 s_{\theta}^3 g_1 [M_{\pi}, T]}{81 M_{\eta}^6 M_{\eta'}^4} + \frac{2 \sqrt{2} c_{\theta}^7 M_0^8 M_{\pi}^4 s_{\theta}^3 g_1 [M_{\pi}, T]}{81 M_{\eta}^6 M_{\eta'}^4} - \\
& \frac{c_{\theta}^5 M_0^8 M_{\pi}^2 s_{\theta}^3 g_1 [M_{\pi}, T]}{27 \sqrt{2} M_{\eta}^4 M_{\eta'}^4} - \frac{\sqrt{2} c_{\theta}^5 M_0^8 M_{\pi}^2 s_{\theta}^3 g_1 [M_{\pi}, T]}{27 M_{\eta}^4 M_{\eta'}^4} - \frac{4 \sqrt{2} c_{\theta}^7 M_0^8 M_K^2 M_{\pi}^2 s_{\theta}^3 g_1 [M_{\pi}, T]}{81 M_{\eta}^8 M_{\eta'}^2} + \\
& \frac{4 \sqrt{2} c_{\theta}^7 M_0^8 M_{\pi}^4 s_{\theta}^3 g_1 [M_{\pi}, T]}{81 M_{\eta}^8 M_{\eta'}^2} - \frac{c_{\theta}^5 M_0^8 M_{\pi}^2 s_{\theta}^3 g_1 [M_{\pi}, T]}{27 \sqrt{2} M_{\eta}^6 M_{\eta'}^2} - \frac{8 c_{\theta}^6 M_0^8 M_K^2 M_{\pi}^2 s_{\theta}^4 g_1 [M_{\pi}, T]}{81 M_{\eta'}^{10}} + \\
& \frac{7 c_{\theta}^6 M_0^8 M_{\pi}^4 s_{\theta}^4 g_1 [M_{\pi}, T]}{162 M_{\eta'}^{10}} + \frac{c_{\theta}^4 M_0^8 M_{\pi}^2 s_{\theta}^4 g_1 [M_{\pi}, T]}{216 M_{\eta}^8} + \frac{8 c_{\theta}^6 M_0^8 M_K^2 M_{\pi}^2 s_{\theta}^4 g_1 [M_{\pi}, T]}{27 M_{\eta'}^{10}} - \\
& \frac{c_{\theta}^6 M_0^8 M_{\pi}^4 s_{\theta}^4 g_1 [M_{\pi}, T]}{3 M_{\eta'}^{10}} + \frac{c_{\theta}^4 M_0^8 M_{\pi}^2 s_{\theta}^4 g_1 [M_{\pi}, T]}{216 M_{\eta}^8} - \frac{130 c_{\theta}^6 M_0^8 M_K^2 M_{\pi}^2 s_{\theta}^4 g_1 [M_{\pi}, T]}{81 M_{\eta}^2 M_{\eta'}^8} + \\
& \frac{41 c_{\theta}^6 M_0^8 M_{\pi}^4 s_{\theta}^4 g_1 [M_{\pi}, T]}{162 M_{\eta}^2 M_{\eta'}^8} + \frac{232 c_{\theta}^6 M_0^8 M_K^2 M_{\pi}^2 s_{\theta}^4 g_1 [M_{\pi}, T]}{81 M_{\eta}^4 M_{\eta'}^6} - \frac{58 c_{\theta}^6 M_0^8 M_{\pi}^4 s_{\theta}^4 g_1 [M_{\pi}, T]}{81 M_{\eta}^4 M_{\eta'}^6} + \\
& \frac{5 c_{\theta}^4 M_0^8 M_{\pi}^2 s_{\theta}^4 g_1 [M_{\pi}, T]}{54 M_{\eta}^2 M_{\eta'}^6} - \frac{62 c_{\theta}^6 M_0^8 M_K^2 M_{\pi}^2 s_{\theta}^4 g_1 [M_{\pi}, T]}{27 M_{\eta}^6 M_{\eta'}^4} + \frac{2 c_{\theta}^6 M_0^8 M_{\pi}^4 s_{\theta}^4 g_1 [M_{\pi}, T]}{3 M_{\eta}^6 M_{\eta'}^4} - \\
& \frac{c_{\theta}^4 M_0^8 M_{\pi}^2 s_{\theta}^4 g_1 [M_{\pi}, T]}{12 M_{\eta}^4 M_{\eta'}^4} + \frac{68 c_{\theta}^6 M_0^8 M_K^2 M_{\pi}^2 s_{\theta}^4 g_1 [M_{\pi}, T]}{81 M_{\eta}^8 M_{\eta'}^2} - \frac{53 c_{\theta}^6 M_0^8 M_{\pi}^4 s_{\theta}^4 g_1 [M_{\pi}, T]}{81 M_{\eta}^8 M_{\eta'}^2} + \\
& \frac{5 c_{\theta}^4 M_0^8 M_{\pi}^2 s_{\theta}^4 g_1 [M_{\pi}, T]}{54 M_{\eta}^6 M_{\eta'}^2} + \frac{\sqrt{2} c_{\theta}^5 M_0^8 M_{\pi}^4 s_{\theta}^5 g_1 [M_{\pi}, T]}{27 M_{\eta'}^{10}} - \frac{c_{\theta}^3 M_0^8 M_{\pi}^2 s_{\theta}^5 g_1 [M_{\pi}, T]}{27 \sqrt{2} M_{\eta}^8} -
\end{aligned}$$

$$\begin{aligned}
& \frac{\sqrt{2} c_{\theta}^5 M_0^8 M_{\pi}^4 s_{\theta}^5 g_1 [M_{\pi}, T]}{27 M_{\eta'}^{10}} - \frac{2 \sqrt{2} c_{\theta}^5 M_0^8 M_K^2 M_{\pi}^2 s_{\theta}^5 g_1 [M_{\pi}, T]}{9 M_{\eta}^2 M_{\eta'}^8} - \frac{8 \sqrt{2} c_{\theta}^5 M_0^8 M_{\pi}^4 s_{\theta}^5 g_1 [M_{\pi}, T]}{27 M_{\eta}^2 M_{\eta'}^8} + \\
& \frac{22 \sqrt{2} c_{\theta}^5 M_0^8 M_K^2 M_{\pi}^2 s_{\theta}^5 g_1 [M_{\pi}, T]}{27 M_{\eta}^4 M_{\eta'}^6} - \frac{5 \sqrt{2} c_{\theta}^5 M_0^8 M_{\pi}^4 s_{\theta}^5 g_1 [M_{\pi}, T]}{27 M_{\eta}^4 M_{\eta'}^6} + \\
& \frac{c_{\theta}^3 M_0^8 M_{\pi}^2 s_{\theta}^5 g_1 [M_{\pi}, T]}{27 \sqrt{2} M_{\eta}^6 M_{\eta'}^4} - \frac{22 \sqrt{2} c_{\theta}^5 M_0^8 M_K^2 M_{\pi}^2 s_{\theta}^5 g_1 [M_{\pi}, T]}{27 M_{\eta}^6 M_{\eta'}^4} + \frac{5 \sqrt{2} c_{\theta}^5 M_0^8 M_{\pi}^4 s_{\theta}^5 g_1 [M_{\pi}, T]}{27 M_{\eta}^6 M_{\eta'}^4} + \\
& \frac{c_{\theta}^3 M_0^8 M_{\pi}^2 s_{\theta}^5 g_1 [M_{\pi}, T]}{27 \sqrt{2} M_{\eta}^4 M_{\eta'}^4} + \frac{\sqrt{2} c_{\theta}^3 M_0^8 M_{\pi}^2 s_{\theta}^5 g_1 [M_{\pi}, T]}{27 M_{\eta}^4 M_{\eta'}^4} + \frac{2 \sqrt{2} c_{\theta}^5 M_0^8 M_K^2 M_{\pi}^2 s_{\theta}^5 g_1 [M_{\pi}, T]}{9 M_{\eta}^8 M_{\eta'}^2} + \\
& \frac{8 \sqrt{2} c_{\theta}^5 M_0^8 M_{\pi}^4 s_{\theta}^5 g_1 [M_{\pi}, T]}{27 M_{\eta}^8 M_{\eta'}^2} - \frac{c_{\theta}^3 M_0^8 M_{\pi}^2 s_{\theta}^5 g_1 [M_{\pi}, T]}{9 \sqrt{2} M_{\eta}^6 M_{\eta'}^2} + \frac{8 c_{\theta}^4 M_0^8 M_K^2 M_{\pi}^2 s_{\theta}^6 g_1 [M_{\pi}, T]}{27 M_{\eta'}^{10}} - \\
& \frac{c_{\theta}^4 M_0^8 M_{\pi}^4 s_{\theta}^6 g_1 [M_{\pi}, T]}{3 M_{\eta'}^{10}} + \frac{c_{\theta}^2 M_0^8 M_{\pi}^2 s_{\theta}^6 g_1 [M_{\pi}, T]}{18 M_{\eta}^8} - \frac{8 c_{\theta}^4 M_0^8 M_K^2 M_{\pi}^2 s_{\theta}^6 g_1 [M_{\pi}, T]}{81 M_{\eta'}^{10}} + \\
& \frac{7 c_{\theta}^4 M_0^8 M_{\pi}^4 s_{\theta}^6 g_1 [M_{\pi}, T]}{162 M_{\eta'}^{10}} + \frac{68 c_{\theta}^4 M_0^8 M_K^2 M_{\pi}^2 s_{\theta}^6 g_1 [M_{\pi}, T]}{81 M_{\eta}^2 M_{\eta'}^8} - \frac{53 c_{\theta}^4 M_0^8 M_{\pi}^4 s_{\theta}^6 g_1 [M_{\pi}, T]}{81 M_{\eta}^2 M_{\eta'}^8} - \\
& \frac{62 c_{\theta}^4 M_0^8 M_K^2 M_{\pi}^2 s_{\theta}^6 g_1 [M_{\pi}, T]}{27 M_{\eta}^4 M_{\eta'}^6} + \frac{2 c_{\theta}^4 M_0^8 M_{\pi}^4 s_{\theta}^6 g_1 [M_{\pi}, T]}{3 M_{\eta}^4 M_{\eta'}^6} + \frac{232 c_{\theta}^4 M_0^8 M_K^2 M_{\pi}^2 s_{\theta}^6 g_1 [M_{\pi}, T]}{81 M_{\eta}^6 M_{\eta'}^4} - \\
& \frac{58 c_{\theta}^4 M_0^8 M_{\pi}^4 s_{\theta}^6 g_1 [M_{\pi}, T]}{81 M_{\eta}^6 M_{\eta'}^4} + \frac{c_{\theta}^2 M_0^8 M_{\pi}^2 s_{\theta}^6 g_1 [M_{\pi}, T]}{18 M_{\eta}^4 M_{\eta'}^4} - \frac{130 c_{\theta}^4 M_0^8 M_K^2 M_{\pi}^2 s_{\theta}^6 g_1 [M_{\pi}, T]}{81 M_{\eta}^8 M_{\eta'}^2} + \\
& \frac{41 c_{\theta}^4 M_0^8 M_{\pi}^4 s_{\theta}^6 g_1 [M_{\pi}, T]}{162 M_{\eta}^8 M_{\eta'}^2} - \frac{c_{\theta}^2 M_0^8 M_{\pi}^2 s_{\theta}^6 g_1 [M_{\pi}, T]}{27 M_{\eta}^6 M_{\eta'}^2} + \frac{8 \sqrt{2} c_{\theta}^3 M_0^8 M_K^2 M_{\pi}^2 s_{\theta}^7 g_1 [M_{\pi}, T]}{81 M_{\eta'}^{10}} + \\
& \frac{16 \sqrt{2} c_{\theta}^3 M_0^8 M_{\pi}^4 s_{\theta}^7 g_1 [M_{\pi}, T]}{81 M_{\eta'}^{10}} - \frac{\sqrt{2} c_{\theta}^3 M_0^8 M_{\pi}^2 s_{\theta}^7 g_1 [M_{\pi}, T]}{27 M_{\eta}^8} + \frac{4 \sqrt{2} c_{\theta}^3 M_0^8 M_K^2 M_{\pi}^2 s_{\theta}^7 g_1 [M_{\pi}, T]}{81 M_{\eta}^2 M_{\eta'}^8} - \\
& \frac{4 \sqrt{2} c_{\theta}^3 M_0^8 M_{\pi}^4 s_{\theta}^7 g_1 [M_{\pi}, T]}{81 M_{\eta}^2 M_{\eta'}^8} - \frac{40 \sqrt{2} c_{\theta}^3 M_0^8 M_K^2 M_{\pi}^2 s_{\theta}^7 g_1 [M_{\pi}, T]}{81 M_{\eta}^4 M_{\eta'}^6} - \\
& \frac{2 \sqrt{2} c_{\theta}^3 M_0^8 M_{\pi}^4 s_{\theta}^7 g_1 [M_{\pi}, T]}{81 M_{\eta}^4 M_{\eta'}^6} + \frac{28 \sqrt{2} c_{\theta}^3 M_0^8 M_K^2 M_{\pi}^2 s_{\theta}^7 g_1 [M_{\pi}, T]}{27 M_{\eta}^6 M_{\eta'}^4} - \\
& \frac{4 \sqrt{2} c_{\theta}^3 M_0^8 M_{\pi}^4 s_{\theta}^7 g_1 [M_{\pi}, T]}{9 M_{\eta}^6 M_{\eta'}^4} - \frac{56 \sqrt{2} c_{\theta}^3 M_0^8 M_K^2 M_{\pi}^2 s_{\theta}^7 g_1 [M_{\pi}, T]}{81 M_{\eta}^8 M_{\eta'}^2} + \\
& \frac{26 \sqrt{2} c_{\theta}^3 M_0^8 M_{\pi}^4 s_{\theta}^7 g_1 [M_{\pi}, T]}{81 M_{\eta}^8 M_{\eta'}^2} + \frac{\sqrt{2} c_{\theta}^3 M_0^8 M_{\pi}^2 s_{\theta}^7 g_1 [M_{\pi}, T]}{27 M_{\eta}^6 M_{\eta'}^2} - \frac{2 c_{\theta}^2 M_0^8 M_K^2 M_{\pi}^2 s_{\theta}^8 g_1 [M_{\pi}, T]}{9 M_{\eta'}^{10}} - \\
& \frac{7 c_{\theta}^2 M_0^8 M_{\pi}^4 s_{\theta}^8 g_1 [M_{\pi}, T]}{27 M_{\eta'}^{10}} + \frac{M_0^8 M_{\pi}^2 s_{\theta}^8 g_1 [M_{\pi}, T]}{54 M_{\eta}^8} + \frac{4 c_{\theta}^2 M_0^8 M_K^2 M_{\pi}^2 s_{\theta}^8 g_1 [M_{\pi}, T]}{27 M_{\eta}^4 M_{\eta'}^6} - \\
& \frac{4 c_{\theta}^2 M_0^8 M_{\pi}^4 s_{\theta}^8 g_1 [M_{\pi}, T]}{27 M_{\eta}^4 M_{\eta'}^6} - \frac{10 c_{\theta}^2 M_0^8 M_K^2 M_{\pi}^2 s_{\theta}^8 g_1 [M_{\pi}, T]}{27 M_{\eta}^6 M_{\eta'}^4} - \frac{c_{\theta}^2 M_0^8 M_{\pi}^4 s_{\theta}^8 g_1 [M_{\pi}, T]}{9 M_{\eta}^6 M_{\eta'}^4} +
\end{aligned}$$

$$\begin{aligned}
& \frac{4 c_{\theta}^2 M_0^8 M_K^2 M_{\pi}^2 s_{\theta}^8 g_1 [M_{\pi}, T]}{9 M_{\eta}^8 M_{\eta'}^2} + \frac{4 c_{\theta}^2 M_0^8 M_{\pi}^4 s_{\theta}^8 g_1 [M_{\pi}, T]}{27 M_{\eta}^8 M_{\eta'}^2} - \frac{4 \sqrt{2} c_{\theta} M_0^8 M_K^2 M_{\pi}^2 s_{\theta}^9 g_1 [M_{\pi}, T]}{27 M_{\eta}^{10}} + \\
& \frac{2 \sqrt{2} c_{\theta} M_0^8 M_{\pi}^4 s_{\theta}^9 g_1 [M_{\pi}, T]}{9 M_{\eta}^{10}} - \frac{10 \sqrt{2} c_{\theta} M_0^8 M_K^2 M_{\pi}^2 s_{\theta}^9 g_1 [M_{\pi}, T]}{81 M_{\eta}^6 M_{\eta'}^4} + \frac{\sqrt{2} c_{\theta} M_0^8 M_{\pi}^4 s_{\theta}^9 g_1 [M_{\pi}, T]}{81 M_{\eta}^6 M_{\eta'}^4} + \\
& \frac{22 \sqrt{2} c_{\theta} M_0^8 M_K^2 M_{\pi}^2 s_{\theta}^9 g_1 [M_{\pi}, T]}{81 M_{\eta}^8 M_{\eta'}^2} - \frac{19 \sqrt{2} c_{\theta} M_0^8 M_{\pi}^4 s_{\theta}^9 g_1 [M_{\pi}, T]}{81 M_{\eta}^8 M_{\eta'}^2} - \frac{4 M_0^8 M_K^2 M_{\pi}^2 s_{\theta}^{10} g_1 [M_{\pi}, T]}{81 M_{\eta}^{10}} - \\
& \frac{2 M_0^8 M_{\pi}^4 s_{\theta}^{10} g_1 [M_{\pi}, T]}{81 M_{\eta}^{10}} + \frac{4 M_0^8 M_K^2 M_{\pi}^2 s_{\theta}^{10} g_1 [M_{\pi}, T]}{81 M_{\eta}^8 M_{\eta'}^2} - \frac{4 M_0^8 M_{\pi}^4 s_{\theta}^{10} g_1 [M_{\pi}, T]}{81 M_{\eta}^8 M_{\eta'}^2} - \\
& \frac{16 c_{\theta}^{12} M_0^8 M_K^4 g_1 [M_{\eta}, T]}{729 M_{\eta'}^{10}} - \frac{4 c_{\theta}^{12} M_0^8 M_K^2 M_{\pi}^2 g_1 [M_{\eta}, T]}{729 M_{\eta'}^{10}} + \frac{2 c_{\theta}^{12} M_0^8 M_{\pi}^4 g_1 [M_{\eta}, T]}{729 M_{\eta'}^{10}} + \\
& \frac{2 c_{\theta}^{10} M_0^8 M_K^2 g_1 [M_{\eta}, T]}{243 M_{\eta'}^8} - \frac{c_{\theta}^{10} M_0^8 M_{\pi}^2 g_1 [M_{\eta}, T]}{486 M_{\eta'}^8} - \frac{32 c_{\theta}^{12} M_0^8 M_K^4 g_1 [M_{\eta}, T]}{729 M_{\eta'}^2 M_{\eta'}^8} + \\
& \frac{52 c_{\theta}^{12} M_0^8 M_K^2 M_{\pi}^2 g_1 [M_{\eta}, T]}{729 M_{\eta'}^2 M_{\eta'}^8} - \frac{20 c_{\theta}^{12} M_0^8 M_{\pi}^4 g_1 [M_{\eta}, T]}{729 M_{\eta'}^2 M_{\eta'}^8} + \frac{8 c_{\theta}^{12} M_0^8 M_K^4 g_1 [M_{\eta}, T]}{243 M_{\eta'}^8 (M_{\eta}^2 - M_{\eta'}^2)} - \\
& \frac{16 c_{\theta}^{12} M_0^8 M_K^2 M_{\pi}^2 g_1 [M_{\eta}, T]}{243 M_{\eta'}^8 (M_{\eta}^2 - M_{\eta'}^2)} + \frac{8 c_{\theta}^{12} M_0^8 M_{\pi}^4 g_1 [M_{\eta}, T]}{243 M_{\eta'}^8 (M_{\eta}^2 - M_{\eta'}^2)} + \frac{80 \sqrt{2} c_{\theta}^{11} M_0^8 M_K^4 s_{\theta} g_1 [M_{\eta}, T]}{729 M_{\eta'}^{10}} - \\
& \frac{76 \sqrt{2} c_{\theta}^{11} M_0^8 M_K^2 M_{\pi}^2 s_{\theta} g_1 [M_{\eta}, T]}{729 M_{\eta'}^{10}} + \frac{14 \sqrt{2} c_{\theta}^{11} M_0^8 M_{\pi}^4 s_{\theta} g_1 [M_{\eta}, T]}{729 M_{\eta'}^{10}} - \\
& \frac{2 \sqrt{2} c_{\theta}^9 M_0^8 M_K^2 s_{\theta} g_1 [M_{\eta}, T]}{81 M_{\eta'}^8} + \frac{\sqrt{2} c_{\theta}^9 M_0^8 M_{\pi}^2 s_{\theta} g_1 [M_{\eta}, T]}{81 M_{\eta'}^8} - \frac{2 \sqrt{2} c_{\theta}^{11} M_0^8 M_K^2 M_{\pi}^2 s_{\theta} g_1 [M_{\eta}, T]}{243 M_{\eta'}^2 M_{\eta'}^8} + \\
& \frac{5 \sqrt{2} c_{\theta}^{11} M_0^8 M_{\pi}^4 s_{\theta} g_1 [M_{\eta}, T]}{243 M_{\eta'}^2 M_{\eta'}^8} - \frac{128 \sqrt{2} c_{\theta}^{11} M_0^8 M_K^4 s_{\theta} g_1 [M_{\eta}, T]}{729 M_{\eta'}^4 M_{\eta'}^6} + \\
& \frac{130 \sqrt{2} c_{\theta}^{11} M_0^8 M_K^2 M_{\pi}^2 s_{\theta} g_1 [M_{\eta}, T]}{729 M_{\eta'}^4 M_{\eta'}^6} - \frac{29 \sqrt{2} c_{\theta}^{11} M_0^8 M_{\pi}^4 s_{\theta} g_1 [M_{\eta}, T]}{729 M_{\eta'}^4 M_{\eta'}^6} + \\
& \frac{8 \sqrt{2} c_{\theta}^9 M_0^8 M_K^2 s_{\theta} g_1 [M_{\eta}, T]}{243 M_{\eta'}^2 M_{\eta'}^6} - \frac{5 \sqrt{2} c_{\theta}^9 M_0^8 M_{\pi}^2 s_{\theta} g_1 [M_{\eta}, T]}{243 M_{\eta'}^2 M_{\eta'}^6} - \frac{40 \sqrt{2} c_{\theta}^{11} M_0^8 M_K^4 s_{\theta} g_1 [M_{\eta}, T]}{243 M_{\eta'}^8 (M_{\eta}^2 - M_{\eta'}^2)} + \\
& \frac{56 \sqrt{2} c_{\theta}^{11} M_0^8 M_K^2 M_{\pi}^2 s_{\theta} g_1 [M_{\eta}, T]}{243 M_{\eta'}^8 (M_{\eta}^2 - M_{\eta'}^2)} - \frac{16 \sqrt{2} c_{\theta}^{11} M_0^8 M_{\pi}^4 s_{\theta} g_1 [M_{\eta}, T]}{243 M_{\eta'}^8 (M_{\eta}^2 - M_{\eta'}^2)} + \\
& \frac{32 \sqrt{2} c_{\theta}^{11} M_0^8 M_K^4 s_{\theta} g_1 [M_{\eta}, T]}{243 M_{\eta'}^2 M_{\eta'}^6 (M_{\eta}^2 - M_{\eta'}^2)} - \frac{40 \sqrt{2} c_{\theta}^{11} M_0^8 M_K^2 M_{\pi}^2 s_{\theta} g_1 [M_{\eta}, T]}{243 M_{\eta'}^2 M_{\eta'}^6 (M_{\eta}^2 - M_{\eta'}^2)} + \\
& \frac{8 \sqrt{2} c_{\theta}^{11} M_0^8 M_{\pi}^4 s_{\theta} g_1 [M_{\eta}, T]}{243 M_{\eta'}^2 M_{\eta'}^6 (M_{\eta}^2 - M_{\eta'}^2)} - \frac{296 c_{\theta}^{10} M_0^8 M_K^4 s_{\theta}^2 g_1 [M_{\eta}, T]}{729 M_{\eta'}^{10}} + \frac{262 c_{\theta}^{10} M_0^8 M_K^2 M_{\pi}^2 s_{\theta}^2 g_1 [M_{\eta}, T]}{729 M_{\eta'}^{10}} -
\end{aligned}$$

$$\begin{aligned}
& \frac{47 c_{\theta}^{10} M_0^8 M_{\pi}^4 s_{\theta}^2 g_1 [M_{\eta}, T]}{729 M_{\eta'}^{10}} + \frac{c_{\theta}^8 M_0^8 M_K^2 s_{\theta}^2 g_1 [M_{\eta}, T]}{27 M_{\eta'}^8} - \frac{2 c_{\theta}^8 M_0^8 M_{\pi}^2 s_{\theta}^2 g_1 [M_{\eta}, T]}{81 M_{\eta'}^8} + \\
& \frac{160 c_{\theta}^{10} M_0^8 M_K^4 s_{\theta}^2 g_1 [M_{\eta}, T]}{243 M_{\eta'}^2 M_{\eta'}^8} - \frac{164 c_{\theta}^{10} M_0^8 M_K^2 M_{\pi}^2 s_{\theta}^2 g_1 [M_{\eta}, T]}{243 M_{\eta'}^2 M_{\eta'}^8} + \frac{40 c_{\theta}^{10} M_0^8 M_{\pi}^4 s_{\theta}^2 g_1 [M_{\eta}, T]}{243 M_{\eta'}^2 M_{\eta'}^8} - \\
& \frac{64 c_{\theta}^{10} M_0^8 M_K^4 s_{\theta}^2 g_1 [M_{\eta}, T]}{729 M_{\eta'}^4 M_{\eta'}^6} + \frac{122 c_{\theta}^{10} M_0^8 M_K^2 M_{\pi}^2 s_{\theta}^2 g_1 [M_{\eta}, T]}{729 M_{\eta'}^4 M_{\eta'}^6} - \frac{85 c_{\theta}^{10} M_0^8 M_{\pi}^4 s_{\theta}^2 g_1 [M_{\eta}, T]}{729 M_{\eta'}^4 M_{\eta'}^6} - \\
& \frac{8 c_{\theta}^8 M_0^8 M_K^2 s_{\theta}^2 g_1 [M_{\eta}, T]}{81 M_{\eta'}^2 M_{\eta'}^6} + \frac{5 c_{\theta}^8 M_0^8 M_{\pi}^2 s_{\theta}^2 g_1 [M_{\eta}, T]}{81 M_{\eta'}^2 M_{\eta'}^6} - \frac{128 c_{\theta}^{10} M_0^8 M_K^4 s_{\theta}^2 g_1 [M_{\eta}, T]}{243 M_{\eta'}^6 M_{\eta'}^4} + \\
& \frac{124 c_{\theta}^{10} M_0^8 M_K^2 M_{\pi}^2 s_{\theta}^2 g_1 [M_{\eta}, T]}{243 M_{\eta'}^6 M_{\eta'}^4} - \frac{32 c_{\theta}^{10} M_0^8 M_{\pi}^4 s_{\theta}^2 g_1 [M_{\eta}, T]}{243 M_{\eta'}^6 M_{\eta'}^4} + \frac{8 c_{\theta}^8 M_0^8 M_K^2 s_{\theta}^2 g_1 [M_{\eta}, T]}{81 M_{\eta'}^4 M_{\eta'}^4} - \\
& \frac{7 c_{\theta}^8 M_0^8 M_{\pi}^2 s_{\theta}^2 g_1 [M_{\eta}, T]}{162 M_{\eta'}^4 M_{\eta'}^4} + \frac{148 c_{\theta}^{10} M_0^8 M_K^4 s_{\theta}^2 g_1 [M_{\eta}, T]}{243 M_{\eta'}^8 (M_{\eta}^2 - M_{\eta'}^2)} - \frac{140 c_{\theta}^{10} M_0^8 M_K^2 M_{\pi}^2 s_{\theta}^2 g_1 [M_{\eta}, T]}{243 M_{\eta'}^8 (M_{\eta}^2 - M_{\eta'}^2)} + \\
& \frac{28 c_{\theta}^{10} M_0^8 M_{\pi}^4 s_{\theta}^2 g_1 [M_{\eta}, T]}{243 M_{\eta'}^8 (M_{\eta}^2 - M_{\eta'}^2)} - \frac{224 c_{\theta}^{10} M_0^8 M_K^4 s_{\theta}^2 g_1 [M_{\eta}, T]}{243 M_{\eta'}^2 M_{\eta'}^6 (M_{\eta}^2 - M_{\eta'}^2)} + \frac{184 c_{\theta}^{10} M_0^8 M_K^2 M_{\pi}^2 s_{\theta}^2 g_1 [M_{\eta}, T]}{243 M_{\eta'}^2 M_{\eta'}^6 (M_{\eta}^2 - M_{\eta'}^2)} - \\
& \frac{32 c_{\theta}^{10} M_0^8 M_{\pi}^4 s_{\theta}^2 g_1 [M_{\eta}, T]}{243 M_{\eta'}^2 M_{\eta'}^6 (M_{\eta}^2 - M_{\eta'}^2)} + \frac{32 c_{\theta}^{10} M_0^8 M_K^4 s_{\theta}^2 g_1 [M_{\eta}, T]}{81 M_{\eta'}^4 M_{\eta'}^4 (M_{\eta}^2 - M_{\eta'}^2)} - \frac{28 c_{\theta}^{10} M_0^8 M_K^2 M_{\pi}^2 s_{\theta}^2 g_1 [M_{\eta}, T]}{81 M_{\eta'}^4 M_{\eta'}^4 (M_{\eta}^2 - M_{\eta'}^2)} + \\
& \frac{8 c_{\theta}^{10} M_0^8 M_{\pi}^4 s_{\theta}^2 g_1 [M_{\eta}, T]}{81 M_{\eta'}^4 M_{\eta'}^4 (M_{\eta}^2 - M_{\eta'}^2)} + \frac{208 \sqrt{2} c_{\theta}^9 M_0^8 M_K^4 s_{\theta}^3 g_1 [M_{\eta}, T]}{729 M_{\eta'}^{10}} - \frac{92 \sqrt{2} c_{\theta}^9 M_0^8 M_K^2 M_{\pi}^2 s_{\theta}^3 g_1 [M_{\eta}, T]}{729 M_{\eta'}^{10}} + \\
& \frac{10 \sqrt{2} c_{\theta}^9 M_0^8 M_{\pi}^4 s_{\theta}^3 g_1 [M_{\eta}, T]}{729 M_{\eta'}^{10}} + \frac{4 \sqrt{2} c_{\theta}^7 M_0^8 M_K^2 s_{\theta}^3 g_1 [M_{\eta}, T]}{243 M_{\eta'}^8} - \frac{5 c_{\theta}^7 M_0^8 M_{\pi}^2 s_{\theta}^3 g_1 [M_{\eta}, T]}{243 \sqrt{2} M_{\eta'}^8} - \\
& \frac{64 \sqrt{2} c_{\theta}^9 M_0^8 M_K^4 s_{\theta}^3 g_1 [M_{\eta}, T]}{81 M_{\eta'}^2 M_{\eta'}^8} + \frac{100 \sqrt{2} c_{\theta}^9 M_0^8 M_K^2 M_{\pi}^2 s_{\theta}^3 g_1 [M_{\eta}, T]}{243 M_{\eta'}^2 M_{\eta'}^8} - \\
& \frac{16 \sqrt{2} c_{\theta}^9 M_0^8 M_{\pi}^4 s_{\theta}^3 g_1 [M_{\eta}, T]}{243 M_{\eta'}^2 M_{\eta'}^8} + \frac{896 \sqrt{2} c_{\theta}^9 M_0^8 M_K^4 s_{\theta}^3 g_1 [M_{\eta}, T]}{729 M_{\eta'}^4 M_{\eta'}^6} - \\
& \frac{652 \sqrt{2} c_{\theta}^9 M_0^8 M_K^2 M_{\pi}^2 s_{\theta}^3 g_1 [M_{\eta}, T]}{729 M_{\eta'}^4 M_{\eta'}^6} + \frac{152 \sqrt{2} c_{\theta}^9 M_0^8 M_{\pi}^4 s_{\theta}^3 g_1 [M_{\eta}, T]}{729 M_{\eta'}^4 M_{\eta'}^6} - \\
& \frac{4 \sqrt{2} c_{\theta}^7 M_0^8 M_K^2 s_{\theta}^3 g_1 [M_{\eta}, T]}{81 M_{\eta'}^2 M_{\eta'}^6} + \frac{5 c_{\theta}^7 M_0^8 M_{\pi}^2 s_{\theta}^3 g_1 [M_{\eta}, T]}{81 \sqrt{2} M_{\eta'}^2 M_{\eta'}^6} - \frac{512 \sqrt{2} c_{\theta}^9 M_0^8 M_K^4 s_{\theta}^3 g_1 [M_{\eta}, T]}{729 M_{\eta'}^6 M_{\eta'}^4} + \\
& \frac{412 \sqrt{2} c_{\theta}^9 M_0^8 M_K^2 M_{\pi}^2 s_{\theta}^3 g_1 [M_{\eta}, T]}{729 M_{\eta'}^6 M_{\eta'}^4} - \frac{44 \sqrt{2} c_{\theta}^9 M_0^8 M_{\pi}^4 s_{\theta}^3 g_1 [M_{\eta}, T]}{729 M_{\eta'}^6 M_{\eta'}^4} - \\
& \frac{c_{\theta}^7 M_0^8 M_{\pi}^2 s_{\theta}^3 g_1 [M_{\eta}, T]}{81 \sqrt{2} M_{\eta'}^4 M_{\eta'}^4} - \frac{\sqrt{2} c_{\theta}^7 M_0^8 M_{\pi}^2 s_{\theta}^3 g_1 [M_{\eta}, T]}{81 M_{\eta'}^4 M_{\eta'}^4} - \frac{256 \sqrt{2} c_{\theta}^9 M_0^8 M_K^4 s_{\theta}^3 g_1 [M_{\eta}, T]}{729 M_{\eta'}^8 M_{\eta'}^2} +
\end{aligned}$$

$$\begin{aligned}
& \frac{272 \sqrt{2} c_{\theta}^9 M_0^8 M_K^2 M_{\pi}^2 s_{\theta}^3 g_1 [M_{\eta}, T]}{729 M_{\eta}^8 M_{\eta'}^2} - \frac{70 \sqrt{2} c_{\theta}^9 M_0^8 M_{\pi}^4 s_{\theta}^3 g_1 [M_{\eta}, T]}{729 M_{\eta}^8 M_{\eta'}^2} + \\
& \frac{16 \sqrt{2} c_{\theta}^7 M_0^8 M_K^2 s_{\theta}^3 g_1 [M_{\eta}, T]}{243 M_{\eta}^6 M_{\eta'}^2} - \frac{17 c_{\theta}^7 M_0^8 M_{\pi}^2 s_{\theta}^3 g_1 [M_{\eta}, T]}{243 \sqrt{2} M_{\eta}^6 M_{\eta'}^2} - \frac{104 \sqrt{2} c_{\theta}^9 M_0^8 M_K^4 s_{\theta}^3 g_1 [M_{\eta}, T]}{243 M_{\eta}^8 (M_{\eta}^2 - M_{\eta'}^2)} + \\
& \frac{64 \sqrt{2} c_{\theta}^9 M_0^8 M_K^2 M_{\pi}^2 s_{\theta}^3 g_1 [M_{\eta}, T]}{243 M_{\eta}^8 (M_{\eta}^2 - M_{\eta'}^2)} - \frac{14 \sqrt{2} c_{\theta}^9 M_0^8 M_{\pi}^4 s_{\theta}^3 g_1 [M_{\eta}, T]}{243 M_{\eta}^8 (M_{\eta}^2 - M_{\eta'}^2)} + \\
& \frac{208 \sqrt{2} c_{\theta}^9 M_0^8 M_K^4 s_{\theta}^3 g_1 [M_{\eta}, T]}{243 M_{\eta}^2 M_{\eta'}^6 (M_{\eta}^2 - M_{\eta'}^2)} - \frac{92 \sqrt{2} c_{\theta}^9 M_0^8 M_K^2 M_{\pi}^2 s_{\theta}^3 g_1 [M_{\eta}, T]}{243 M_{\eta}^2 M_{\eta'}^6 (M_{\eta}^2 - M_{\eta'}^2)} + \\
& \frac{10 \sqrt{2} c_{\theta}^9 M_0^8 M_{\pi}^4 s_{\theta}^3 g_1 [M_{\eta}, T]}{243 M_{\eta}^2 M_{\eta'}^6 (M_{\eta}^2 - M_{\eta'}^2)} - \frac{64 \sqrt{2} c_{\theta}^9 M_0^8 M_K^4 s_{\theta}^3 g_1 [M_{\eta}, T]}{81 M_{\eta}^4 M_{\eta'}^4 (M_{\eta}^2 - M_{\eta'}^2)} + \\
& \frac{44 \sqrt{2} c_{\theta}^9 M_0^8 M_K^2 M_{\pi}^2 s_{\theta}^3 g_1 [M_{\eta}, T]}{81 M_{\eta}^4 M_{\eta'}^4 (M_{\eta}^2 - M_{\eta'}^2)} - \frac{10 \sqrt{2} c_{\theta}^9 M_0^8 M_{\pi}^4 s_{\theta}^3 g_1 [M_{\eta}, T]}{81 M_{\eta}^4 M_{\eta'}^4 (M_{\eta}^2 - M_{\eta'}^2)} + \\
& \frac{64 \sqrt{2} c_{\theta}^9 M_0^8 M_K^4 s_{\theta}^3 g_1 [M_{\eta}, T]}{243 M_{\eta}^6 M_{\eta'}^2 (M_{\eta}^2 - M_{\eta'}^2)} - \frac{56 \sqrt{2} c_{\theta}^9 M_0^8 M_K^2 M_{\pi}^2 s_{\theta}^3 g_1 [M_{\eta}, T]}{243 M_{\eta}^6 M_{\eta'}^2 (M_{\eta}^2 - M_{\eta'}^2)} + \\
& \frac{10 \sqrt{2} c_{\theta}^9 M_0^8 M_{\pi}^4 s_{\theta}^3 g_1 [M_{\eta}, T]}{243 M_{\eta}^6 M_{\eta'}^2 (M_{\eta}^2 - M_{\eta'}^2)} - \frac{128 c_{\theta}^8 M_0^8 M_K^4 s_{\theta}^4 g_1 [M_{\eta}, T]}{729 M_{\eta}^{10}} + \frac{112 c_{\theta}^8 M_0^8 M_K^2 M_{\pi}^2 s_{\theta}^4 g_1 [M_{\eta}, T]}{729 M_{\eta}^{10}} - \\
& \frac{49 c_{\theta}^8 M_0^8 M_{\pi}^4 s_{\theta}^4 g_1 [M_{\eta}, T]}{1458 M_{\eta}^{10}} + \frac{8 c_{\theta}^6 M_0^8 M_K^2 s_{\theta}^4 g_1 [M_{\eta}, T]}{243 M_{\eta}^8} - \frac{31 c_{\theta}^6 M_0^8 M_{\pi}^2 s_{\theta}^4 g_1 [M_{\eta}, T]}{1944 M_{\eta}^8} + \\
& \frac{80 c_{\theta}^8 M_0^8 M_K^4 s_{\theta}^4 g_1 [M_{\eta}, T]}{729 M_{\eta}^{10}} - \frac{40 c_{\theta}^8 M_0^8 M_K^2 M_{\pi}^2 s_{\theta}^4 g_1 [M_{\eta}, T]}{729 M_{\eta}^{10}} + \frac{5 c_{\theta}^8 M_0^8 M_{\pi}^4 s_{\theta}^4 g_1 [M_{\eta}, T]}{729 M_{\eta}^{10}} - \\
& \frac{4 c_{\theta}^6 M_0^8 M_K^2 s_{\theta}^4 g_1 [M_{\eta}, T]}{81 M_{\eta}^8} + \frac{19 c_{\theta}^6 M_0^8 M_{\pi}^2 s_{\theta}^4 g_1 [M_{\eta}, T]}{648 M_{\eta}^8} - \frac{40 c_{\theta}^8 M_0^8 M_K^4 s_{\theta}^4 g_1 [M_{\eta}, T]}{81 M_{\eta}^2 M_{\eta'}^8} + \\
& \frac{46 c_{\theta}^8 M_0^8 M_K^2 M_{\pi}^2 s_{\theta}^4 g_1 [M_{\eta}, T]}{243 M_{\eta}^2 M_{\eta'}^8} + \frac{19 c_{\theta}^8 M_0^8 M_{\pi}^4 s_{\theta}^4 g_1 [M_{\eta}, T]}{486 M_{\eta}^2 M_{\eta'}^8} + \frac{64 c_{\theta}^8 M_0^8 M_K^4 s_{\theta}^4 g_1 [M_{\eta}, T]}{729 M_{\eta}^4 M_{\eta'}^6} + \\
& \frac{268 c_{\theta}^8 M_0^8 M_K^2 M_{\pi}^2 s_{\theta}^4 g_1 [M_{\eta}, T]}{729 M_{\eta}^4 M_{\eta'}^6} - \frac{116 c_{\theta}^8 M_0^8 M_{\pi}^4 s_{\theta}^4 g_1 [M_{\eta}, T]}{729 M_{\eta}^4 M_{\eta'}^6} + \frac{44 c_{\theta}^6 M_0^8 M_K^2 s_{\theta}^4 g_1 [M_{\eta}, T]}{243 M_{\eta}^2 M_{\eta'}^6} - \\
& \frac{55 c_{\theta}^6 M_0^8 M_{\pi}^2 s_{\theta}^4 g_1 [M_{\eta}, T]}{486 M_{\eta}^2 M_{\eta'}^6} + \frac{1088 c_{\theta}^8 M_0^8 M_K^4 s_{\theta}^4 g_1 [M_{\eta}, T]}{729 M_{\eta}^6 M_{\eta'}^4} - \frac{1318 c_{\theta}^8 M_0^8 M_K^2 M_{\pi}^2 s_{\theta}^4 g_1 [M_{\eta}, T]}{729 M_{\eta}^6 M_{\eta'}^4} + \\
& \frac{248 c_{\theta}^8 M_0^8 M_{\pi}^4 s_{\theta}^4 g_1 [M_{\eta}, T]}{729 M_{\eta}^6 M_{\eta'}^4} - \frac{8 c_{\theta}^6 M_0^8 M_K^2 s_{\theta}^4 g_1 [M_{\eta}, T]}{27 M_{\eta}^4 M_{\eta'}^4} + \frac{19 c_{\theta}^6 M_0^8 M_{\pi}^2 s_{\theta}^4 g_1 [M_{\eta}, T]}{108 M_{\eta}^4 M_{\eta'}^4} - \\
& \frac{448 c_{\theta}^8 M_0^8 M_K^4 s_{\theta}^4 g_1 [M_{\eta}, T]}{243 M_{\eta}^8 M_{\eta'}^2} + \frac{160 c_{\theta}^8 M_0^8 M_K^2 M_{\pi}^2 s_{\theta}^4 g_1 [M_{\eta}, T]}{81 M_{\eta}^8 M_{\eta'}^2} - \frac{137 c_{\theta}^8 M_0^8 M_{\pi}^4 s_{\theta}^4 g_1 [M_{\eta}, T]}{243 M_{\eta}^8 M_{\eta'}^2} +
\end{aligned}$$



$$\begin{aligned}
& \frac{16 c_{\theta}^6 M_0^8 M_K^2 S_{\theta}^4 g_1 [M_{\eta}, T]}{81 M_{\eta}^6 M_{\eta'}^2} - \frac{13 c_{\theta}^6 M_0^8 M_{\pi}^2 S_{\theta}^4 g_1 [M_{\eta}, T]}{162 M_{\eta}^6 M_{\eta'}^2} + \frac{32 c_{\theta}^8 M_0^8 M_K^4 S_{\theta}^4 g_1 [M_{\eta}, T]}{243 M_{\eta}^8 (M_{\eta}^2 - M_{\eta'}^2)} - \\
& \frac{40 c_{\theta}^8 M_0^8 M_K^2 M_{\pi}^2 S_{\theta}^4 g_1 [M_{\eta}, T]}{243 M_{\eta}^8 (M_{\eta}^2 - M_{\eta'}^2)} + \frac{25 c_{\theta}^8 M_0^8 M_{\pi}^4 S_{\theta}^4 g_1 [M_{\eta}, T]}{486 M_{\eta}^8 (M_{\eta}^2 - M_{\eta'}^2)} - \frac{40 c_{\theta}^8 M_0^8 M_K^4 S_{\theta}^4 g_1 [M_{\eta}, T]}{243 M_{\eta'}^8 (M_{\eta}^2 - M_{\eta'}^2)} + \\
& \frac{38 c_{\theta}^8 M_0^8 M_K^2 M_{\pi}^2 S_{\theta}^4 g_1 [M_{\eta}, T]}{243 M_{\eta'}^8 (M_{\eta}^2 - M_{\eta'}^2)} - \frac{23 c_{\theta}^8 M_0^8 M_{\pi}^4 S_{\theta}^4 g_1 [M_{\eta}, T]}{486 M_{\eta'}^8 (M_{\eta}^2 - M_{\eta'}^2)} + \frac{176 c_{\theta}^8 M_0^8 M_K^4 S_{\theta}^4 g_1 [M_{\eta}, T]}{243 M_{\eta}^2 M_{\eta'}^6 (M_{\eta}^2 - M_{\eta'}^2)} - \\
& \frac{148 c_{\theta}^8 M_0^8 M_K^2 M_{\pi}^2 S_{\theta}^4 g_1 [M_{\eta}, T]}{243 M_{\eta}^2 M_{\eta'}^6 (M_{\eta}^2 - M_{\eta'}^2)} + \frac{26 c_{\theta}^8 M_0^8 M_{\pi}^4 S_{\theta}^4 g_1 [M_{\eta}, T]}{243 M_{\eta}^2 M_{\eta'}^6 (M_{\eta}^2 - M_{\eta'}^2)} - \frac{32 c_{\theta}^8 M_0^8 M_K^4 S_{\theta}^4 g_1 [M_{\eta}, T]}{81 M_{\eta}^4 M_{\eta'}^4 (M_{\eta}^2 - M_{\eta'}^2)} + \\
& \frac{10 c_{\theta}^8 M_0^8 M_K^2 M_{\pi}^2 S_{\theta}^4 g_1 [M_{\eta}, T]}{81 M_{\eta}^4 M_{\eta'}^4 (M_{\eta}^2 - M_{\eta'}^2)} + \frac{c_{\theta}^8 M_0^8 M_{\pi}^4 S_{\theta}^4 g_1 [M_{\eta}, T]}{81 M_{\eta}^4 M_{\eta'}^4 (M_{\eta}^2 - M_{\eta'}^2)} - \frac{64 c_{\theta}^8 M_0^8 M_K^4 S_{\theta}^4 g_1 [M_{\eta}, T]}{243 M_{\eta}^6 M_{\eta'}^2 (M_{\eta}^2 - M_{\eta'}^2)} + \\
& \frac{104 c_{\theta}^8 M_0^8 M_K^2 M_{\pi}^2 S_{\theta}^4 g_1 [M_{\eta}, T]}{243 M_{\eta}^6 M_{\eta'}^2 (M_{\eta}^2 - M_{\eta'}^2)} - \frac{22 c_{\theta}^8 M_0^8 M_{\pi}^4 S_{\theta}^4 g_1 [M_{\eta}, T]}{243 M_{\eta}^6 M_{\eta'}^2 (M_{\eta}^2 - M_{\eta'}^2)} - \frac{512 \sqrt{2} c_{\theta}^7 M_0^8 M_K^4 S_{\theta}^5 g_1 [M_{\eta}, T]}{729 M_{\eta}^{10}} + \\
& \frac{544 \sqrt{2} c_{\theta}^7 M_0^8 M_K^2 M_{\pi}^2 S_{\theta}^5 g_1 [M_{\eta}, T]}{729 M_{\eta}^{10}} - \frac{140 \sqrt{2} c_{\theta}^7 M_0^8 M_{\pi}^4 S_{\theta}^5 g_1 [M_{\eta}, T]}{729 M_{\eta}^{10}} + \\
& \frac{8 \sqrt{2} c_{\theta}^5 M_0^8 M_K^2 S_{\theta}^5 g_1 [M_{\eta}, T]}{81 M_{\eta}^8} - \frac{17 c_{\theta}^5 M_0^8 M_{\pi}^2 S_{\theta}^5 g_1 [M_{\eta}, T]}{162 \sqrt{2} M_{\eta}^8} - \frac{256 \sqrt{2} c_{\theta}^7 M_0^8 M_K^4 S_{\theta}^5 g_1 [M_{\eta}, T]}{729 M_{\eta'}^{10}} + \\
& \frac{140 \sqrt{2} c_{\theta}^7 M_0^8 M_K^2 M_{\pi}^2 S_{\theta}^5 g_1 [M_{\eta}, T]}{729 M_{\eta'}^{10}} - \frac{19 \sqrt{2} c_{\theta}^7 M_0^8 M_{\pi}^4 S_{\theta}^5 g_1 [M_{\eta}, T]}{729 M_{\eta'}^{10}} + \\
& \frac{c_{\theta}^5 M_0^8 M_{\pi}^2 S_{\theta}^5 g_1 [M_{\eta}, T]}{162 \sqrt{2} M_{\eta'}^8} + \frac{320 \sqrt{2} c_{\theta}^7 M_0^8 M_K^4 S_{\theta}^5 g_1 [M_{\eta}, T]}{243 M_{\eta}^2 M_{\eta'}^8} - \frac{88 \sqrt{2} c_{\theta}^7 M_0^8 M_K^2 M_{\pi}^2 S_{\theta}^5 g_1 [M_{\eta}, T]}{243 M_{\eta}^2 M_{\eta'}^8} - \\
& \frac{16 \sqrt{2} c_{\theta}^7 M_0^8 M_{\pi}^4 S_{\theta}^5 g_1 [M_{\eta}, T]}{243 M_{\eta}^2 M_{\eta'}^8} - \frac{1760 \sqrt{2} c_{\theta}^7 M_0^8 M_K^4 S_{\theta}^5 g_1 [M_{\eta}, T]}{729 M_{\eta}^4 M_{\eta'}^6} + \\
& \frac{592 \sqrt{2} c_{\theta}^7 M_0^8 M_K^2 M_{\pi}^2 S_{\theta}^5 g_1 [M_{\eta}, T]}{729 M_{\eta}^4 M_{\eta'}^6} + \frac{34 \sqrt{2} c_{\theta}^7 M_0^8 M_{\pi}^4 S_{\theta}^5 g_1 [M_{\eta}, T]}{729 M_{\eta}^4 M_{\eta'}^6} + \\
& \frac{4 \sqrt{2} c_{\theta}^5 M_0^8 M_K^2 S_{\theta}^5 g_1 [M_{\eta}, T]}{81 M_{\eta}^2 M_{\eta'}^6} - \frac{5 c_{\theta}^5 M_0^8 M_{\pi}^2 S_{\theta}^5 g_1 [M_{\eta}, T]}{81 \sqrt{2} M_{\eta}^2 M_{\eta'}^6} + \frac{2048 \sqrt{2} c_{\theta}^7 M_0^8 M_K^4 S_{\theta}^5 g_1 [M_{\eta}, T]}{729 M_{\eta}^6 M_{\eta'}^4} - \\
& \frac{1228 \sqrt{2} c_{\theta}^7 M_0^8 M_K^2 M_{\pi}^2 S_{\theta}^5 g_1 [M_{\eta}, T]}{729 M_{\eta}^6 M_{\eta'}^4} + \frac{206 \sqrt{2} c_{\theta}^7 M_0^8 M_{\pi}^4 S_{\theta}^5 g_1 [M_{\eta}, T]}{729 M_{\eta}^6 M_{\eta'}^4} - \\
& \frac{8 \sqrt{2} c_{\theta}^5 M_0^8 M_K^2 S_{\theta}^5 g_1 [M_{\eta}, T]}{81 M_{\eta}^4 M_{\eta'}^4} + \frac{5 \sqrt{2} c_{\theta}^5 M_0^8 M_{\pi}^2 S_{\theta}^5 g_1 [M_{\eta}, T]}{81 M_{\eta}^4 M_{\eta'}^4} - \frac{320 \sqrt{2} c_{\theta}^7 M_0^8 M_K^4 S_{\theta}^5 g_1 [M_{\eta}, T]}{243 M_{\eta}^8 M_{\eta'}^2} + \\
& \frac{232 \sqrt{2} c_{\theta}^7 M_0^8 M_K^2 M_{\pi}^2 S_{\theta}^5 g_1 [M_{\eta}, T]}{243 M_{\eta}^8 M_{\eta'}^2} - \frac{11 \sqrt{2} c_{\theta}^7 M_0^8 M_{\pi}^4 S_{\theta}^5 g_1 [M_{\eta}, T]}{243 M_{\eta}^8 M_{\eta'}^2} - \frac{5 c_{\theta}^5 M_0^8 M_{\pi}^2 S_{\theta}^5 g_1 [M_{\eta}, T]}{81 \sqrt{2} M_{\eta}^6 M_{\eta'}^2} +
\end{aligned}$$

$$\begin{aligned}
& \frac{32 \sqrt{2} c_{\theta}^7 M_0^8 M_K^4 s_{\theta}^5 g_1 [M_{\eta}, T]}{243 M_{\eta}^8 (M_{\eta}^2 - M_{\eta'}^2)} - \frac{16 \sqrt{2} c_{\theta}^7 M_0^8 M_K^2 M_{\pi}^2 s_{\theta}^5 g_1 [M_{\eta}, T]}{243 M_{\eta}^8 (M_{\eta}^2 - M_{\eta'}^2)} - \frac{5 c_{\theta}^7 M_0^8 M_{\pi}^4 s_{\theta}^5 g_1 [M_{\eta}, T]}{243 \sqrt{2} M_{\eta}^8 (M_{\eta}^2 - M_{\eta'}^2)} + \\
& \frac{128 \sqrt{2} c_{\theta}^7 M_0^8 M_K^4 s_{\theta}^5 g_1 [M_{\eta}, T]}{243 M_{\eta'}^8 (M_{\eta}^2 - M_{\eta'}^2)} - \frac{88 \sqrt{2} c_{\theta}^7 M_0^8 M_K^2 M_{\pi}^2 s_{\theta}^5 g_1 [M_{\eta}, T]}{243 M_{\eta'}^8 (M_{\eta}^2 - M_{\eta'}^2)} + \frac{37 c_{\theta}^7 M_0^8 M_{\pi}^4 s_{\theta}^5 g_1 [M_{\eta}, T]}{243 \sqrt{2} M_{\eta'}^8 (M_{\eta}^2 - M_{\eta'}^2)} - \\
& \frac{400 \sqrt{2} c_{\theta}^7 M_0^8 M_K^4 s_{\theta}^5 g_1 [M_{\eta}, T]}{243 M_{\eta}^2 M_{\eta'}^6 (M_{\eta}^2 - M_{\eta'}^2)} + \frac{200 \sqrt{2} c_{\theta}^7 M_0^8 M_K^2 M_{\pi}^2 s_{\theta}^5 g_1 [M_{\eta}, T]}{243 M_{\eta}^2 M_{\eta'}^6 (M_{\eta}^2 - M_{\eta'}^2)} - \\
& \frac{25 \sqrt{2} c_{\theta}^7 M_0^8 M_{\pi}^4 s_{\theta}^5 g_1 [M_{\eta}, T]}{243 M_{\eta}^2 M_{\eta'}^6 (M_{\eta}^2 - M_{\eta'}^2)} + \frac{160 \sqrt{2} c_{\theta}^7 M_0^8 M_K^4 s_{\theta}^5 g_1 [M_{\eta}, T]}{81 M_{\eta}^4 M_{\eta'}^4 (M_{\eta}^2 - M_{\eta'}^2)} - \\
& \frac{68 \sqrt{2} c_{\theta}^7 M_0^8 M_K^2 M_{\pi}^2 s_{\theta}^5 g_1 [M_{\eta}, T]}{81 M_{\eta}^4 M_{\eta'}^4 (M_{\eta}^2 - M_{\eta'}^2)} + \frac{4 \sqrt{2} c_{\theta}^7 M_0^8 M_{\pi}^4 s_{\theta}^5 g_1 [M_{\eta}, T]}{81 M_{\eta}^4 M_{\eta'}^4 (M_{\eta}^2 - M_{\eta'}^2)} - \\
& \frac{256 \sqrt{2} c_{\theta}^7 M_0^8 M_K^4 s_{\theta}^5 g_1 [M_{\eta}, T]}{243 M_{\eta}^6 M_{\eta'}^2 (M_{\eta}^2 - M_{\eta'}^2)} + \frac{140 \sqrt{2} c_{\theta}^7 M_0^8 M_K^2 M_{\pi}^2 s_{\theta}^5 g_1 [M_{\eta}, T]}{243 M_{\eta}^6 M_{\eta'}^2 (M_{\eta}^2 - M_{\eta'}^2)} - \\
& \frac{19 \sqrt{2} c_{\theta}^7 M_0^8 M_{\pi}^4 s_{\theta}^5 g_1 [M_{\eta}, T]}{243 M_{\eta}^6 M_{\eta'}^2 (M_{\eta}^2 - M_{\eta'}^2)} - \frac{1792 c_{\theta}^6 M_0^8 M_K^4 s_{\theta}^6 g_1 [M_{\eta}, T]}{729 M_{\eta}^{10}} + \frac{1808 c_{\theta}^6 M_0^8 M_K^2 M_{\pi}^2 s_{\theta}^6 g_1 [M_{\eta}, T]}{729 M_{\eta}^{10}} - \\
& \frac{484 c_{\theta}^6 M_0^8 M_{\pi}^4 s_{\theta}^6 g_1 [M_{\eta}, T]}{729 M_{\eta}^{10}} + \frac{20 c_{\theta}^4 M_0^8 M_K^2 s_{\theta}^6 g_1 [M_{\eta}, T]}{81 M_{\eta}^8} - \frac{35 c_{\theta}^4 M_0^8 M_{\pi}^2 s_{\theta}^6 g_1 [M_{\eta}, T]}{324 M_{\eta}^8} + \\
& \frac{160 c_{\theta}^6 M_0^8 M_K^4 s_{\theta}^6 g_1 [M_{\eta}, T]}{729 M_{\eta'}^{10}} - \frac{194 c_{\theta}^6 M_0^8 M_K^2 M_{\pi}^2 s_{\theta}^6 g_1 [M_{\eta}, T]}{729 M_{\eta'}^{10}} + \frac{77 c_{\theta}^6 M_0^8 M_{\pi}^4 s_{\theta}^6 g_1 [M_{\eta}, T]}{1458 M_{\eta'}^{10}} + \\
& \frac{4 c_{\theta}^4 M_0^8 M_K^2 s_{\theta}^6 g_1 [M_{\eta}, T]}{243 M_{\eta'}^8} - \frac{7 c_{\theta}^4 M_0^8 M_{\pi}^2 s_{\theta}^6 g_1 [M_{\eta}, T]}{972 M_{\eta'}^8} - \frac{32 c_{\theta}^6 M_0^8 M_K^4 s_{\theta}^6 g_1 [M_{\eta}, T]}{243 M_{\eta}^2 M_{\eta'}^8} + \\
& \frac{104 c_{\theta}^6 M_0^8 M_K^2 M_{\pi}^2 s_{\theta}^6 g_1 [M_{\eta}, T]}{243 M_{\eta}^2 M_{\eta'}^8} - \frac{4 c_{\theta}^6 M_0^8 M_{\pi}^4 s_{\theta}^6 g_1 [M_{\eta}, T]}{27 M_{\eta}^2 M_{\eta'}^8} - \frac{400 c_{\theta}^6 M_0^8 M_K^4 s_{\theta}^6 g_1 [M_{\eta}, T]}{729 M_{\eta}^4 M_{\eta'}^6} + \\
& \frac{86 c_{\theta}^6 M_0^8 M_K^2 M_{\pi}^2 s_{\theta}^6 g_1 [M_{\eta}, T]}{729 M_{\eta}^4 M_{\eta'}^6} + \frac{62 c_{\theta}^6 M_0^8 M_{\pi}^4 s_{\theta}^6 g_1 [M_{\eta}, T]}{729 M_{\eta}^4 M_{\eta'}^6} - \frac{8 c_{\theta}^4 M_0^8 M_K^2 s_{\theta}^6 g_1 [M_{\eta}, T]}{81 M_{\eta}^2 M_{\eta'}^6} + \\
& \frac{5 c_{\theta}^4 M_0^8 M_{\pi}^2 s_{\theta}^6 g_1 [M_{\eta}, T]}{81 M_{\eta}^2 M_{\eta'}^6} + \frac{352 c_{\theta}^6 M_0^8 M_K^4 s_{\theta}^6 g_1 [M_{\eta}, T]}{729 M_{\eta}^6 M_{\eta'}^4} - \frac{164 c_{\theta}^6 M_0^8 M_K^2 M_{\pi}^2 s_{\theta}^6 g_1 [M_{\eta}, T]}{729 M_{\eta}^6 M_{\eta'}^4} + \\
& \frac{46 c_{\theta}^6 M_0^8 M_{\pi}^4 s_{\theta}^6 g_1 [M_{\eta}, T]}{729 M_{\eta}^6 M_{\eta'}^4} + \frac{2 c_{\theta}^4 M_0^8 M_K^2 s_{\theta}^6 g_1 [M_{\eta}, T]}{9 M_{\eta}^4 M_{\eta'}^4} - \frac{4 c_{\theta}^4 M_0^8 M_{\pi}^2 s_{\theta}^6 g_1 [M_{\eta}, T]}{27 M_{\eta}^4 M_{\eta'}^4} + \\
& \frac{352 c_{\theta}^6 M_0^8 M_K^4 s_{\theta}^6 g_1 [M_{\eta}, T]}{243 M_{\eta}^8 M_{\eta'}^2} - \frac{376 c_{\theta}^6 M_0^8 M_K^2 M_{\pi}^2 s_{\theta}^6 g_1 [M_{\eta}, T]}{243 M_{\eta}^8 M_{\eta'}^2} + \frac{19 c_{\theta}^6 M_0^8 M_{\pi}^4 s_{\theta}^6 g_1 [M_{\eta}, T]}{162 M_{\eta}^8 M_{\eta'}^2} - \\
& \frac{80 c_{\theta}^4 M_0^8 M_K^2 s_{\theta}^6 g_1 [M_{\eta}, T]}{243 M_{\eta}^6 M_{\eta'}^2} + \frac{50 c_{\theta}^4 M_0^8 M_{\pi}^2 s_{\theta}^6 g_1 [M_{\eta}, T]}{243 M_{\eta}^6 M_{\eta'}^2} - \frac{80 c_{\theta}^6 M_0^8 M_K^4 s_{\theta}^6 g_1 [M_{\eta}, T]}{243 M_{\eta}^8 (M_{\eta}^2 - M_{\eta'}^2)} +
\end{aligned}$$

$$\begin{aligned}
& \frac{88 c_{\theta}^6 M_0^8 M_K^2 M_{\pi}^2 s_{\theta}^6 g_1 [M_{\eta}, T]}{243 M_{\eta}^8 (M_{\eta}^2 - M_{\eta'}^2)} - \frac{59 c_{\theta}^6 M_0^8 M_{\pi}^4 s_{\theta}^6 g_1 [M_{\eta}, T]}{972 M_{\eta}^8 (M_{\eta}^2 - M_{\eta'}^2)} - \frac{80 c_{\theta}^6 M_0^8 M_K^4 s_{\theta}^6 g_1 [M_{\eta}, T]}{243 M_{\eta'}^8 (M_{\eta}^2 - M_{\eta'}^2)} + \\
& \frac{88 c_{\theta}^6 M_0^8 M_K^2 M_{\pi}^2 s_{\theta}^6 g_1 [M_{\eta}, T]}{243 M_{\eta'}^8 (M_{\eta}^2 - M_{\eta'}^2)} - \frac{59 c_{\theta}^6 M_0^8 M_{\pi}^4 s_{\theta}^6 g_1 [M_{\eta}, T]}{972 M_{\eta'}^8 (M_{\eta}^2 - M_{\eta'}^2)} + \frac{64 c_{\theta}^6 M_0^8 M_K^4 s_{\theta}^6 g_1 [M_{\eta}, T]}{243 M_{\eta}^2 M_{\eta'}^6 (M_{\eta}^2 - M_{\eta'}^2)} - \\
& \frac{92 c_{\theta}^6 M_0^8 M_K^2 M_{\pi}^2 s_{\theta}^6 g_1 [M_{\eta}, T]}{243 M_{\eta}^2 M_{\eta'}^6 (M_{\eta}^2 - M_{\eta'}^2)} + \frac{19 c_{\theta}^6 M_0^8 M_{\pi}^4 s_{\theta}^6 g_1 [M_{\eta}, T]}{243 M_{\eta}^2 M_{\eta'}^6 (M_{\eta}^2 - M_{\eta'}^2)} + \frac{8 c_{\theta}^6 M_0^8 M_K^4 s_{\theta}^6 g_1 [M_{\eta}, T]}{81 M_{\eta}^4 M_{\eta'}^4 (M_{\eta}^2 - M_{\eta'}^2)} + \\
& \frac{8 c_{\theta}^6 M_0^8 M_K^2 M_{\pi}^2 s_{\theta}^6 g_1 [M_{\eta}, T]}{81 M_{\eta}^4 M_{\eta'}^4 (M_{\eta}^2 - M_{\eta'}^2)} - \frac{11 c_{\theta}^6 M_0^8 M_{\pi}^4 s_{\theta}^6 g_1 [M_{\eta}, T]}{162 M_{\eta}^4 M_{\eta'}^4 (M_{\eta}^2 - M_{\eta'}^2)} + \frac{64 c_{\theta}^6 M_0^8 M_K^4 s_{\theta}^6 g_1 [M_{\eta}, T]}{243 M_{\eta}^6 M_{\eta'}^2 (M_{\eta}^2 - M_{\eta'}^2)} - \\
& \frac{92 c_{\theta}^6 M_0^8 M_K^2 M_{\pi}^2 s_{\theta}^6 g_1 [M_{\eta}, T]}{243 M_{\eta}^6 M_{\eta'}^2 (M_{\eta}^2 - M_{\eta'}^2)} + \frac{19 c_{\theta}^6 M_0^8 M_{\pi}^4 s_{\theta}^6 g_1 [M_{\eta}, T]}{243 M_{\eta}^6 M_{\eta'}^2 (M_{\eta}^2 - M_{\eta'}^2)} - \frac{1792 \sqrt{2} c_{\theta}^5 M_0^8 M_K^4 s_{\theta}^7 g_1 [M_{\eta}, T]}{729 M_{\eta}^{10}} + \\
& \frac{1712 \sqrt{2} c_{\theta}^5 M_0^8 M_K^2 M_{\pi}^2 s_{\theta}^7 g_1 [M_{\eta}, T]}{729 M_{\eta}^{10}} - \frac{352 \sqrt{2} c_{\theta}^5 M_0^8 M_{\pi}^4 s_{\theta}^7 g_1 [M_{\eta}, T]}{729 M_{\eta}^{10}} + \\
& \frac{40 \sqrt{2} c_{\theta}^3 M_0^8 M_K^2 s_{\theta}^7 g_1 [M_{\eta}, T]}{243 M_{\eta}^8} - \frac{25 \sqrt{2} c_{\theta}^3 M_0^8 M_{\pi}^2 s_{\theta}^7 g_1 [M_{\eta}, T]}{243 M_{\eta}^8} + \frac{64 \sqrt{2} c_{\theta}^5 M_0^8 M_K^4 s_{\theta}^7 g_1 [M_{\eta}, T]}{729 M_{\eta'}^{10}} - \\
& \frac{68 \sqrt{2} c_{\theta}^5 M_0^8 M_K^2 M_{\pi}^2 s_{\theta}^7 g_1 [M_{\eta}, T]}{729 M_{\eta'}^{10}} + \frac{13 \sqrt{2} c_{\theta}^5 M_0^8 M_{\pi}^4 s_{\theta}^7 g_1 [M_{\eta}, T]}{729 M_{\eta'}^{10}} - \\
& \frac{64 \sqrt{2} c_{\theta}^5 M_0^8 M_K^4 s_{\theta}^7 g_1 [M_{\eta}, T]}{81 M_{\eta}^2 M_{\eta'}^8} + \frac{140 \sqrt{2} c_{\theta}^5 M_0^8 M_K^2 M_{\pi}^2 s_{\theta}^7 g_1 [M_{\eta}, T]}{243 M_{\eta}^2 M_{\eta'}^8} - \\
& \frac{32 \sqrt{2} c_{\theta}^5 M_0^8 M_{\pi}^4 s_{\theta}^7 g_1 [M_{\eta}, T]}{243 M_{\eta}^2 M_{\eta'}^8} + \frac{1376 \sqrt{2} c_{\theta}^5 M_0^8 M_K^4 s_{\theta}^7 g_1 [M_{\eta}, T]}{729 M_{\eta}^4 M_{\eta'}^6} - \\
& \frac{628 \sqrt{2} c_{\theta}^5 M_0^8 M_K^2 M_{\pi}^2 s_{\theta}^7 g_1 [M_{\eta}, T]}{729 M_{\eta}^4 M_{\eta'}^6} + \frac{62 \sqrt{2} c_{\theta}^5 M_0^8 M_{\pi}^4 s_{\theta}^7 g_1 [M_{\eta}, T]}{729 M_{\eta}^4 M_{\eta'}^6} - \\
& \frac{8 \sqrt{2} c_{\theta}^3 M_0^8 M_K^2 s_{\theta}^7 g_1 [M_{\eta}, T]}{243 M_{\eta}^2 M_{\eta'}^6} + \frac{5 \sqrt{2} c_{\theta}^3 M_0^8 M_{\pi}^2 s_{\theta}^7 g_1 [M_{\eta}, T]}{243 M_{\eta}^2 M_{\eta'}^6} - \frac{2048 \sqrt{2} c_{\theta}^5 M_0^8 M_K^4 s_{\theta}^7 g_1 [M_{\eta}, T]}{729 M_{\eta}^6 M_{\eta'}^4} + \\
& \frac{1060 \sqrt{2} c_{\theta}^5 M_0^8 M_K^2 M_{\pi}^2 s_{\theta}^7 g_1 [M_{\eta}, T]}{729 M_{\eta}^6 M_{\eta'}^4} - \frac{164 \sqrt{2} c_{\theta}^5 M_0^8 M_{\pi}^4 s_{\theta}^7 g_1 [M_{\eta}, T]}{729 M_{\eta}^6 M_{\eta'}^4} + \\
& \frac{4 \sqrt{2} c_{\theta}^3 M_0^8 M_K^2 s_{\theta}^7 g_1 [M_{\eta}, T]}{27 M_{\eta}^4 M_{\eta'}^4} - \frac{2 \sqrt{2} c_{\theta}^3 M_0^8 M_{\pi}^2 s_{\theta}^7 g_1 [M_{\eta}, T]}{27 M_{\eta}^4 M_{\eta'}^4} + \frac{832 \sqrt{2} c_{\theta}^5 M_0^8 M_K^4 s_{\theta}^7 g_1 [M_{\eta}, T]}{243 M_{\eta}^8 M_{\eta'}^2} - \\
& \frac{224 \sqrt{2} c_{\theta}^5 M_0^8 M_K^2 M_{\pi}^2 s_{\theta}^7 g_1 [M_{\eta}, T]}{81 M_{\eta}^8 M_{\eta'}^2} + \frac{179 \sqrt{2} c_{\theta}^5 M_0^8 M_{\pi}^4 s_{\theta}^7 g_1 [M_{\eta}, T]}{243 M_{\eta}^8 M_{\eta'}^2} - \\
& \frac{20 \sqrt{2} c_{\theta}^3 M_0^8 M_K^2 s_{\theta}^7 g_1 [M_{\eta}, T]}{81 M_{\eta}^6 M_{\eta'}^2} + \frac{10 \sqrt{2} c_{\theta}^3 M_0^8 M_{\pi}^2 s_{\theta}^7 g_1 [M_{\eta}, T]}{81 M_{\eta}^6 M_{\eta'}^2} - \frac{128 \sqrt{2} c_{\theta}^5 M_0^8 M_K^4 s_{\theta}^7 g_1 [M_{\eta}, T]}{243 M_{\eta}^8 (M_{\eta}^2 - M_{\eta'}^2)} +
\end{aligned}$$

$$\begin{aligned}
& \frac{88 \sqrt{2} c_{\theta}^5 M_0^8 M_K^2 M_{\pi}^2 s_{\theta}^7 g_1 [M_{\eta}, T]}{243 M_{\eta}^8 (M_{\eta}^2 - M_{\eta'}^2)} - \frac{37 c_{\theta}^5 M_0^8 M_{\pi}^4 s_{\theta}^7 g_1 [M_{\eta}, T]}{243 \sqrt{2} M_{\eta}^8 (M_{\eta}^2 - M_{\eta'}^2)} - \frac{32 \sqrt{2} c_{\theta}^5 M_0^8 M_K^4 s_{\theta}^7 g_1 [M_{\eta}, T]}{243 M_{\eta'}^8 (M_{\eta}^2 - M_{\eta'}^2)} + \\
& \frac{16 \sqrt{2} c_{\theta}^5 M_0^8 M_K^2 M_{\pi}^2 s_{\theta}^7 g_1 [M_{\eta}, T]}{243 M_{\eta'}^8 (M_{\eta}^2 - M_{\eta'}^2)} + \frac{5 c_{\theta}^5 M_0^8 M_{\pi}^4 s_{\theta}^7 g_1 [M_{\eta}, T]}{243 \sqrt{2} M_{\eta'}^8 (M_{\eta}^2 - M_{\eta'}^2)} + \frac{256 \sqrt{2} c_{\theta}^5 M_0^8 M_K^4 s_{\theta}^7 g_1 [M_{\eta}, T]}{243 M_{\eta}^2 M_{\eta'}^6 (M_{\eta}^2 - M_{\eta'}^2)} - \\
& \frac{140 \sqrt{2} c_{\theta}^5 M_0^8 M_K^2 M_{\pi}^2 s_{\theta}^7 g_1 [M_{\eta}, T]}{243 M_{\eta}^2 M_{\eta'}^6 (M_{\eta}^2 - M_{\eta'}^2)} + \frac{19 \sqrt{2} c_{\theta}^5 M_0^8 M_{\pi}^4 s_{\theta}^7 g_1 [M_{\eta}, T]}{243 M_{\eta}^2 M_{\eta'}^6 (M_{\eta}^2 - M_{\eta'}^2)} - \\
& \frac{160 \sqrt{2} c_{\theta}^5 M_0^8 M_K^4 s_{\theta}^7 g_1 [M_{\eta}, T]}{81 M_{\eta}^4 M_{\eta'}^4 (M_{\eta}^2 - M_{\eta'}^2)} + \frac{68 \sqrt{2} c_{\theta}^5 M_0^8 M_K^2 M_{\pi}^2 s_{\theta}^7 g_1 [M_{\eta}, T]}{81 M_{\eta}^4 M_{\eta'}^4 (M_{\eta}^2 - M_{\eta'}^2)} - \\
& \frac{4 \sqrt{2} c_{\theta}^5 M_0^8 M_{\pi}^4 s_{\theta}^7 g_1 [M_{\eta}, T]}{81 M_{\eta}^4 M_{\eta'}^4 (M_{\eta}^2 - M_{\eta'}^2)} + \frac{400 \sqrt{2} c_{\theta}^5 M_0^8 M_K^4 s_{\theta}^7 g_1 [M_{\eta}, T]}{243 M_{\eta}^6 M_{\eta'}^2 (M_{\eta}^2 - M_{\eta'}^2)} - \\
& \frac{200 \sqrt{2} c_{\theta}^5 M_0^8 M_K^2 M_{\pi}^2 s_{\theta}^7 g_1 [M_{\eta}, T]}{243 M_{\eta}^6 M_{\eta'}^2 (M_{\eta}^2 - M_{\eta'}^2)} + \frac{25 \sqrt{2} c_{\theta}^5 M_0^8 M_{\pi}^4 s_{\theta}^7 g_1 [M_{\eta}, T]}{243 M_{\eta}^6 M_{\eta'}^2 (M_{\eta}^2 - M_{\eta'}^2)} - \\
& \frac{2240 c_{\theta}^4 M_0^8 M_K^4 s_{\theta}^8 g_1 [M_{\eta}, T]}{729 M_{\eta}^{10}} + \frac{2236 c_{\theta}^4 M_0^8 M_K^2 M_{\pi}^2 s_{\theta}^8 g_1 [M_{\eta}, T]}{729 M_{\eta}^{10}} - \frac{698 c_{\theta}^4 M_0^8 M_{\pi}^4 s_{\theta}^8 g_1 [M_{\eta}, T]}{729 M_{\eta}^{10}} + \\
& \frac{10 c_{\theta}^2 M_0^8 M_K^2 s_{\theta}^8 g_1 [M_{\eta}, T]}{81 M_{\eta}^8} - \frac{5 c_{\theta}^2 M_0^8 M_{\pi}^2 s_{\theta}^8 g_1 [M_{\eta}, T]}{162 M_{\eta}^8} - \frac{64 c_{\theta}^4 M_0^8 M_K^4 s_{\theta}^8 g_1 [M_{\eta}, T]}{729 M_{\eta}^{10}} + \\
& \frac{44 c_{\theta}^4 M_0^8 M_K^2 M_{\pi}^2 s_{\theta}^8 g_1 [M_{\eta}, T]}{729 M_{\eta}^{10}} - \frac{7 c_{\theta}^4 M_0^8 M_{\pi}^4 s_{\theta}^8 g_1 [M_{\eta}, T]}{729 M_{\eta}^{10}} + \frac{32 c_{\theta}^4 M_0^8 M_K^4 s_{\theta}^8 g_1 [M_{\eta}, T]}{243 M_{\eta}^2 M_{\eta'}^8} - \\
& \frac{10 c_{\theta}^4 M_0^8 M_K^2 M_{\pi}^2 s_{\theta}^8 g_1 [M_{\eta}, T]}{243 M_{\eta}^2 M_{\eta'}^8} - \frac{13 c_{\theta}^4 M_0^8 M_{\pi}^4 s_{\theta}^8 g_1 [M_{\eta}, T]}{243 M_{\eta}^2 M_{\eta'}^8} + \frac{640 c_{\theta}^4 M_0^8 M_K^4 s_{\theta}^8 g_1 [M_{\eta}, T]}{729 M_{\eta}^4 M_{\eta'}^6} - \\
& \frac{536 c_{\theta}^4 M_0^8 M_K^2 M_{\pi}^2 s_{\theta}^8 g_1 [M_{\eta}, T]}{729 M_{\eta}^4 M_{\eta'}^6} + \frac{112 c_{\theta}^4 M_0^8 M_{\pi}^4 s_{\theta}^8 g_1 [M_{\eta}, T]}{729 M_{\eta}^4 M_{\eta'}^6} - \frac{2128 c_{\theta}^4 M_0^8 M_K^4 s_{\theta}^8 g_1 [M_{\eta}, T]}{729 M_{\eta}^6 M_{\eta'}^4} + \\
& \frac{1922 c_{\theta}^4 M_0^8 M_K^2 M_{\pi}^2 s_{\theta}^8 g_1 [M_{\eta}, T]}{729 M_{\eta}^6 M_{\eta'}^4} - \frac{361 c_{\theta}^4 M_0^8 M_{\pi}^4 s_{\theta}^8 g_1 [M_{\eta}, T]}{729 M_{\eta}^6 M_{\eta'}^4} + \frac{4 c_{\theta}^2 M_0^8 M_K^2 s_{\theta}^8 g_1 [M_{\eta}, T]}{81 M_{\eta}^4 M_{\eta'}^4} - \\
& \frac{c_{\theta}^2 M_0^8 M_{\pi}^2 s_{\theta}^8 g_1 [M_{\eta}, T]}{81 M_{\eta}^4 M_{\eta'}^4} + \frac{1072 c_{\theta}^4 M_0^8 M_K^4 s_{\theta}^8 g_1 [M_{\eta}, T]}{243 M_{\eta}^8 M_{\eta'}^2} - \frac{1052 c_{\theta}^4 M_0^8 M_K^2 M_{\pi}^2 s_{\theta}^8 g_1 [M_{\eta}, T]}{243 M_{\eta}^8 M_{\eta'}^2} + \\
& \frac{241 c_{\theta}^4 M_0^8 M_{\pi}^4 s_{\theta}^8 g_1 [M_{\eta}, T]}{243 M_{\eta}^8 M_{\eta'}^2} - \frac{4 c_{\theta}^2 M_0^8 M_K^2 s_{\theta}^8 g_1 [M_{\eta}, T]}{27 M_{\eta}^6 M_{\eta'}^2} + \frac{4 c_{\theta}^2 M_0^8 M_{\pi}^2 s_{\theta}^8 g_1 [M_{\eta}, T]}{81 M_{\eta}^6 M_{\eta'}^2} - \\
& \frac{40 c_{\theta}^4 M_0^8 M_K^4 s_{\theta}^8 g_1 [M_{\eta}, T]}{243 M_{\eta}^8 (M_{\eta}^2 - M_{\eta'}^2)} + \frac{38 c_{\theta}^4 M_0^8 M_K^2 M_{\pi}^2 s_{\theta}^8 g_1 [M_{\eta}, T]}{243 M_{\eta}^8 (M_{\eta}^2 - M_{\eta'}^2)} - \frac{23 c_{\theta}^4 M_0^8 M_{\pi}^4 s_{\theta}^8 g_1 [M_{\eta}, T]}{486 M_{\eta}^8 (M_{\eta}^2 - M_{\eta'}^2)} + \\
& \frac{32 c_{\theta}^4 M_0^8 M_K^4 s_{\theta}^8 g_1 [M_{\eta}, T]}{243 M_{\eta'}^8 (M_{\eta}^2 - M_{\eta'}^2)} - \frac{40 c_{\theta}^4 M_0^8 M_K^2 M_{\pi}^2 s_{\theta}^8 g_1 [M_{\eta}, T]}{243 M_{\eta'}^8 (M_{\eta}^2 - M_{\eta'}^2)} + \frac{25 c_{\theta}^4 M_0^8 M_{\pi}^4 s_{\theta}^8 g_1 [M_{\eta}, T]}{486 M_{\eta'}^8 (M_{\eta}^2 - M_{\eta'}^2)} -
\end{aligned}$$

$$\begin{aligned}
& \frac{64 c_{\theta}^4 M_0^8 M_K^4 s_{\theta}^8 g_1 [M_{\eta}, T]}{243 M_{\eta}^2 M_{\eta'}^6 (M_{\eta}^2 - M_{\eta'}^2)} + \frac{104 c_{\theta}^4 M_0^8 M_K^2 M_{\pi}^2 s_{\theta}^8 g_1 [M_{\eta}, T]}{243 M_{\eta}^2 M_{\eta'}^6 (M_{\eta}^2 - M_{\eta'}^2)} - \frac{22 c_{\theta}^4 M_0^8 M_{\pi}^4 s_{\theta}^8 g_1 [M_{\eta}, T]}{243 M_{\eta}^2 M_{\eta'}^6 (M_{\eta}^2 - M_{\eta'}^2)} - \\
& \frac{32 c_{\theta}^4 M_0^8 M_K^4 s_{\theta}^8 g_1 [M_{\eta}, T]}{81 M_{\eta}^4 M_{\eta'}^4 (M_{\eta}^2 - M_{\eta'}^2)} + \frac{10 c_{\theta}^4 M_0^8 M_K^2 M_{\pi}^2 s_{\theta}^8 g_1 [M_{\eta}, T]}{81 M_{\eta}^4 M_{\eta'}^4 (M_{\eta}^2 - M_{\eta'}^2)} + \frac{c_{\theta}^4 M_0^8 M_{\pi}^4 s_{\theta}^8 g_1 [M_{\eta}, T]}{81 M_{\eta}^4 M_{\eta'}^4 (M_{\eta}^2 - M_{\eta'}^2)} + \\
& \frac{176 c_{\theta}^4 M_0^8 M_K^4 s_{\theta}^8 g_1 [M_{\eta}, T]}{243 M_{\eta}^6 M_{\eta'}^2 (M_{\eta}^2 - M_{\eta'}^2)} - \frac{148 c_{\theta}^4 M_0^8 M_K^2 M_{\pi}^2 s_{\theta}^8 g_1 [M_{\eta}, T]}{243 M_{\eta}^6 M_{\eta'}^2 (M_{\eta}^2 - M_{\eta'}^2)} + \frac{26 c_{\theta}^4 M_0^8 M_{\pi}^4 s_{\theta}^8 g_1 [M_{\eta}, T]}{243 M_{\eta}^6 M_{\eta'}^2 (M_{\eta}^2 - M_{\eta'}^2)} - \\
& \frac{896 \sqrt{2} c_{\theta}^3 M_0^8 M_K^4 s_{\theta}^9 g_1 [M_{\eta}, T]}{729 M_{\eta}^{10}} + \frac{976 \sqrt{2} c_{\theta}^3 M_0^8 M_K^2 M_{\pi}^2 s_{\theta}^9 g_1 [M_{\eta}, T]}{729 M_{\eta}^{10}} - \\
& \frac{152 \sqrt{2} c_{\theta}^3 M_0^8 M_{\pi}^4 s_{\theta}^9 g_1 [M_{\eta}, T]}{729 M_{\eta}^{10}} + \frac{2 \sqrt{2} c_{\theta}^3 M_0^8 M_K^2 s_{\theta}^9 g_1 [M_{\eta}, T]}{81 M_{\eta}^8} - \frac{2 \sqrt{2} c_{\theta}^3 M_0^8 M_{\pi}^2 s_{\theta}^9 g_1 [M_{\eta}, T]}{81 M_{\eta}^8} + \\
& \frac{128 \sqrt{2} c_{\theta}^3 M_0^8 M_K^4 s_{\theta}^9 g_1 [M_{\eta}, T]}{729 M_{\eta}^2 M_{\eta'}^8} - \frac{130 \sqrt{2} c_{\theta}^3 M_0^8 M_K^2 M_{\pi}^2 s_{\theta}^9 g_1 [M_{\eta}, T]}{729 M_{\eta}^2 M_{\eta'}^8} + \\
& \frac{29 \sqrt{2} c_{\theta}^3 M_0^8 M_{\pi}^4 s_{\theta}^9 g_1 [M_{\eta}, T]}{729 M_{\eta}^2 M_{\eta'}^8} - \frac{320 \sqrt{2} c_{\theta}^3 M_0^8 M_K^4 s_{\theta}^9 g_1 [M_{\eta}, T]}{729 M_{\eta}^4 M_{\eta'}^6} + \\
& \frac{238 \sqrt{2} c_{\theta}^3 M_0^8 M_K^2 M_{\pi}^2 s_{\theta}^9 g_1 [M_{\eta}, T]}{729 M_{\eta}^4 M_{\eta'}^6} - \frac{71 \sqrt{2} c_{\theta}^3 M_0^8 M_{\pi}^4 s_{\theta}^9 g_1 [M_{\eta}, T]}{729 M_{\eta}^4 M_{\eta'}^6} - \\
& \frac{64 \sqrt{2} c_{\theta}^3 M_0^8 M_K^4 s_{\theta}^9 g_1 [M_{\eta}, T]}{729 M_{\eta}^6 M_{\eta'}^4} + \frac{380 \sqrt{2} c_{\theta}^3 M_0^8 M_K^2 M_{\pi}^2 s_{\theta}^9 g_1 [M_{\eta}, T]}{729 M_{\eta}^6 M_{\eta'}^4} - \\
& \frac{118 \sqrt{2} c_{\theta}^3 M_0^8 M_{\pi}^4 s_{\theta}^9 g_1 [M_{\eta}, T]}{729 M_{\eta}^6 M_{\eta'}^4} + \frac{304 \sqrt{2} c_{\theta}^3 M_0^8 M_K^4 s_{\theta}^9 g_1 [M_{\eta}, T]}{243 M_{\eta}^8 M_{\eta'}^2} - \\
& \frac{136 \sqrt{2} c_{\theta}^3 M_0^8 M_K^2 M_{\pi}^2 s_{\theta}^9 g_1 [M_{\eta}, T]}{81 M_{\eta}^8 M_{\eta'}^2} + \frac{104 \sqrt{2} c_{\theta}^3 M_0^8 M_{\pi}^4 s_{\theta}^9 g_1 [M_{\eta}, T]}{243 M_{\eta}^8 M_{\eta'}^2} - \\
& \frac{4 \sqrt{2} c_{\theta}^3 M_0^8 M_K^2 s_{\theta}^9 g_1 [M_{\eta}, T]}{243 M_{\eta}^6 M_{\eta'}^2} + \frac{4 \sqrt{2} c_{\theta}^3 M_0^8 M_{\pi}^2 s_{\theta}^9 g_1 [M_{\eta}, T]}{243 M_{\eta}^6 M_{\eta'}^2} + \frac{104 \sqrt{2} c_{\theta}^3 M_0^8 M_K^4 s_{\theta}^9 g_1 [M_{\eta}, T]}{243 M_{\eta}^8 (M_{\eta}^2 - M_{\eta'}^2)} - \\
& \frac{64 \sqrt{2} c_{\theta}^3 M_0^8 M_K^2 M_{\pi}^2 s_{\theta}^9 g_1 [M_{\eta}, T]}{243 M_{\eta}^8 (M_{\eta}^2 - M_{\eta'}^2)} + \frac{14 \sqrt{2} c_{\theta}^3 M_0^8 M_{\pi}^4 s_{\theta}^9 g_1 [M_{\eta}, T]}{243 M_{\eta}^8 (M_{\eta}^2 - M_{\eta'}^2)} - \\
& \frac{64 \sqrt{2} c_{\theta}^3 M_0^8 M_K^4 s_{\theta}^9 g_1 [M_{\eta}, T]}{243 M_{\eta}^2 M_{\eta'}^6 (M_{\eta}^2 - M_{\eta'}^2)} + \frac{56 \sqrt{2} c_{\theta}^3 M_0^8 M_K^2 M_{\pi}^2 s_{\theta}^9 g_1 [M_{\eta}, T]}{243 M_{\eta}^2 M_{\eta'}^6 (M_{\eta}^2 - M_{\eta'}^2)} - \\
& \frac{10 \sqrt{2} c_{\theta}^3 M_0^8 M_{\pi}^4 s_{\theta}^9 g_1 [M_{\eta}, T]}{243 M_{\eta}^2 M_{\eta'}^6 (M_{\eta}^2 - M_{\eta'}^2)} + \frac{64 \sqrt{2} c_{\theta}^3 M_0^8 M_K^4 s_{\theta}^9 g_1 [M_{\eta}, T]}{81 M_{\eta}^4 M_{\eta'}^4 (M_{\eta}^2 - M_{\eta'}^2)} - \\
& \frac{44 \sqrt{2} c_{\theta}^3 M_0^8 M_K^2 M_{\pi}^2 s_{\theta}^9 g_1 [M_{\eta}, T]}{81 M_{\eta}^4 M_{\eta'}^4 (M_{\eta}^2 - M_{\eta'}^2)} + \frac{10 \sqrt{2} c_{\theta}^3 M_0^8 M_{\pi}^4 s_{\theta}^9 g_1 [M_{\eta}, T]}{81 M_{\eta}^4 M_{\eta'}^4 (M_{\eta}^2 - M_{\eta'}^2)} -
\end{aligned}$$

$$\begin{aligned}
& \frac{208 \sqrt{2} c_{\theta}^3 M_0^8 M_K^4 s_{\theta}^9 g_1 [M_{\eta}, T]}{243 M_{\eta}^6 M_{\eta'}^2 (M_{\eta}^2 - M_{\eta'}^2)} + \frac{92 \sqrt{2} c_{\theta}^3 M_0^8 M_K^2 M_{\pi}^2 s_{\theta}^9 g_1 [M_{\eta}, T]}{243 M_{\eta}^6 M_{\eta'}^2 (M_{\eta}^2 - M_{\eta'}^2)} - \\
& \frac{10 \sqrt{2} c_{\theta}^3 M_0^8 M_{\pi}^4 s_{\theta}^9 g_1 [M_{\eta}, T]}{243 M_{\eta}^6 M_{\eta'}^2 (M_{\eta}^2 - M_{\eta'}^2)} - \frac{448 c_{\theta}^2 M_0^8 M_K^4 s_{\theta}^{10} g_1 [M_{\eta}, T]}{729 M_{\eta}^{10}} + \frac{464 c_{\theta}^2 M_0^8 M_K^2 M_{\pi}^2 s_{\theta}^{10} g_1 [M_{\eta}, T]}{729 M_{\eta}^{10}} - \\
& \frac{232 c_{\theta}^2 M_0^8 M_{\pi}^4 s_{\theta}^{10} g_1 [M_{\eta}, T]}{729 M_{\eta}^{10}} + \frac{M_0^8 M_K^2 s_{\theta}^{10} g_1 [M_{\eta}, T]}{243 M_{\eta}^8} + \frac{M_0^8 M_{\pi}^2 s_{\theta}^{10} g_1 [M_{\eta}, T]}{486 M_{\eta}^8} - \\
& \frac{64 c_{\theta}^2 M_0^8 M_K^4 s_{\theta}^{10} g_1 [M_{\eta}, T]}{243 M_{\eta}^4 M_{\eta'}^6} + \frac{68 c_{\theta}^2 M_0^8 M_K^2 M_{\pi}^2 s_{\theta}^{10} g_1 [M_{\eta}, T]}{243 M_{\eta}^4 M_{\eta'}^6} - \frac{22 c_{\theta}^2 M_0^8 M_{\pi}^4 s_{\theta}^{10} g_1 [M_{\eta}, T]}{243 M_{\eta}^4 M_{\eta'}^6} + \\
& \frac{352 c_{\theta}^2 M_0^8 M_K^4 s_{\theta}^{10} g_1 [M_{\eta}, T]}{729 M_{\eta}^6 M_{\eta'}^4} - \frac{284 c_{\theta}^2 M_0^8 M_K^2 M_{\pi}^2 s_{\theta}^{10} g_1 [M_{\eta}, T]}{729 M_{\eta}^6 M_{\eta'}^4} + \frac{22 c_{\theta}^2 M_0^8 M_{\pi}^4 s_{\theta}^{10} g_1 [M_{\eta}, T]}{729 M_{\eta}^6 M_{\eta'}^4} + \\
& \frac{40 c_{\theta}^2 M_0^8 M_K^4 s_{\theta}^{10} g_1 [M_{\eta}, T]}{243 M_{\eta}^8 M_{\eta'}^2} - \frac{8 c_{\theta}^2 M_0^8 M_K^2 M_{\pi}^2 s_{\theta}^{10} g_1 [M_{\eta}, T]}{27 M_{\eta}^8 M_{\eta'}^2} + \frac{56 c_{\theta}^2 M_0^8 M_{\pi}^4 s_{\theta}^{10} g_1 [M_{\eta}, T]}{243 M_{\eta}^8 M_{\eta'}^2} + \\
& \frac{148 c_{\theta}^2 M_0^8 M_K^4 s_{\theta}^{10} g_1 [M_{\eta}, T]}{243 M_{\eta}^8 (M_{\eta}^2 - M_{\eta'}^2)} - \frac{140 c_{\theta}^2 M_0^8 M_K^2 M_{\pi}^2 s_{\theta}^{10} g_1 [M_{\eta}, T]}{243 M_{\eta}^8 (M_{\eta}^2 - M_{\eta'}^2)} + \frac{28 c_{\theta}^2 M_0^8 M_{\pi}^4 s_{\theta}^{10} g_1 [M_{\eta}, T]}{243 M_{\eta}^8 (M_{\eta}^2 - M_{\eta'}^2)} + \\
& \frac{32 c_{\theta}^2 M_0^8 M_K^4 s_{\theta}^{10} g_1 [M_{\eta}, T]}{81 M_{\eta}^4 M_{\eta'}^4 (M_{\eta}^2 - M_{\eta'}^2)} - \frac{28 c_{\theta}^2 M_0^8 M_K^2 M_{\pi}^2 s_{\theta}^{10} g_1 [M_{\eta}, T]}{81 M_{\eta}^4 M_{\eta'}^4 (M_{\eta}^2 - M_{\eta'}^2)} + \frac{8 c_{\theta}^2 M_0^8 M_{\pi}^4 s_{\theta}^{10} g_1 [M_{\eta}, T]}{81 M_{\eta}^4 M_{\eta'}^4 (M_{\eta}^2 - M_{\eta'}^2)} - \\
& \frac{224 c_{\theta}^2 M_0^8 M_K^4 s_{\theta}^{10} g_1 [M_{\eta}, T]}{243 M_{\eta}^6 M_{\eta'}^2 (M_{\eta}^2 - M_{\eta'}^2)} + \frac{184 c_{\theta}^2 M_0^8 M_K^2 M_{\pi}^2 s_{\theta}^{10} g_1 [M_{\eta}, T]}{243 M_{\eta}^6 M_{\eta'}^2 (M_{\eta}^2 - M_{\eta'}^2)} - \frac{32 c_{\theta}^2 M_0^8 M_{\pi}^4 s_{\theta}^{10} g_1 [M_{\eta}, T]}{243 M_{\eta}^6 M_{\eta'}^2 (M_{\eta}^2 - M_{\eta'}^2)} - \\
& \frac{64 \sqrt{2} c_{\theta} M_0^8 M_K^4 s_{\theta}^{11} g_1 [M_{\eta}, T]}{729 M_{\eta}^{10}} + \frac{32 \sqrt{2} c_{\theta} M_0^8 M_K^2 M_{\pi}^2 s_{\theta}^{11} g_1 [M_{\eta}, T]}{729 M_{\eta}^{10}} + \\
& \frac{32 \sqrt{2} c_{\theta} M_0^8 M_{\pi}^4 s_{\theta}^{11} g_1 [M_{\eta}, T]}{729 M_{\eta}^{10}} + \frac{64 \sqrt{2} c_{\theta} M_0^8 M_K^4 s_{\theta}^{11} g_1 [M_{\eta}, T]}{729 M_{\eta}^6 M_{\eta'}^4} - \\
& \frac{80 \sqrt{2} c_{\theta} M_0^8 M_K^2 M_{\pi}^2 s_{\theta}^{11} g_1 [M_{\eta}, T]}{729 M_{\eta}^6 M_{\eta'}^4} + \frac{16 \sqrt{2} c_{\theta} M_0^8 M_{\pi}^4 s_{\theta}^{11} g_1 [M_{\eta}, T]}{729 M_{\eta}^6 M_{\eta'}^4} - \\
& \frac{16 \sqrt{2} c_{\theta} M_0^8 M_K^4 s_{\theta}^{11} g_1 [M_{\eta}, T]}{243 M_{\eta}^8 M_{\eta'}^2} + \frac{32 \sqrt{2} c_{\theta} M_0^8 M_K^2 M_{\pi}^2 s_{\theta}^{11} g_1 [M_{\eta}, T]}{243 M_{\eta}^8 M_{\eta'}^2} - \\
& \frac{16 \sqrt{2} c_{\theta} M_0^8 M_{\pi}^4 s_{\theta}^{11} g_1 [M_{\eta}, T]}{243 M_{\eta}^8 M_{\eta'}^2} + \frac{40 \sqrt{2} c_{\theta} M_0^8 M_K^4 s_{\theta}^{11} g_1 [M_{\eta}, T]}{243 M_{\eta}^8 (M_{\eta}^2 - M_{\eta'}^2)} - \\
& \frac{56 \sqrt{2} c_{\theta} M_0^8 M_K^2 M_{\pi}^2 s_{\theta}^{11} g_1 [M_{\eta}, T]}{243 M_{\eta}^8 (M_{\eta}^2 - M_{\eta'}^2)} + \frac{16 \sqrt{2} c_{\theta} M_0^8 M_{\pi}^4 s_{\theta}^{11} g_1 [M_{\eta}, T]}{243 M_{\eta}^8 (M_{\eta}^2 - M_{\eta'}^2)} - \\
& \frac{32 \sqrt{2} c_{\theta} M_0^8 M_K^4 s_{\theta}^{11} g_1 [M_{\eta}, T]}{243 M_{\eta}^6 M_{\eta'}^2 (M_{\eta}^2 - M_{\eta'}^2)} + \frac{40 \sqrt{2} c_{\theta} M_0^8 M_K^2 M_{\pi}^2 s_{\theta}^{11} g_1 [M_{\eta}, T]}{243 M_{\eta}^6 M_{\eta'}^2 (M_{\eta}^2 - M_{\eta'}^2)} -
\end{aligned}$$

$$\begin{aligned}
& \frac{8 \sqrt{2} c_{\theta} M_0^8 M_{\pi}^4 s_{\theta}^{11} g_1 [M_{\eta}, T]}{243 M_{\eta}^6 M_{\eta'}^2 (M_{\eta}^2 - M_{\eta'}^2)} - \frac{8 M_0^8 M_K^4 s_{\theta}^{12} g_1 [M_{\eta}, T]}{729 M_{\eta}^{10}} - \frac{8 M_0^8 M_K^2 M_{\pi}^2 s_{\theta}^{12} g_1 [M_{\eta}, T]}{729 M_{\eta}^{10}} - \\
& \frac{2 M_0^8 M_{\pi}^4 s_{\theta}^{12} g_1 [M_{\eta}, T]}{729 M_{\eta}^{10}} - \frac{16 M_0^8 M_K^4 s_{\theta}^{12} g_1 [M_{\eta}, T]}{729 M_{\eta}^8 M_{\eta'}^2} + \frac{32 M_0^8 M_K^2 M_{\pi}^2 s_{\theta}^{12} g_1 [M_{\eta}, T]}{729 M_{\eta}^8 M_{\eta'}^2} - \\
& \frac{16 M_0^8 M_{\pi}^4 s_{\theta}^{12} g_1 [M_{\eta}, T]}{729 M_{\eta}^8 M_{\eta'}^2} + \frac{8 M_0^8 M_K^4 s_{\theta}^{12} g_1 [M_{\eta}, T]}{243 M_{\eta}^8 (M_{\eta}^2 - M_{\eta'}^2)} - \frac{16 M_0^8 M_K^2 M_{\pi}^2 s_{\theta}^{12} g_1 [M_{\eta}, T]}{243 M_{\eta}^8 (M_{\eta}^2 - M_{\eta'}^2)} + \\
& \frac{8 M_0^8 M_{\pi}^4 s_{\theta}^{12} g_1 [M_{\eta}, T]}{243 M_{\eta}^8 (M_{\eta}^2 - M_{\eta'}^2)} - \frac{8 c_{\theta}^{12} M_0^8 M_K^4 g_1 [M_{\eta'}, T]}{729 M_{\eta'}^{10}} - \frac{8 c_{\theta}^{12} M_0^8 M_K^2 M_{\pi}^2 g_1 [M_{\eta'}, T]}{729 M_{\eta'}^{10}} - \\
& \frac{2 c_{\theta}^{12} M_0^8 M_{\pi}^4 g_1 [M_{\eta'}, T]}{729 M_{\eta'}^{10}} + \frac{c_{\theta}^{10} M_0^8 M_K^2 g_1 [M_{\eta'}, T]}{243 M_{\eta'}^8} + \frac{c_{\theta}^{10} M_0^8 M_{\pi}^2 g_1 [M_{\eta'}, T]}{486 M_{\eta'}^8} - \\
& \frac{16 c_{\theta}^{12} M_0^8 M_K^4 g_1 [M_{\eta'}, T]}{729 M_{\eta'}^2 M_{\eta'}^8} + \frac{32 c_{\theta}^{12} M_0^8 M_K^2 M_{\pi}^2 g_1 [M_{\eta'}, T]}{729 M_{\eta'}^2 M_{\eta'}^8} - \frac{16 c_{\theta}^{12} M_0^8 M_{\pi}^4 g_1 [M_{\eta'}, T]}{729 M_{\eta'}^2 M_{\eta'}^8} - \\
& \frac{8 c_{\theta}^{12} M_0^8 M_K^4 g_1 [M_{\eta'}, T]}{243 M_{\eta'}^8 (M_{\eta}^2 - M_{\eta'}^2)} + \frac{16 c_{\theta}^{12} M_0^8 M_K^2 M_{\pi}^2 g_1 [M_{\eta'}, T]}{243 M_{\eta'}^8 (M_{\eta}^2 - M_{\eta'}^2)} - \frac{8 c_{\theta}^{12} M_0^8 M_{\pi}^4 g_1 [M_{\eta'}, T]}{243 M_{\eta'}^8 (M_{\eta}^2 - M_{\eta'}^2)} + \\
& \frac{64 \sqrt{2} c_{\theta}^{11} M_0^8 M_K^4 s_{\theta} g_1 [M_{\eta'}, T]}{729 M_{\eta'}^{10}} - \frac{32 \sqrt{2} c_{\theta}^{11} M_0^8 M_K^2 M_{\pi}^2 s_{\theta} g_1 [M_{\eta'}, T]}{729 M_{\eta'}^{10}} - \\
& \frac{32 \sqrt{2} c_{\theta}^{11} M_0^8 M_{\pi}^4 s_{\theta} g_1 [M_{\eta'}, T]}{729 M_{\eta'}^{10}} - \frac{2 \sqrt{2} c_{\theta}^9 M_0^8 M_K^2 s_{\theta} g_1 [M_{\eta'}, T]}{81 M_{\eta'}^8} + \frac{2 \sqrt{2} c_{\theta}^9 M_0^8 M_{\pi}^2 s_{\theta} g_1 [M_{\eta'}, T]}{81 M_{\eta'}^8} + \\
& \frac{16 \sqrt{2} c_{\theta}^{11} M_0^8 M_K^4 s_{\theta} g_1 [M_{\eta'}, T]}{243 M_{\eta'}^2 M_{\eta'}^8} - \frac{32 \sqrt{2} c_{\theta}^{11} M_0^8 M_K^2 M_{\pi}^2 s_{\theta} g_1 [M_{\eta'}, T]}{243 M_{\eta'}^2 M_{\eta'}^8} + \\
& \frac{16 \sqrt{2} c_{\theta}^{11} M_0^8 M_{\pi}^4 s_{\theta} g_1 [M_{\eta'}, T]}{243 M_{\eta'}^2 M_{\eta'}^8} - \frac{64 \sqrt{2} c_{\theta}^{11} M_0^8 M_K^4 s_{\theta} g_1 [M_{\eta'}, T]}{729 M_{\eta'}^4 M_{\eta'}^6} + \\
& \frac{80 \sqrt{2} c_{\theta}^{11} M_0^8 M_K^2 M_{\pi}^2 s_{\theta} g_1 [M_{\eta'}, T]}{729 M_{\eta'}^4 M_{\eta'}^6} - \frac{16 \sqrt{2} c_{\theta}^{11} M_0^8 M_{\pi}^4 s_{\theta} g_1 [M_{\eta'}, T]}{729 M_{\eta'}^4 M_{\eta'}^6} + \\
& \frac{4 \sqrt{2} c_{\theta}^9 M_0^8 M_K^2 s_{\theta} g_1 [M_{\eta'}, T]}{243 M_{\eta'}^2 M_{\eta'}^6} - \frac{4 \sqrt{2} c_{\theta}^9 M_0^8 M_{\pi}^2 s_{\theta} g_1 [M_{\eta'}, T]}{243 M_{\eta'}^2 M_{\eta'}^6} + \frac{40 \sqrt{2} c_{\theta}^{11} M_0^8 M_K^4 s_{\theta} g_1 [M_{\eta'}, T]}{243 M_{\eta'}^8 (M_{\eta}^2 - M_{\eta'}^2)} - \\
& \frac{56 \sqrt{2} c_{\theta}^{11} M_0^8 M_K^2 M_{\pi}^2 s_{\theta} g_1 [M_{\eta'}, T]}{243 M_{\eta'}^8 (M_{\eta}^2 - M_{\eta'}^2)} + \frac{16 \sqrt{2} c_{\theta}^{11} M_0^8 M_{\pi}^4 s_{\theta} g_1 [M_{\eta'}, T]}{243 M_{\eta'}^8 (M_{\eta}^2 - M_{\eta'}^2)} - \\
& \frac{32 \sqrt{2} c_{\theta}^{11} M_0^8 M_K^4 s_{\theta} g_1 [M_{\eta'}, T]}{243 M_{\eta'}^2 M_{\eta'}^6 (M_{\eta}^2 - M_{\eta'}^2)} + \frac{40 \sqrt{2} c_{\theta}^{11} M_0^8 M_K^2 M_{\pi}^2 s_{\theta} g_1 [M_{\eta'}, T]}{243 M_{\eta'}^2 M_{\eta'}^6 (M_{\eta}^2 - M_{\eta'}^2)} - \\
& \frac{8 \sqrt{2} c_{\theta}^{11} M_0^8 M_{\pi}^4 s_{\theta} g_1 [M_{\eta'}, T]}{243 M_{\eta'}^2 M_{\eta'}^6 (M_{\eta}^2 - M_{\eta'}^2)} - \frac{448 c_{\theta}^{10} M_0^8 M_K^4 s_{\theta}^2 g_1 [M_{\eta'}, T]}{729 M_{\eta'}^{10}} +
\end{aligned}$$

$$\begin{aligned}
& \frac{464 c_{\theta}^{10} M_0^8 M_K^2 M_{\pi}^2 S_{\theta}^2 g_1 [M_{\eta'}, T]}{729 M_{\eta'}^{10}} - \frac{232 c_{\theta}^{10} M_0^8 M_{\pi}^4 S_{\theta}^2 g_1 [M_{\eta'}, T]}{729 M_{\eta'}^{10}} + \frac{10 c_{\theta}^8 M_0^8 M_K^2 S_{\theta}^2 g_1 [M_{\eta'}, T]}{81 M_{\eta'}^8} - \\
& \frac{5 c_{\theta}^8 M_0^8 M_{\pi}^2 S_{\theta}^2 g_1 [M_{\eta'}, T]}{162 M_{\eta'}^8} + \frac{40 c_{\theta}^{10} M_0^8 M_K^4 S_{\theta}^2 g_1 [M_{\eta'}, T]}{243 M_{\eta'}^2 M_{\eta'}^8} - \frac{8 c_{\theta}^{10} M_0^8 M_K^2 M_{\pi}^2 S_{\theta}^2 g_1 [M_{\eta'}, T]}{27 M_{\eta'}^2 M_{\eta'}^8} + \\
& \frac{56 c_{\theta}^{10} M_0^8 M_{\pi}^4 S_{\theta}^2 g_1 [M_{\eta'}, T]}{243 M_{\eta'}^2 M_{\eta'}^8} + \frac{352 c_{\theta}^{10} M_0^8 M_K^4 S_{\theta}^2 g_1 [M_{\eta'}, T]}{729 M_{\eta'}^4 M_{\eta'}^6} - \frac{284 c_{\theta}^{10} M_0^8 M_K^2 M_{\pi}^2 S_{\theta}^2 g_1 [M_{\eta'}, T]}{729 M_{\eta'}^4 M_{\eta'}^6} + \\
& \frac{22 c_{\theta}^{10} M_0^8 M_{\pi}^4 S_{\theta}^2 g_1 [M_{\eta'}, T]}{729 M_{\eta'}^4 M_{\eta'}^6} - \frac{4 c_{\theta}^8 M_0^8 M_K^2 S_{\theta}^2 g_1 [M_{\eta'}, T]}{27 M_{\eta'}^2 M_{\eta'}^6} + \frac{4 c_{\theta}^8 M_0^8 M_{\pi}^2 S_{\theta}^2 g_1 [M_{\eta'}, T]}{81 M_{\eta'}^2 M_{\eta'}^6} - \\
& \frac{64 c_{\theta}^{10} M_0^8 M_K^4 S_{\theta}^2 g_1 [M_{\eta'}, T]}{243 M_{\eta'}^6 M_{\eta'}^4} + \frac{68 c_{\theta}^{10} M_0^8 M_K^2 M_{\pi}^2 S_{\theta}^2 g_1 [M_{\eta'}, T]}{243 M_{\eta'}^6 M_{\eta'}^4} - \frac{22 c_{\theta}^{10} M_0^8 M_{\pi}^4 S_{\theta}^2 g_1 [M_{\eta'}, T]}{243 M_{\eta'}^6 M_{\eta'}^4} + \\
& \frac{4 c_{\theta}^8 M_0^8 M_K^2 S_{\theta}^2 g_1 [M_{\eta'}, T]}{81 M_{\eta'}^4 M_{\eta'}^4} - \frac{c_{\theta}^8 M_0^8 M_{\pi}^2 S_{\theta}^2 g_1 [M_{\eta'}, T]}{81 M_{\eta'}^4 M_{\eta'}^4} - \frac{148 c_{\theta}^{10} M_0^8 M_K^4 S_{\theta}^2 g_1 [M_{\eta'}, T]}{243 M_{\eta'}^8 (M_{\eta'}^2 - M_{\eta'}^2)} + \\
& \frac{140 c_{\theta}^{10} M_0^8 M_K^2 M_{\pi}^2 S_{\theta}^2 g_1 [M_{\eta'}, T]}{243 M_{\eta'}^8 (M_{\eta'}^2 - M_{\eta'}^2)} - \frac{28 c_{\theta}^{10} M_0^8 M_{\pi}^4 S_{\theta}^2 g_1 [M_{\eta'}, T]}{243 M_{\eta'}^8 (M_{\eta'}^2 - M_{\eta'}^2)} + \frac{224 c_{\theta}^{10} M_0^8 M_K^4 S_{\theta}^2 g_1 [M_{\eta'}, T]}{243 M_{\eta'}^2 M_{\eta'}^6 (M_{\eta'}^2 - M_{\eta'}^2)} - \\
& \frac{184 c_{\theta}^{10} M_0^8 M_K^2 M_{\pi}^2 S_{\theta}^2 g_1 [M_{\eta'}, T]}{243 M_{\eta'}^2 M_{\eta'}^6 (M_{\eta'}^2 - M_{\eta'}^2)} + \frac{32 c_{\theta}^{10} M_0^8 M_{\pi}^4 S_{\theta}^2 g_1 [M_{\eta'}, T]}{243 M_{\eta'}^2 M_{\eta'}^6 (M_{\eta'}^2 - M_{\eta'}^2)} - \frac{32 c_{\theta}^{10} M_0^8 M_K^4 S_{\theta}^2 g_1 [M_{\eta'}, T]}{81 M_{\eta'}^4 M_{\eta'}^4 (M_{\eta'}^2 - M_{\eta'}^2)} + \\
& \frac{28 c_{\theta}^{10} M_0^8 M_K^2 M_{\pi}^2 S_{\theta}^2 g_1 [M_{\eta'}, T]}{81 M_{\eta'}^4 M_{\eta'}^4 (M_{\eta'}^2 - M_{\eta'}^2)} - \frac{8 c_{\theta}^{10} M_0^8 M_{\pi}^4 S_{\theta}^2 g_1 [M_{\eta'}, T]}{81 M_{\eta'}^4 M_{\eta'}^4 (M_{\eta'}^2 - M_{\eta'}^2)} + \frac{896 \sqrt{2} c_{\theta}^9 M_0^8 M_K^4 S_{\theta}^3 g_1 [M_{\eta'}, T]}{729 M_{\eta'}^{10}} - \\
& \frac{976 \sqrt{2} c_{\theta}^9 M_0^8 M_K^2 M_{\pi}^2 S_{\theta}^3 g_1 [M_{\eta'}, T]}{729 M_{\eta'}^{10}} + \frac{152 \sqrt{2} c_{\theta}^9 M_0^8 M_{\pi}^4 S_{\theta}^3 g_1 [M_{\eta'}, T]}{729 M_{\eta'}^{10}} - \\
& \frac{40 \sqrt{2} c_{\theta}^7 M_0^8 M_K^2 S_{\theta}^3 g_1 [M_{\eta'}, T]}{243 M_{\eta'}^8} + \frac{25 \sqrt{2} c_{\theta}^7 M_0^8 M_{\pi}^2 S_{\theta}^3 g_1 [M_{\eta'}, T]}{243 M_{\eta'}^8} - \\
& \frac{304 \sqrt{2} c_{\theta}^9 M_0^8 M_K^4 S_{\theta}^3 g_1 [M_{\eta'}, T]}{243 M_{\eta'}^2 M_{\eta'}^8} + \frac{136 \sqrt{2} c_{\theta}^9 M_0^8 M_K^2 M_{\pi}^2 S_{\theta}^3 g_1 [M_{\eta'}, T]}{81 M_{\eta'}^2 M_{\eta'}^8} - \\
& \frac{104 \sqrt{2} c_{\theta}^9 M_0^8 M_{\pi}^4 S_{\theta}^3 g_1 [M_{\eta'}, T]}{243 M_{\eta'}^2 M_{\eta'}^8} + \frac{64 \sqrt{2} c_{\theta}^9 M_0^8 M_K^4 S_{\theta}^3 g_1 [M_{\eta'}, T]}{729 M_{\eta'}^4 M_{\eta'}^6} - \\
& \frac{380 \sqrt{2} c_{\theta}^9 M_0^8 M_K^2 M_{\pi}^2 S_{\theta}^3 g_1 [M_{\eta'}, T]}{729 M_{\eta'}^4 M_{\eta'}^6} + \frac{118 \sqrt{2} c_{\theta}^9 M_0^8 M_{\pi}^4 S_{\theta}^3 g_1 [M_{\eta'}, T]}{729 M_{\eta'}^4 M_{\eta'}^6} + \\
& \frac{20 \sqrt{2} c_{\theta}^7 M_0^8 M_K^2 S_{\theta}^3 g_1 [M_{\eta'}, T]}{81 M_{\eta'}^2 M_{\eta'}^6} - \frac{10 \sqrt{2} c_{\theta}^7 M_0^8 M_{\pi}^2 S_{\theta}^3 g_1 [M_{\eta'}, T]}{81 M_{\eta'}^2 M_{\eta'}^6} + \\
& \frac{320 \sqrt{2} c_{\theta}^9 M_0^8 M_K^4 S_{\theta}^3 g_1 [M_{\eta'}, T]}{729 M_{\eta'}^6 M_{\eta'}^4} - \frac{238 \sqrt{2} c_{\theta}^9 M_0^8 M_K^2 M_{\pi}^2 S_{\theta}^3 g_1 [M_{\eta'}, T]}{729 M_{\eta'}^6 M_{\eta'}^4} +
\end{aligned}$$



$$\begin{aligned}
& \frac{71 \sqrt{2} c_{\theta}^9 M_0^8 M_{\pi}^4 s_{\theta}^3 g_1 [M_{\eta'}, T]}{729 M_{\eta}^6 M_{\eta'}^4} - \frac{4 \sqrt{2} c_{\theta}^7 M_0^8 M_K^2 s_{\theta}^3 g_1 [M_{\eta'}, T]}{27 M_{\eta}^4 M_{\eta'}^4} + \frac{2 \sqrt{2} c_{\theta}^7 M_0^8 M_{\pi}^2 s_{\theta}^3 g_1 [M_{\eta'}, T]}{27 M_{\eta}^4 M_{\eta'}^4} - \\
& \frac{128 \sqrt{2} c_{\theta}^9 M_0^8 M_K^4 s_{\theta}^3 g_1 [M_{\eta'}, T]}{729 M_{\eta}^8 M_{\eta'}^2} + \frac{130 \sqrt{2} c_{\theta}^9 M_0^8 M_K^2 M_{\pi}^2 s_{\theta}^3 g_1 [M_{\eta'}, T]}{729 M_{\eta}^8 M_{\eta'}^2} - \\
& \frac{29 \sqrt{2} c_{\theta}^9 M_0^8 M_{\pi}^4 s_{\theta}^3 g_1 [M_{\eta'}, T]}{729 M_{\eta}^8 M_{\eta'}^2} + \frac{8 \sqrt{2} c_{\theta}^7 M_0^8 M_K^2 s_{\theta}^3 g_1 [M_{\eta'}, T]}{243 M_{\eta}^6 M_{\eta'}^2} - \frac{5 \sqrt{2} c_{\theta}^7 M_0^8 M_{\pi}^2 s_{\theta}^3 g_1 [M_{\eta'}, T]}{243 M_{\eta}^6 M_{\eta'}^2} + \\
& \frac{104 \sqrt{2} c_{\theta}^9 M_0^8 M_K^4 s_{\theta}^3 g_1 [M_{\eta'}, T]}{243 M_{\eta'}^8 (M_{\eta}^2 - M_{\eta'}^2)} - \frac{64 \sqrt{2} c_{\theta}^9 M_0^8 M_K^2 M_{\pi}^2 s_{\theta}^3 g_1 [M_{\eta'}, T]}{243 M_{\eta'}^8 (M_{\eta}^2 - M_{\eta'}^2)} + \\
& \frac{14 \sqrt{2} c_{\theta}^9 M_0^8 M_{\pi}^4 s_{\theta}^3 g_1 [M_{\eta'}, T]}{243 M_{\eta'}^8 (M_{\eta}^2 - M_{\eta'}^2)} - \frac{208 \sqrt{2} c_{\theta}^9 M_0^8 M_K^4 s_{\theta}^3 g_1 [M_{\eta'}, T]}{243 M_{\eta}^2 M_{\eta'}^6 (M_{\eta}^2 - M_{\eta'}^2)} + \\
& \frac{92 \sqrt{2} c_{\theta}^9 M_0^8 M_K^2 M_{\pi}^2 s_{\theta}^3 g_1 [M_{\eta'}, T]}{243 M_{\eta}^2 M_{\eta'}^6 (M_{\eta}^2 - M_{\eta'}^2)} - \frac{10 \sqrt{2} c_{\theta}^9 M_0^8 M_{\pi}^4 s_{\theta}^3 g_1 [M_{\eta'}, T]}{243 M_{\eta}^2 M_{\eta'}^6 (M_{\eta}^2 - M_{\eta'}^2)} + \\
& \frac{64 \sqrt{2} c_{\theta}^9 M_0^8 M_K^4 s_{\theta}^3 g_1 [M_{\eta'}, T]}{81 M_{\eta}^4 M_{\eta'}^4 (M_{\eta}^2 - M_{\eta'}^2)} - \frac{44 \sqrt{2} c_{\theta}^9 M_0^8 M_K^2 M_{\pi}^2 s_{\theta}^3 g_1 [M_{\eta'}, T]}{81 M_{\eta}^4 M_{\eta'}^4 (M_{\eta}^2 - M_{\eta'}^2)} + \\
& \frac{10 \sqrt{2} c_{\theta}^9 M_0^8 M_{\pi}^4 s_{\theta}^3 g_1 [M_{\eta'}, T]}{81 M_{\eta}^4 M_{\eta'}^4 (M_{\eta}^2 - M_{\eta'}^2)} - \frac{64 \sqrt{2} c_{\theta}^9 M_0^8 M_K^4 s_{\theta}^3 g_1 [M_{\eta'}, T]}{243 M_{\eta}^6 M_{\eta'}^2 (M_{\eta}^2 - M_{\eta'}^2)} + \\
& \frac{56 \sqrt{2} c_{\theta}^9 M_0^8 M_K^2 M_{\pi}^2 s_{\theta}^3 g_1 [M_{\eta'}, T]}{243 M_{\eta}^6 M_{\eta'}^2 (M_{\eta}^2 - M_{\eta'}^2)} - \frac{10 \sqrt{2} c_{\theta}^9 M_0^8 M_{\pi}^4 s_{\theta}^3 g_1 [M_{\eta'}, T]}{243 M_{\eta}^6 M_{\eta'}^2 (M_{\eta}^2 - M_{\eta'}^2)} - \\
& \frac{64 c_{\theta}^8 M_0^8 M_K^4 s_{\theta}^4 g_1 [M_{\eta'}, T]}{729 M_{\eta}^{10}} + \frac{44 c_{\theta}^8 M_0^8 M_K^2 M_{\pi}^2 s_{\theta}^4 g_1 [M_{\eta'}, T]}{729 M_{\eta}^{10}} - \frac{7 c_{\theta}^8 M_0^8 M_{\pi}^4 s_{\theta}^4 g_1 [M_{\eta'}, T]}{729 M_{\eta}^{10}} + \\
& \frac{4 c_{\theta}^6 M_0^8 M_K^2 s_{\theta}^4 g_1 [M_{\eta'}, T]}{243 M_{\eta}^8} - \frac{7 c_{\theta}^6 M_0^8 M_{\pi}^2 s_{\theta}^4 g_1 [M_{\eta'}, T]}{972 M_{\eta}^8} - \frac{2240 c_{\theta}^8 M_0^8 M_K^4 s_{\theta}^4 g_1 [M_{\eta'}, T]}{729 M_{\eta'}^{10}} + \\
& \frac{2236 c_{\theta}^8 M_0^8 M_K^2 M_{\pi}^2 s_{\theta}^4 g_1 [M_{\eta'}, T]}{729 M_{\eta'}^{10}} - \frac{698 c_{\theta}^8 M_0^8 M_{\pi}^4 s_{\theta}^4 g_1 [M_{\eta'}, T]}{729 M_{\eta'}^{10}} + \frac{20 c_{\theta}^6 M_0^8 M_K^2 s_{\theta}^4 g_1 [M_{\eta'}, T]}{81 M_{\eta'}^8} - \\
& \frac{35 c_{\theta}^6 M_0^8 M_{\pi}^2 s_{\theta}^4 g_1 [M_{\eta'}, T]}{324 M_{\eta'}^8} + \frac{1072 c_{\theta}^8 M_0^8 M_K^4 s_{\theta}^4 g_1 [M_{\eta'}, T]}{243 M_{\eta}^2 M_{\eta'}^8} - \frac{1052 c_{\theta}^8 M_0^8 M_K^2 M_{\pi}^2 s_{\theta}^4 g_1 [M_{\eta'}, T]}{243 M_{\eta}^2 M_{\eta'}^8} + \\
& \frac{241 c_{\theta}^8 M_0^8 M_{\pi}^4 s_{\theta}^4 g_1 [M_{\eta'}, T]}{243 M_{\eta}^2 M_{\eta'}^8} - \frac{2128 c_{\theta}^8 M_0^8 M_K^4 s_{\theta}^4 g_1 [M_{\eta'}, T]}{729 M_{\eta}^4 M_{\eta'}^6} + \frac{1922 c_{\theta}^8 M_0^8 M_K^2 M_{\pi}^2 s_{\theta}^4 g_1 [M_{\eta'}, T]}{729 M_{\eta}^4 M_{\eta'}^6} - \\
& \frac{361 c_{\theta}^8 M_0^8 M_{\pi}^4 s_{\theta}^4 g_1 [M_{\eta'}, T]}{729 M_{\eta}^4 M_{\eta'}^6} - \frac{80 c_{\theta}^6 M_0^8 M_K^2 s_{\theta}^4 g_1 [M_{\eta'}, T]}{243 M_{\eta}^2 M_{\eta'}^6} + \frac{50 c_{\theta}^6 M_0^8 M_{\pi}^2 s_{\theta}^4 g_1 [M_{\eta'}, T]}{243 M_{\eta}^2 M_{\eta'}^6} + \\
& \frac{640 c_{\theta}^8 M_0^8 M_K^4 s_{\theta}^4 g_1 [M_{\eta'}, T]}{729 M_{\eta}^6 M_{\eta'}^4} - \frac{536 c_{\theta}^8 M_0^8 M_K^2 M_{\pi}^2 s_{\theta}^4 g_1 [M_{\eta'}, T]}{729 M_{\eta}^6 M_{\eta'}^4} + \frac{112 c_{\theta}^8 M_0^8 M_{\pi}^4 s_{\theta}^4 g_1 [M_{\eta'}, T]}{729 M_{\eta}^6 M_{\eta'}^4} +
\end{aligned}$$

$$\begin{aligned}
& \frac{2 c_{\theta}^6 M_0^8 M_K^2 s_{\theta}^4 g_1 [M_{\eta'}, T]}{9 M_{\eta}^4 M_{\eta'}^4} - \frac{4 c_{\theta}^6 M_0^8 M_{\pi}^2 s_{\theta}^4 g_1 [M_{\eta'}, T]}{27 M_{\eta}^4 M_{\eta'}^4} + \frac{32 c_{\theta}^8 M_0^8 M_K^4 s_{\theta}^4 g_1 [M_{\eta'}, T]}{243 M_{\eta}^8 M_{\eta'}^2} - \\
& \frac{10 c_{\theta}^8 M_0^8 M_K^2 M_{\pi}^2 s_{\theta}^4 g_1 [M_{\eta'}, T]}{243 M_{\eta}^8 M_{\eta'}^2} - \frac{13 c_{\theta}^8 M_0^8 M_{\pi}^4 s_{\theta}^4 g_1 [M_{\eta'}, T]}{243 M_{\eta}^8 M_{\eta'}^2} - \frac{8 c_{\theta}^6 M_0^8 M_K^2 s_{\theta}^4 g_1 [M_{\eta'}, T]}{81 M_{\eta}^6 M_{\eta'}^2} + \\
& \frac{5 c_{\theta}^6 M_0^8 M_{\pi}^2 s_{\theta}^4 g_1 [M_{\eta'}, T]}{81 M_{\eta}^6 M_{\eta'}^2} - \frac{32 c_{\theta}^8 M_0^8 M_K^4 s_{\theta}^4 g_1 [M_{\eta'}, T]}{243 M_{\eta}^8 (M_{\eta}^2 - M_{\eta'}^2)} + \frac{40 c_{\theta}^8 M_0^8 M_K^2 M_{\pi}^2 s_{\theta}^4 g_1 [M_{\eta'}, T]}{243 M_{\eta}^8 (M_{\eta}^2 - M_{\eta'}^2)} - \\
& \frac{25 c_{\theta}^8 M_0^8 M_{\pi}^4 s_{\theta}^4 g_1 [M_{\eta'}, T]}{486 M_{\eta}^8 (M_{\eta}^2 - M_{\eta'}^2)} + \frac{40 c_{\theta}^8 M_0^8 M_K^4 s_{\theta}^4 g_1 [M_{\eta'}, T]}{243 M_{\eta'}^8 (M_{\eta}^2 - M_{\eta'}^2)} - \frac{38 c_{\theta}^8 M_0^8 M_K^2 M_{\pi}^2 s_{\theta}^4 g_1 [M_{\eta'}, T]}{243 M_{\eta'}^8 (M_{\eta}^2 - M_{\eta'}^2)} + \\
& \frac{23 c_{\theta}^8 M_0^8 M_{\pi}^4 s_{\theta}^4 g_1 [M_{\eta'}, T]}{486 M_{\eta'}^8 (M_{\eta}^2 - M_{\eta'}^2)} - \frac{176 c_{\theta}^8 M_0^8 M_K^4 s_{\theta}^4 g_1 [M_{\eta'}, T]}{243 M_{\eta}^2 M_{\eta'}^6 (M_{\eta}^2 - M_{\eta'}^2)} + \frac{148 c_{\theta}^8 M_0^8 M_K^2 M_{\pi}^2 s_{\theta}^4 g_1 [M_{\eta'}, T]}{243 M_{\eta}^2 M_{\eta'}^6 (M_{\eta}^2 - M_{\eta'}^2)} - \\
& \frac{26 c_{\theta}^8 M_0^8 M_{\pi}^4 s_{\theta}^4 g_1 [M_{\eta'}, T]}{243 M_{\eta}^2 M_{\eta'}^6 (M_{\eta}^2 - M_{\eta'}^2)} + \frac{32 c_{\theta}^8 M_0^8 M_K^4 s_{\theta}^4 g_1 [M_{\eta'}, T]}{81 M_{\eta}^4 M_{\eta'}^4 (M_{\eta}^2 - M_{\eta'}^2)} - \frac{10 c_{\theta}^8 M_0^8 M_K^2 M_{\pi}^2 s_{\theta}^4 g_1 [M_{\eta'}, T]}{81 M_{\eta}^4 M_{\eta'}^4 (M_{\eta}^2 - M_{\eta'}^2)} - \\
& \frac{c_{\theta}^8 M_0^8 M_{\pi}^4 s_{\theta}^4 g_1 [M_{\eta'}, T]}{81 M_{\eta}^4 M_{\eta'}^4 (M_{\eta}^2 - M_{\eta'}^2)} + \frac{64 c_{\theta}^8 M_0^8 M_K^4 s_{\theta}^4 g_1 [M_{\eta'}, T]}{243 M_{\eta}^6 M_{\eta'}^2 (M_{\eta}^2 - M_{\eta'}^2)} - \frac{104 c_{\theta}^8 M_0^8 M_K^2 M_{\pi}^2 s_{\theta}^4 g_1 [M_{\eta'}, T]}{243 M_{\eta}^6 M_{\eta'}^2 (M_{\eta}^2 - M_{\eta'}^2)} + \\
& \frac{22 c_{\theta}^8 M_0^8 M_{\pi}^4 s_{\theta}^4 g_1 [M_{\eta'}, T]}{243 M_{\eta}^6 M_{\eta'}^2 (M_{\eta}^2 - M_{\eta'}^2)} - \frac{64 \sqrt{2} c_{\theta}^7 M_0^8 M_K^4 s_{\theta}^5 g_1 [M_{\eta'}, T]}{729 M_{\eta}^{10}} + \frac{68 \sqrt{2} c_{\theta}^7 M_0^8 M_K^2 M_{\pi}^2 s_{\theta}^5 g_1 [M_{\eta'}, T]}{729 M_{\eta}^{10}} - \\
& \frac{13 \sqrt{2} c_{\theta}^7 M_0^8 M_{\pi}^4 s_{\theta}^5 g_1 [M_{\eta'}, T]}{729 M_{\eta}^{10}} - \frac{c_{\theta}^5 M_0^8 M_{\pi}^2 s_{\theta}^5 g_1 [M_{\eta'}, T]}{162 \sqrt{2} M_{\eta}^8} + \frac{1792 \sqrt{2} c_{\theta}^7 M_0^8 M_K^4 s_{\theta}^5 g_1 [M_{\eta'}, T]}{729 M_{\eta}^{10}} - \\
& \frac{1712 \sqrt{2} c_{\theta}^7 M_0^8 M_K^2 M_{\pi}^2 s_{\theta}^5 g_1 [M_{\eta'}, T]}{729 M_{\eta}^{10}} + \frac{352 \sqrt{2} c_{\theta}^7 M_0^8 M_{\pi}^4 s_{\theta}^5 g_1 [M_{\eta'}, T]}{729 M_{\eta}^{10}} - \\
& \frac{8 \sqrt{2} c_{\theta}^5 M_0^8 M_K^2 s_{\theta}^5 g_1 [M_{\eta'}, T]}{81 M_{\eta}^8} + \frac{17 c_{\theta}^5 M_0^8 M_{\pi}^2 s_{\theta}^5 g_1 [M_{\eta'}, T]}{162 \sqrt{2} M_{\eta}^8} - \frac{832 \sqrt{2} c_{\theta}^7 M_0^8 M_K^4 s_{\theta}^5 g_1 [M_{\eta'}, T]}{243 M_{\eta}^2 M_{\eta'}^8} + \\
& \frac{224 \sqrt{2} c_{\theta}^7 M_0^8 M_K^2 M_{\pi}^2 s_{\theta}^5 g_1 [M_{\eta'}, T]}{81 M_{\eta}^2 M_{\eta'}^8} - \frac{179 \sqrt{2} c_{\theta}^7 M_0^8 M_{\pi}^4 s_{\theta}^5 g_1 [M_{\eta'}, T]}{243 M_{\eta}^2 M_{\eta'}^8} + \\
& \frac{2048 \sqrt{2} c_{\theta}^7 M_0^8 M_K^4 s_{\theta}^5 g_1 [M_{\eta'}, T]}{729 M_{\eta}^4 M_{\eta'}^6} - \frac{1060 \sqrt{2} c_{\theta}^7 M_0^8 M_K^2 M_{\pi}^2 s_{\theta}^5 g_1 [M_{\eta'}, T]}{729 M_{\eta}^4 M_{\eta'}^6} + \\
& \frac{164 \sqrt{2} c_{\theta}^7 M_0^8 M_{\pi}^4 s_{\theta}^5 g_1 [M_{\eta'}, T]}{729 M_{\eta}^4 M_{\eta'}^6} + \frac{5 c_{\theta}^5 M_0^8 M_{\pi}^2 s_{\theta}^5 g_1 [M_{\eta'}, T]}{81 \sqrt{2} M_{\eta}^2 M_{\eta'}^6} - \frac{1376 \sqrt{2} c_{\theta}^7 M_0^8 M_K^4 s_{\theta}^5 g_1 [M_{\eta'}, T]}{729 M_{\eta}^6 M_{\eta'}^4} + \\
& \frac{628 \sqrt{2} c_{\theta}^7 M_0^8 M_K^2 M_{\pi}^2 s_{\theta}^5 g_1 [M_{\eta'}, T]}{729 M_{\eta}^6 M_{\eta'}^4} - \frac{62 \sqrt{2} c_{\theta}^7 M_0^8 M_{\pi}^4 s_{\theta}^5 g_1 [M_{\eta'}, T]}{729 M_{\eta}^6 M_{\eta'}^4} + \\
& \frac{8 \sqrt{2} c_{\theta}^5 M_0^8 M_K^2 s_{\theta}^5 g_1 [M_{\eta'}, T]}{81 M_{\eta}^4 M_{\eta'}^4} - \frac{5 \sqrt{2} c_{\theta}^5 M_0^8 M_{\pi}^2 s_{\theta}^5 g_1 [M_{\eta'}, T]}{81 M_{\eta}^4 M_{\eta'}^4} + \frac{64 \sqrt{2} c_{\theta}^7 M_0^8 M_K^4 s_{\theta}^5 g_1 [M_{\eta'}, T]}{81 M_{\eta}^8 M_{\eta'}^2} -
\end{aligned}$$

$$\begin{aligned}
& \frac{140 \sqrt{2} c_{\theta}^7 M_0^8 M_K^2 M_{\pi}^2 s_{\theta}^5 g_1 [M_{\eta'}, T]}{243 M_{\eta}^8 M_{\eta'}^2} + \frac{32 \sqrt{2} c_{\theta}^7 M_0^8 M_{\pi}^4 s_{\theta}^5 g_1 [M_{\eta'}, T]}{243 M_{\eta}^8 M_{\eta'}^2} - \\
& \frac{4 \sqrt{2} c_{\theta}^5 M_0^8 M_K^2 s_{\theta}^5 g_1 [M_{\eta'}, T]}{81 M_{\eta}^6 M_{\eta'}^2} + \frac{5 c_{\theta}^5 M_0^8 M_{\pi}^2 s_{\theta}^5 g_1 [M_{\eta'}, T]}{81 \sqrt{2} M_{\eta}^6 M_{\eta'}^2} - \frac{32 \sqrt{2} c_{\theta}^7 M_0^8 M_K^4 s_{\theta}^5 g_1 [M_{\eta'}, T]}{243 M_{\eta}^8 (M_{\eta}^2 - M_{\eta'}^2)} + \\
& \frac{16 \sqrt{2} c_{\theta}^7 M_0^8 M_K^2 M_{\pi}^2 s_{\theta}^5 g_1 [M_{\eta'}, T]}{243 M_{\eta}^8 (M_{\eta}^2 - M_{\eta'}^2)} + \frac{5 c_{\theta}^7 M_0^8 M_{\pi}^4 s_{\theta}^5 g_1 [M_{\eta'}, T]}{243 \sqrt{2} M_{\eta}^8 (M_{\eta}^2 - M_{\eta'}^2)} - \frac{128 \sqrt{2} c_{\theta}^7 M_0^8 M_K^4 s_{\theta}^5 g_1 [M_{\eta'}, T]}{243 M_{\eta'}^8 (M_{\eta}^2 - M_{\eta'}^2)} + \\
& \frac{88 \sqrt{2} c_{\theta}^7 M_0^8 M_K^2 M_{\pi}^2 s_{\theta}^5 g_1 [M_{\eta'}, T]}{243 M_{\eta'}^8 (M_{\eta}^2 - M_{\eta'}^2)} - \frac{37 c_{\theta}^7 M_0^8 M_{\pi}^4 s_{\theta}^5 g_1 [M_{\eta'}, T]}{243 \sqrt{2} M_{\eta'}^8 (M_{\eta}^2 - M_{\eta'}^2)} + \\
& \frac{400 \sqrt{2} c_{\theta}^7 M_0^8 M_K^4 s_{\theta}^5 g_1 [M_{\eta'}, T]}{243 M_{\eta}^2 M_{\eta'}^6 (M_{\eta}^2 - M_{\eta'}^2)} - \frac{200 \sqrt{2} c_{\theta}^7 M_0^8 M_K^2 M_{\pi}^2 s_{\theta}^5 g_1 [M_{\eta'}, T]}{243 M_{\eta}^2 M_{\eta'}^6 (M_{\eta}^2 - M_{\eta'}^2)} + \\
& \frac{25 \sqrt{2} c_{\theta}^7 M_0^8 M_{\pi}^4 s_{\theta}^5 g_1 [M_{\eta'}, T]}{243 M_{\eta}^2 M_{\eta'}^6 (M_{\eta}^2 - M_{\eta'}^2)} - \frac{160 \sqrt{2} c_{\theta}^7 M_0^8 M_K^4 s_{\theta}^5 g_1 [M_{\eta'}, T]}{81 M_{\eta}^4 M_{\eta'}^4 (M_{\eta}^2 - M_{\eta'}^2)} + \\
& \frac{68 \sqrt{2} c_{\theta}^7 M_0^8 M_K^2 M_{\pi}^2 s_{\theta}^5 g_1 [M_{\eta'}, T]}{81 M_{\eta}^4 M_{\eta'}^4 (M_{\eta}^2 - M_{\eta'}^2)} - \frac{4 \sqrt{2} c_{\theta}^7 M_0^8 M_{\pi}^4 s_{\theta}^5 g_1 [M_{\eta'}, T]}{81 M_{\eta}^4 M_{\eta'}^4 (M_{\eta}^2 - M_{\eta'}^2)} + \\
& \frac{256 \sqrt{2} c_{\theta}^7 M_0^8 M_K^4 s_{\theta}^5 g_1 [M_{\eta'}, T]}{243 M_{\eta}^6 M_{\eta'}^2 (M_{\eta}^2 - M_{\eta'}^2)} - \frac{140 \sqrt{2} c_{\theta}^7 M_0^8 M_K^2 M_{\pi}^2 s_{\theta}^5 g_1 [M_{\eta'}, T]}{243 M_{\eta}^6 M_{\eta'}^2 (M_{\eta}^2 - M_{\eta'}^2)} + \\
& \frac{19 \sqrt{2} c_{\theta}^7 M_0^8 M_{\pi}^4 s_{\theta}^5 g_1 [M_{\eta'}, T]}{243 M_{\eta}^6 M_{\eta'}^2 (M_{\eta}^2 - M_{\eta'}^2)} + \frac{160 c_{\theta}^6 M_0^8 M_K^4 s_{\theta}^6 g_1 [M_{\eta'}, T]}{729 M_{\eta}^{10}} - \frac{194 c_{\theta}^6 M_0^8 M_K^2 M_{\pi}^2 s_{\theta}^6 g_1 [M_{\eta'}, T]}{729 M_{\eta}^{10}} + \\
& \frac{77 c_{\theta}^6 M_0^8 M_{\pi}^4 s_{\theta}^6 g_1 [M_{\eta'}, T]}{1458 M_{\eta}^{10}} - \frac{4 c_{\theta}^4 M_0^8 M_K^2 s_{\theta}^6 g_1 [M_{\eta'}, T]}{81 M_{\eta}^8} + \frac{19 c_{\theta}^4 M_0^8 M_{\pi}^2 s_{\theta}^6 g_1 [M_{\eta'}, T]}{648 M_{\eta}^8} - \\
& \frac{1792 c_{\theta}^6 M_0^8 M_K^4 s_{\theta}^6 g_1 [M_{\eta'}, T]}{729 M_{\eta}^{10}} + \frac{1808 c_{\theta}^6 M_0^8 M_K^2 M_{\pi}^2 s_{\theta}^6 g_1 [M_{\eta'}, T]}{729 M_{\eta}^{10}} - \frac{484 c_{\theta}^6 M_0^8 M_{\pi}^4 s_{\theta}^6 g_1 [M_{\eta'}, T]}{729 M_{\eta}^{10}} + \\
& \frac{8 c_{\theta}^4 M_0^8 M_K^2 s_{\theta}^6 g_1 [M_{\eta'}, T]}{243 M_{\eta}^8} - \frac{31 c_{\theta}^4 M_0^8 M_{\pi}^2 s_{\theta}^6 g_1 [M_{\eta'}, T]}{1944 M_{\eta}^8} + \frac{352 c_{\theta}^6 M_0^8 M_K^4 s_{\theta}^6 g_1 [M_{\eta'}, T]}{243 M_{\eta}^2 M_{\eta'}^8} - \\
& \frac{376 c_{\theta}^6 M_0^8 M_K^2 M_{\pi}^2 s_{\theta}^6 g_1 [M_{\eta'}, T]}{243 M_{\eta}^2 M_{\eta'}^8} + \frac{19 c_{\theta}^6 M_0^8 M_{\pi}^4 s_{\theta}^6 g_1 [M_{\eta'}, T]}{162 M_{\eta}^2 M_{\eta'}^8} + \frac{352 c_{\theta}^6 M_0^8 M_K^4 s_{\theta}^6 g_1 [M_{\eta'}, T]}{729 M_{\eta}^4 M_{\eta'}^6} - \\
& \frac{164 c_{\theta}^6 M_0^8 M_K^2 M_{\pi}^2 s_{\theta}^6 g_1 [M_{\eta'}, T]}{729 M_{\eta}^4 M_{\eta'}^6} + \frac{46 c_{\theta}^6 M_0^8 M_{\pi}^4 s_{\theta}^6 g_1 [M_{\eta'}, T]}{729 M_{\eta}^4 M_{\eta'}^6} + \frac{16 c_{\theta}^4 M_0^8 M_K^2 s_{\theta}^6 g_1 [M_{\eta'}, T]}{81 M_{\eta}^2 M_{\eta'}^6} - \\
& \frac{13 c_{\theta}^4 M_0^8 M_{\pi}^2 s_{\theta}^6 g_1 [M_{\eta'}, T]}{162 M_{\eta}^2 M_{\eta'}^6} - \frac{400 c_{\theta}^6 M_0^8 M_K^4 s_{\theta}^6 g_1 [M_{\eta'}, T]}{729 M_{\eta}^6 M_{\eta'}^4} + \frac{86 c_{\theta}^6 M_0^8 M_K^2 M_{\pi}^2 s_{\theta}^6 g_1 [M_{\eta'}, T]}{729 M_{\eta}^6 M_{\eta'}^4} + \\
& \frac{62 c_{\theta}^6 M_0^8 M_{\pi}^4 s_{\theta}^6 g_1 [M_{\eta'}, T]}{729 M_{\eta}^6 M_{\eta'}^4} - \frac{8 c_{\theta}^4 M_0^8 M_K^2 s_{\theta}^6 g_1 [M_{\eta'}, T]}{27 M_{\eta}^4 M_{\eta'}^4} + \frac{19 c_{\theta}^4 M_0^8 M_{\pi}^2 s_{\theta}^6 g_1 [M_{\eta'}, T]}{108 M_{\eta}^4 M_{\eta'}^4} -
\end{aligned}$$

$$\begin{aligned}
& \frac{32 c_{\theta}^6 M_0^8 M_K^4 s_{\theta}^6 g_1 [M_{\eta'}, T]}{243 M_{\eta}^8 M_{\eta'}^2} + \frac{104 c_{\theta}^6 M_0^8 M_K^2 M_{\pi}^2 s_{\theta}^6 g_1 [M_{\eta'}, T]}{243 M_{\eta}^8 M_{\eta'}^2} - \frac{4 c_{\theta}^6 M_0^8 M_{\pi}^4 s_{\theta}^6 g_1 [M_{\eta'}, T]}{27 M_{\eta}^8 M_{\eta'}^2} + \\
& \frac{44 c_{\theta}^4 M_0^8 M_K^2 s_{\theta}^6 g_1 [M_{\eta'}, T]}{243 M_{\eta}^6 M_{\eta'}^2} - \frac{55 c_{\theta}^4 M_0^8 M_{\pi}^2 s_{\theta}^6 g_1 [M_{\eta'}, T]}{486 M_{\eta}^6 M_{\eta'}^2} + \frac{80 c_{\theta}^6 M_0^8 M_K^4 s_{\theta}^6 g_1 [M_{\eta'}, T]}{243 M_{\eta}^8 (M_{\eta}^2 - M_{\eta'}^2)} - \\
& \frac{88 c_{\theta}^6 M_0^8 M_K^2 M_{\pi}^2 s_{\theta}^6 g_1 [M_{\eta'}, T]}{243 M_{\eta}^8 (M_{\eta}^2 - M_{\eta'}^2)} + \frac{59 c_{\theta}^6 M_0^8 M_{\pi}^4 s_{\theta}^6 g_1 [M_{\eta'}, T]}{972 M_{\eta}^8 (M_{\eta}^2 - M_{\eta'}^2)} + \frac{80 c_{\theta}^6 M_0^8 M_K^4 s_{\theta}^6 g_1 [M_{\eta'}, T]}{243 M_{\eta'}^8 (M_{\eta}^2 - M_{\eta'}^2)} - \\
& \frac{88 c_{\theta}^6 M_0^8 M_K^2 M_{\pi}^2 s_{\theta}^6 g_1 [M_{\eta'}, T]}{243 M_{\eta'}^8 (M_{\eta}^2 - M_{\eta'}^2)} + \frac{59 c_{\theta}^6 M_0^8 M_{\pi}^4 s_{\theta}^6 g_1 [M_{\eta'}, T]}{972 M_{\eta'}^8 (M_{\eta}^2 - M_{\eta'}^2)} - \frac{64 c_{\theta}^6 M_0^8 M_K^4 s_{\theta}^6 g_1 [M_{\eta'}, T]}{243 M_{\eta}^2 M_{\eta'}^6 (M_{\eta}^2 - M_{\eta'}^2)} + \\
& \frac{92 c_{\theta}^6 M_0^8 M_K^2 M_{\pi}^2 s_{\theta}^6 g_1 [M_{\eta'}, T]}{243 M_{\eta}^2 M_{\eta'}^6 (M_{\eta}^2 - M_{\eta'}^2)} - \frac{19 c_{\theta}^6 M_0^8 M_{\pi}^4 s_{\theta}^6 g_1 [M_{\eta'}, T]}{243 M_{\eta}^2 M_{\eta'}^6 (M_{\eta}^2 - M_{\eta'}^2)} - \frac{8 c_{\theta}^6 M_0^8 M_K^4 s_{\theta}^6 g_1 [M_{\eta'}, T]}{81 M_{\eta}^4 M_{\eta'}^4 (M_{\eta}^2 - M_{\eta'}^2)} - \\
& \frac{8 c_{\theta}^6 M_0^8 M_K^2 M_{\pi}^2 s_{\theta}^6 g_1 [M_{\eta'}, T]}{81 M_{\eta}^4 M_{\eta'}^4 (M_{\eta}^2 - M_{\eta'}^2)} + \frac{11 c_{\theta}^6 M_0^8 M_{\pi}^4 s_{\theta}^6 g_1 [M_{\eta'}, T]}{162 M_{\eta}^4 M_{\eta'}^4 (M_{\eta}^2 - M_{\eta'}^2)} - \frac{64 c_{\theta}^6 M_0^8 M_K^4 s_{\theta}^6 g_1 [M_{\eta'}, T]}{243 M_{\eta}^6 M_{\eta'}^2 (M_{\eta}^2 - M_{\eta'}^2)} + \\
& \frac{92 c_{\theta}^6 M_0^8 M_K^2 M_{\pi}^2 s_{\theta}^6 g_1 [M_{\eta'}, T]}{243 M_{\eta}^6 M_{\eta'}^2 (M_{\eta}^2 - M_{\eta'}^2)} - \frac{19 c_{\theta}^6 M_0^8 M_{\pi}^4 s_{\theta}^6 g_1 [M_{\eta'}, T]}{243 M_{\eta}^6 M_{\eta'}^2 (M_{\eta}^2 - M_{\eta'}^2)} + \frac{256 \sqrt{2} c_{\theta}^5 M_0^8 M_K^4 s_{\theta}^7 g_1 [M_{\eta'}, T]}{729 M_{\eta}^{10}} - \\
& \frac{140 \sqrt{2} c_{\theta}^5 M_0^8 M_K^2 M_{\pi}^2 s_{\theta}^7 g_1 [M_{\eta'}, T]}{729 M_{\eta}^{10}} + \frac{19 \sqrt{2} c_{\theta}^5 M_0^8 M_{\pi}^4 s_{\theta}^7 g_1 [M_{\eta'}, T]}{729 M_{\eta}^{10}} - \\
& \frac{4 \sqrt{2} c_{\theta}^3 M_0^8 M_K^2 s_{\theta}^7 g_1 [M_{\eta'}, T]}{243 M_{\eta}^8} + \frac{5 c_{\theta}^3 M_0^8 M_{\pi}^2 s_{\theta}^7 g_1 [M_{\eta'}, T]}{243 \sqrt{2} M_{\eta}^8} + \frac{512 \sqrt{2} c_{\theta}^5 M_0^8 M_K^4 s_{\theta}^7 g_1 [M_{\eta'}, T]}{729 M_{\eta}^{10}} - \\
& \frac{544 \sqrt{2} c_{\theta}^5 M_0^8 M_K^2 M_{\pi}^2 s_{\theta}^7 g_1 [M_{\eta'}, T]}{729 M_{\eta}^{10}} + \frac{140 \sqrt{2} c_{\theta}^5 M_0^8 M_{\pi}^4 s_{\theta}^7 g_1 [M_{\eta'}, T]}{729 M_{\eta}^{10}} + \\
& \frac{320 \sqrt{2} c_{\theta}^5 M_0^8 M_K^4 s_{\theta}^7 g_1 [M_{\eta'}, T]}{243 M_{\eta}^2 M_{\eta'}^8} - \frac{232 \sqrt{2} c_{\theta}^5 M_0^8 M_K^2 M_{\pi}^2 s_{\theta}^7 g_1 [M_{\eta'}, T]}{243 M_{\eta}^2 M_{\eta'}^8} + \\
& \frac{11 \sqrt{2} c_{\theta}^5 M_0^8 M_{\pi}^4 s_{\theta}^7 g_1 [M_{\eta'}, T]}{243 M_{\eta}^2 M_{\eta'}^8} - \frac{2048 \sqrt{2} c_{\theta}^5 M_0^8 M_K^4 s_{\theta}^7 g_1 [M_{\eta'}, T]}{729 M_{\eta}^4 M_{\eta'}^6} + \\
& \frac{1228 \sqrt{2} c_{\theta}^5 M_0^8 M_K^2 M_{\pi}^2 s_{\theta}^7 g_1 [M_{\eta'}, T]}{729 M_{\eta}^4 M_{\eta'}^6} - \frac{206 \sqrt{2} c_{\theta}^5 M_0^8 M_{\pi}^4 s_{\theta}^7 g_1 [M_{\eta'}, T]}{729 M_{\eta}^4 M_{\eta'}^6} - \\
& \frac{16 \sqrt{2} c_{\theta}^3 M_0^8 M_K^2 s_{\theta}^7 g_1 [M_{\eta'}, T]}{243 M_{\eta}^2 M_{\eta'}^6} + \frac{17 c_{\theta}^3 M_0^8 M_{\pi}^2 s_{\theta}^7 g_1 [M_{\eta'}, T]}{243 \sqrt{2} M_{\eta}^2 M_{\eta'}^6} + \frac{1760 \sqrt{2} c_{\theta}^5 M_0^8 M_K^4 s_{\theta}^7 g_1 [M_{\eta'}, T]}{729 M_{\eta}^6 M_{\eta'}^4} - \\
& \frac{592 \sqrt{2} c_{\theta}^5 M_0^8 M_K^2 M_{\pi}^2 s_{\theta}^7 g_1 [M_{\eta'}, T]}{729 M_{\eta}^6 M_{\eta'}^4} - \frac{34 \sqrt{2} c_{\theta}^5 M_0^8 M_{\pi}^4 s_{\theta}^7 g_1 [M_{\eta'}, T]}{729 M_{\eta}^6 M_{\eta'}^4} + \\
& \frac{c_{\theta}^3 M_0^8 M_{\pi}^2 s_{\theta}^7 g_1 [M_{\eta'}, T]}{81 \sqrt{2} M_{\eta}^4 M_{\eta'}^4} + \frac{\sqrt{2} c_{\theta}^3 M_0^8 M_{\pi}^2 s_{\theta}^7 g_1 [M_{\eta'}, T]}{81 M_{\eta}^4 M_{\eta'}^4} - \frac{320 \sqrt{2} c_{\theta}^5 M_0^8 M_K^4 s_{\theta}^7 g_1 [M_{\eta'}, T]}{243 M_{\eta}^8 M_{\eta'}^2} +
\end{aligned}$$

$$\begin{aligned}
& \frac{88 \sqrt{2} c_{\theta}^5 M_0^8 M_K^2 M_{\pi}^2 s_{\theta}^7 g_1 [M_{\eta'}, T]}{243 M_{\eta}^8 M_{\eta'}^2} + \frac{16 \sqrt{2} c_{\theta}^5 M_0^8 M_{\pi}^4 s_{\theta}^7 g_1 [M_{\eta'}, T]}{243 M_{\eta}^8 M_{\eta'}^2} + \\
& \frac{4 \sqrt{2} c_{\theta}^3 M_0^8 M_K^2 s_{\theta}^7 g_1 [M_{\eta'}, T]}{81 M_{\eta}^6 M_{\eta'}^2} - \frac{5 c_{\theta}^3 M_0^8 M_{\pi}^2 s_{\theta}^7 g_1 [M_{\eta'}, T]}{81 \sqrt{2} M_{\eta}^6 M_{\eta'}^2} + \frac{128 \sqrt{2} c_{\theta}^5 M_0^8 M_K^4 s_{\theta}^7 g_1 [M_{\eta'}, T]}{243 M_{\eta}^8 (M_{\eta}^2 - M_{\eta'}^2)} - \\
& \frac{88 \sqrt{2} c_{\theta}^5 M_0^8 M_K^2 M_{\pi}^2 s_{\theta}^7 g_1 [M_{\eta'}, T]}{243 M_{\eta}^8 (M_{\eta}^2 - M_{\eta'}^2)} + \frac{37 c_{\theta}^5 M_0^8 M_{\pi}^4 s_{\theta}^7 g_1 [M_{\eta'}, T]}{243 \sqrt{2} M_{\eta}^8 (M_{\eta}^2 - M_{\eta'}^2)} + \frac{32 \sqrt{2} c_{\theta}^5 M_0^8 M_K^4 s_{\theta}^7 g_1 [M_{\eta'}, T]}{243 M_{\eta'}^8 (M_{\eta}^2 - M_{\eta'}^2)} - \\
& \frac{16 \sqrt{2} c_{\theta}^5 M_0^8 M_K^2 M_{\pi}^2 s_{\theta}^7 g_1 [M_{\eta'}, T]}{243 M_{\eta'}^8 (M_{\eta}^2 - M_{\eta'}^2)} - \frac{5 c_{\theta}^5 M_0^8 M_{\pi}^4 s_{\theta}^7 g_1 [M_{\eta'}, T]}{243 \sqrt{2} M_{\eta'}^8 (M_{\eta}^2 - M_{\eta'}^2)} - \frac{256 \sqrt{2} c_{\theta}^5 M_0^8 M_K^4 s_{\theta}^7 g_1 [M_{\eta'}, T]}{243 M_{\eta}^2 M_{\eta'}^6 (M_{\eta}^2 - M_{\eta'}^2)} + \\
& \frac{140 \sqrt{2} c_{\theta}^5 M_0^8 M_K^2 M_{\pi}^2 s_{\theta}^7 g_1 [M_{\eta'}, T]}{243 M_{\eta}^2 M_{\eta'}^6 (M_{\eta}^2 - M_{\eta'}^2)} - \frac{19 \sqrt{2} c_{\theta}^5 M_0^8 M_{\pi}^4 s_{\theta}^7 g_1 [M_{\eta'}, T]}{243 M_{\eta}^2 M_{\eta'}^6 (M_{\eta}^2 - M_{\eta'}^2)} + \\
& \frac{160 \sqrt{2} c_{\theta}^5 M_0^8 M_K^4 s_{\theta}^7 g_1 [M_{\eta'}, T]}{81 M_{\eta}^4 M_{\eta'}^4 (M_{\eta}^2 - M_{\eta'}^2)} - \frac{68 \sqrt{2} c_{\theta}^5 M_0^8 M_K^2 M_{\pi}^2 s_{\theta}^7 g_1 [M_{\eta'}, T]}{81 M_{\eta}^4 M_{\eta'}^4 (M_{\eta}^2 - M_{\eta'}^2)} + \\
& \frac{4 \sqrt{2} c_{\theta}^5 M_0^8 M_{\pi}^4 s_{\theta}^7 g_1 [M_{\eta'}, T]}{81 M_{\eta}^4 M_{\eta'}^4 (M_{\eta}^2 - M_{\eta'}^2)} - \frac{400 \sqrt{2} c_{\theta}^5 M_0^8 M_K^4 s_{\theta}^7 g_1 [M_{\eta'}, T]}{243 M_{\eta}^6 M_{\eta'}^2 (M_{\eta}^2 - M_{\eta'}^2)} + \\
& \frac{200 \sqrt{2} c_{\theta}^5 M_0^8 M_K^2 M_{\pi}^2 s_{\theta}^7 g_1 [M_{\eta'}, T]}{243 M_{\eta}^6 M_{\eta'}^2 (M_{\eta}^2 - M_{\eta'}^2)} - \frac{25 \sqrt{2} c_{\theta}^5 M_0^8 M_{\pi}^4 s_{\theta}^7 g_1 [M_{\eta'}, T]}{243 M_{\eta}^6 M_{\eta'}^2 (M_{\eta}^2 - M_{\eta'}^2)} + \\
& \frac{80 c_{\theta}^4 M_0^8 M_K^4 s_{\theta}^8 g_1 [M_{\eta'}, T]}{729 M_{\eta}^{10}} - \frac{40 c_{\theta}^4 M_0^8 M_K^2 M_{\pi}^2 s_{\theta}^8 g_1 [M_{\eta'}, T]}{729 M_{\eta}^{10}} + \frac{5 c_{\theta}^4 M_0^8 M_{\pi}^4 s_{\theta}^8 g_1 [M_{\eta'}, T]}{729 M_{\eta}^{10}} + \\
& \frac{c_{\theta}^2 M_0^8 M_K^2 s_{\theta}^8 g_1 [M_{\eta'}, T]}{27 M_{\eta}^8} - \frac{2 c_{\theta}^2 M_0^8 M_{\pi}^2 s_{\theta}^8 g_1 [M_{\eta'}, T]}{81 M_{\eta}^8} - \frac{128 c_{\theta}^4 M_0^8 M_K^4 s_{\theta}^8 g_1 [M_{\eta'}, T]}{729 M_{\eta'}^{10}} + \\
& \frac{112 c_{\theta}^4 M_0^8 M_K^2 M_{\pi}^2 s_{\theta}^8 g_1 [M_{\eta'}, T]}{729 M_{\eta'}^{10}} - \frac{49 c_{\theta}^4 M_0^8 M_{\pi}^4 s_{\theta}^8 g_1 [M_{\eta'}, T]}{1458 M_{\eta'}^{10}} - \frac{448 c_{\theta}^4 M_0^8 M_K^4 s_{\theta}^8 g_1 [M_{\eta'}, T]}{243 M_{\eta}^2 M_{\eta'}^8} + \\
& \frac{160 c_{\theta}^4 M_0^8 M_K^2 M_{\pi}^2 s_{\theta}^8 g_1 [M_{\eta'}, T]}{81 M_{\eta}^2 M_{\eta'}^8} - \frac{137 c_{\theta}^4 M_0^8 M_{\pi}^4 s_{\theta}^8 g_1 [M_{\eta'}, T]}{243 M_{\eta}^2 M_{\eta'}^8} + \frac{1088 c_{\theta}^4 M_0^8 M_K^4 s_{\theta}^8 g_1 [M_{\eta'}, T]}{729 M_{\eta}^4 M_{\eta'}^6} - \\
& \frac{1318 c_{\theta}^4 M_0^8 M_K^2 M_{\pi}^2 s_{\theta}^8 g_1 [M_{\eta'}, T]}{729 M_{\eta}^4 M_{\eta'}^6} + \frac{248 c_{\theta}^4 M_0^8 M_{\pi}^4 s_{\theta}^8 g_1 [M_{\eta'}, T]}{729 M_{\eta}^4 M_{\eta'}^6} + \frac{64 c_{\theta}^4 M_0^8 M_K^4 s_{\theta}^8 g_1 [M_{\eta'}, T]}{729 M_{\eta}^6 M_{\eta'}^4} + \\
& \frac{268 c_{\theta}^4 M_0^8 M_K^2 M_{\pi}^2 s_{\theta}^8 g_1 [M_{\eta'}, T]}{729 M_{\eta}^6 M_{\eta'}^4} - \frac{116 c_{\theta}^4 M_0^8 M_{\pi}^4 s_{\theta}^8 g_1 [M_{\eta'}, T]}{729 M_{\eta}^6 M_{\eta'}^4} + \frac{8 c_{\theta}^2 M_0^8 M_K^2 s_{\theta}^8 g_1 [M_{\eta'}, T]}{81 M_{\eta}^4 M_{\eta'}^4} - \\
& \frac{7 c_{\theta}^2 M_0^8 M_{\pi}^2 s_{\theta}^8 g_1 [M_{\eta'}, T]}{162 M_{\eta}^4 M_{\eta'}^4} - \frac{40 c_{\theta}^4 M_0^8 M_K^4 s_{\theta}^8 g_1 [M_{\eta'}, T]}{81 M_{\eta}^8 M_{\eta'}^2} + \frac{46 c_{\theta}^4 M_0^8 M_K^2 M_{\pi}^2 s_{\theta}^8 g_1 [M_{\eta'}, T]}{243 M_{\eta}^8 M_{\eta'}^2} + \\
& \frac{19 c_{\theta}^4 M_0^8 M_{\pi}^4 s_{\theta}^8 g_1 [M_{\eta'}, T]}{486 M_{\eta}^8 M_{\eta'}^2} - \frac{8 c_{\theta}^2 M_0^8 M_K^2 s_{\theta}^8 g_1 [M_{\eta'}, T]}{81 M_{\eta}^6 M_{\eta'}^2} + \frac{5 c_{\theta}^2 M_0^8 M_{\pi}^2 s_{\theta}^8 g_1 [M_{\eta'}, T]}{81 M_{\eta}^6 M_{\eta'}^2} +
\end{aligned}$$

$$\begin{aligned}
& \frac{40 c_{\theta}^4 M_0^8 M_K^4 s_{\theta}^8 g_1 [M_{\eta'}, T]}{243 M_{\eta}^8 (M_{\eta}^2 - M_{\eta'}^2)} - \frac{38 c_{\theta}^4 M_0^8 M_K^2 M_{\pi}^2 s_{\theta}^8 g_1 [M_{\eta'}, T]}{243 M_{\eta}^8 (M_{\eta}^2 - M_{\eta'}^2)} + \frac{23 c_{\theta}^4 M_0^8 M_{\pi}^4 s_{\theta}^8 g_1 [M_{\eta'}, T]}{486 M_{\eta}^8 (M_{\eta}^2 - M_{\eta'}^2)} - \\
& \frac{32 c_{\theta}^4 M_0^8 M_K^4 s_{\theta}^8 g_1 [M_{\eta'}, T]}{243 M_{\eta'}^8 (M_{\eta}^2 - M_{\eta'}^2)} + \frac{40 c_{\theta}^4 M_0^8 M_K^2 M_{\pi}^2 s_{\theta}^8 g_1 [M_{\eta'}, T]}{243 M_{\eta'}^8 (M_{\eta}^2 - M_{\eta'}^2)} - \frac{25 c_{\theta}^4 M_0^8 M_{\pi}^4 s_{\theta}^8 g_1 [M_{\eta'}, T]}{486 M_{\eta'}^8 (M_{\eta}^2 - M_{\eta'}^2)} + \\
& \frac{64 c_{\theta}^4 M_0^8 M_K^4 s_{\theta}^8 g_1 [M_{\eta'}, T]}{243 M_{\eta}^2 M_{\eta'}^6 (M_{\eta}^2 - M_{\eta'}^2)} - \frac{104 c_{\theta}^4 M_0^8 M_K^2 M_{\pi}^2 s_{\theta}^8 g_1 [M_{\eta'}, T]}{243 M_{\eta}^2 M_{\eta'}^6 (M_{\eta}^2 - M_{\eta'}^2)} + \frac{22 c_{\theta}^4 M_0^8 M_{\pi}^4 s_{\theta}^8 g_1 [M_{\eta'}, T]}{243 M_{\eta}^2 M_{\eta'}^6 (M_{\eta}^2 - M_{\eta'}^2)} + \\
& \frac{32 c_{\theta}^4 M_0^8 M_K^4 s_{\theta}^8 g_1 [M_{\eta'}, T]}{81 M_{\eta}^4 M_{\eta'}^4 (M_{\eta}^2 - M_{\eta'}^2)} - \frac{10 c_{\theta}^4 M_0^8 M_K^2 M_{\pi}^2 s_{\theta}^8 g_1 [M_{\eta'}, T]}{81 M_{\eta}^4 M_{\eta'}^4 (M_{\eta}^2 - M_{\eta'}^2)} - \frac{c_{\theta}^4 M_0^8 M_{\pi}^4 s_{\theta}^8 g_1 [M_{\eta'}, T]}{81 M_{\eta}^4 M_{\eta'}^4 (M_{\eta}^2 - M_{\eta'}^2)} - \\
& \frac{176 c_{\theta}^4 M_0^8 M_K^4 s_{\theta}^8 g_1 [M_{\eta'}, T]}{243 M_{\eta}^6 M_{\eta'}^2 (M_{\eta}^2 - M_{\eta'}^2)} + \frac{148 c_{\theta}^4 M_0^8 M_K^2 M_{\pi}^2 s_{\theta}^8 g_1 [M_{\eta'}, T]}{243 M_{\eta}^6 M_{\eta'}^2 (M_{\eta}^2 - M_{\eta'}^2)} - \frac{26 c_{\theta}^4 M_0^8 M_{\pi}^4 s_{\theta}^8 g_1 [M_{\eta'}, T]}{243 M_{\eta}^6 M_{\eta'}^2 (M_{\eta}^2 - M_{\eta'}^2)} - \\
& \frac{208 \sqrt{2} c_{\theta}^3 M_0^8 M_K^4 s_{\theta}^9 g_1 [M_{\eta'}, T]}{729 M_{\eta}^{10}} + \frac{92 \sqrt{2} c_{\theta}^3 M_0^8 M_K^2 M_{\pi}^2 s_{\theta}^9 g_1 [M_{\eta'}, T]}{729 M_{\eta}^{10}} - \\
& \frac{10 \sqrt{2} c_{\theta}^3 M_0^8 M_{\pi}^4 s_{\theta}^9 g_1 [M_{\eta'}, T]}{729 M_{\eta}^{10}} + \frac{2 \sqrt{2} c_{\theta}^3 M_0^8 M_K^2 s_{\theta}^9 g_1 [M_{\eta'}, T]}{81 M_{\eta}^8} - \frac{\sqrt{2} c_{\theta}^3 M_0^8 M_{\pi}^2 s_{\theta}^9 g_1 [M_{\eta'}, T]}{81 M_{\eta}^8} + \\
& \frac{256 \sqrt{2} c_{\theta}^3 M_0^8 M_K^4 s_{\theta}^9 g_1 [M_{\eta'}, T]}{729 M_{\eta}^2 M_{\eta'}^8} - \frac{272 \sqrt{2} c_{\theta}^3 M_0^8 M_K^2 M_{\pi}^2 s_{\theta}^9 g_1 [M_{\eta'}, T]}{729 M_{\eta}^2 M_{\eta'}^8} + \\
& \frac{70 \sqrt{2} c_{\theta}^3 M_0^8 M_{\pi}^4 s_{\theta}^9 g_1 [M_{\eta'}, T]}{729 M_{\eta}^2 M_{\eta'}^8} + \frac{512 \sqrt{2} c_{\theta}^3 M_0^8 M_K^4 s_{\theta}^9 g_1 [M_{\eta'}, T]}{729 M_{\eta}^4 M_{\eta'}^6} - \\
& \frac{412 \sqrt{2} c_{\theta}^3 M_0^8 M_K^2 M_{\pi}^2 s_{\theta}^9 g_1 [M_{\eta'}, T]}{729 M_{\eta}^4 M_{\eta'}^6} + \frac{44 \sqrt{2} c_{\theta}^3 M_0^8 M_{\pi}^4 s_{\theta}^9 g_1 [M_{\eta'}, T]}{729 M_{\eta}^4 M_{\eta'}^6} - \\
& \frac{896 \sqrt{2} c_{\theta}^3 M_0^8 M_K^4 s_{\theta}^9 g_1 [M_{\eta'}, T]}{729 M_{\eta}^6 M_{\eta'}^4} + \frac{652 \sqrt{2} c_{\theta}^3 M_0^8 M_K^2 M_{\pi}^2 s_{\theta}^9 g_1 [M_{\eta'}, T]}{729 M_{\eta}^6 M_{\eta'}^4} - \\
& \frac{152 \sqrt{2} c_{\theta}^3 M_0^8 M_{\pi}^4 s_{\theta}^9 g_1 [M_{\eta'}, T]}{729 M_{\eta}^6 M_{\eta'}^4} + \frac{64 \sqrt{2} c_{\theta}^3 M_0^8 M_K^4 s_{\theta}^9 g_1 [M_{\eta'}, T]}{81 M_{\eta}^8 M_{\eta'}^2} - \\
& \frac{100 \sqrt{2} c_{\theta}^3 M_0^8 M_K^2 M_{\pi}^2 s_{\theta}^9 g_1 [M_{\eta'}, T]}{243 M_{\eta}^8 M_{\eta'}^2} + \frac{16 \sqrt{2} c_{\theta}^3 M_0^8 M_{\pi}^4 s_{\theta}^9 g_1 [M_{\eta'}, T]}{243 M_{\eta}^8 M_{\eta'}^2} - \\
& \frac{8 \sqrt{2} c_{\theta}^3 M_0^8 M_K^2 s_{\theta}^9 g_1 [M_{\eta'}, T]}{243 M_{\eta}^6 M_{\eta'}^2} + \frac{5 \sqrt{2} c_{\theta}^3 M_0^8 M_{\pi}^2 s_{\theta}^9 g_1 [M_{\eta'}, T]}{243 M_{\eta}^6 M_{\eta'}^2} - \frac{104 \sqrt{2} c_{\theta}^3 M_0^8 M_K^4 s_{\theta}^9 g_1 [M_{\eta'}, T]}{243 M_{\eta}^8 (M_{\eta}^2 - M_{\eta'}^2)} + \\
& \frac{64 \sqrt{2} c_{\theta}^3 M_0^8 M_K^2 M_{\pi}^2 s_{\theta}^9 g_1 [M_{\eta'}, T]}{243 M_{\eta}^8 (M_{\eta}^2 - M_{\eta'}^2)} - \frac{14 \sqrt{2} c_{\theta}^3 M_0^8 M_{\pi}^4 s_{\theta}^9 g_1 [M_{\eta'}, T]}{243 M_{\eta}^8 (M_{\eta}^2 - M_{\eta'}^2)} + \\
& \frac{64 \sqrt{2} c_{\theta}^3 M_0^8 M_K^4 s_{\theta}^9 g_1 [M_{\eta'}, T]}{243 M_{\eta}^2 M_{\eta'}^6 (M_{\eta}^2 - M_{\eta'}^2)} - \frac{56 \sqrt{2} c_{\theta}^3 M_0^8 M_K^2 M_{\pi}^2 s_{\theta}^9 g_1 [M_{\eta'}, T]}{243 M_{\eta}^2 M_{\eta'}^6 (M_{\eta}^2 - M_{\eta'}^2)} +
\end{aligned}$$

$$\begin{aligned}
& \frac{10 \sqrt{2} c_{\theta}^3 M_0^8 M_{\pi}^4 s_{\theta}^9 g_1 [M_{\eta'}, T]}{243 M_{\eta}^2 M_{\eta'}^6 (M_{\eta}^2 - M_{\eta'}^2)} - \frac{64 \sqrt{2} c_{\theta}^3 M_0^8 M_K^4 s_{\theta}^9 g_1 [M_{\eta'}, T]}{81 M_{\eta}^4 M_{\eta'}^4 (M_{\eta}^2 - M_{\eta'}^2)} + \\
& \frac{44 \sqrt{2} c_{\theta}^3 M_0^8 M_K^2 M_{\pi}^2 s_{\theta}^9 g_1 [M_{\eta'}, T]}{81 M_{\eta}^4 M_{\eta'}^4 (M_{\eta}^2 - M_{\eta'}^2)} - \frac{10 \sqrt{2} c_{\theta}^3 M_0^8 M_{\pi}^4 s_{\theta}^9 g_1 [M_{\eta'}, T]}{81 M_{\eta}^4 M_{\eta'}^4 (M_{\eta}^2 - M_{\eta'}^2)} + \\
& \frac{208 \sqrt{2} c_{\theta}^3 M_0^8 M_K^4 s_{\theta}^9 g_1 [M_{\eta'}, T]}{243 M_{\eta}^6 M_{\eta'}^2 (M_{\eta}^2 - M_{\eta'}^2)} - \frac{92 \sqrt{2} c_{\theta}^3 M_0^8 M_K^2 M_{\pi}^2 s_{\theta}^9 g_1 [M_{\eta'}, T]}{243 M_{\eta}^6 M_{\eta'}^2 (M_{\eta}^2 - M_{\eta'}^2)} + \\
& \frac{10 \sqrt{2} c_{\theta}^3 M_0^8 M_{\pi}^4 s_{\theta}^9 g_1 [M_{\eta'}, T]}{243 M_{\eta}^6 M_{\eta'}^2 (M_{\eta}^2 - M_{\eta'}^2)} - \frac{296 c_{\theta}^2 M_0^8 M_K^4 s_{\theta}^{10} g_1 [M_{\eta'}, T]}{729 M_{\eta}^{10}} + \frac{262 c_{\theta}^2 M_0^8 M_K^2 M_{\pi}^2 s_{\theta}^{10} g_1 [M_{\eta'}, T]}{729 M_{\eta}^{10}} - \\
& \frac{47 c_{\theta}^2 M_0^8 M_{\pi}^4 s_{\theta}^{10} g_1 [M_{\eta'}, T]}{729 M_{\eta}^{10}} + \frac{2 M_0^8 M_K^2 s_{\theta}^{10} g_1 [M_{\eta'}, T]}{243 M_{\eta}^8} - \frac{M_0^8 M_{\pi}^2 s_{\theta}^{10} g_1 [M_{\eta'}, T]}{486 M_{\eta}^8} - \\
& \frac{128 c_{\theta}^2 M_0^8 M_K^4 s_{\theta}^{10} g_1 [M_{\eta'}, T]}{243 M_{\eta}^4 M_{\eta'}^6} + \frac{124 c_{\theta}^2 M_0^8 M_K^2 M_{\pi}^2 s_{\theta}^{10} g_1 [M_{\eta'}, T]}{243 M_{\eta}^4 M_{\eta'}^6} - \frac{32 c_{\theta}^2 M_0^8 M_{\pi}^4 s_{\theta}^{10} g_1 [M_{\eta'}, T]}{243 M_{\eta}^4 M_{\eta'}^6} - \\
& \frac{64 c_{\theta}^2 M_0^8 M_K^4 s_{\theta}^{10} g_1 [M_{\eta'}, T]}{729 M_{\eta}^6 M_{\eta'}^4} + \frac{122 c_{\theta}^2 M_0^8 M_K^2 M_{\pi}^2 s_{\theta}^{10} g_1 [M_{\eta'}, T]}{729 M_{\eta}^6 M_{\eta'}^4} - \frac{85 c_{\theta}^2 M_0^8 M_{\pi}^4 s_{\theta}^{10} g_1 [M_{\eta'}, T]}{729 M_{\eta}^6 M_{\eta'}^4} + \\
& \frac{160 c_{\theta}^2 M_0^8 M_K^4 s_{\theta}^{10} g_1 [M_{\eta'}, T]}{243 M_{\eta}^8 M_{\eta'}^2} - \frac{164 c_{\theta}^2 M_0^8 M_K^2 M_{\pi}^2 s_{\theta}^{10} g_1 [M_{\eta'}, T]}{243 M_{\eta}^8 M_{\eta'}^2} + \frac{40 c_{\theta}^2 M_0^8 M_{\pi}^4 s_{\theta}^{10} g_1 [M_{\eta'}, T]}{243 M_{\eta}^8 M_{\eta'}^2} - \\
& \frac{148 c_{\theta}^2 M_0^8 M_K^4 s_{\theta}^{10} g_1 [M_{\eta'}, T]}{243 M_{\eta}^8 (M_{\eta}^2 - M_{\eta'}^2)} + \frac{140 c_{\theta}^2 M_0^8 M_K^2 M_{\pi}^2 s_{\theta}^{10} g_1 [M_{\eta'}, T]}{243 M_{\eta}^8 (M_{\eta}^2 - M_{\eta'}^2)} - \frac{28 c_{\theta}^2 M_0^8 M_{\pi}^4 s_{\theta}^{10} g_1 [M_{\eta'}, T]}{243 M_{\eta}^8 (M_{\eta}^2 - M_{\eta'}^2)} - \\
& \frac{32 c_{\theta}^2 M_0^8 M_K^4 s_{\theta}^{10} g_1 [M_{\eta'}, T]}{81 M_{\eta}^4 M_{\eta'}^4 (M_{\eta}^2 - M_{\eta'}^2)} + \frac{28 c_{\theta}^2 M_0^8 M_K^2 M_{\pi}^2 s_{\theta}^{10} g_1 [M_{\eta'}, T]}{81 M_{\eta}^4 M_{\eta'}^4 (M_{\eta}^2 - M_{\eta'}^2)} - \frac{8 c_{\theta}^2 M_0^8 M_{\pi}^4 s_{\theta}^{10} g_1 [M_{\eta'}, T]}{81 M_{\eta}^4 M_{\eta'}^4 (M_{\eta}^2 - M_{\eta'}^2)} + \\
& \frac{224 c_{\theta}^2 M_0^8 M_K^4 s_{\theta}^{10} g_1 [M_{\eta'}, T]}{243 M_{\eta}^6 M_{\eta'}^2 (M_{\eta}^2 - M_{\eta'}^2)} - \frac{184 c_{\theta}^2 M_0^8 M_K^2 M_{\pi}^2 s_{\theta}^{10} g_1 [M_{\eta'}, T]}{243 M_{\eta}^6 M_{\eta'}^2 (M_{\eta}^2 - M_{\eta'}^2)} + \frac{32 c_{\theta}^2 M_0^8 M_{\pi}^4 s_{\theta}^{10} g_1 [M_{\eta'}, T]}{243 M_{\eta}^6 M_{\eta'}^2 (M_{\eta}^2 - M_{\eta'}^2)} - \\
& \frac{80 \sqrt{2} c_{\theta} M_0^8 M_K^4 s_{\theta}^{11} g_1 [M_{\eta'}, T]}{729 M_{\eta}^{10}} + \frac{76 \sqrt{2} c_{\theta} M_0^8 M_K^2 M_{\pi}^2 s_{\theta}^{11} g_1 [M_{\eta'}, T]}{729 M_{\eta}^{10}} - \\
& \frac{14 \sqrt{2} c_{\theta} M_0^8 M_{\pi}^4 s_{\theta}^{11} g_1 [M_{\eta'}, T]}{729 M_{\eta}^{10}} + \frac{128 \sqrt{2} c_{\theta} M_0^8 M_K^4 s_{\theta}^{11} g_1 [M_{\eta'}, T]}{729 M_{\eta}^6 M_{\eta'}^4} - \\
& \frac{130 \sqrt{2} c_{\theta} M_0^8 M_K^2 M_{\pi}^2 s_{\theta}^{11} g_1 [M_{\eta'}, T]}{729 M_{\eta}^6 M_{\eta'}^4} + \frac{29 \sqrt{2} c_{\theta} M_0^8 M_{\pi}^4 s_{\theta}^{11} g_1 [M_{\eta'}, T]}{729 M_{\eta}^6 M_{\eta'}^4} + \\
& \frac{2 \sqrt{2} c_{\theta} M_0^8 M_K^2 M_{\pi}^2 s_{\theta}^{11} g_1 [M_{\eta'}, T]}{243 M_{\eta}^8 M_{\eta'}^2} - \frac{5 \sqrt{2} c_{\theta} M_0^8 M_{\pi}^4 s_{\theta}^{11} g_1 [M_{\eta'}, T]}{243 M_{\eta}^8 M_{\eta'}^2} - \\
& \frac{40 \sqrt{2} c_{\theta} M_0^8 M_K^4 s_{\theta}^{11} g_1 [M_{\eta'}, T]}{243 M_{\eta}^8 (M_{\eta}^2 - M_{\eta'}^2)} + \frac{56 \sqrt{2} c_{\theta} M_0^8 M_K^2 M_{\pi}^2 s_{\theta}^{11} g_1 [M_{\eta'}, T]}{243 M_{\eta}^8 (M_{\eta}^2 - M_{\eta'}^2)} -
\end{aligned}$$

$$\begin{aligned}
& \frac{16 \sqrt{2} c_{\theta} M_0^8 M_{\pi}^4 s_{\theta}^{11} g_1 [M_{\eta'}, T]}{243 M_{\eta}^8 (M_{\eta}^2 - M_{\eta'}^2)} + \frac{32 \sqrt{2} c_{\theta} M_0^8 M_K^4 s_{\theta}^{11} g_1 [M_{\eta'}, T]}{243 M_{\eta}^6 M_{\eta'}^2 (M_{\eta}^2 - M_{\eta'}^2)} - \\
& \frac{40 \sqrt{2} c_{\theta} M_0^8 M_K^2 M_{\pi}^2 s_{\theta}^{11} g_1 [M_{\eta'}, T]}{243 M_{\eta}^6 M_{\eta'}^2 (M_{\eta}^2 - M_{\eta'}^2)} + \frac{8 \sqrt{2} c_{\theta} M_0^8 M_{\pi}^4 s_{\theta}^{11} g_1 [M_{\eta'}, T]}{243 M_{\eta}^6 M_{\eta'}^2 (M_{\eta}^2 - M_{\eta'}^2)} - \\
& \frac{16 M_0^8 M_K^4 s_{\theta}^{12} g_1 [M_{\eta'}, T]}{729 M_{\eta}^{10}} - \frac{4 M_0^8 M_K^2 M_{\pi}^2 s_{\theta}^{12} g_1 [M_{\eta'}, T]}{729 M_{\eta}^{10}} + \frac{2 M_0^8 M_{\pi}^4 s_{\theta}^{12} g_1 [M_{\eta'}, T]}{729 M_{\eta}^{10}} - \\
& \frac{32 M_0^8 M_K^4 s_{\theta}^{12} g_1 [M_{\eta'}, T]}{729 M_{\eta}^8 M_{\eta'}^2} + \frac{52 M_0^8 M_K^2 M_{\pi}^2 s_{\theta}^{12} g_1 [M_{\eta'}, T]}{729 M_{\eta}^8 M_{\eta'}^2} - \frac{20 M_0^8 M_{\pi}^4 s_{\theta}^{12} g_1 [M_{\eta'}, T]}{729 M_{\eta}^8 M_{\eta'}^2} - \\
& \frac{8 M_0^8 M_K^4 s_{\theta}^{12} g_1 [M_{\eta'}, T]}{243 M_{\eta}^8 (M_{\eta}^2 - M_{\eta'}^2)} + \frac{16 M_0^8 M_K^2 M_{\pi}^2 s_{\theta}^{12} g_1 [M_{\eta'}, T]}{243 M_{\eta}^8 (M_{\eta}^2 - M_{\eta'}^2)} - \frac{8 M_0^8 M_{\pi}^4 s_{\theta}^{12} g_1 [M_{\eta'}, T]}{243 M_{\eta}^8 (M_{\eta}^2 - M_{\eta'}^2)} - \\
& \frac{2 c_{\theta}^8 M_0^8 M_K^4 g_2 [M_K, T]}{27 M_{\eta'}^8} + \frac{4 \sqrt{2} c_{\theta}^7 M_0^8 M_K^4 s_{\theta} g_2 [M_K, T]}{27 M_{\eta'}^8} - \frac{2 \sqrt{2} c_{\theta}^7 M_0^8 M_K^2 M_{\pi}^2 s_{\theta} g_2 [M_K, T]}{27 M_{\eta'}^8} - \\
& \frac{4 \sqrt{2} c_{\theta}^7 M_0^8 M_K^4 s_{\theta} g_2 [M_K, T]}{27 M_{\eta}^2 M_{\eta'}^6} + \frac{2 \sqrt{2} c_{\theta}^7 M_0^8 M_K^2 M_{\pi}^2 s_{\theta} g_2 [M_K, T]}{27 M_{\eta}^2 M_{\eta'}^6} - \frac{4 c_{\theta}^6 M_0^8 M_K^4 s_{\theta}^2 g_2 [M_K, T]}{27 M_{\eta'}^8} + \\
& \frac{5 c_{\theta}^6 M_0^8 M_K^2 M_{\pi}^2 s_{\theta}^2 g_2 [M_K, T]}{27 M_{\eta'}^8} - \frac{c_{\theta}^6 M_0^8 M_{\pi}^4 s_{\theta}^2 g_2 [M_K, T]}{27 M_{\eta'}^8} - \frac{10 c_{\theta}^6 M_0^8 M_K^2 M_{\pi}^2 s_{\theta}^2 g_2 [M_K, T]}{27 M_{\eta}^2 M_{\eta'}^6} + \\
& \frac{2 c_{\theta}^6 M_0^8 M_{\pi}^4 s_{\theta}^2 g_2 [M_K, T]}{27 M_{\eta}^2 M_{\eta'}^6} - \frac{4 c_{\theta}^6 M_0^8 M_K^4 s_{\theta}^2 g_2 [M_K, T]}{27 M_{\eta}^4 M_{\eta'}^4} + \frac{5 c_{\theta}^6 M_0^8 M_K^2 M_{\pi}^2 s_{\theta}^2 g_2 [M_K, T]}{27 M_{\eta}^4 M_{\eta'}^4} - \\
& \frac{c_{\theta}^6 M_0^8 M_{\pi}^4 s_{\theta}^2 g_2 [M_K, T]}{27 M_{\eta}^4 M_{\eta'}^4} - \frac{\sqrt{2} c_{\theta}^5 M_0^8 M_K^2 M_{\pi}^2 s_{\theta}^3 g_2 [M_K, T]}{27 M_{\eta'}^8} + \frac{c_{\theta}^5 M_0^8 M_{\pi}^4 s_{\theta}^3 g_2 [M_K, T]}{27 \sqrt{2} M_{\eta'}^8} + \\
& \frac{4 \sqrt{2} c_{\theta}^5 M_0^8 M_K^4 s_{\theta}^3 g_2 [M_K, T]}{9 M_{\eta}^2 M_{\eta'}^6} - \frac{\sqrt{2} c_{\theta}^5 M_0^8 M_K^2 M_{\pi}^2 s_{\theta}^3 g_2 [M_K, T]}{9 M_{\eta}^2 M_{\eta'}^6} - \frac{c_{\theta}^5 M_0^8 M_{\pi}^4 s_{\theta}^3 g_2 [M_K, T]}{9 \sqrt{2} M_{\eta}^2 M_{\eta'}^6} - \\
& \frac{4 \sqrt{2} c_{\theta}^5 M_0^8 M_K^4 s_{\theta}^3 g_2 [M_K, T]}{9 M_{\eta}^4 M_{\eta'}^4} + \frac{\sqrt{2} c_{\theta}^5 M_0^8 M_K^2 M_{\pi}^2 s_{\theta}^3 g_2 [M_K, T]}{9 M_{\eta}^4 M_{\eta'}^4} + \frac{c_{\theta}^5 M_0^8 M_{\pi}^4 s_{\theta}^3 g_2 [M_K, T]}{9 \sqrt{2} M_{\eta}^4 M_{\eta'}^4} + \\
& \frac{\sqrt{2} c_{\theta}^5 M_0^8 M_K^2 M_{\pi}^2 s_{\theta}^3 g_2 [M_K, T]}{27 M_{\eta}^6 M_{\eta'}^2} - \frac{c_{\theta}^5 M_0^8 M_{\pi}^4 s_{\theta}^3 g_2 [M_K, T]}{27 \sqrt{2} M_{\eta}^6 M_{\eta'}^2} - \frac{c_{\theta}^4 M_0^8 M_{\pi}^4 s_{\theta}^4 g_2 [M_K, T]}{216 M_{\eta}^8} - \\
& \frac{c_{\theta}^4 M_0^8 M_{\pi}^4 s_{\theta}^4 g_2 [M_K, T]}{216 M_{\eta'}^8} - \frac{8 c_{\theta}^4 M_0^8 M_K^4 s_{\theta}^4 g_2 [M_K, T]}{27 M_{\eta}^2 M_{\eta'}^6} + \frac{10 c_{\theta}^4 M_0^8 M_K^2 M_{\pi}^2 s_{\theta}^4 g_2 [M_K, T]}{27 M_{\eta}^2 M_{\eta'}^6} - \\
& \frac{c_{\theta}^4 M_0^8 M_{\pi}^4 s_{\theta}^4 g_2 [M_K, T]}{18 M_{\eta}^2 M_{\eta'}^6} + \frac{4 c_{\theta}^4 M_0^8 M_K^4 s_{\theta}^4 g_2 [M_K, T]}{27 M_{\eta}^4 M_{\eta'}^4} - \frac{20 c_{\theta}^4 M_0^8 M_K^2 M_{\pi}^2 s_{\theta}^4 g_2 [M_K, T]}{27 M_{\eta}^4 M_{\eta'}^4} + \\
& \frac{13 c_{\theta}^4 M_0^8 M_{\pi}^4 s_{\theta}^4 g_2 [M_K, T]}{108 M_{\eta}^4 M_{\eta'}^4} - \frac{8 c_{\theta}^4 M_0^8 M_K^4 s_{\theta}^4 g_2 [M_K, T]}{27 M_{\eta}^6 M_{\eta'}^2} + \frac{10 c_{\theta}^4 M_0^8 M_K^2 M_{\pi}^2 s_{\theta}^4 g_2 [M_K, T]}{27 M_{\eta}^6 M_{\eta'}^2} -
\end{aligned}$$



$$\begin{aligned}
& \frac{c_\theta^4 M_0^8 M_\pi^4 s_\theta^4 g_2 [M_K, T]}{18 M_\eta^6 M_{\eta'}^2} + \frac{\sqrt{2} c_\theta^3 M_0^8 M_K^2 M_\pi^2 s_\theta^5 g_2 [M_K, T]}{27 M_\eta^8} - \frac{c_\theta^3 M_0^8 M_\pi^4 s_\theta^5 g_2 [M_K, T]}{27 \sqrt{2} M_\eta^8} - \\
& \frac{\sqrt{2} c_\theta^3 M_0^8 M_K^2 M_\pi^2 s_\theta^5 g_2 [M_K, T]}{27 M_\eta^2 M_{\eta'}^6} + \frac{c_\theta^3 M_0^8 M_\pi^4 s_\theta^5 g_2 [M_K, T]}{27 \sqrt{2} M_\eta^2 M_{\eta'}^6} + \frac{4 \sqrt{2} c_\theta^3 M_0^8 M_K^4 s_\theta^5 g_2 [M_K, T]}{9 M_\eta^4 M_{\eta'}^4} - \\
& \frac{\sqrt{2} c_\theta^3 M_0^8 M_K^2 M_\pi^2 s_\theta^5 g_2 [M_K, T]}{9 M_\eta^4 M_{\eta'}^4} - \frac{c_\theta^3 M_0^8 M_\pi^4 s_\theta^5 g_2 [M_K, T]}{9 \sqrt{2} M_\eta^4 M_{\eta'}^4} - \frac{4 \sqrt{2} c_\theta^3 M_0^8 M_K^4 s_\theta^5 g_2 [M_K, T]}{9 M_\eta^6 M_{\eta'}^2} + \\
& \frac{\sqrt{2} c_\theta^3 M_0^8 M_K^2 M_\pi^2 s_\theta^5 g_2 [M_K, T]}{9 M_\eta^6 M_{\eta'}^2} + \frac{c_\theta^3 M_0^8 M_\pi^4 s_\theta^5 g_2 [M_K, T]}{9 \sqrt{2} M_\eta^6 M_{\eta'}^2} - \frac{4 c_\theta^2 M_0^8 M_K^4 s_\theta^6 g_2 [M_K, T]}{27 M_\eta^8} + \\
& \frac{5 c_\theta^2 M_0^8 M_K^2 M_\pi^2 s_\theta^6 g_2 [M_K, T]}{27 M_\eta^8} - \frac{c_\theta^2 M_0^8 M_\pi^4 s_\theta^6 g_2 [M_K, T]}{27 M_\eta^8} - \frac{4 c_\theta^2 M_0^8 M_K^4 s_\theta^6 g_2 [M_K, T]}{27 M_\eta^4 M_{\eta'}^4} + \\
& \frac{5 c_\theta^2 M_0^8 M_K^2 M_\pi^2 s_\theta^6 g_2 [M_K, T]}{27 M_\eta^4 M_{\eta'}^4} - \frac{c_\theta^2 M_0^8 M_\pi^4 s_\theta^6 g_2 [M_K, T]}{27 M_\eta^4 M_{\eta'}^4} - \frac{10 c_\theta^2 M_0^8 M_K^2 M_\pi^2 s_\theta^6 g_2 [M_K, T]}{27 M_\eta^6 M_{\eta'}^2} + \\
& \frac{2 c_\theta^2 M_0^8 M_\pi^4 s_\theta^6 g_2 [M_K, T]}{27 M_\eta^6 M_{\eta'}^2} - \frac{4 \sqrt{2} c_\theta M_0^8 M_K^4 s_\theta^7 g_2 [M_K, T]}{27 M_\eta^8} + \frac{2 \sqrt{2} c_\theta M_0^8 M_K^2 M_\pi^2 s_\theta^7 g_2 [M_K, T]}{27 M_\eta^8} + \\
& \frac{4 \sqrt{2} c_\theta M_0^8 M_K^4 s_\theta^7 g_2 [M_K, T]}{27 M_\eta^6 M_{\eta'}^2} - \frac{2 \sqrt{2} c_\theta M_0^8 M_K^2 M_\pi^2 s_\theta^7 g_2 [M_K, T]}{27 M_\eta^6 M_{\eta'}^2} - \frac{2 M_0^8 M_K^4 s_\theta^8 g_2 [M_K, T]}{27 M_\eta^8} - \\
& \frac{c_\theta^8 M_0^8 M_\pi^4 g_2 [M_\pi, T]}{18 M_{\eta'}^8} - \frac{\sqrt{2} c_\theta^7 M_0^8 M_\pi^4 s_\theta g_2 [M_\pi, T]}{9 M_{\eta'}^8} + \frac{\sqrt{2} c_\theta^7 M_0^8 M_\pi^4 s_\theta g_2 [M_\pi, T]}{9 M_\eta^2 M_{\eta'}^6} - \\
& \frac{c_\theta^6 M_0^8 M_\pi^4 s_\theta^2 g_2 [M_\pi, T]}{6 M_{\eta'}^8} + \frac{c_\theta^6 M_0^8 M_\pi^4 s_\theta^2 g_2 [M_\pi, T]}{9 M_\eta^2 M_{\eta'}^6} - \frac{c_\theta^6 M_0^8 M_\pi^4 s_\theta^2 g_2 [M_\pi, T]}{6 M_\eta^4 M_{\eta'}^4} - \frac{c_\theta^5 M_0^8 M_\pi^4 s_\theta^3 g_2 [M_\pi, T]}{9 \sqrt{2} M_{\eta'}^8} - \\
& \frac{c_\theta^5 M_0^8 M_\pi^4 s_\theta^3 g_2 [M_\pi, T]}{3 \sqrt{2} M_\eta^2 M_{\eta'}^6} + \frac{c_\theta^5 M_0^8 M_\pi^4 s_\theta^3 g_2 [M_\pi, T]}{3 \sqrt{2} M_\eta^4 M_{\eta'}^4} + \frac{c_\theta^5 M_0^8 M_\pi^4 s_\theta^3 g_2 [M_\pi, T]}{9 \sqrt{2} M_\eta^6 M_{\eta'}^2} - \frac{c_\theta^4 M_0^8 M_\pi^4 s_\theta^4 g_2 [M_\pi, T]}{72 M_\eta^8} - \\
& \frac{c_\theta^4 M_0^8 M_\pi^4 s_\theta^4 g_2 [M_\pi, T]}{72 M_{\eta'}^8} - \frac{5 c_\theta^4 M_0^8 M_\pi^4 s_\theta^4 g_2 [M_\pi, T]}{18 M_\eta^2 M_{\eta'}^6} + \frac{c_\theta^4 M_0^8 M_\pi^4 s_\theta^4 g_2 [M_\pi, T]}{4 M_\eta^4 M_{\eta'}^4} - \\
& \frac{5 c_\theta^4 M_0^8 M_\pi^4 s_\theta^4 g_2 [M_\pi, T]}{18 M_\eta^6 M_{\eta'}^2} + \frac{c_\theta^3 M_0^8 M_\pi^4 s_\theta^5 g_2 [M_\pi, T]}{9 \sqrt{2} M_\eta^8} - \frac{c_\theta^3 M_0^8 M_\pi^4 s_\theta^5 g_2 [M_\pi, T]}{9 \sqrt{2} M_\eta^2 M_{\eta'}^6} - \\
& \frac{c_\theta^3 M_0^8 M_\pi^4 s_\theta^5 g_2 [M_\pi, T]}{3 \sqrt{2} M_\eta^4 M_{\eta'}^4} + \frac{c_\theta^3 M_0^8 M_\pi^4 s_\theta^5 g_2 [M_\pi, T]}{3 \sqrt{2} M_\eta^6 M_{\eta'}^2} - \frac{c_\theta^2 M_0^8 M_\pi^4 s_\theta^6 g_2 [M_\pi, T]}{6 M_\eta^8} - \\
& \frac{c_\theta^2 M_0^8 M_\pi^4 s_\theta^6 g_2 [M_\pi, T]}{6 M_\eta^4 M_{\eta'}^4} + \frac{c_\theta^2 M_0^8 M_\pi^4 s_\theta^6 g_2 [M_\pi, T]}{9 M_\eta^6 M_{\eta'}^2} + \frac{\sqrt{2} c_\theta M_0^8 M_\pi^4 s_\theta^7 g_2 [M_\pi, T]}{9 M_\eta^8} - \\
& \frac{\sqrt{2} c_\theta M_0^8 M_\pi^4 s_\theta^7 g_2 [M_\pi, T]}{9 M_\eta^6 M_{\eta'}^2} - \frac{M_0^8 M_\pi^4 s_\theta^8 g_2 [M_\pi, T]}{18 M_\eta^8} - \frac{8 c_\theta^{12} M_0^8 M_K^4 g_2 [M_\eta, T]}{243 M_{\eta'}^8} +
\end{aligned}$$

$$\begin{aligned}
& \frac{4 c_{\theta}^{12} M_0^8 M_K^2 M_{\pi}^2 g_2 [M_{\eta}, T]}{243 M_{\eta'}^8} - \frac{c_{\theta}^{12} M_0^8 M_{\pi}^4 g_2 [M_{\eta}, T]}{486 M_{\eta'}^8} + \frac{16 \sqrt{2} c_{\theta}^{11} M_0^8 M_K^4 s_{\theta} g_2 [M_{\eta}, T]}{243 M_{\eta'}^8} - \\
& \frac{8 \sqrt{2} c_{\theta}^{11} M_0^8 M_K^2 M_{\pi}^2 s_{\theta} g_2 [M_{\eta}, T]}{243 M_{\eta'}^8} + \frac{\sqrt{2} c_{\theta}^{11} M_0^8 M_{\pi}^4 s_{\theta} g_2 [M_{\eta}, T]}{243 M_{\eta'}^8} - \frac{32 \sqrt{2} c_{\theta}^{11} M_0^8 M_K^4 s_{\theta} g_2 [M_{\eta}, T]}{243 M_{\eta'}^2 M_{\eta'}^6} + \\
& \frac{28 \sqrt{2} c_{\theta}^{11} M_0^8 M_K^2 M_{\pi}^2 s_{\theta} g_2 [M_{\eta}, T]}{243 M_{\eta'}^2 M_{\eta'}^6} - \frac{5 \sqrt{2} c_{\theta}^{11} M_0^8 M_{\pi}^4 s_{\theta} g_2 [M_{\eta}, T]}{243 M_{\eta'}^2 M_{\eta'}^6} + \frac{8 c_{\theta}^{10} M_0^8 M_K^4 s_{\theta}^2 g_2 [M_{\eta}, T]}{243 M_{\eta'}^8} - \\
& \frac{4 c_{\theta}^{10} M_0^8 M_K^2 M_{\pi}^2 s_{\theta}^2 g_2 [M_{\eta}, T]}{243 M_{\eta'}^8} + \frac{c_{\theta}^{10} M_0^8 M_{\pi}^4 s_{\theta}^2 g_2 [M_{\eta}, T]}{486 M_{\eta'}^8} + \frac{32 c_{\theta}^{10} M_0^8 M_K^4 s_{\theta}^2 g_2 [M_{\eta}, T]}{243 M_{\eta'}^2 M_{\eta'}^6} - \\
& \frac{52 c_{\theta}^{10} M_0^8 M_K^2 M_{\pi}^2 s_{\theta}^2 g_2 [M_{\eta}, T]}{243 M_{\eta'}^2 M_{\eta'}^6} + \frac{11 c_{\theta}^{10} M_0^8 M_{\pi}^4 s_{\theta}^2 g_2 [M_{\eta}, T]}{243 M_{\eta'}^2 M_{\eta'}^6} - \frac{32 c_{\theta}^{10} M_0^8 M_K^4 s_{\theta}^2 g_2 [M_{\eta}, T]}{81 M_{\eta'}^4 M_{\eta'}^4} + \\
& \frac{34 c_{\theta}^{10} M_0^8 M_K^2 M_{\pi}^2 s_{\theta}^2 g_2 [M_{\eta}, T]}{81 M_{\eta'}^4 M_{\eta'}^4} - \frac{19 c_{\theta}^{10} M_0^8 M_{\pi}^4 s_{\theta}^2 g_2 [M_{\eta}, T]}{162 M_{\eta'}^4 M_{\eta'}^4} - \frac{40 \sqrt{2} c_{\theta}^9 M_0^8 M_K^4 s_{\theta}^3 g_2 [M_{\eta}, T]}{243 M_{\eta'}^8} + \\
& \frac{20 \sqrt{2} c_{\theta}^9 M_0^8 M_K^2 M_{\pi}^2 s_{\theta}^3 g_2 [M_{\eta}, T]}{243 M_{\eta'}^8} - \frac{5 c_{\theta}^9 M_0^8 M_{\pi}^4 s_{\theta}^3 g_2 [M_{\eta}, T]}{243 \sqrt{2} M_{\eta'}^8} + \frac{128 \sqrt{2} c_{\theta}^9 M_0^8 M_K^4 s_{\theta}^3 g_2 [M_{\eta}, T]}{243 M_{\eta'}^2 M_{\eta'}^6} - \\
& \frac{70 \sqrt{2} c_{\theta}^9 M_0^8 M_K^2 M_{\pi}^2 s_{\theta}^3 g_2 [M_{\eta}, T]}{243 M_{\eta'}^2 M_{\eta'}^6} + \frac{19 c_{\theta}^9 M_0^8 M_{\pi}^4 s_{\theta}^3 g_2 [M_{\eta}, T]}{243 \sqrt{2} M_{\eta'}^2 M_{\eta'}^6} - \frac{32 \sqrt{2} c_{\theta}^9 M_0^8 M_K^4 s_{\theta}^3 g_2 [M_{\eta}, T]}{81 M_{\eta'}^4 M_{\eta'}^4} + \\
& \frac{22 \sqrt{2} c_{\theta}^9 M_0^8 M_K^2 M_{\pi}^2 s_{\theta}^3 g_2 [M_{\eta}, T]}{81 M_{\eta'}^4 M_{\eta'}^4} - \frac{c_{\theta}^9 M_0^8 M_{\pi}^4 s_{\theta}^3 g_2 [M_{\eta}, T]}{81 \sqrt{2} M_{\eta'}^4 M_{\eta'}^4} - \frac{64 \sqrt{2} c_{\theta}^9 M_0^8 M_K^4 s_{\theta}^3 g_2 [M_{\eta}, T]}{243 M_{\eta'}^6 M_{\eta'}^2} + \\
& \frac{68 \sqrt{2} c_{\theta}^9 M_0^8 M_K^2 M_{\pi}^2 s_{\theta}^3 g_2 [M_{\eta}, T]}{243 M_{\eta'}^6 M_{\eta'}^2} - \frac{35 c_{\theta}^9 M_0^8 M_{\pi}^4 s_{\theta}^3 g_2 [M_{\eta}, T]}{243 \sqrt{2} M_{\eta'}^6 M_{\eta'}^2} - \frac{32 c_{\theta}^8 M_0^8 M_K^4 s_{\theta}^4 g_2 [M_{\eta}, T]}{243 M_{\eta'}^8} + \\
& \frac{28 c_{\theta}^8 M_0^8 M_K^2 M_{\pi}^2 s_{\theta}^4 g_2 [M_{\eta}, T]}{243 M_{\eta'}^8} - \frac{49 c_{\theta}^8 M_0^8 M_{\pi}^4 s_{\theta}^4 g_2 [M_{\eta}, T]}{1944 M_{\eta'}^8} - \frac{2 c_{\theta}^8 M_0^8 M_K^4 s_{\theta}^4 g_2 [M_{\eta}, T]}{243 M_{\eta'}^8} + \\
& \frac{c_{\theta}^8 M_0^8 M_K^2 M_{\pi}^2 s_{\theta}^4 g_2 [M_{\eta}, T]}{243 M_{\eta'}^8} - \frac{c_{\theta}^8 M_0^8 M_{\pi}^4 s_{\theta}^4 g_2 [M_{\eta}, T]}{1944 M_{\eta'}^8} - \frac{32 c_{\theta}^8 M_0^8 M_K^4 s_{\theta}^4 g_2 [M_{\eta}, T]}{243 M_{\eta'}^2 M_{\eta'}^6} + \\
& \frac{46 c_{\theta}^8 M_0^8 M_K^2 M_{\pi}^2 s_{\theta}^4 g_2 [M_{\eta}, T]}{243 M_{\eta'}^2 M_{\eta'}^6} - \frac{19 c_{\theta}^8 M_0^8 M_{\pi}^4 s_{\theta}^4 g_2 [M_{\eta}, T]}{486 M_{\eta'}^2 M_{\eta'}^6} + \frac{80 c_{\theta}^8 M_0^8 M_K^4 s_{\theta}^4 g_2 [M_{\eta}, T]}{81 M_{\eta'}^4 M_{\eta'}^4} - \\
& \frac{91 c_{\theta}^8 M_0^8 M_K^2 M_{\pi}^2 s_{\theta}^4 g_2 [M_{\eta}, T]}{81 M_{\eta'}^4 M_{\eta'}^4} + \frac{65 c_{\theta}^8 M_0^8 M_{\pi}^4 s_{\theta}^4 g_2 [M_{\eta}, T]}{324 M_{\eta'}^4 M_{\eta'}^4} - \frac{320 c_{\theta}^8 M_0^8 M_K^4 s_{\theta}^4 g_2 [M_{\eta}, T]}{243 M_{\eta'}^6 M_{\eta'}^2} + \\
& \frac{340 c_{\theta}^8 M_0^8 M_K^2 M_{\pi}^2 s_{\theta}^4 g_2 [M_{\eta}, T]}{243 M_{\eta'}^6 M_{\eta'}^2} - \frac{193 c_{\theta}^8 M_0^8 M_{\pi}^4 s_{\theta}^4 g_2 [M_{\eta}, T]}{486 M_{\eta'}^6 M_{\eta'}^2} - \frac{128 \sqrt{2} c_{\theta}^7 M_0^8 M_K^4 s_{\theta}^5 g_2 [M_{\eta}, T]}{243 M_{\eta'}^8} + \\
& \frac{136 \sqrt{2} c_{\theta}^7 M_0^8 M_K^2 M_{\pi}^2 s_{\theta}^5 g_2 [M_{\eta}, T]}{243 M_{\eta'}^8} - \frac{35 \sqrt{2} c_{\theta}^7 M_0^8 M_{\pi}^4 s_{\theta}^5 g_2 [M_{\eta}, T]}{243 M_{\eta'}^8} +
\end{aligned}$$

$$\begin{aligned}
& \frac{40 \sqrt{2} c_{\theta}^7 M_0^8 M_K^4 s_{\theta}^5 g_2 [M_{\eta}, T]}{243 M_{\eta'}^8} - \frac{20 \sqrt{2} c_{\theta}^7 M_0^8 M_K^2 M_{\pi}^2 s_{\theta}^5 g_2 [M_{\eta}, T]}{243 M_{\eta'}^8} + \frac{5 c_{\theta}^7 M_0^8 M_{\pi}^4 s_{\theta}^5 g_2 [M_{\eta}, T]}{243 \sqrt{2} M_{\eta'}^8} - \\
& \frac{200 \sqrt{2} c_{\theta}^7 M_0^8 M_K^4 s_{\theta}^5 g_2 [M_{\eta}, T]}{243 M_{\eta'}^2 M_{\eta'}^6} + \frac{100 \sqrt{2} c_{\theta}^7 M_0^8 M_K^2 M_{\pi}^2 s_{\theta}^5 g_2 [M_{\eta}, T]}{243 M_{\eta'}^2 M_{\eta'}^6} - \frac{25 c_{\theta}^7 M_0^8 M_{\pi}^4 s_{\theta}^5 g_2 [M_{\eta}, T]}{243 \sqrt{2} M_{\eta'}^2 M_{\eta'}^6} + \\
& \frac{128 \sqrt{2} c_{\theta}^7 M_0^8 M_K^4 s_{\theta}^5 g_2 [M_{\eta}, T]}{81 M_{\eta'}^4 M_{\eta'}^4} - \frac{82 \sqrt{2} c_{\theta}^7 M_0^8 M_K^2 M_{\pi}^2 s_{\theta}^5 g_2 [M_{\eta}, T]}{81 M_{\eta'}^4 M_{\eta'}^4} + \frac{31 c_{\theta}^7 M_0^8 M_{\pi}^4 s_{\theta}^5 g_2 [M_{\eta}, T]}{81 \sqrt{2} M_{\eta'}^4 M_{\eta'}^4} - \\
& \frac{224 \sqrt{2} c_{\theta}^7 M_0^8 M_K^4 s_{\theta}^5 g_2 [M_{\eta}, T]}{243 M_{\eta'}^6 M_{\eta'}^2} + \frac{166 \sqrt{2} c_{\theta}^7 M_0^8 M_K^2 M_{\pi}^2 s_{\theta}^5 g_2 [M_{\eta}, T]}{243 M_{\eta'}^6 M_{\eta'}^2} - \\
& \frac{19 c_{\theta}^7 M_0^8 M_{\pi}^4 s_{\theta}^5 g_2 [M_{\eta}, T]}{243 \sqrt{2} M_{\eta'}^6 M_{\eta'}^2} - \frac{448 c_{\theta}^6 M_0^8 M_K^4 s_{\theta}^6 g_2 [M_{\eta}, T]}{243 M_{\eta'}^8} + \frac{452 c_{\theta}^6 M_0^8 M_K^2 M_{\pi}^2 s_{\theta}^6 g_2 [M_{\eta}, T]}{243 M_{\eta'}^8} - \\
& \frac{121 c_{\theta}^6 M_0^8 M_{\pi}^4 s_{\theta}^6 g_2 [M_{\eta}, T]}{243 M_{\eta'}^8} + \frac{8 c_{\theta}^6 M_0^8 M_K^4 s_{\theta}^6 g_2 [M_{\eta}, T]}{243 M_{\eta'}^8} - \frac{4 c_{\theta}^6 M_0^8 M_K^2 M_{\pi}^2 s_{\theta}^6 g_2 [M_{\eta}, T]}{243 M_{\eta'}^8} + \\
& \frac{c_{\theta}^6 M_0^8 M_{\pi}^4 s_{\theta}^6 g_2 [M_{\eta}, T]}{486 M_{\eta'}^8} - \frac{88 c_{\theta}^6 M_0^8 M_K^4 s_{\theta}^6 g_2 [M_{\eta}, T]}{243 M_{\eta'}^2 M_{\eta'}^6} + \frac{74 c_{\theta}^6 M_0^8 M_K^2 M_{\pi}^2 s_{\theta}^6 g_2 [M_{\eta}, T]}{243 M_{\eta'}^2 M_{\eta'}^6} - \\
& \frac{13 c_{\theta}^6 M_0^8 M_{\pi}^4 s_{\theta}^6 g_2 [M_{\eta}, T]}{243 M_{\eta'}^2 M_{\eta'}^6} + \frac{40 c_{\theta}^6 M_0^8 M_K^4 s_{\theta}^6 g_2 [M_{\eta}, T]}{81 M_{\eta'}^4 M_{\eta'}^4} - \frac{32 c_{\theta}^6 M_0^8 M_K^2 M_{\pi}^2 s_{\theta}^6 g_2 [M_{\eta}, T]}{81 M_{\eta'}^4 M_{\eta'}^4} + \\
& \frac{17 c_{\theta}^6 M_0^8 M_{\pi}^4 s_{\theta}^6 g_2 [M_{\eta}, T]}{162 M_{\eta'}^4 M_{\eta'}^4} + \frac{224 c_{\theta}^6 M_0^8 M_K^4 s_{\theta}^6 g_2 [M_{\eta}, T]}{243 M_{\eta'}^6 M_{\eta'}^2} - \frac{238 c_{\theta}^6 M_0^8 M_K^2 M_{\pi}^2 s_{\theta}^6 g_2 [M_{\eta}, T]}{243 M_{\eta'}^6 M_{\eta'}^2} + \\
& \frac{14 c_{\theta}^6 M_0^8 M_{\pi}^4 s_{\theta}^6 g_2 [M_{\eta}, T]}{243 M_{\eta'}^6 M_{\eta'}^2} - \frac{448 \sqrt{2} c_{\theta}^5 M_0^8 M_K^4 s_{\theta}^7 g_2 [M_{\eta}, T]}{243 M_{\eta'}^8} + \frac{428 \sqrt{2} c_{\theta}^5 M_0^8 M_K^2 M_{\pi}^2 s_{\theta}^7 g_2 [M_{\eta}, T]}{243 M_{\eta'}^8} - \\
& \frac{88 \sqrt{2} c_{\theta}^5 M_0^8 M_{\pi}^4 s_{\theta}^7 g_2 [M_{\eta}, T]}{243 M_{\eta'}^8} - \frac{16 \sqrt{2} c_{\theta}^5 M_0^8 M_K^4 s_{\theta}^7 g_2 [M_{\eta}, T]}{243 M_{\eta'}^8} + \\
& \frac{8 \sqrt{2} c_{\theta}^5 M_0^8 M_K^2 M_{\pi}^2 s_{\theta}^7 g_2 [M_{\eta}, T]}{243 M_{\eta'}^8} - \frac{\sqrt{2} c_{\theta}^5 M_0^8 M_{\pi}^4 s_{\theta}^7 g_2 [M_{\eta}, T]}{243 M_{\eta'}^8} + \frac{104 \sqrt{2} c_{\theta}^5 M_0^8 M_K^4 s_{\theta}^7 g_2 [M_{\eta}, T]}{243 M_{\eta'}^2 M_{\eta'}^6} - \\
& \frac{46 \sqrt{2} c_{\theta}^5 M_0^8 M_K^2 M_{\pi}^2 s_{\theta}^7 g_2 [M_{\eta}, T]}{243 M_{\eta'}^2 M_{\eta'}^6} + \frac{5 \sqrt{2} c_{\theta}^5 M_0^8 M_{\pi}^4 s_{\theta}^7 g_2 [M_{\eta}, T]}{243 M_{\eta'}^2 M_{\eta'}^6} - \\
& \frac{104 \sqrt{2} c_{\theta}^5 M_0^8 M_K^4 s_{\theta}^7 g_2 [M_{\eta}, T]}{81 M_{\eta'}^4 M_{\eta'}^4} + \frac{58 \sqrt{2} c_{\theta}^5 M_0^8 M_K^2 M_{\pi}^2 s_{\theta}^7 g_2 [M_{\eta}, T]}{81 M_{\eta'}^4 M_{\eta'}^4} - \\
& \frac{11 \sqrt{2} c_{\theta}^5 M_0^8 M_{\pi}^4 s_{\theta}^7 g_2 [M_{\eta}, T]}{81 M_{\eta'}^4 M_{\eta'}^4} + \frac{560 \sqrt{2} c_{\theta}^5 M_0^8 M_K^4 s_{\theta}^7 g_2 [M_{\eta}, T]}{243 M_{\eta'}^6 M_{\eta'}^2} - \\
& \frac{460 \sqrt{2} c_{\theta}^5 M_0^8 M_K^2 M_{\pi}^2 s_{\theta}^7 g_2 [M_{\eta}, T]}{243 M_{\eta'}^6 M_{\eta'}^2} + \frac{125 \sqrt{2} c_{\theta}^5 M_0^8 M_{\pi}^4 s_{\theta}^7 g_2 [M_{\eta}, T]}{243 M_{\eta'}^6 M_{\eta'}^2} -
\end{aligned}$$

$$\begin{aligned}
& \frac{560 c_{\theta}^4 M_0^8 M_K^4 s_{\theta}^8 g_2 [M_{\eta}, T]}{243 M_{\eta}^8} + \frac{559 c_{\theta}^4 M_0^8 M_K^2 M_{\pi}^2 s_{\theta}^8 g_2 [M_{\eta}, T]}{243 M_{\eta}^8} - \frac{349 c_{\theta}^4 M_0^8 M_{\pi}^4 s_{\theta}^8 g_2 [M_{\eta}, T]}{486 M_{\eta}^8} - \\
& \frac{8 c_{\theta}^4 M_0^8 M_K^4 s_{\theta}^8 g_2 [M_{\eta}, T]}{243 M_{\eta'}^8} + \frac{4 c_{\theta}^4 M_0^8 M_K^2 M_{\pi}^2 s_{\theta}^8 g_2 [M_{\eta}, T]}{243 M_{\eta'}^8} - \frac{c_{\theta}^4 M_0^8 M_{\pi}^4 s_{\theta}^8 g_2 [M_{\eta}, T]}{486 M_{\eta'}^8} + \\
& \frac{112 c_{\theta}^4 M_0^8 M_K^4 s_{\theta}^8 g_2 [M_{\eta}, T]}{243 M_{\eta}^2 M_{\eta'}^6} - \frac{92 c_{\theta}^4 M_0^8 M_K^2 M_{\pi}^2 s_{\theta}^8 g_2 [M_{\eta}, T]}{243 M_{\eta}^2 M_{\eta'}^6} + \frac{16 c_{\theta}^4 M_0^8 M_{\pi}^4 s_{\theta}^8 g_2 [M_{\eta}, T]}{243 M_{\eta}^2 M_{\eta'}^6} - \\
& \frac{148 c_{\theta}^4 M_0^8 M_K^4 s_{\theta}^8 g_2 [M_{\eta}, T]}{81 M_{\eta}^4 M_{\eta'}^4} + \frac{137 c_{\theta}^4 M_0^8 M_K^2 M_{\pi}^2 s_{\theta}^8 g_2 [M_{\eta}, T]}{81 M_{\eta}^4 M_{\eta'}^4} - \frac{53 c_{\theta}^4 M_0^8 M_{\pi}^4 s_{\theta}^8 g_2 [M_{\eta}, T]}{162 M_{\eta}^4 M_{\eta'}^4} + \\
& \frac{784 c_{\theta}^4 M_0^8 M_K^4 s_{\theta}^8 g_2 [M_{\eta}, T]}{243 M_{\eta}^6 M_{\eta'}^2} - \frac{770 c_{\theta}^4 M_0^8 M_K^2 M_{\pi}^2 s_{\theta}^8 g_2 [M_{\eta}, T]}{243 M_{\eta}^6 M_{\eta'}^2} + \frac{175 c_{\theta}^4 M_0^8 M_{\pi}^4 s_{\theta}^8 g_2 [M_{\eta}, T]}{243 M_{\eta}^6 M_{\eta'}^2} - \\
& \frac{224 \sqrt{2} c_{\theta}^3 M_0^8 M_K^4 s_{\theta}^9 g_2 [M_{\eta}, T]}{243 M_{\eta}^8} + \frac{244 \sqrt{2} c_{\theta}^3 M_0^8 M_K^2 M_{\pi}^2 s_{\theta}^9 g_2 [M_{\eta}, T]}{243 M_{\eta}^8} - \\
& \frac{38 \sqrt{2} c_{\theta}^3 M_0^8 M_{\pi}^4 s_{\theta}^9 g_2 [M_{\eta}, T]}{243 M_{\eta}^8} + \frac{16 \sqrt{2} c_{\theta}^3 M_0^8 M_K^4 s_{\theta}^9 g_2 [M_{\eta}, T]}{243 M_{\eta}^2 M_{\eta'}^6} - \\
& \frac{20 \sqrt{2} c_{\theta}^3 M_0^8 M_K^2 M_{\pi}^2 s_{\theta}^9 g_2 [M_{\eta}, T]}{243 M_{\eta}^2 M_{\eta'}^6} + \frac{4 \sqrt{2} c_{\theta}^3 M_0^8 M_{\pi}^4 s_{\theta}^9 g_2 [M_{\eta}, T]}{243 M_{\eta}^2 M_{\eta'}^6} - \\
& \frac{40 \sqrt{2} c_{\theta}^3 M_0^8 M_K^4 s_{\theta}^9 g_2 [M_{\eta}, T]}{81 M_{\eta}^4 M_{\eta'}^4} + \frac{50 \sqrt{2} c_{\theta}^3 M_0^8 M_K^2 M_{\pi}^2 s_{\theta}^9 g_2 [M_{\eta}, T]}{81 M_{\eta}^4 M_{\eta'}^4} - \\
& \frac{13 \sqrt{2} c_{\theta}^3 M_0^8 M_{\pi}^4 s_{\theta}^9 g_2 [M_{\eta}, T]}{81 M_{\eta}^4 M_{\eta'}^4} + \frac{280 \sqrt{2} c_{\theta}^3 M_0^8 M_K^4 s_{\theta}^9 g_2 [M_{\eta}, T]}{243 M_{\eta}^6 M_{\eta'}^2} - \\
& \frac{338 \sqrt{2} c_{\theta}^3 M_0^8 M_K^2 M_{\pi}^2 s_{\theta}^9 g_2 [M_{\eta}, T]}{243 M_{\eta}^6 M_{\eta'}^2} + \frac{85 \sqrt{2} c_{\theta}^3 M_0^8 M_{\pi}^4 s_{\theta}^9 g_2 [M_{\eta}, T]}{243 M_{\eta}^6 M_{\eta'}^2} - \\
& \frac{112 c_{\theta}^2 M_0^8 M_K^4 s_{\theta}^{10} g_2 [M_{\eta}, T]}{243 M_{\eta}^8} + \frac{116 c_{\theta}^2 M_0^8 M_K^2 M_{\pi}^2 s_{\theta}^{10} g_2 [M_{\eta}, T]}{243 M_{\eta}^8} - \frac{58 c_{\theta}^2 M_0^8 M_{\pi}^4 s_{\theta}^{10} g_2 [M_{\eta}, T]}{243 M_{\eta}^8} - \\
& \frac{8 c_{\theta}^2 M_0^8 M_K^4 s_{\theta}^{10} g_2 [M_{\eta}, T]}{81 M_{\eta}^4 M_{\eta'}^4} + \frac{10 c_{\theta}^2 M_0^8 M_K^2 M_{\pi}^2 s_{\theta}^{10} g_2 [M_{\eta}, T]}{81 M_{\eta}^4 M_{\eta'}^4} - \frac{5 c_{\theta}^2 M_0^8 M_{\pi}^4 s_{\theta}^{10} g_2 [M_{\eta}, T]}{81 M_{\eta}^4 M_{\eta'}^4} + \\
& \frac{104 c_{\theta}^2 M_0^8 M_K^4 s_{\theta}^{10} g_2 [M_{\eta}, T]}{243 M_{\eta}^6 M_{\eta'}^2} - \frac{124 c_{\theta}^2 M_0^8 M_K^2 M_{\pi}^2 s_{\theta}^{10} g_2 [M_{\eta}, T]}{243 M_{\eta}^6 M_{\eta'}^2} + \frac{56 c_{\theta}^2 M_0^8 M_{\pi}^4 s_{\theta}^{10} g_2 [M_{\eta}, T]}{243 M_{\eta}^6 M_{\eta'}^2} - \\
& \frac{16 \sqrt{2} c_{\theta} M_0^8 M_K^4 s_{\theta}^{11} g_2 [M_{\eta}, T]}{243 M_{\eta}^8} + \frac{8 \sqrt{2} c_{\theta} M_0^8 M_K^2 M_{\pi}^2 s_{\theta}^{11} g_2 [M_{\eta}, T]}{243 M_{\eta}^8} + \\
& \frac{8 \sqrt{2} c_{\theta} M_0^8 M_{\pi}^4 s_{\theta}^{11} g_2 [M_{\eta}, T]}{243 M_{\eta}^8} + \frac{8 \sqrt{2} c_{\theta} M_0^8 M_K^4 s_{\theta}^{11} g_2 [M_{\eta}, T]}{243 M_{\eta}^6 M_{\eta'}^2} -
\end{aligned}$$

$$\begin{aligned}
& \frac{4 \sqrt{2} c_{\theta} M_0^8 M_K^2 M_{\pi}^2 s_{\theta}^{11} g_2 [M_{\eta}, T]}{243 M_{\eta}^6 M_{\eta'}^2} - \frac{4 \sqrt{2} c_{\theta} M_0^8 M_{\pi}^4 s_{\theta}^{11} g_2 [M_{\eta}, T]}{243 M_{\eta}^6 M_{\eta'}^2} - \frac{2 M_0^8 M_K^4 s_{\theta}^{12} g_2 [M_{\eta}, T]}{243 M_{\eta}^8} - \\
& \frac{2 M_0^8 M_K^2 M_{\pi}^2 s_{\theta}^{12} g_2 [M_{\eta}, T]}{243 M_{\eta}^8} - \frac{M_0^8 M_{\pi}^4 s_{\theta}^{12} g_2 [M_{\eta}, T]}{486 M_{\eta}^8} - \frac{2 c_{\theta}^{12} M_0^8 M_K^4 g_2 [M_{\eta'}, T]}{243 M_{\eta'}^8} - \\
& \frac{2 c_{\theta}^{12} M_0^8 M_K^2 M_{\pi}^2 g_2 [M_{\eta'}, T]}{243 M_{\eta'}^8} - \frac{c_{\theta}^{12} M_0^8 M_{\pi}^4 g_2 [M_{\eta'}, T]}{486 M_{\eta'}^8} + \frac{16 \sqrt{2} c_{\theta}^{11} M_0^8 M_K^4 s_{\theta} g_2 [M_{\eta'}, T]}{243 M_{\eta'}^8} - \\
& \frac{8 \sqrt{2} c_{\theta}^{11} M_0^8 M_K^2 M_{\pi}^2 s_{\theta} g_2 [M_{\eta'}, T]}{243 M_{\eta'}^8} - \frac{8 \sqrt{2} c_{\theta}^{11} M_0^8 M_{\pi}^4 s_{\theta} g_2 [M_{\eta'}, T]}{243 M_{\eta'}^8} - \\
& \frac{8 \sqrt{2} c_{\theta}^{11} M_0^8 M_K^4 s_{\theta} g_2 [M_{\eta'}, T]}{243 M_{\eta'}^2 M_{\eta'}^6} + \frac{4 \sqrt{2} c_{\theta}^{11} M_0^8 M_K^2 M_{\pi}^2 s_{\theta} g_2 [M_{\eta'}, T]}{243 M_{\eta'}^2 M_{\eta'}^6} + \\
& \frac{4 \sqrt{2} c_{\theta}^{11} M_0^8 M_{\pi}^4 s_{\theta} g_2 [M_{\eta'}, T]}{243 M_{\eta'}^2 M_{\eta'}^6} - \frac{112 c_{\theta}^{10} M_0^8 M_K^4 s_{\theta}^2 g_2 [M_{\eta'}, T]}{243 M_{\eta'}^8} + \\
& \frac{116 c_{\theta}^{10} M_0^8 M_K^2 M_{\pi}^2 s_{\theta}^2 g_2 [M_{\eta'}, T]}{243 M_{\eta'}^8} - \frac{58 c_{\theta}^{10} M_0^8 M_{\pi}^4 s_{\theta}^2 g_2 [M_{\eta'}, T]}{243 M_{\eta'}^8} + \frac{104 c_{\theta}^{10} M_0^8 M_K^4 s_{\theta}^2 g_2 [M_{\eta'}, T]}{243 M_{\eta'}^2 M_{\eta'}^6} - \\
& \frac{124 c_{\theta}^{10} M_0^8 M_K^2 M_{\pi}^2 s_{\theta}^2 g_2 [M_{\eta'}, T]}{243 M_{\eta'}^2 M_{\eta'}^6} + \frac{56 c_{\theta}^{10} M_0^8 M_{\pi}^4 s_{\theta}^2 g_2 [M_{\eta'}, T]}{243 M_{\eta'}^2 M_{\eta'}^6} - \frac{8 c_{\theta}^{10} M_0^8 M_K^4 s_{\theta}^2 g_2 [M_{\eta'}, T]}{81 M_{\eta'}^4 M_{\eta'}^4} + \\
& \frac{10 c_{\theta}^{10} M_0^8 M_K^2 M_{\pi}^2 s_{\theta}^2 g_2 [M_{\eta'}, T]}{81 M_{\eta'}^4 M_{\eta'}^4} - \frac{5 c_{\theta}^{10} M_0^8 M_{\pi}^4 s_{\theta}^2 g_2 [M_{\eta'}, T]}{81 M_{\eta'}^4 M_{\eta'}^4} + \frac{224 \sqrt{2} c_{\theta}^9 M_0^8 M_K^4 s_{\theta}^3 g_2 [M_{\eta'}, T]}{243 M_{\eta'}^8} - \\
& \frac{244 \sqrt{2} c_{\theta}^9 M_0^8 M_K^2 M_{\pi}^2 s_{\theta}^3 g_2 [M_{\eta'}, T]}{243 M_{\eta'}^8} + \frac{38 \sqrt{2} c_{\theta}^9 M_0^8 M_{\pi}^4 s_{\theta}^3 g_2 [M_{\eta'}, T]}{243 M_{\eta'}^8} - \\
& \frac{280 \sqrt{2} c_{\theta}^9 M_0^8 M_K^4 s_{\theta}^3 g_2 [M_{\eta'}, T]}{243 M_{\eta'}^2 M_{\eta'}^6} + \frac{338 \sqrt{2} c_{\theta}^9 M_0^8 M_K^2 M_{\pi}^2 s_{\theta}^3 g_2 [M_{\eta'}, T]}{243 M_{\eta'}^2 M_{\eta'}^6} - \\
& \frac{85 \sqrt{2} c_{\theta}^9 M_0^8 M_{\pi}^4 s_{\theta}^3 g_2 [M_{\eta'}, T]}{243 M_{\eta'}^2 M_{\eta'}^6} + \frac{40 \sqrt{2} c_{\theta}^9 M_0^8 M_K^4 s_{\theta}^3 g_2 [M_{\eta'}, T]}{81 M_{\eta'}^4 M_{\eta'}^4} - \\
& \frac{50 \sqrt{2} c_{\theta}^9 M_0^8 M_K^2 M_{\pi}^2 s_{\theta}^3 g_2 [M_{\eta'}, T]}{81 M_{\eta'}^4 M_{\eta'}^4} + \frac{13 \sqrt{2} c_{\theta}^9 M_0^8 M_{\pi}^4 s_{\theta}^3 g_2 [M_{\eta'}, T]}{81 M_{\eta'}^4 M_{\eta'}^4} - \\
& \frac{16 \sqrt{2} c_{\theta}^9 M_0^8 M_K^4 s_{\theta}^3 g_2 [M_{\eta'}, T]}{243 M_{\eta'}^6 M_{\eta'}^2} + \frac{20 \sqrt{2} c_{\theta}^9 M_0^8 M_K^2 M_{\pi}^2 s_{\theta}^3 g_2 [M_{\eta'}, T]}{243 M_{\eta'}^6 M_{\eta'}^2} - \\
& \frac{4 \sqrt{2} c_{\theta}^9 M_0^8 M_{\pi}^4 s_{\theta}^3 g_2 [M_{\eta'}, T]}{243 M_{\eta'}^6 M_{\eta'}^2} - \frac{8 c_{\theta}^8 M_0^8 M_K^4 s_{\theta}^4 g_2 [M_{\eta'}, T]}{243 M_{\eta'}^8} + \frac{4 c_{\theta}^8 M_0^8 M_K^2 M_{\pi}^2 s_{\theta}^4 g_2 [M_{\eta'}, T]}{243 M_{\eta'}^8} - \\
& \frac{c_{\theta}^8 M_0^8 M_{\pi}^4 s_{\theta}^4 g_2 [M_{\eta'}, T]}{486 M_{\eta'}^8} - \frac{560 c_{\theta}^8 M_0^8 M_K^4 s_{\theta}^4 g_2 [M_{\eta'}, T]}{243 M_{\eta'}^8} + \frac{559 c_{\theta}^8 M_0^8 M_K^2 M_{\pi}^2 s_{\theta}^4 g_2 [M_{\eta'}, T]}{243 M_{\eta'}^8} -
\end{aligned}$$

$$\begin{aligned}
& \frac{349 c_{\theta}^8 M_0^8 M_{\pi}^4 s_{\theta}^4 g_2 [M_{\eta'}, T]}{486 M_{\eta'}^8} + \frac{784 c_{\theta}^8 M_0^8 M_K^4 s_{\theta}^4 g_2 [M_{\eta'}, T]}{243 M_{\eta'}^2 M_{\eta'}^6} - \frac{770 c_{\theta}^8 M_0^8 M_K^2 M_{\pi}^2 s_{\theta}^4 g_2 [M_{\eta'}, T]}{243 M_{\eta'}^2 M_{\eta'}^6} + \\
& \frac{175 c_{\theta}^8 M_0^8 M_{\pi}^4 s_{\theta}^4 g_2 [M_{\eta'}, T]}{243 M_{\eta'}^2 M_{\eta'}^6} - \frac{148 c_{\theta}^8 M_0^8 M_K^4 s_{\theta}^4 g_2 [M_{\eta'}, T]}{81 M_{\eta'}^4 M_{\eta'}^4} + \frac{137 c_{\theta}^8 M_0^8 M_K^2 M_{\pi}^2 s_{\theta}^4 g_2 [M_{\eta'}, T]}{81 M_{\eta'}^4 M_{\eta'}^4} - \\
& \frac{53 c_{\theta}^8 M_0^8 M_{\pi}^4 s_{\theta}^4 g_2 [M_{\eta'}, T]}{162 M_{\eta'}^4 M_{\eta'}^4} + \frac{112 c_{\theta}^8 M_0^8 M_K^4 s_{\theta}^4 g_2 [M_{\eta'}, T]}{243 M_{\eta'}^6 M_{\eta'}^2} - \frac{92 c_{\theta}^8 M_0^8 M_K^2 M_{\pi}^2 s_{\theta}^4 g_2 [M_{\eta'}, T]}{243 M_{\eta'}^6 M_{\eta'}^2} + \\
& \frac{16 c_{\theta}^8 M_0^8 M_{\pi}^4 s_{\theta}^4 g_2 [M_{\eta'}, T]}{243 M_{\eta'}^6 M_{\eta'}^2} + \frac{16 \sqrt{2} c_{\theta}^7 M_0^8 M_K^4 s_{\theta}^5 g_2 [M_{\eta'}, T]}{243 M_{\eta'}^8} - \frac{8 \sqrt{2} c_{\theta}^7 M_0^8 M_K^2 M_{\pi}^2 s_{\theta}^5 g_2 [M_{\eta'}, T]}{243 M_{\eta'}^8} + \\
& \frac{\sqrt{2} c_{\theta}^7 M_0^8 M_{\pi}^4 s_{\theta}^5 g_2 [M_{\eta'}, T]}{243 M_{\eta'}^8} + \frac{448 \sqrt{2} c_{\theta}^7 M_0^8 M_K^4 s_{\theta}^5 g_2 [M_{\eta'}, T]}{243 M_{\eta'}^8} - \\
& \frac{428 \sqrt{2} c_{\theta}^7 M_0^8 M_K^2 M_{\pi}^2 s_{\theta}^5 g_2 [M_{\eta'}, T]}{243 M_{\eta'}^8} + \frac{88 \sqrt{2} c_{\theta}^7 M_0^8 M_{\pi}^4 s_{\theta}^5 g_2 [M_{\eta'}, T]}{243 M_{\eta'}^8} - \\
& \frac{560 \sqrt{2} c_{\theta}^7 M_0^8 M_K^4 s_{\theta}^5 g_2 [M_{\eta'}, T]}{243 M_{\eta'}^2 M_{\eta'}^6} + \frac{460 \sqrt{2} c_{\theta}^7 M_0^8 M_K^2 M_{\pi}^2 s_{\theta}^5 g_2 [M_{\eta'}, T]}{243 M_{\eta'}^2 M_{\eta'}^6} - \\
& \frac{125 \sqrt{2} c_{\theta}^7 M_0^8 M_{\pi}^4 s_{\theta}^5 g_2 [M_{\eta'}, T]}{243 M_{\eta'}^2 M_{\eta'}^6} + \frac{104 \sqrt{2} c_{\theta}^7 M_0^8 M_K^4 s_{\theta}^5 g_2 [M_{\eta'}, T]}{81 M_{\eta'}^4 M_{\eta'}^4} - \\
& \frac{58 \sqrt{2} c_{\theta}^7 M_0^8 M_K^2 M_{\pi}^2 s_{\theta}^5 g_2 [M_{\eta'}, T]}{81 M_{\eta'}^4 M_{\eta'}^4} + \frac{11 \sqrt{2} c_{\theta}^7 M_0^8 M_{\pi}^4 s_{\theta}^5 g_2 [M_{\eta'}, T]}{81 M_{\eta'}^4 M_{\eta'}^4} - \\
& \frac{104 \sqrt{2} c_{\theta}^7 M_0^8 M_K^4 s_{\theta}^5 g_2 [M_{\eta'}, T]}{243 M_{\eta'}^6 M_{\eta'}^2} + \frac{46 \sqrt{2} c_{\theta}^7 M_0^8 M_K^2 M_{\pi}^2 s_{\theta}^5 g_2 [M_{\eta'}, T]}{243 M_{\eta'}^6 M_{\eta'}^2} - \\
& \frac{5 \sqrt{2} c_{\theta}^7 M_0^8 M_{\pi}^4 s_{\theta}^5 g_2 [M_{\eta'}, T]}{243 M_{\eta'}^6 M_{\eta'}^2} + \frac{8 c_{\theta}^6 M_0^8 M_K^4 s_{\theta}^6 g_2 [M_{\eta'}, T]}{243 M_{\eta'}^8} - \frac{4 c_{\theta}^6 M_0^8 M_K^2 M_{\pi}^2 s_{\theta}^6 g_2 [M_{\eta'}, T]}{243 M_{\eta'}^8} + \\
& \frac{c_{\theta}^6 M_0^8 M_{\pi}^4 s_{\theta}^6 g_2 [M_{\eta'}, T]}{486 M_{\eta'}^8} - \frac{448 c_{\theta}^6 M_0^8 M_K^4 s_{\theta}^6 g_2 [M_{\eta'}, T]}{243 M_{\eta'}^8} + \frac{452 c_{\theta}^6 M_0^8 M_K^2 M_{\pi}^2 s_{\theta}^6 g_2 [M_{\eta'}, T]}{243 M_{\eta'}^8} - \\
& \frac{121 c_{\theta}^6 M_0^8 M_{\pi}^4 s_{\theta}^6 g_2 [M_{\eta'}, T]}{243 M_{\eta'}^8} + \frac{224 c_{\theta}^6 M_0^8 M_K^4 s_{\theta}^6 g_2 [M_{\eta'}, T]}{243 M_{\eta'}^2 M_{\eta'}^6} - \frac{238 c_{\theta}^6 M_0^8 M_K^2 M_{\pi}^2 s_{\theta}^6 g_2 [M_{\eta'}, T]}{243 M_{\eta'}^2 M_{\eta'}^6} + \\
& \frac{14 c_{\theta}^6 M_0^8 M_{\pi}^4 s_{\theta}^6 g_2 [M_{\eta'}, T]}{243 M_{\eta'}^2 M_{\eta'}^6} + \frac{40 c_{\theta}^6 M_0^8 M_K^4 s_{\theta}^6 g_2 [M_{\eta'}, T]}{81 M_{\eta'}^4 M_{\eta'}^4} - \frac{32 c_{\theta}^6 M_0^8 M_K^2 M_{\pi}^2 s_{\theta}^6 g_2 [M_{\eta'}, T]}{81 M_{\eta'}^4 M_{\eta'}^4} + \\
& \frac{17 c_{\theta}^6 M_0^8 M_{\pi}^4 s_{\theta}^6 g_2 [M_{\eta'}, T]}{162 M_{\eta'}^4 M_{\eta'}^4} - \frac{88 c_{\theta}^6 M_0^8 M_K^4 s_{\theta}^6 g_2 [M_{\eta'}, T]}{243 M_{\eta'}^6 M_{\eta'}^2} + \frac{74 c_{\theta}^6 M_0^8 M_K^2 M_{\pi}^2 s_{\theta}^6 g_2 [M_{\eta'}, T]}{243 M_{\eta'}^6 M_{\eta'}^2} - \\
& \frac{13 c_{\theta}^6 M_0^8 M_{\pi}^4 s_{\theta}^6 g_2 [M_{\eta'}, T]}{243 M_{\eta'}^6 M_{\eta'}^2} - \frac{40 \sqrt{2} c_{\theta}^5 M_0^8 M_K^4 s_{\theta}^7 g_2 [M_{\eta'}, T]}{243 M_{\eta'}^8} + \frac{20 \sqrt{2} c_{\theta}^5 M_0^8 M_K^2 M_{\pi}^2 s_{\theta}^7 g_2 [M_{\eta'}, T]}{243 M_{\eta'}^8} -
\end{aligned}$$

$$\begin{aligned}
& \frac{5 c_{\theta}^5 M_0^8 M_{\pi}^4 s_{\theta}^7 g_2 [M_{\eta'}, T]}{243 \sqrt{2} M_{\eta}^8} + \frac{128 \sqrt{2} c_{\theta}^5 M_0^8 M_K^4 s_{\theta}^7 g_2 [M_{\eta'}, T]}{243 M_{\eta'}^8} - \frac{136 \sqrt{2} c_{\theta}^5 M_0^8 M_K^2 M_{\pi}^2 s_{\theta}^7 g_2 [M_{\eta'}, T]}{243 M_{\eta'}^8} + \\
& \frac{35 \sqrt{2} c_{\theta}^5 M_0^8 M_{\pi}^4 s_{\theta}^7 g_2 [M_{\eta'}, T]}{243 M_{\eta'}^8} + \frac{224 \sqrt{2} c_{\theta}^5 M_0^8 M_K^4 s_{\theta}^7 g_2 [M_{\eta'}, T]}{243 M_{\eta}^2 M_{\eta'}^6} - \\
& \frac{166 \sqrt{2} c_{\theta}^5 M_0^8 M_K^2 M_{\pi}^2 s_{\theta}^7 g_2 [M_{\eta'}, T]}{243 M_{\eta}^2 M_{\eta'}^6} + \frac{19 c_{\theta}^5 M_0^8 M_{\pi}^4 s_{\theta}^7 g_2 [M_{\eta'}, T]}{243 \sqrt{2} M_{\eta}^2 M_{\eta'}^6} - \\
& \frac{128 \sqrt{2} c_{\theta}^5 M_0^8 M_K^4 s_{\theta}^7 g_2 [M_{\eta'}, T]}{81 M_{\eta}^4 M_{\eta'}^4} + \frac{82 \sqrt{2} c_{\theta}^5 M_0^8 M_K^2 M_{\pi}^2 s_{\theta}^7 g_2 [M_{\eta'}, T]}{81 M_{\eta}^4 M_{\eta'}^4} - \frac{31 c_{\theta}^5 M_0^8 M_{\pi}^4 s_{\theta}^7 g_2 [M_{\eta'}, T]}{81 \sqrt{2} M_{\eta}^4 M_{\eta'}^4} + \\
& \frac{200 \sqrt{2} c_{\theta}^5 M_0^8 M_K^4 s_{\theta}^7 g_2 [M_{\eta'}, T]}{243 M_{\eta}^6 M_{\eta'}^2} - \frac{100 \sqrt{2} c_{\theta}^5 M_0^8 M_K^2 M_{\pi}^2 s_{\theta}^7 g_2 [M_{\eta'}, T]}{243 M_{\eta}^6 M_{\eta'}^2} + \\
& \frac{25 c_{\theta}^5 M_0^8 M_{\pi}^4 s_{\theta}^7 g_2 [M_{\eta'}, T]}{243 \sqrt{2} M_{\eta}^6 M_{\eta'}^2} - \frac{2 c_{\theta}^4 M_0^8 M_K^4 s_{\theta}^8 g_2 [M_{\eta'}, T]}{243 M_{\eta}^8} + \frac{c_{\theta}^4 M_0^8 M_K^2 M_{\pi}^2 s_{\theta}^8 g_2 [M_{\eta'}, T]}{243 M_{\eta}^8} - \\
& \frac{c_{\theta}^4 M_0^8 M_{\pi}^4 s_{\theta}^8 g_2 [M_{\eta'}, T]}{1944 M_{\eta}^8} - \frac{32 c_{\theta}^4 M_0^8 M_K^4 s_{\theta}^8 g_2 [M_{\eta'}, T]}{243 M_{\eta'}^8} + \frac{28 c_{\theta}^4 M_0^8 M_K^2 M_{\pi}^2 s_{\theta}^8 g_2 [M_{\eta'}, T]}{243 M_{\eta'}^8} - \\
& \frac{49 c_{\theta}^4 M_0^8 M_{\pi}^4 s_{\theta}^8 g_2 [M_{\eta'}, T]}{1944 M_{\eta'}^8} - \frac{320 c_{\theta}^4 M_0^8 M_K^4 s_{\theta}^8 g_2 [M_{\eta'}, T]}{243 M_{\eta}^2 M_{\eta'}^6} + \frac{340 c_{\theta}^4 M_0^8 M_K^2 M_{\pi}^2 s_{\theta}^8 g_2 [M_{\eta'}, T]}{243 M_{\eta}^2 M_{\eta'}^6} - \\
& \frac{193 c_{\theta}^4 M_0^8 M_{\pi}^4 s_{\theta}^8 g_2 [M_{\eta'}, T]}{486 M_{\eta}^2 M_{\eta'}^6} + \frac{80 c_{\theta}^4 M_0^8 M_K^4 s_{\theta}^8 g_2 [M_{\eta'}, T]}{81 M_{\eta}^4 M_{\eta'}^4} - \frac{91 c_{\theta}^4 M_0^8 M_K^2 M_{\pi}^2 s_{\theta}^8 g_2 [M_{\eta'}, T]}{81 M_{\eta}^4 M_{\eta'}^4} + \\
& \frac{65 c_{\theta}^4 M_0^8 M_{\pi}^4 s_{\theta}^8 g_2 [M_{\eta'}, T]}{324 M_{\eta}^4 M_{\eta'}^4} - \frac{32 c_{\theta}^4 M_0^8 M_K^4 s_{\theta}^8 g_2 [M_{\eta'}, T]}{243 M_{\eta}^6 M_{\eta'}^2} + \frac{46 c_{\theta}^4 M_0^8 M_K^2 M_{\pi}^2 s_{\theta}^8 g_2 [M_{\eta'}, T]}{243 M_{\eta}^6 M_{\eta'}^2} - \\
& \frac{19 c_{\theta}^4 M_0^8 M_{\pi}^4 s_{\theta}^8 g_2 [M_{\eta'}, T]}{486 M_{\eta}^6 M_{\eta'}^2} + \frac{40 \sqrt{2} c_{\theta}^3 M_0^8 M_K^4 s_{\theta}^9 g_2 [M_{\eta'}, T]}{243 M_{\eta}^8} - \frac{20 \sqrt{2} c_{\theta}^3 M_0^8 M_K^2 M_{\pi}^2 s_{\theta}^9 g_2 [M_{\eta'}, T]}{243 M_{\eta}^8} + \\
& \frac{5 c_{\theta}^3 M_0^8 M_{\pi}^4 s_{\theta}^9 g_2 [M_{\eta'}, T]}{243 \sqrt{2} M_{\eta}^8} + \frac{64 \sqrt{2} c_{\theta}^3 M_0^8 M_K^4 s_{\theta}^9 g_2 [M_{\eta'}, T]}{243 M_{\eta}^2 M_{\eta'}^6} - \frac{68 \sqrt{2} c_{\theta}^3 M_0^8 M_K^2 M_{\pi}^2 s_{\theta}^9 g_2 [M_{\eta'}, T]}{243 M_{\eta}^2 M_{\eta'}^6} + \\
& \frac{35 c_{\theta}^3 M_0^8 M_{\pi}^4 s_{\theta}^9 g_2 [M_{\eta'}, T]}{243 \sqrt{2} M_{\eta}^2 M_{\eta'}^6} + \frac{32 \sqrt{2} c_{\theta}^3 M_0^8 M_K^4 s_{\theta}^9 g_2 [M_{\eta'}, T]}{81 M_{\eta}^4 M_{\eta'}^4} - \frac{22 \sqrt{2} c_{\theta}^3 M_0^8 M_K^2 M_{\pi}^2 s_{\theta}^9 g_2 [M_{\eta'}, T]}{81 M_{\eta}^4 M_{\eta'}^4} + \\
& \frac{c_{\theta}^3 M_0^8 M_{\pi}^4 s_{\theta}^9 g_2 [M_{\eta'}, T]}{81 \sqrt{2} M_{\eta}^4 M_{\eta'}^4} - \frac{128 \sqrt{2} c_{\theta}^3 M_0^8 M_K^4 s_{\theta}^9 g_2 [M_{\eta'}, T]}{243 M_{\eta}^6 M_{\eta'}^2} + \frac{70 \sqrt{2} c_{\theta}^3 M_0^8 M_K^2 M_{\pi}^2 s_{\theta}^9 g_2 [M_{\eta'}, T]}{243 M_{\eta}^6 M_{\eta'}^2} - \\
& \frac{19 c_{\theta}^3 M_0^8 M_{\pi}^4 s_{\theta}^9 g_2 [M_{\eta'}, T]}{243 \sqrt{2} M_{\eta}^6 M_{\eta'}^2} + \frac{8 c_{\theta}^2 M_0^8 M_K^4 s_{\theta}^{10} g_2 [M_{\eta'}, T]}{243 M_{\eta}^8} - \frac{4 c_{\theta}^2 M_0^8 M_K^2 M_{\pi}^2 s_{\theta}^{10} g_2 [M_{\eta'}, T]}{243 M_{\eta}^8} + \\
& \frac{c_{\theta}^2 M_0^8 M_{\pi}^4 s_{\theta}^{10} g_2 [M_{\eta'}, T]}{486 M_{\eta}^8} - \frac{32 c_{\theta}^2 M_0^8 M_K^4 s_{\theta}^{10} g_2 [M_{\eta'}, T]}{81 M_{\eta}^4 M_{\eta'}^4} + \frac{34 c_{\theta}^2 M_0^8 M_K^2 M_{\pi}^2 s_{\theta}^{10} g_2 [M_{\eta'}, T]}{81 M_{\eta}^4 M_{\eta'}^4} -
\end{aligned}$$

$$\begin{aligned}
& \frac{19 \, c_\theta^2 \, M_\theta^8 \, M_\pi^4 \, s_\theta^{10} \, g_2 [M_{\eta'}, T]}{162 \, M_\eta^4 \, M_{\eta'}^4} + \frac{32 \, c_\theta^2 \, M_\theta^8 \, M_K^4 \, s_\theta^{10} \, g_2 [M_{\eta'}, T]}{243 \, M_\eta^6 \, M_{\eta'}^2} - \frac{52 \, c_\theta^2 \, M_\theta^8 \, M_K^2 \, M_\pi^2 \, s_\theta^{10} \, g_2 [M_{\eta'}, T]}{243 \, M_\eta^6 \, M_{\eta'}^2} + \\
& \frac{11 \, c_\theta^2 \, M_\theta^8 \, M_\pi^4 \, s_\theta^{10} \, g_2 [M_{\eta'}, T]}{243 \, M_\eta^6 \, M_{\eta'}^2} - \frac{16 \, \sqrt{2} \, c_\theta \, M_\theta^8 \, M_K^4 \, s_\theta^{11} \, g_2 [M_{\eta'}, T]}{243 \, M_\eta^8} + \frac{8 \, \sqrt{2} \, c_\theta \, M_\theta^8 \, M_K^2 \, M_\pi^2 \, s_\theta^{11} \, g_2 [M_{\eta'}, T]}{243 \, M_\eta^8} - \\
& \frac{\sqrt{2} \, c_\theta \, M_\theta^8 \, M_\pi^4 \, s_\theta^{11} \, g_2 [M_{\eta'}, T]}{243 \, M_\eta^8} + \frac{32 \, \sqrt{2} \, c_\theta \, M_\theta^8 \, M_K^4 \, s_\theta^{11} \, g_2 [M_{\eta'}, T]}{243 \, M_\eta^6 \, M_{\eta'}^2} - \\
& \frac{28 \, \sqrt{2} \, c_\theta \, M_\theta^8 \, M_K^2 \, M_\pi^2 \, s_\theta^{11} \, g_2 [M_{\eta'}, T]}{243 \, M_\eta^6 \, M_{\eta'}^2} + \frac{5 \, \sqrt{2} \, c_\theta \, M_\theta^8 \, M_\pi^4 \, s_\theta^{11} \, g_2 [M_{\eta'}, T]}{243 \, M_\eta^6 \, M_{\eta'}^2} - \\
& \frac{8 \, M_\theta^8 \, M_K^4 \, s_\theta^{12} \, g_2 [M_{\eta'}, T]}{243 \, M_\eta^8} + \frac{4 \, M_\theta^8 \, M_K^2 \, M_\pi^2 \, s_\theta^{12} \, g_2 [M_{\eta'}, T]}{243 \, M_\eta^8} - \frac{M_\theta^8 \, M_\pi^4 \, s_\theta^{12} \, g_2 [M_{\eta'}, T]}{486 \, M_\eta^8}
\end{aligned}$$
